# Supplementary material for: Testing the Froggatt-Nielsen Mechanism with Lepton Flavor and Number Violating Processes
Source: arXiv:2501.00629 ancillary file (2025-12-15)

Majorana,  $X_L = \{2, 0, -1\}$ ,  $X_e = \{7, 6, 4\}$ ,

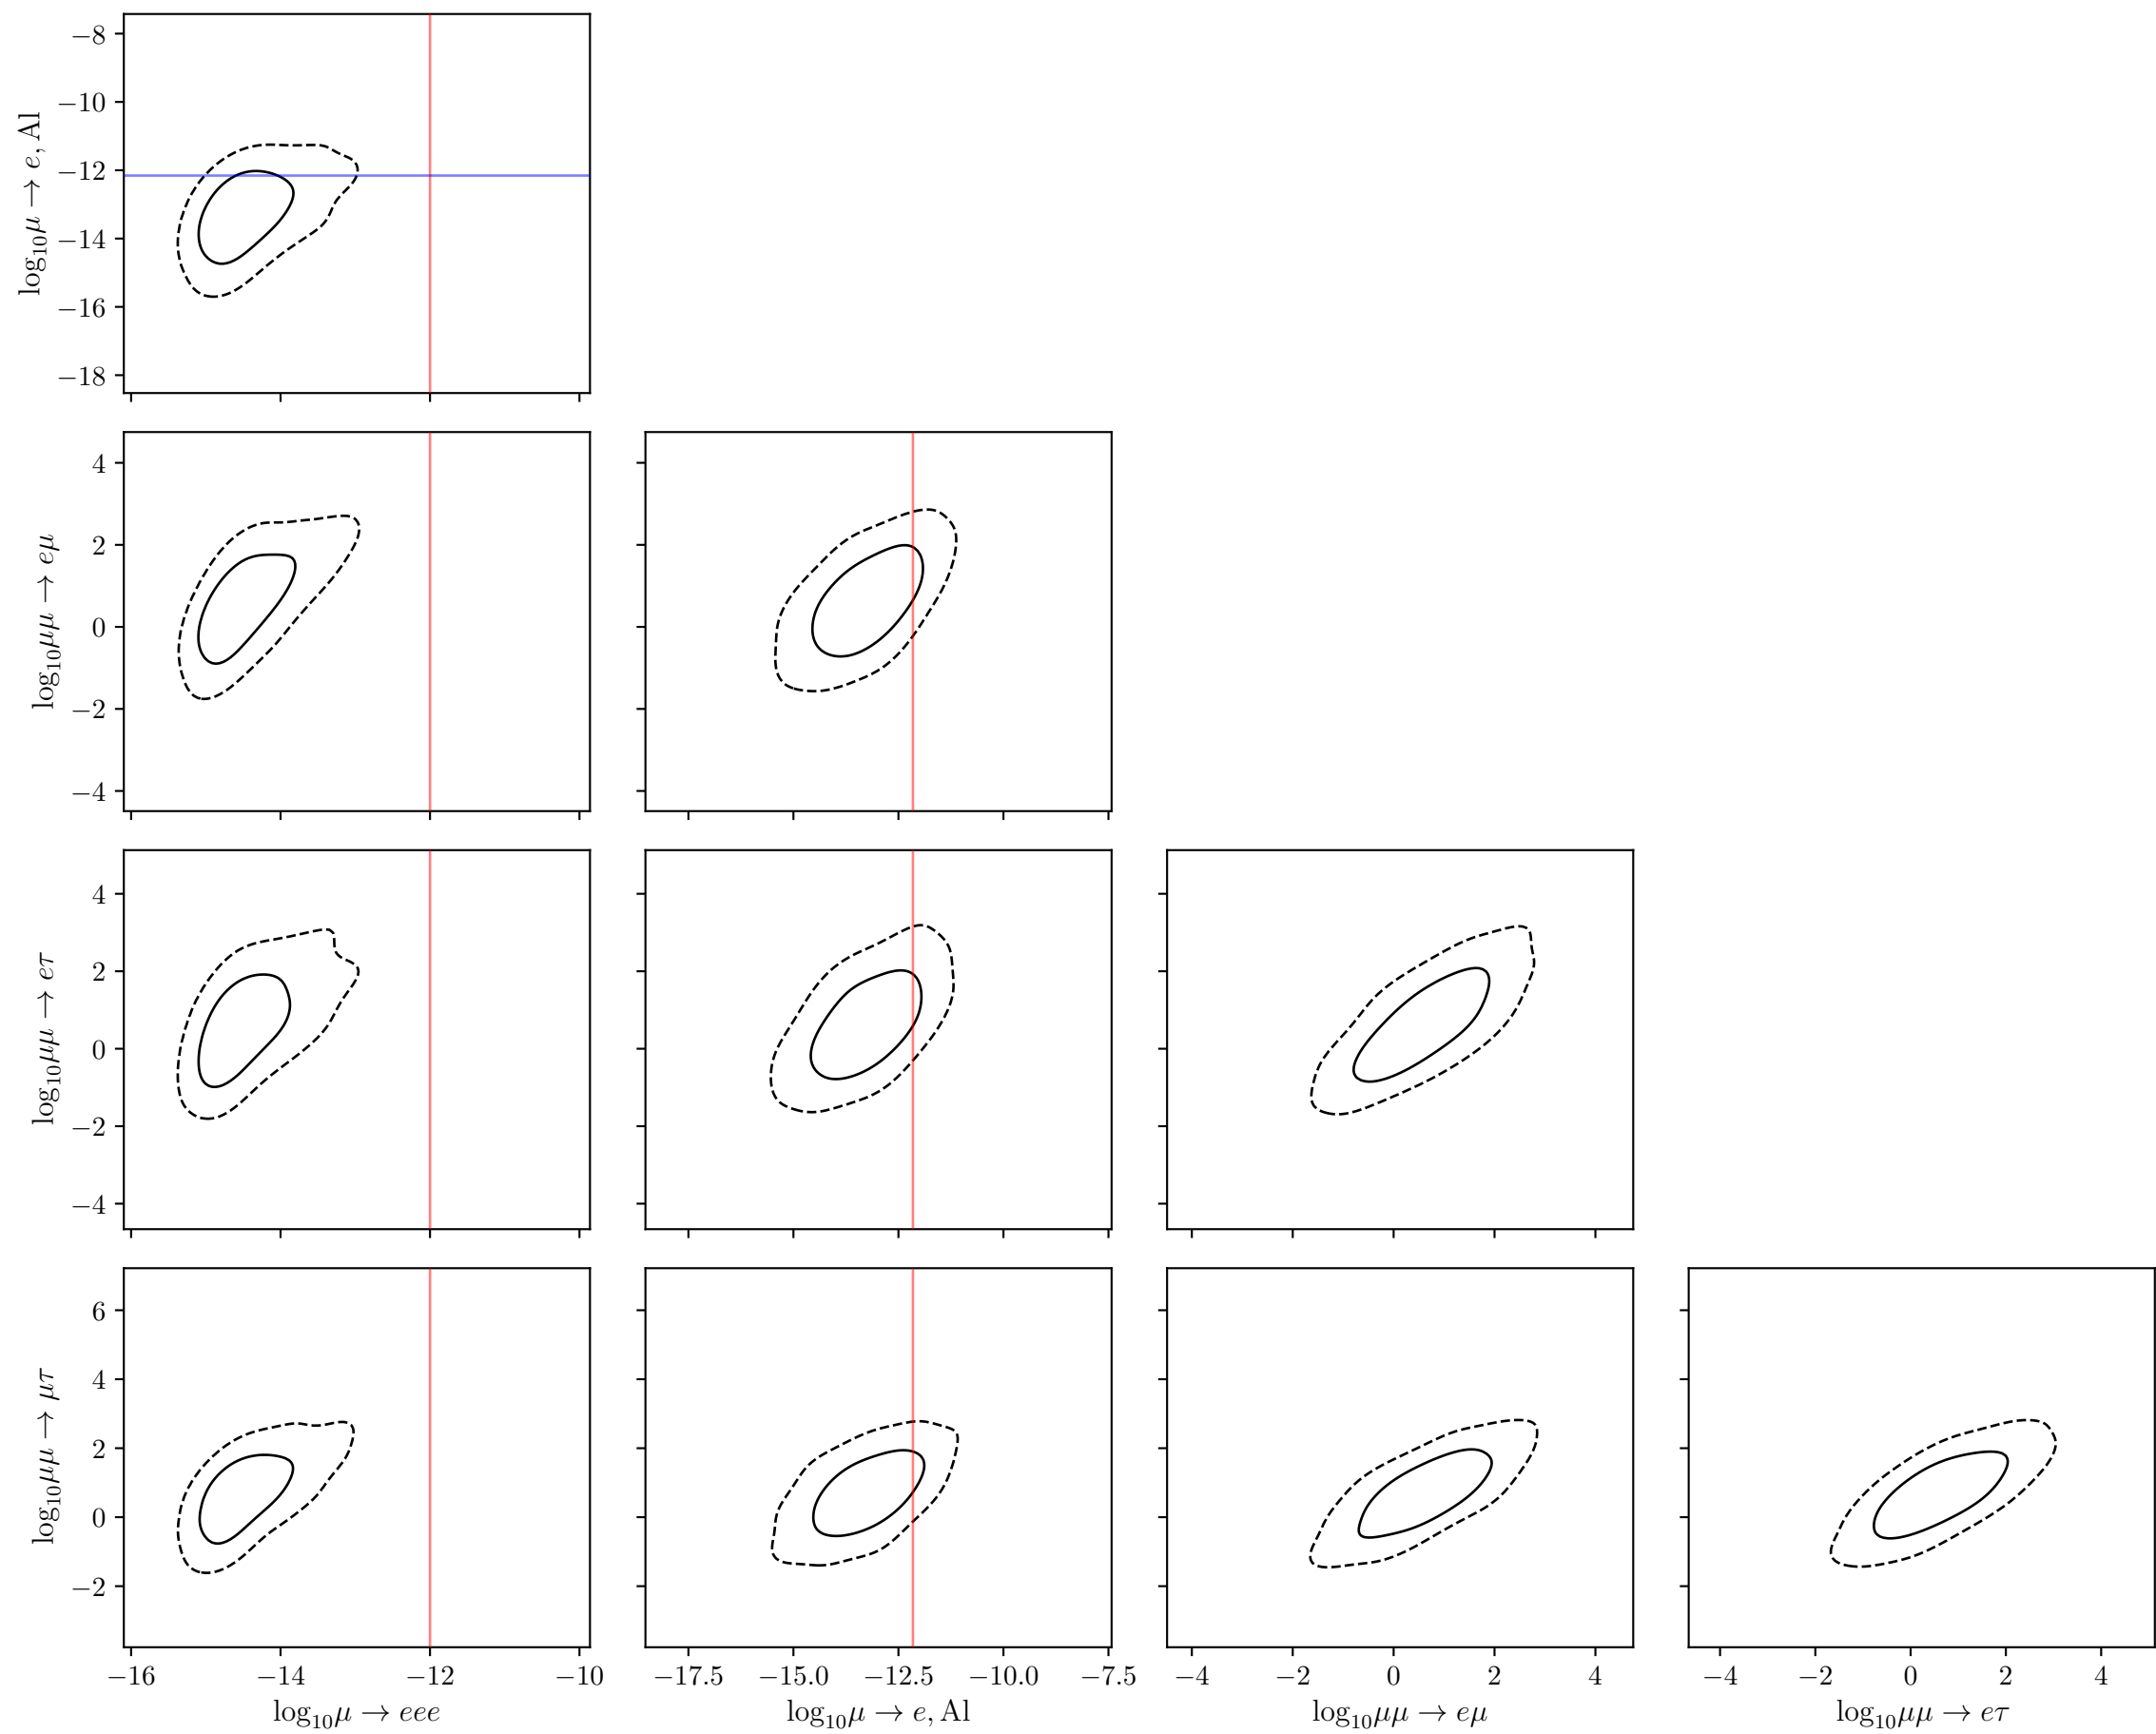

Majorana,  $X_L = \{5, 5, -2\}$ ,  $X_e = \{-3, -2, 7\}$ ,

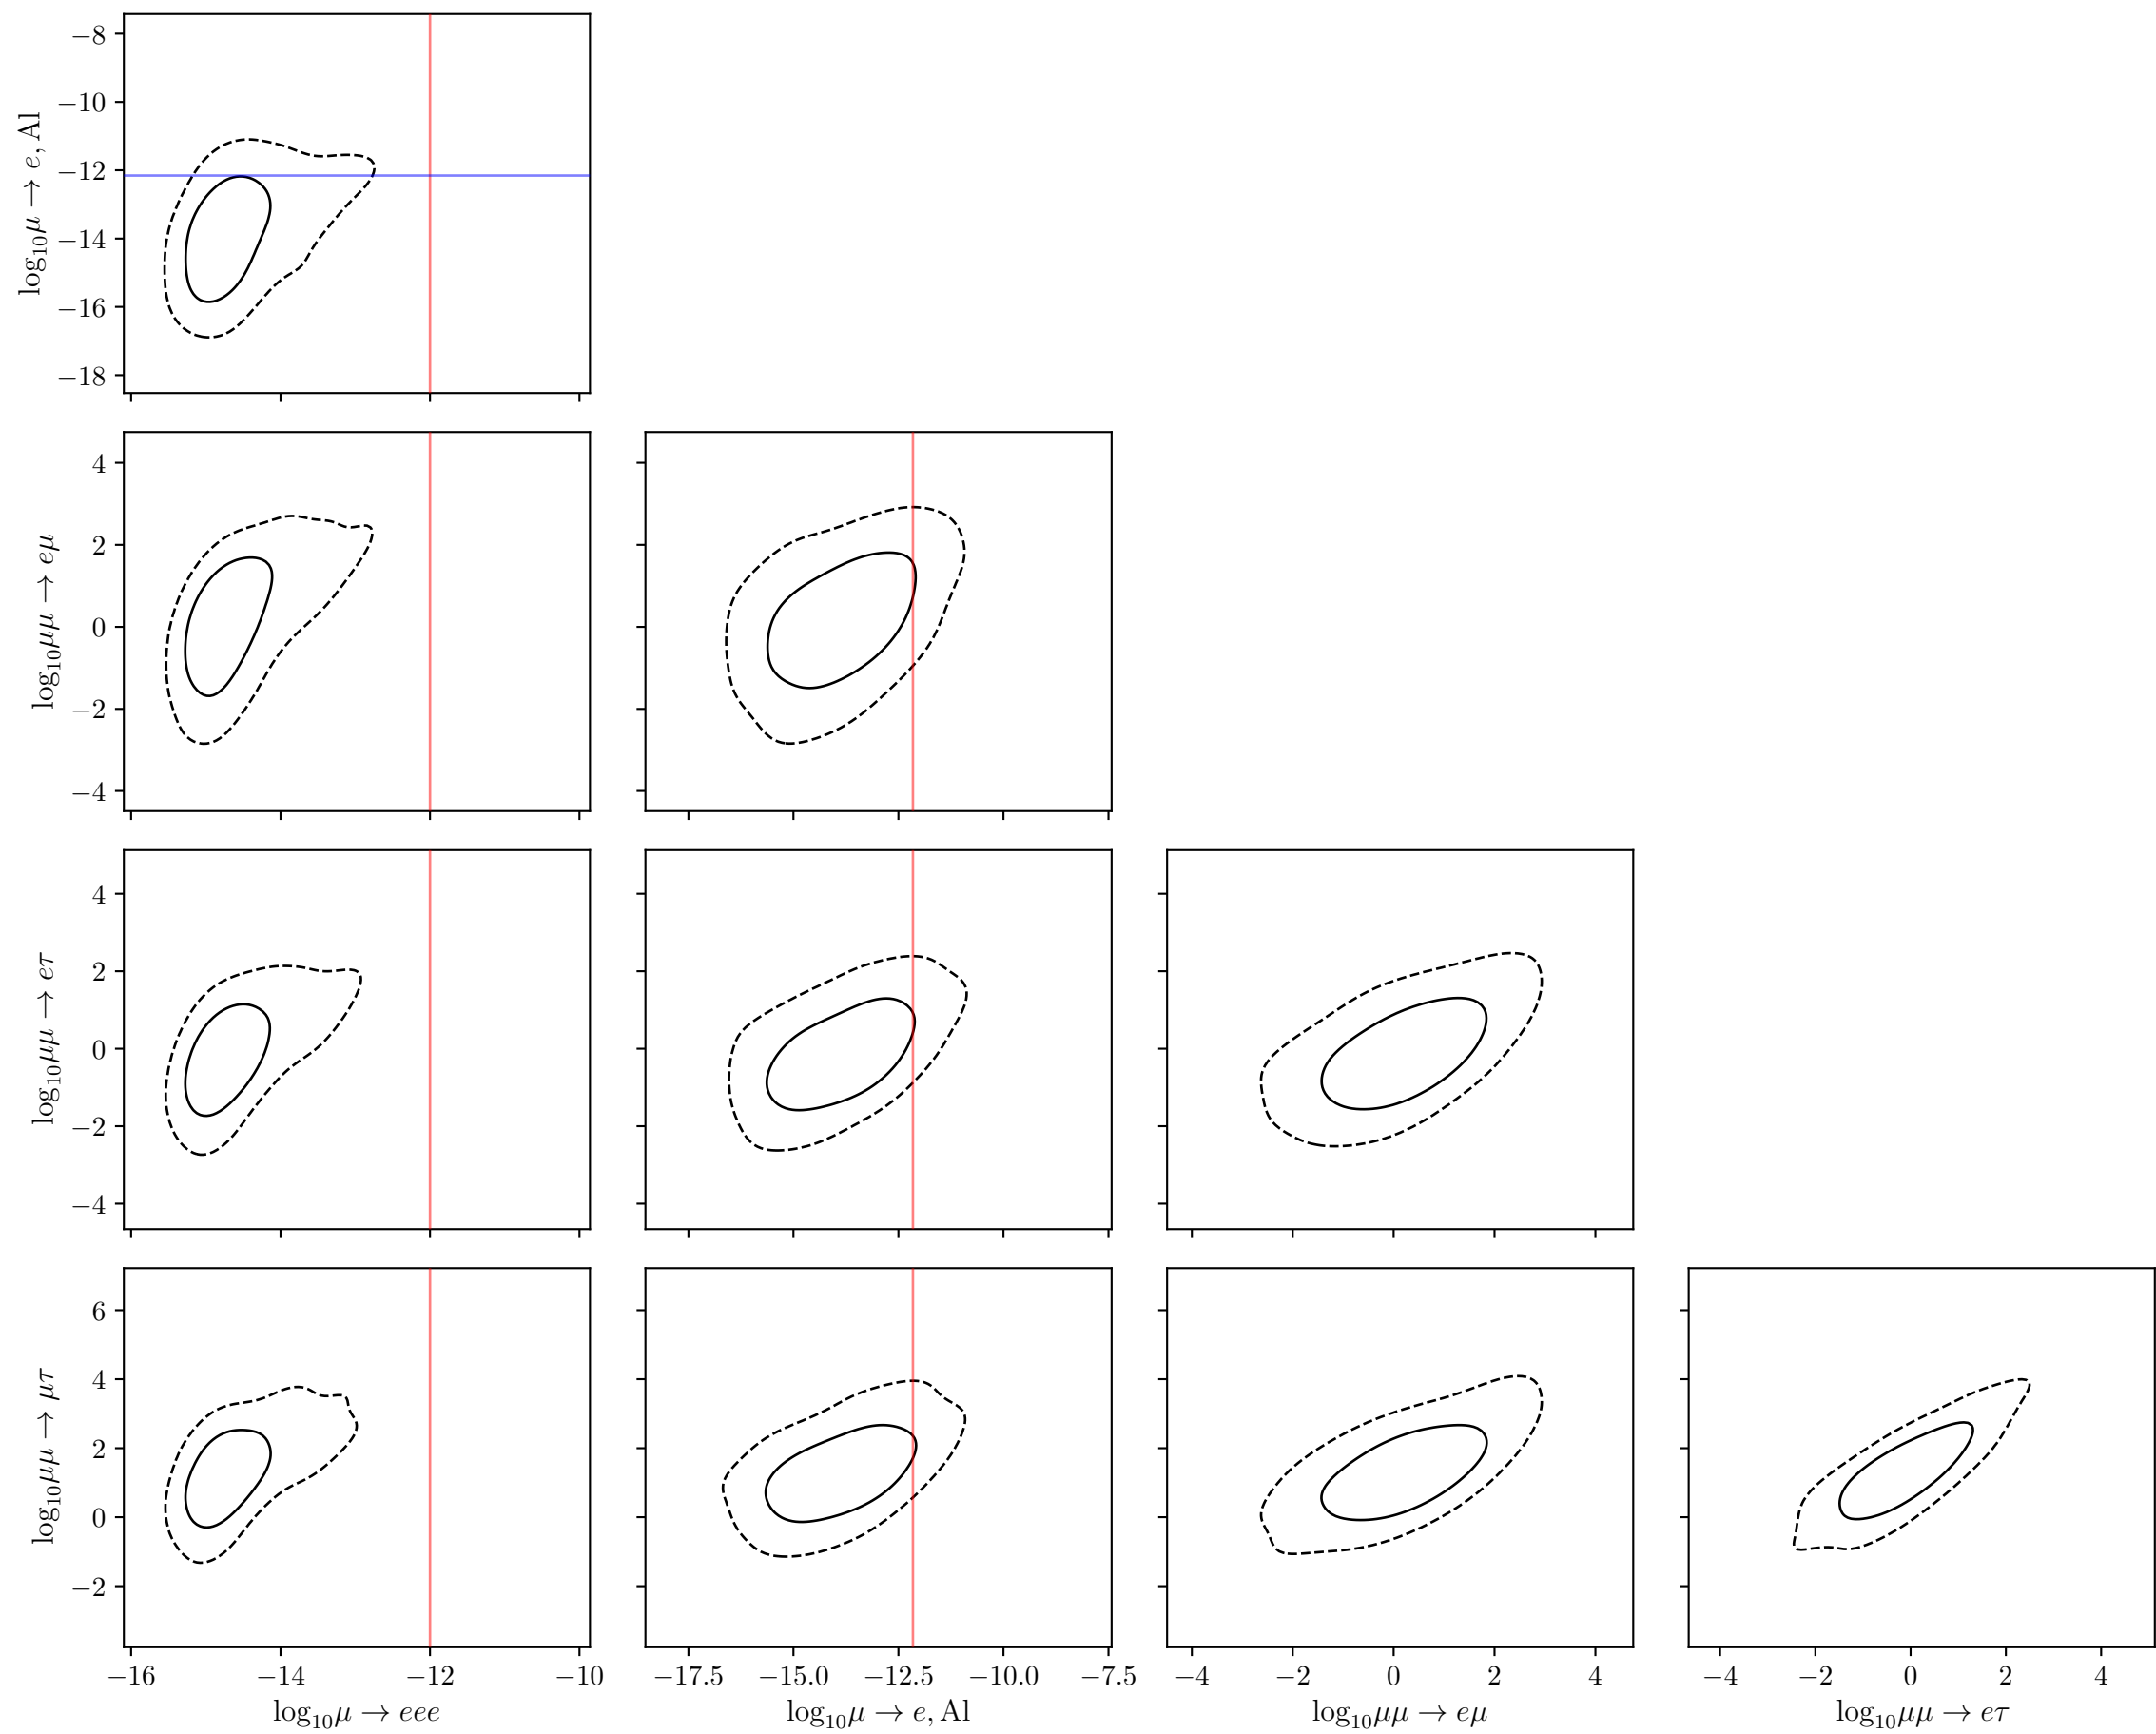

Majorana,  $X_L = \{4, 4, 3\}$ ,  $X_e = \{5, 2, 0\}$ ,

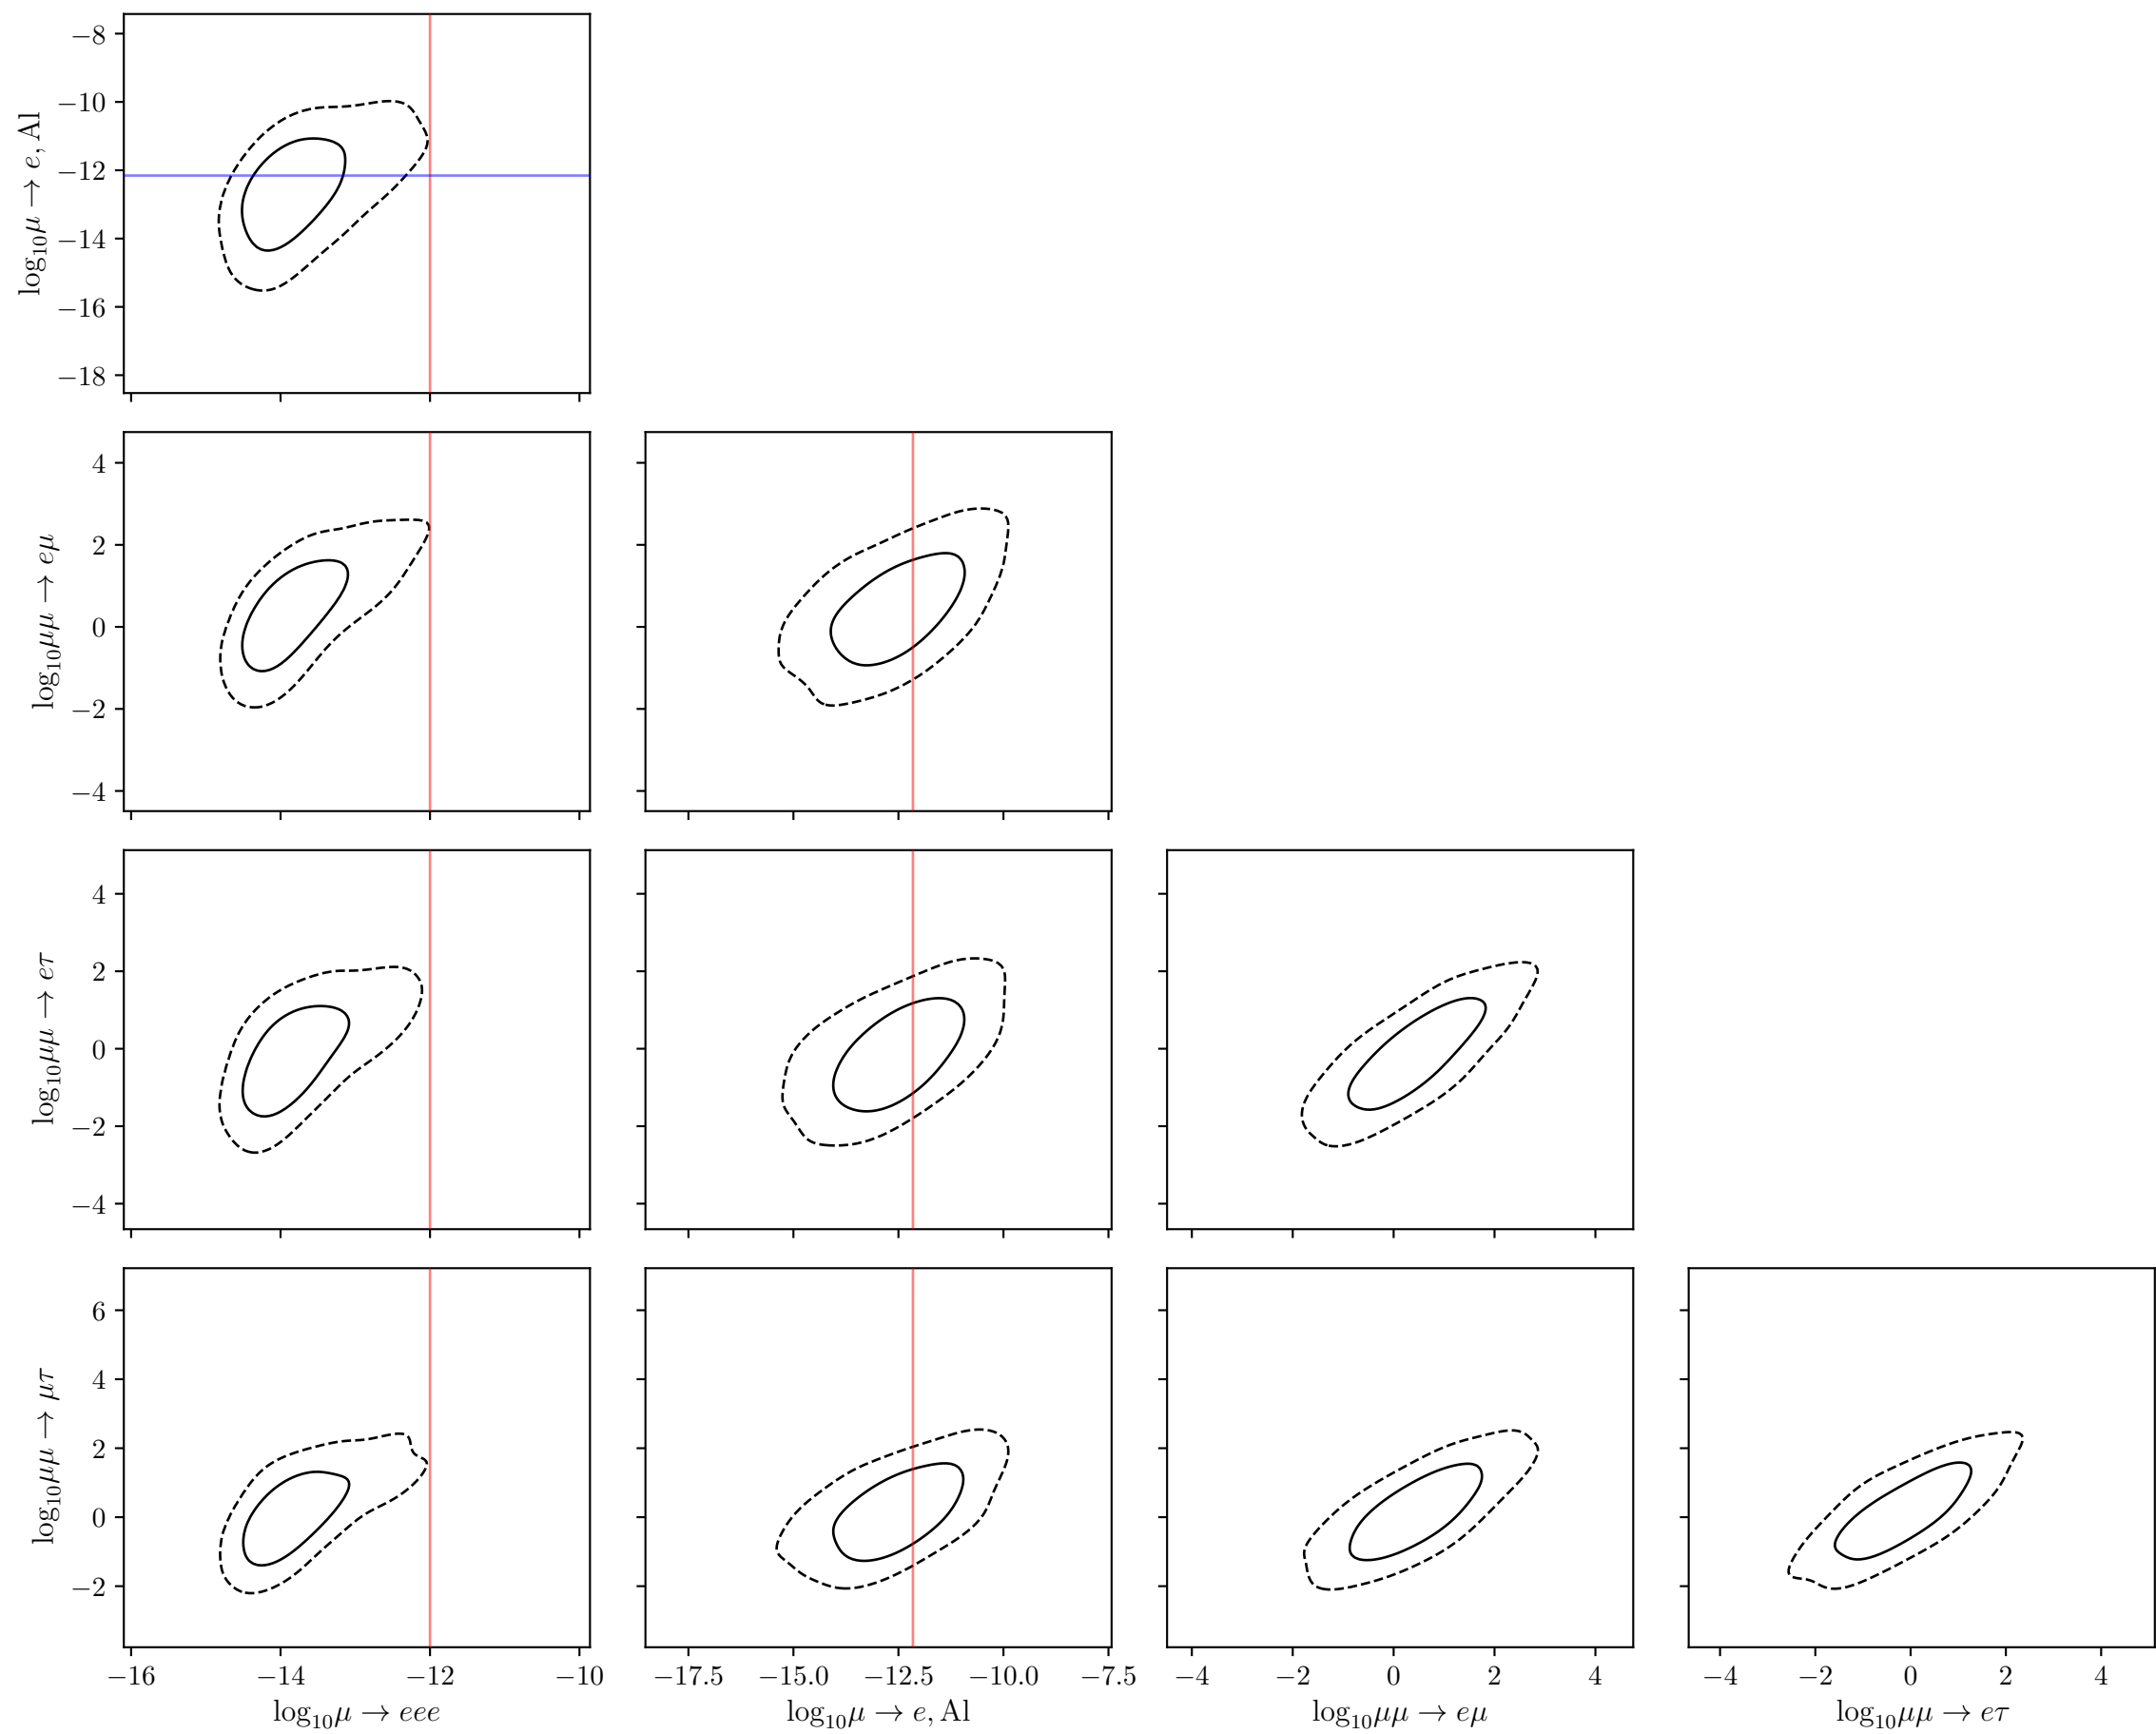

Majorana,  $X_L = \{7, 6, 5\}$ ,  $X_e = \{7, 3, 0\}$ ,

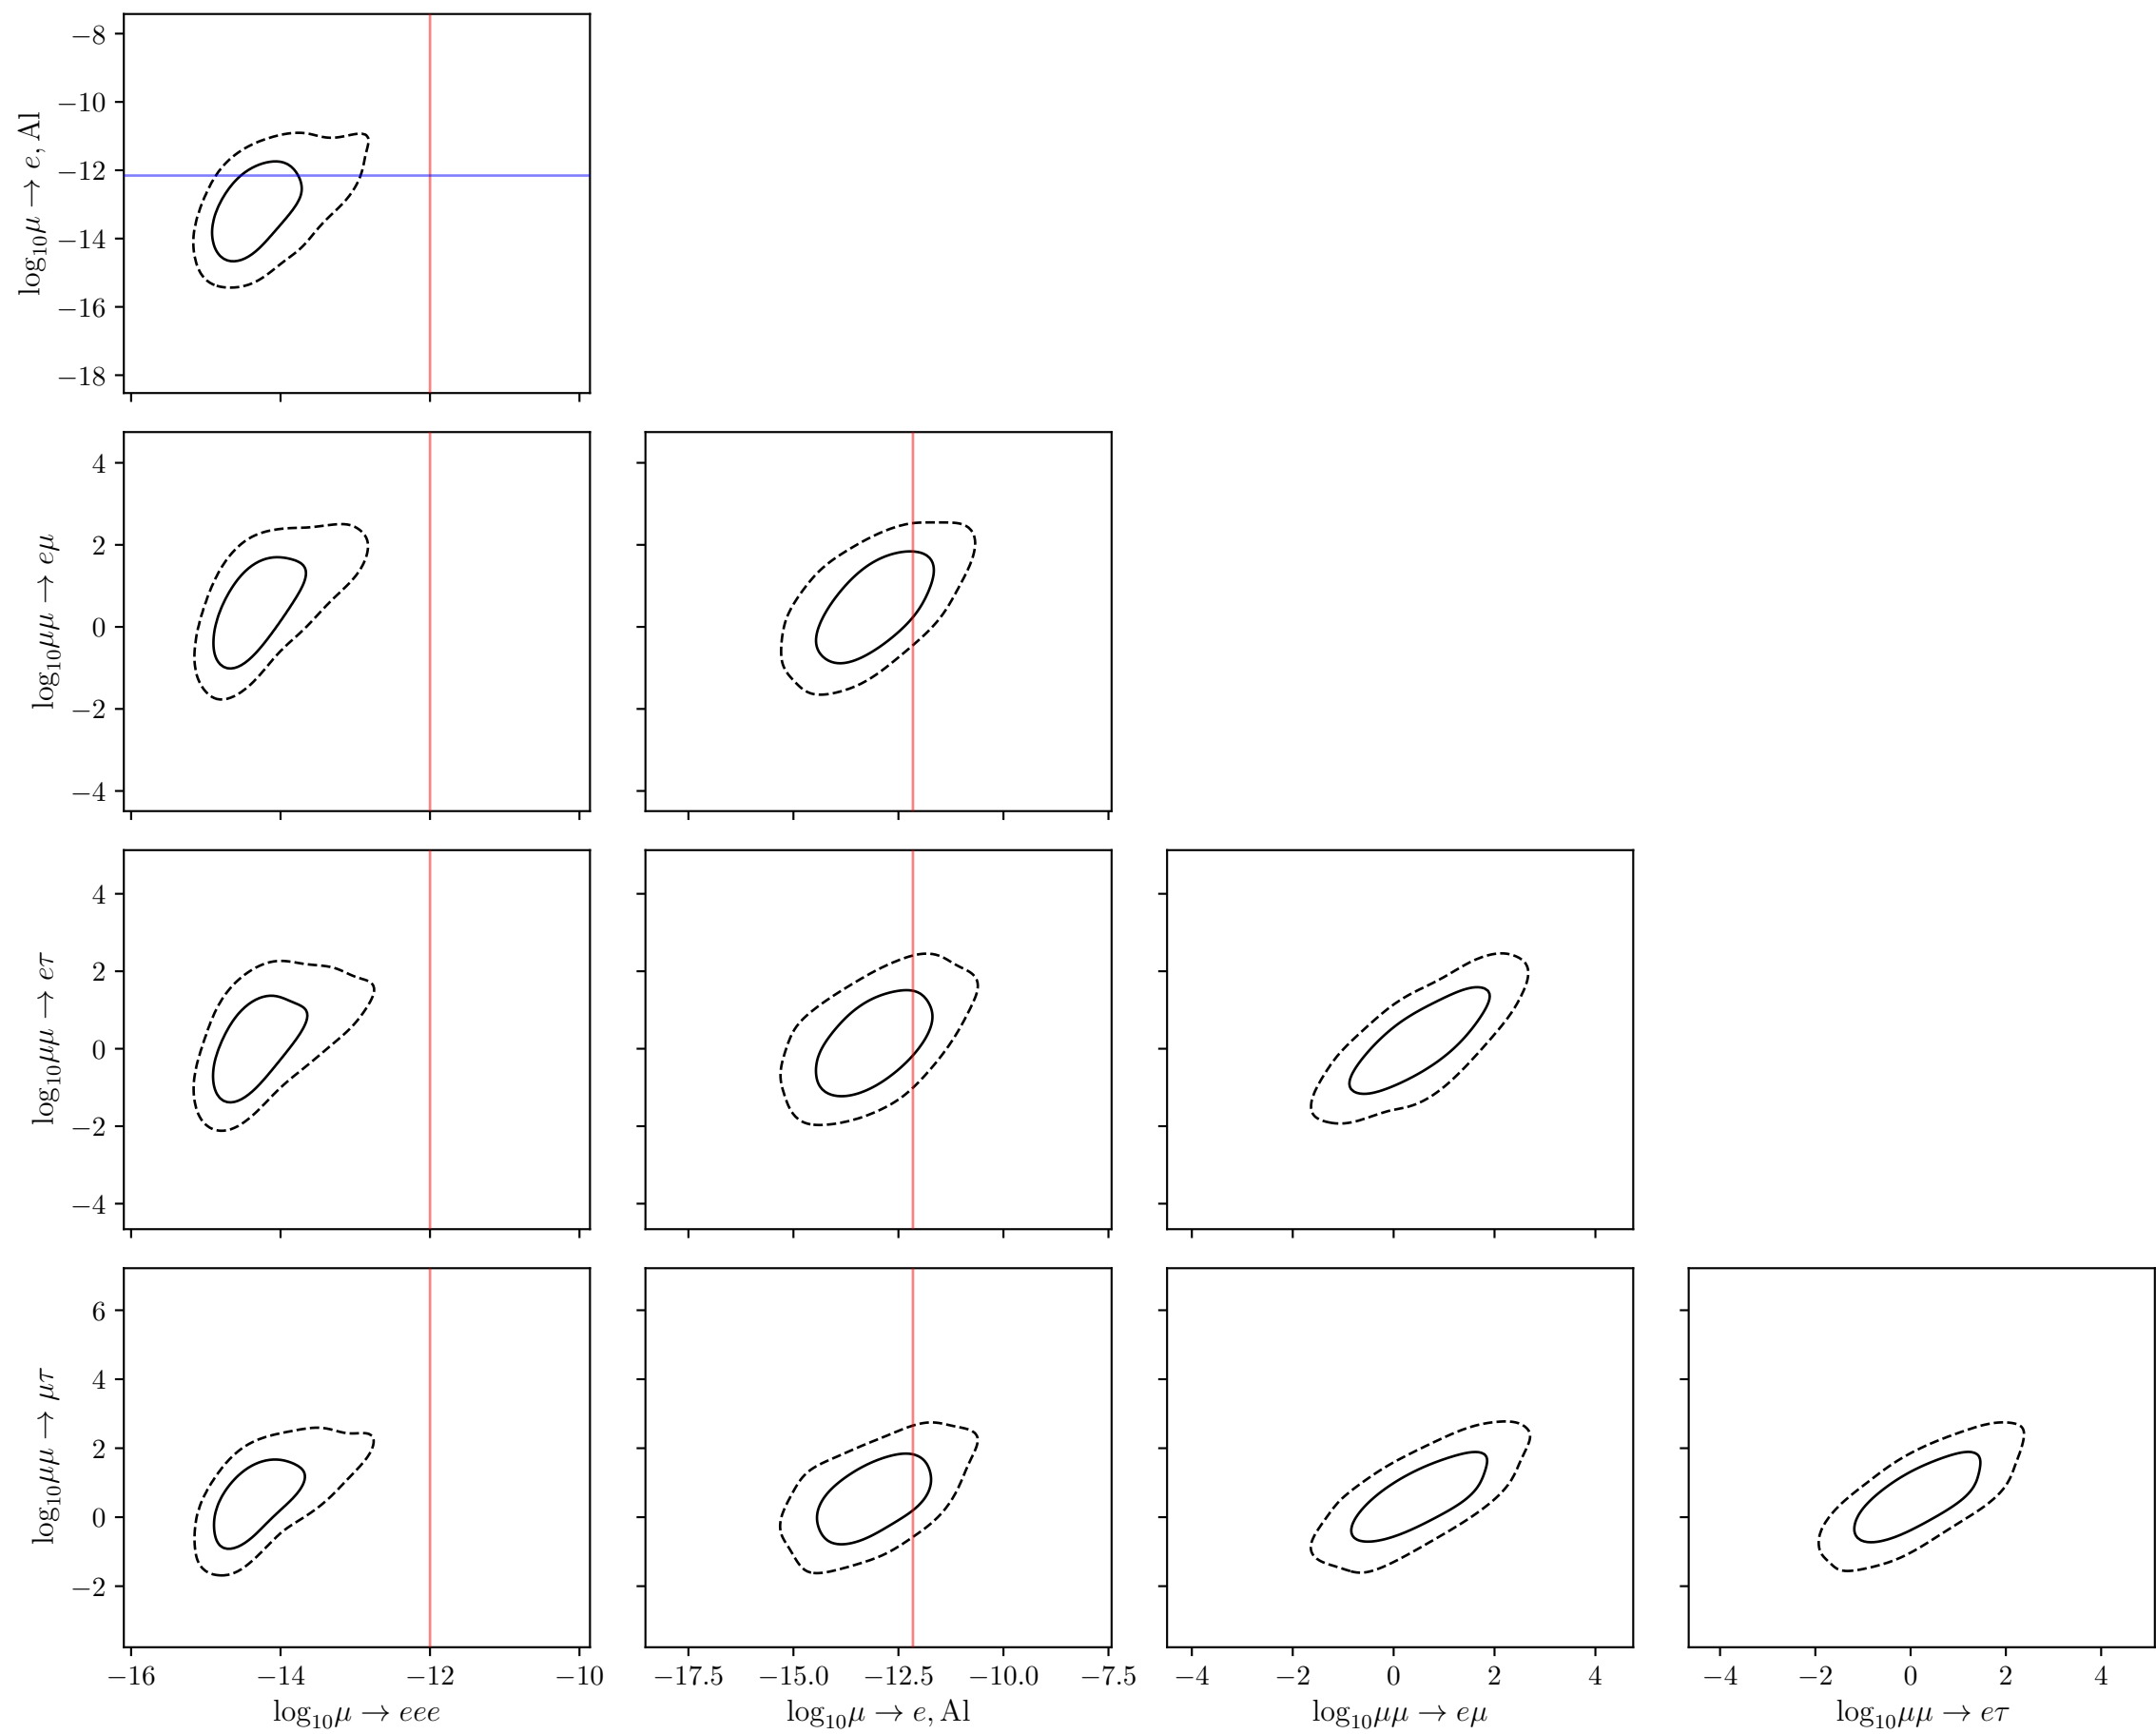

Majorana,  $X_L = \{6, 6, 5\}$ ,  $X_e = \{-1, 1, 5\}$ ,

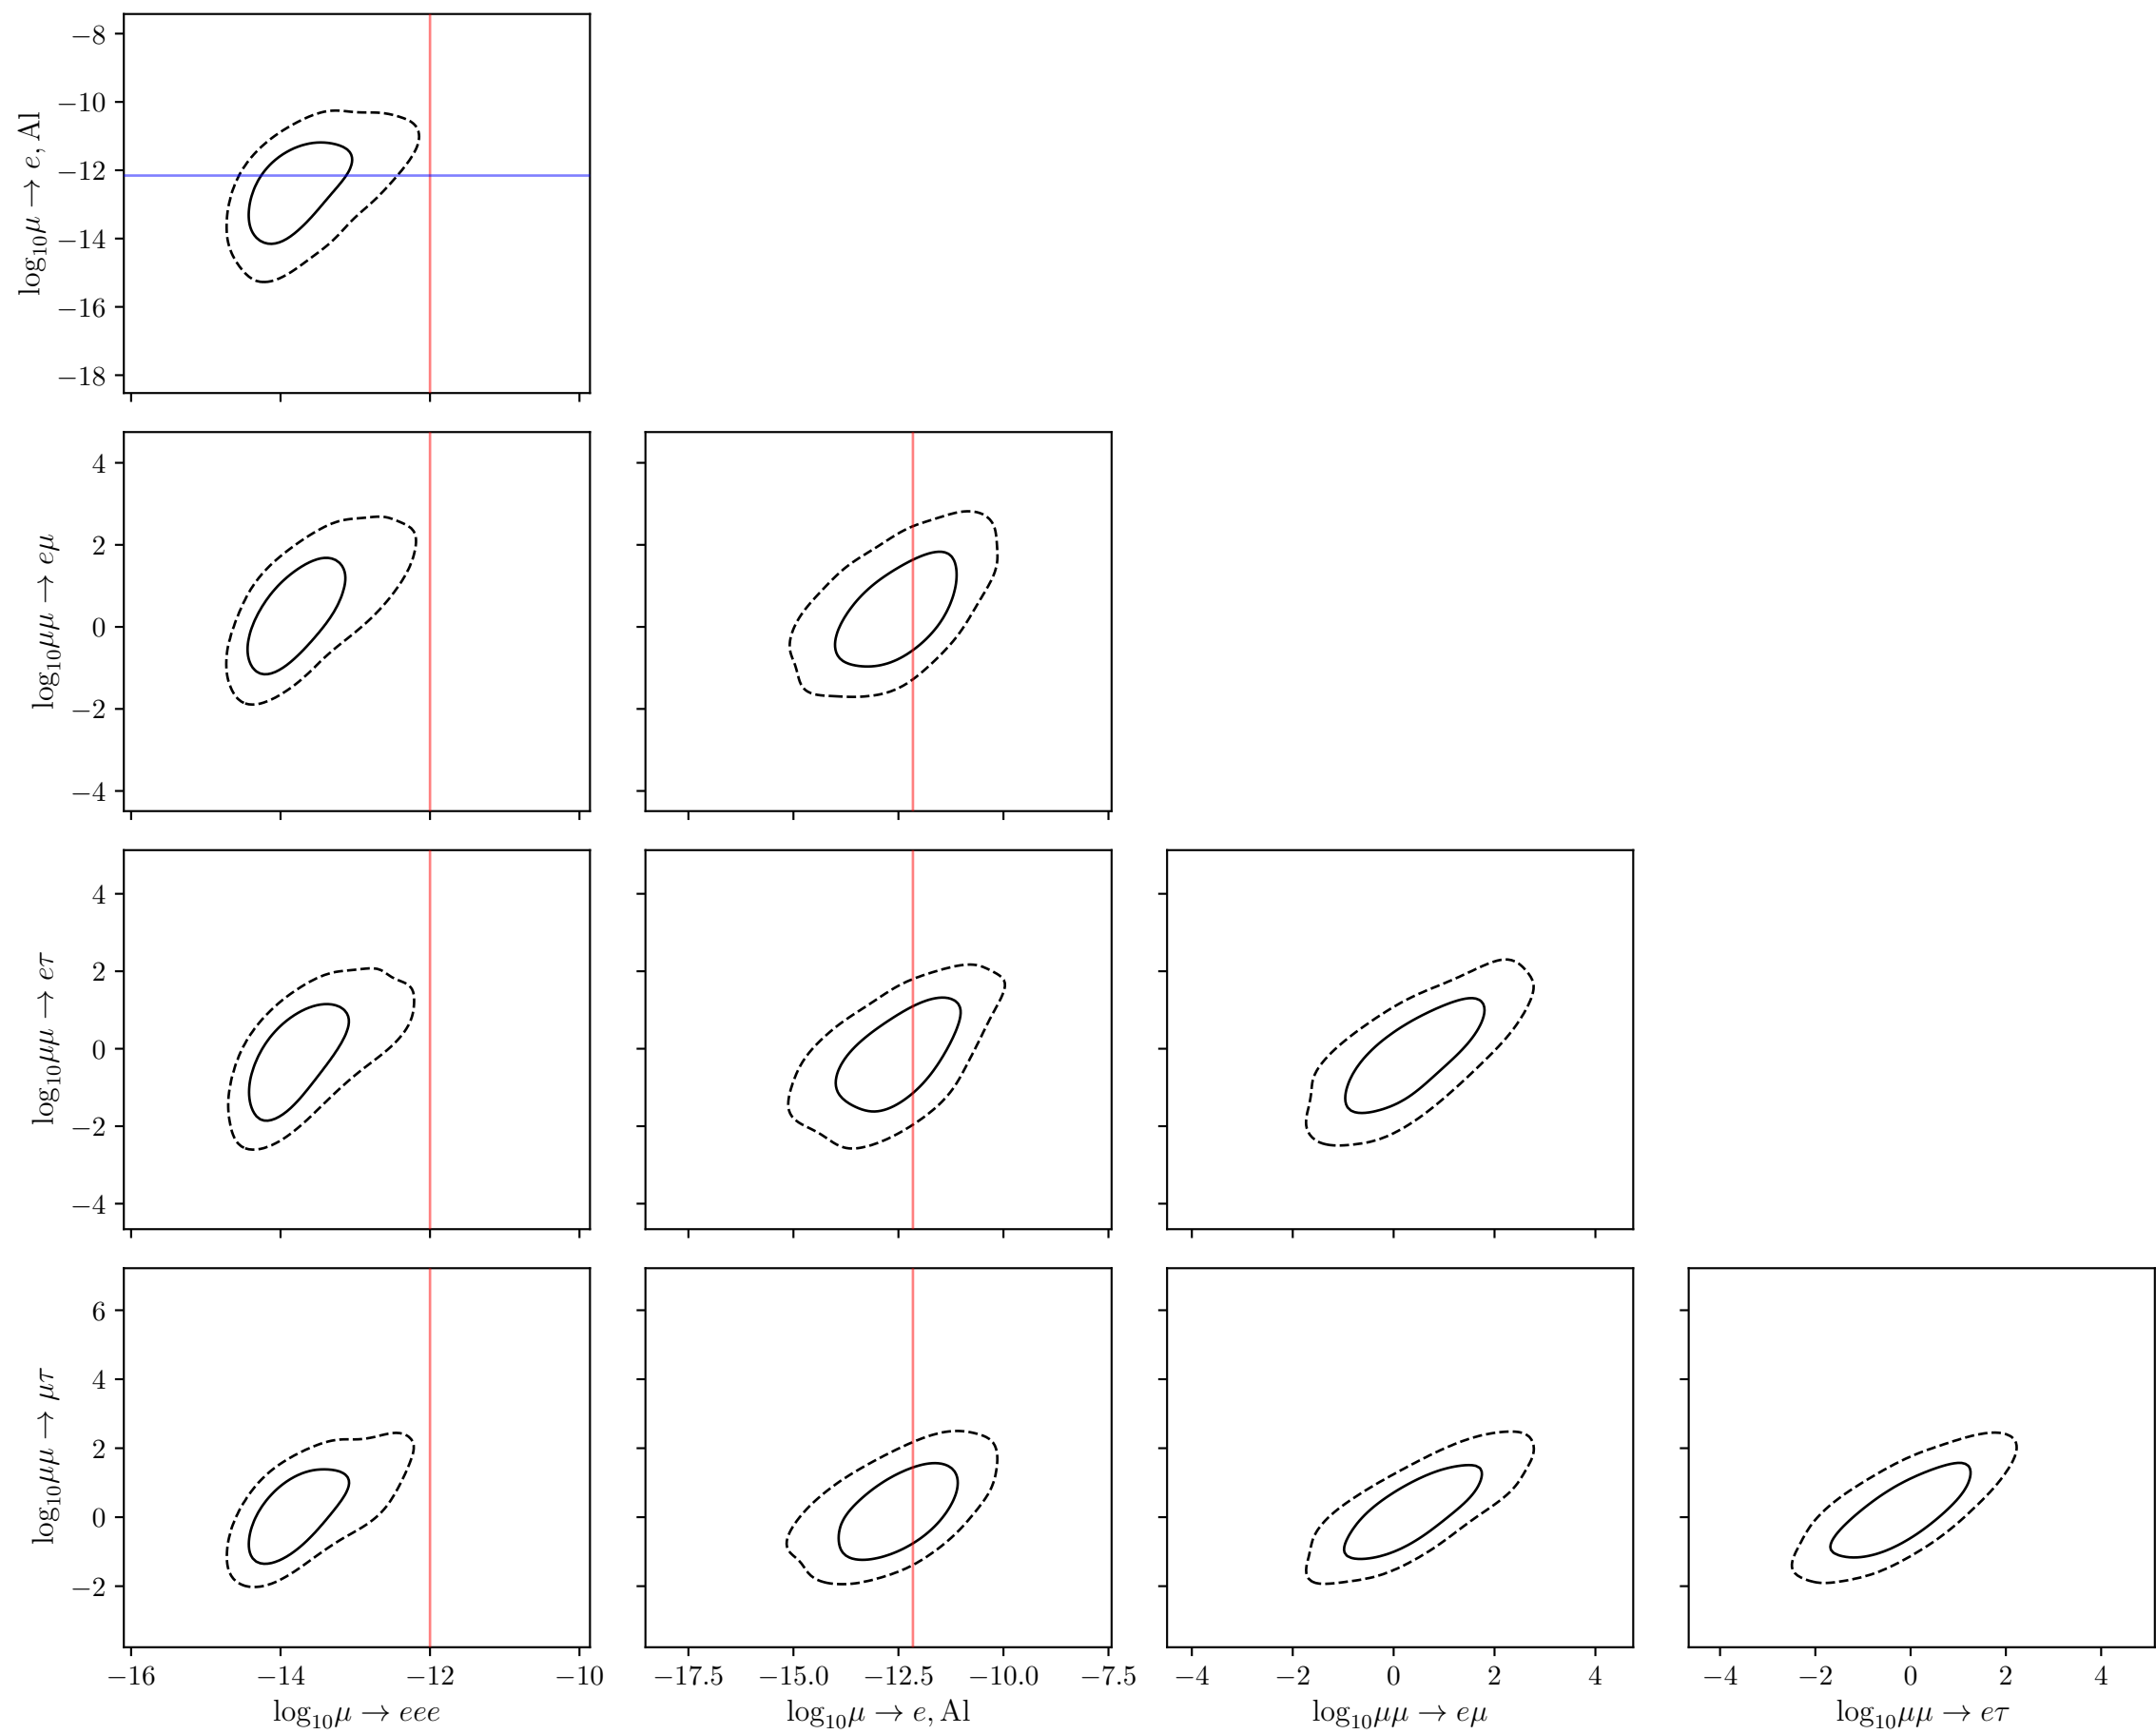

Majorana,  $X_L = \{7, 7, 6\}$ ,  $X_e = \{-3, -1, 2\}$ ,

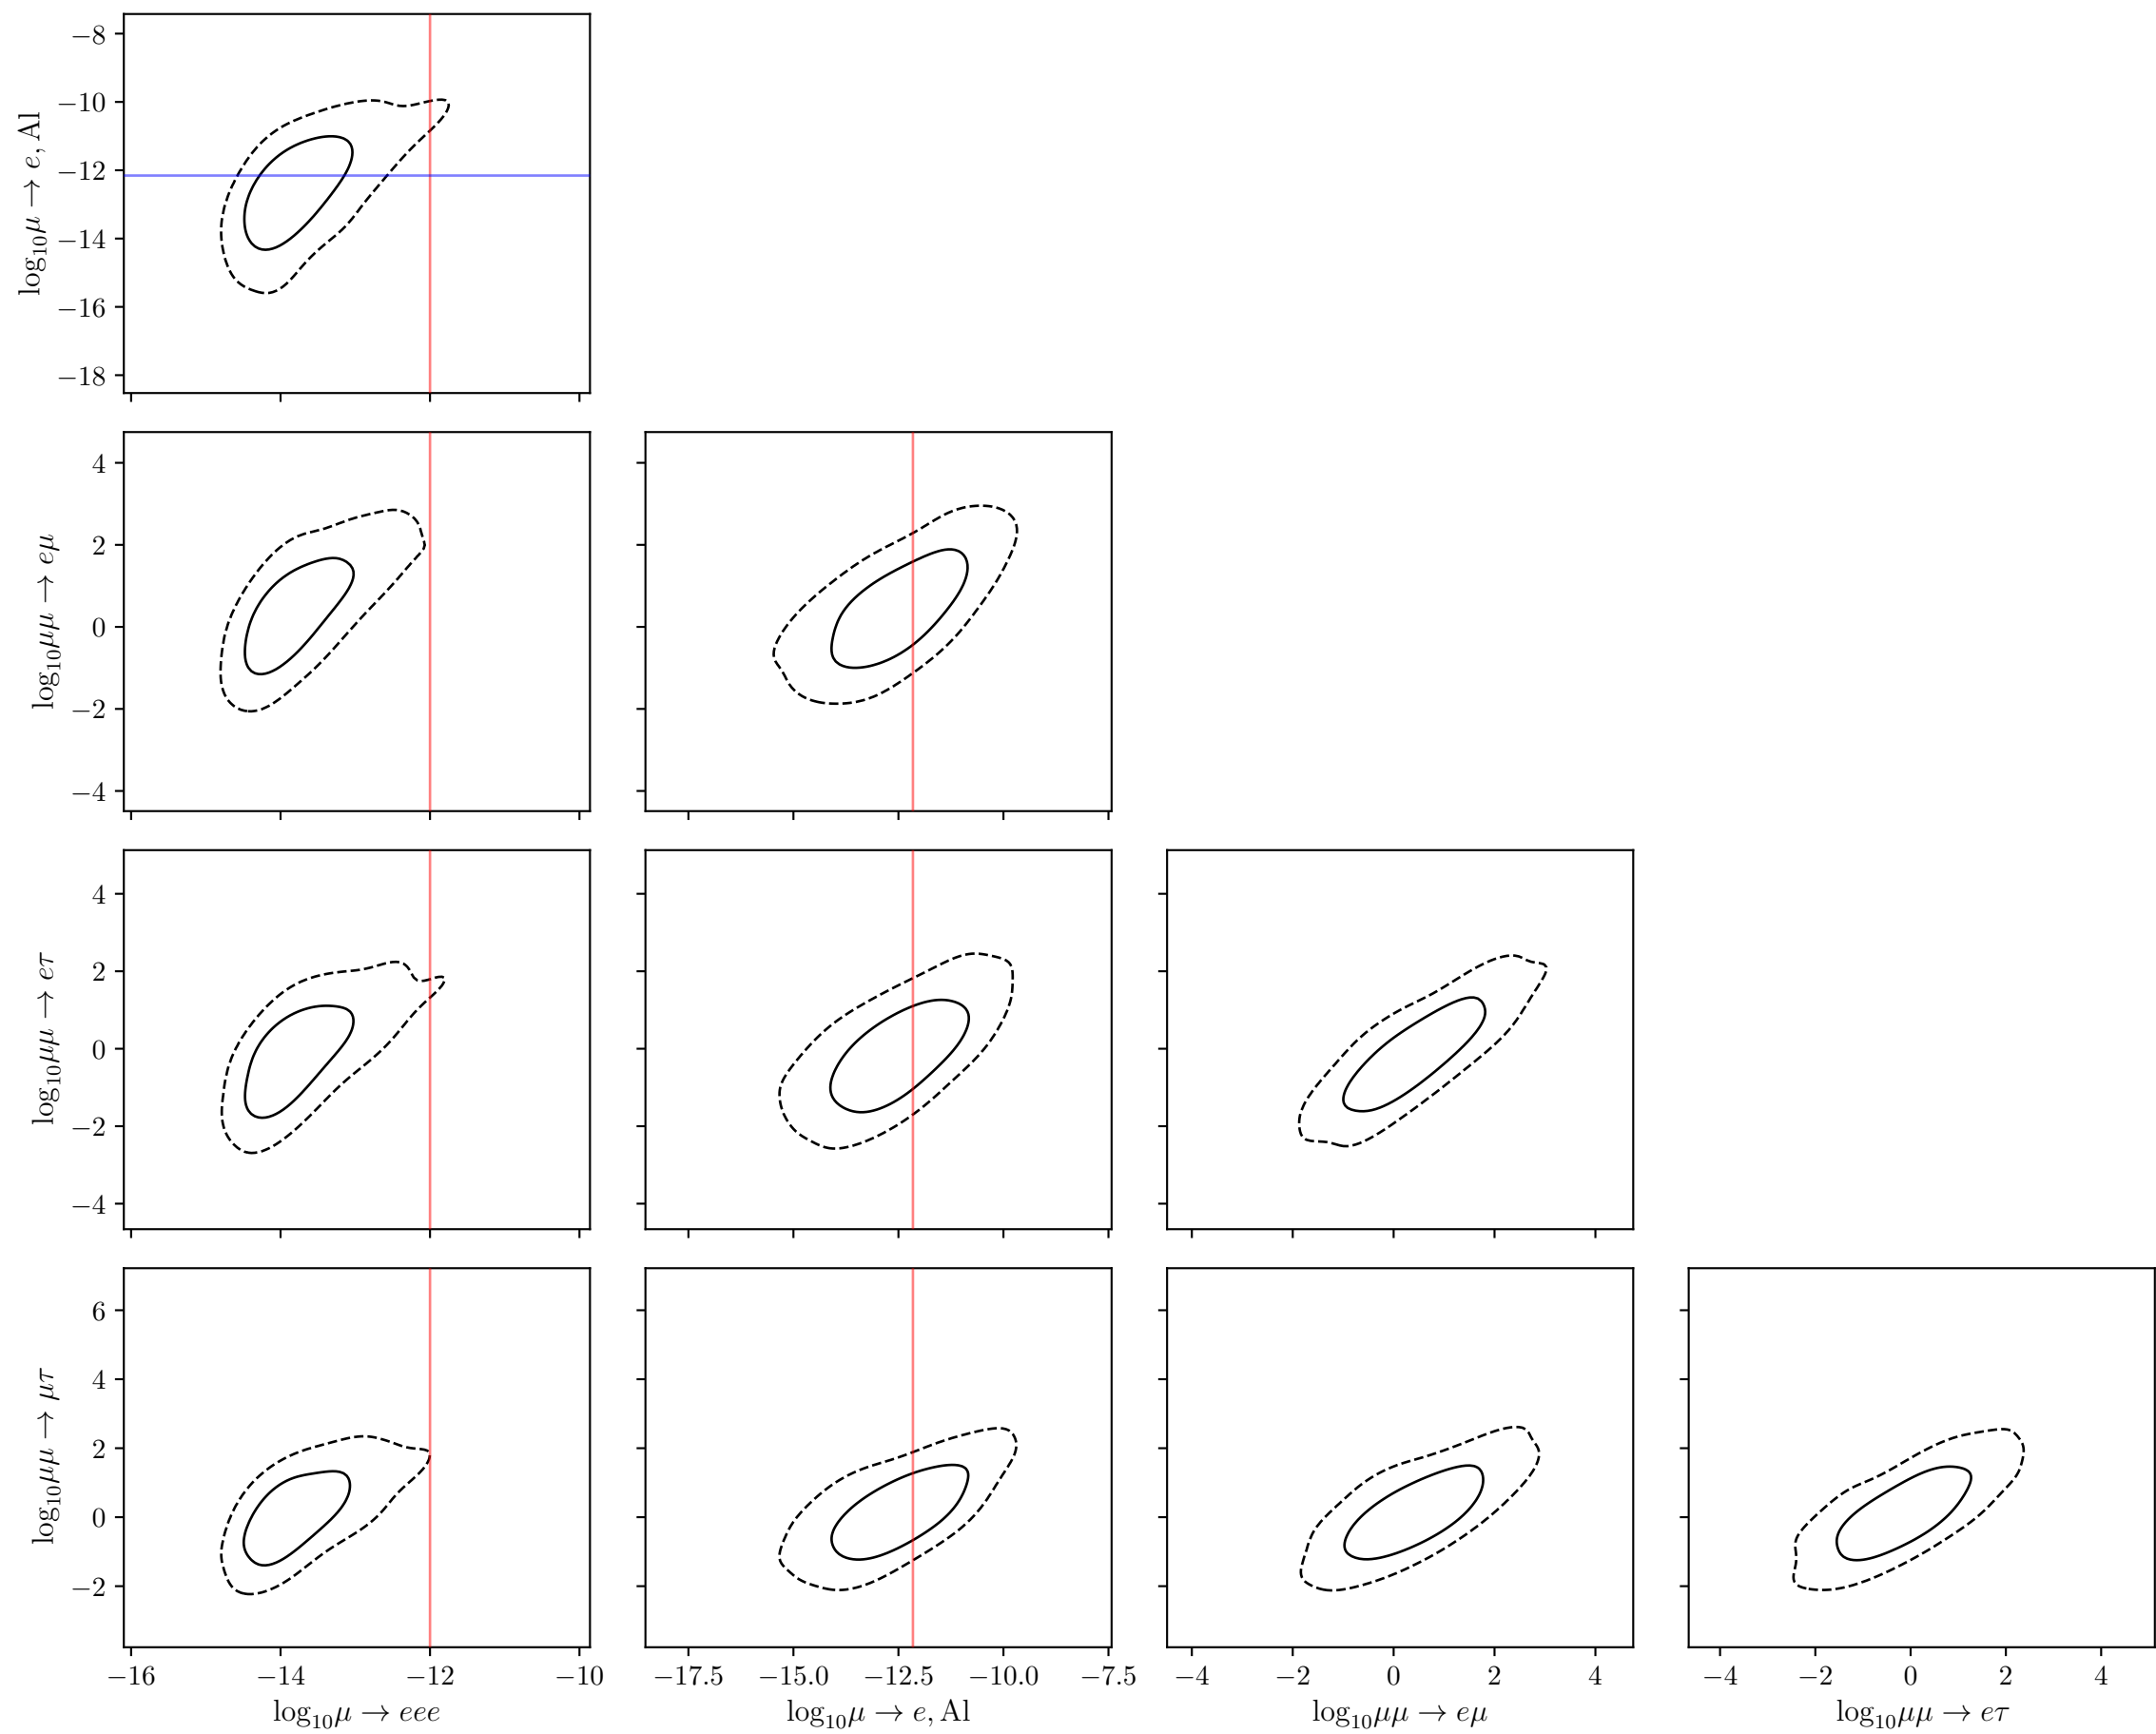

Majorana,  $X_L = \{5, 5, -2\}$ ,  $X_e = \{-7, -2, 7\}$ ,

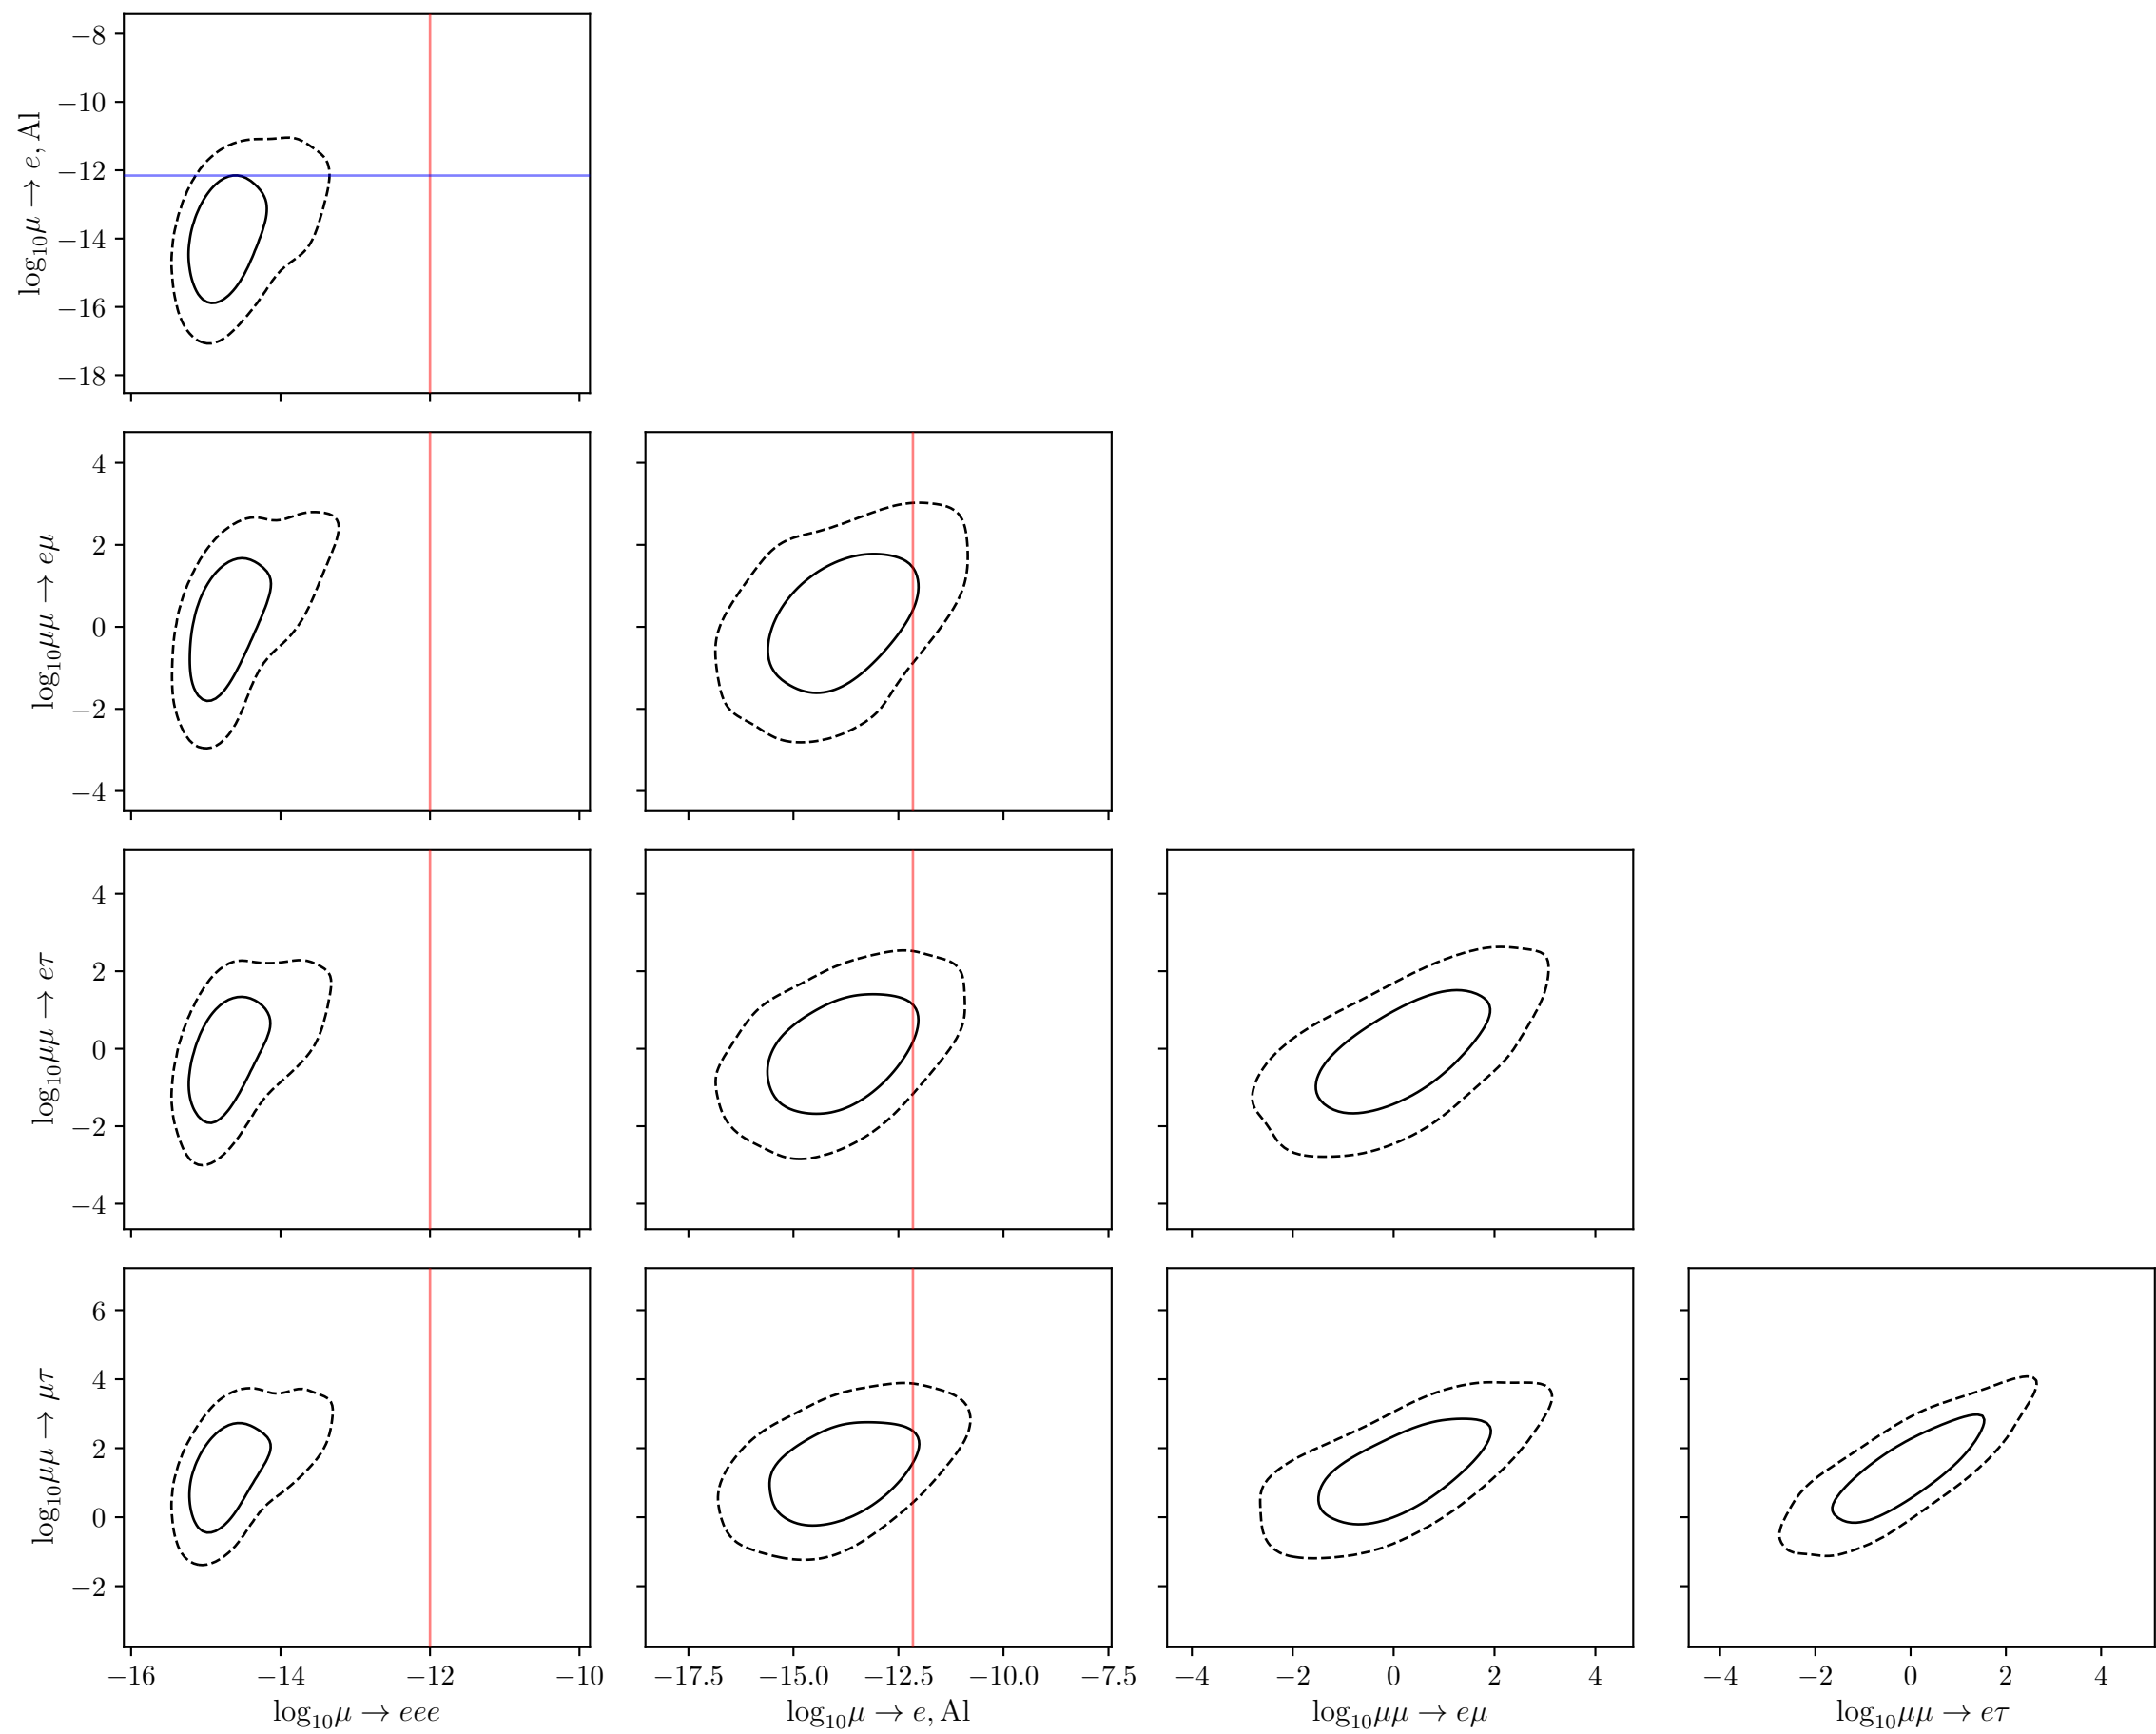

Majorana,  $X_L = \{7, 7, 6\}$ ,  $X_e = \{-2, 0, 4\}$ ,

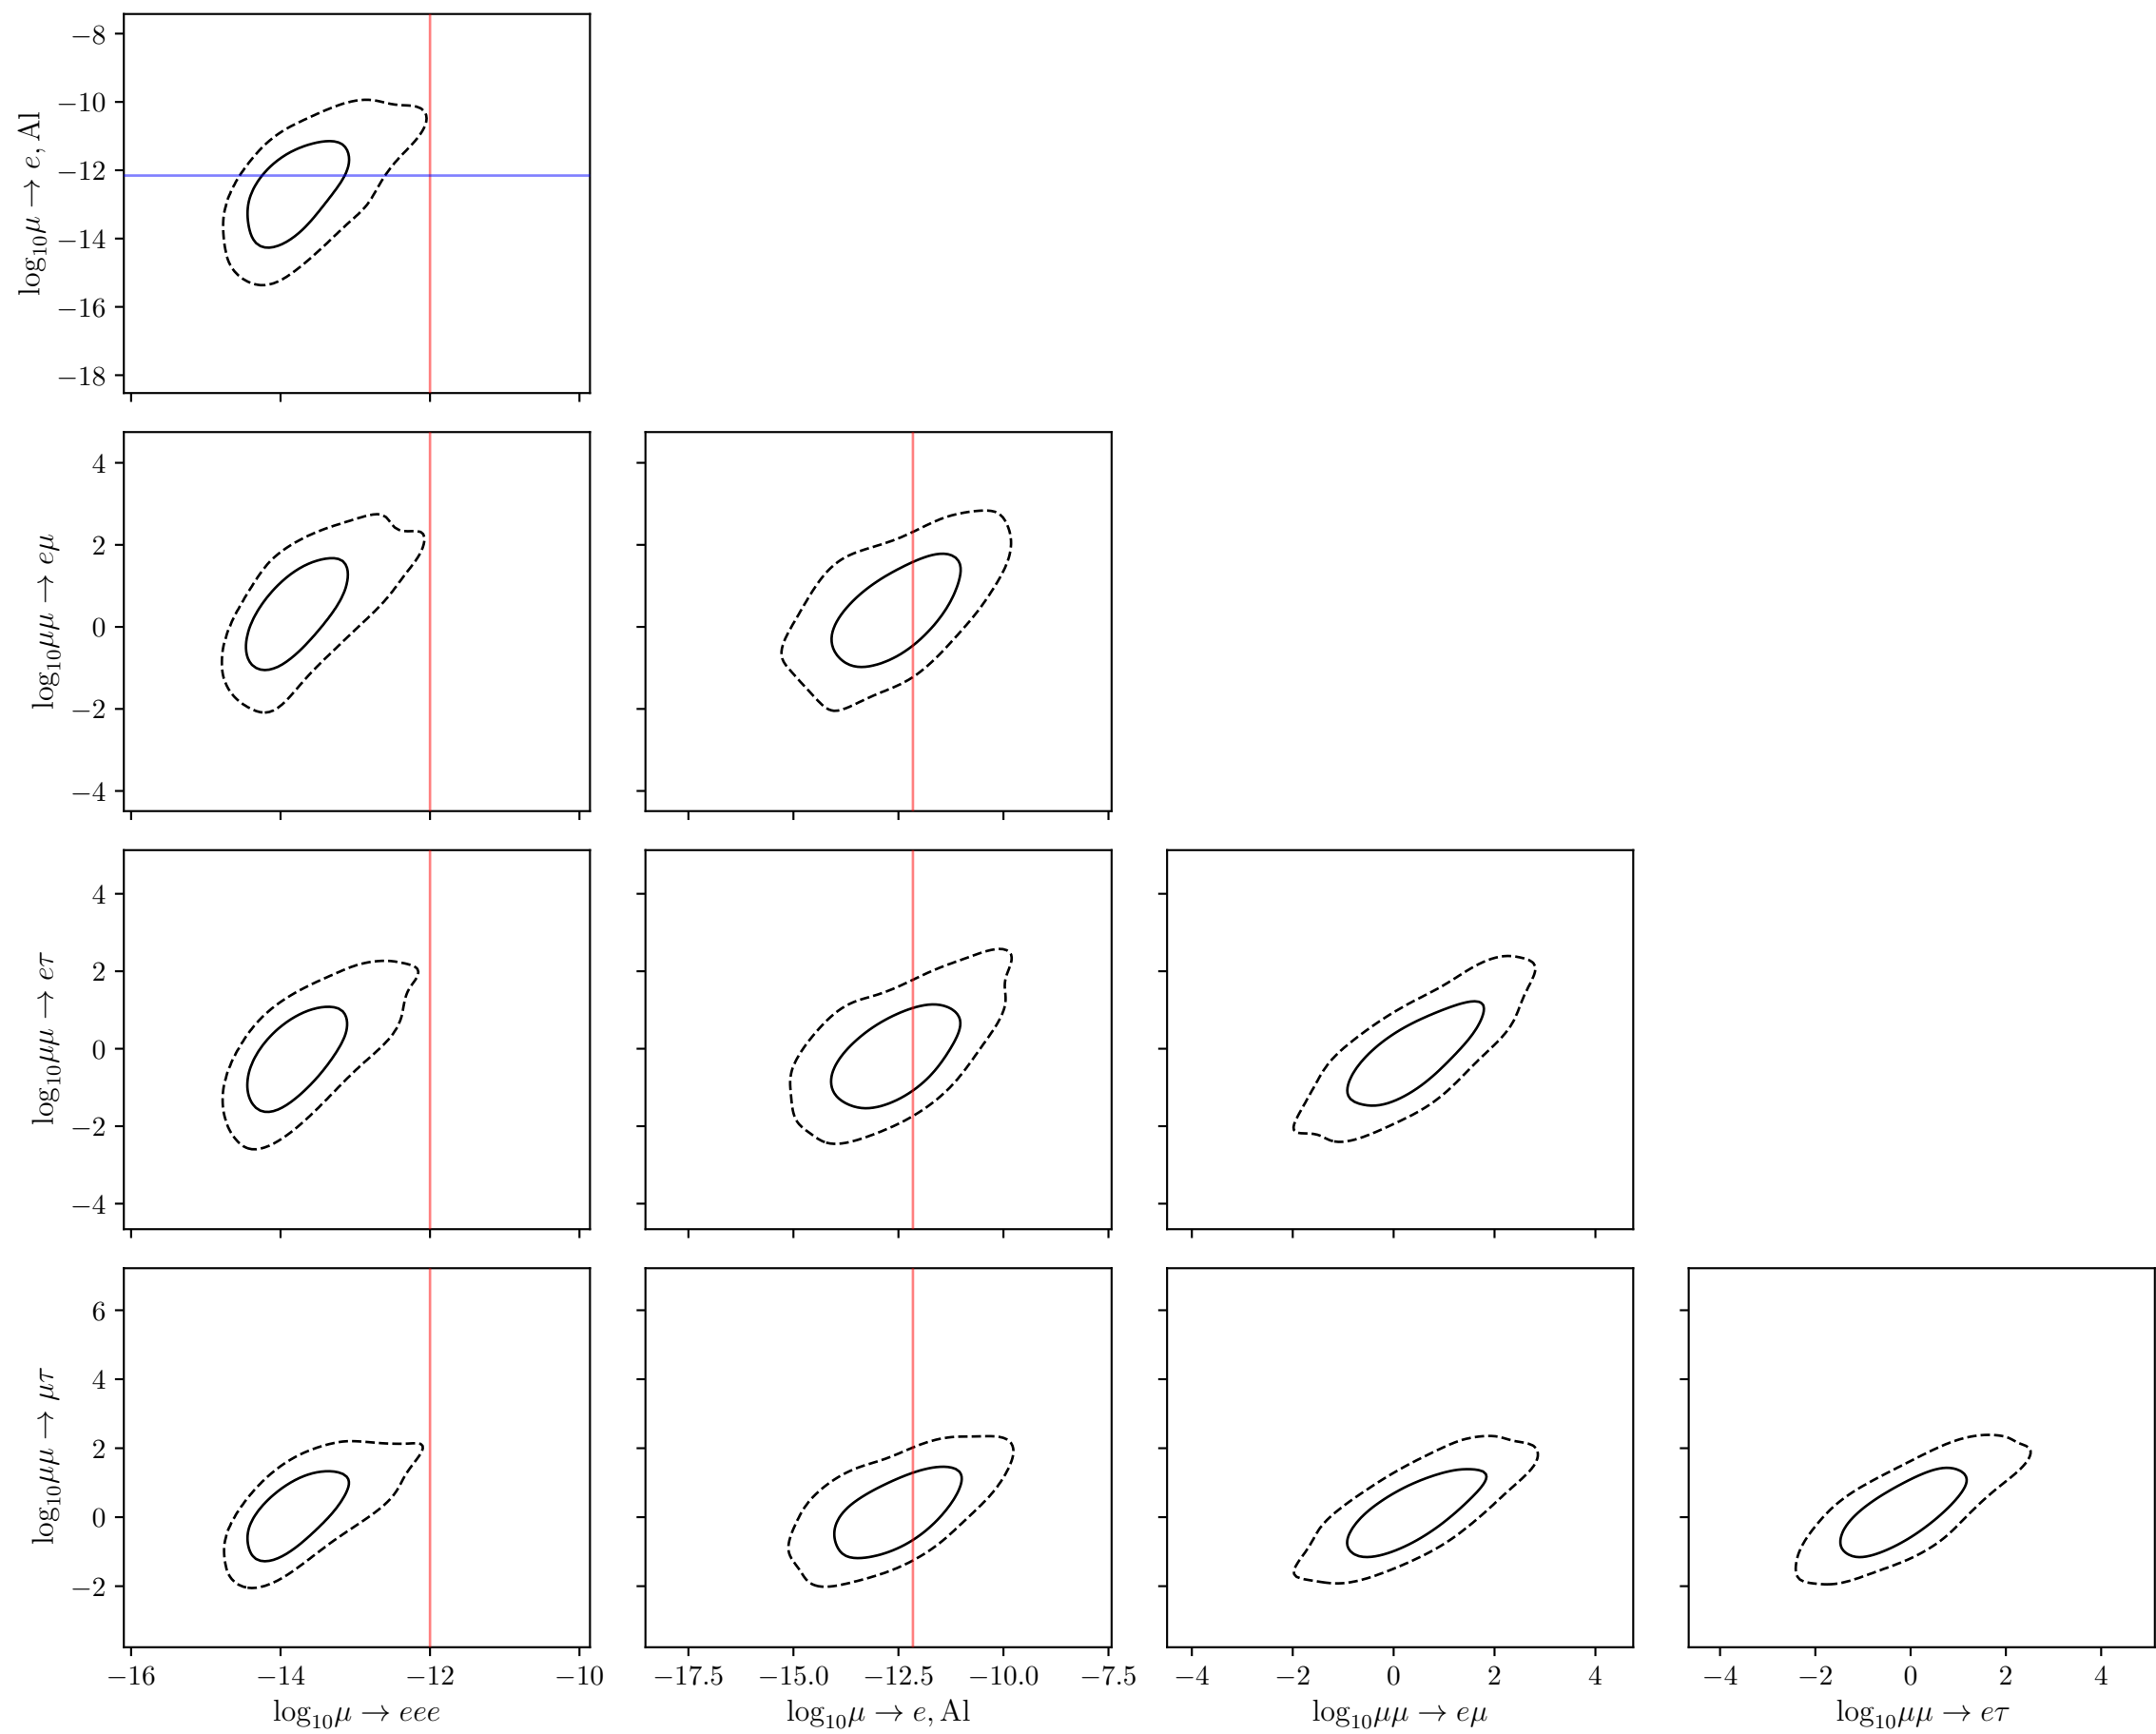



Majorana,  $X_L = \{5, 5, 4\}$ ,  $X_e = \{6, 2, 0\}$ ,

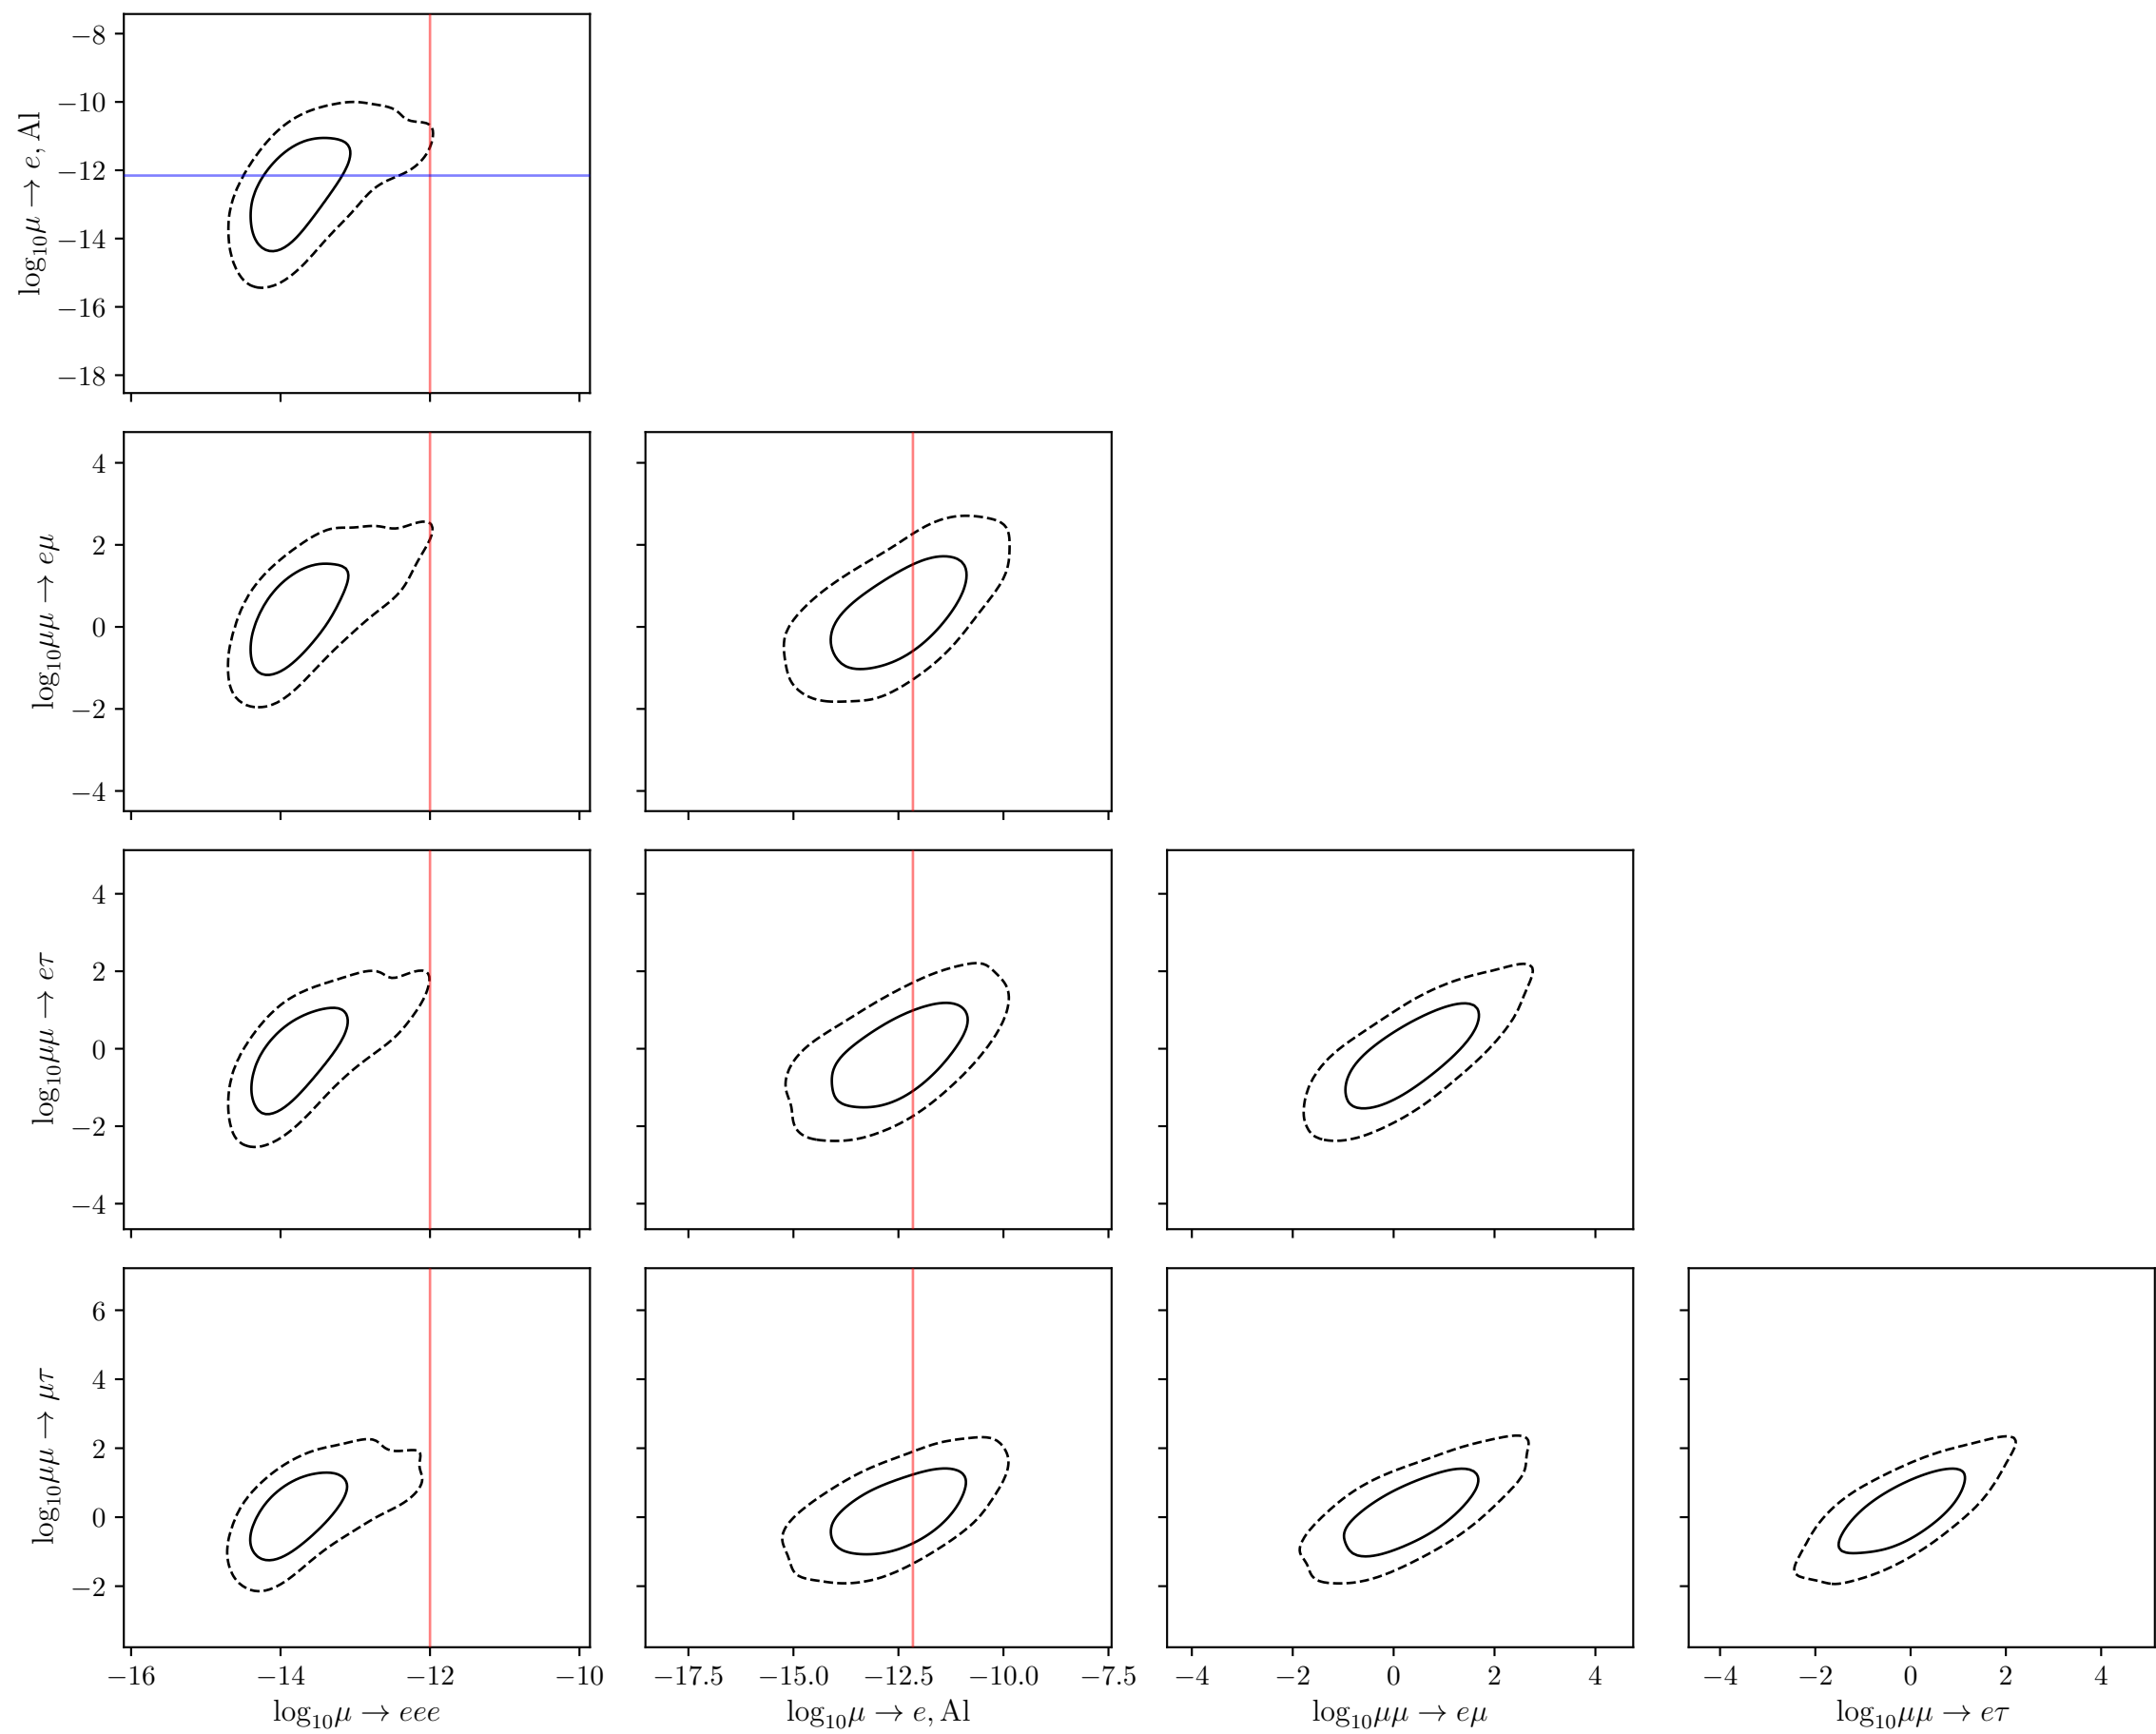

Majorana,  $X_L = \{1, 1, -1\}$ ,  $X_e = \{-7, -5, -4\}$ ,

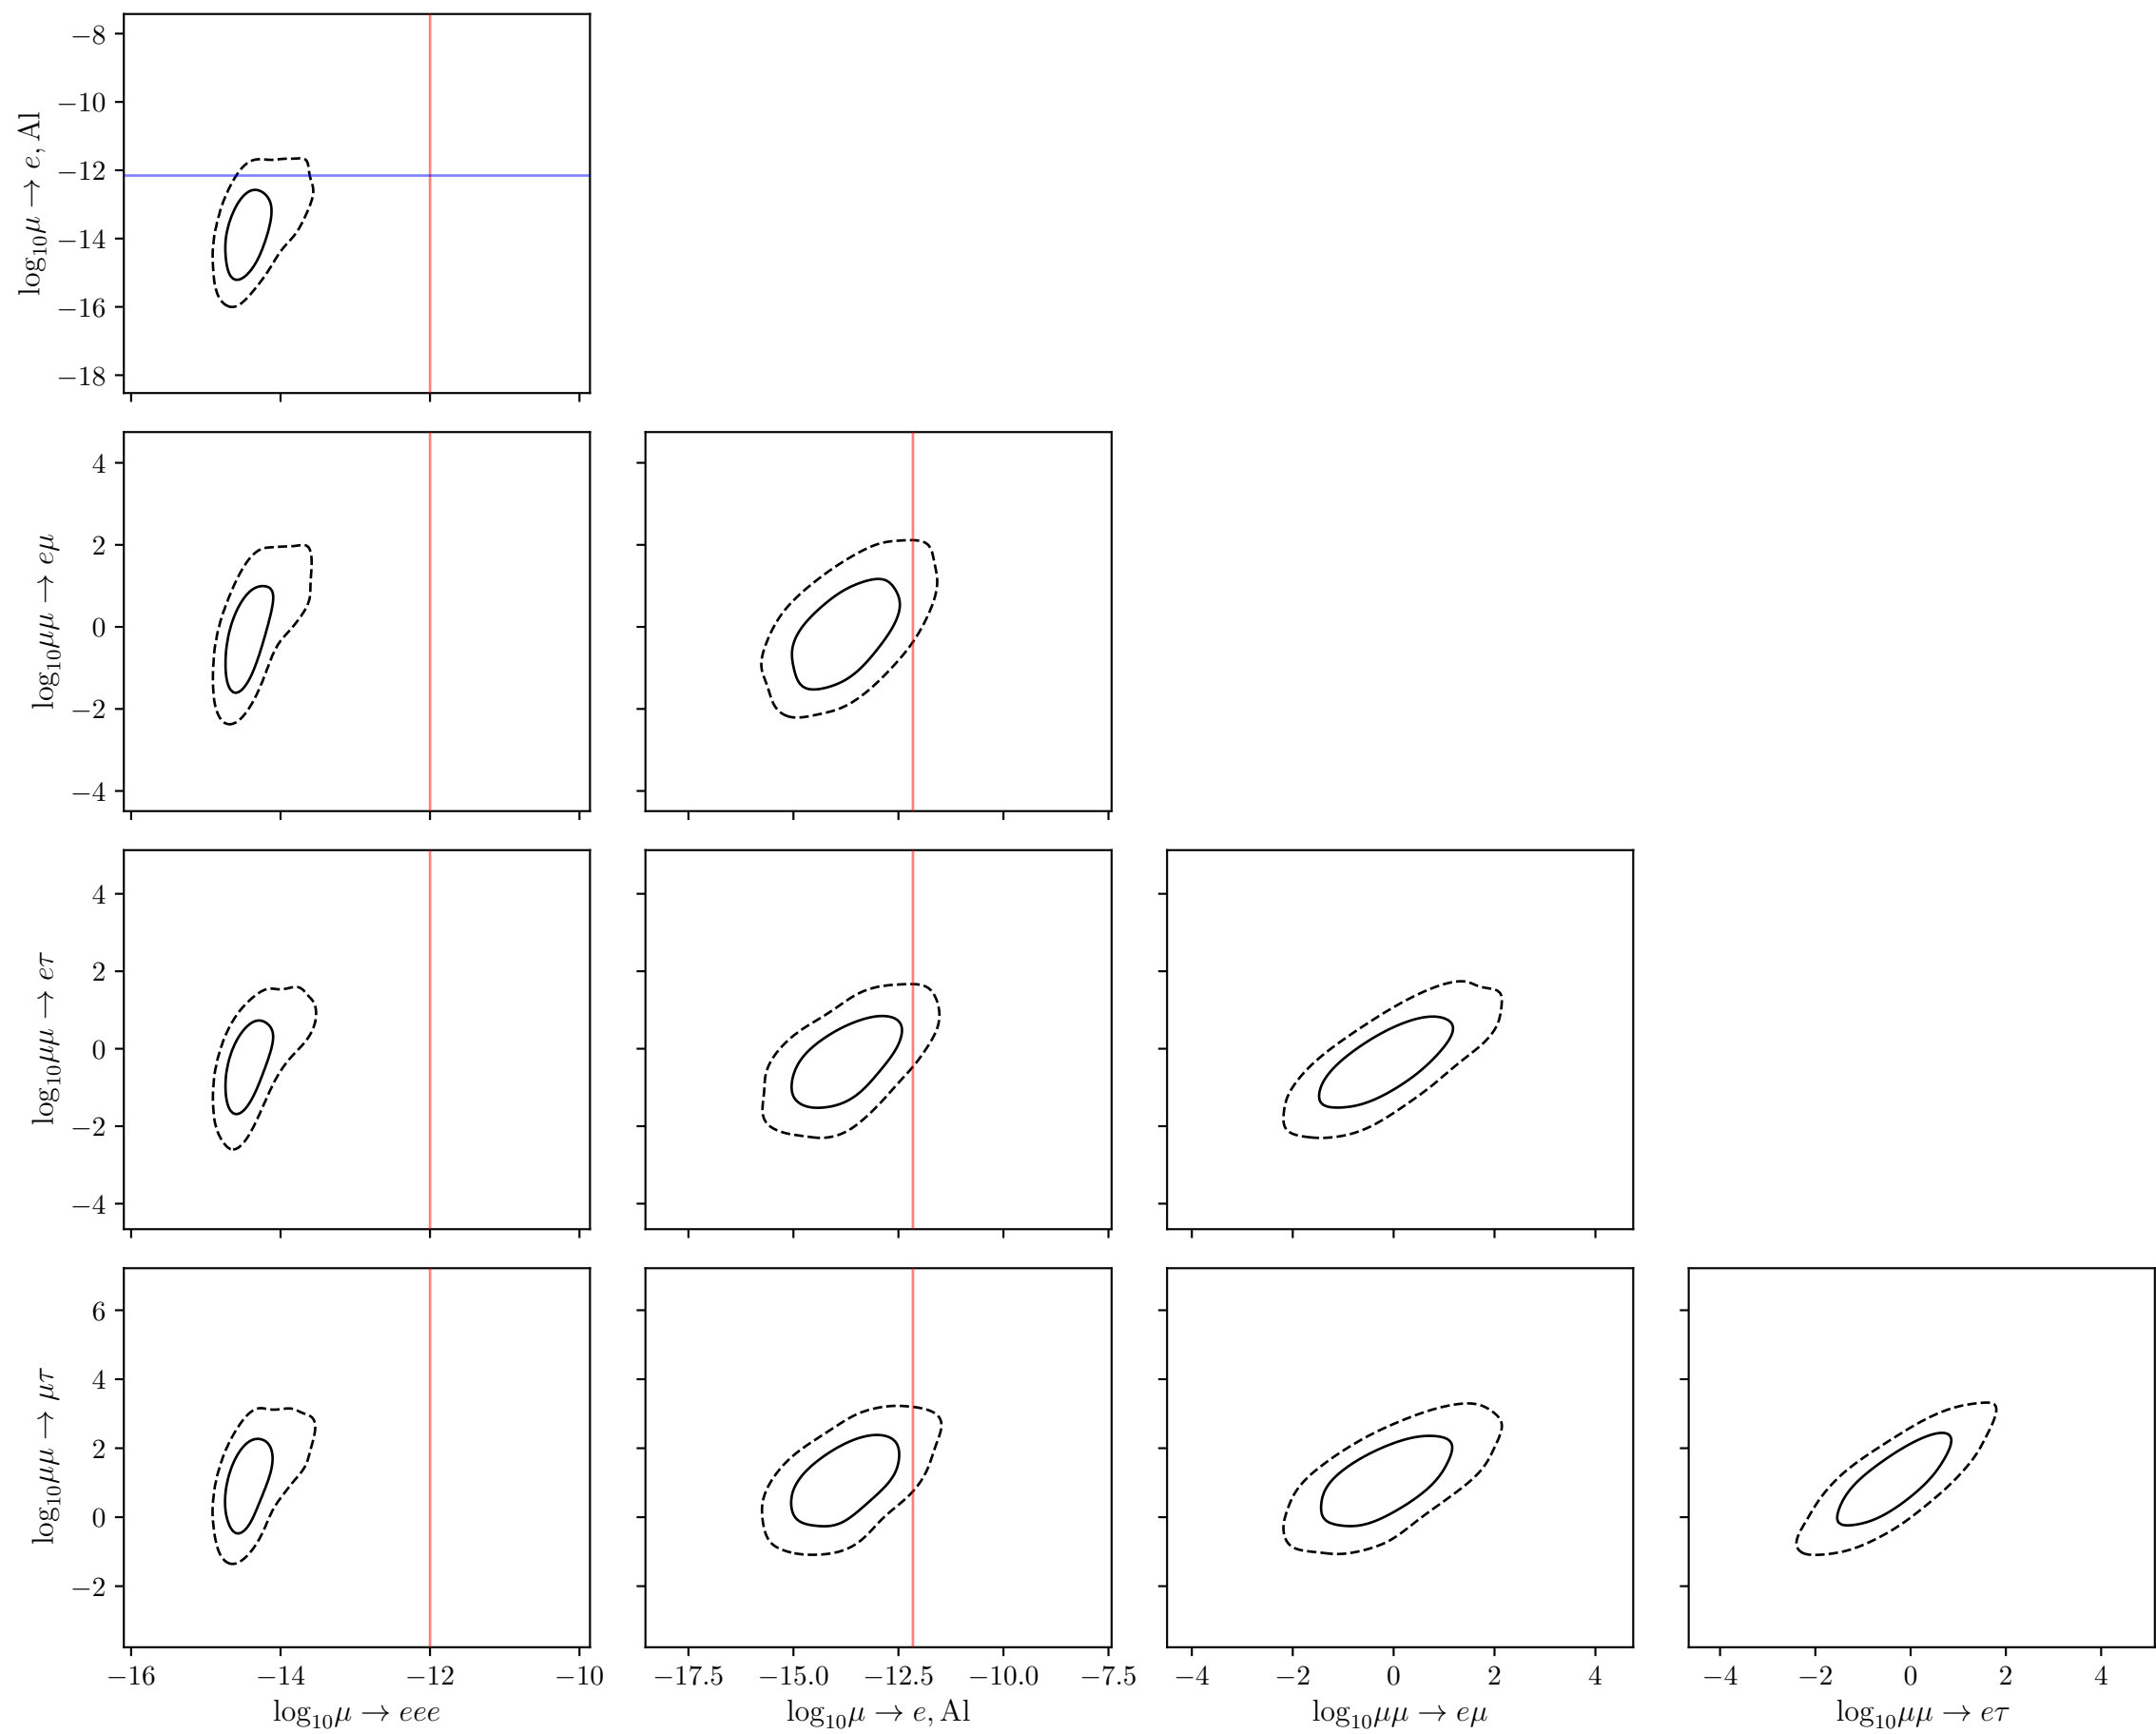

Majorana,  $X_L = \{2, 2, 1\}$ ,  $X_e = \{7, 4, 2\}$ ,

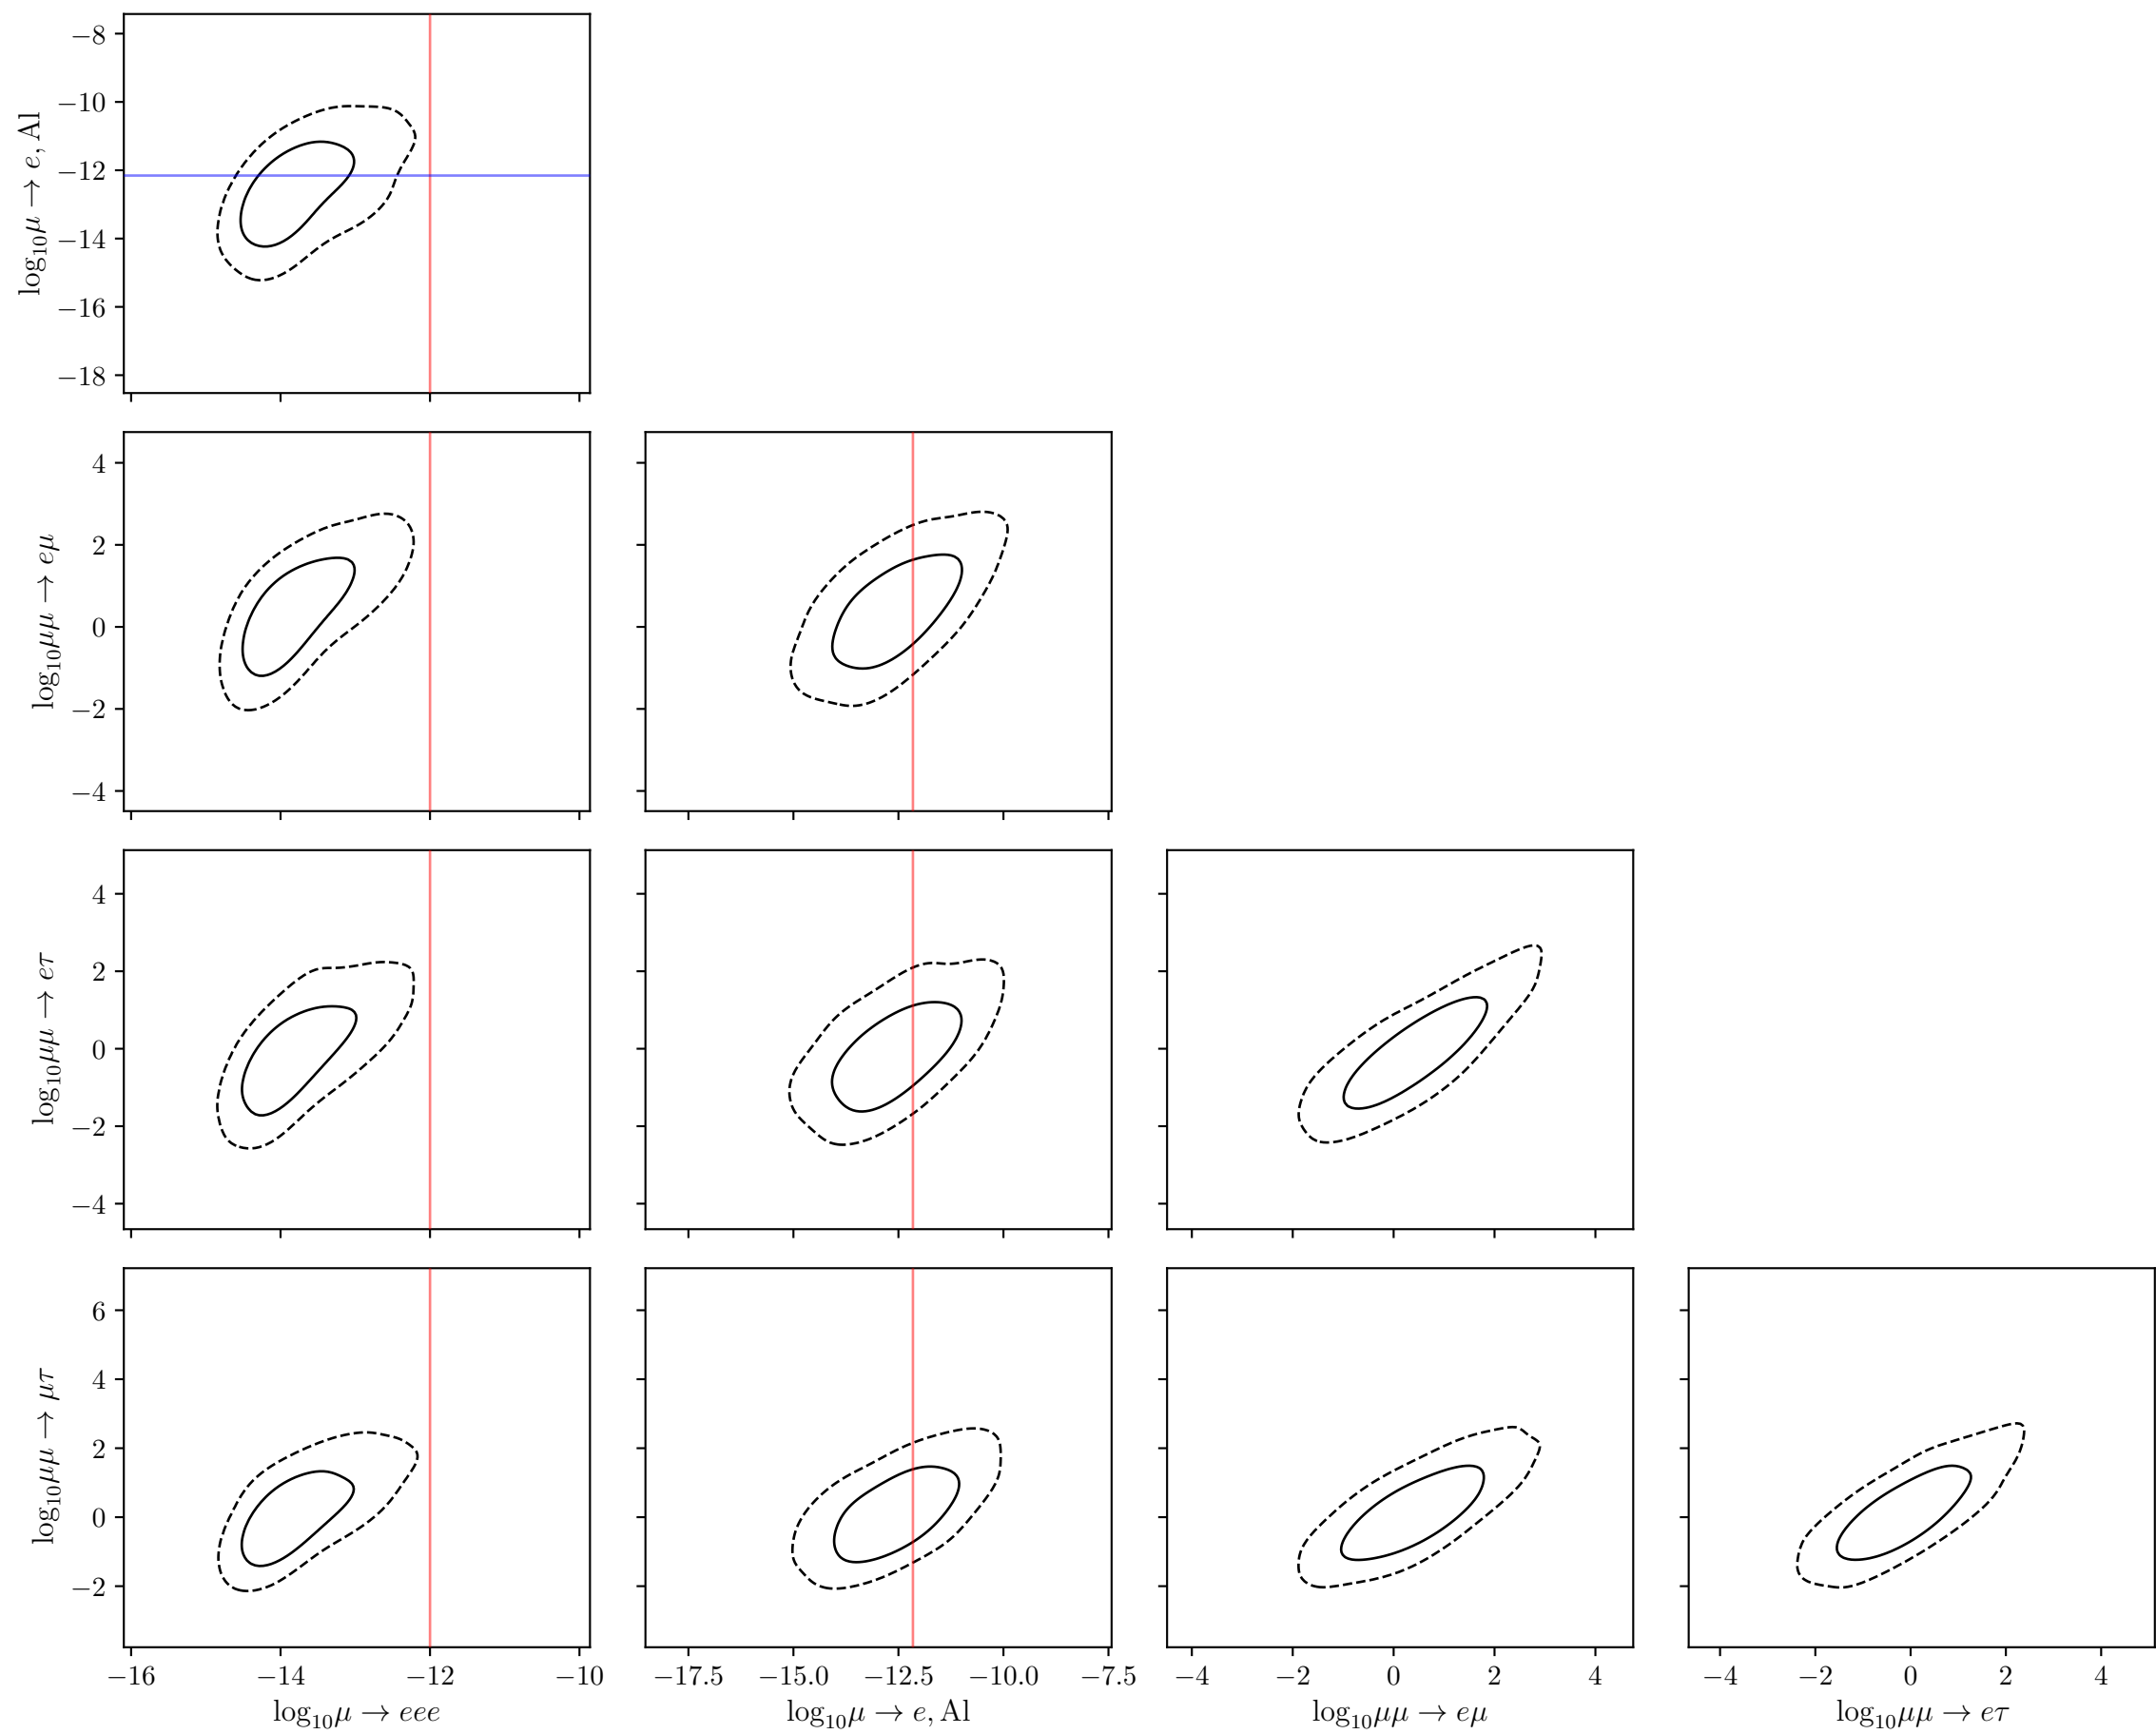

Majorana,  $X_L = \{7, 5, 5\}$ ,  $X_e = \{7, 3, 0\}$ ,

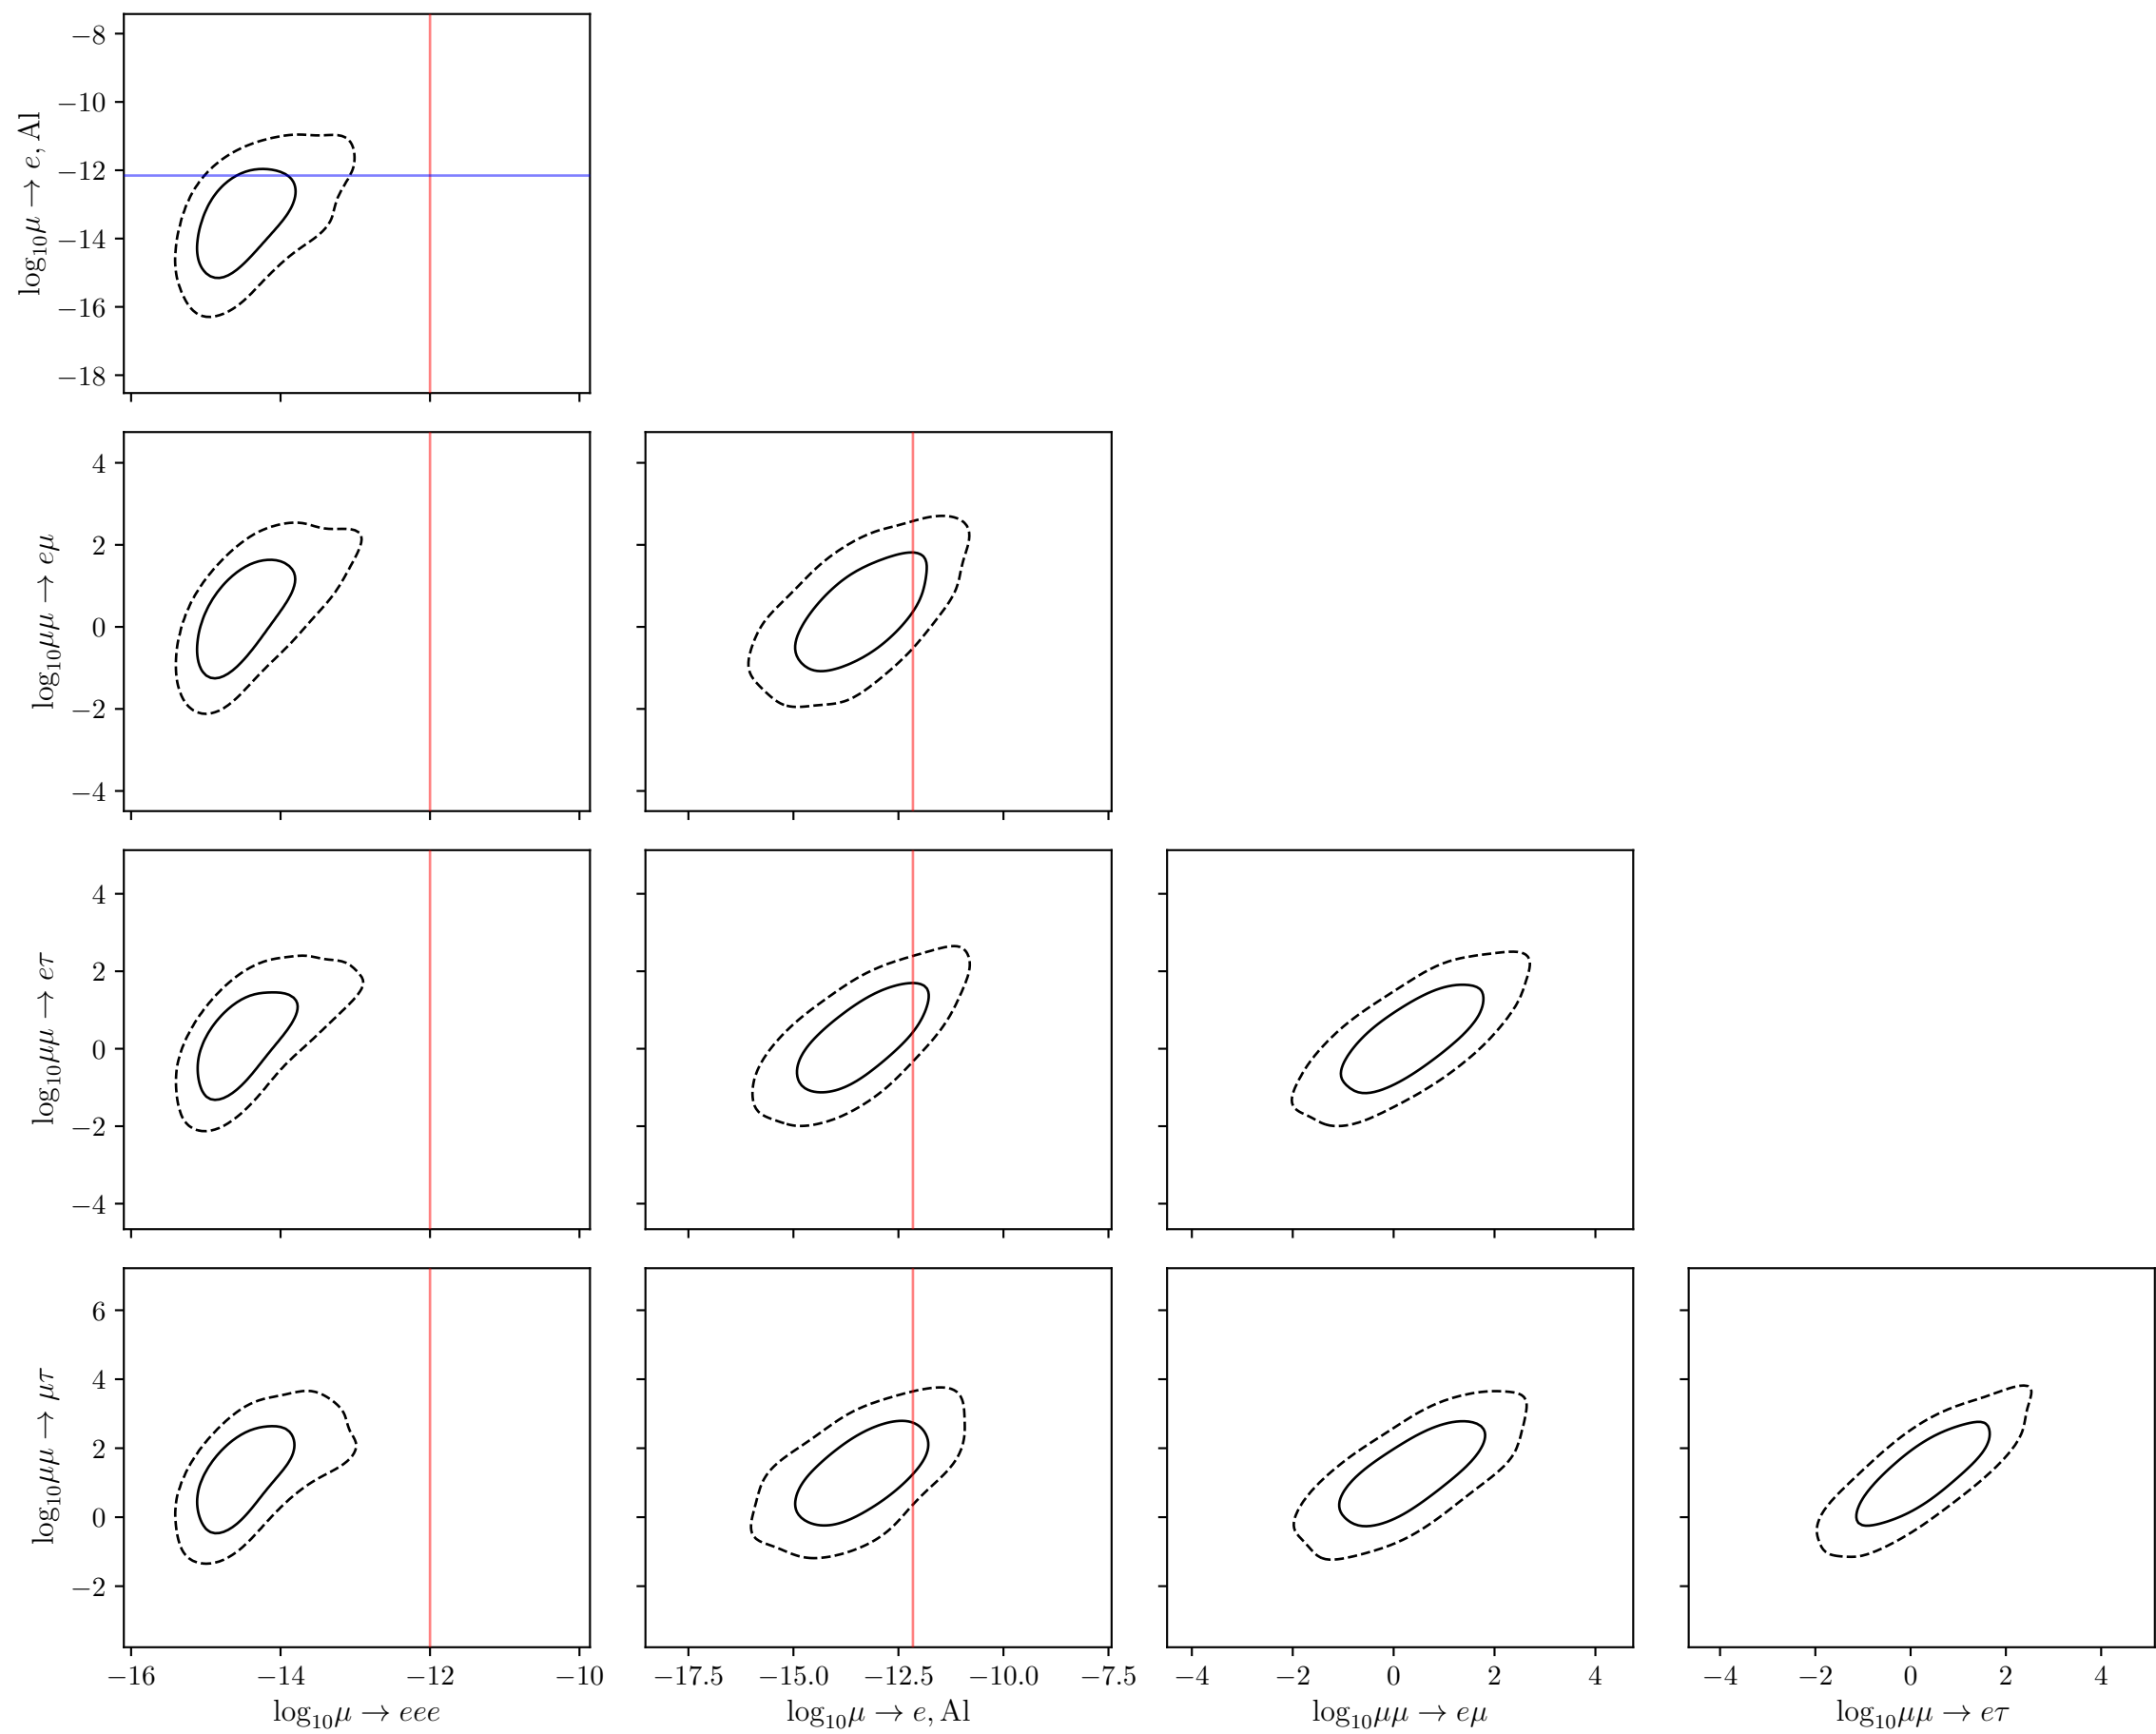

Majorana,  $X_L = \{6, 5, 4\}$ ,  $X_e = \{7, 3, 1\}$ ,

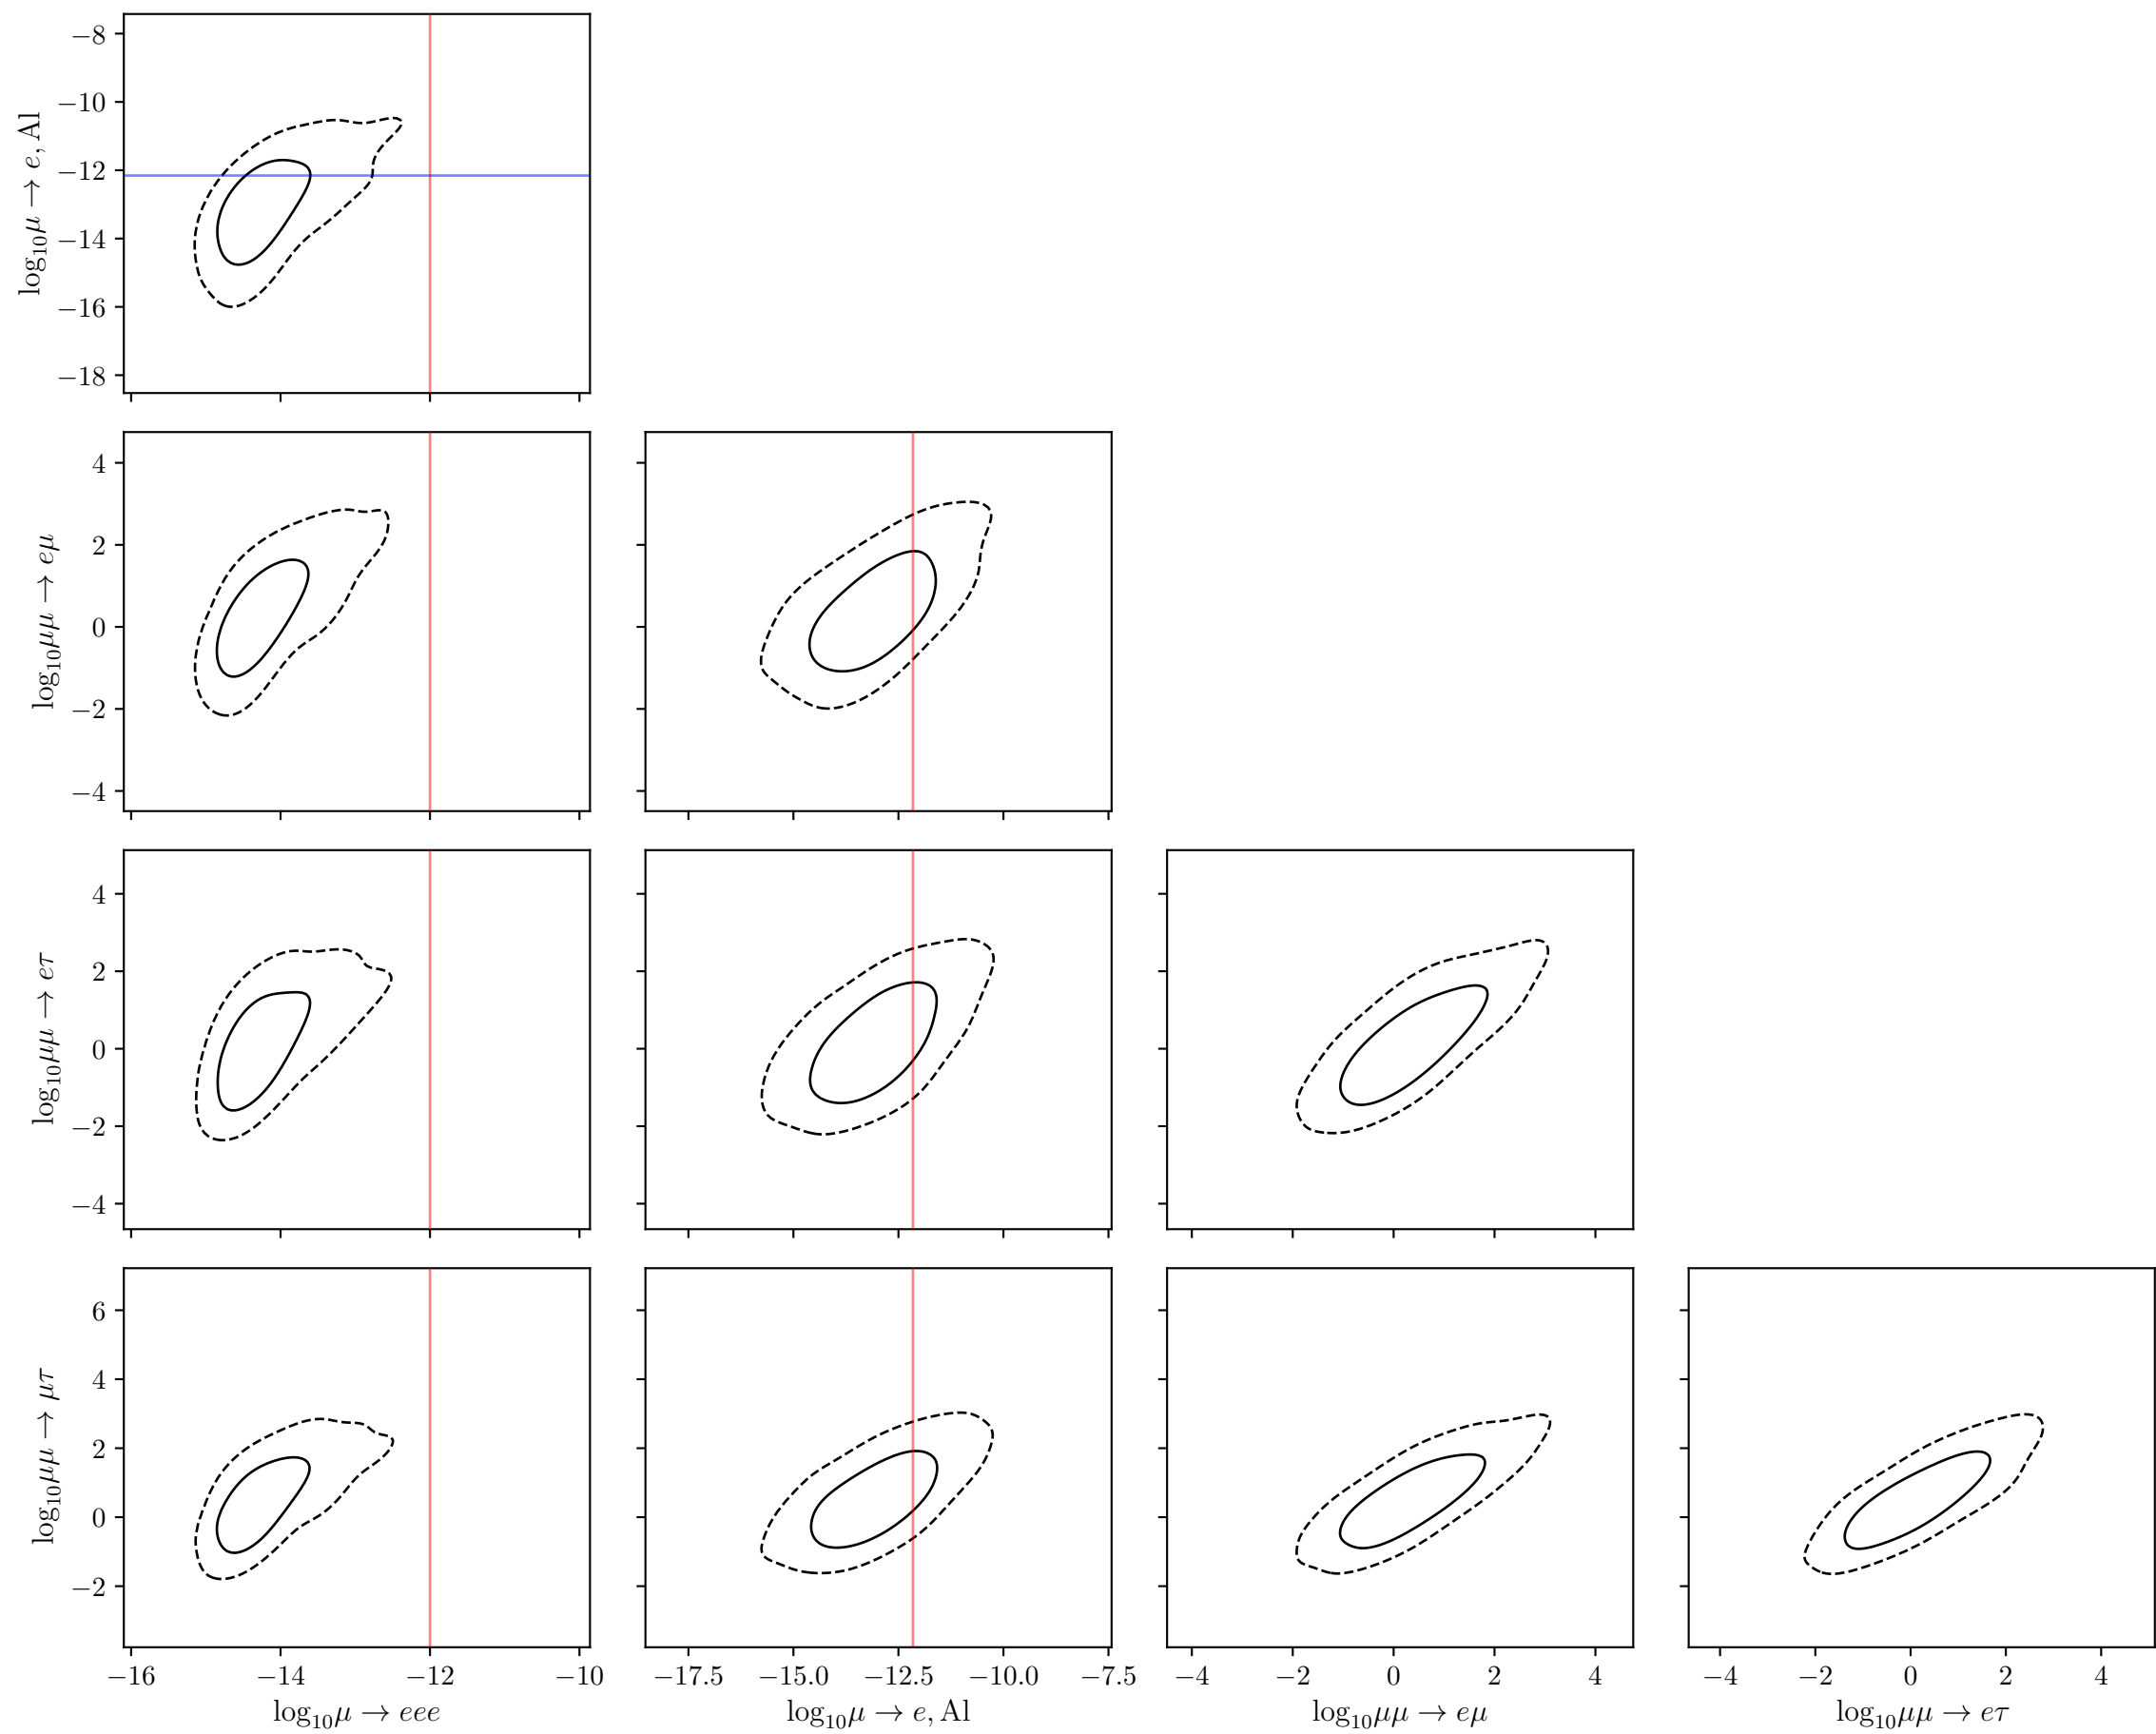

Majorana,  $X_L = \{6, 5, 4\}$ ,  $X_e = \{6, 3, 0\}$ ,

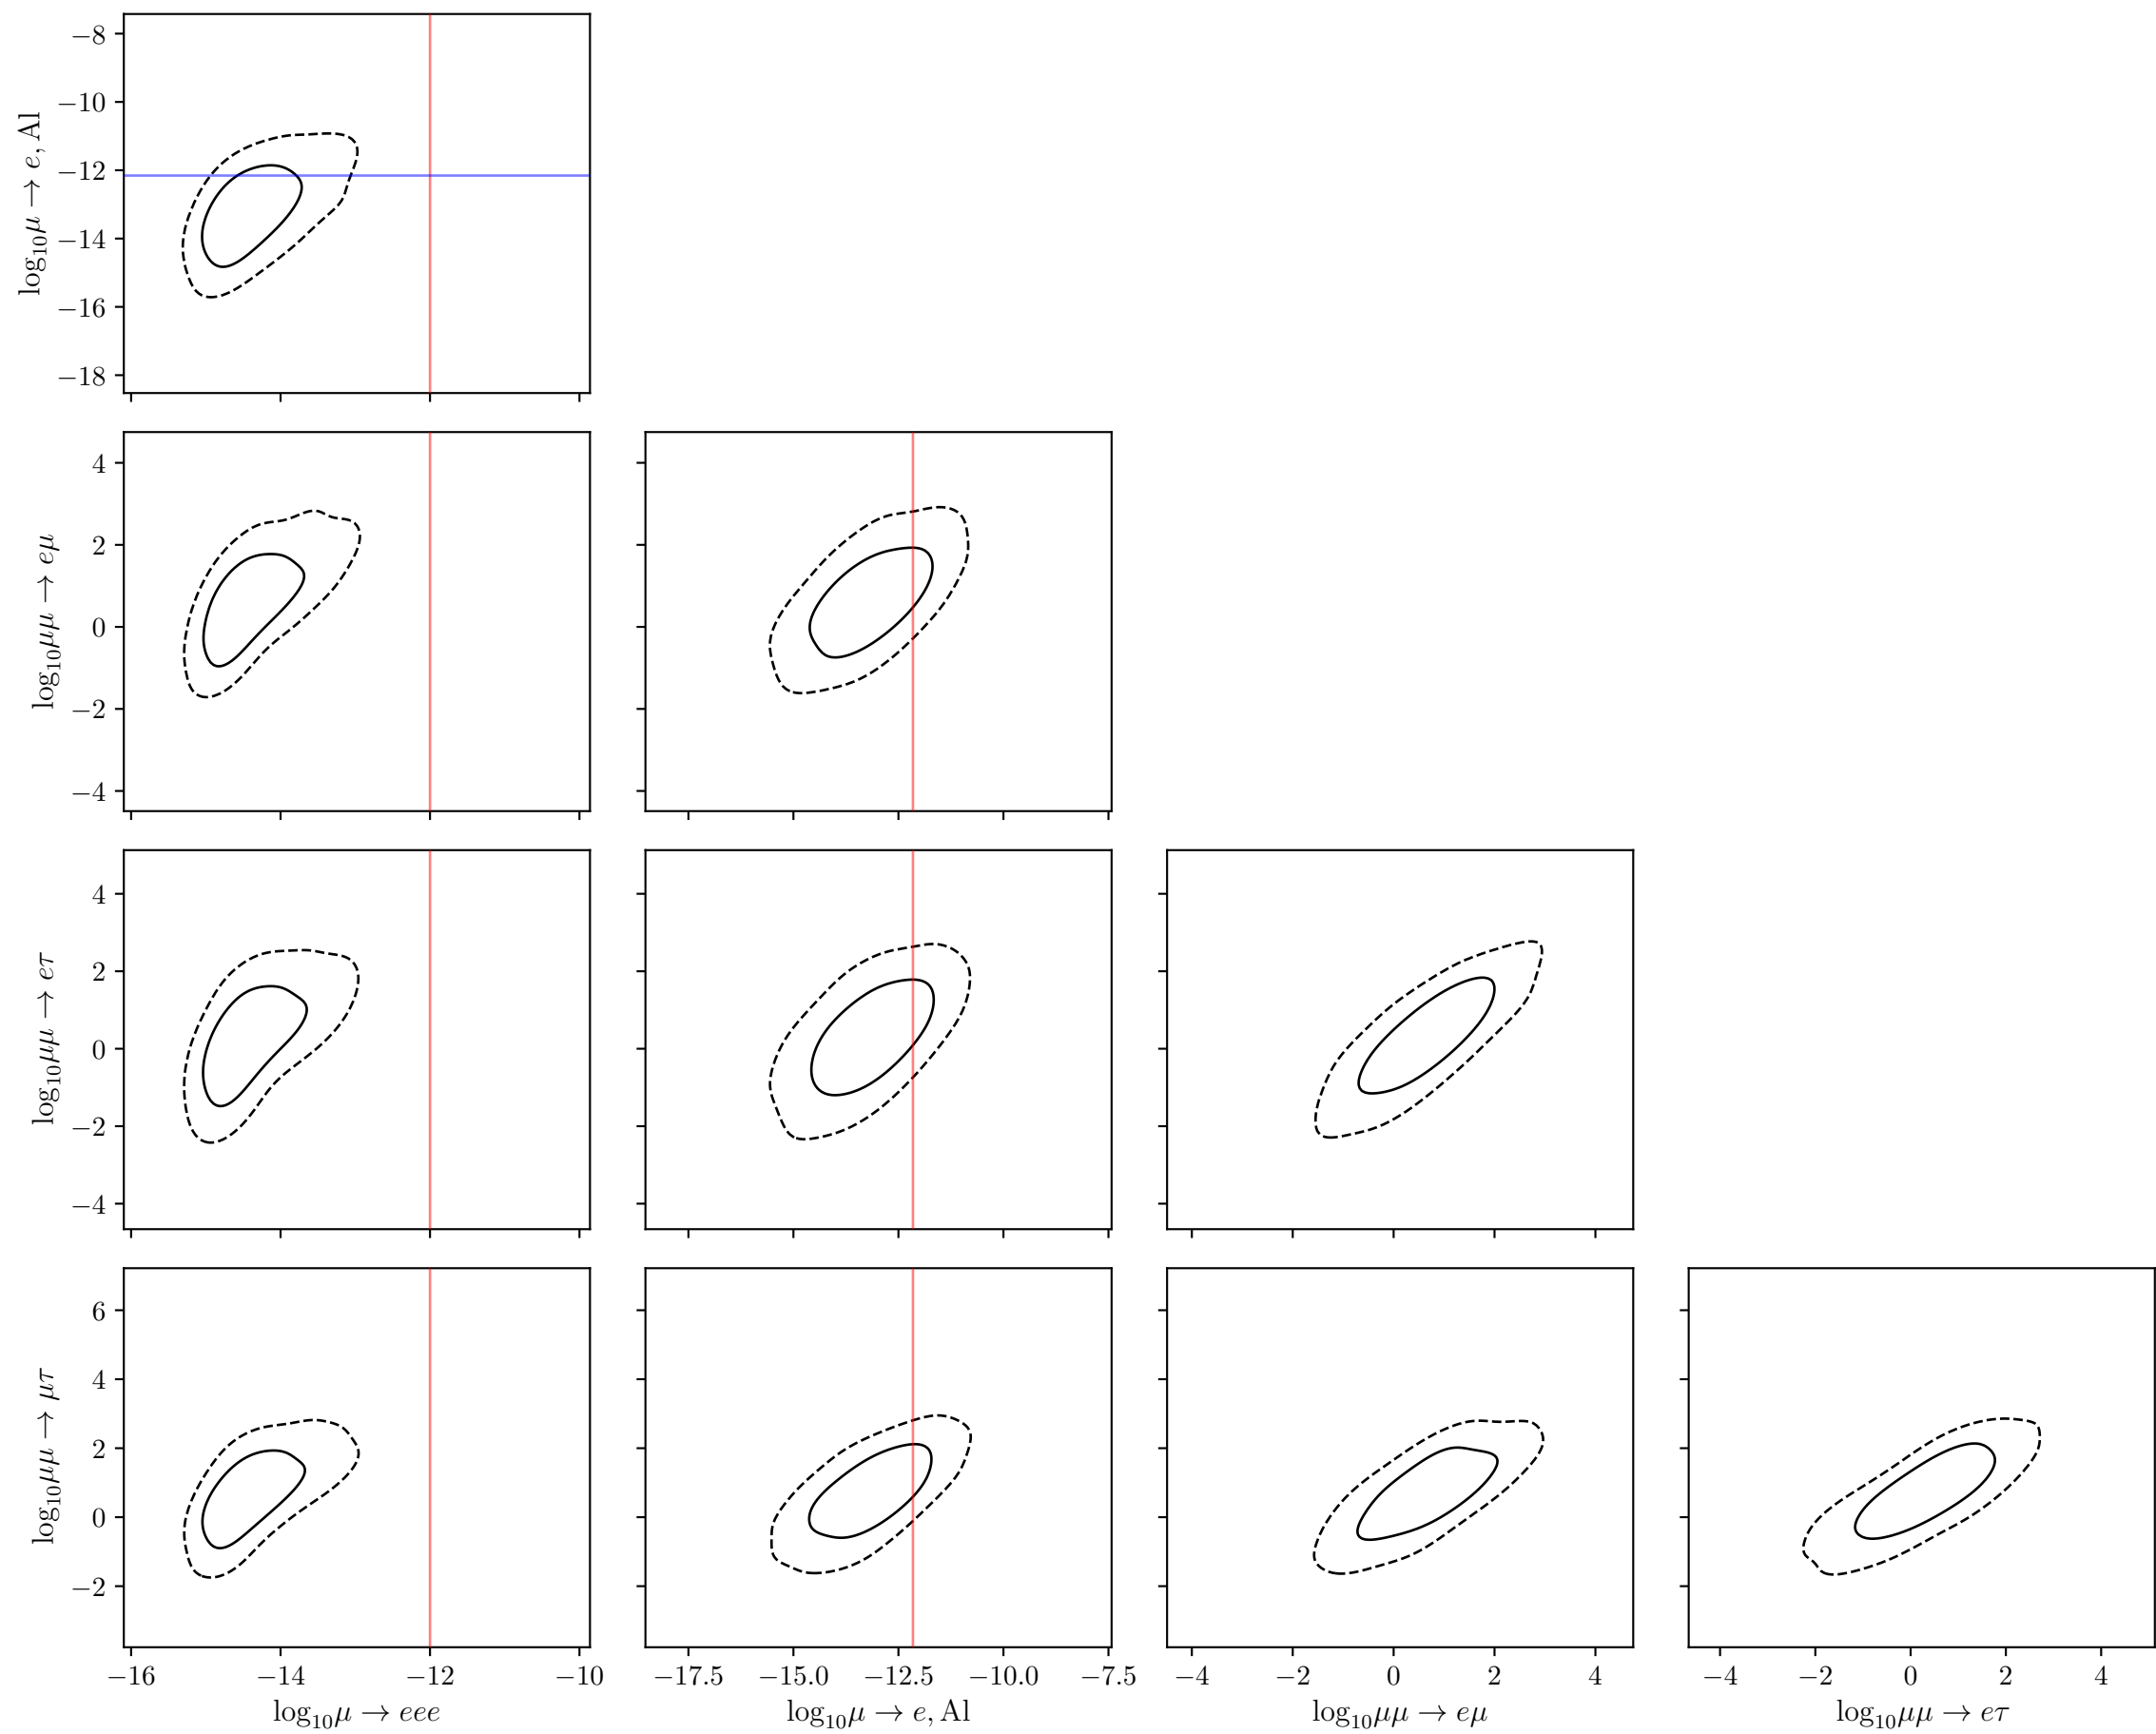

Majorana,  $X_L = \{3, 3, 2\}$ ,  $X_e = \{6, 3, 1\}$ ,

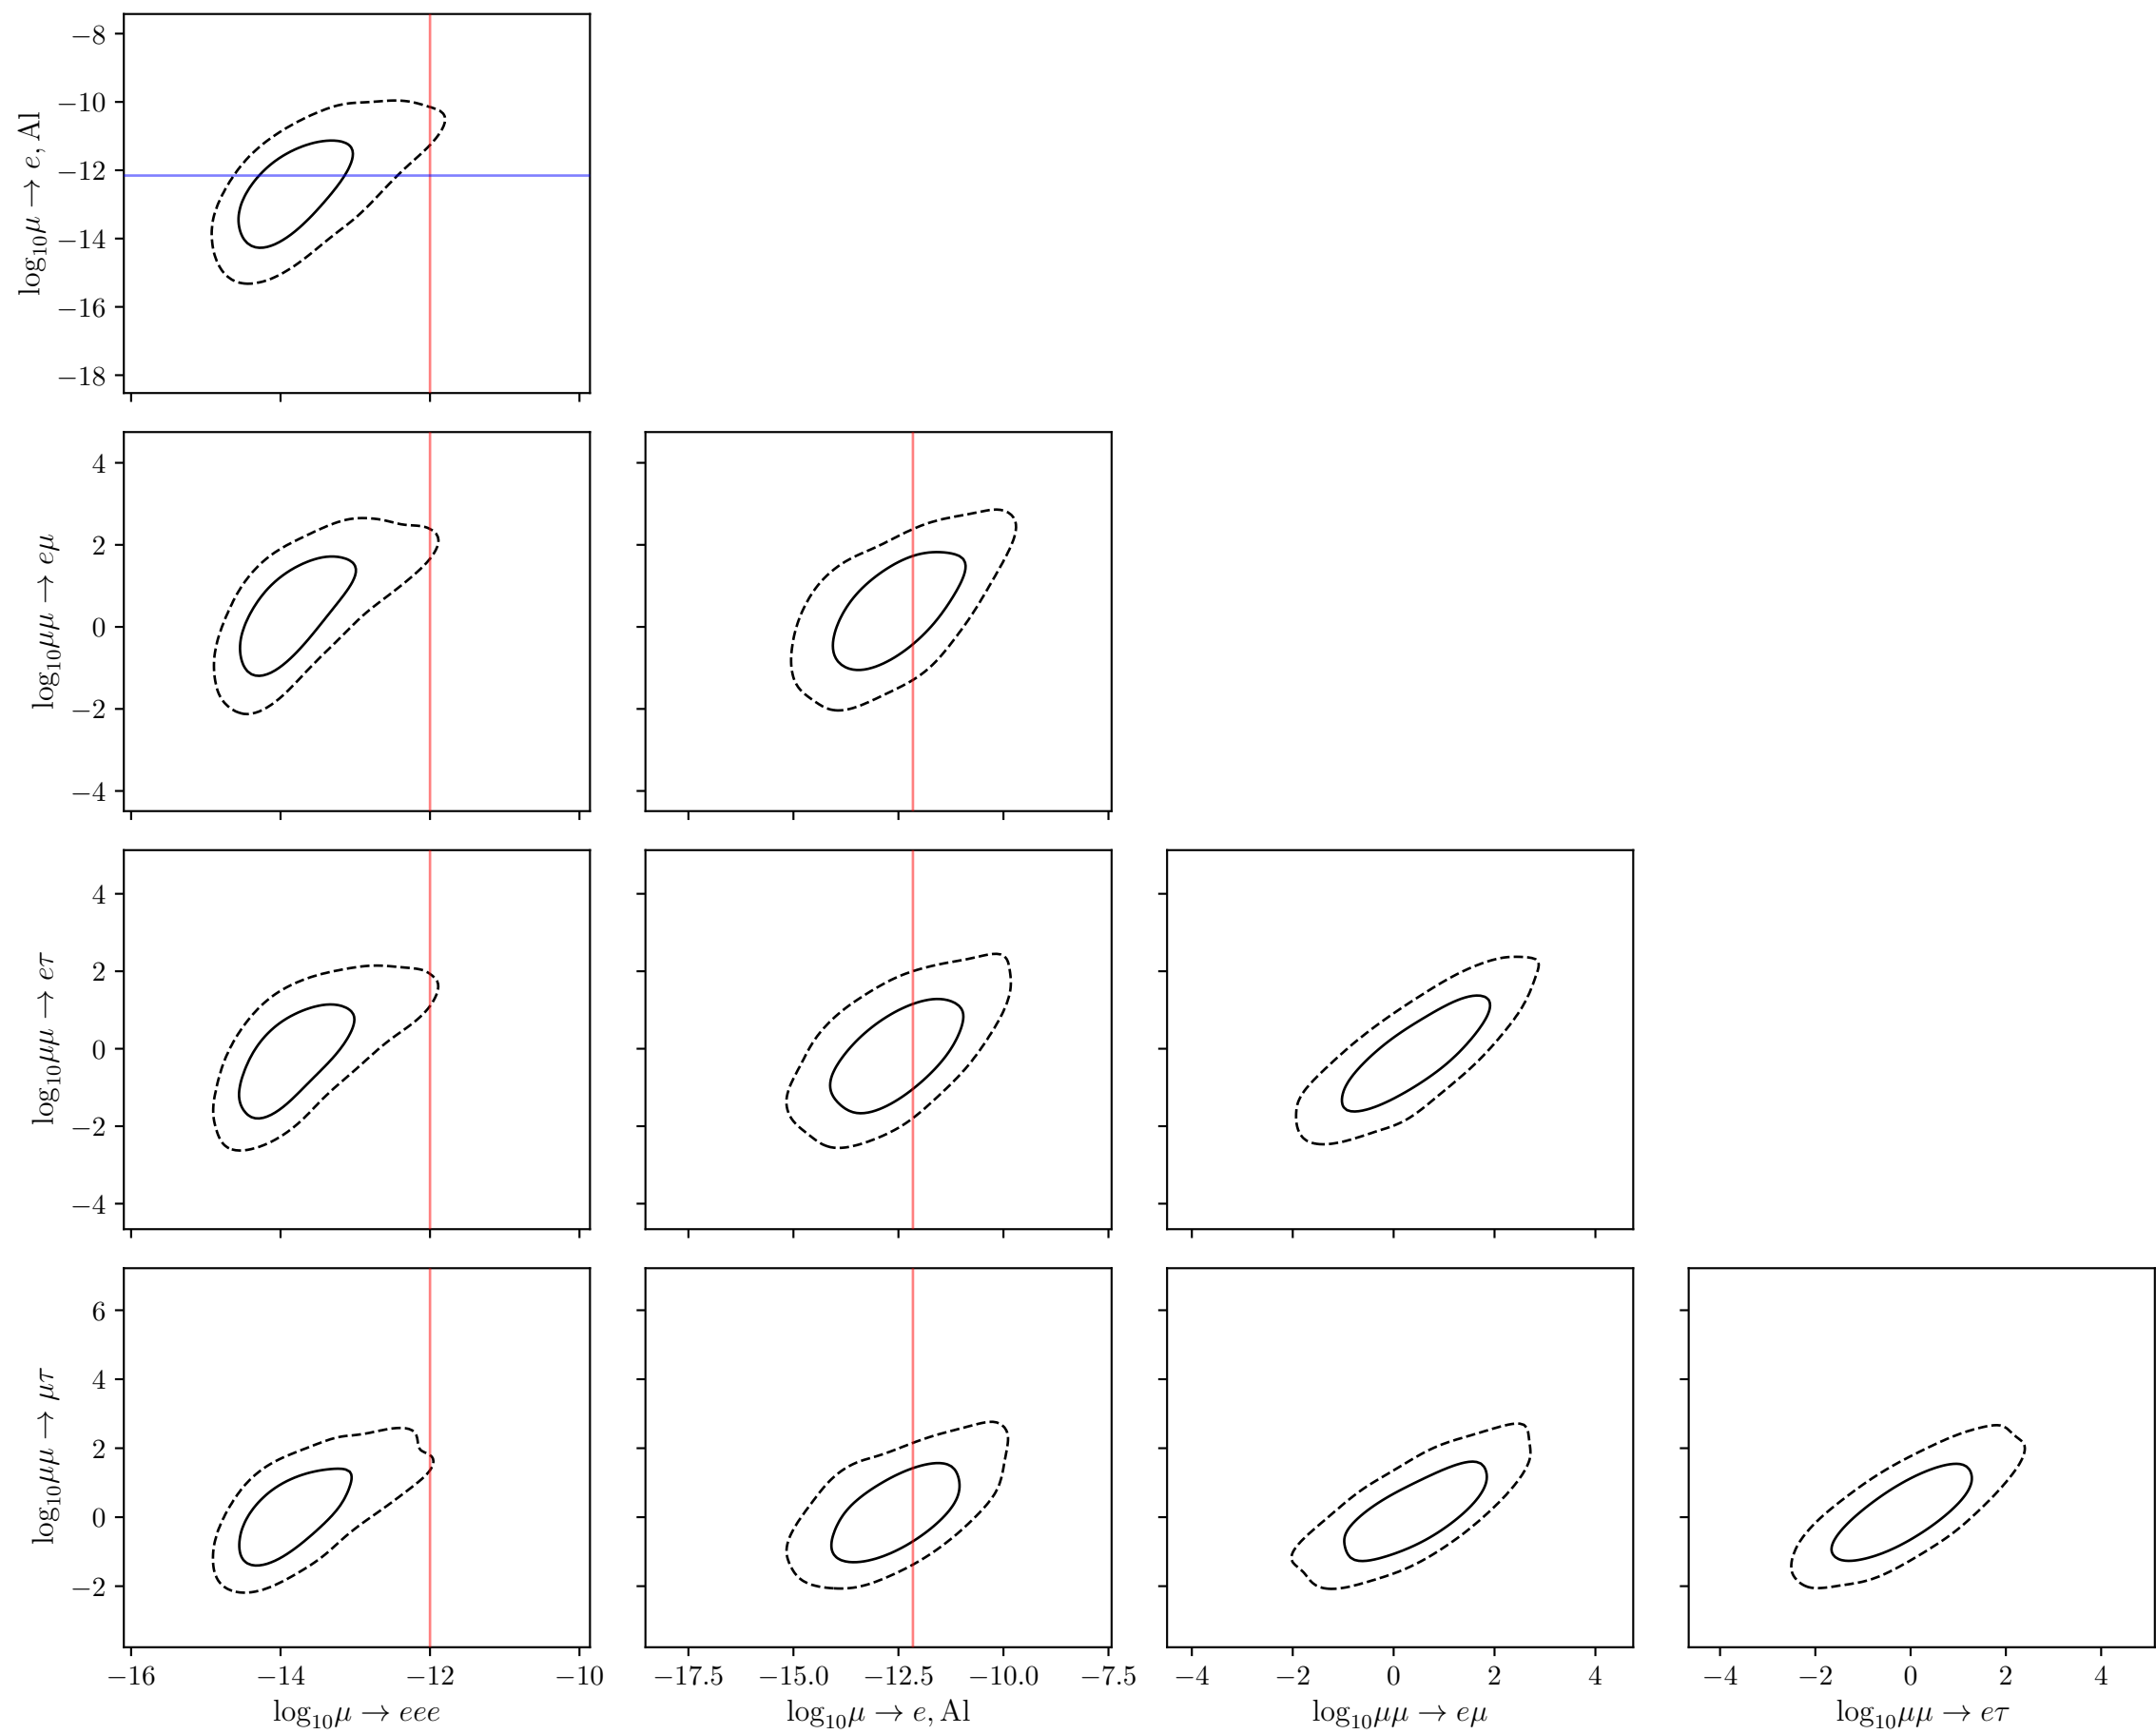

Majorana,  $X_L = \{5, 5, 4\}$ ,  $X_e = \{-1, 1, 4\}$ ,

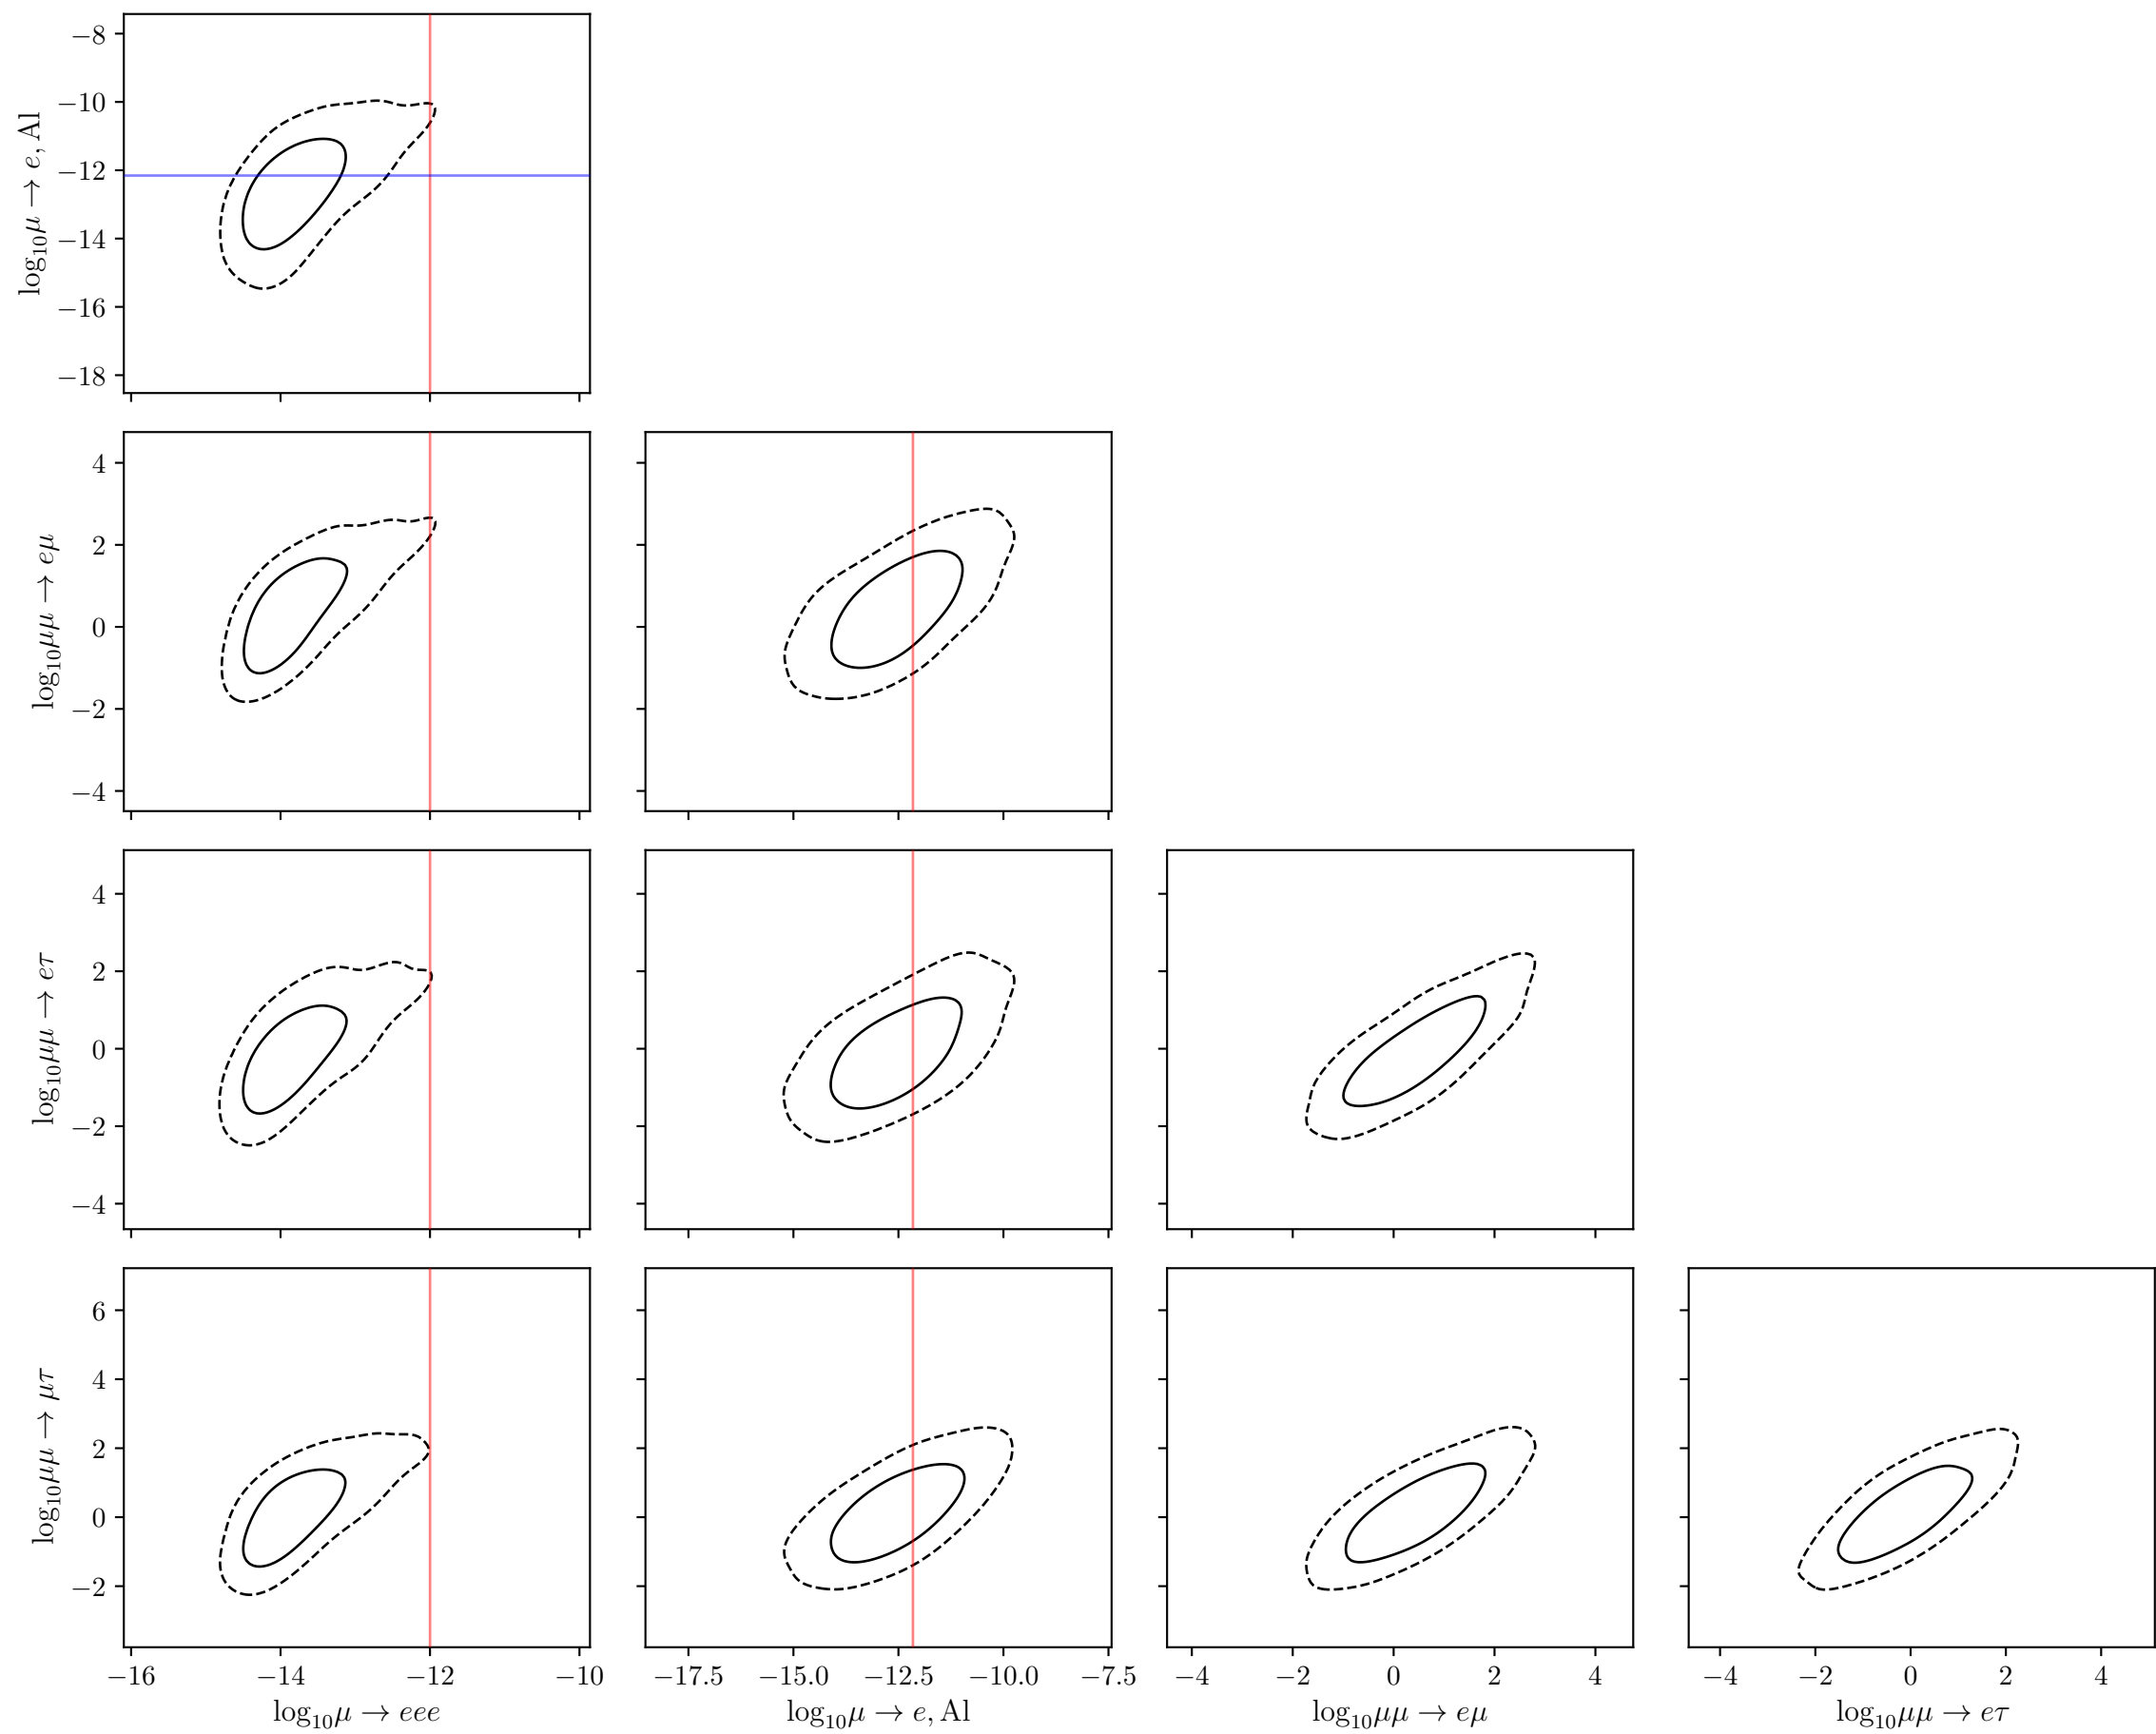



Majorana,  $X_L = \{7, 7, 6\}$ ,  $X_e = \{-1, 2, 7\}$ ,

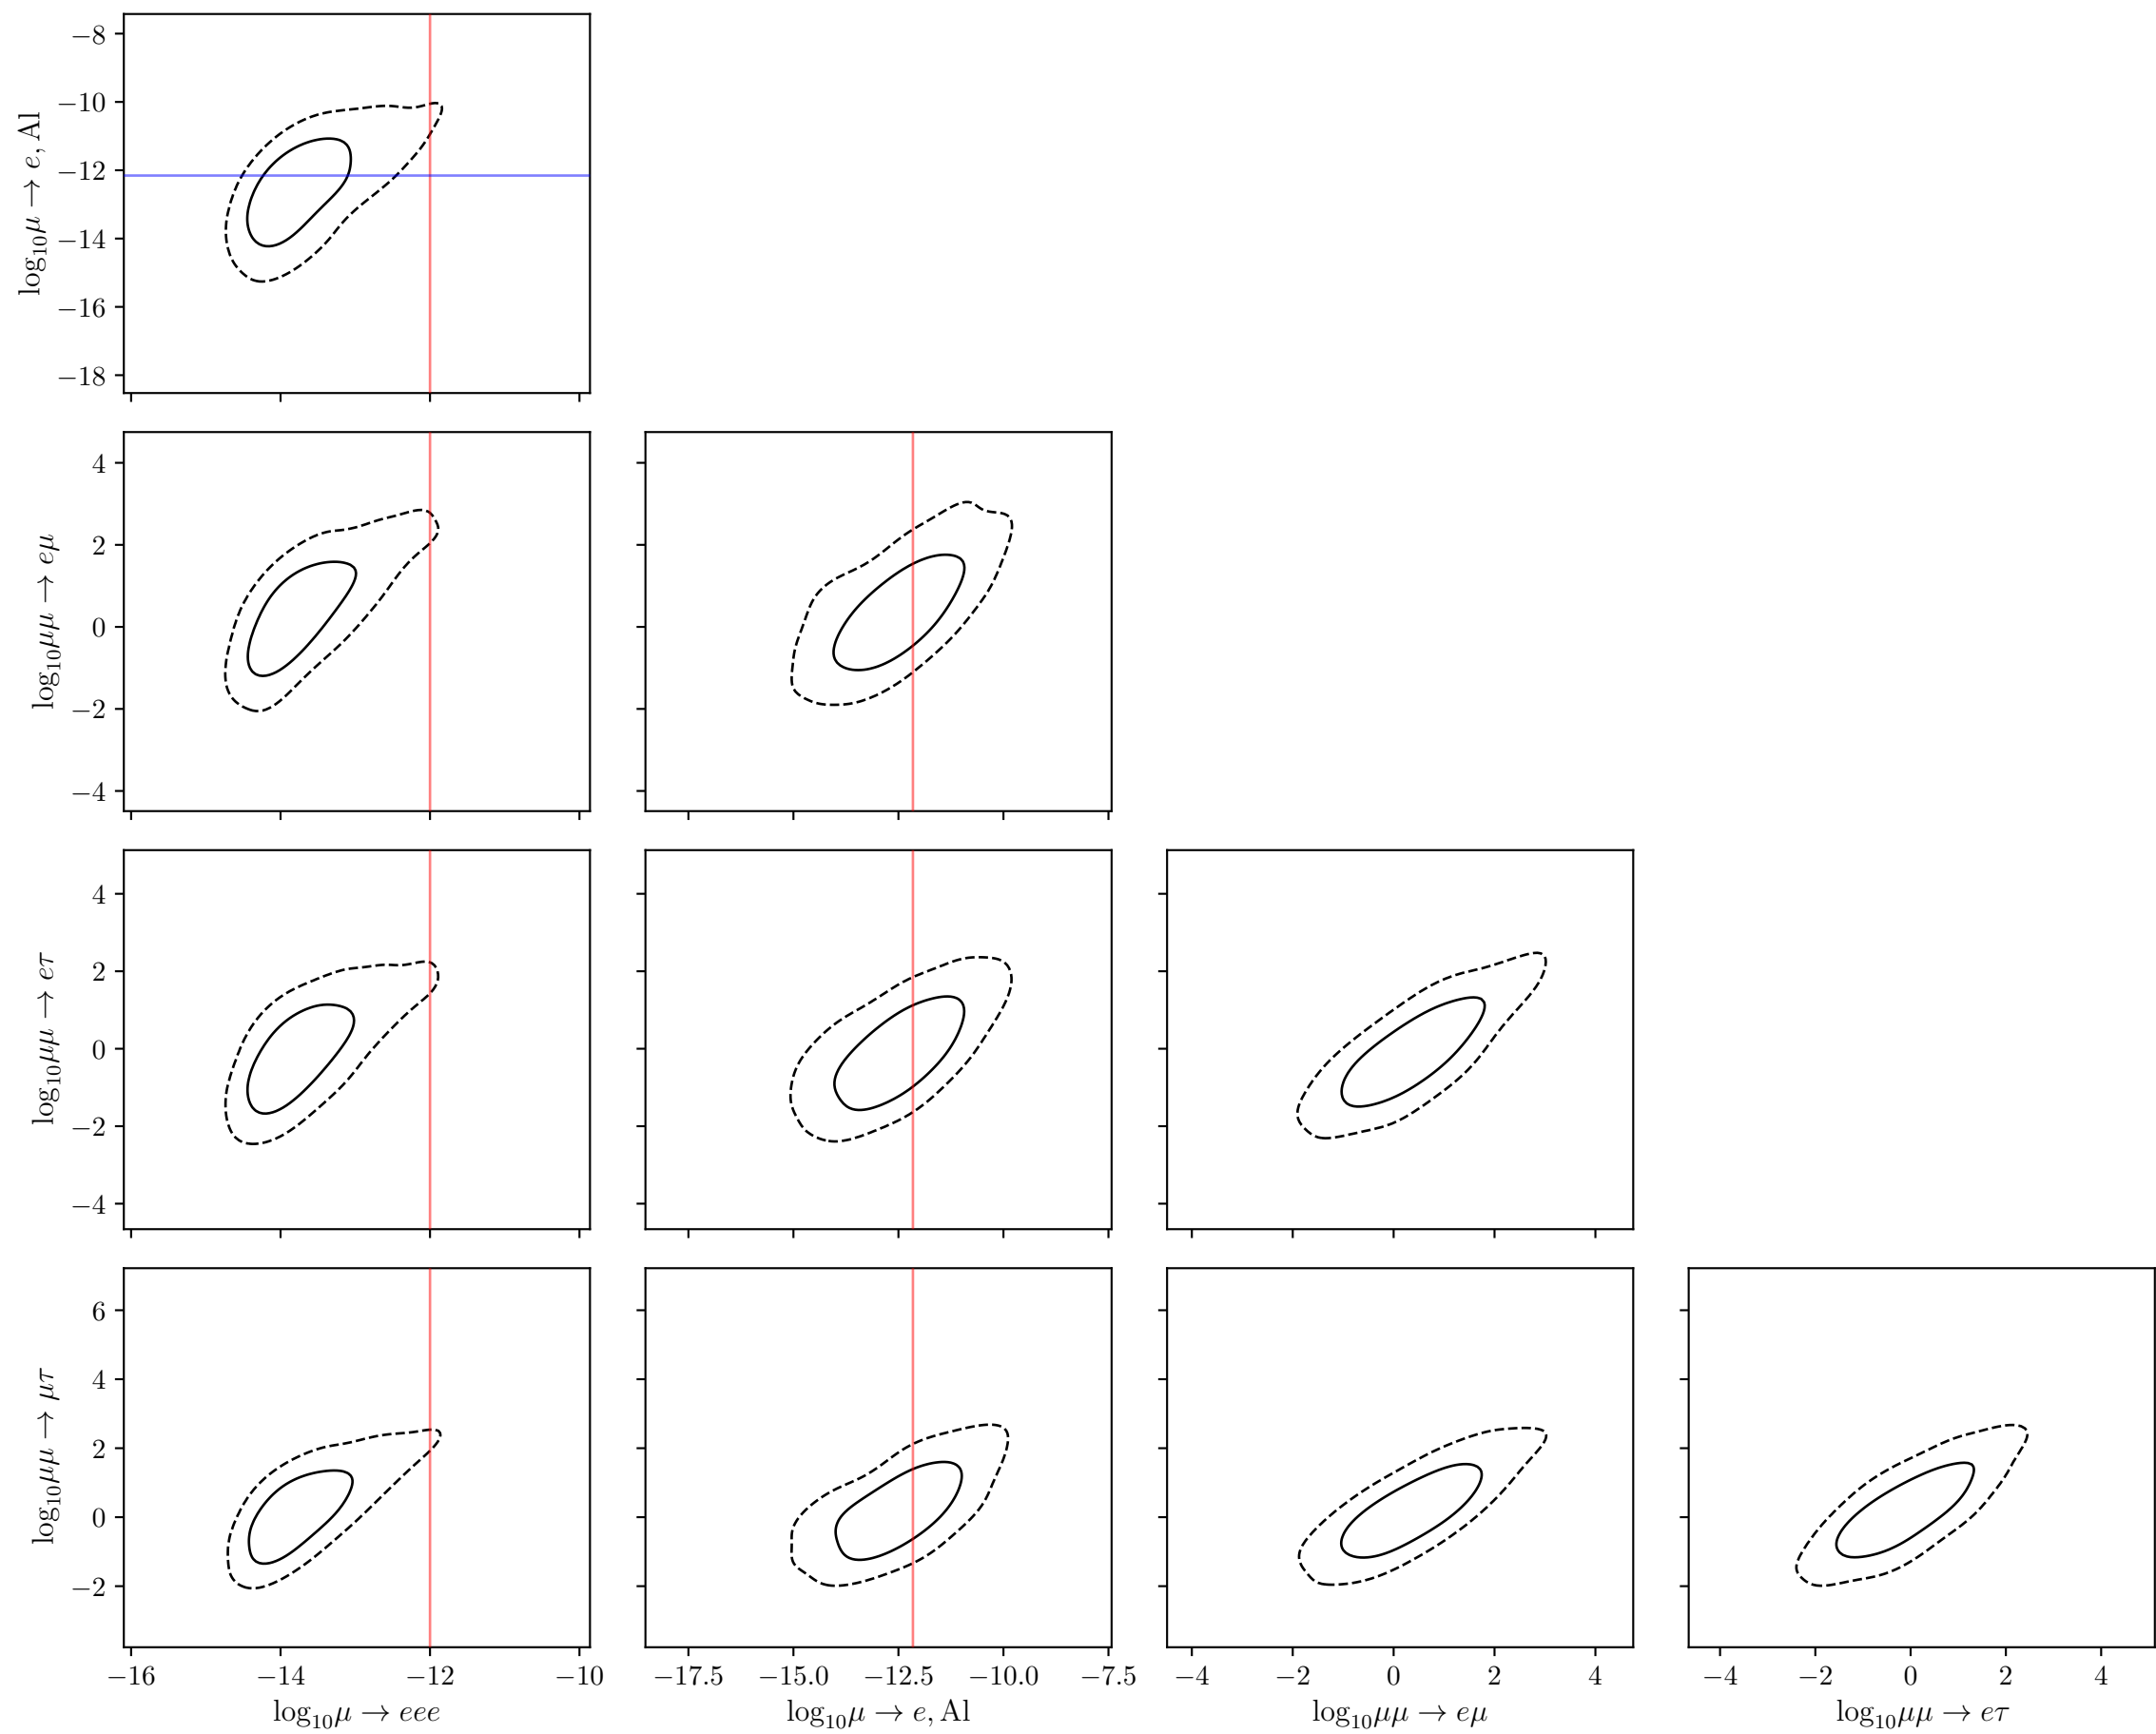

Majorana,  $X_L = \{5, 4, 3\}$ ,  $X_e = \{7, 4, 1\}$ ,

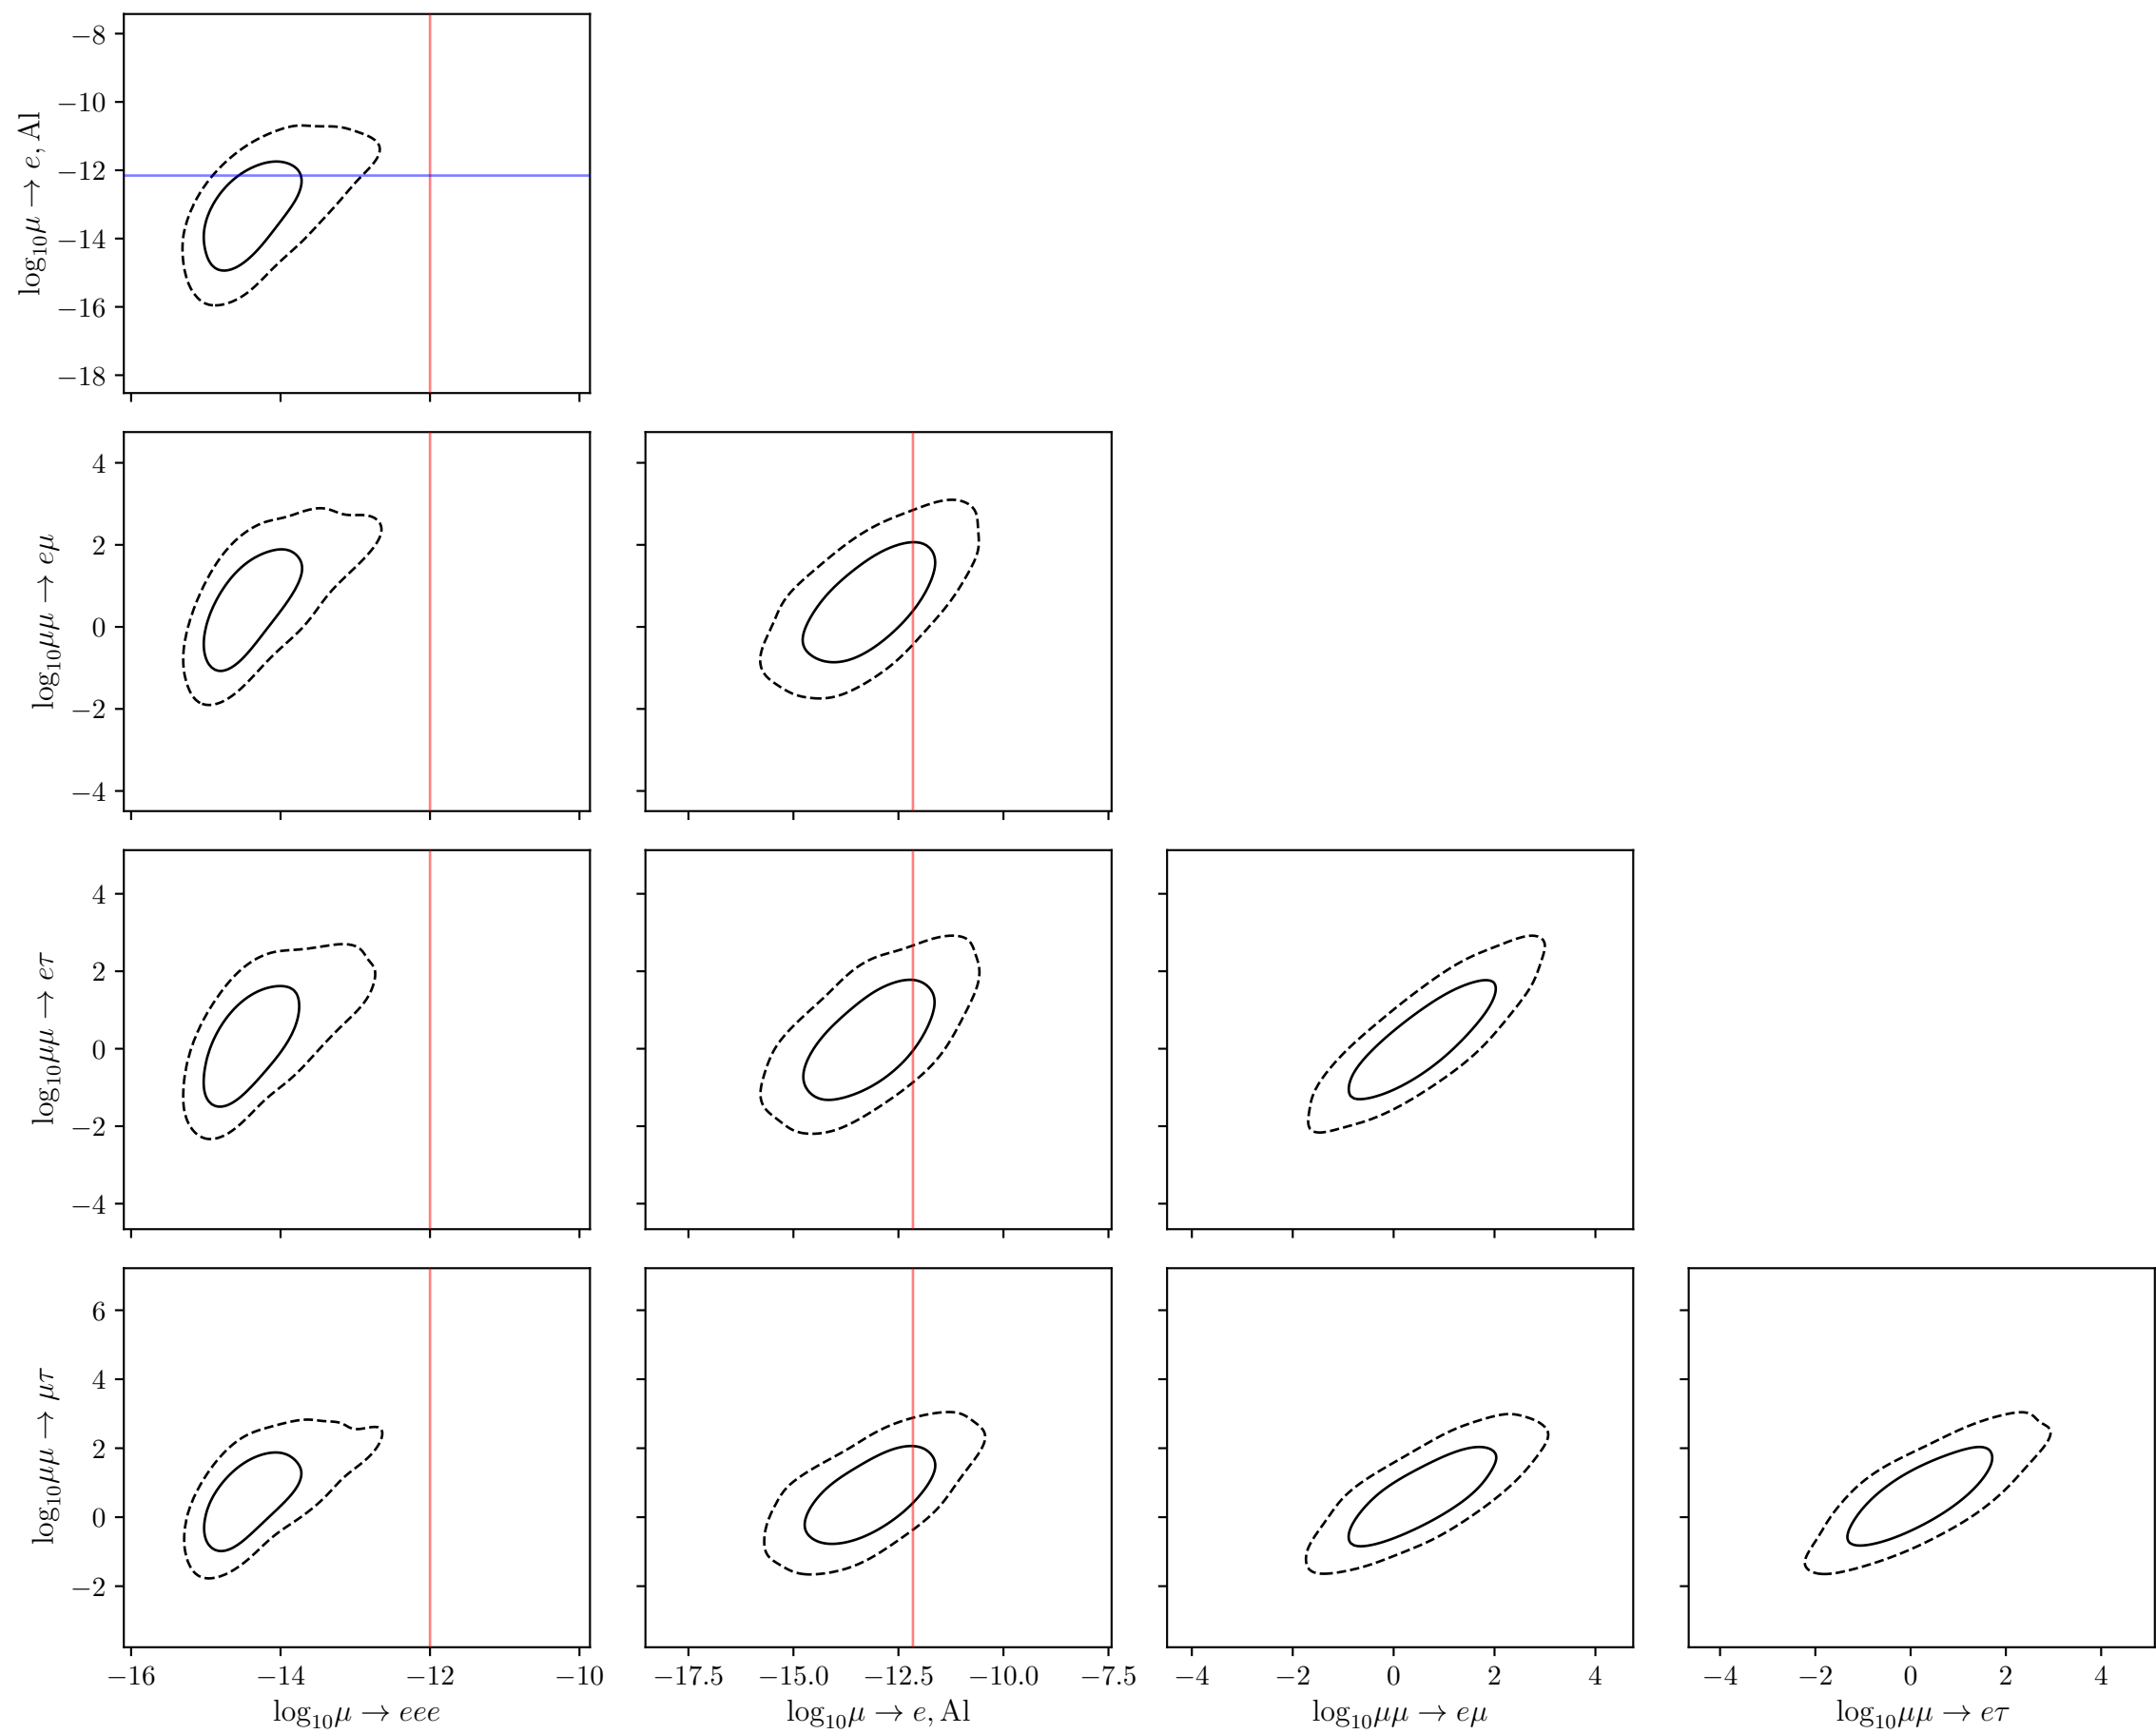

Majorana,  $X_L = \{7, 6, 5\}$ ,  $X_e = \{7, 2, 0\}$ ,

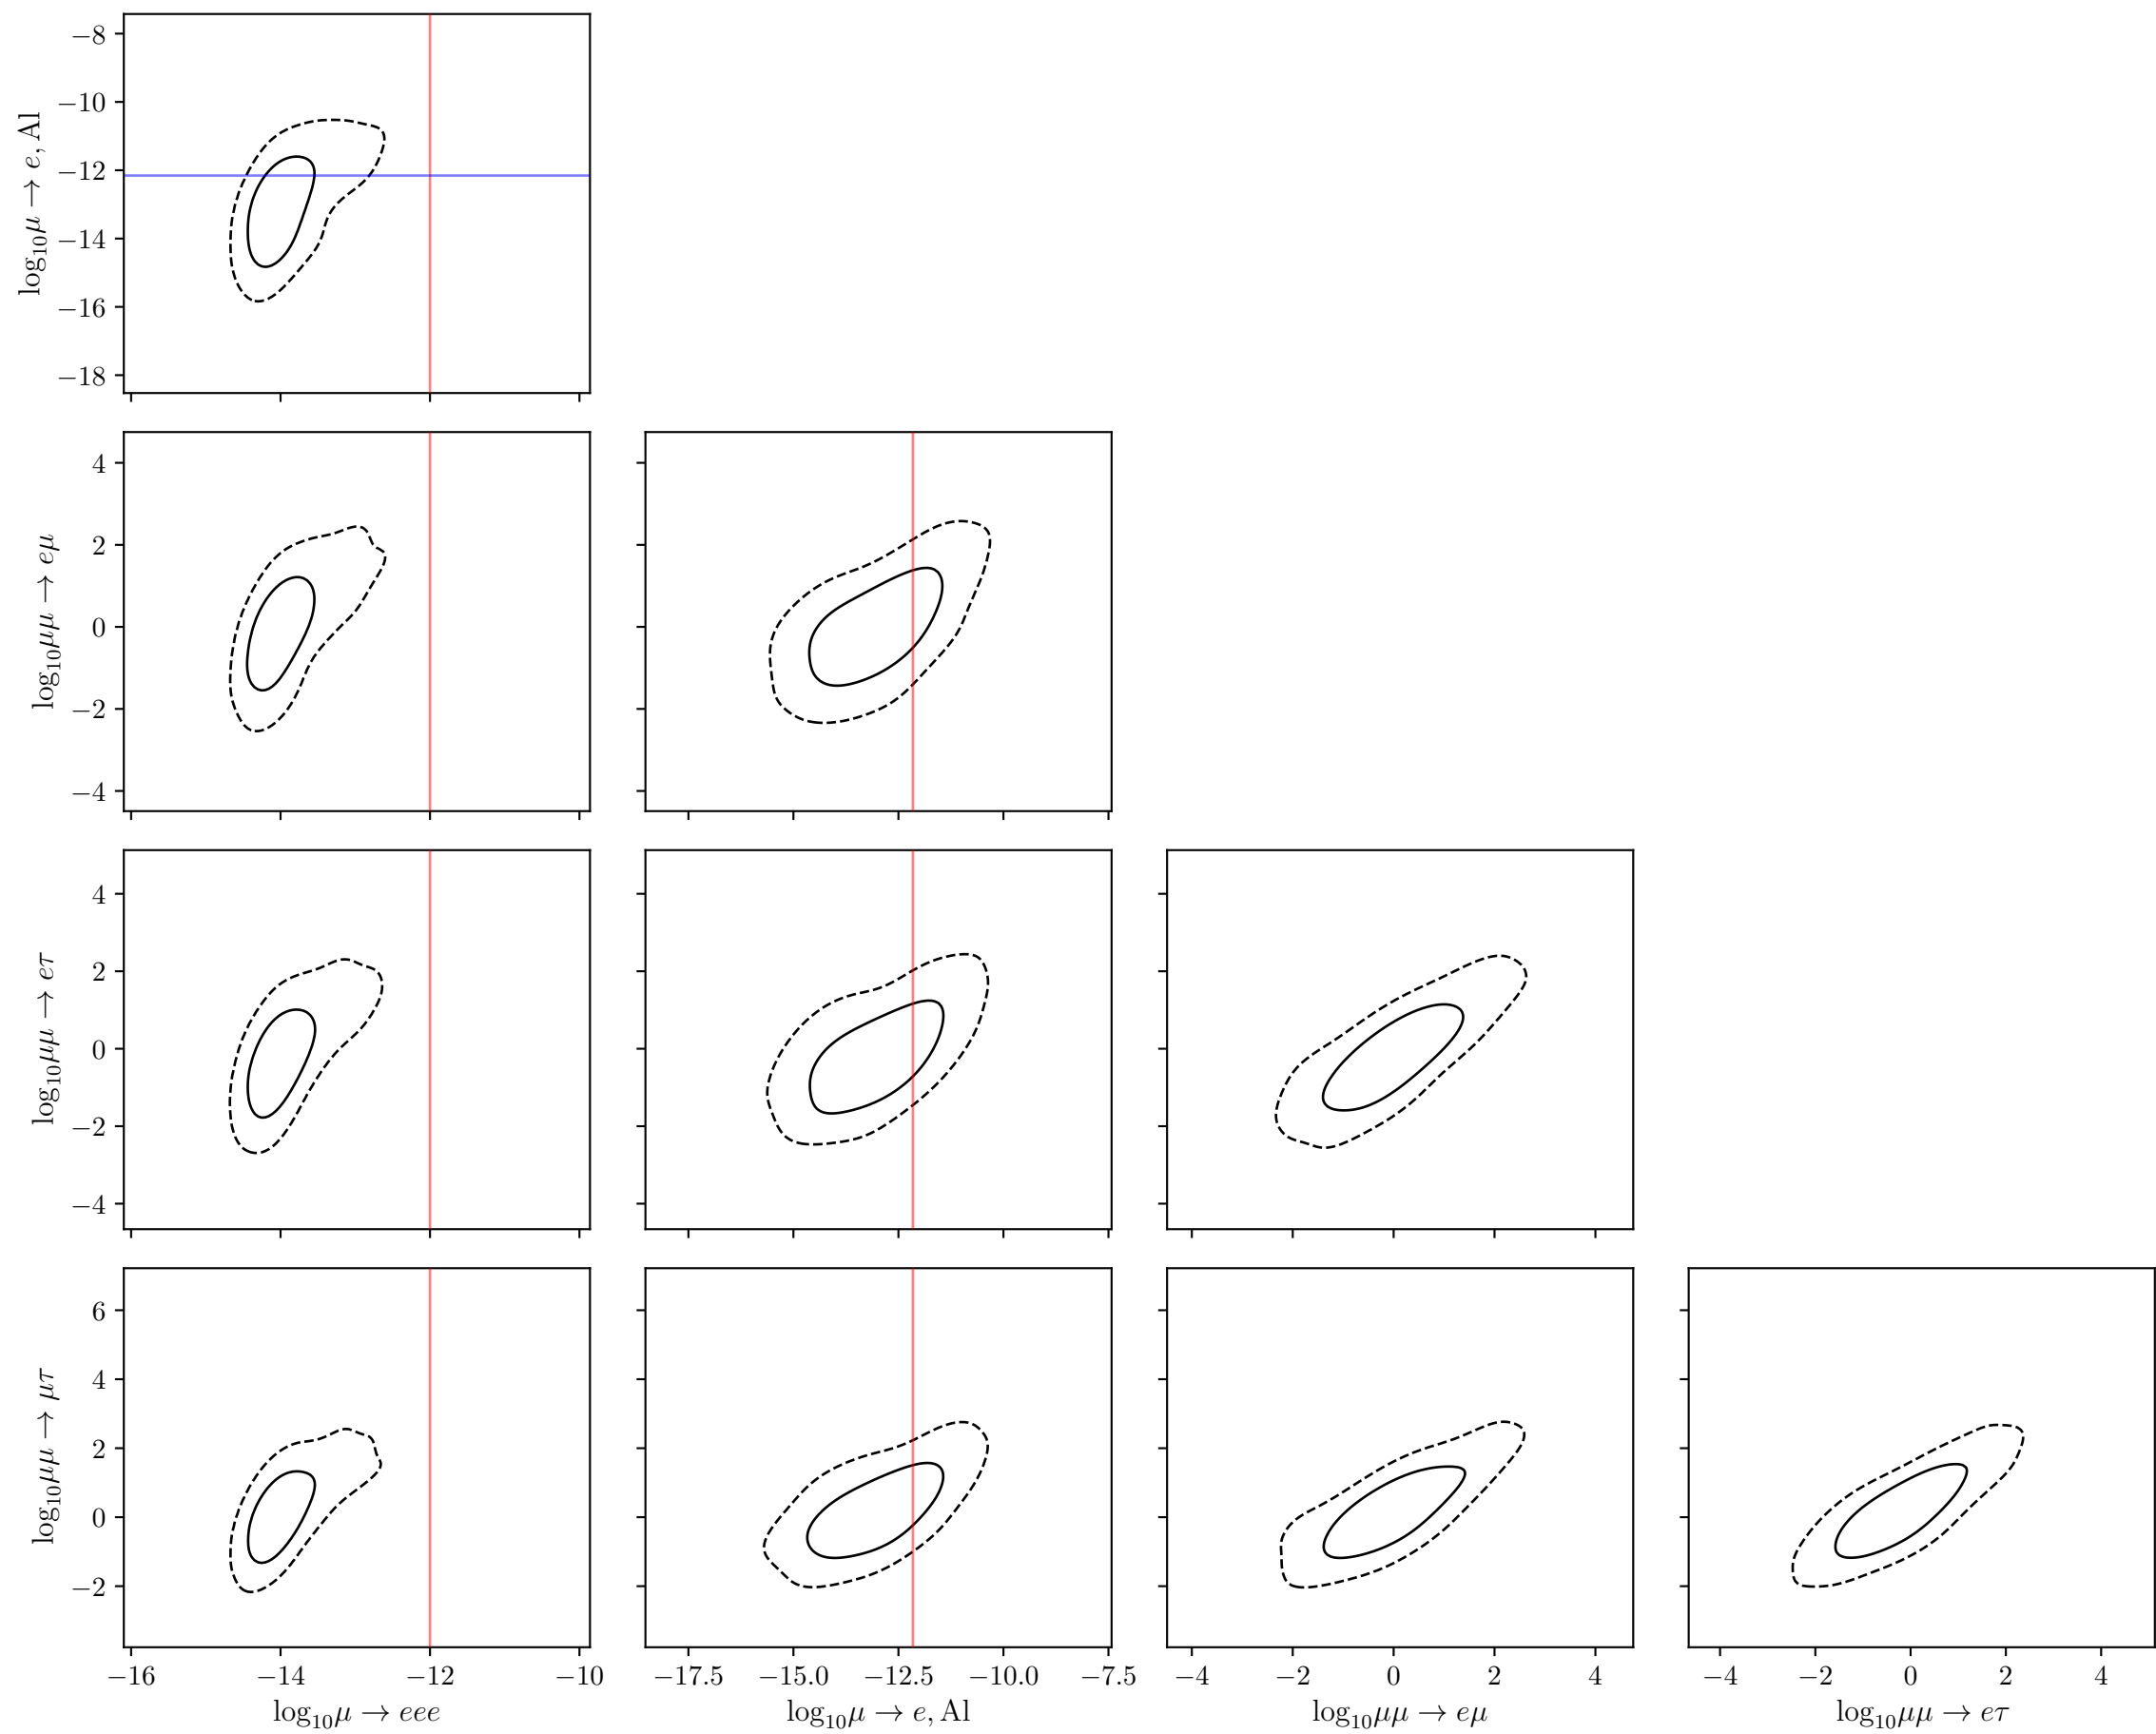

Majorana,  $X_L = \{6, 6, 5\}$ ,  $X_e = \{6, 2, 0\}$ ,

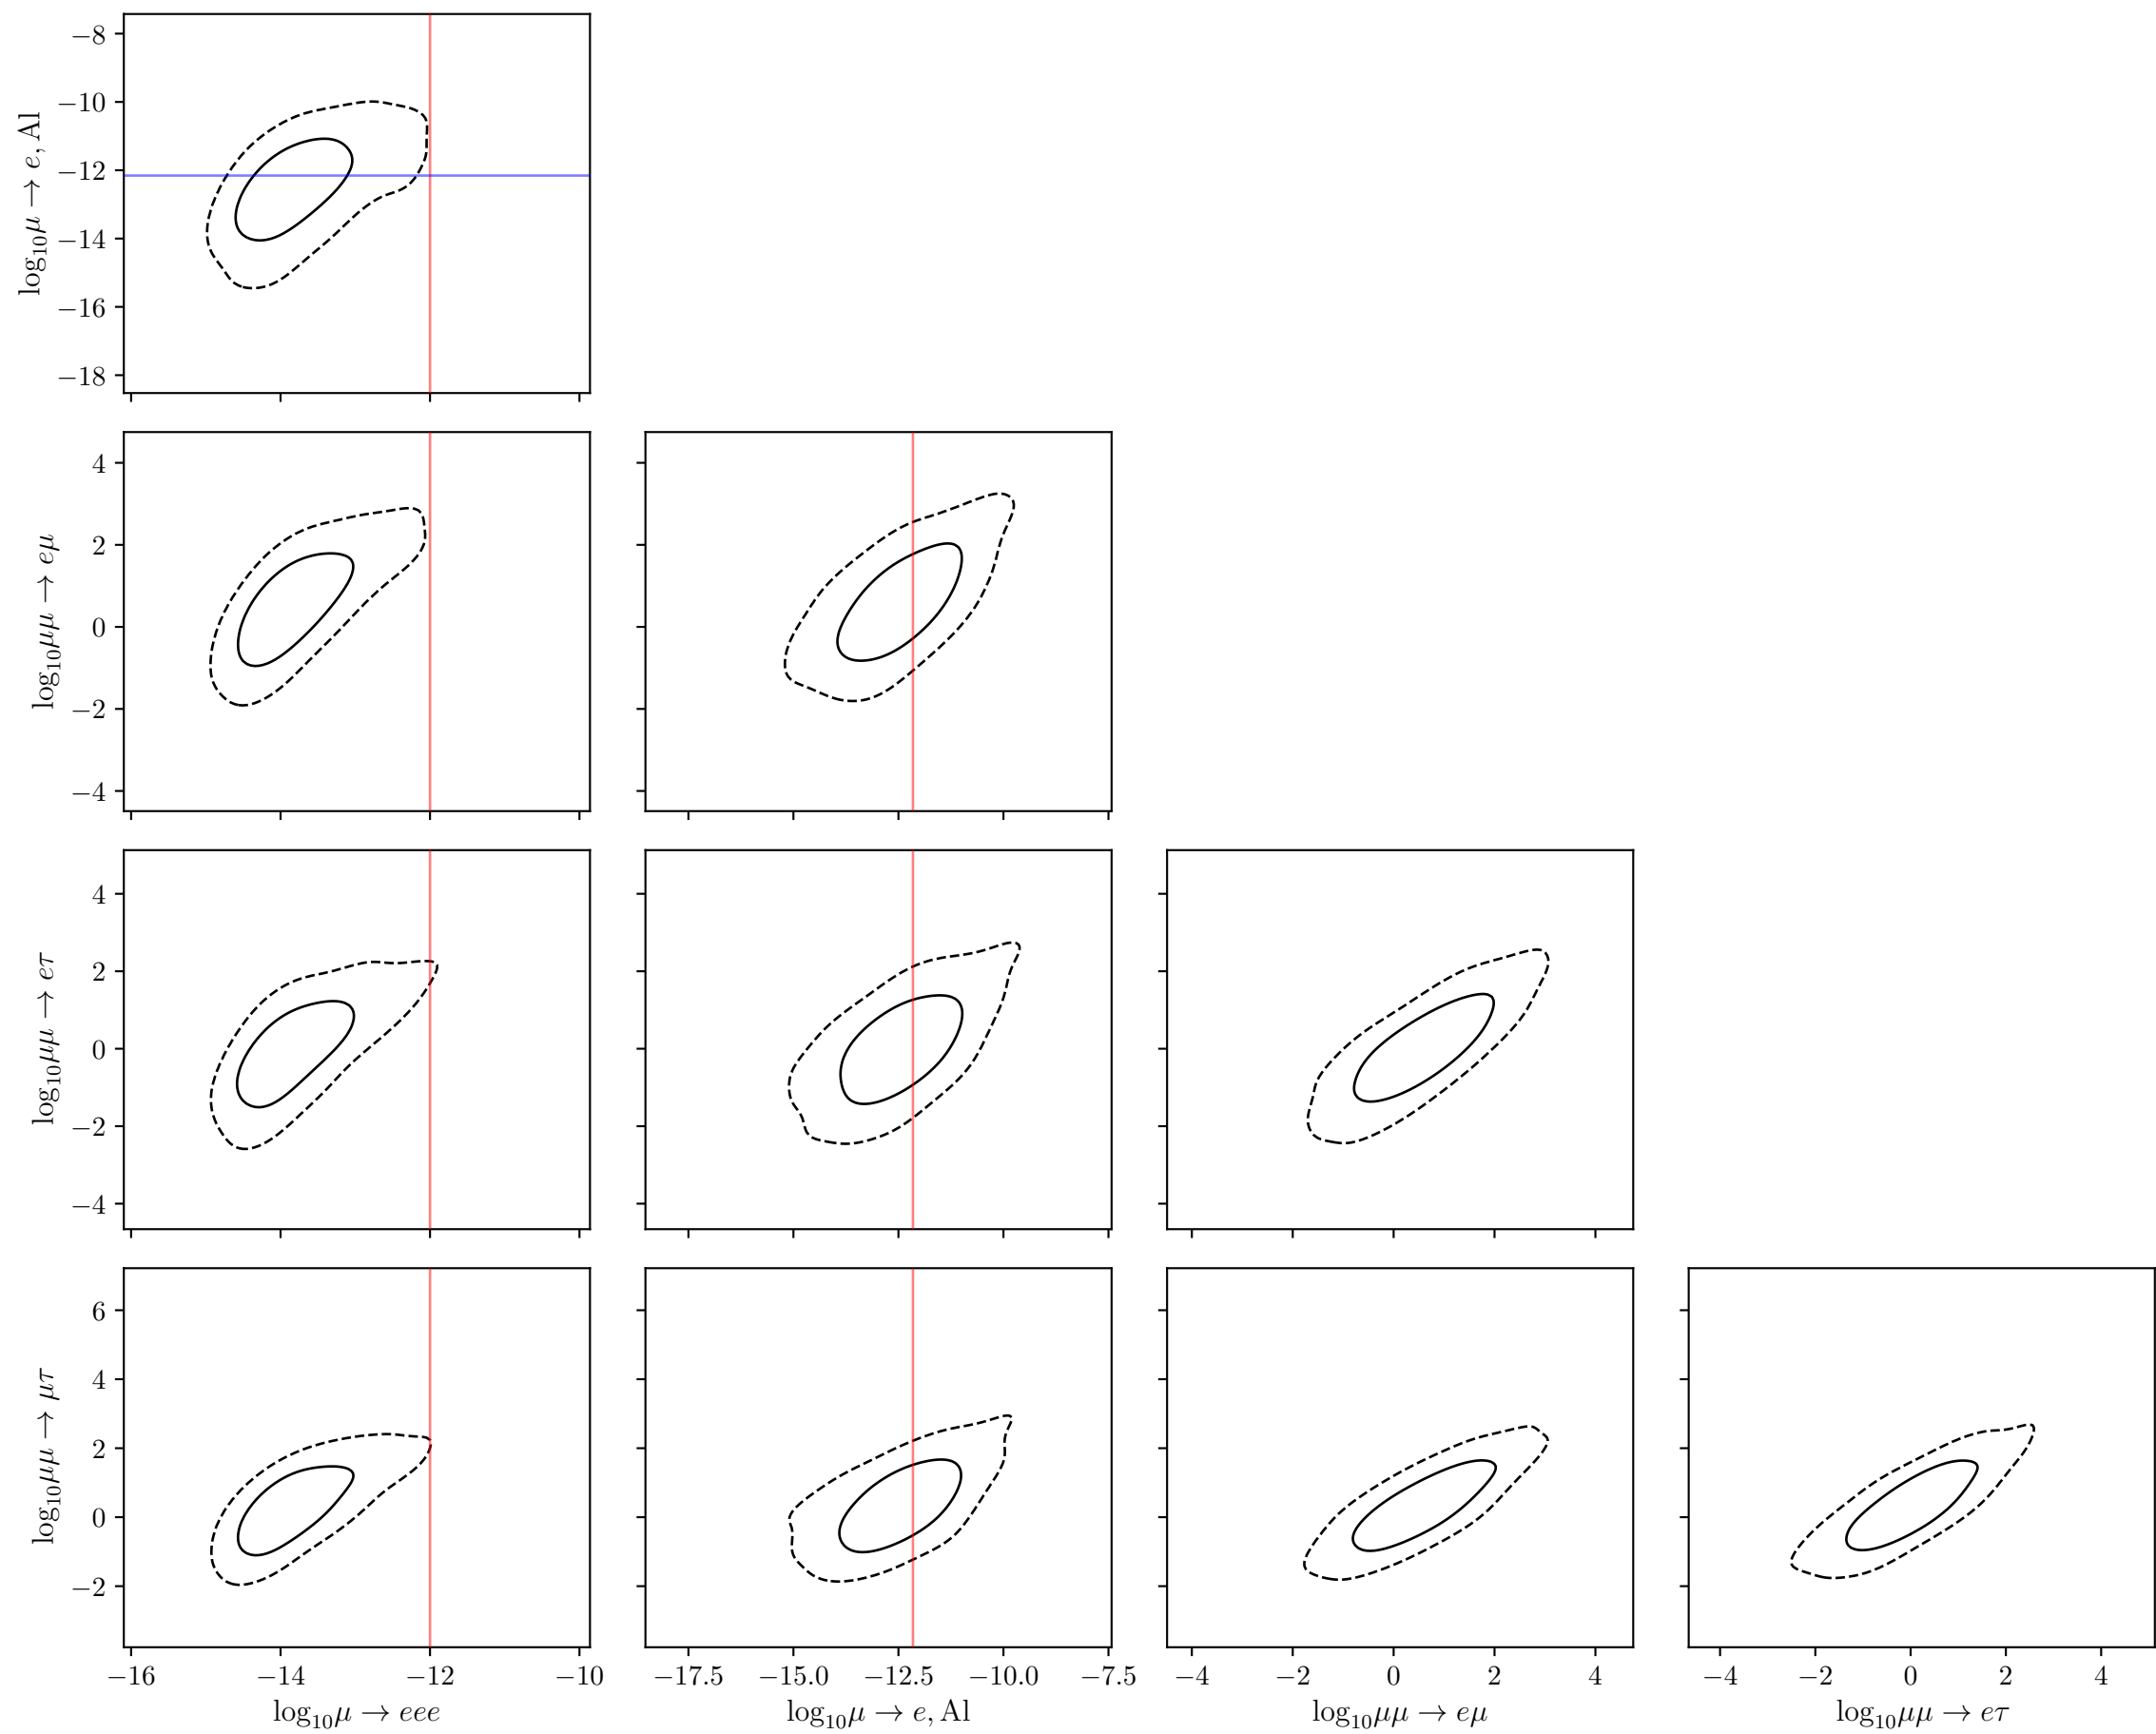

Majorana,  $X_L = \{6, 5, 4\}$ ,  $X_e = \{7, 3, 0\}$ ,

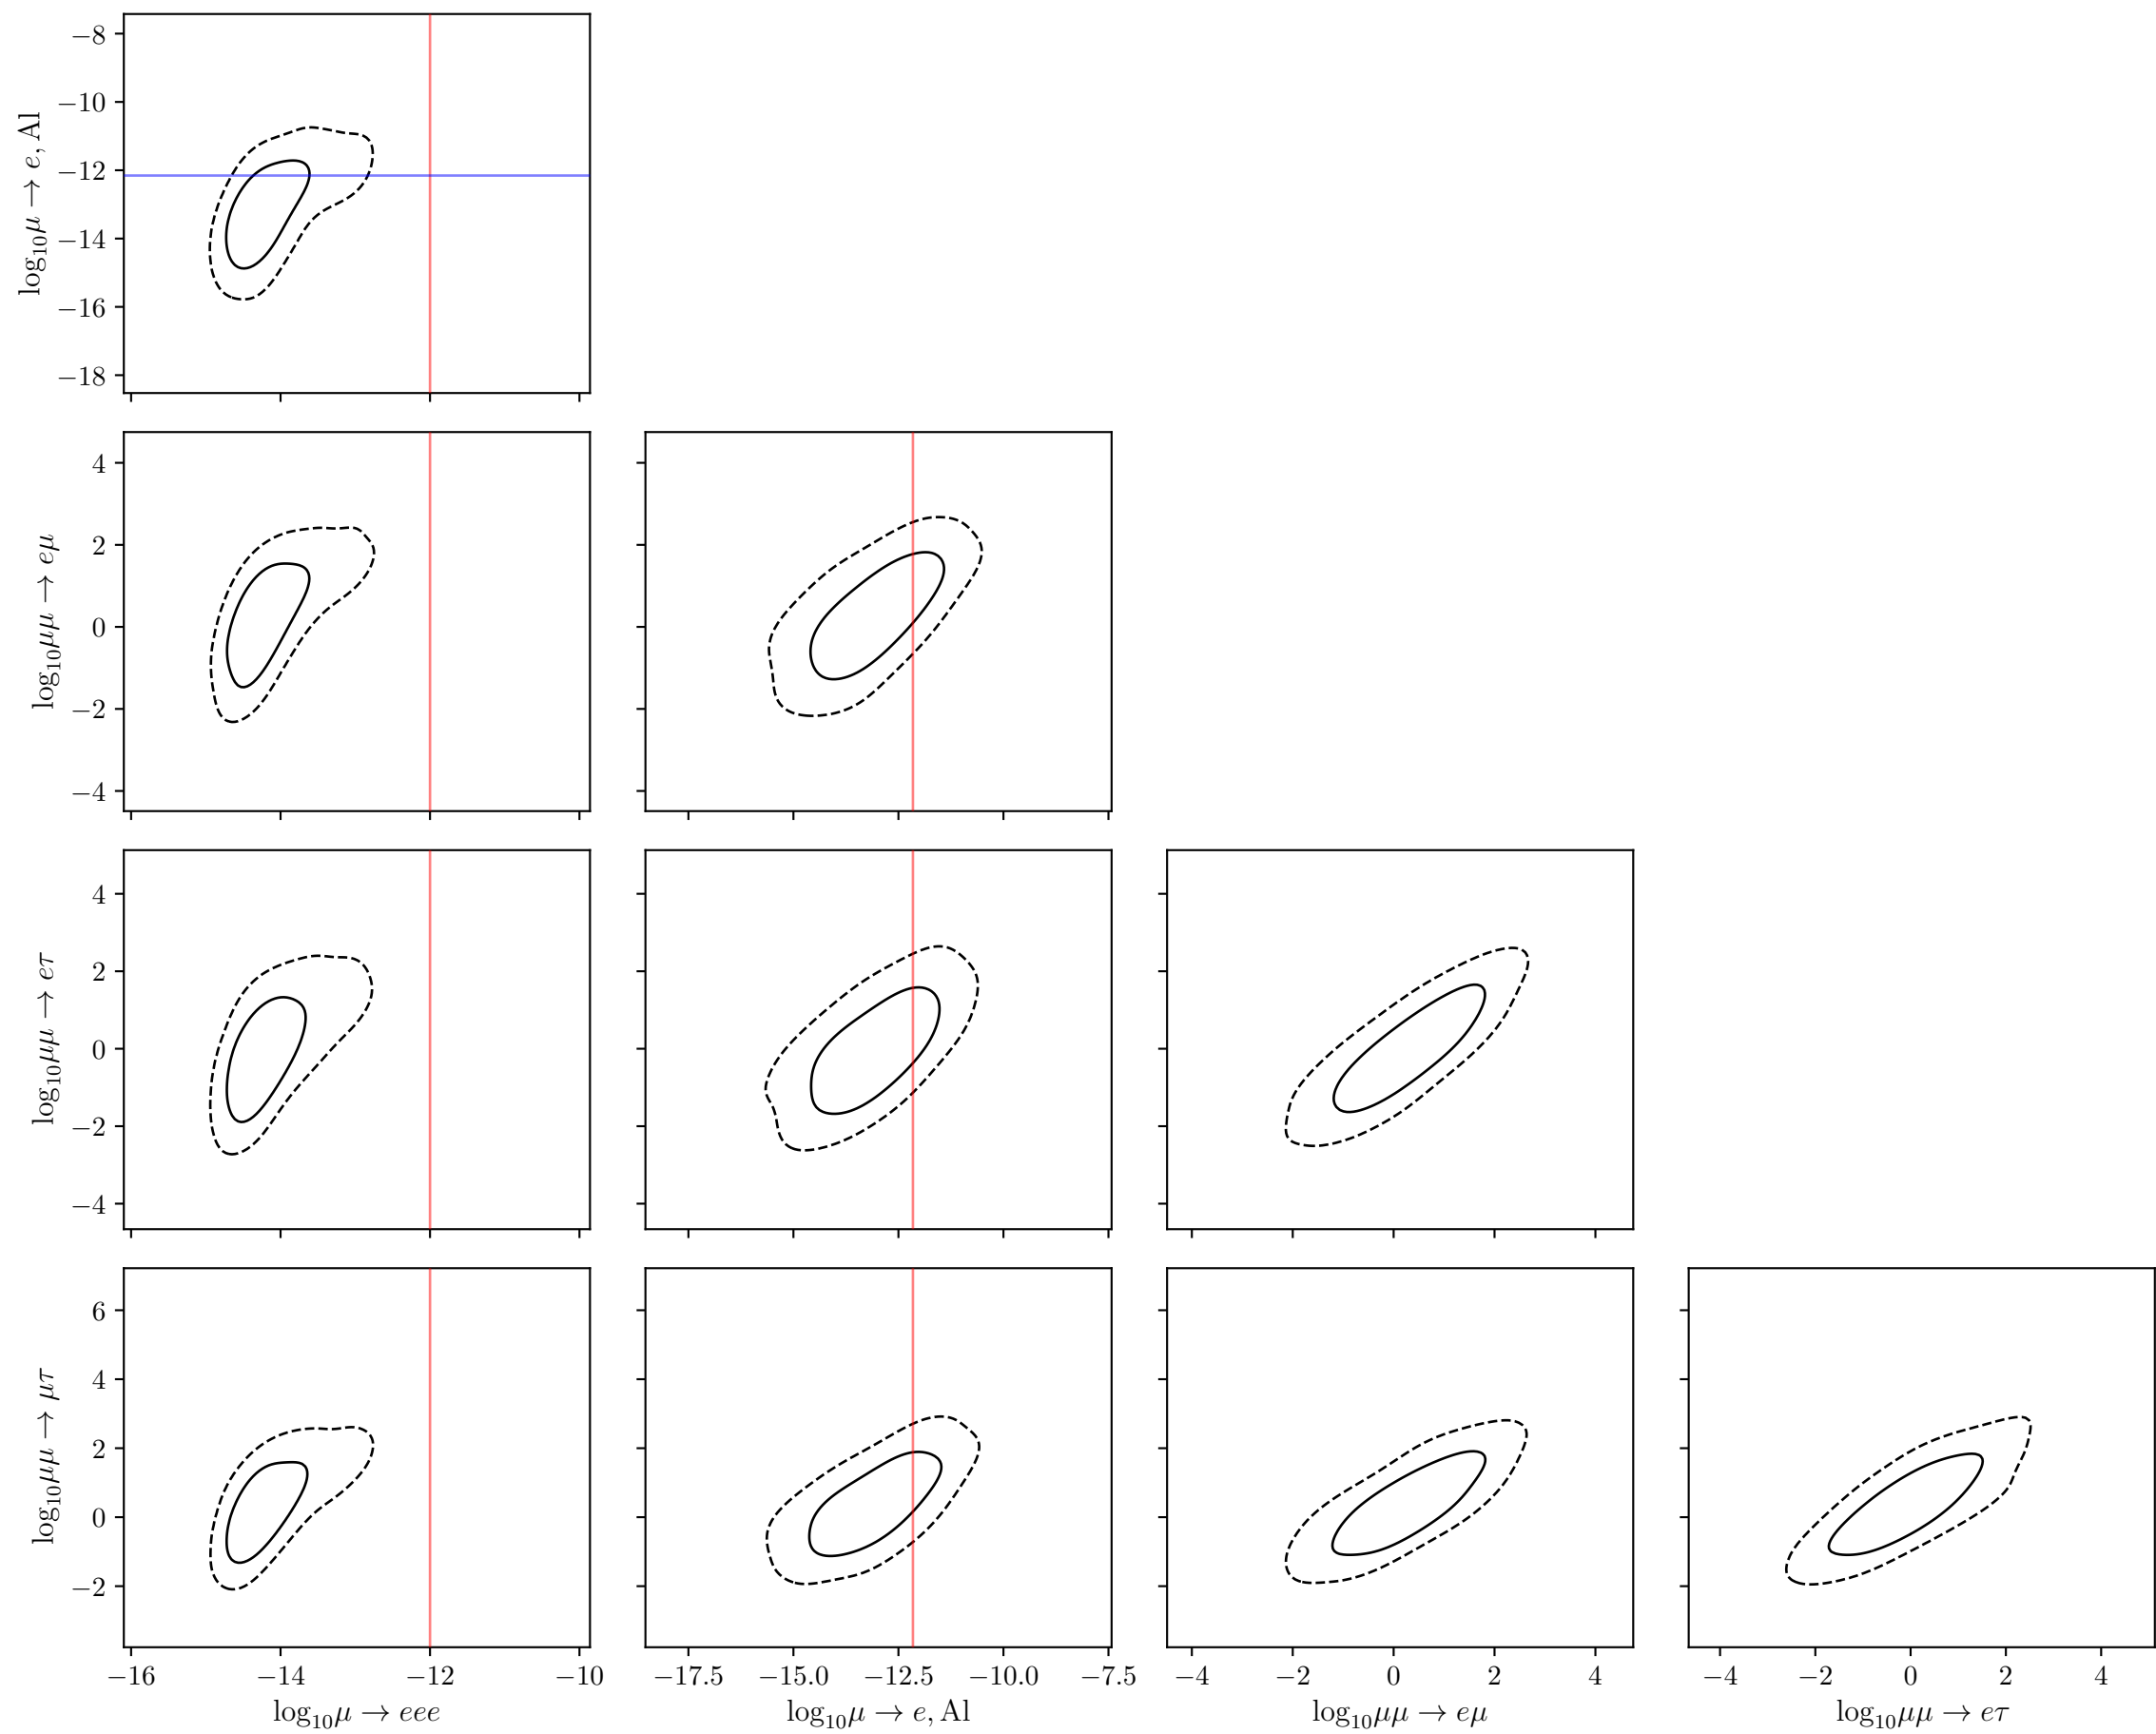

Majorana,  $X_L = \{6, 5, 4\}$ ,  $X_e = \{6, 2, 0\}$ ,

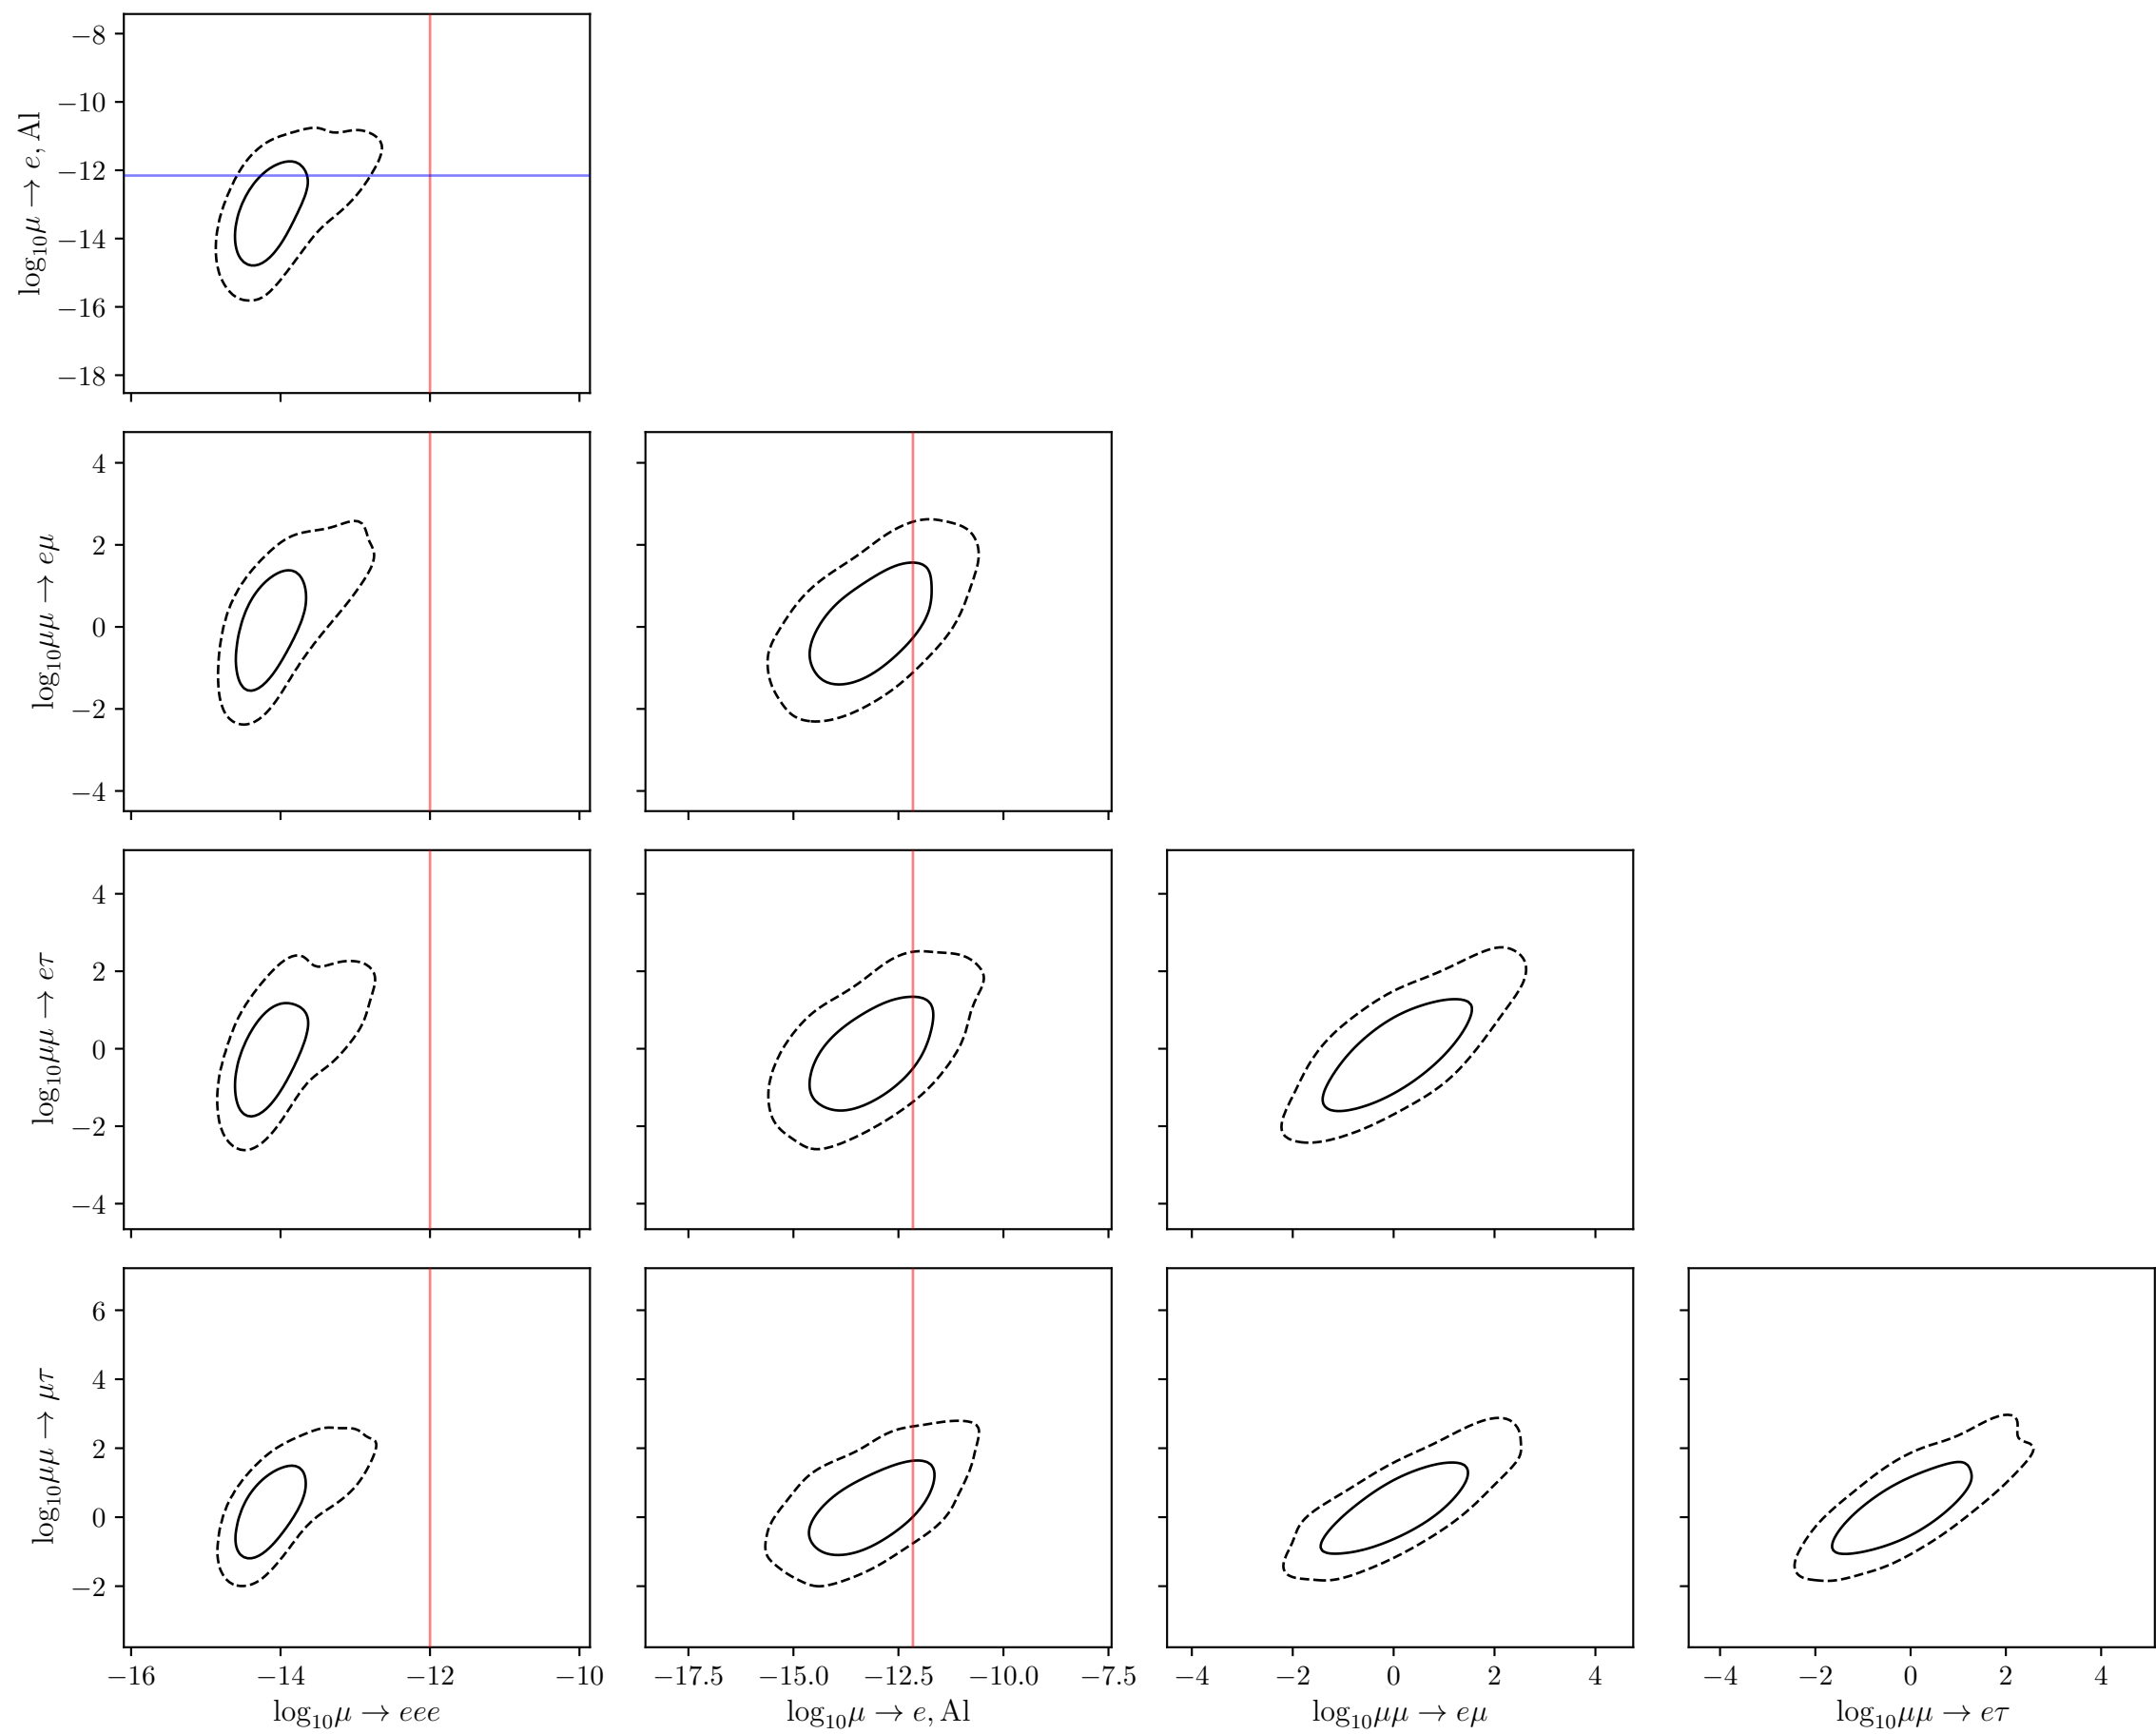

Majorana,  $X_L = \{7, 6, 5\}$ ,  $X_e = \{6, 2, 0\}$ ,

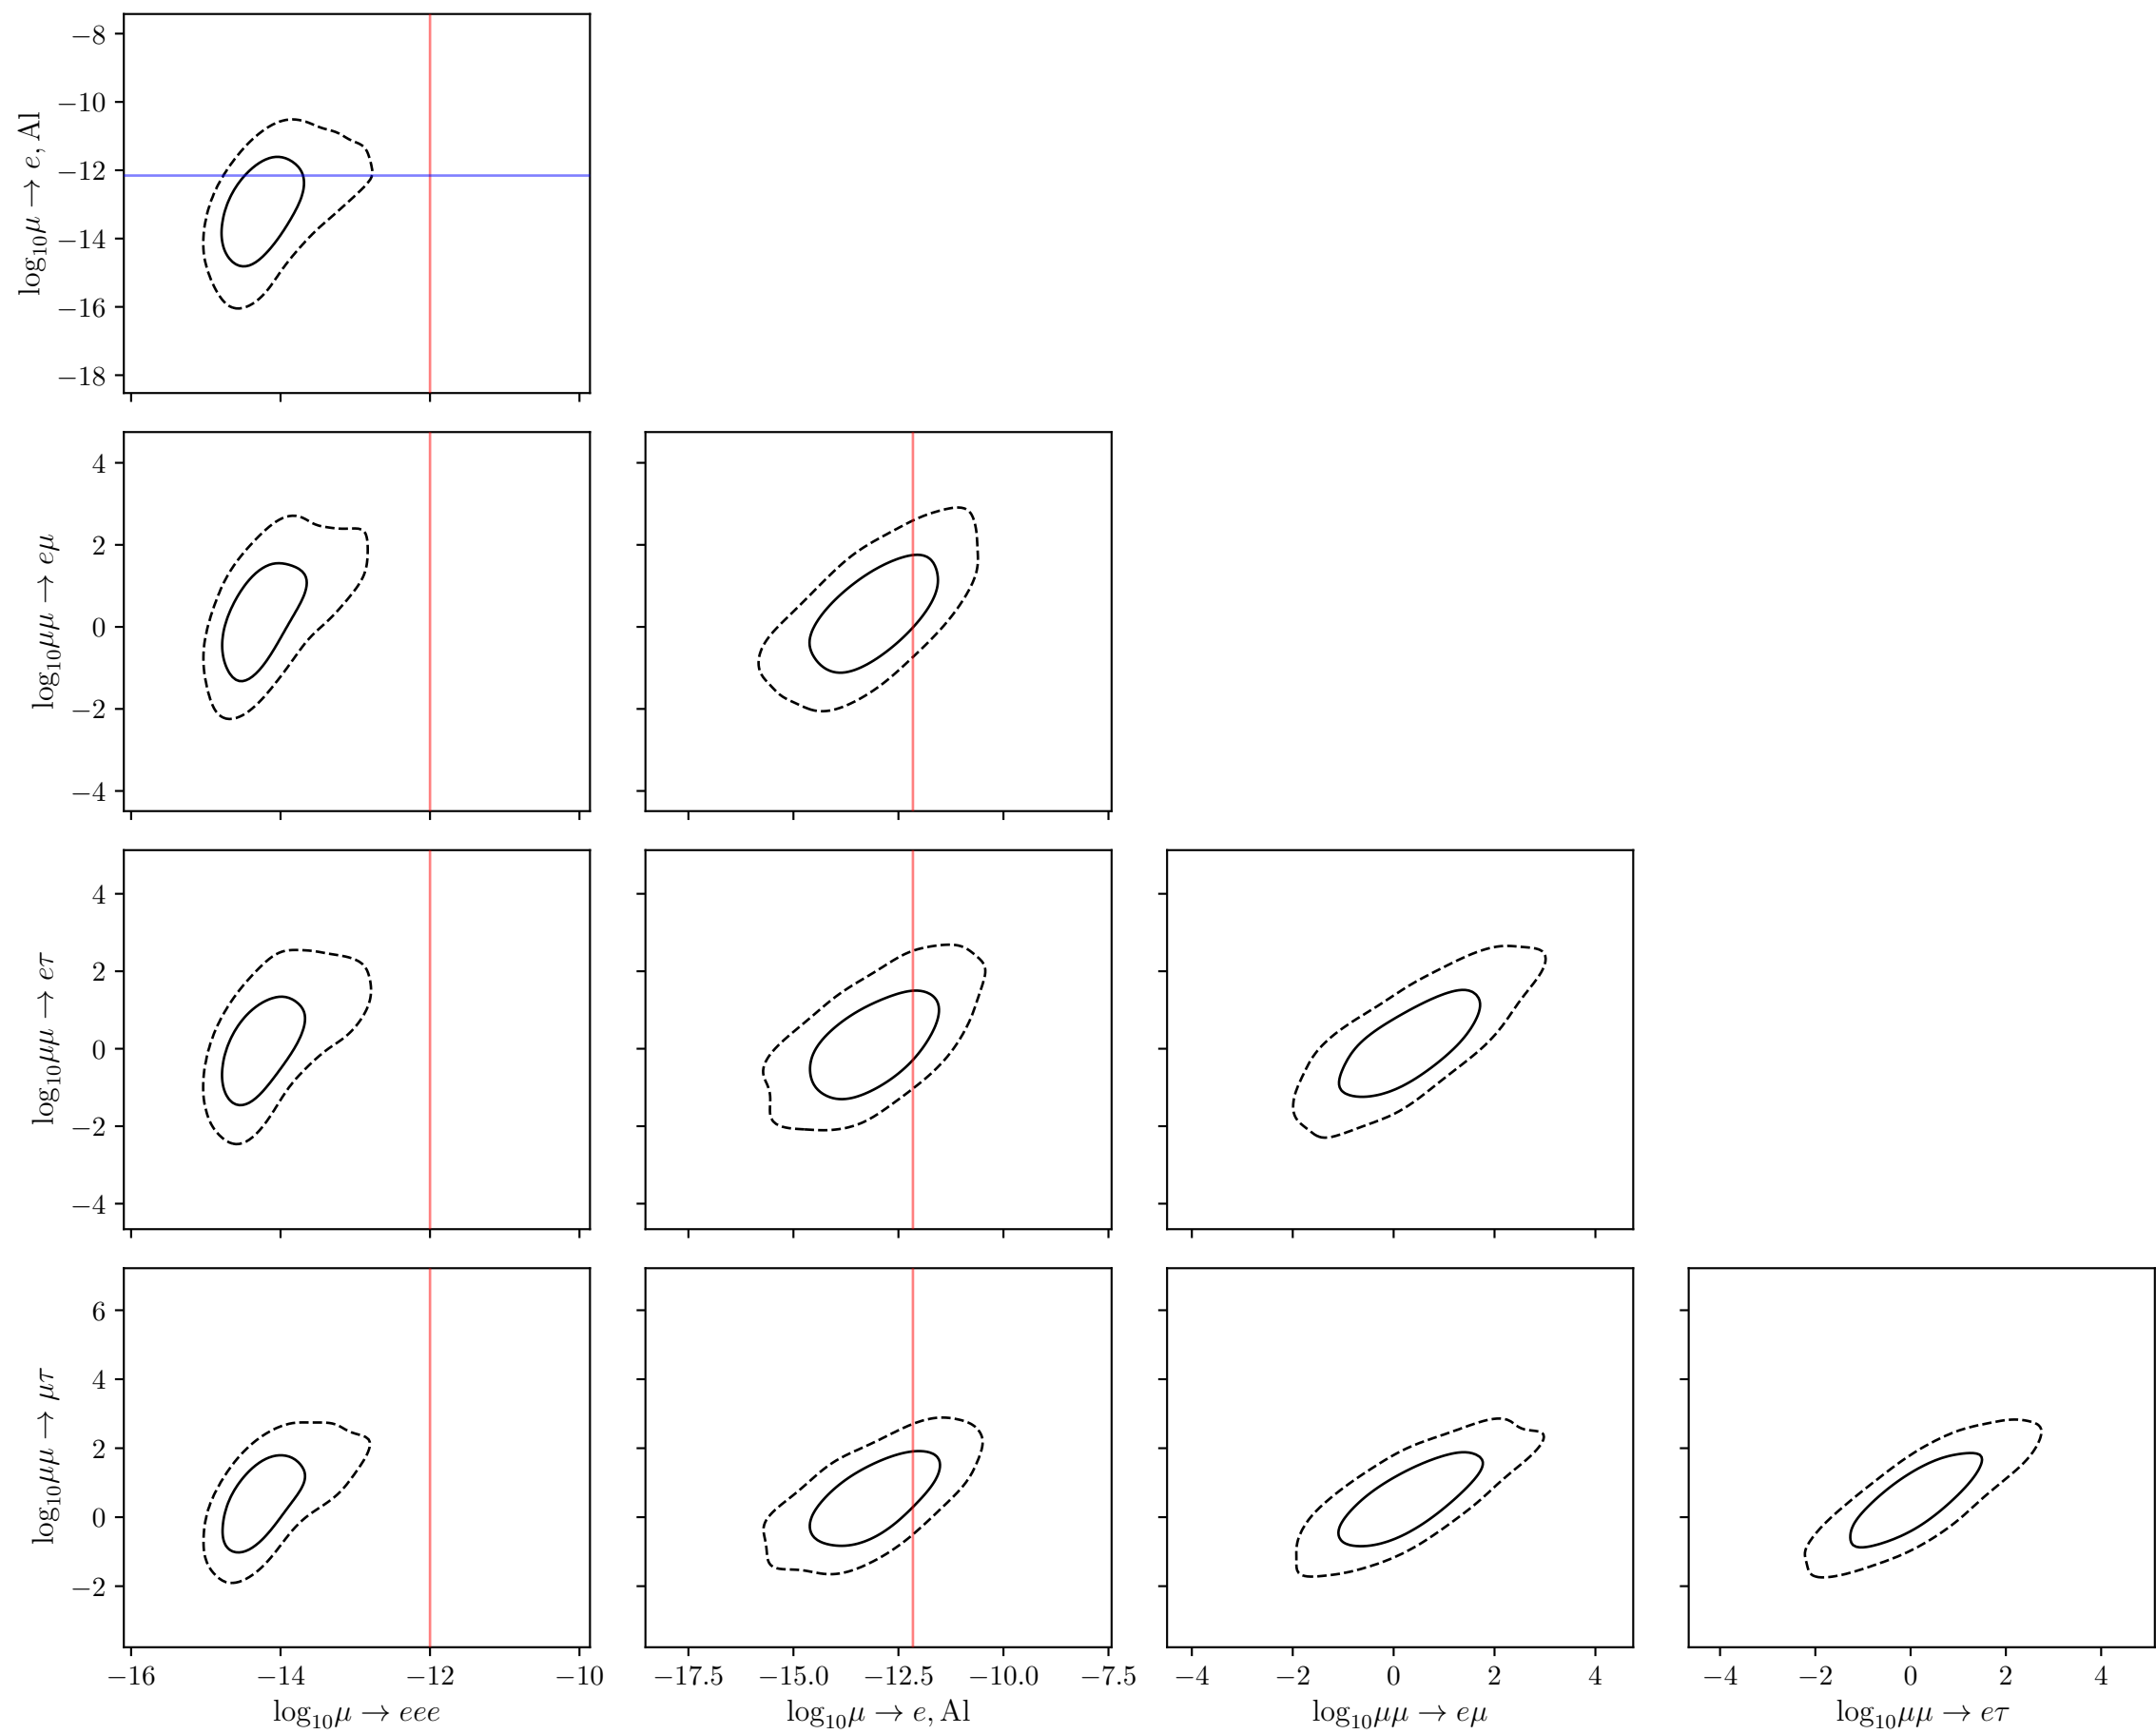

Majorana,  $X_L = \{5, 4, 3\}$ ,  $X_e = \{7, 3, 1\}$ ,

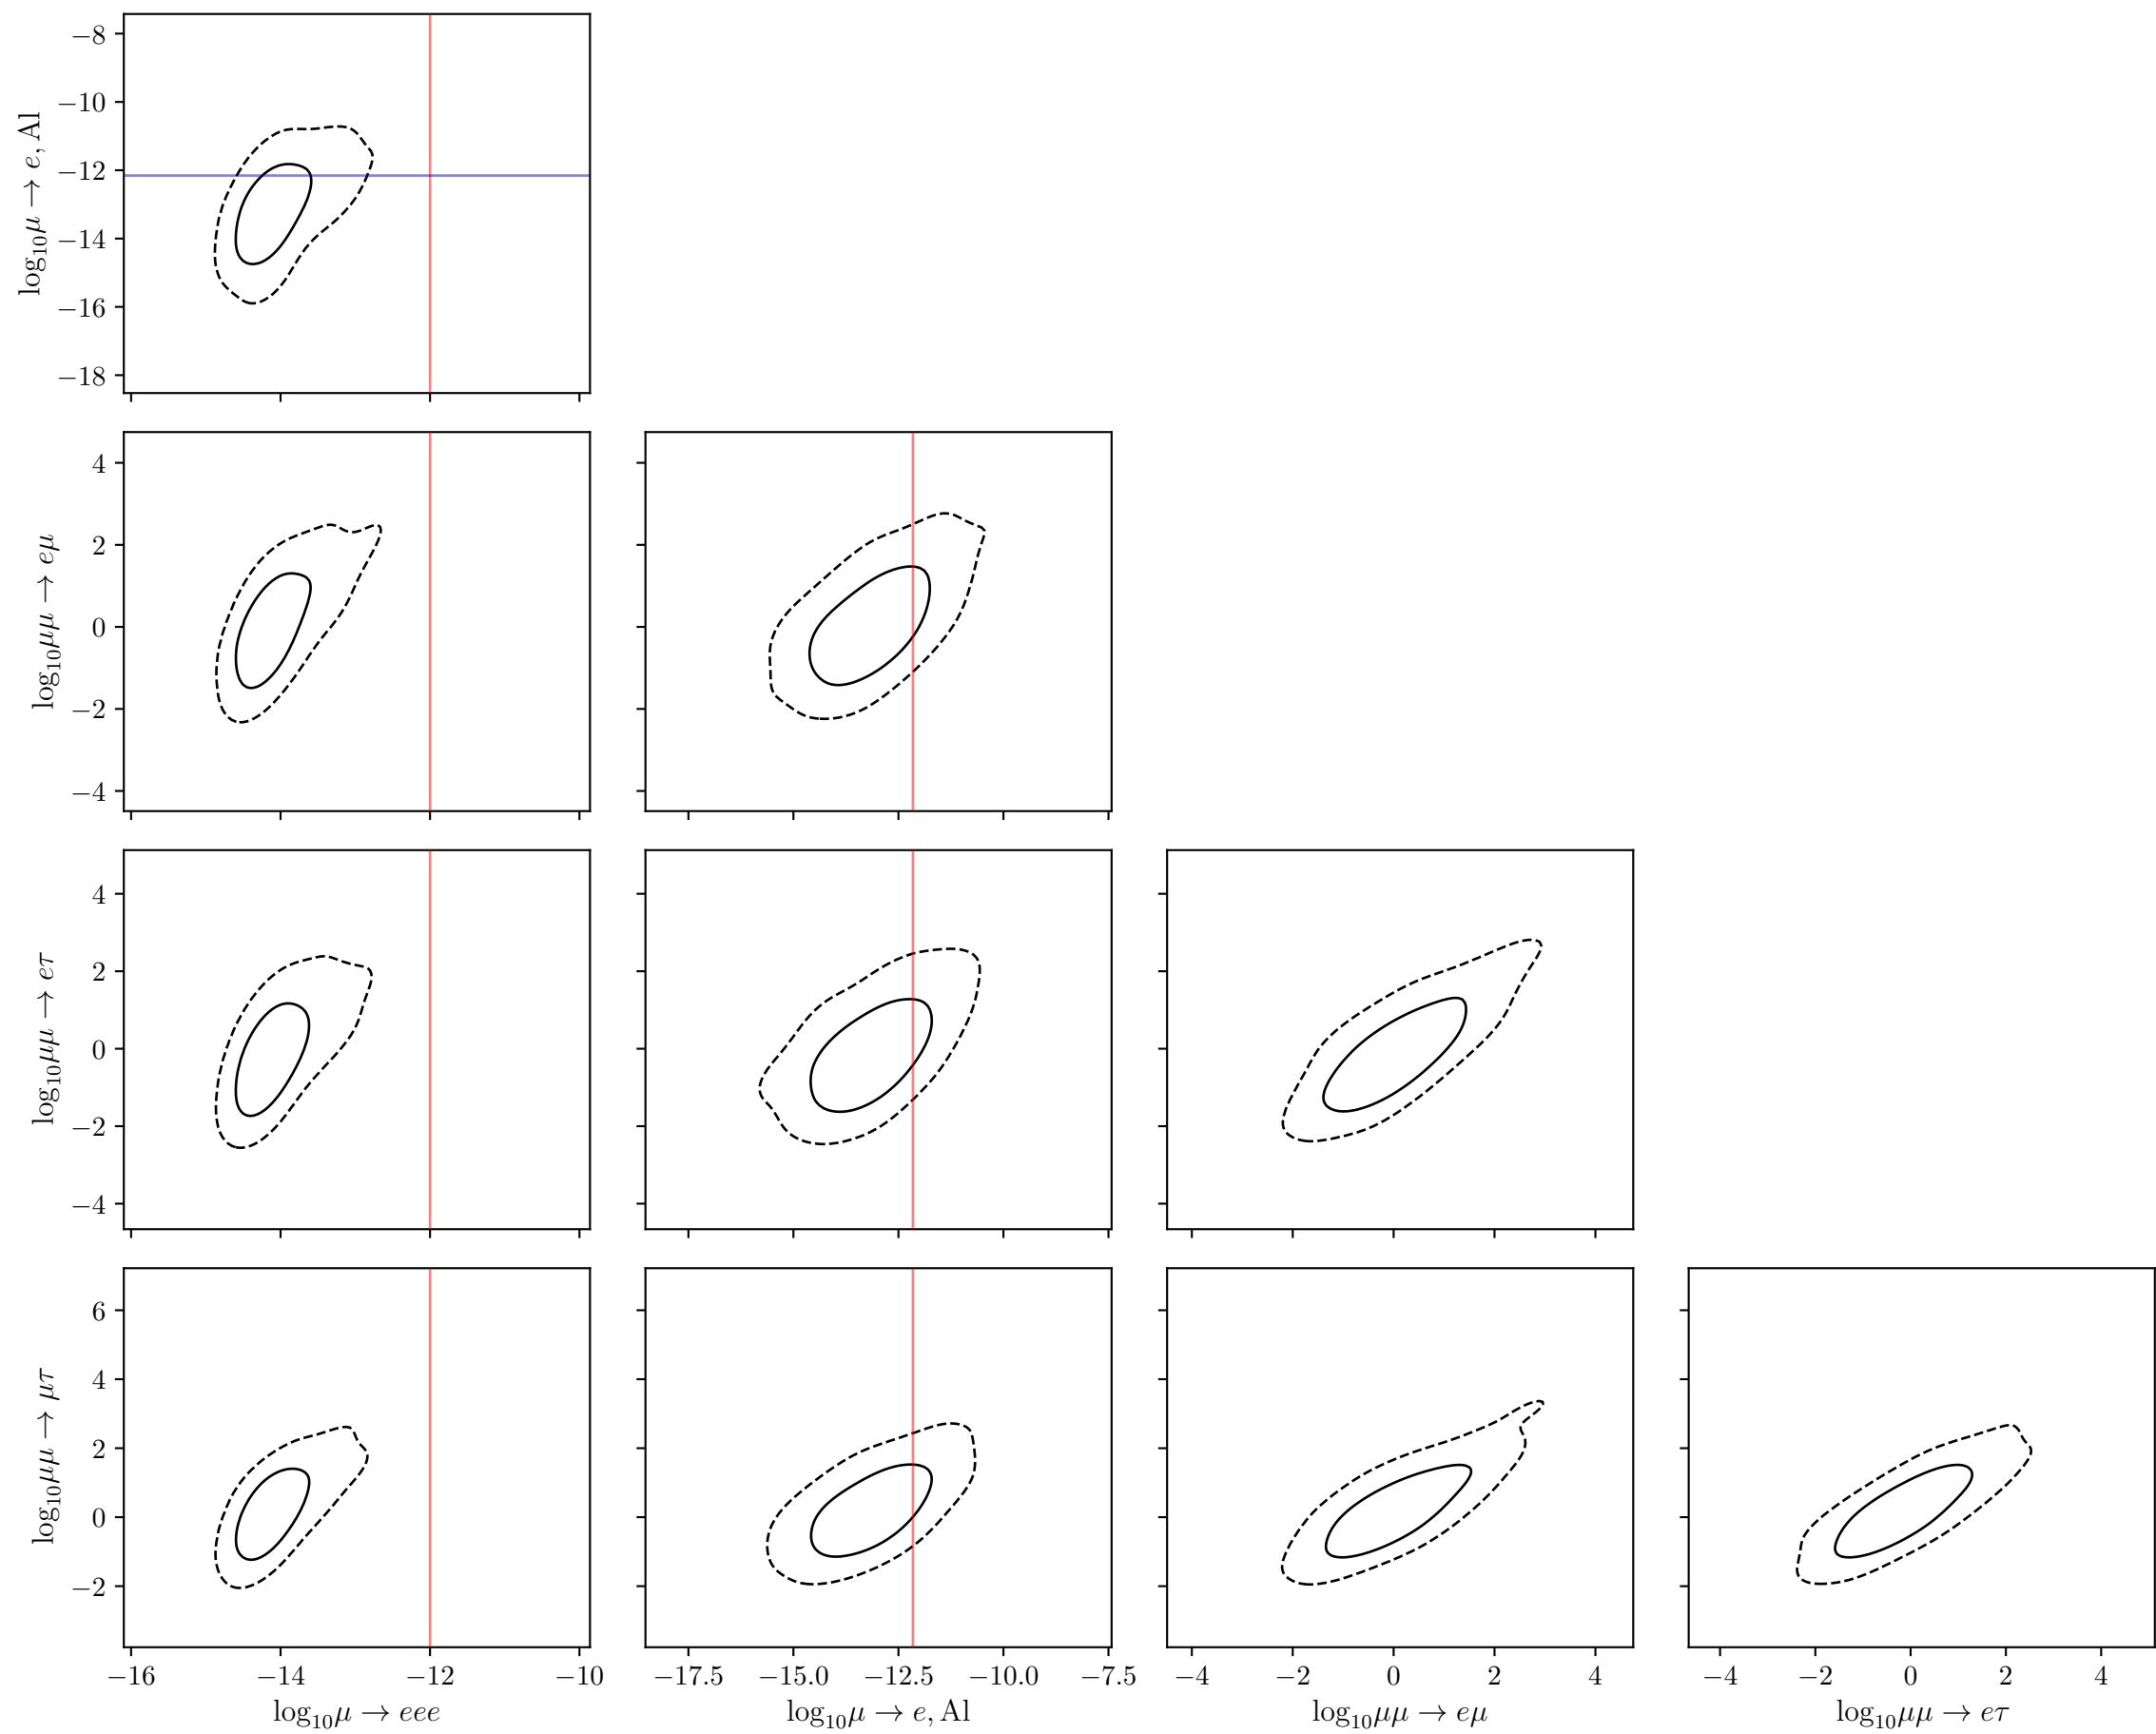



Majorana,  $X_L = \{6, 5, 4\}$ ,  $X_e = \{5, 2, 0\}$ ,

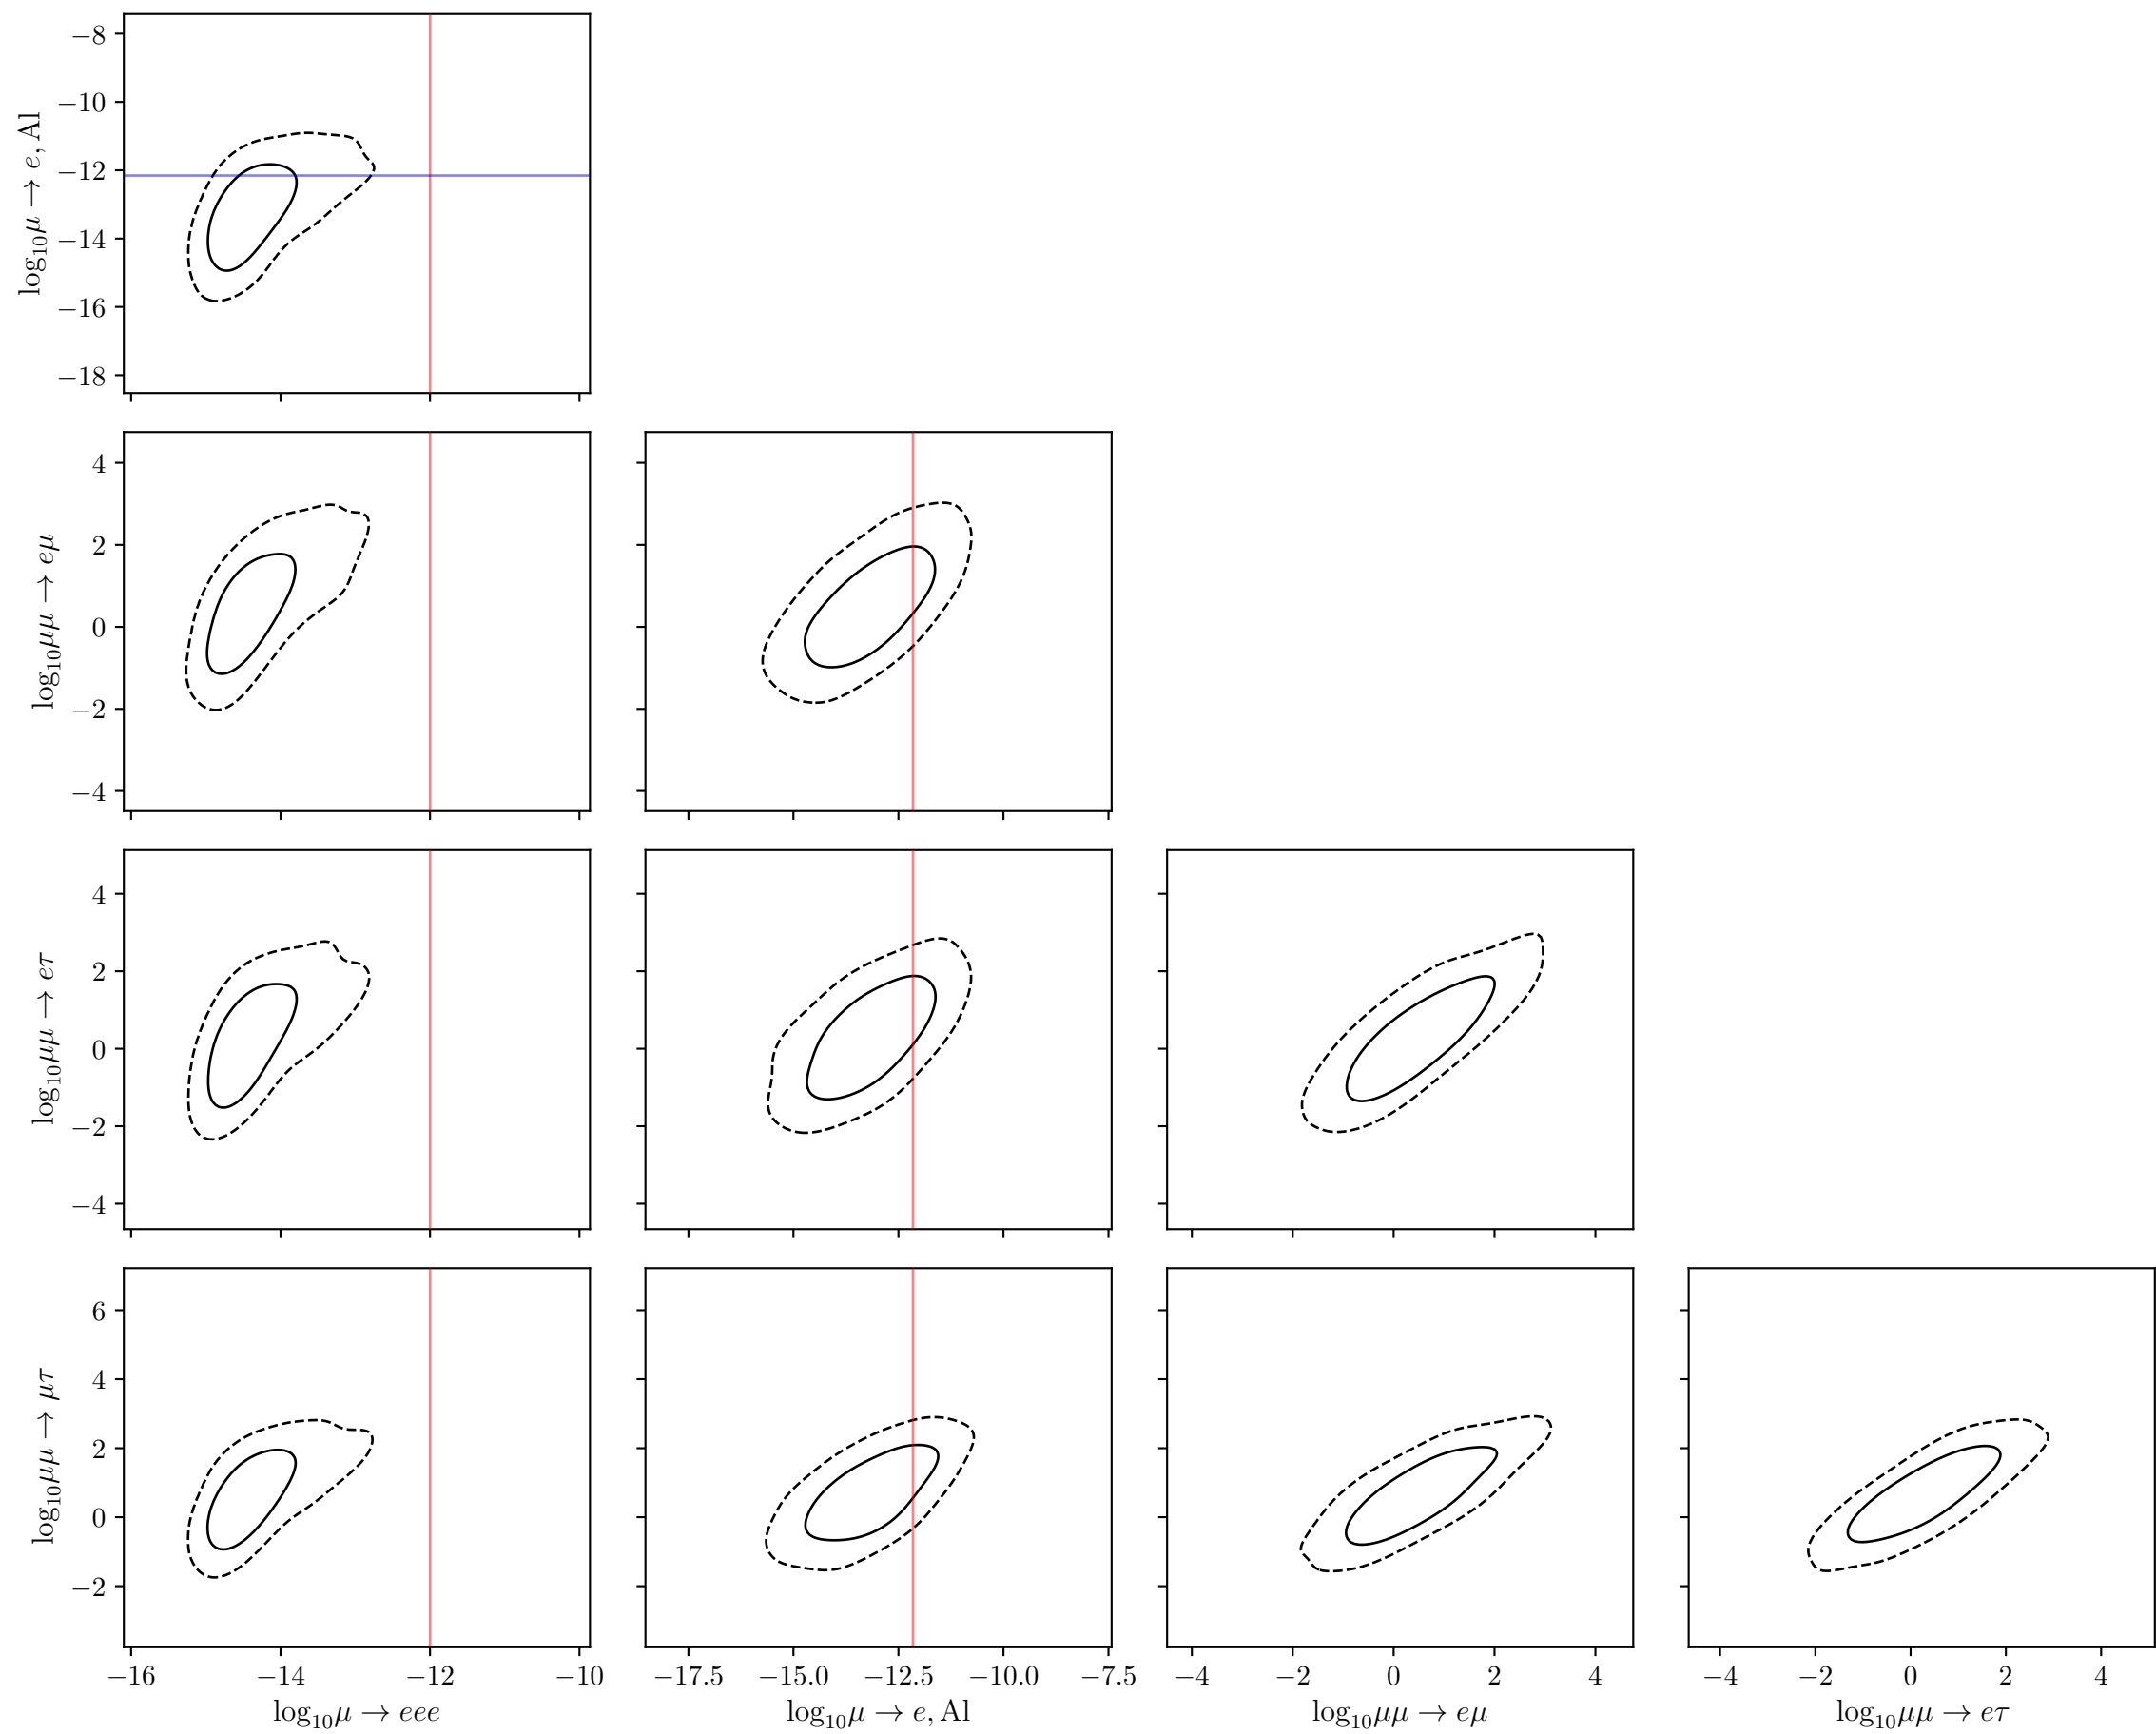

Majorana,  $X_L = \{5, -2, -2\}$ ,  $X_e = \{-1, 4, 6\}$ ,

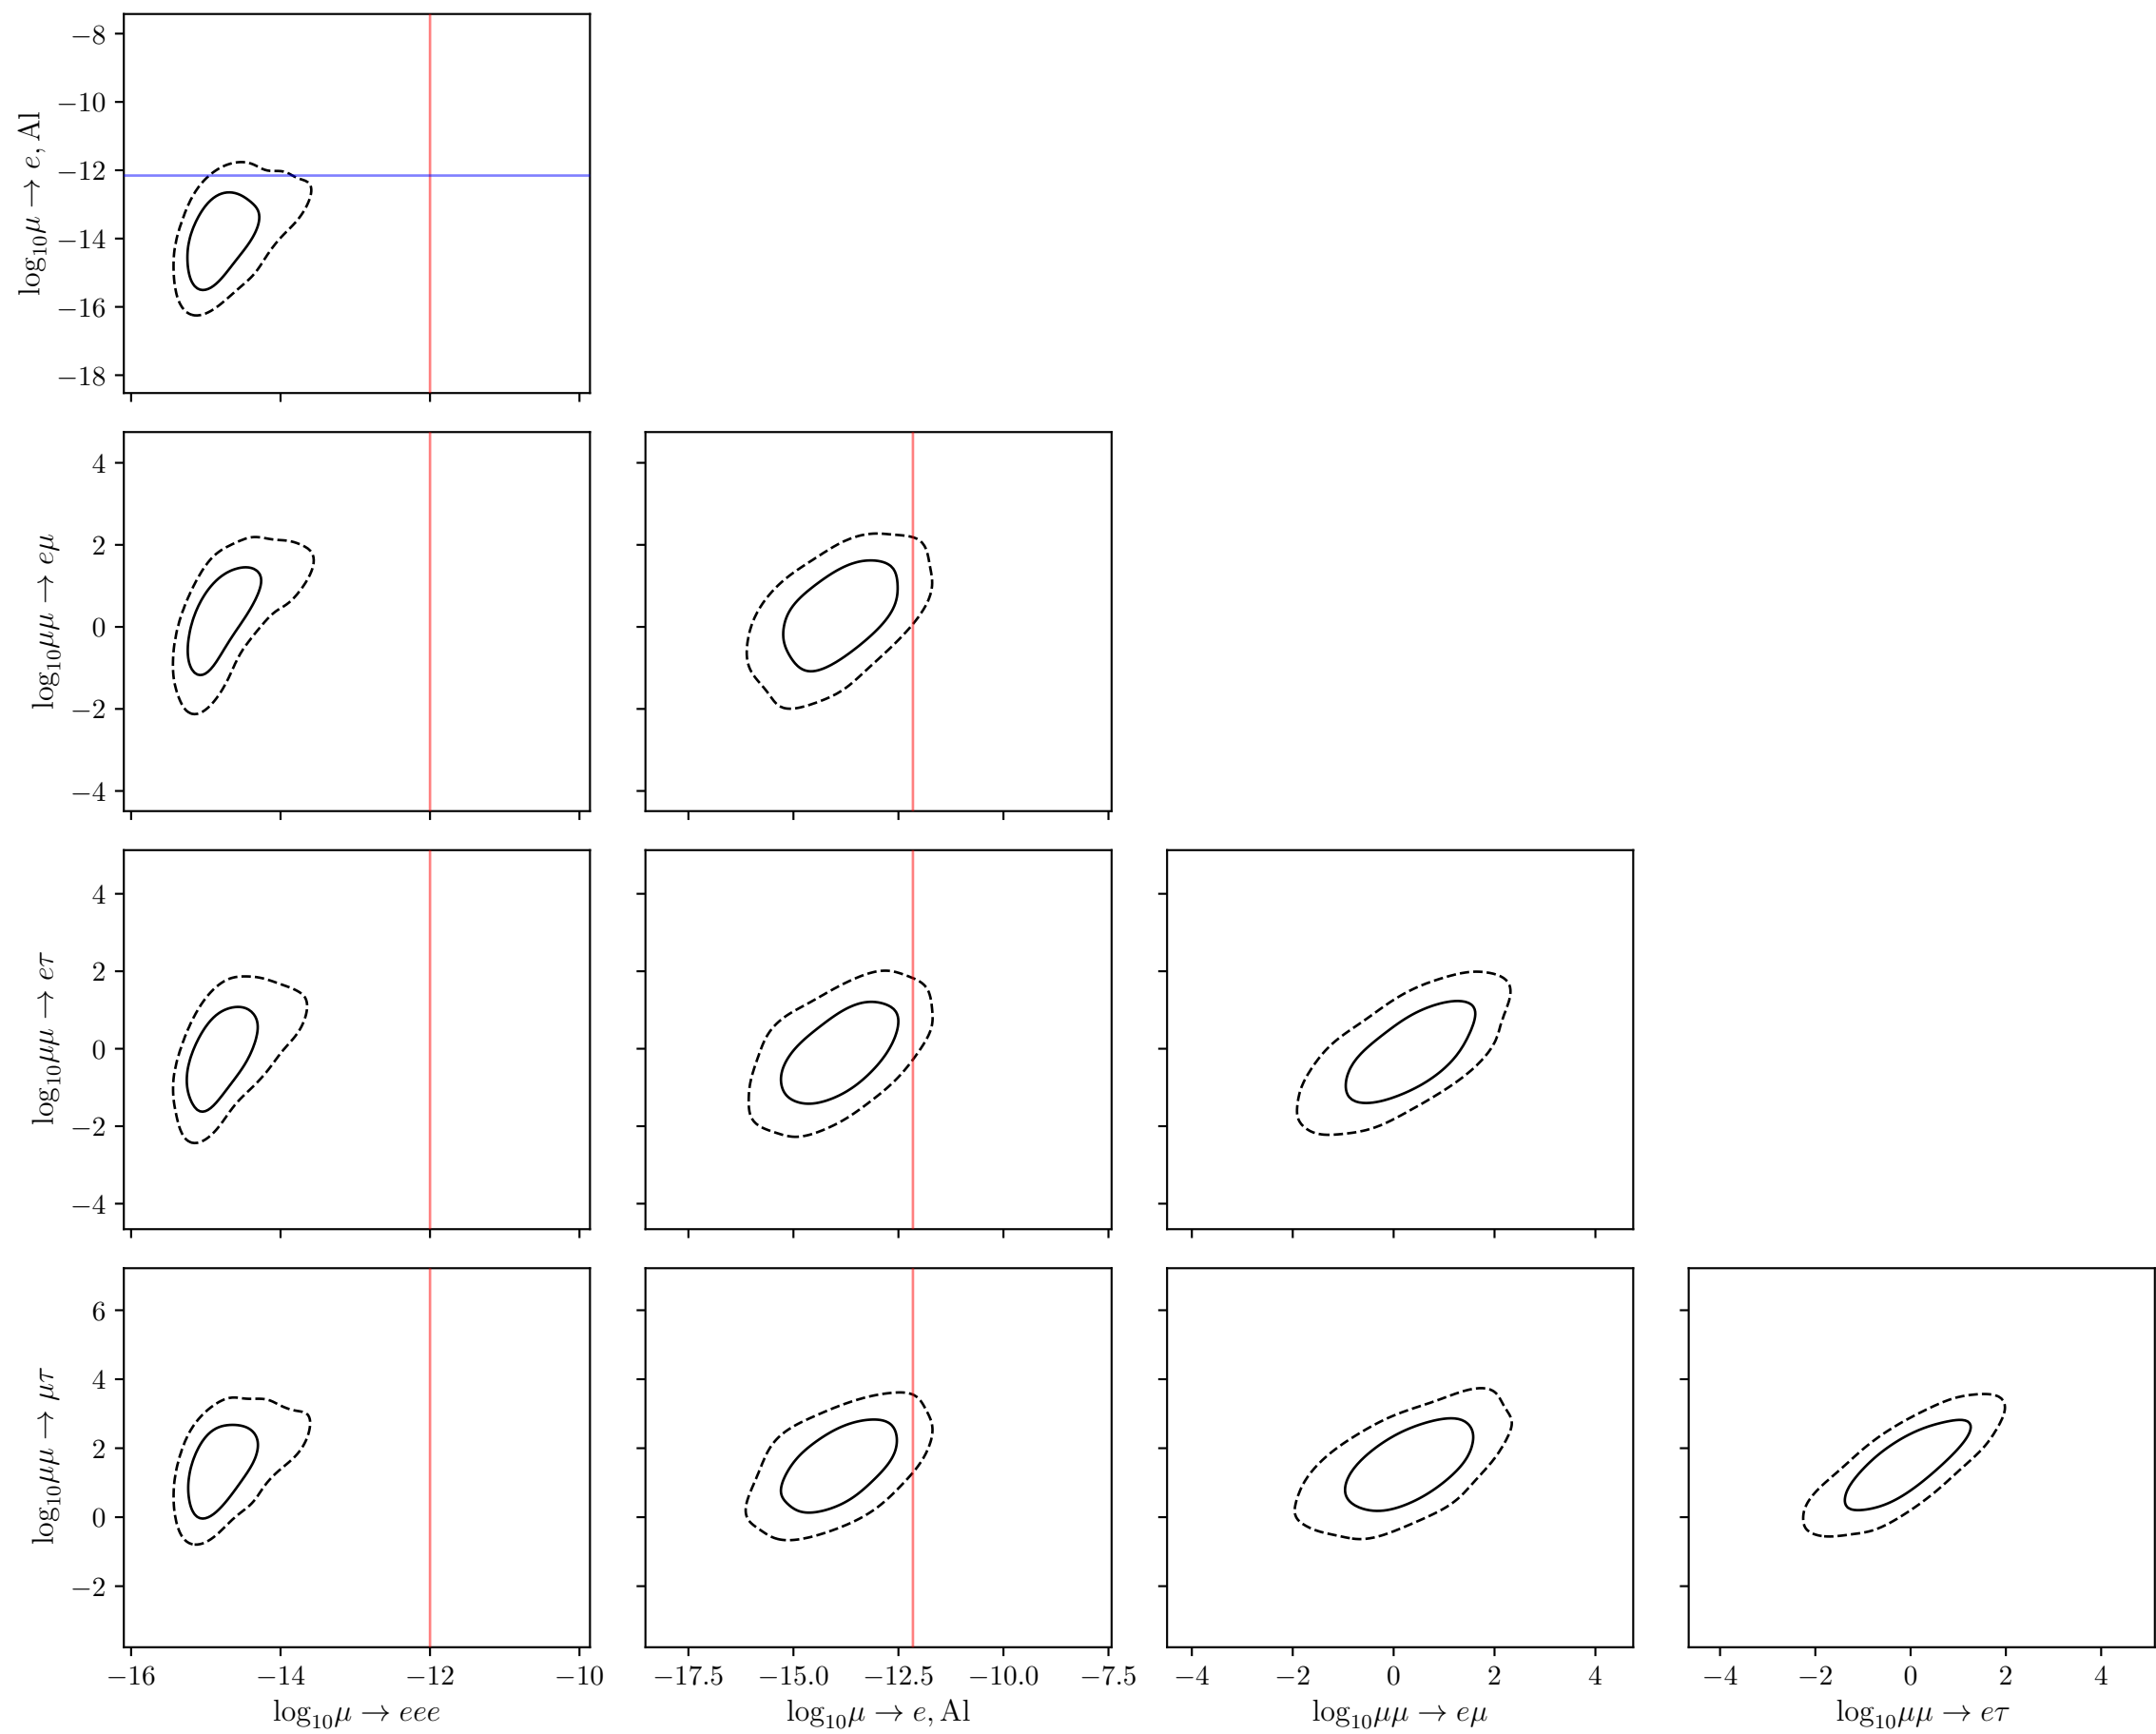

Majorana,  $X_L = \{5, 4, 3\}$ ,  $X_e = \{6, 3, 1\}$ ,

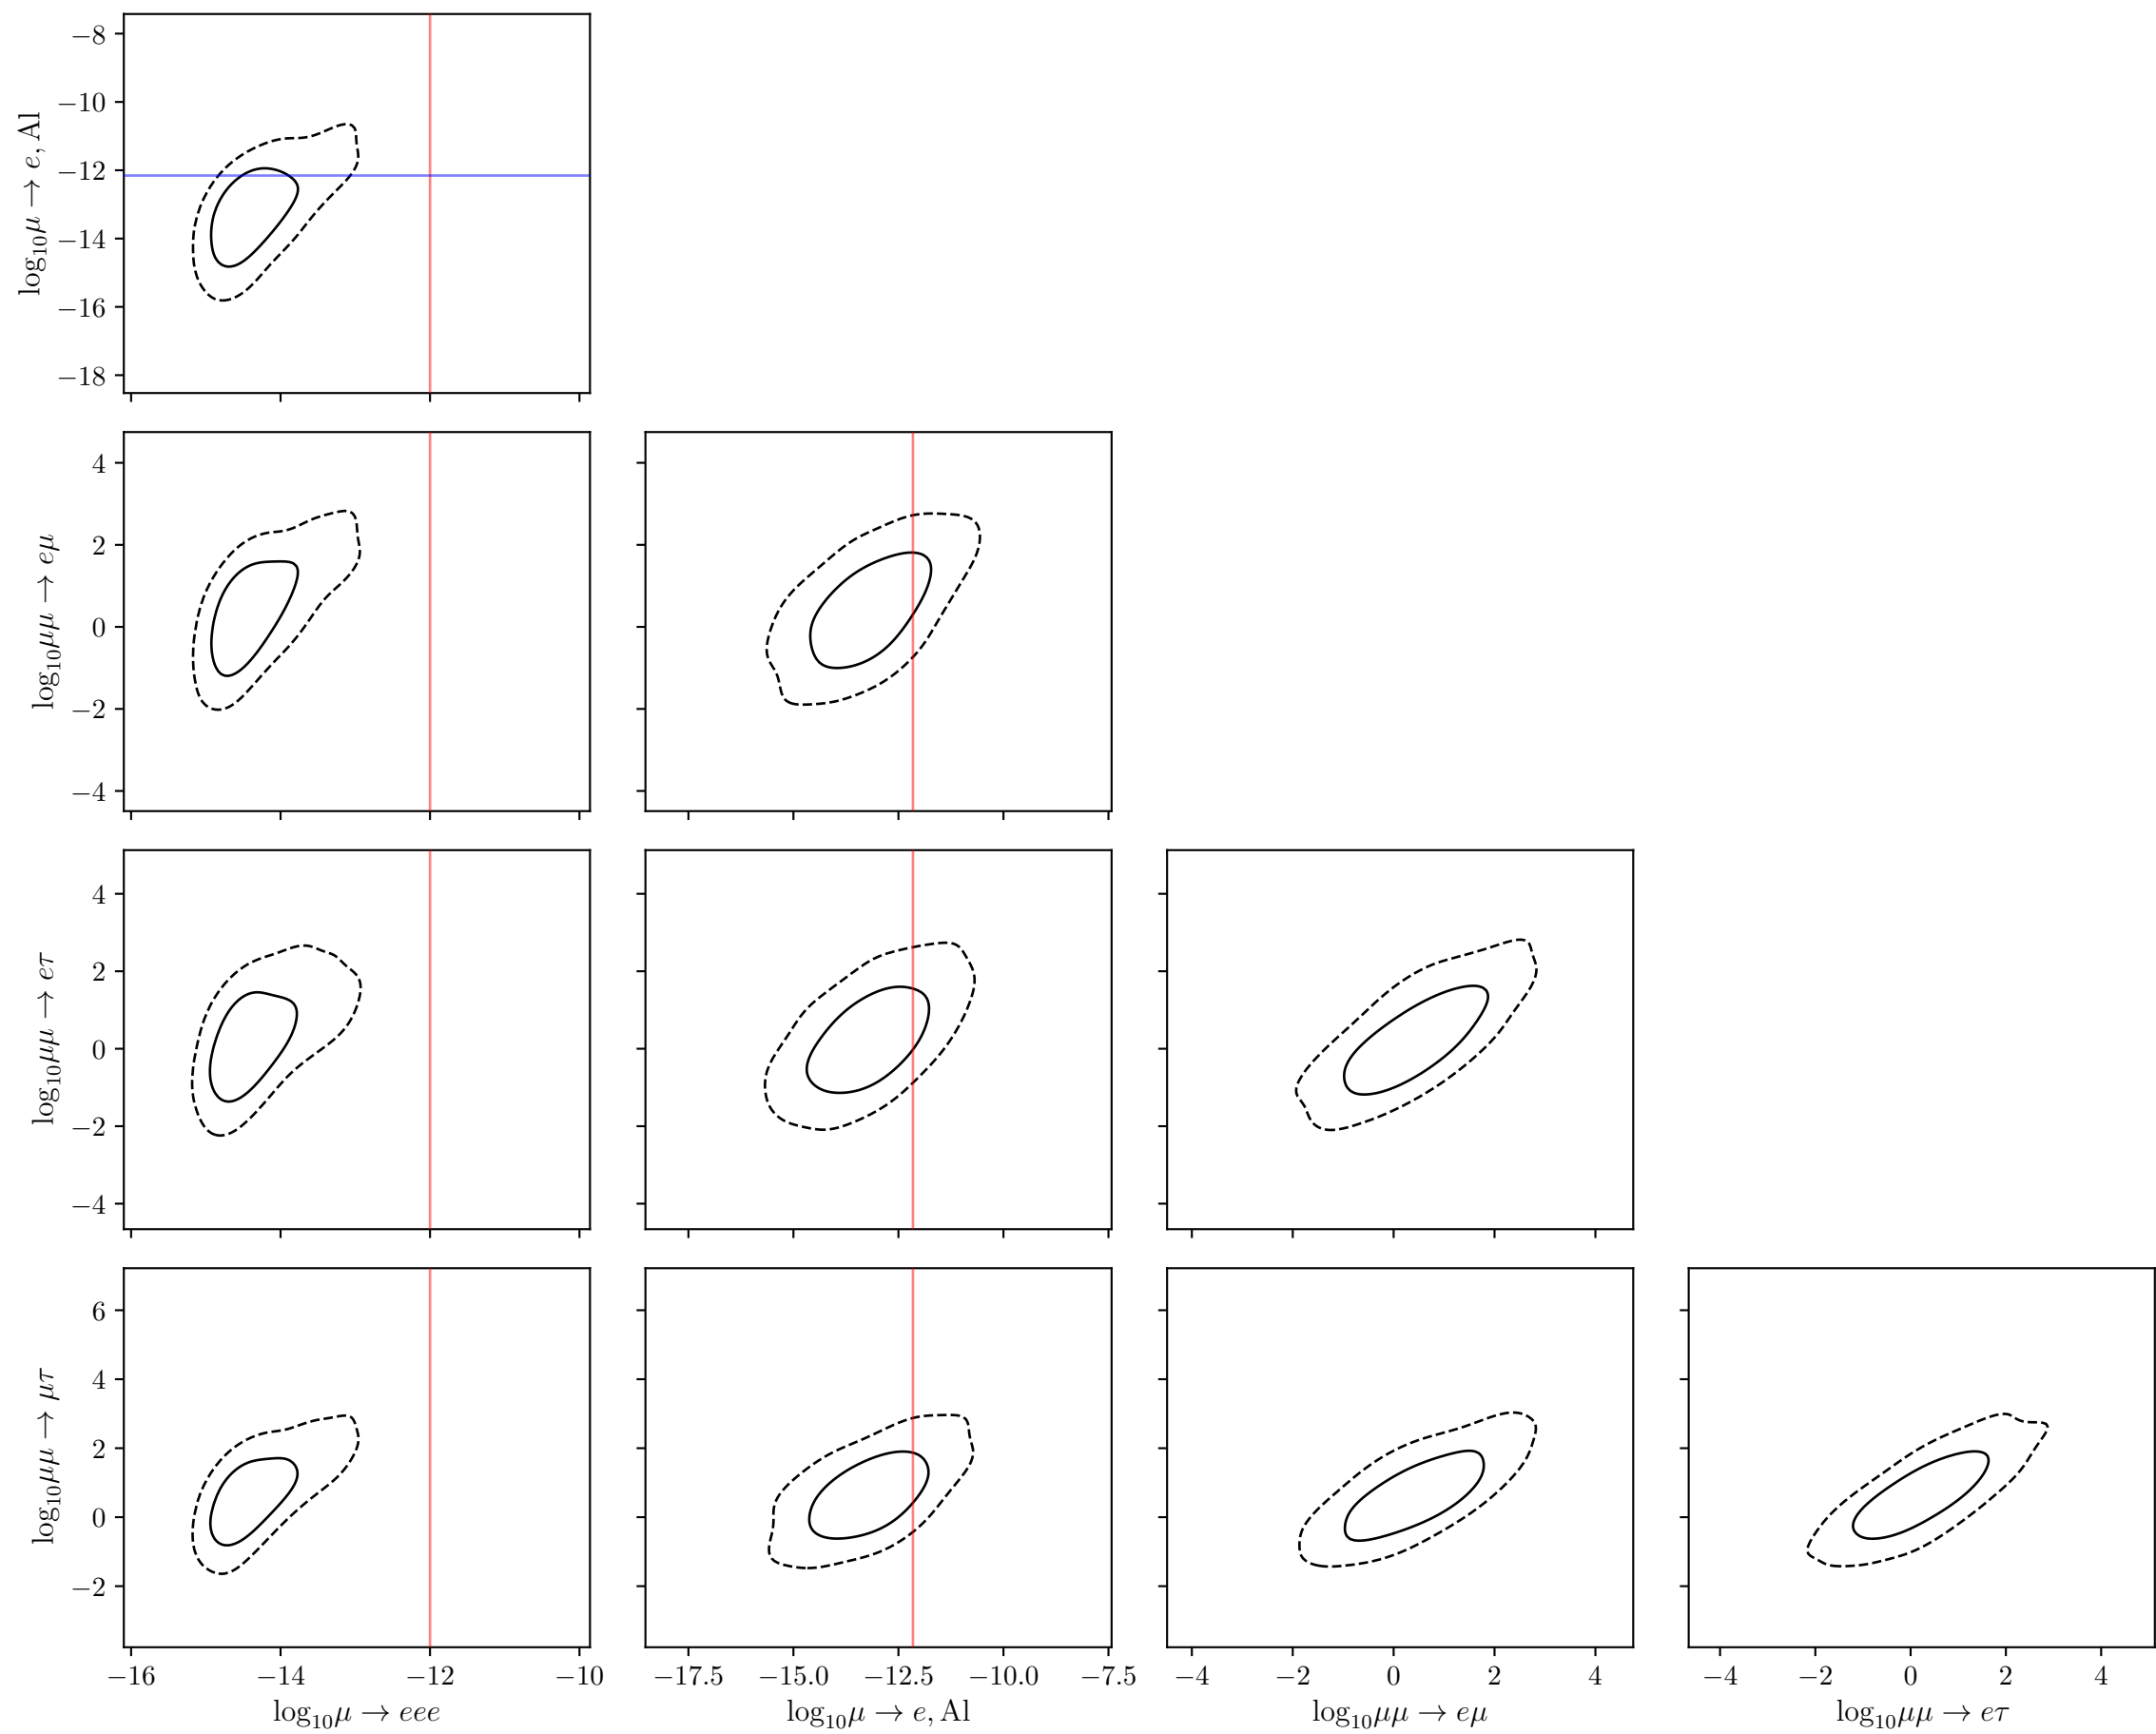

Majorana,  $X_L = \{7, 6, 5\}$ ,  $X_e = \{-1, 1, 5\}$ ,

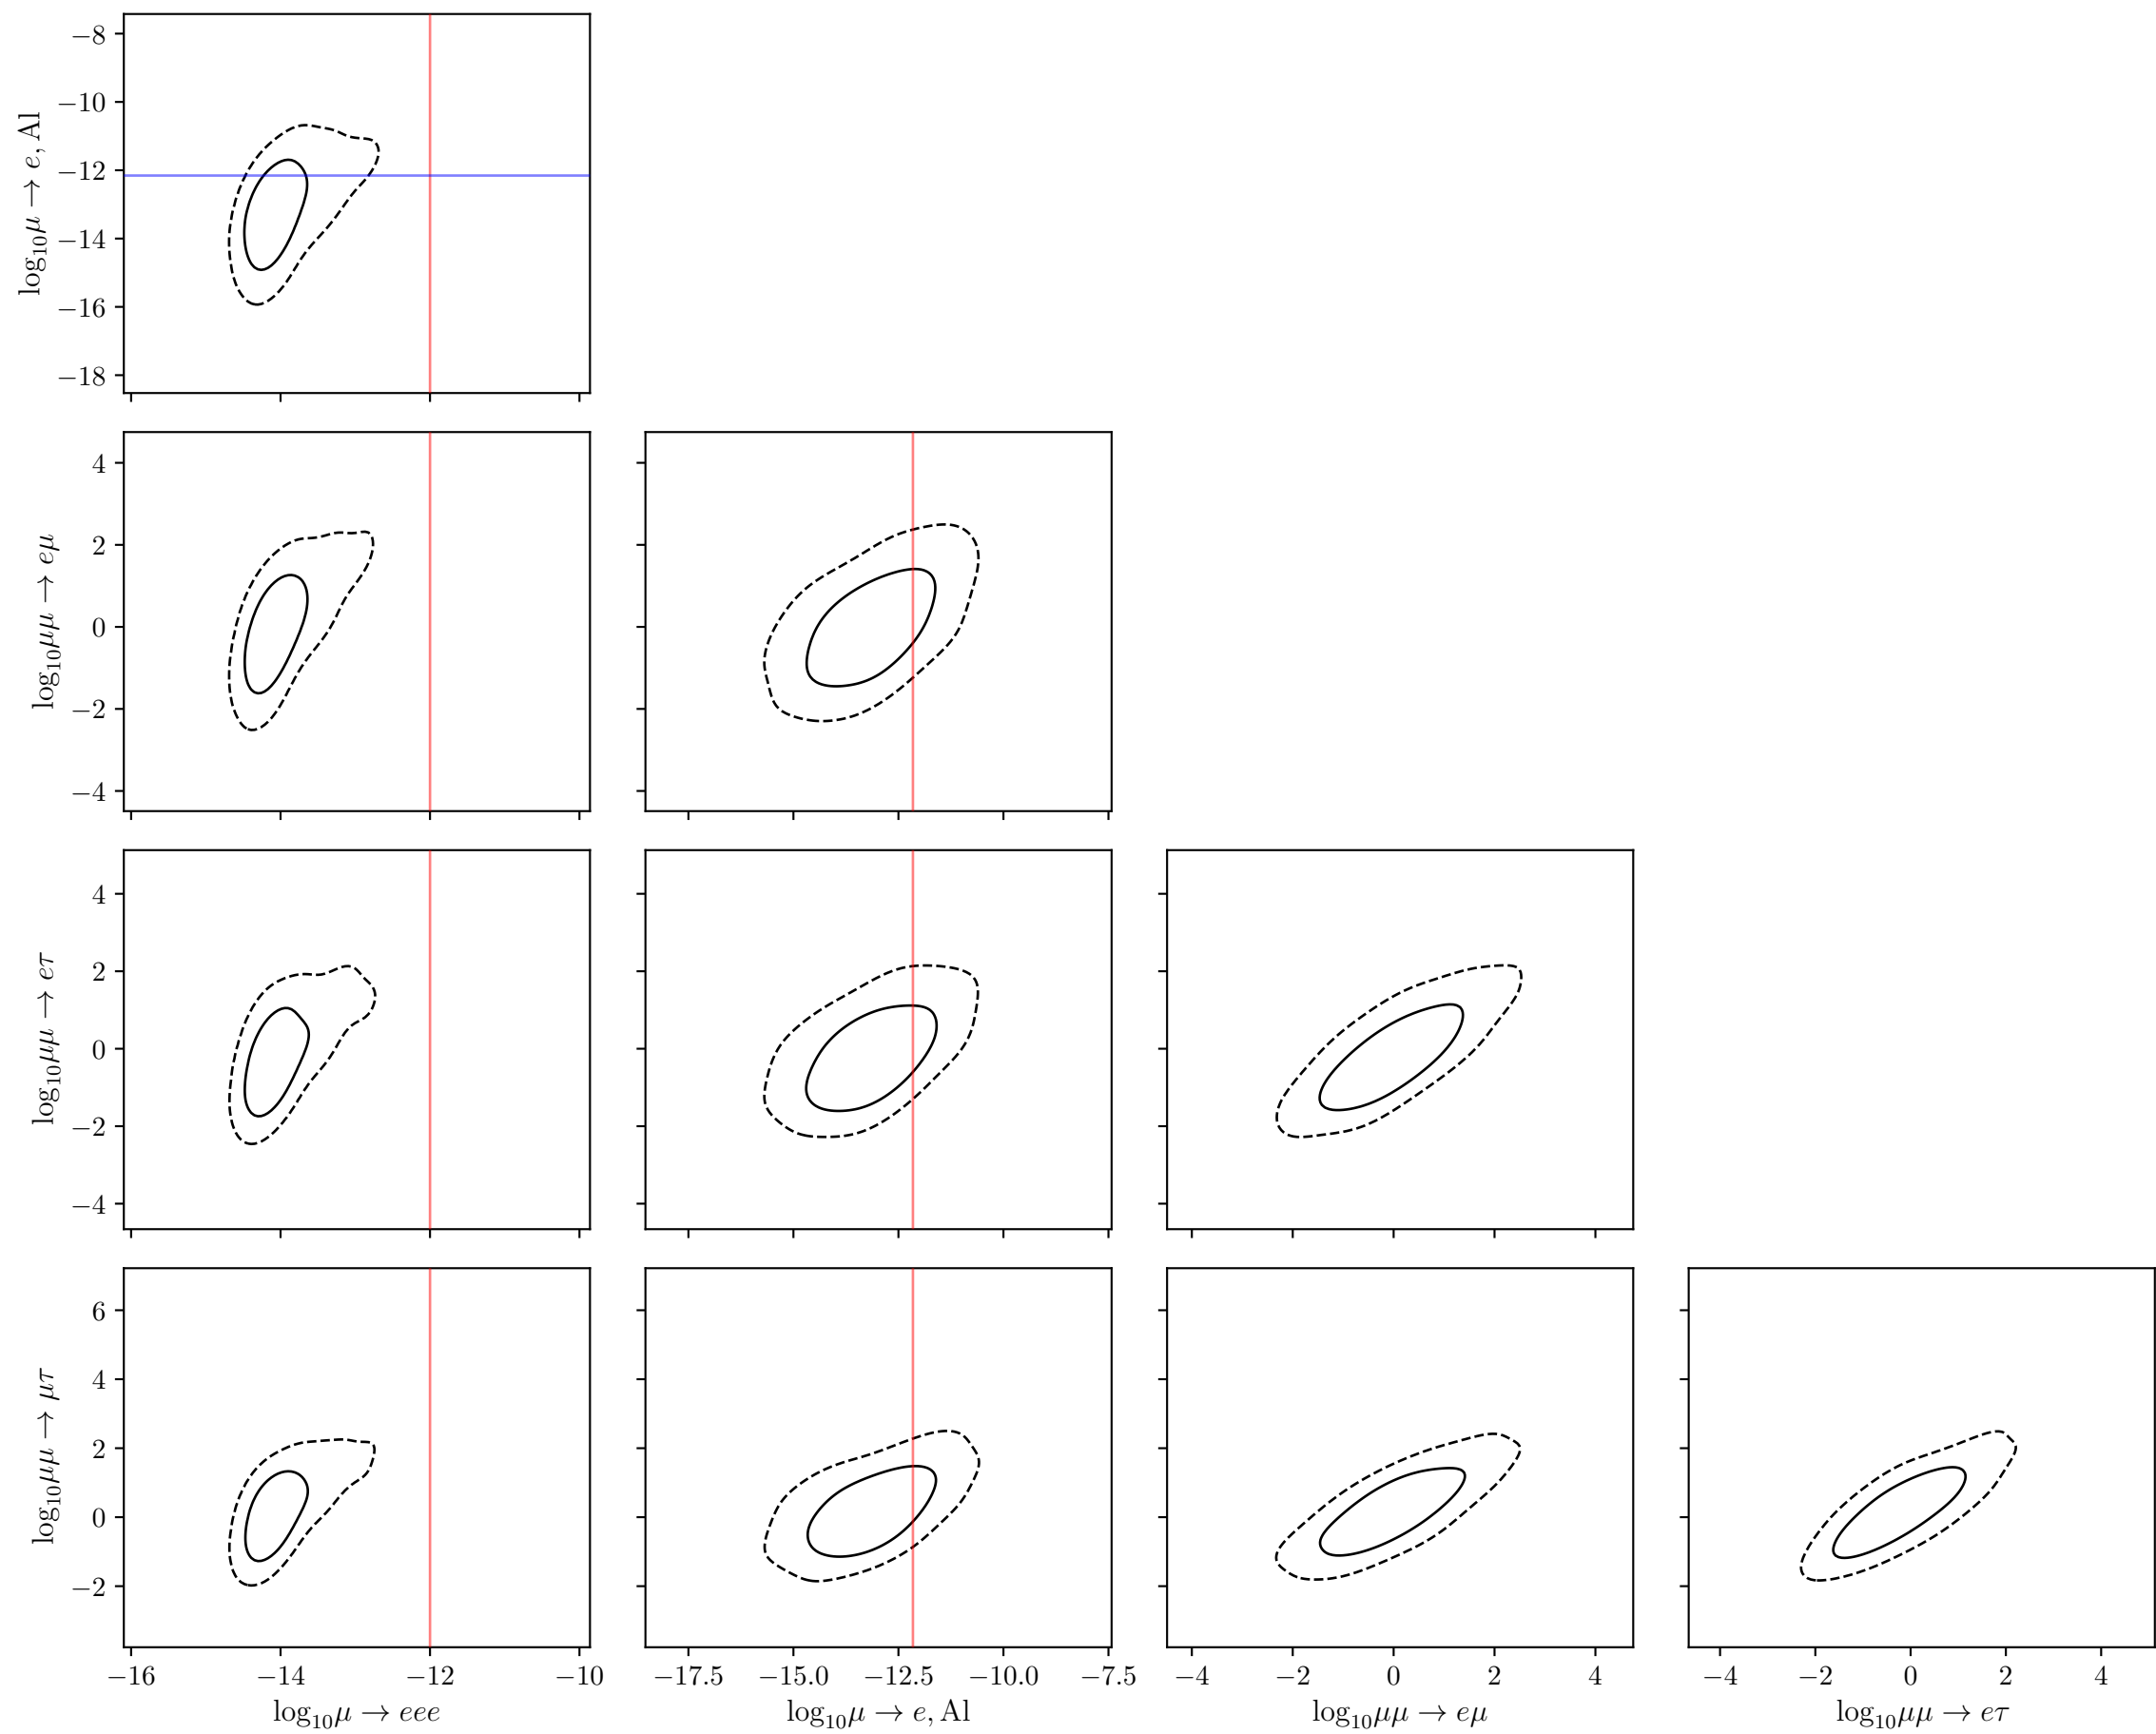

Majorana,  $X_L = \{7, 6, 5\}$ ,  $X_e = \{-1, 2, 5\}$ ,

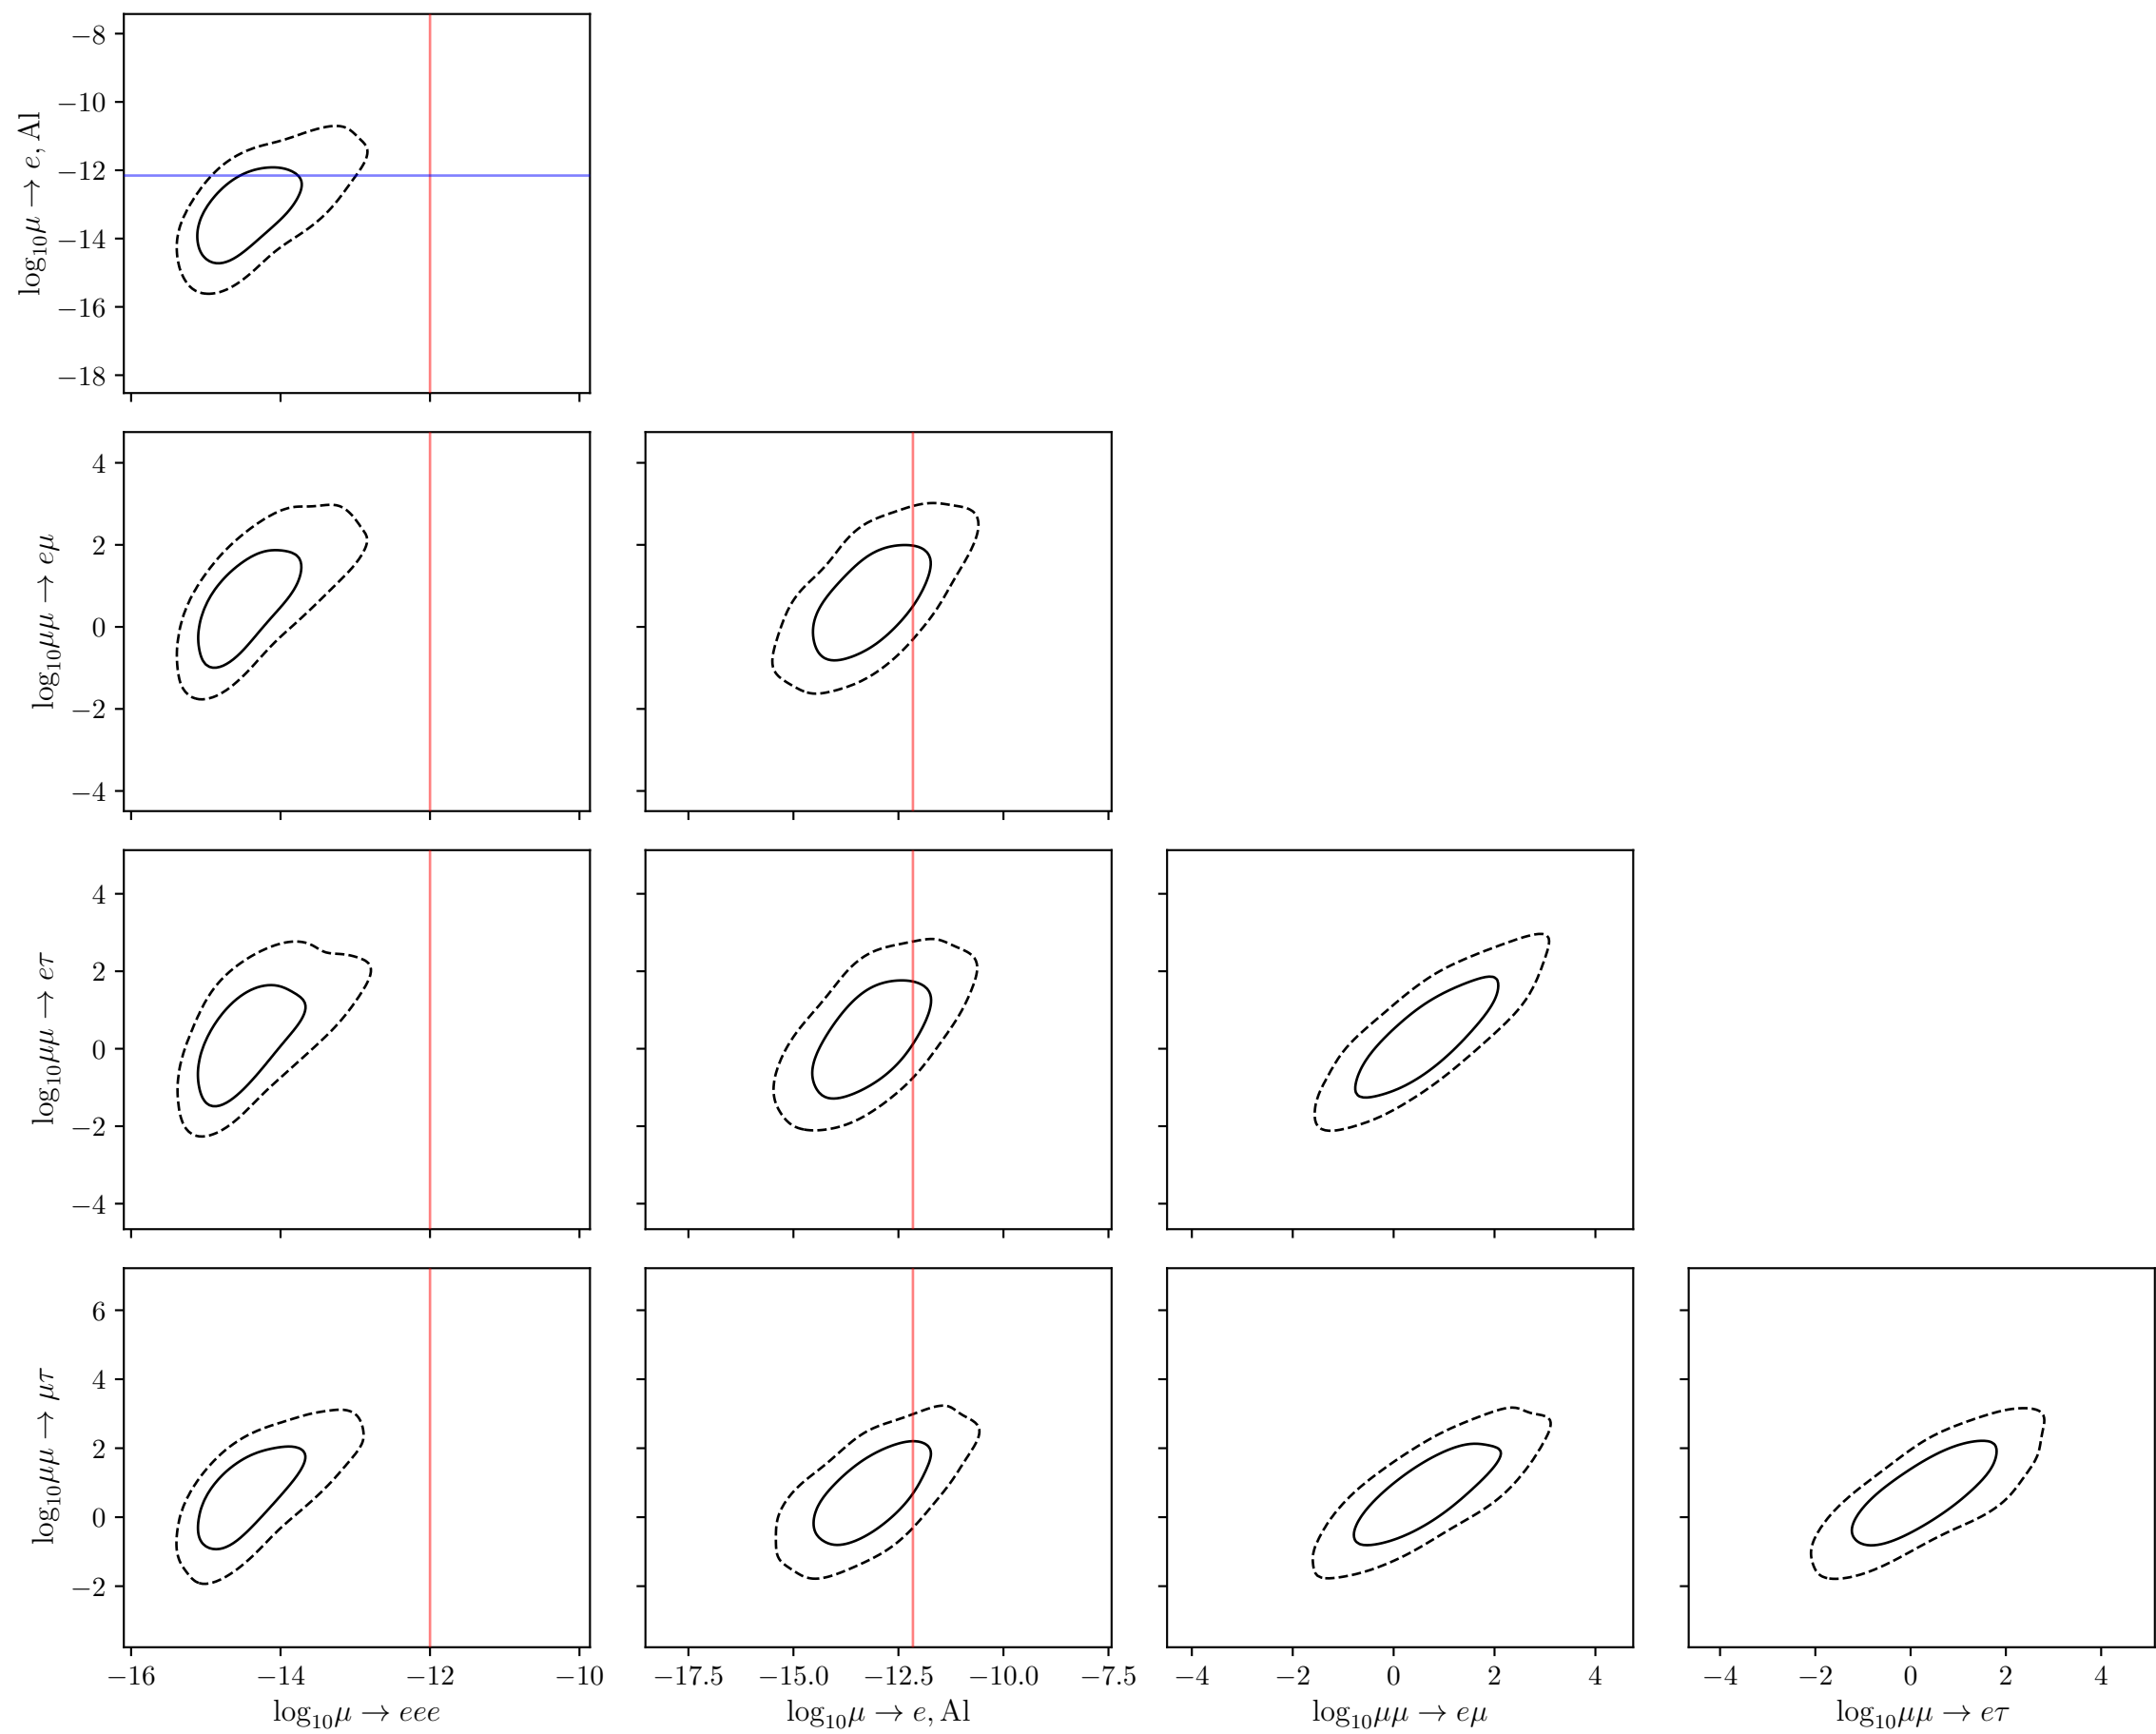

Majorana,  $X_L = \{6, 6, 5\}$ ,  $X_e = \{-2, 0, 3\}$ ,

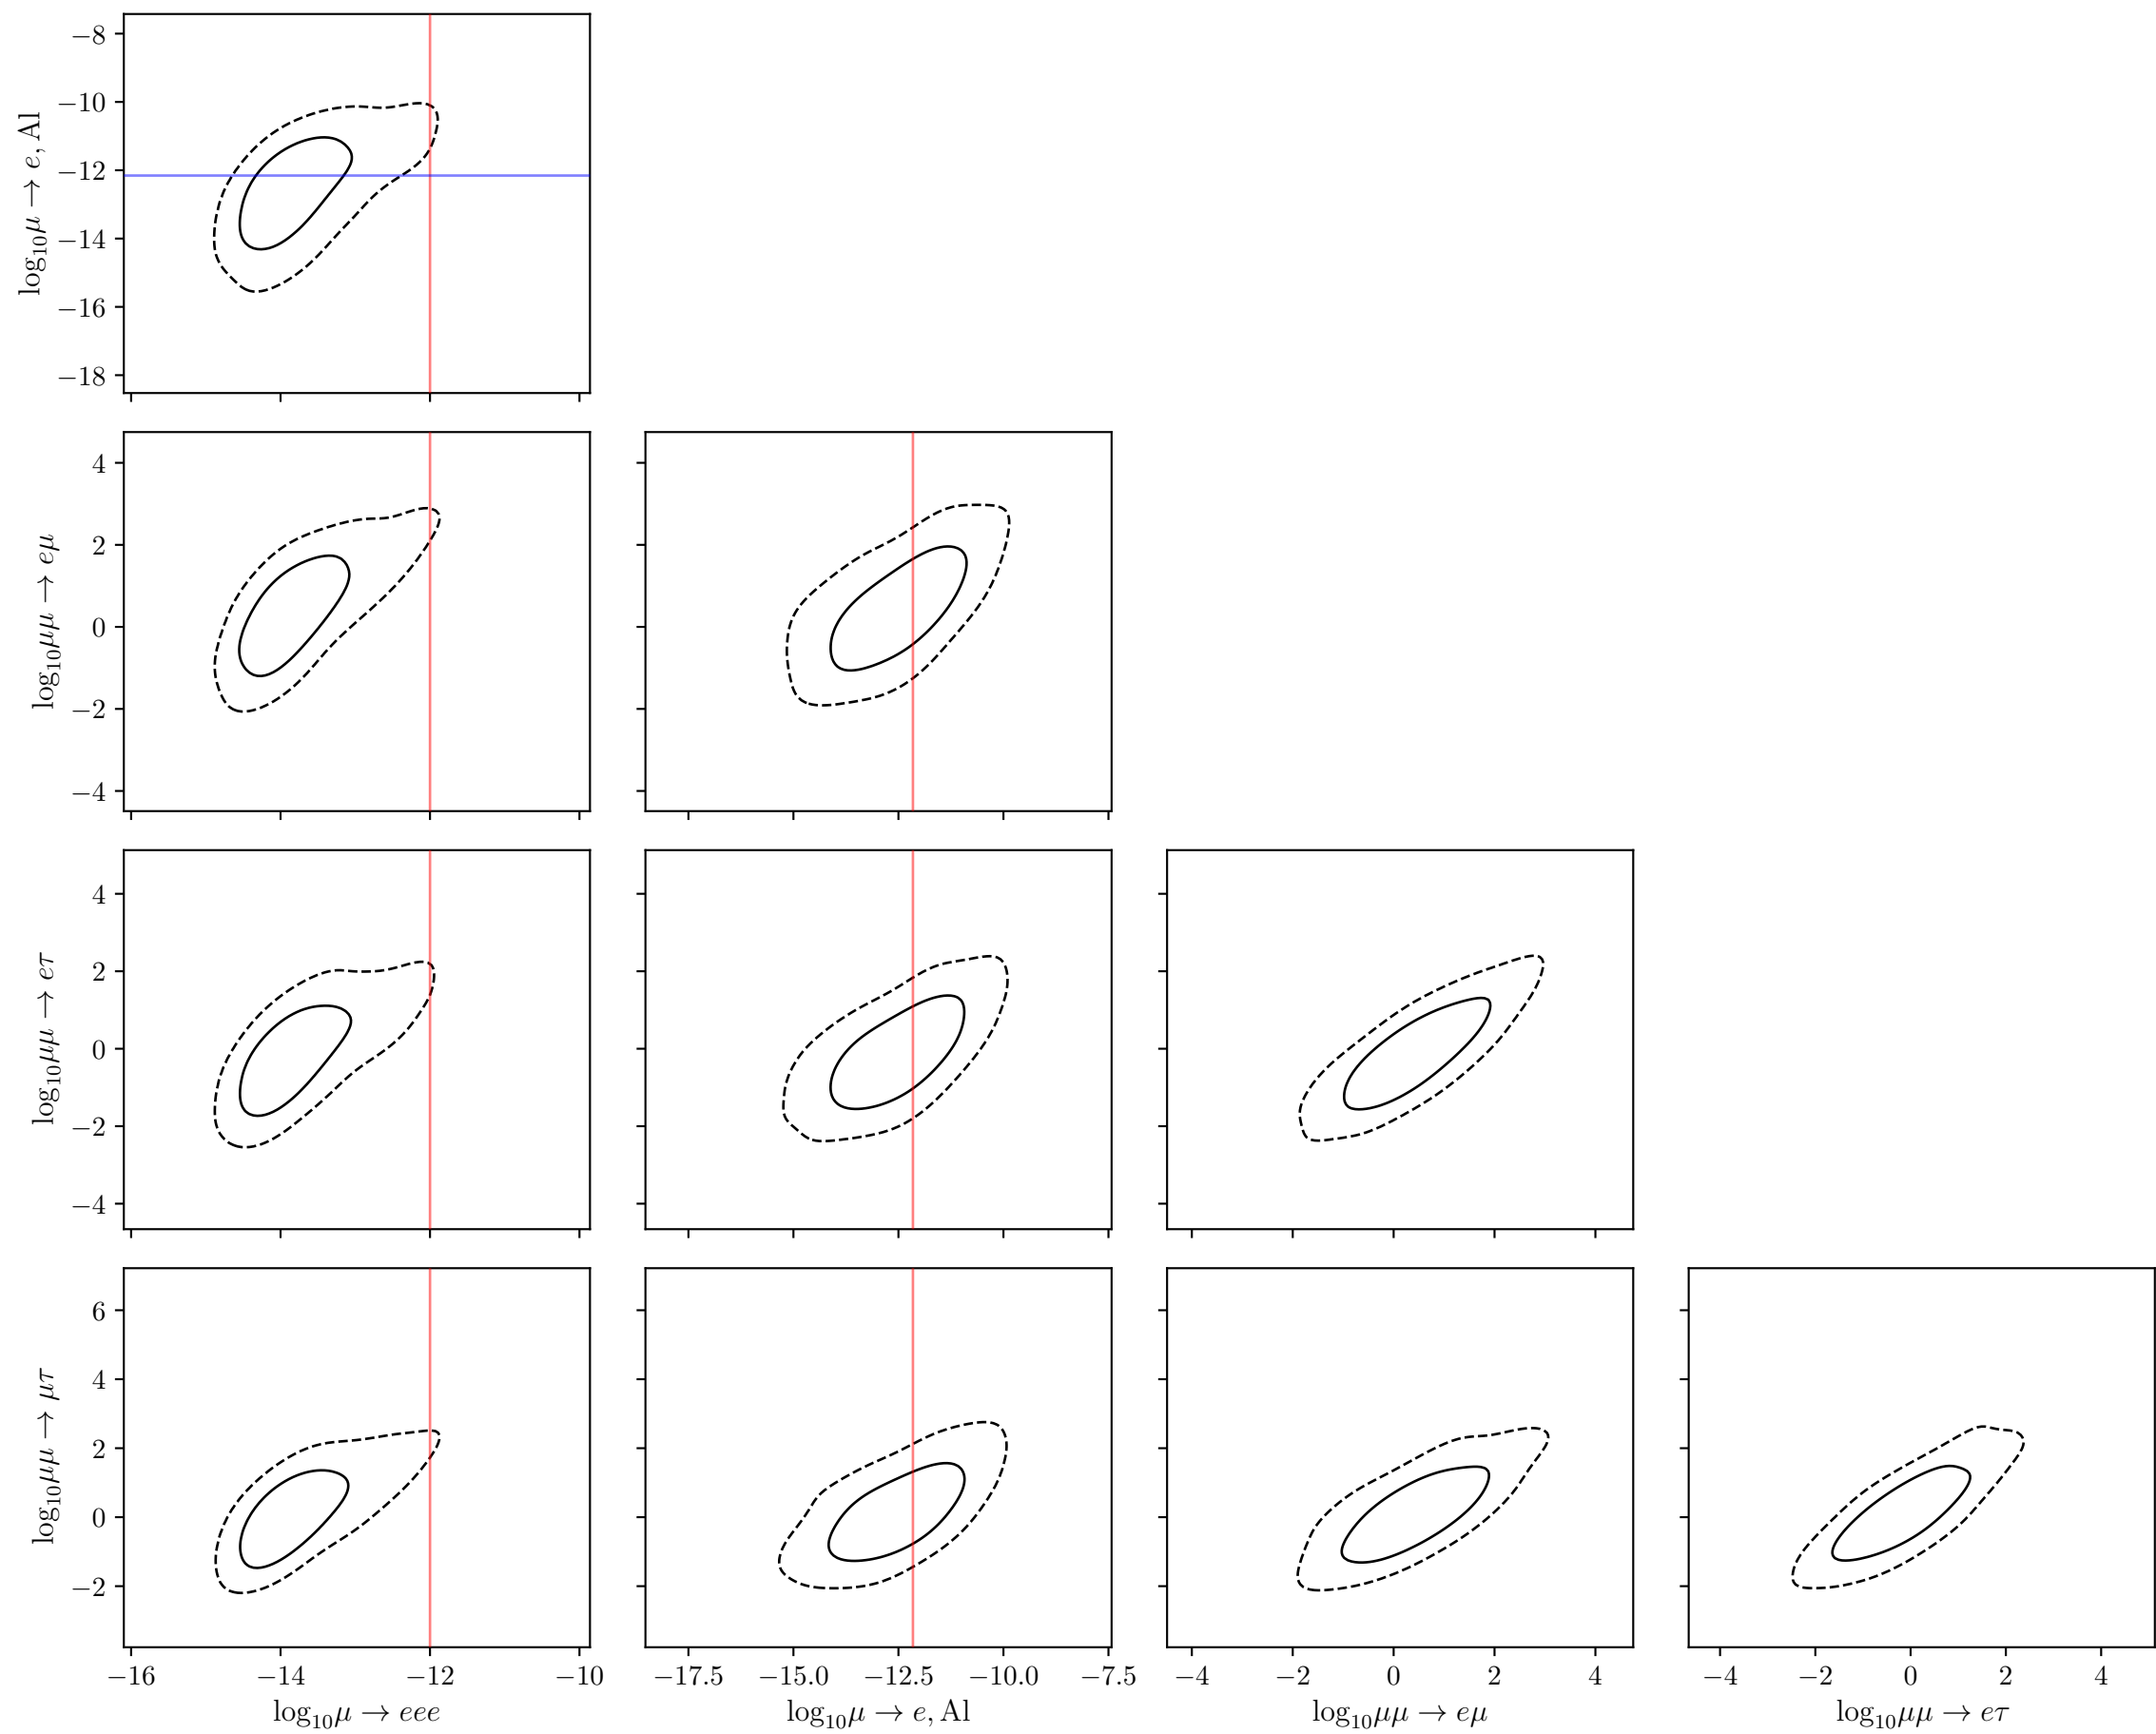

Majorana,  $X_L = \{6, 6, 5\}$ ,  $X_e = \{-1, 2, 6\}$ ,

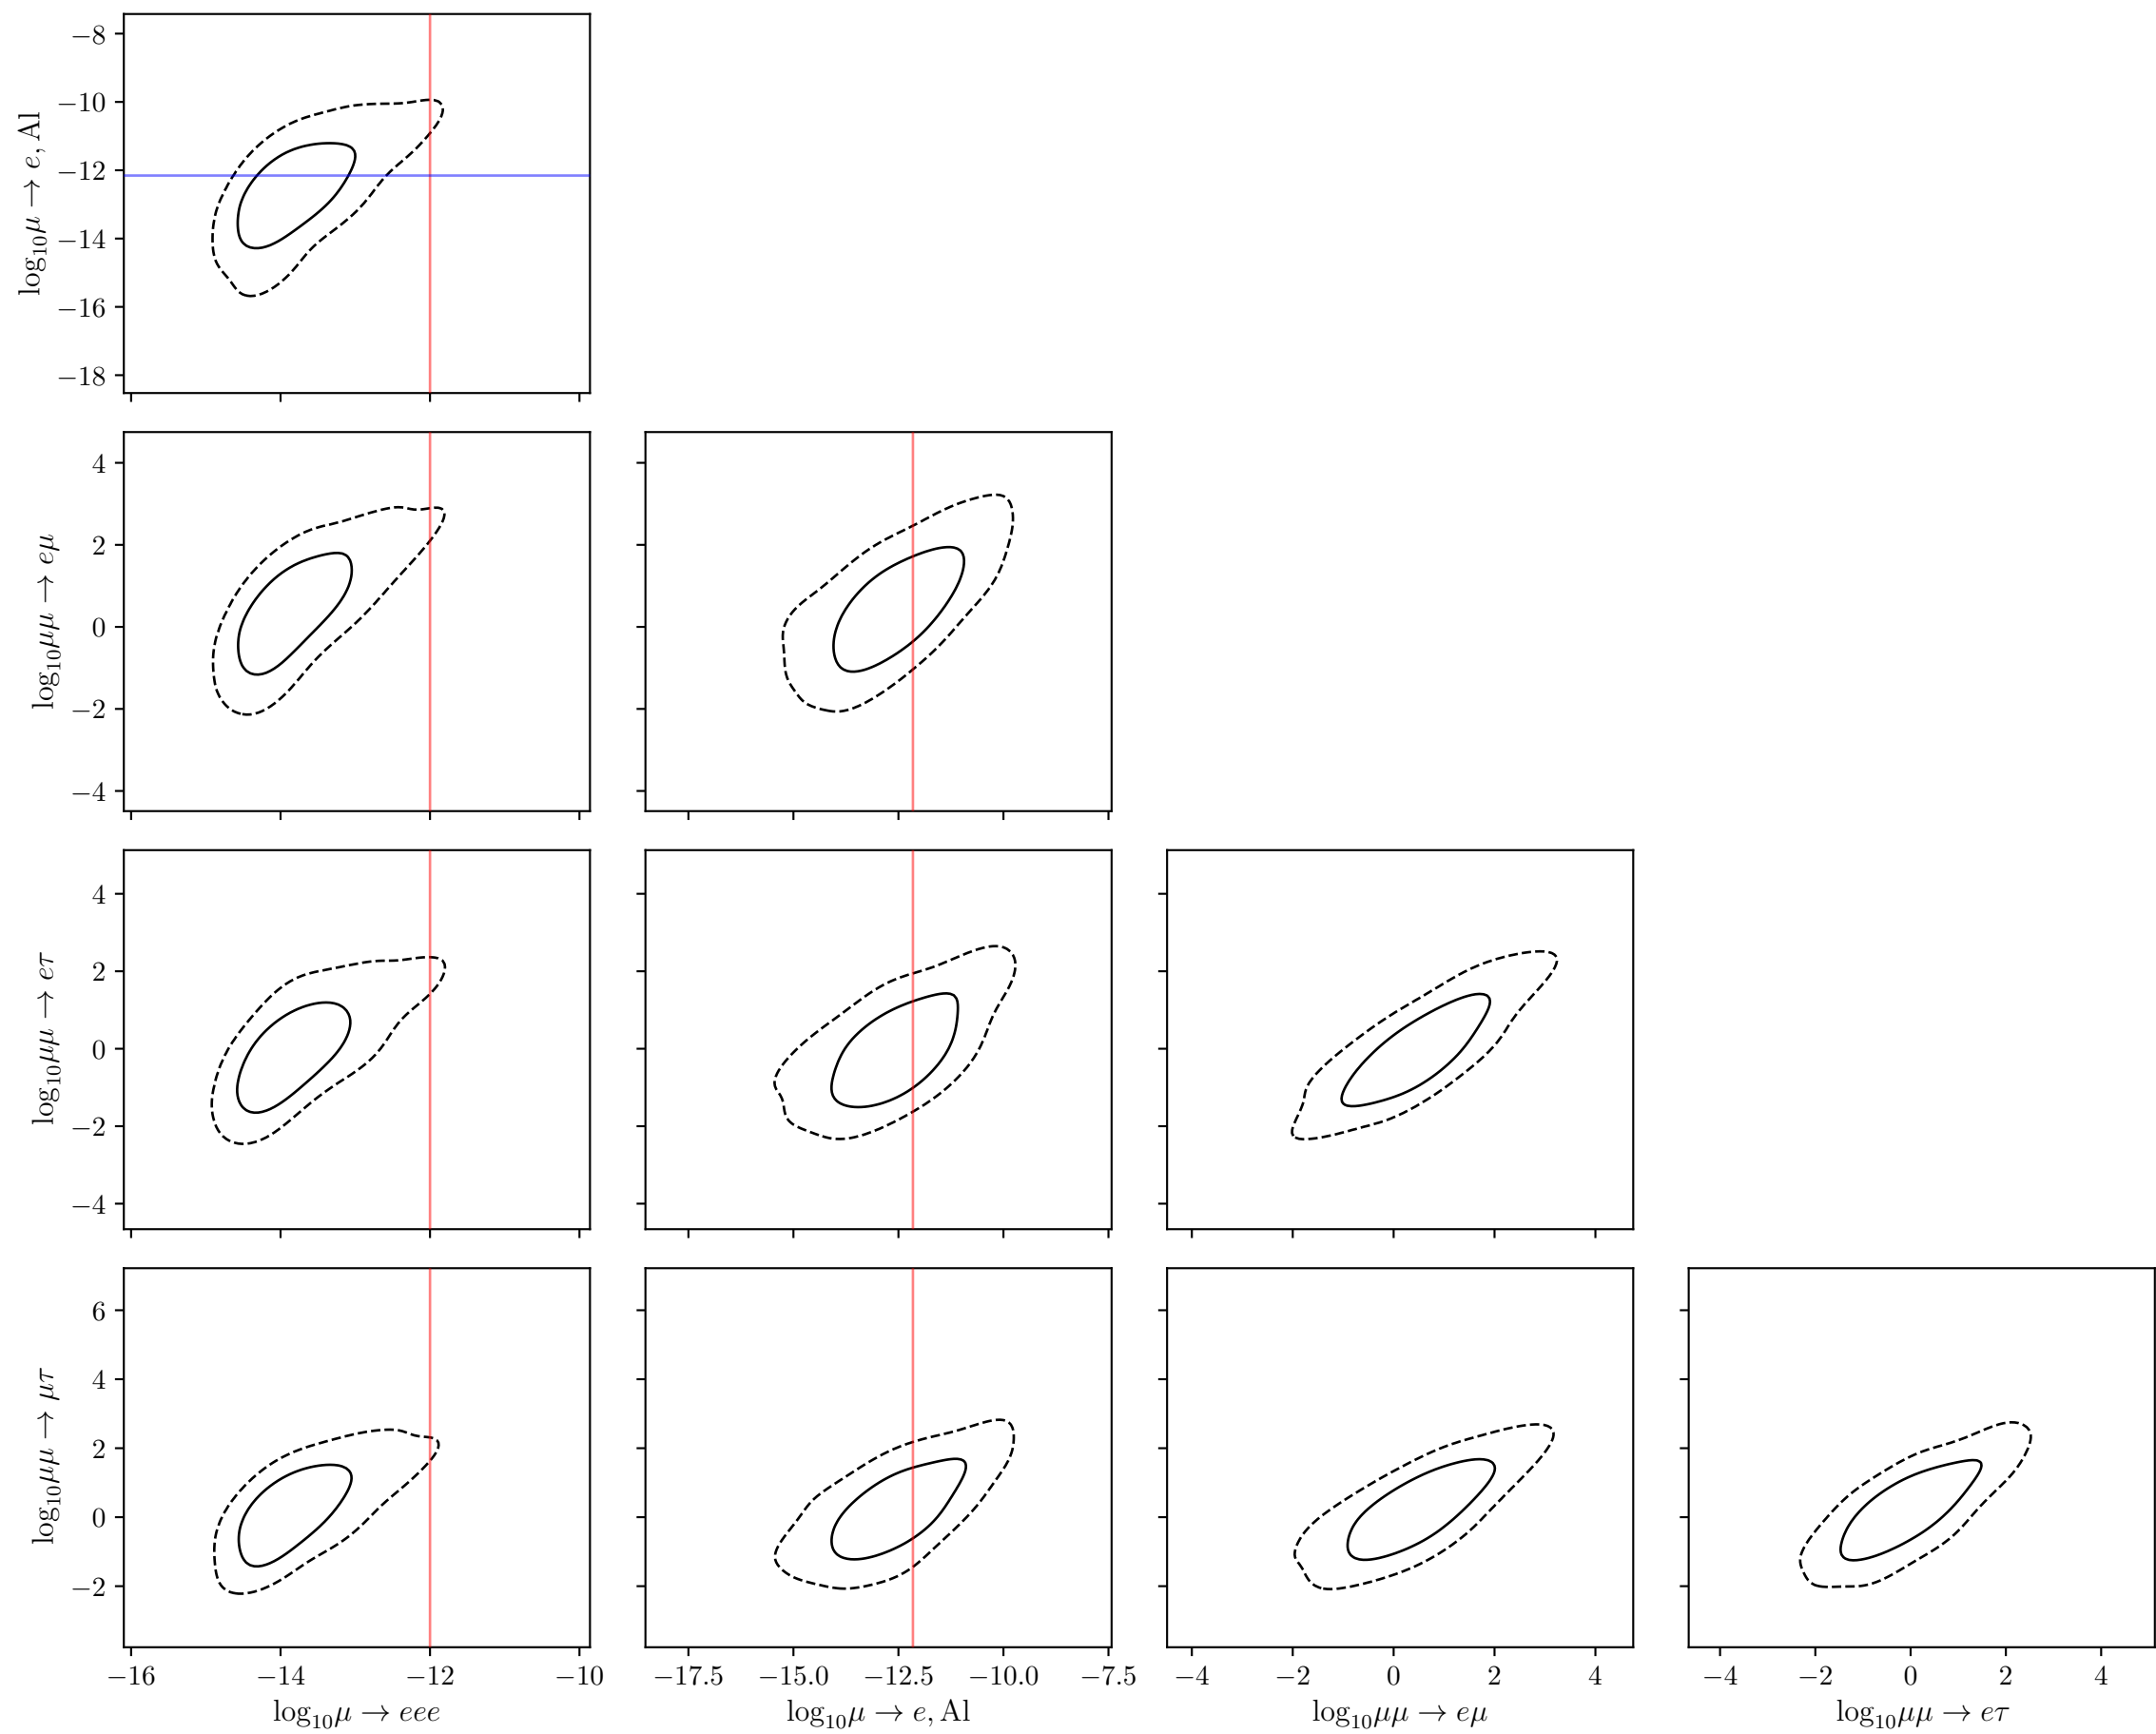

Majorana,  $X_L = \{5, 5, 4\}$ ,  $X_e = \{6, 3, 0\}$ ,

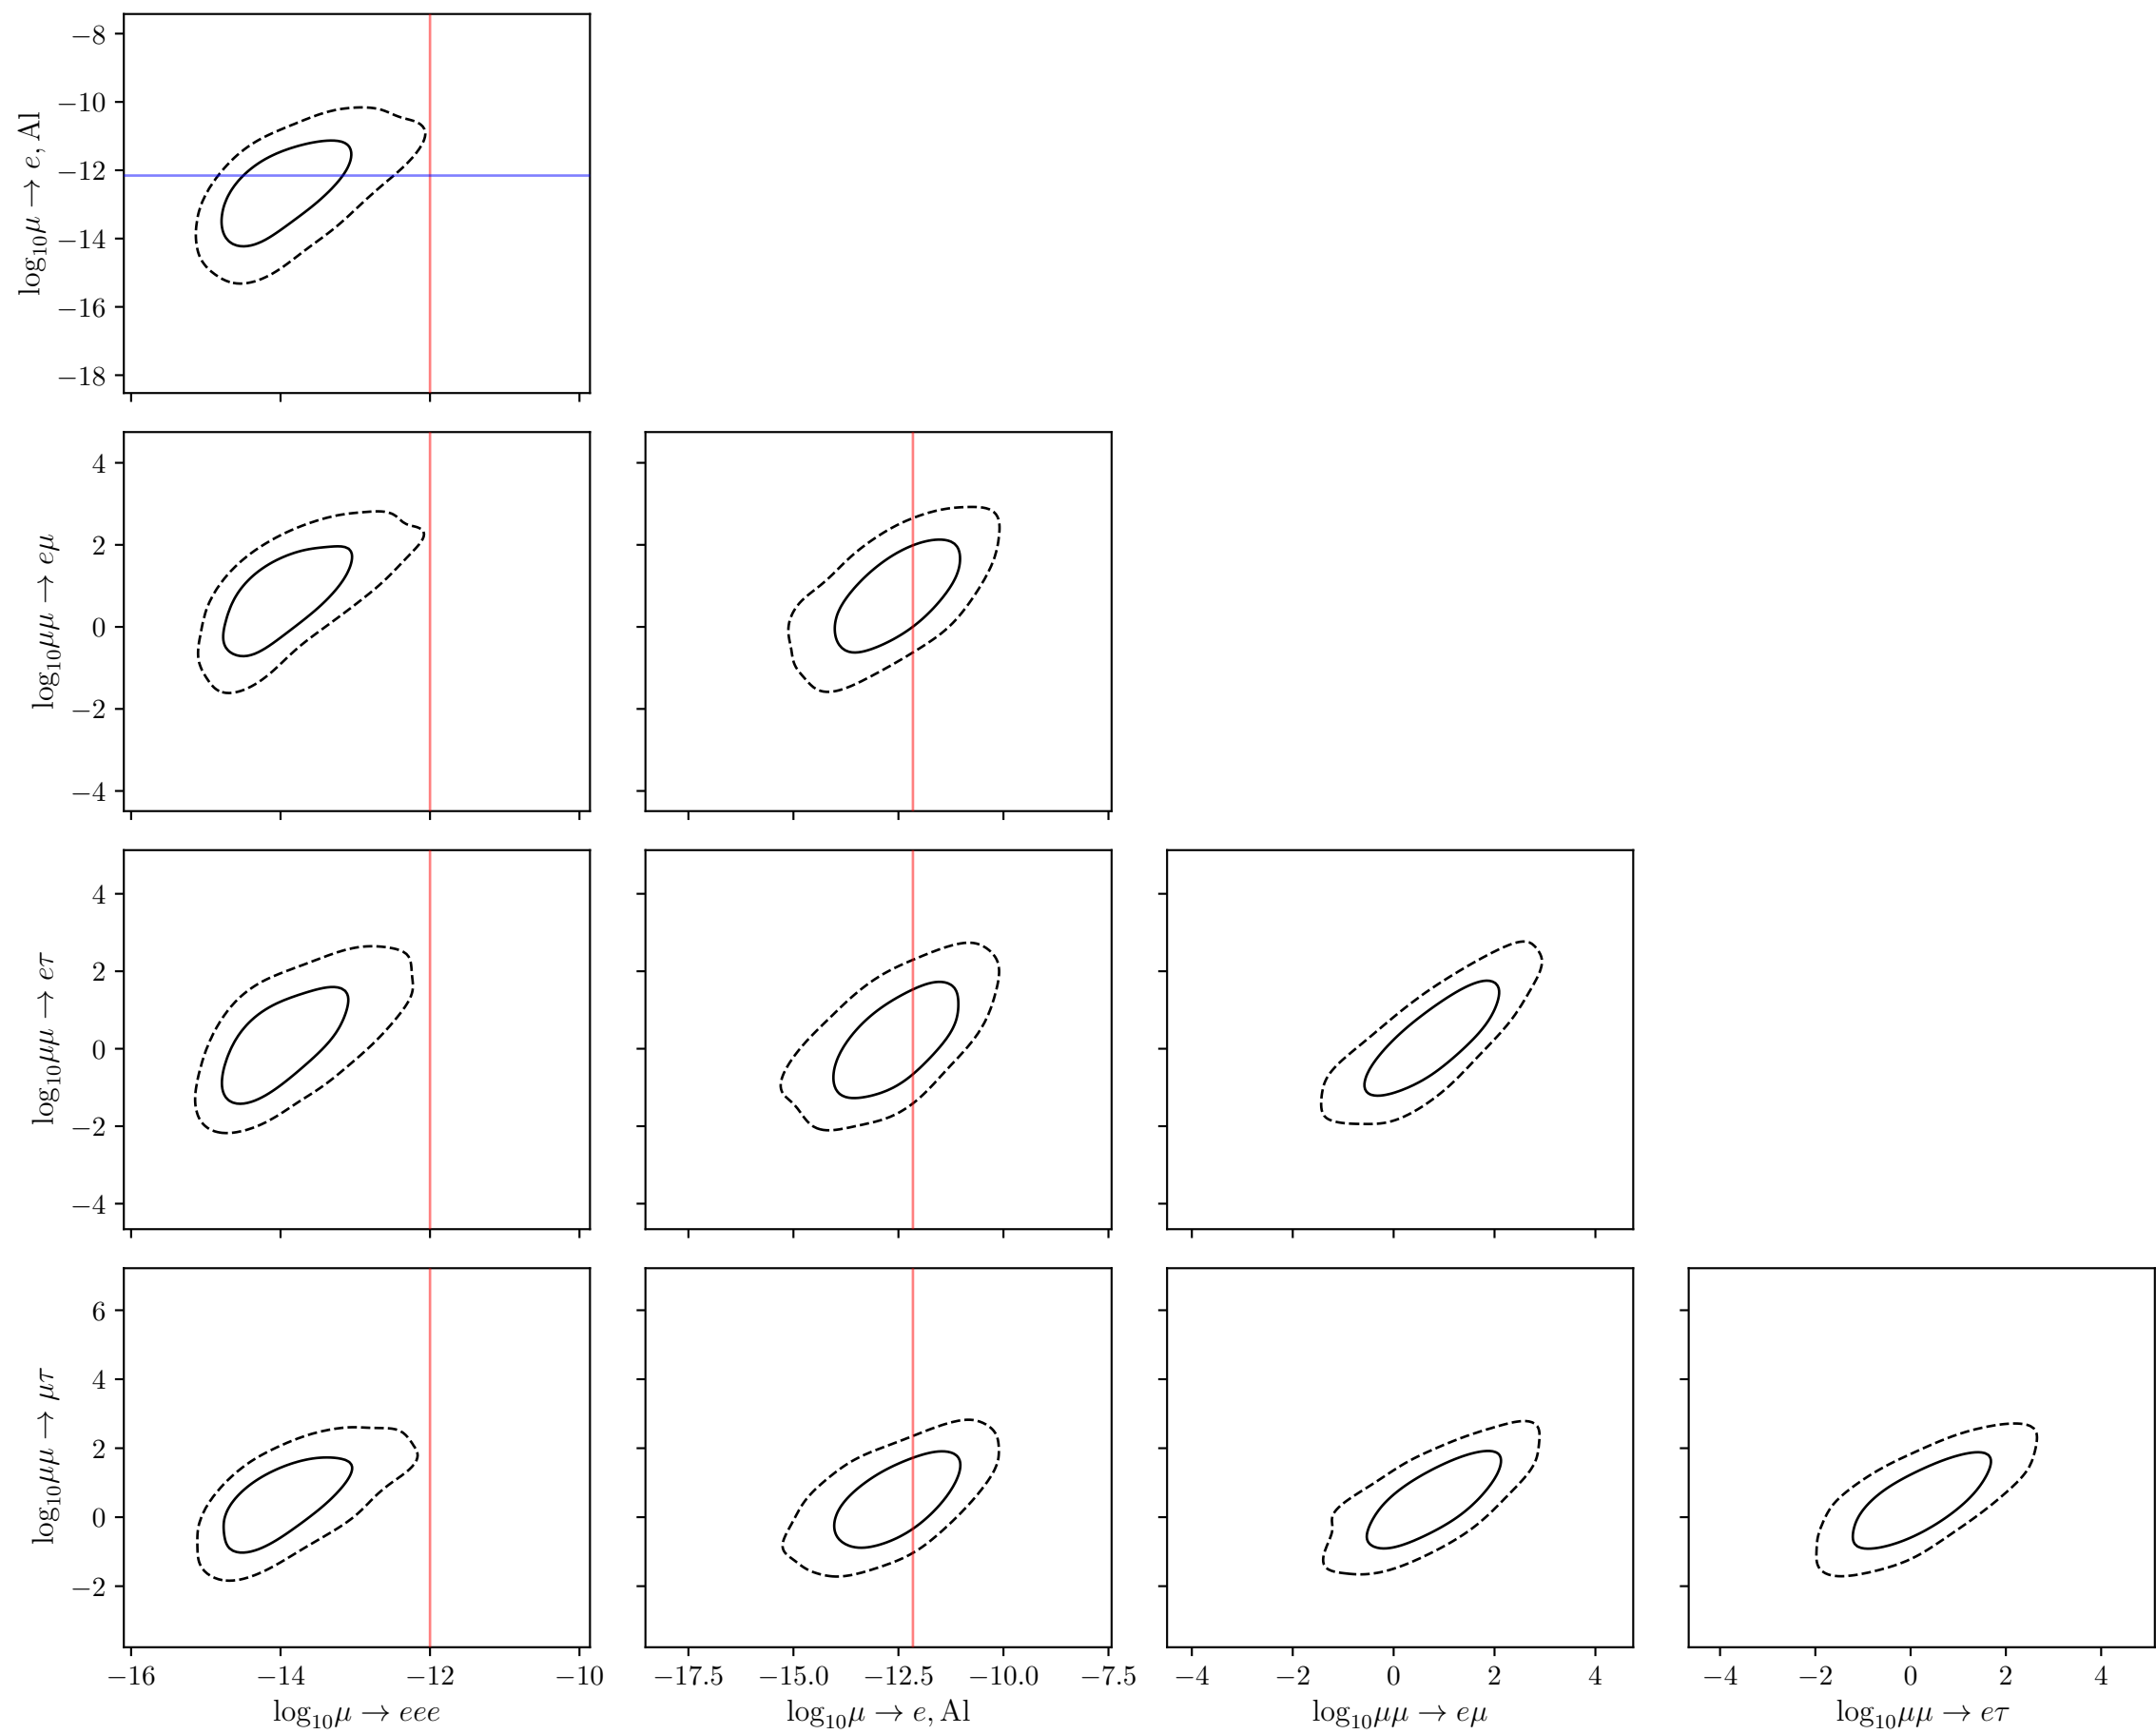



Majorana,  $X_L = \{6, 5, 4\}$ ,  $X_e = \{7, 4, 1\}$ ,

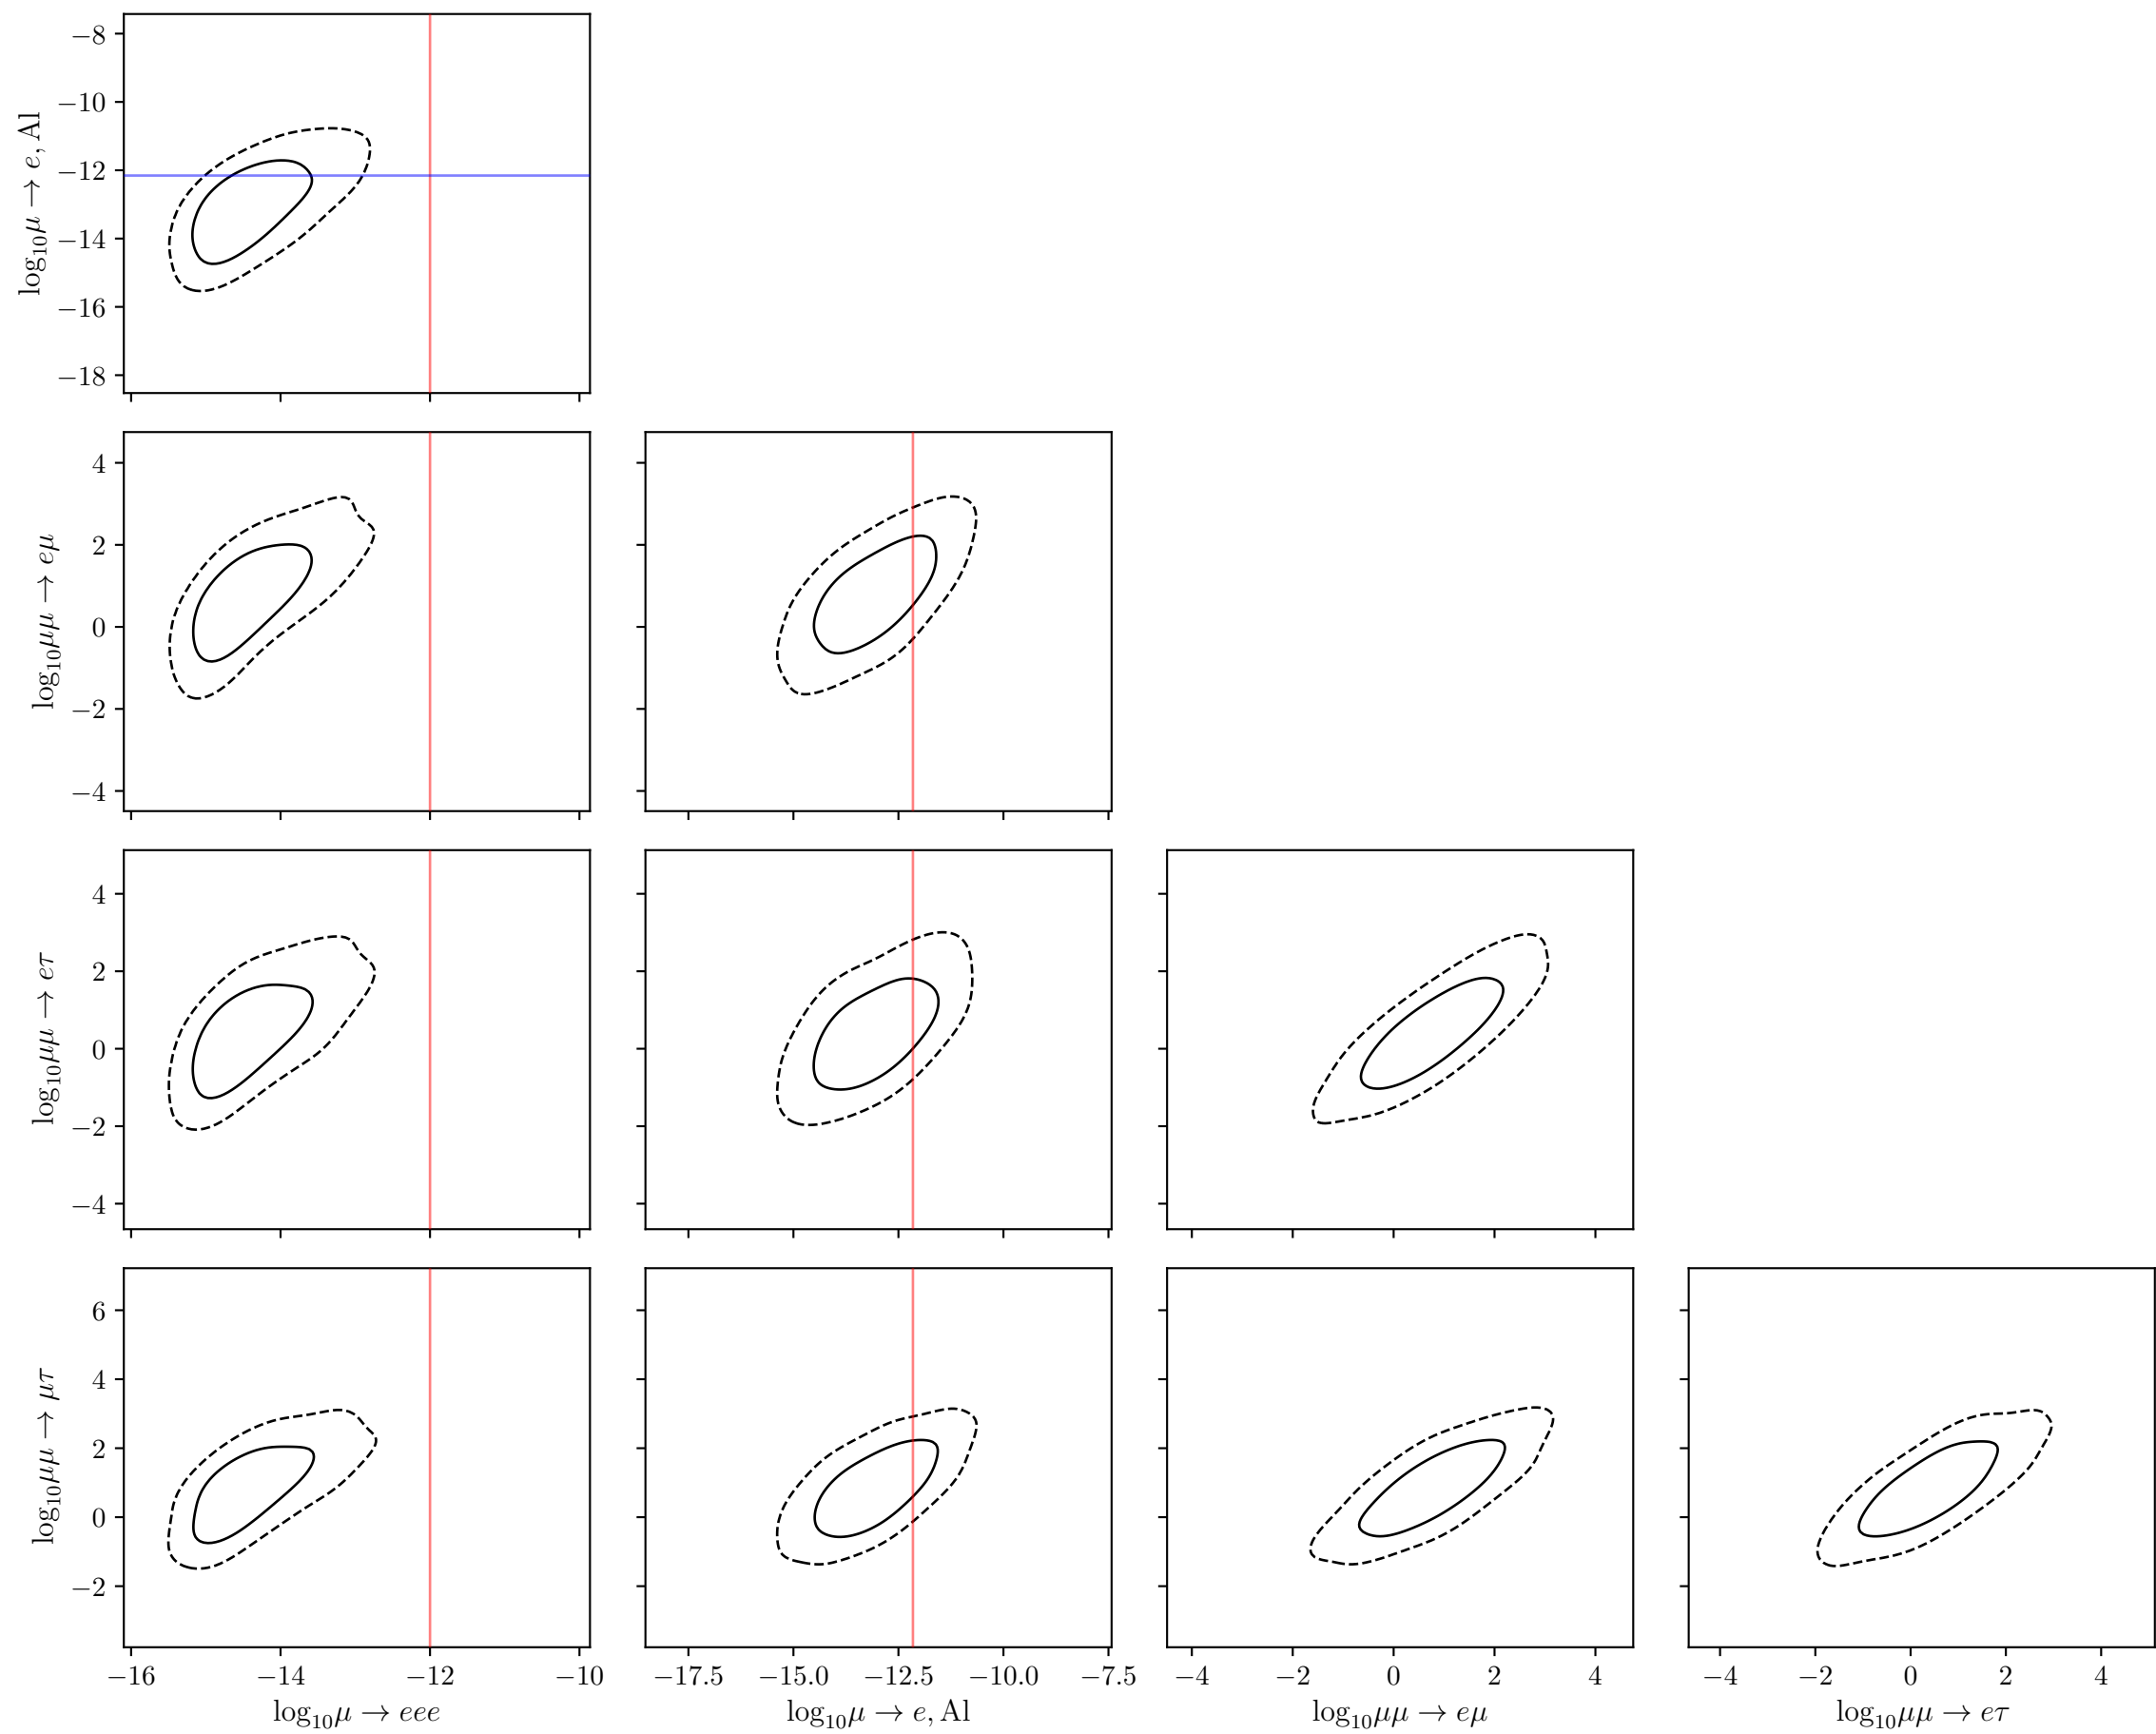

Majorana,  $X_L = \{7, 7, 6\}$ ,  $X_e = \{-1, 1, 6\}$ ,

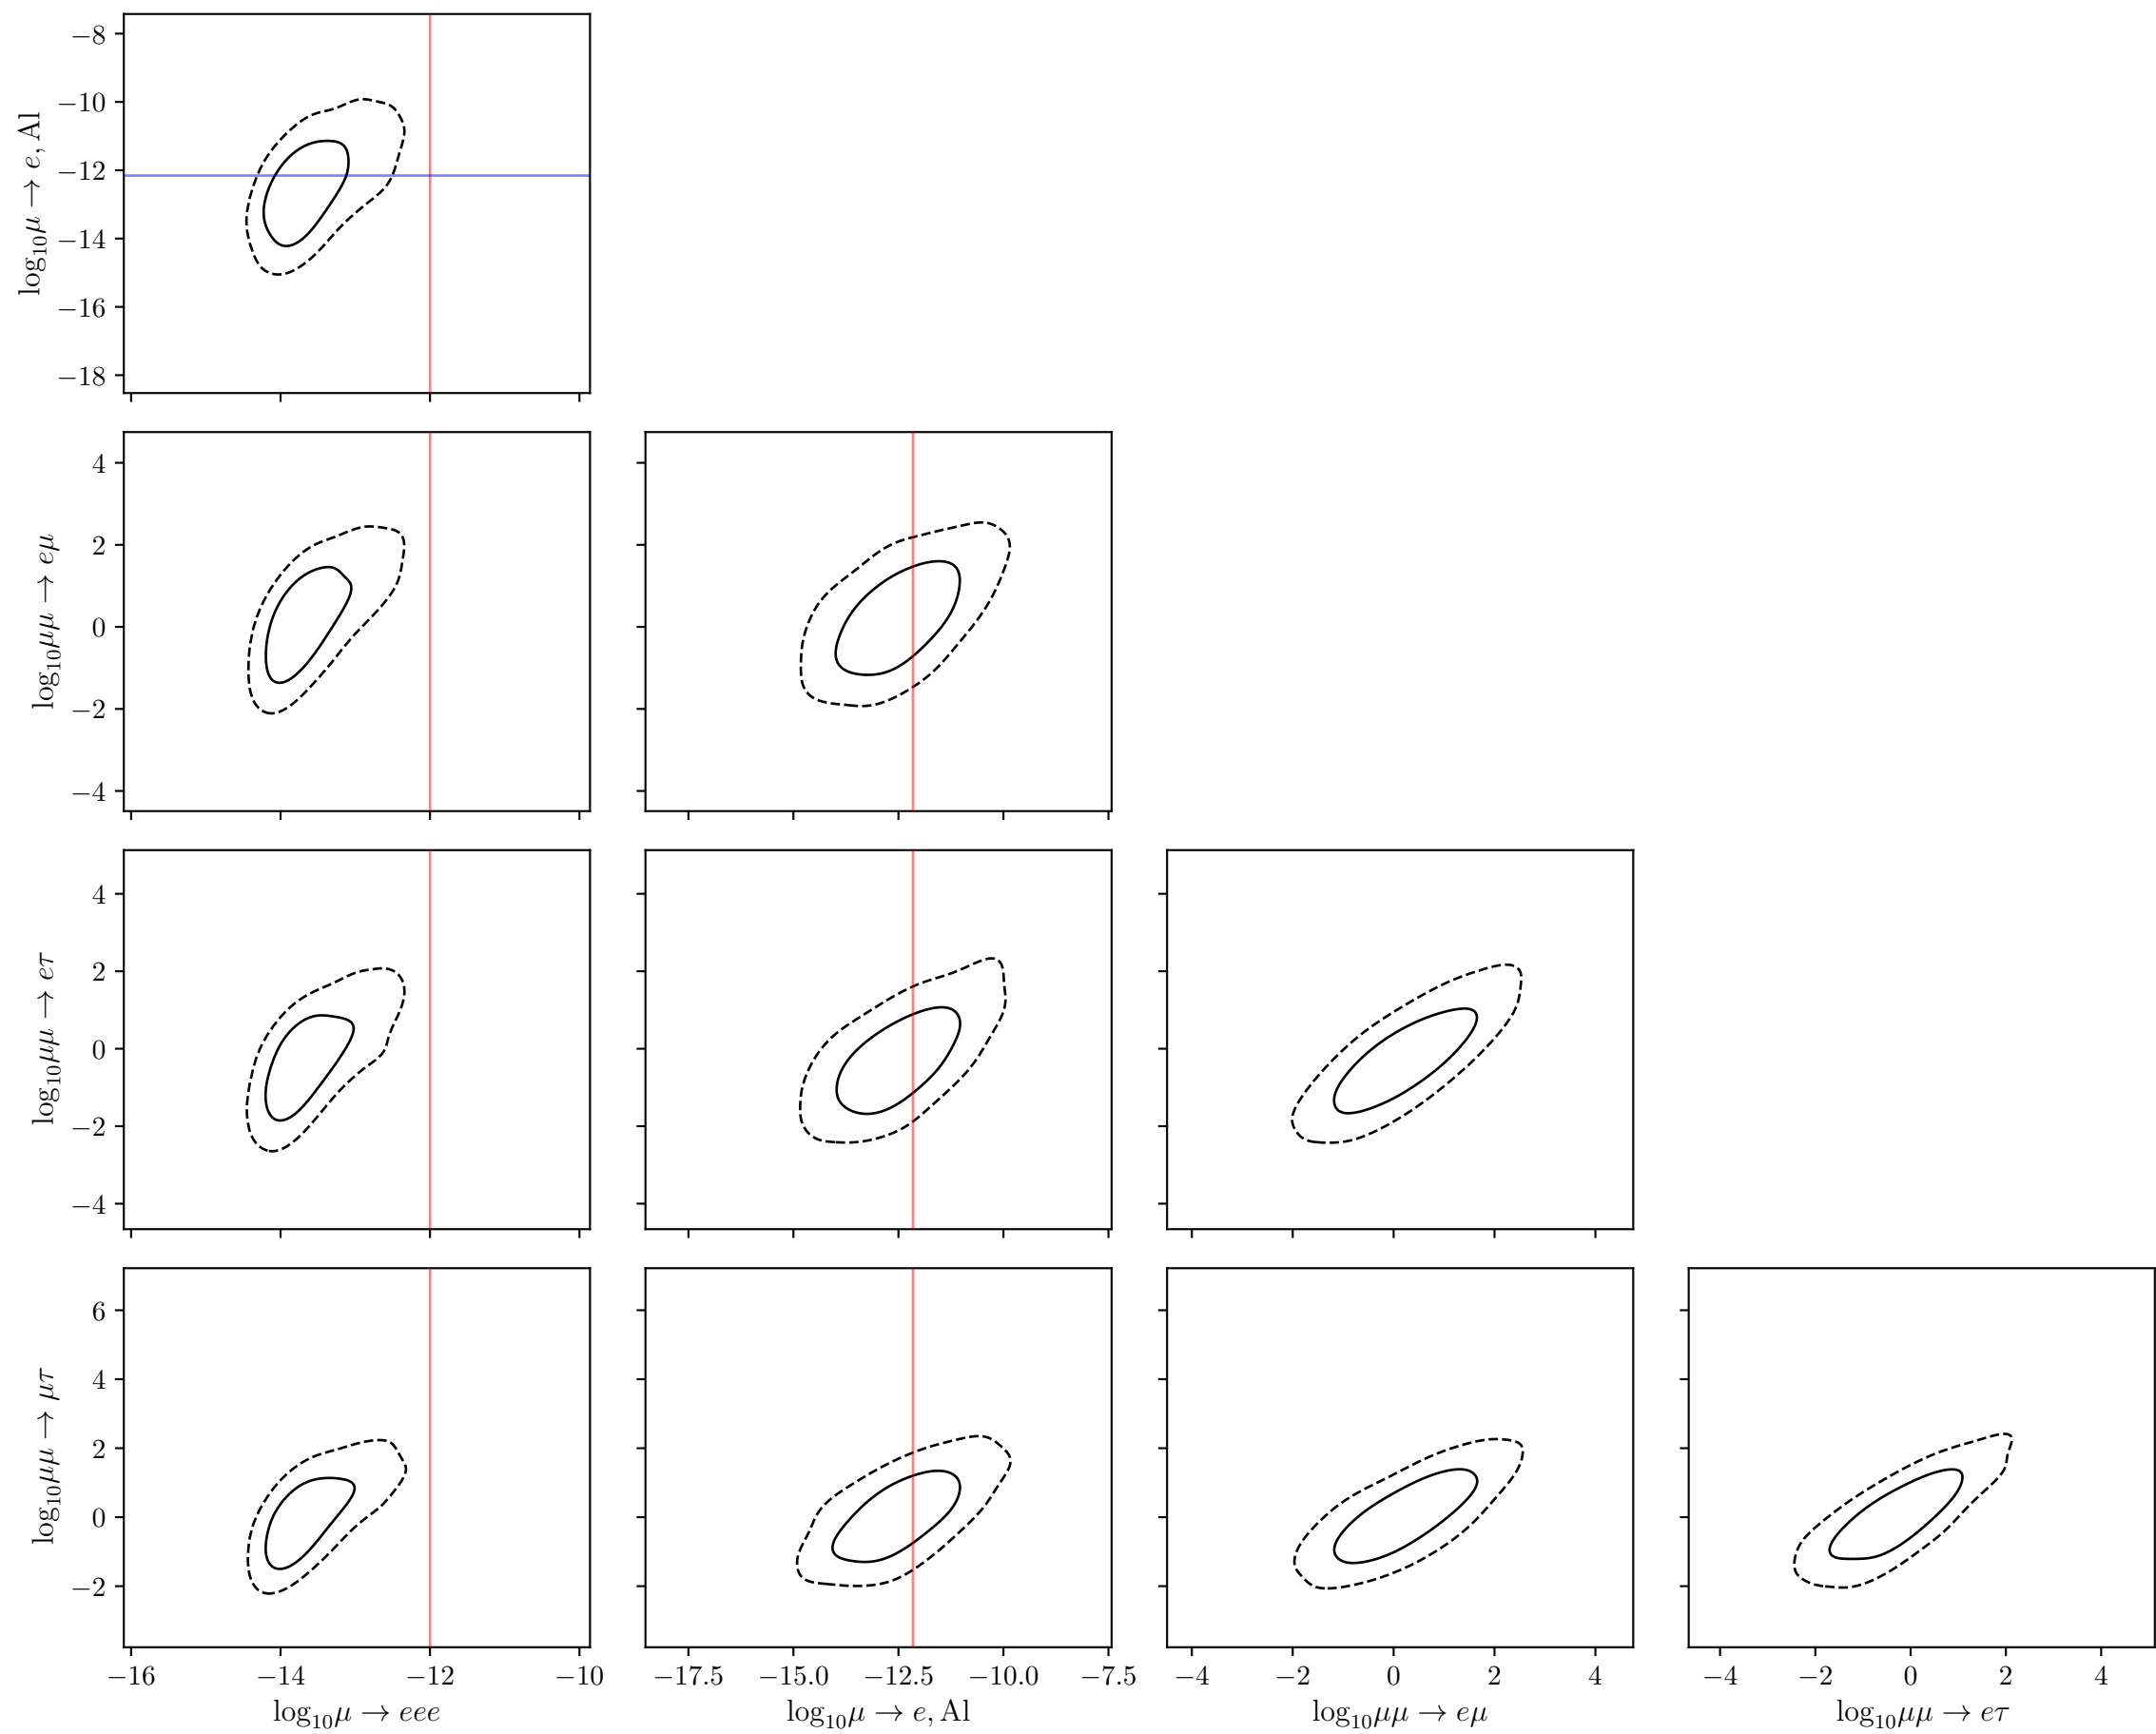

Majorana,  $X_L = \{5, 5, 4\}$ ,  $X_e = \{7, 3, 0\}$ ,

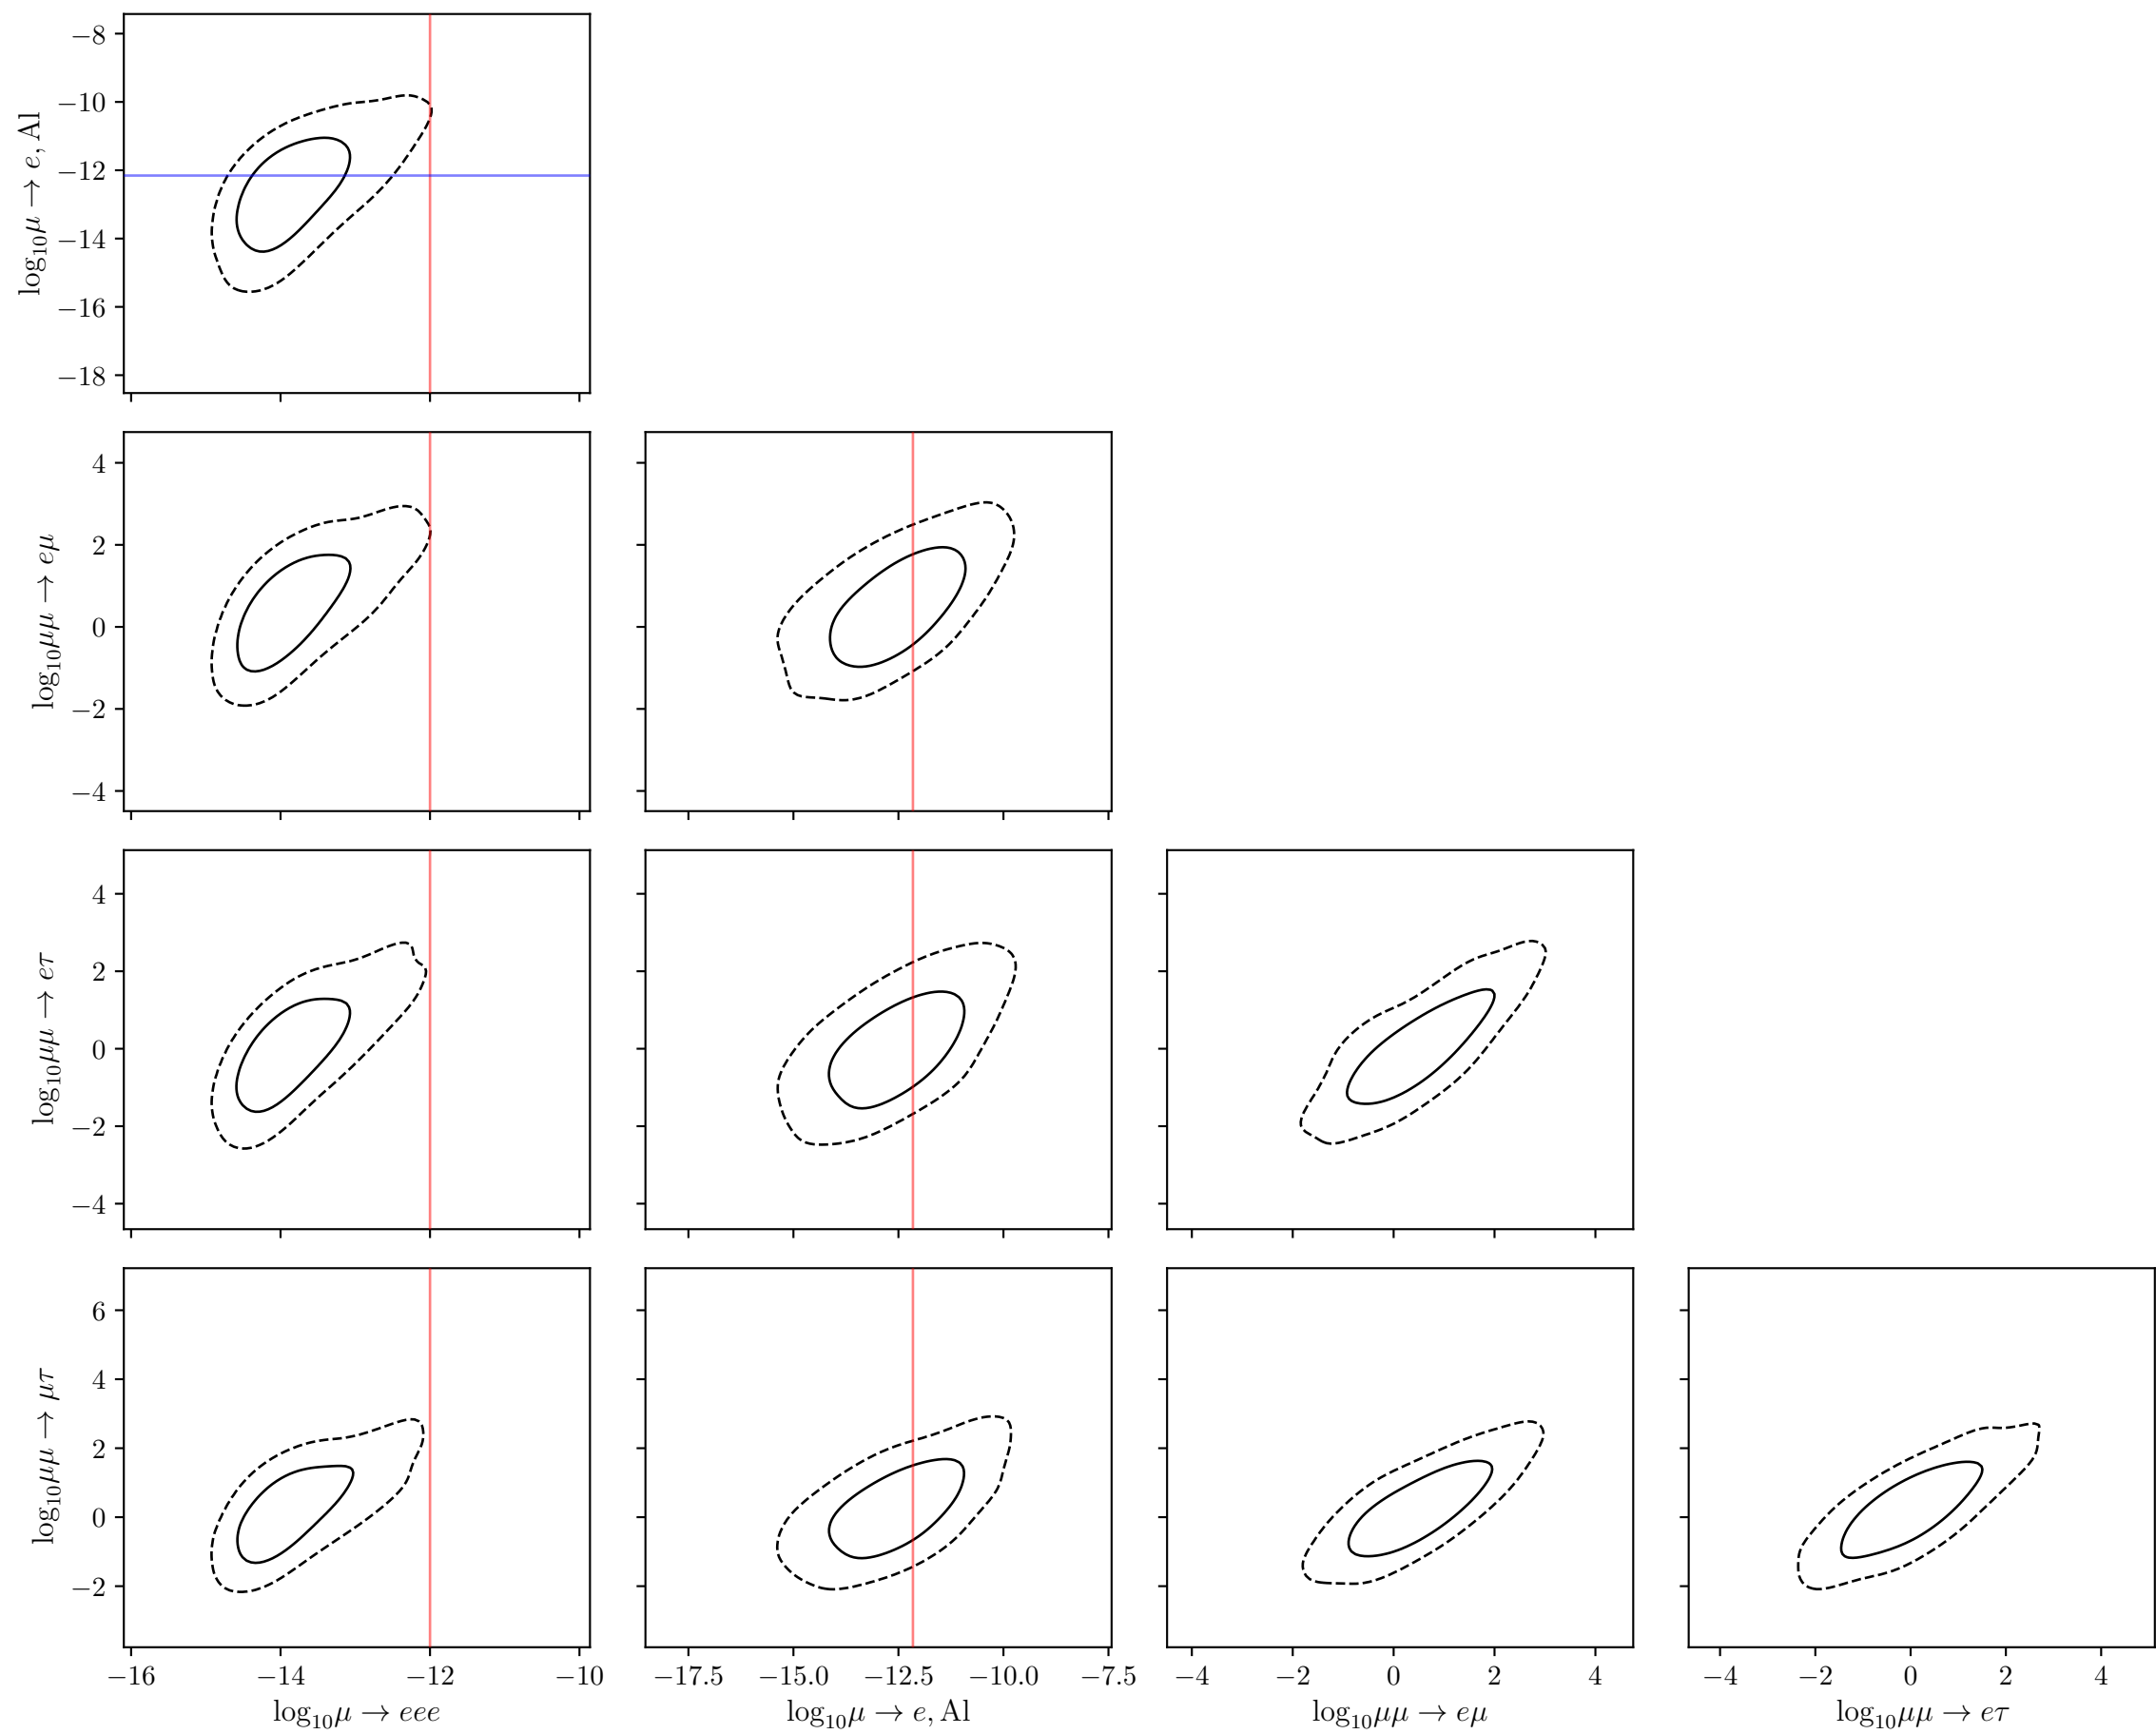

Majorana,  $X_L = \{5, 5, 4\}$ ,  $X_e = \{5, 2, 0\}$ ,

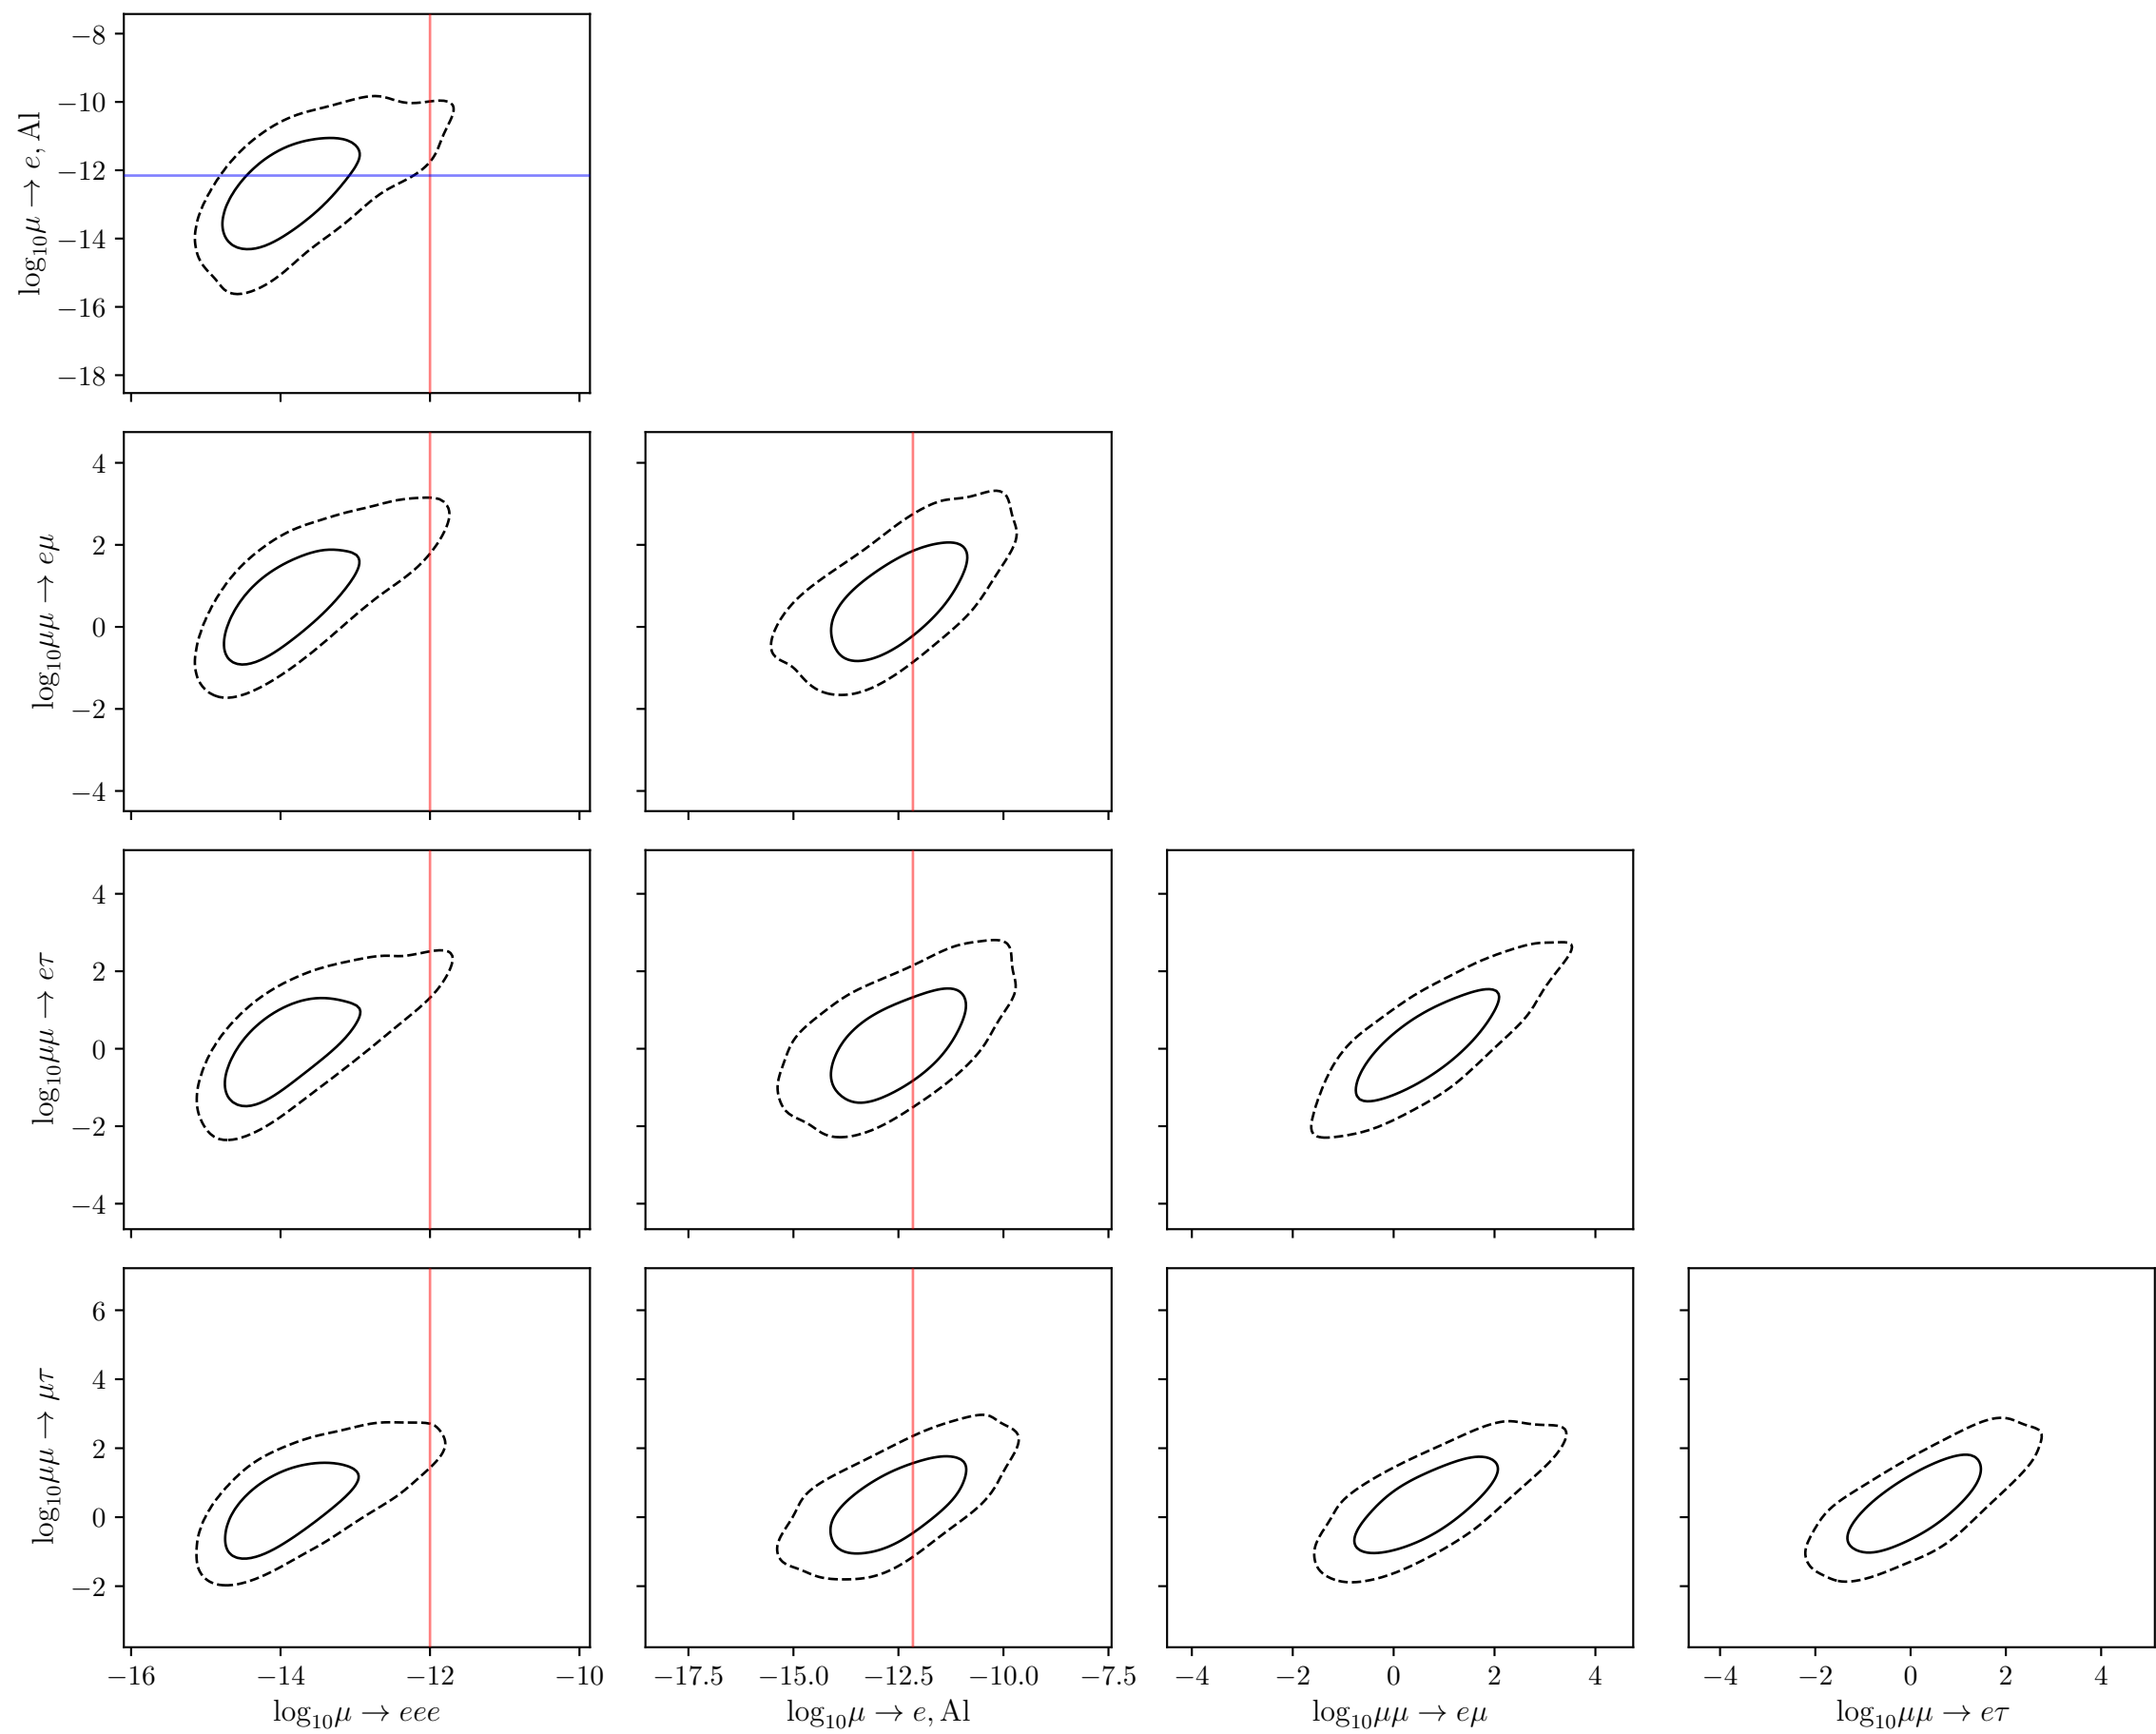

Majorana,  $X_L = \{6, 6, 5\}$ ,  $X_e = \{-1, 1, 4\}$ ,

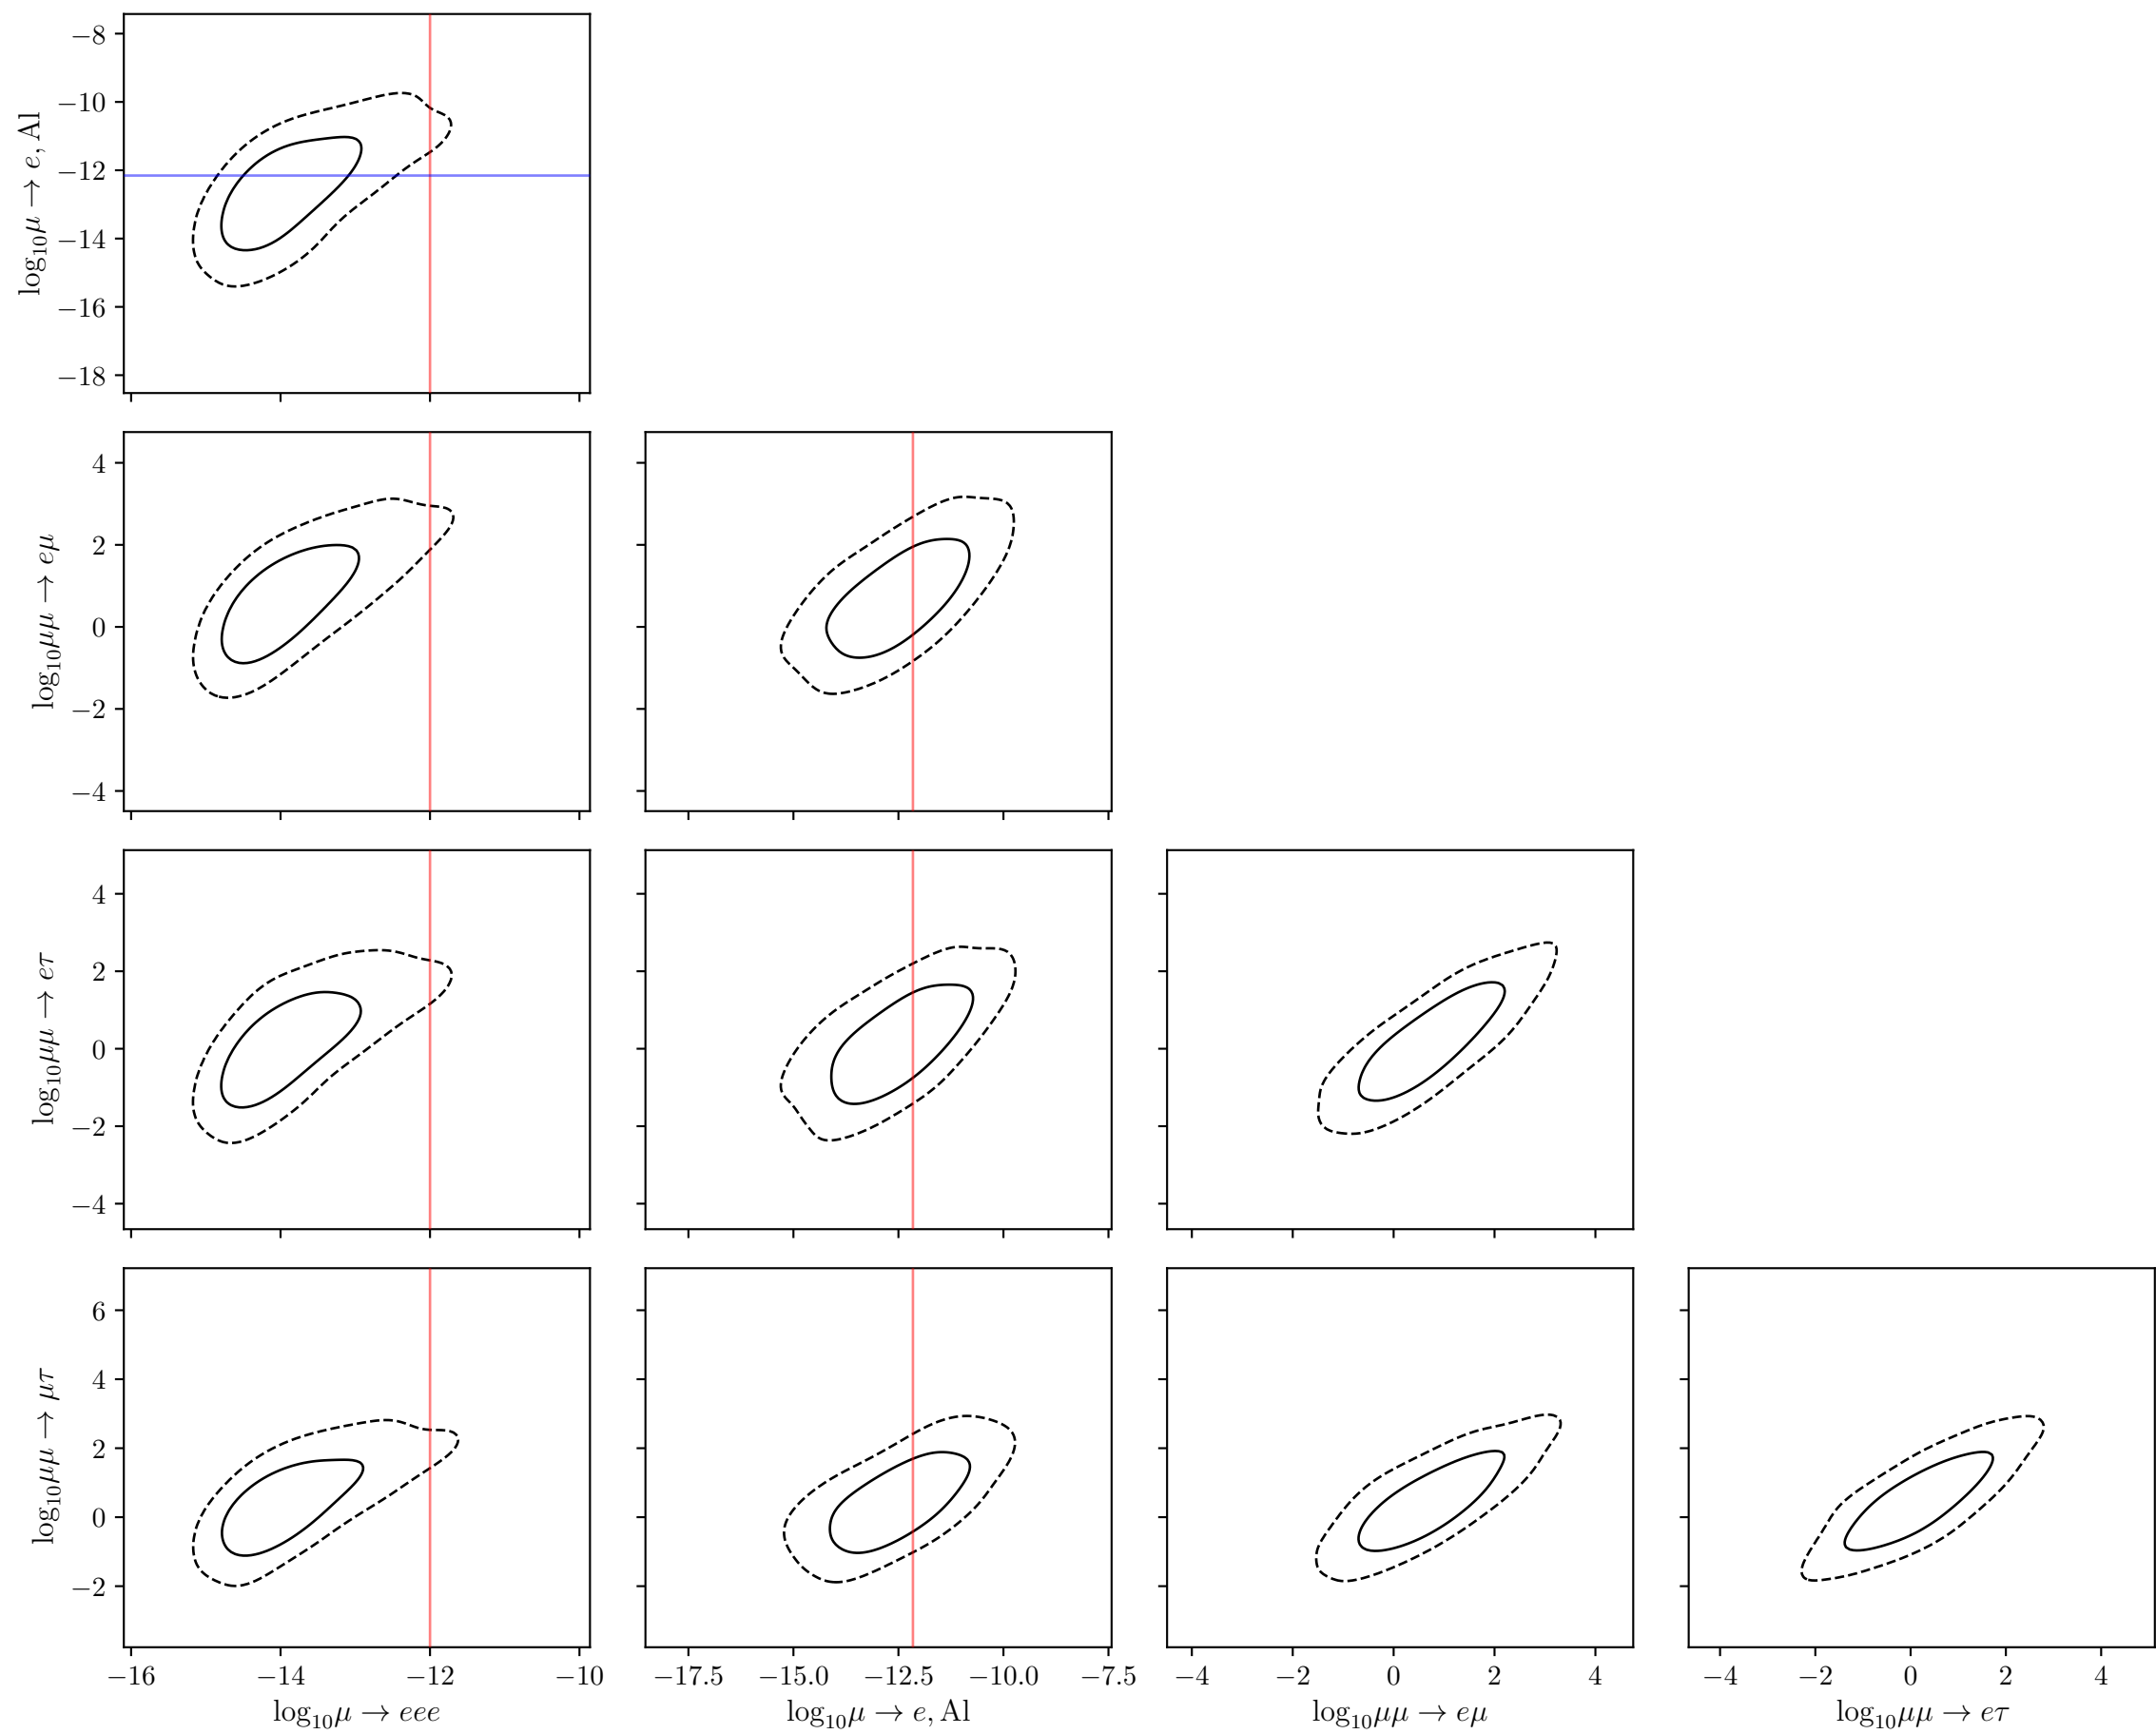

Majorana,  $X_L = \{7, 7, 6\}$ ,  $X_e = \{-2, 1, 5\}$ ,

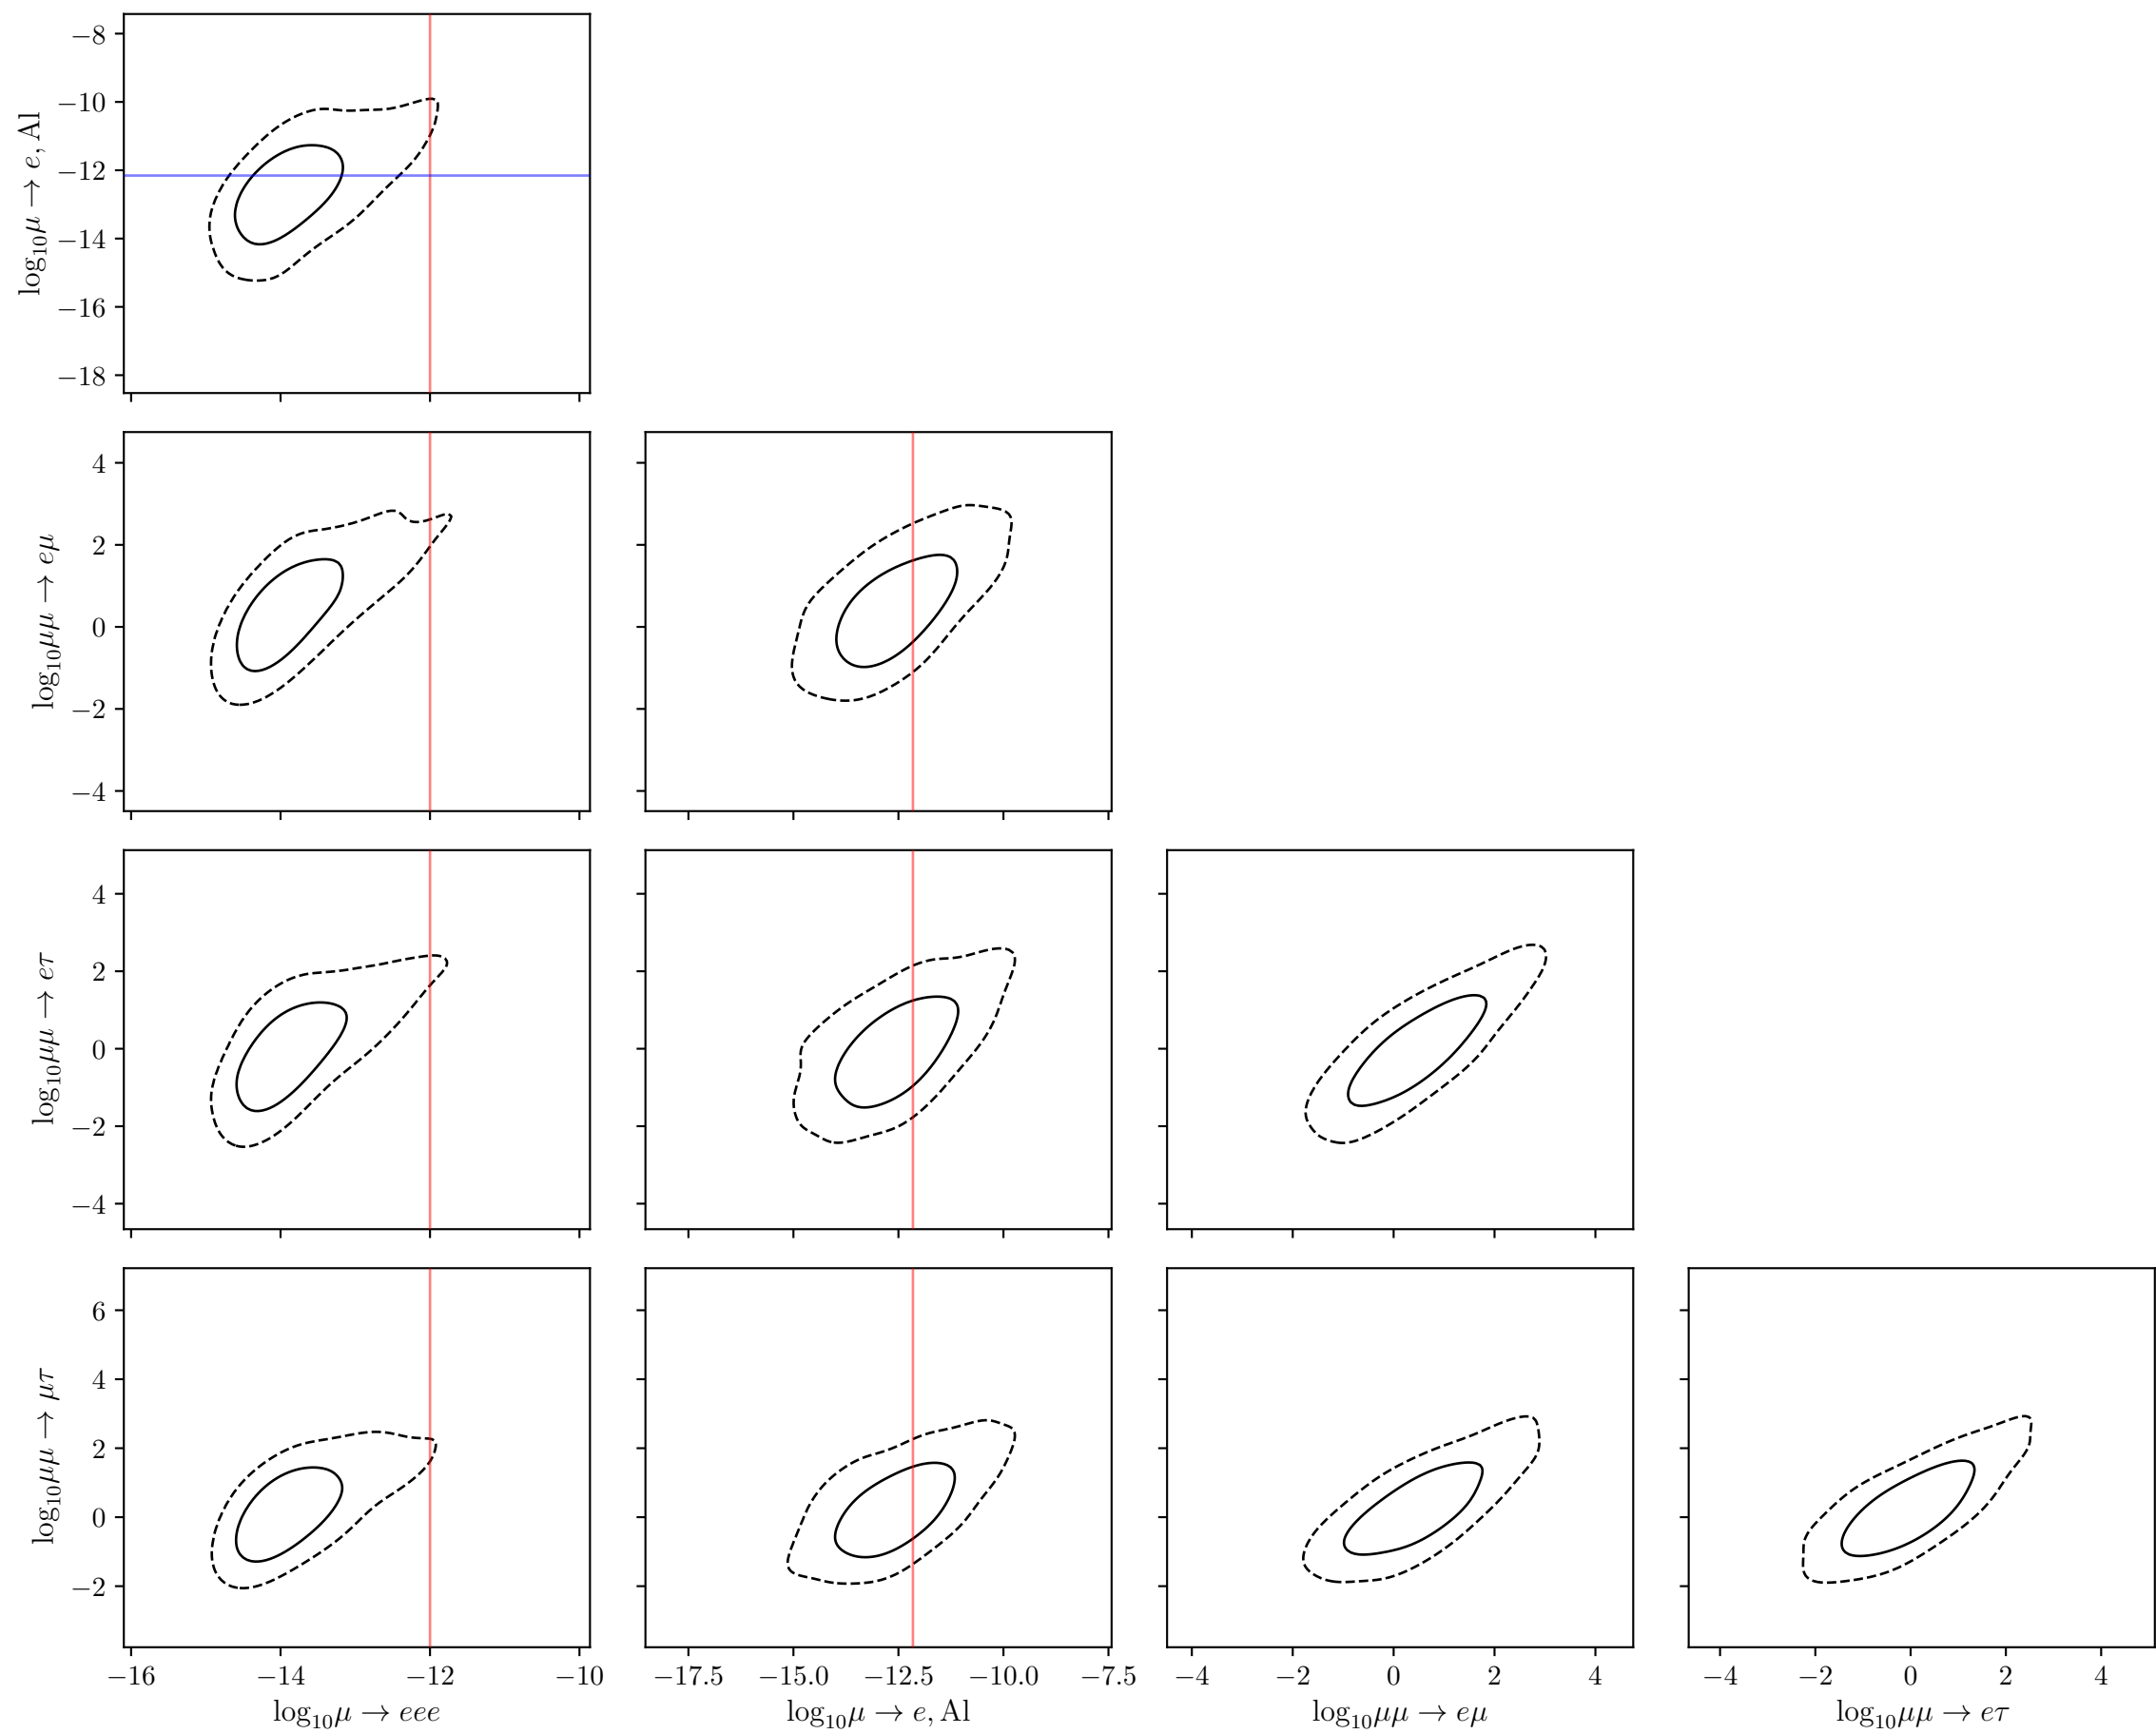

Majorana,  $X_L = \{4, 4, 3\}$ ,  $X_e = \{6, 3, 1\}$ ,

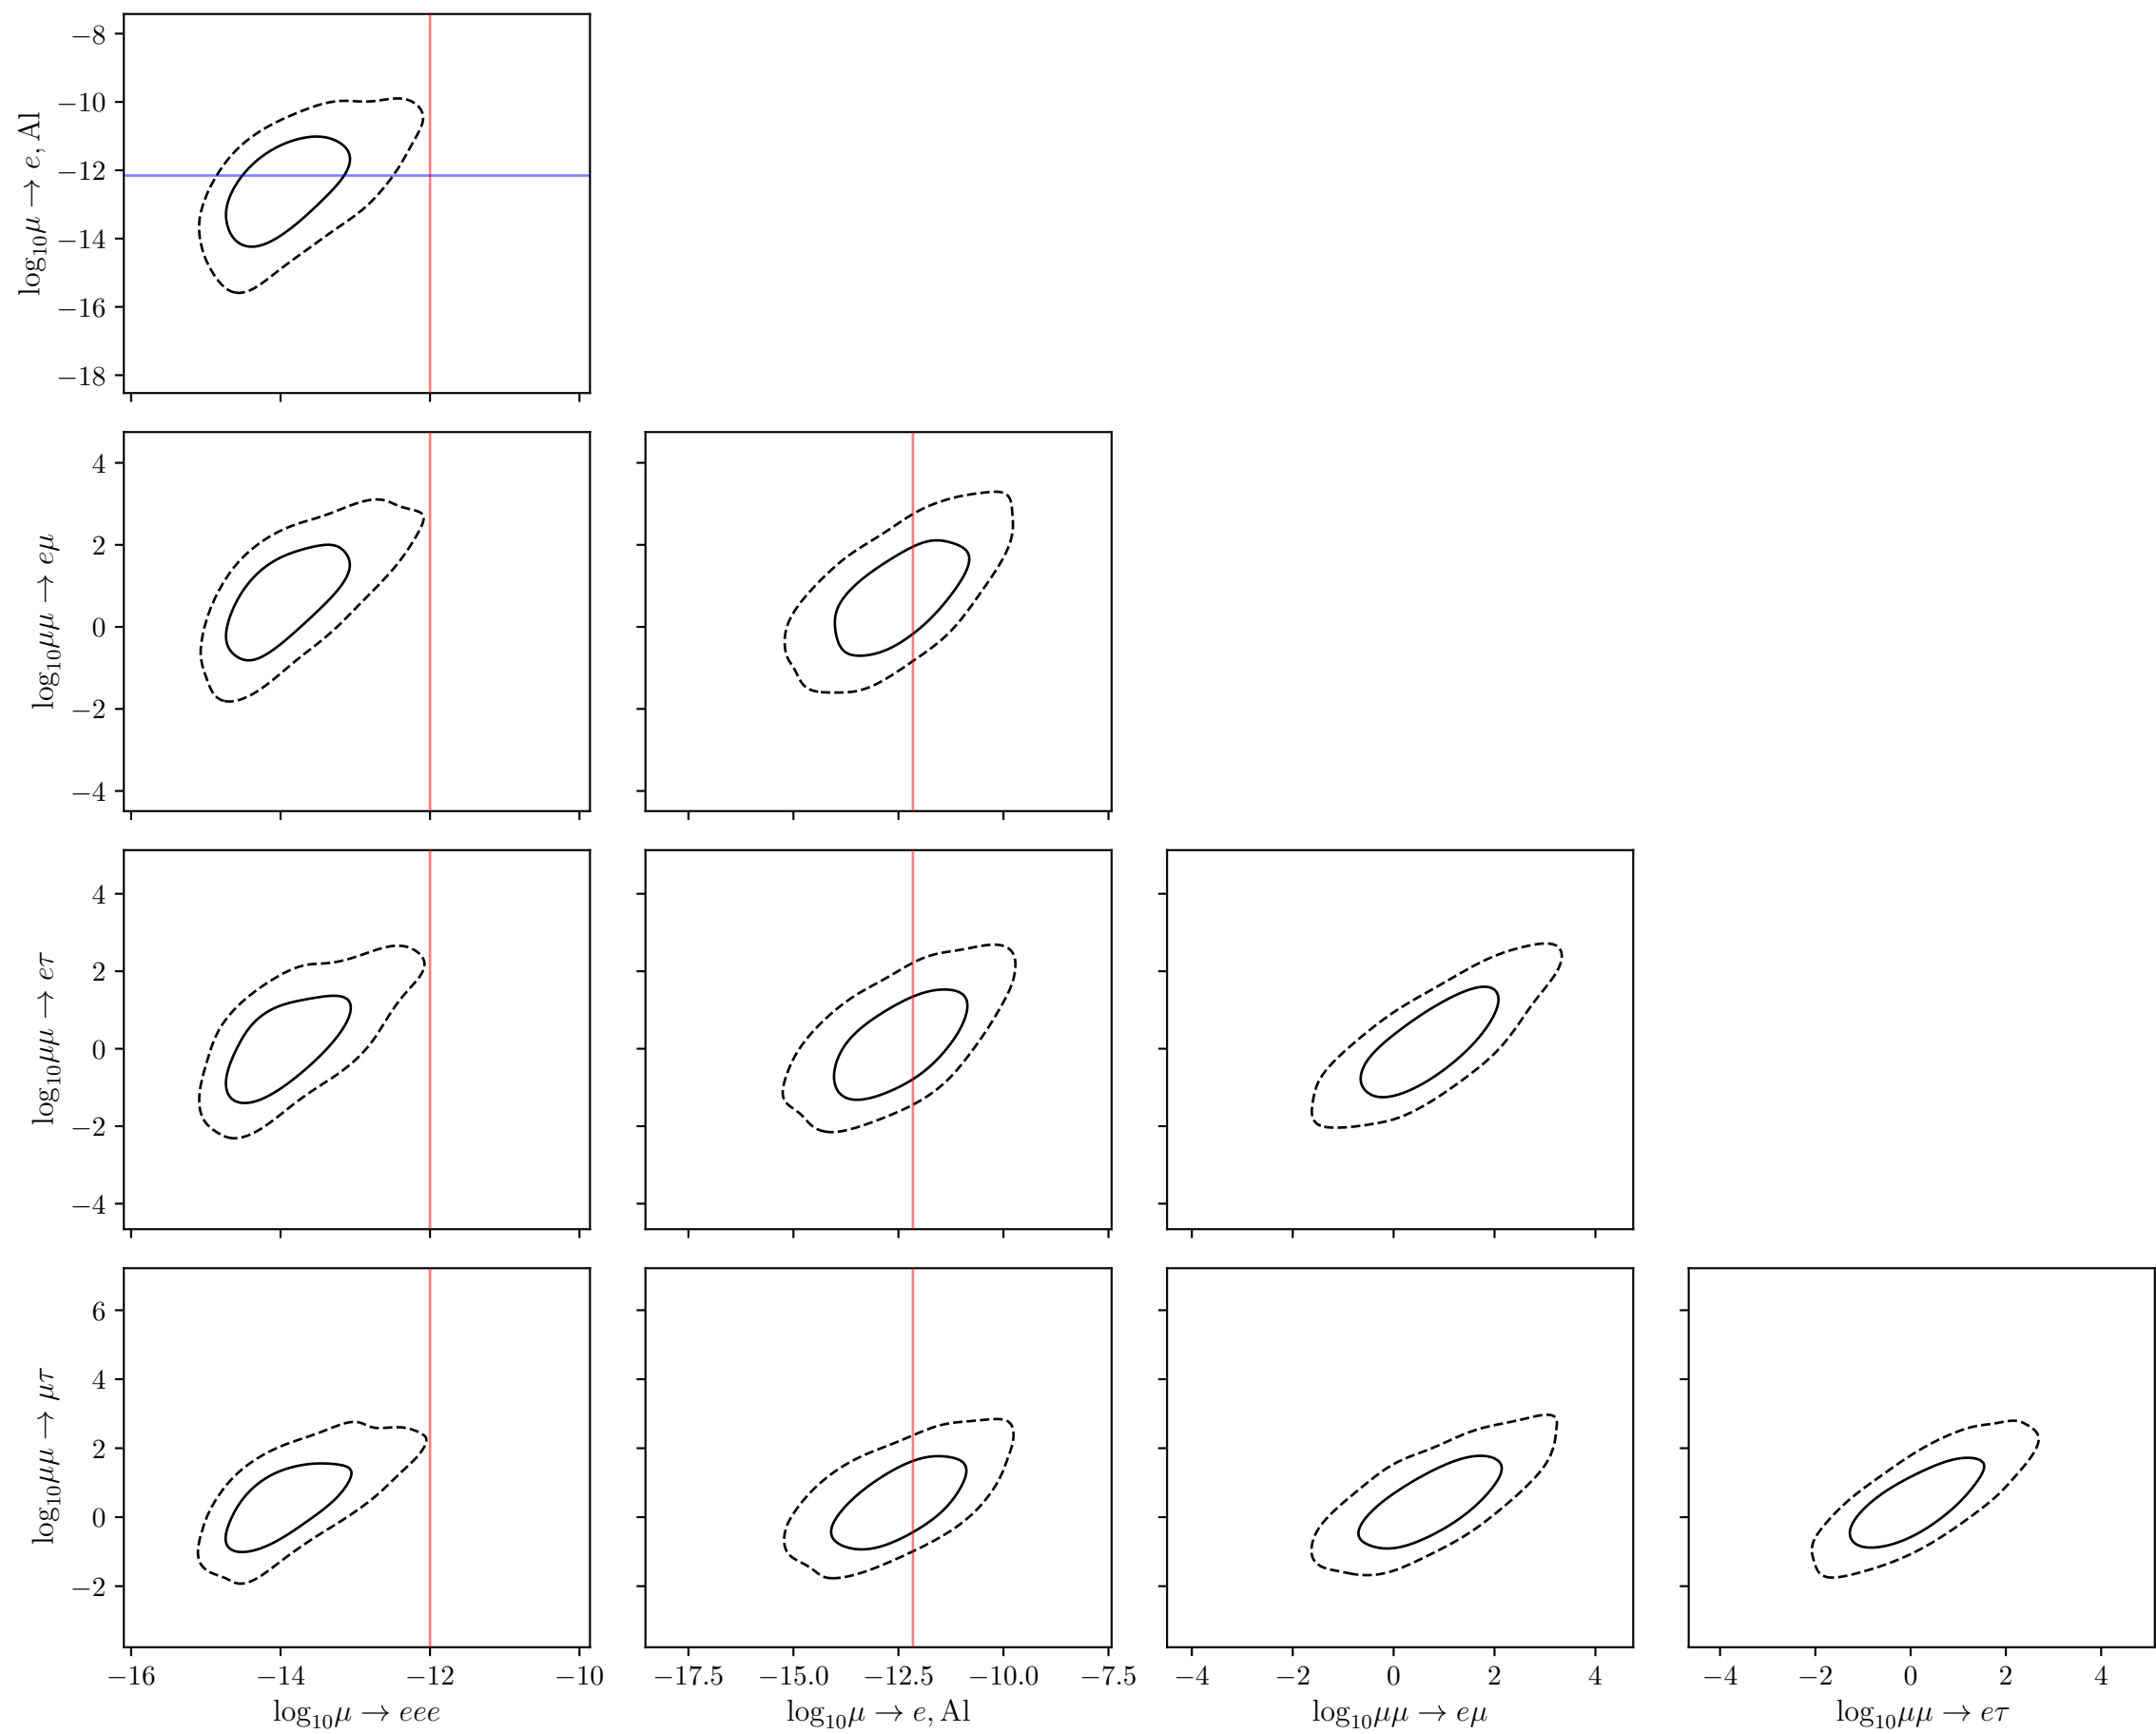

Majorana,  $X_L = \{7, 6, 5\}$ ,  $X_e = \{6, 3, 0\}$ ,

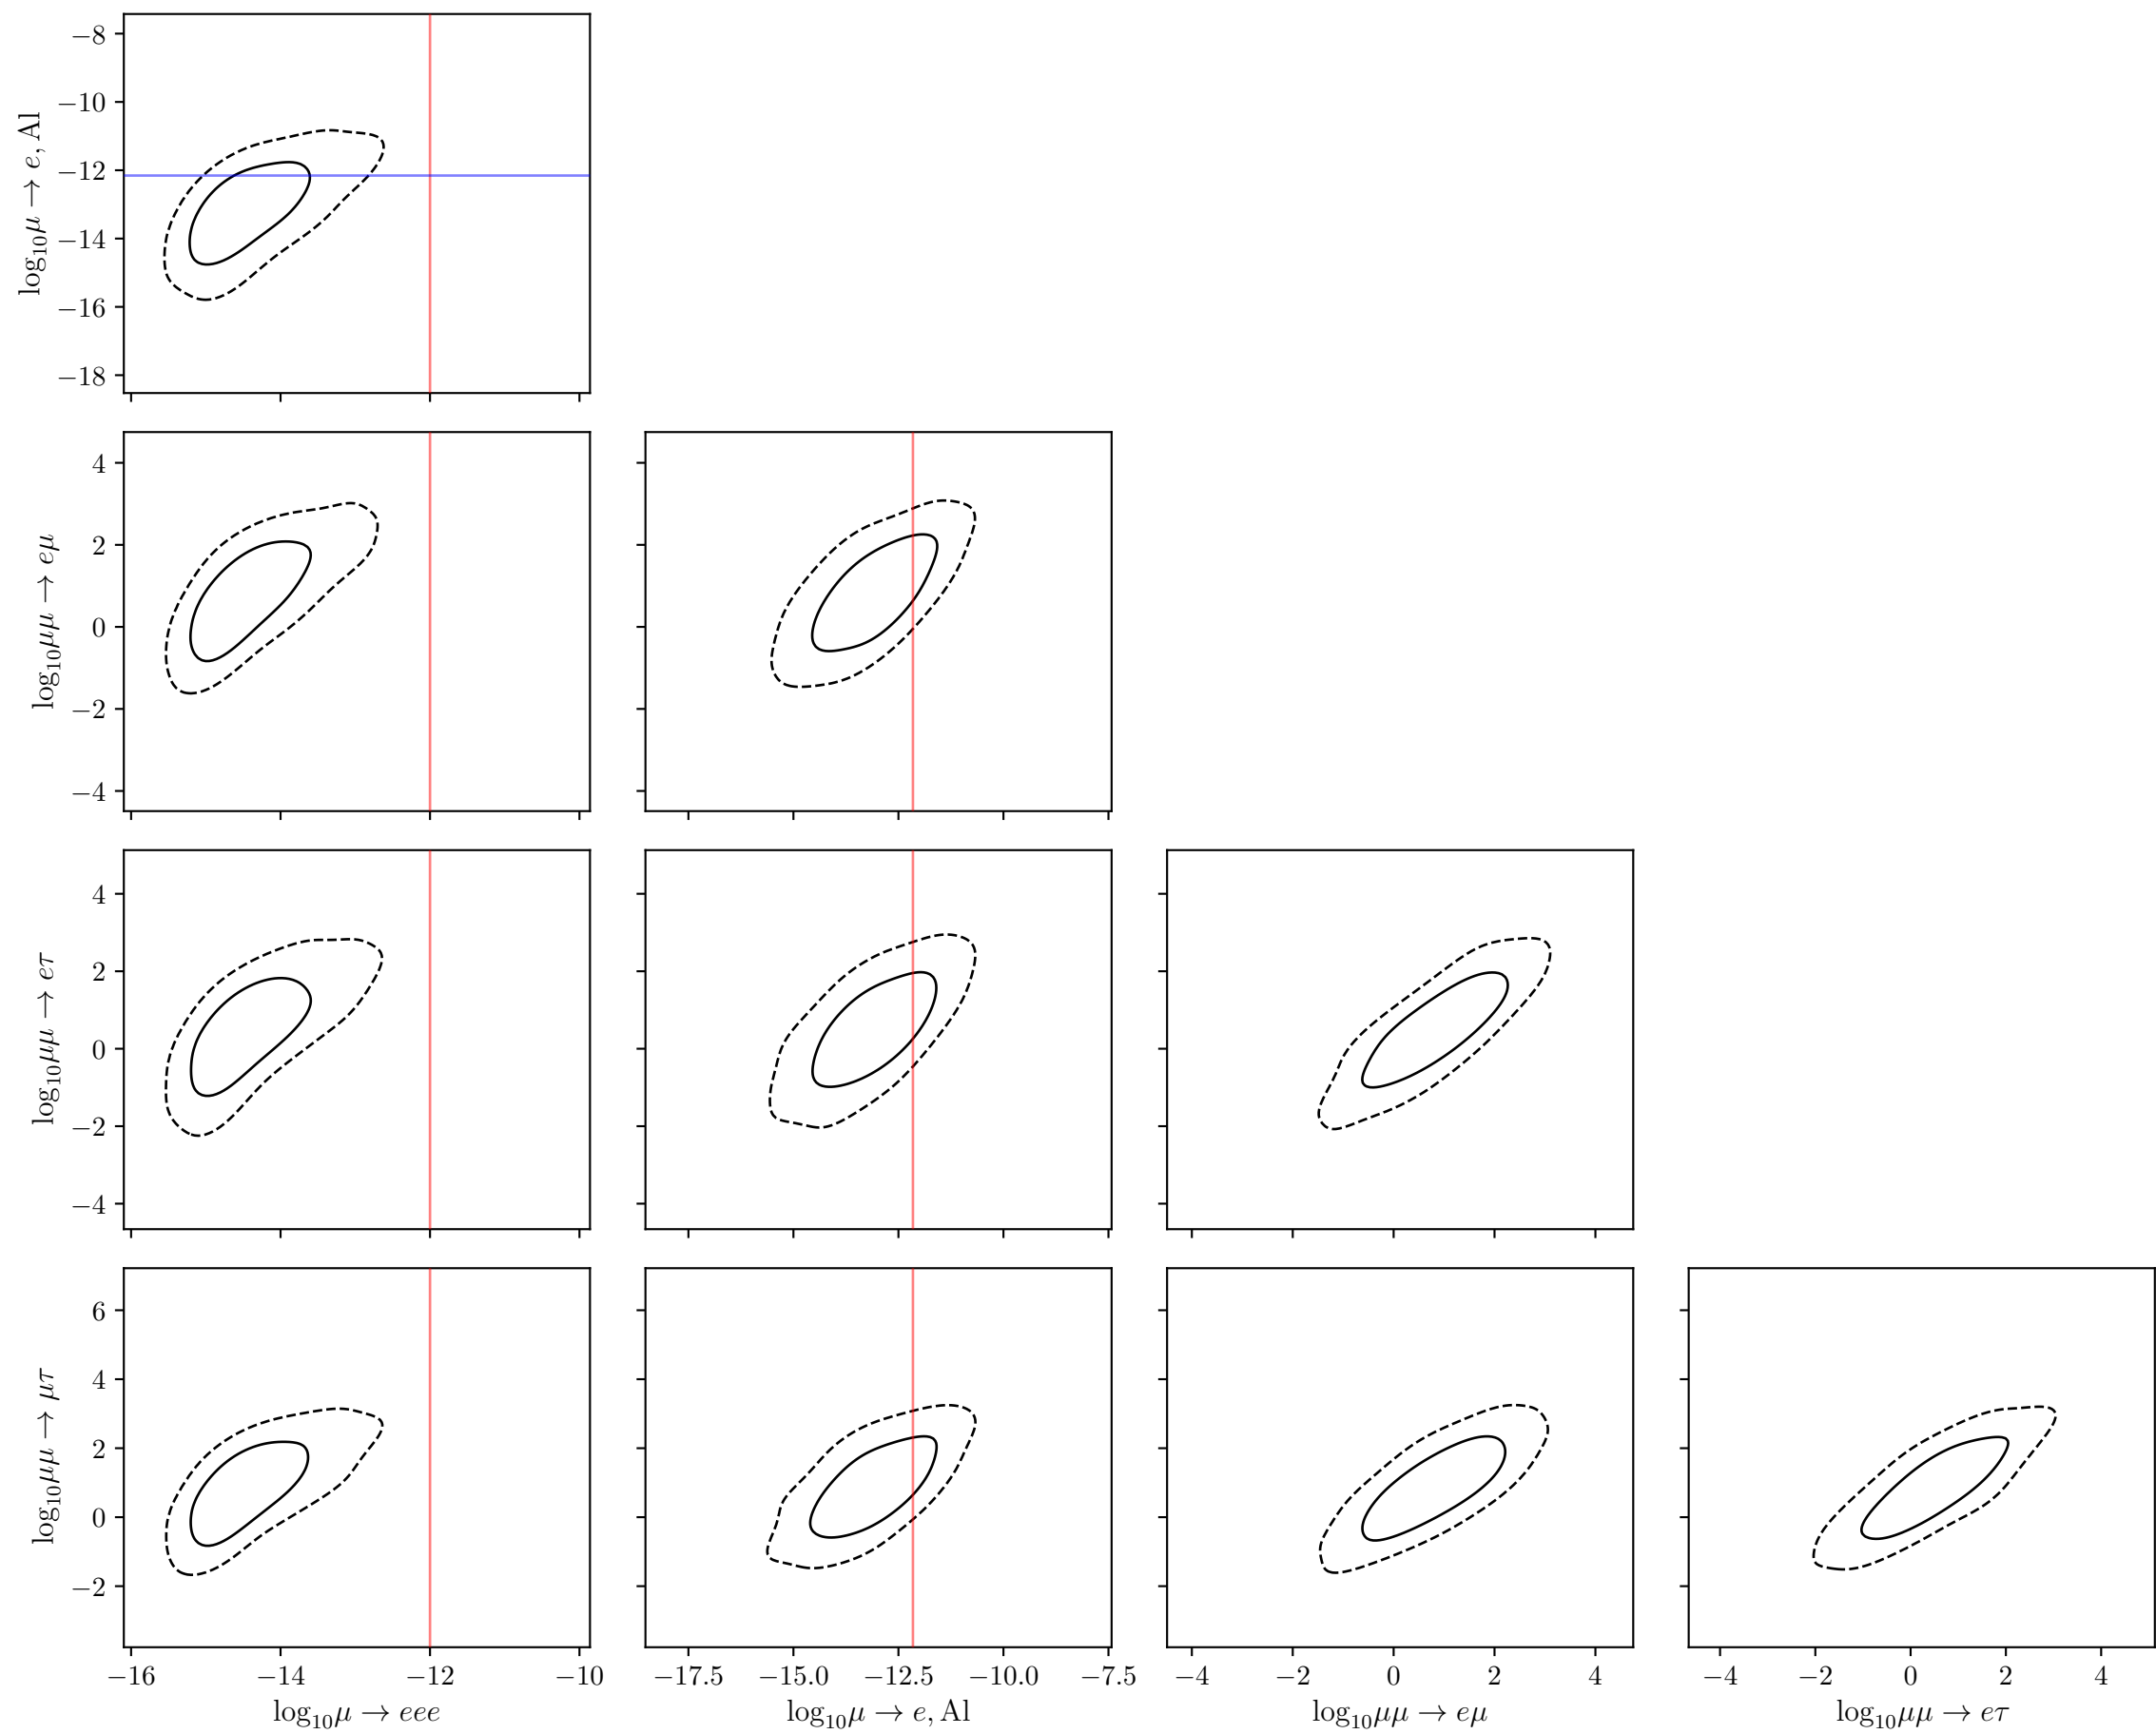



Majorana,  $X_L = \{7, 7, 6\}$ ,  $X_e = \{-1, 1, 5\}$ ,

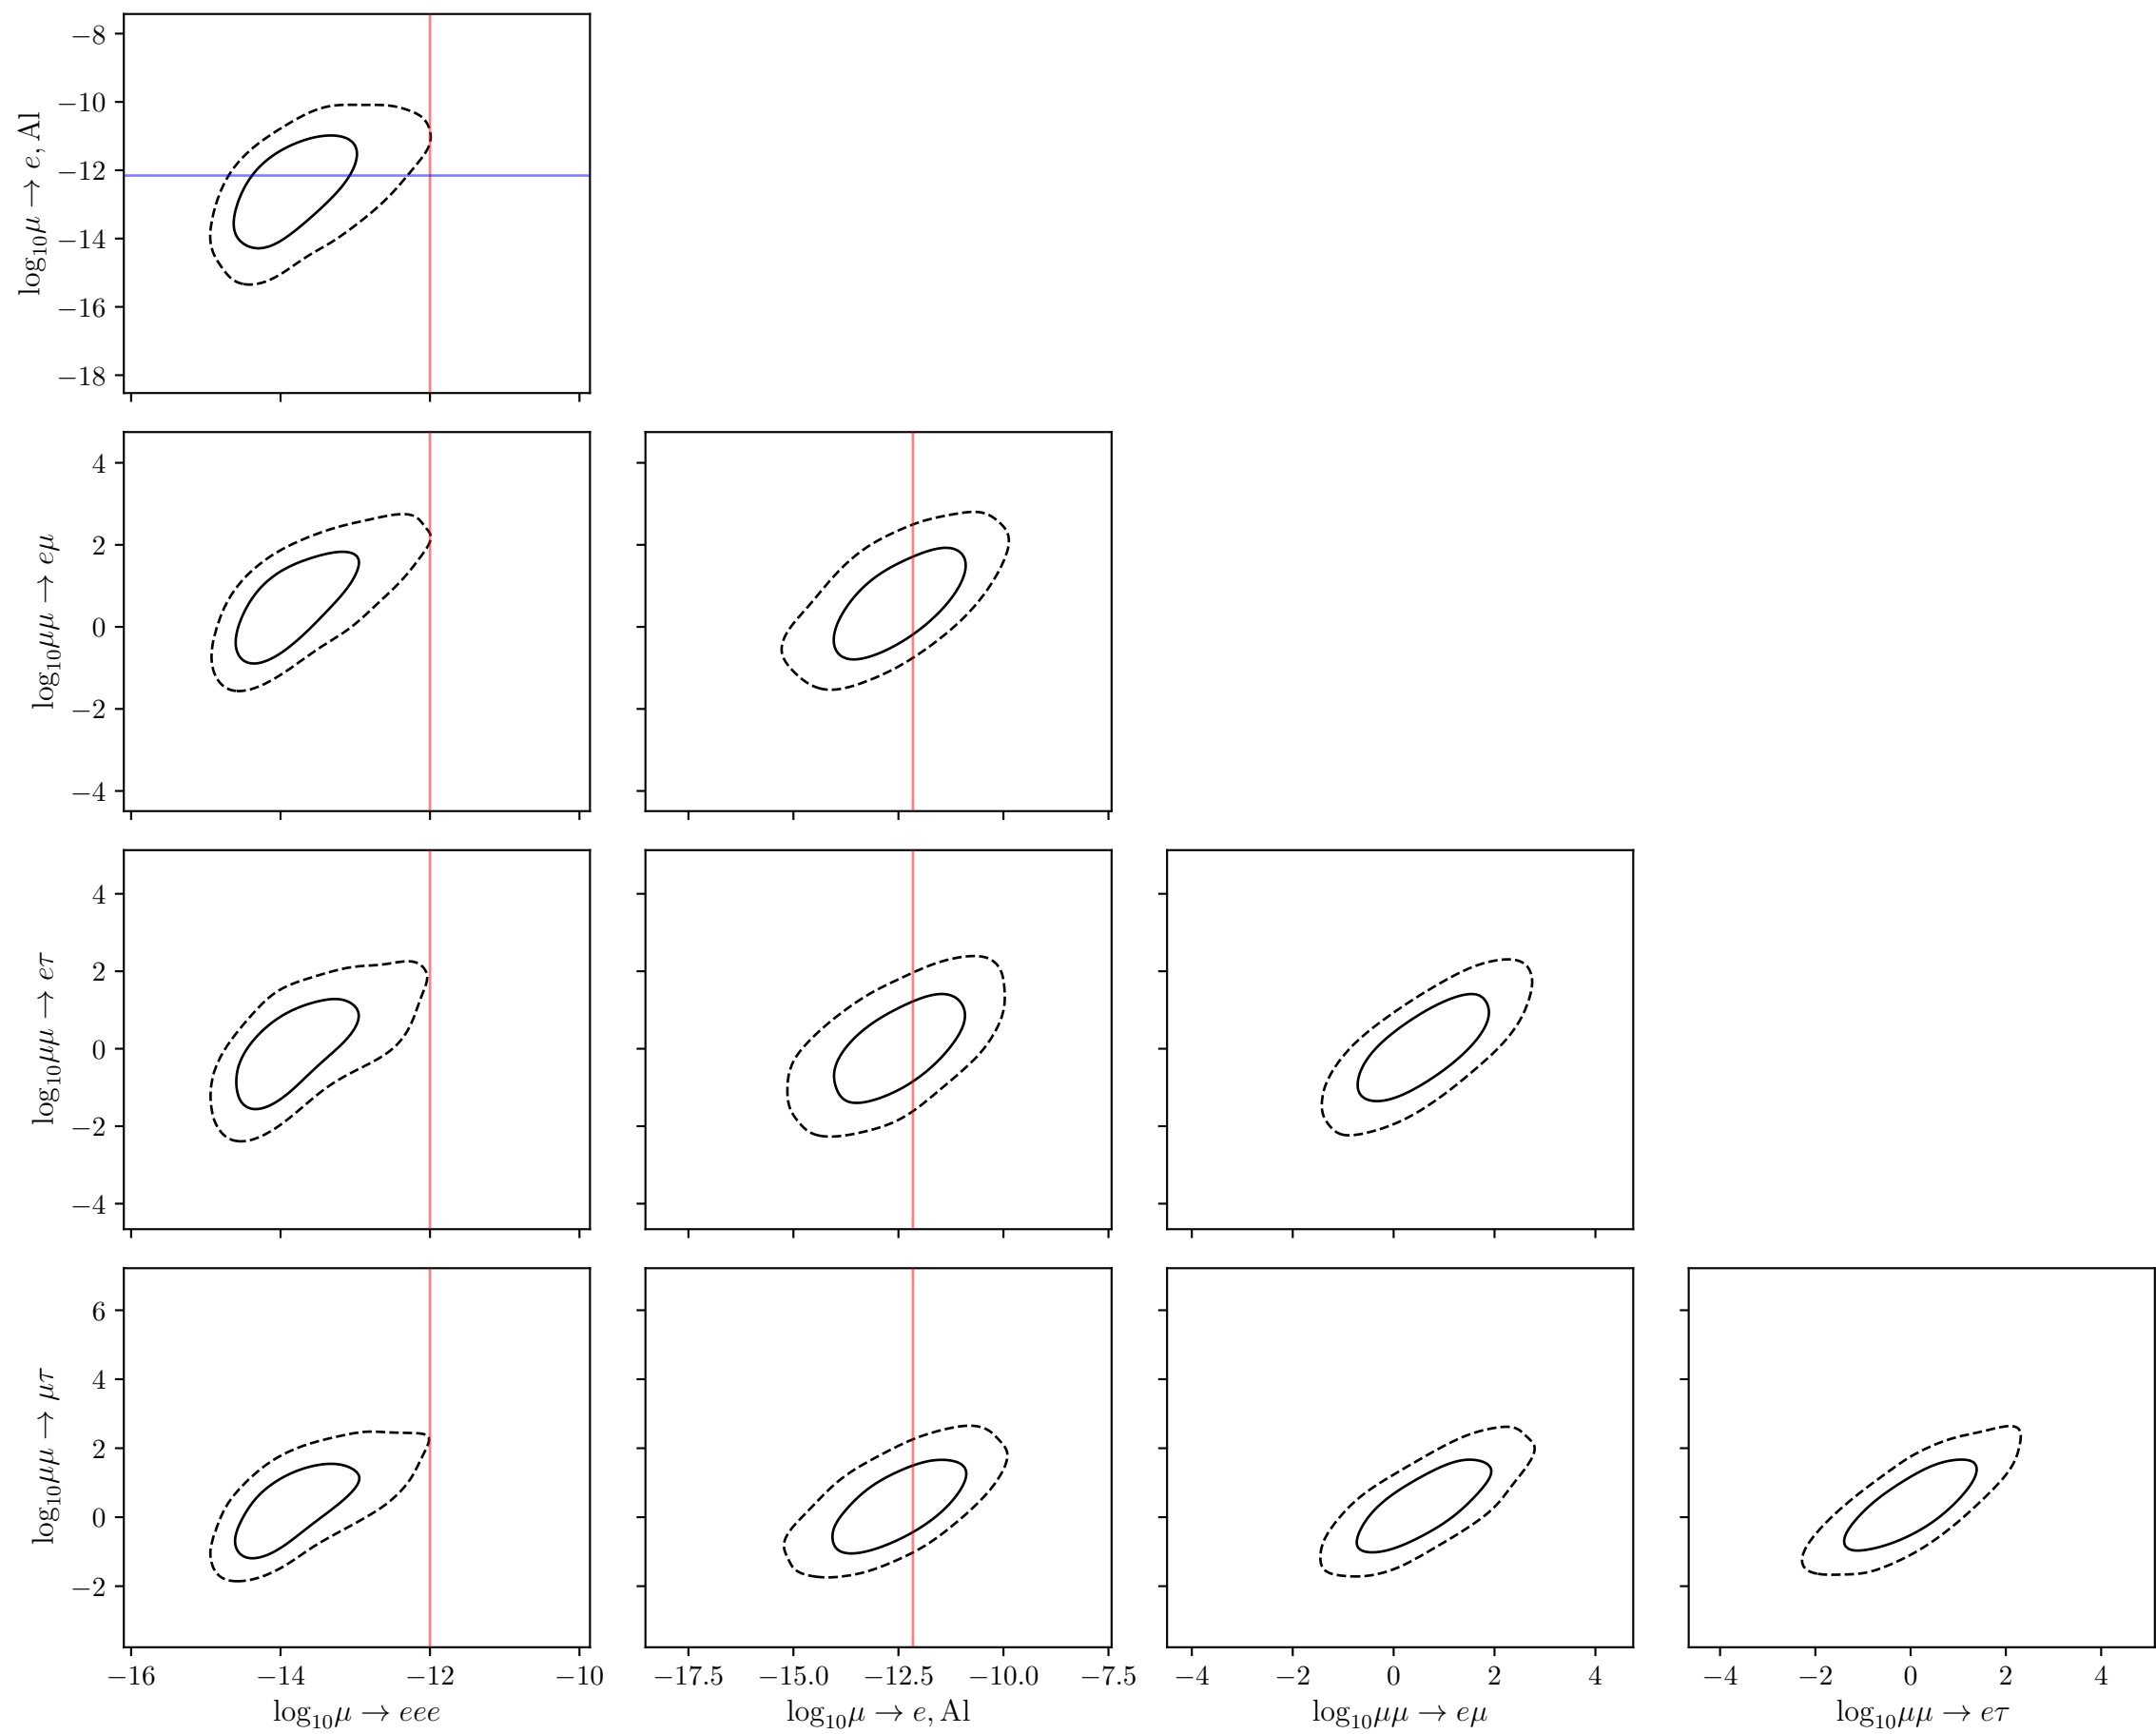

Majorana,  $X_L = \{7, 7, 6\}$ ,  $X_e = \{-2, 0, 3\}$ ,

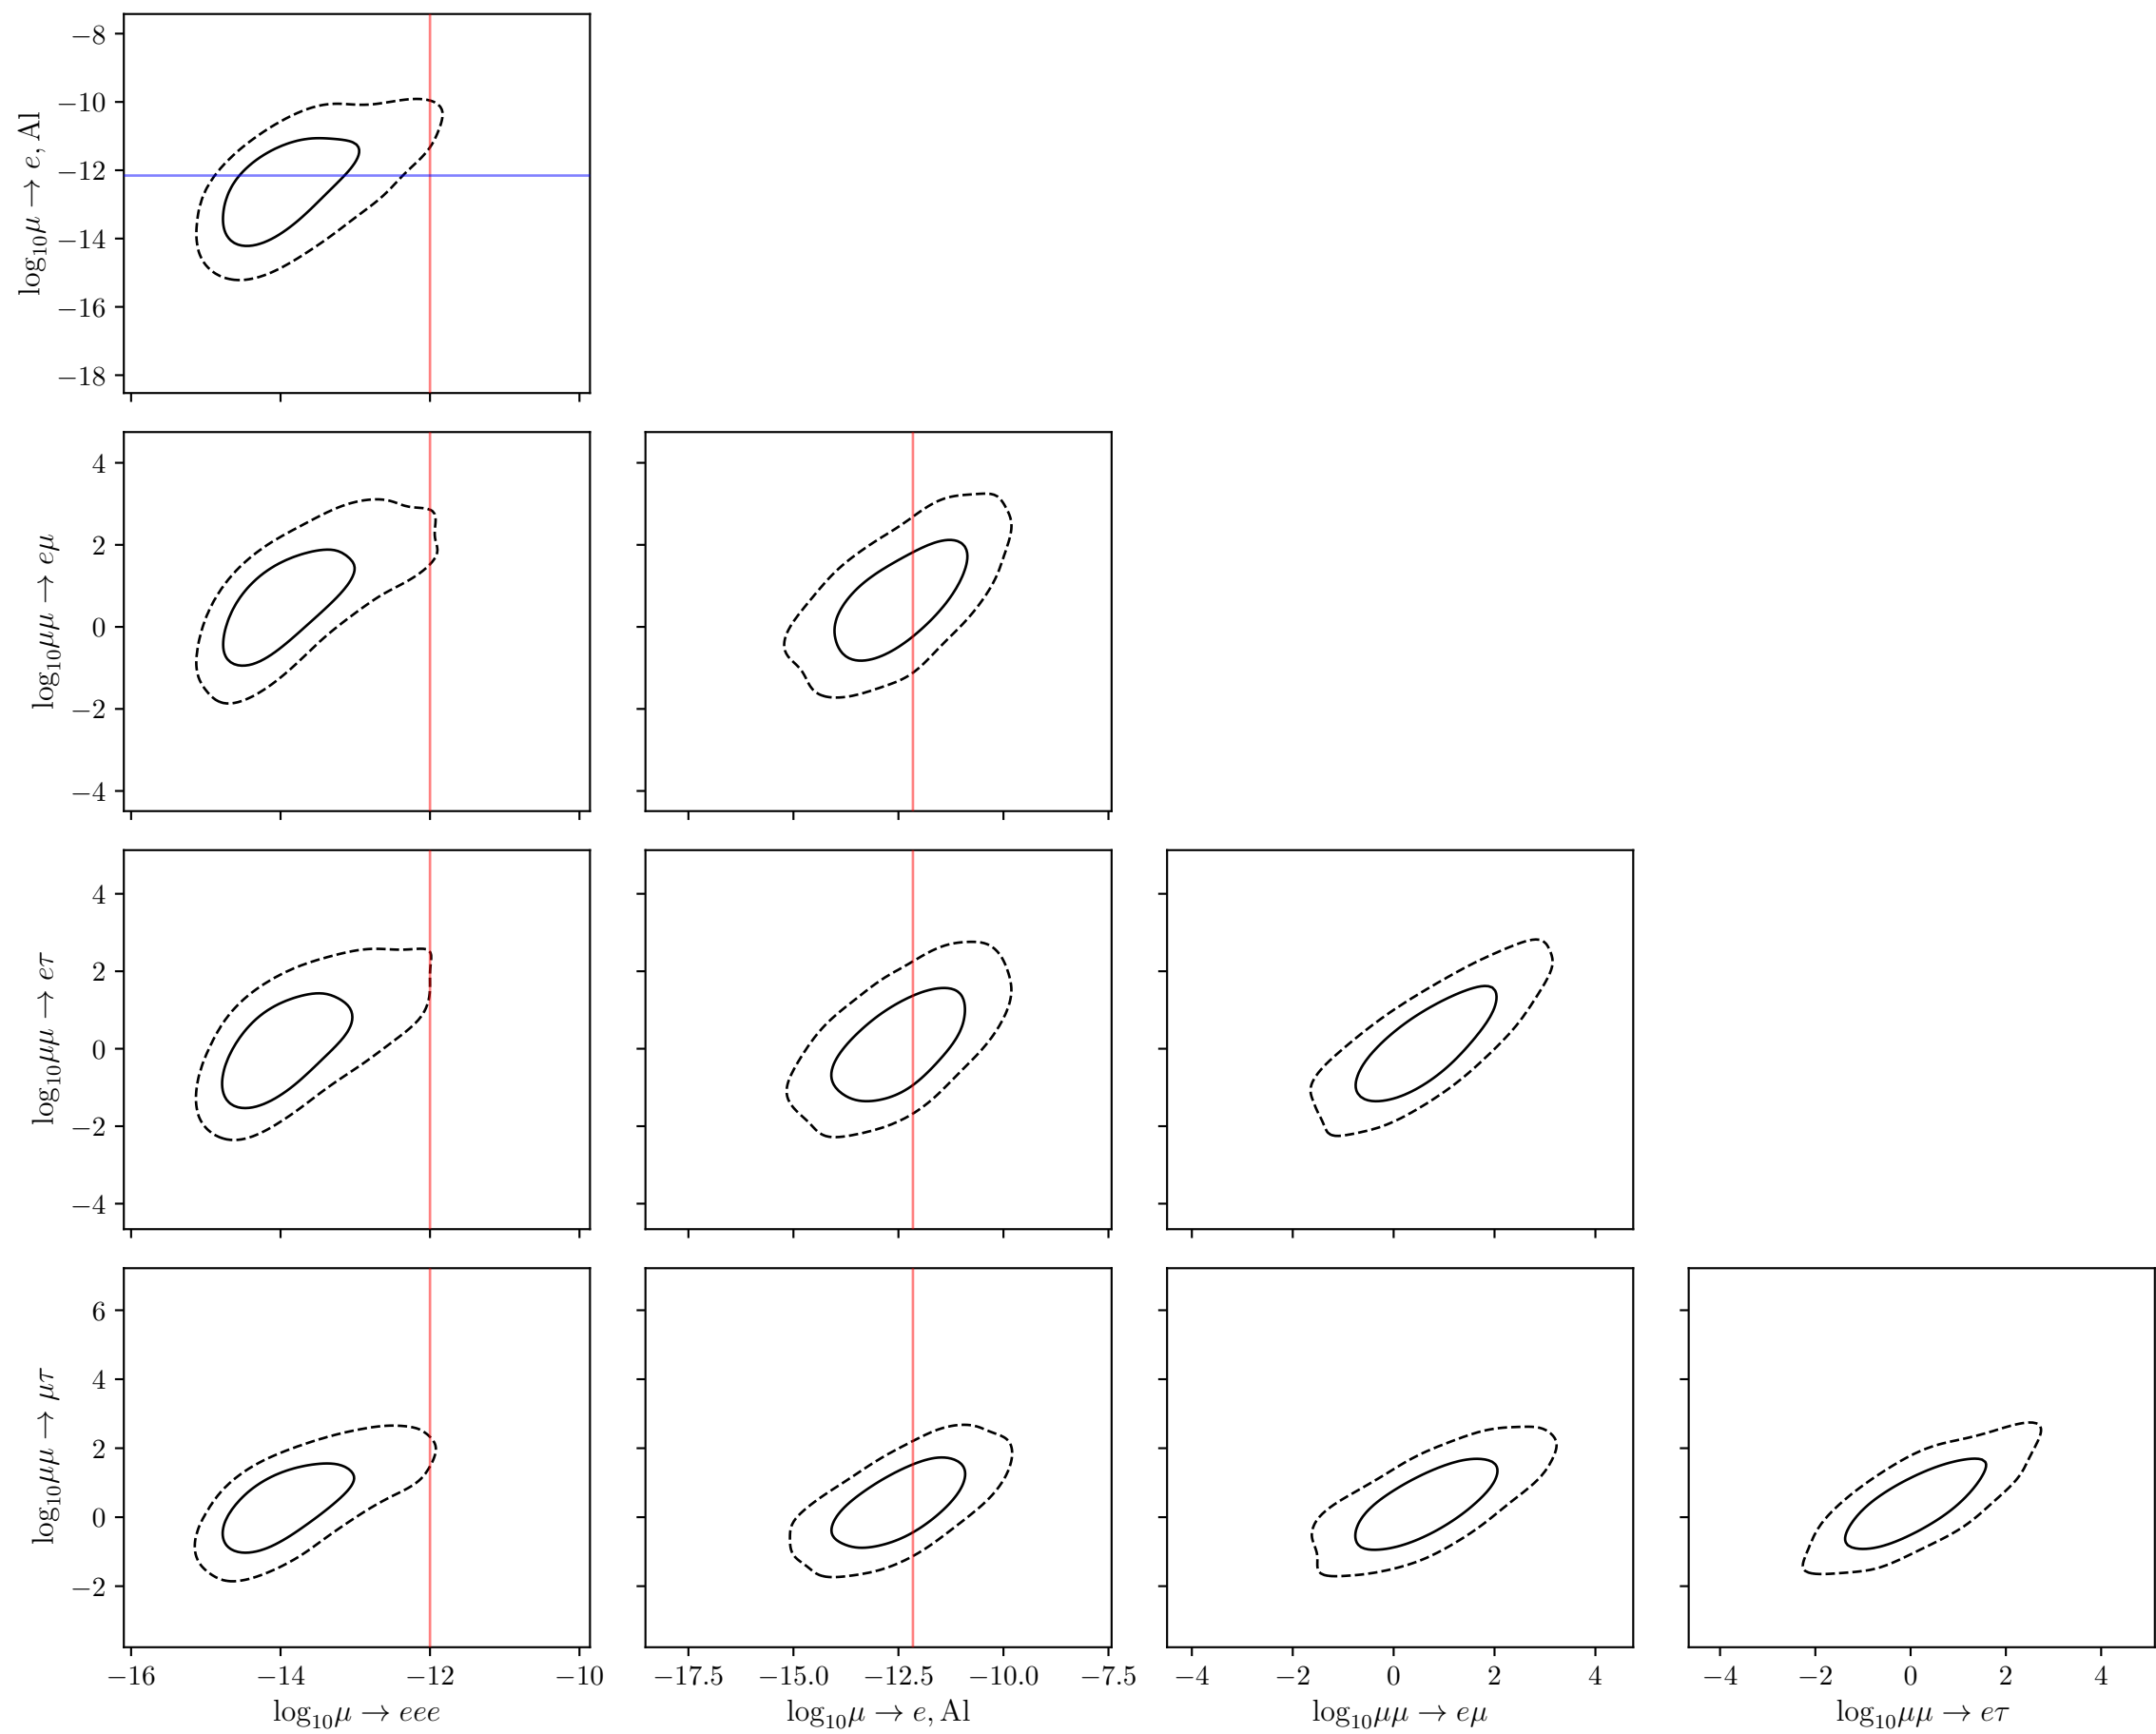

Majorana,  $X_L = \{4, 4, 3\}$ ,  $X_e = \{7, 3, 1\}$ ,

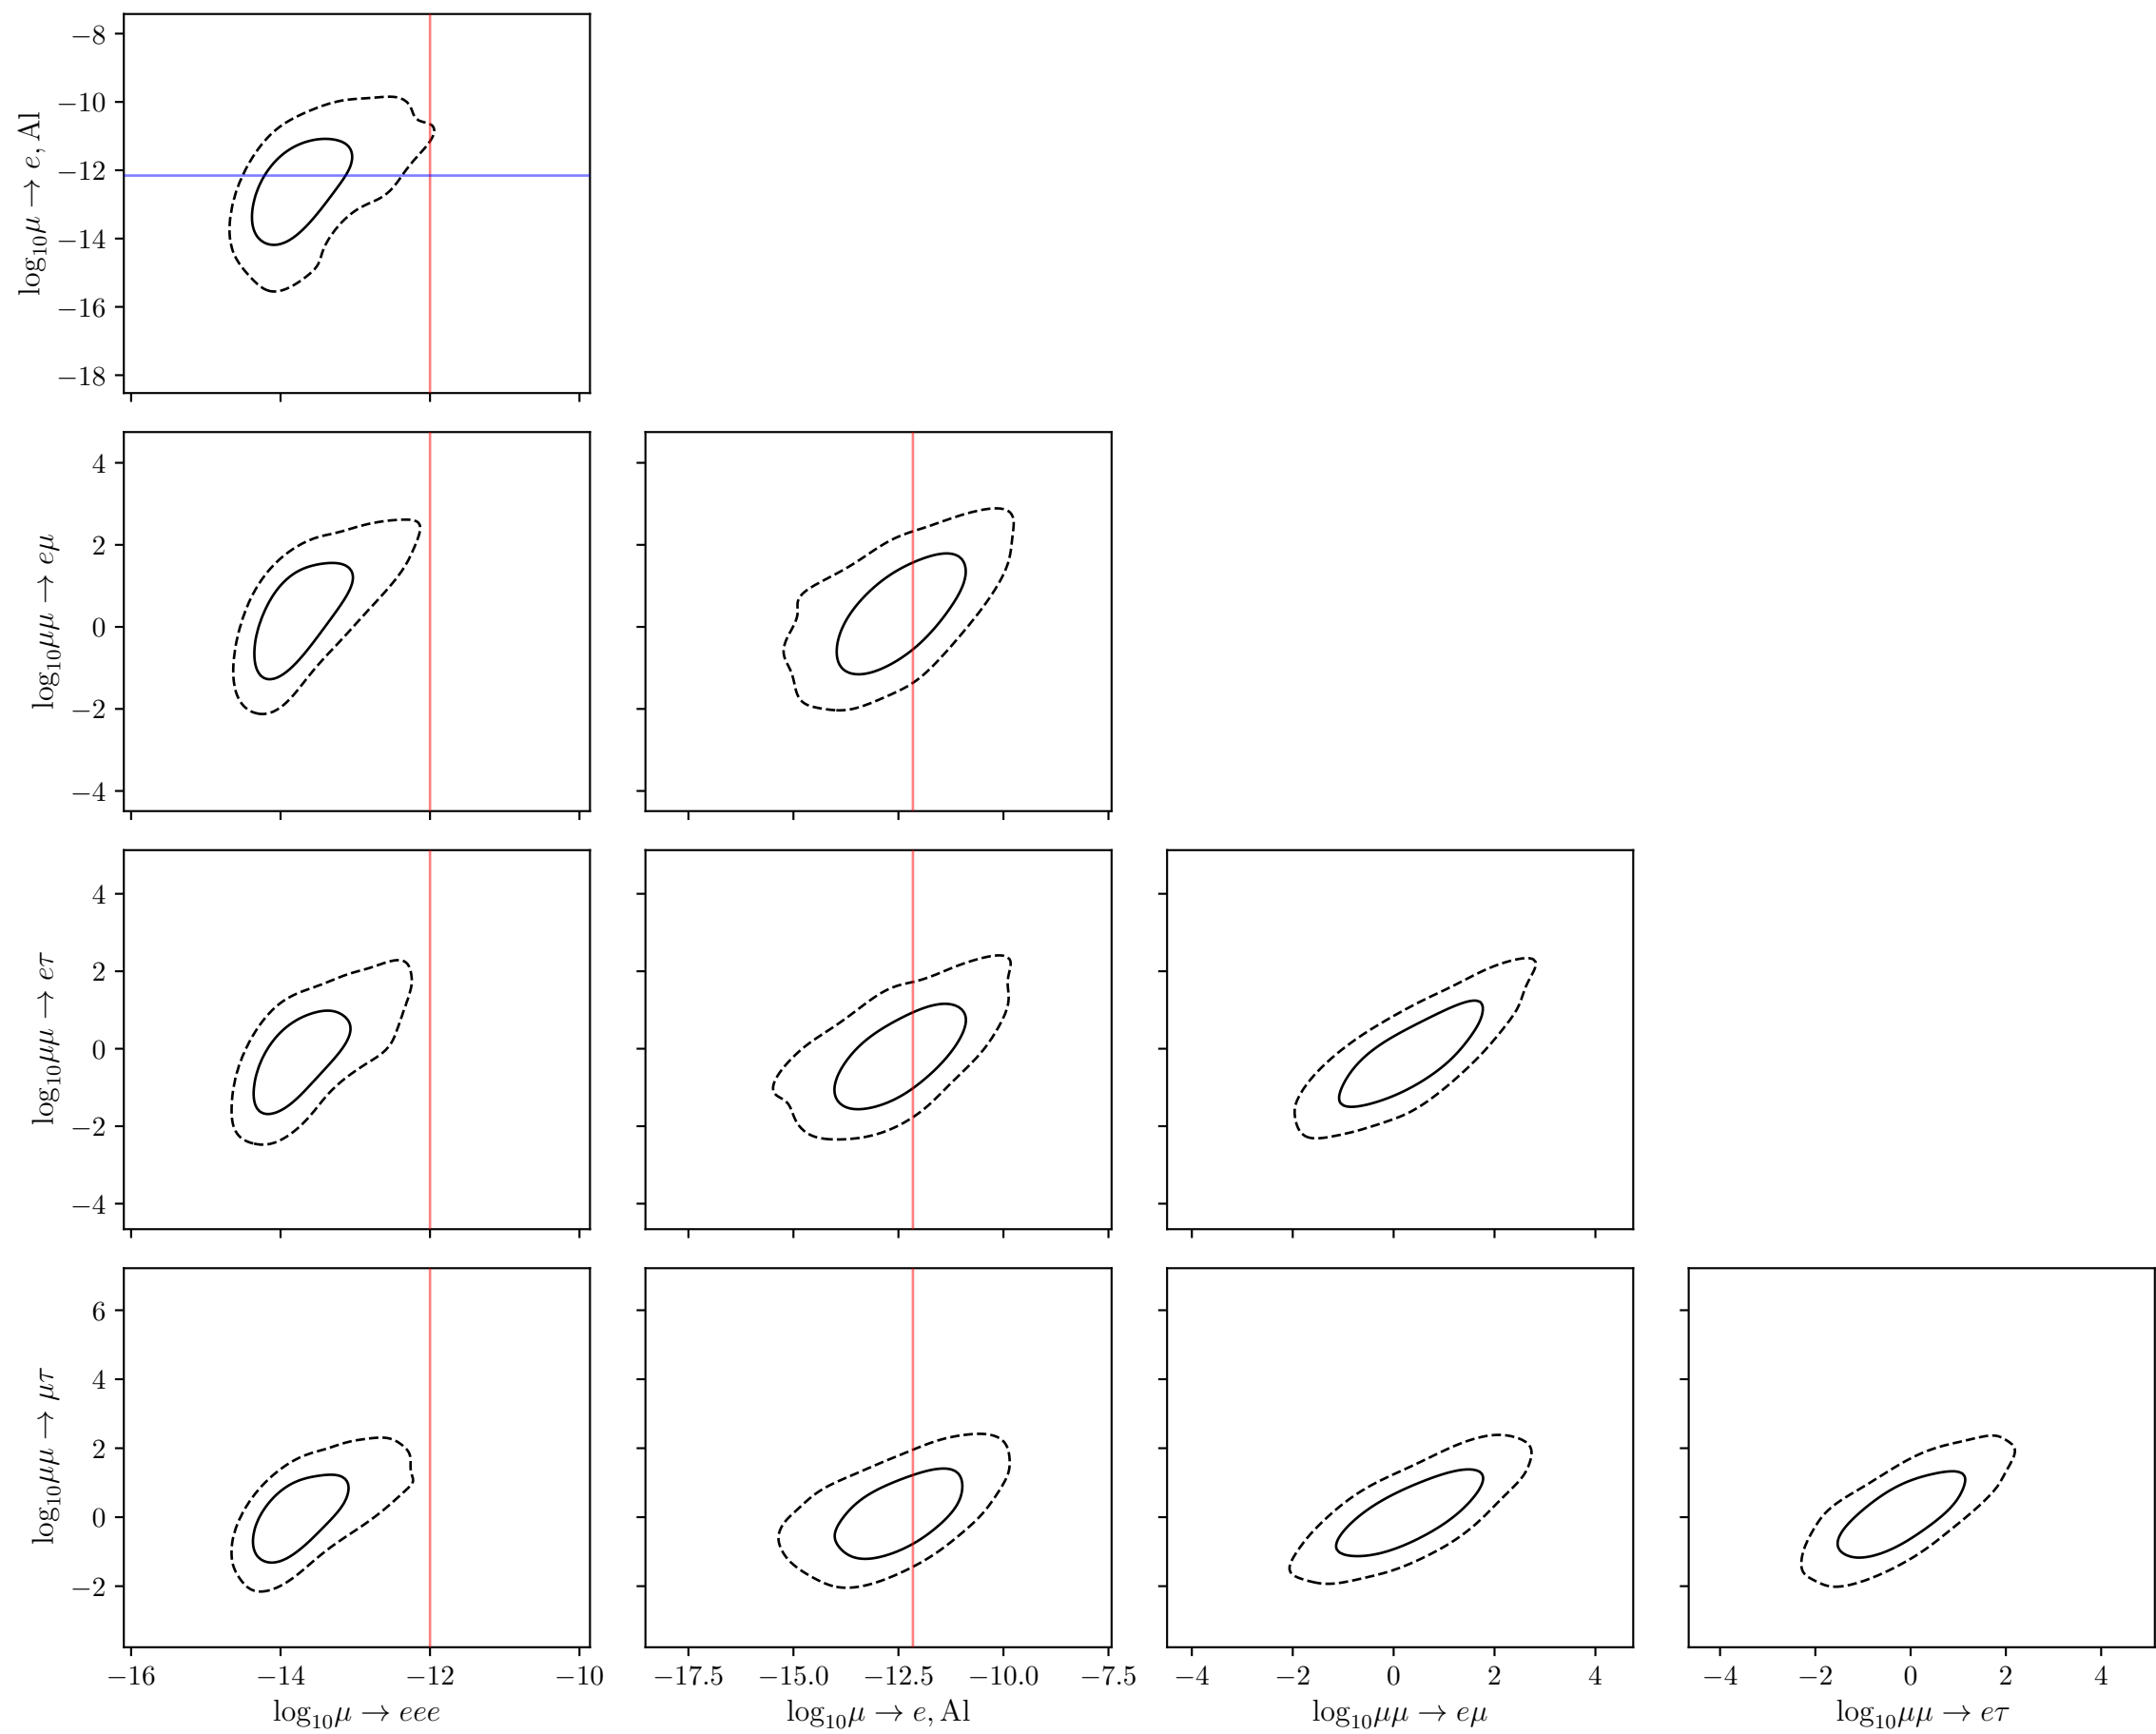

Majorana,  $X_L = \{7, 6, 5\}$ ,  $X_e = \{-1, 2, 6\}$ ,

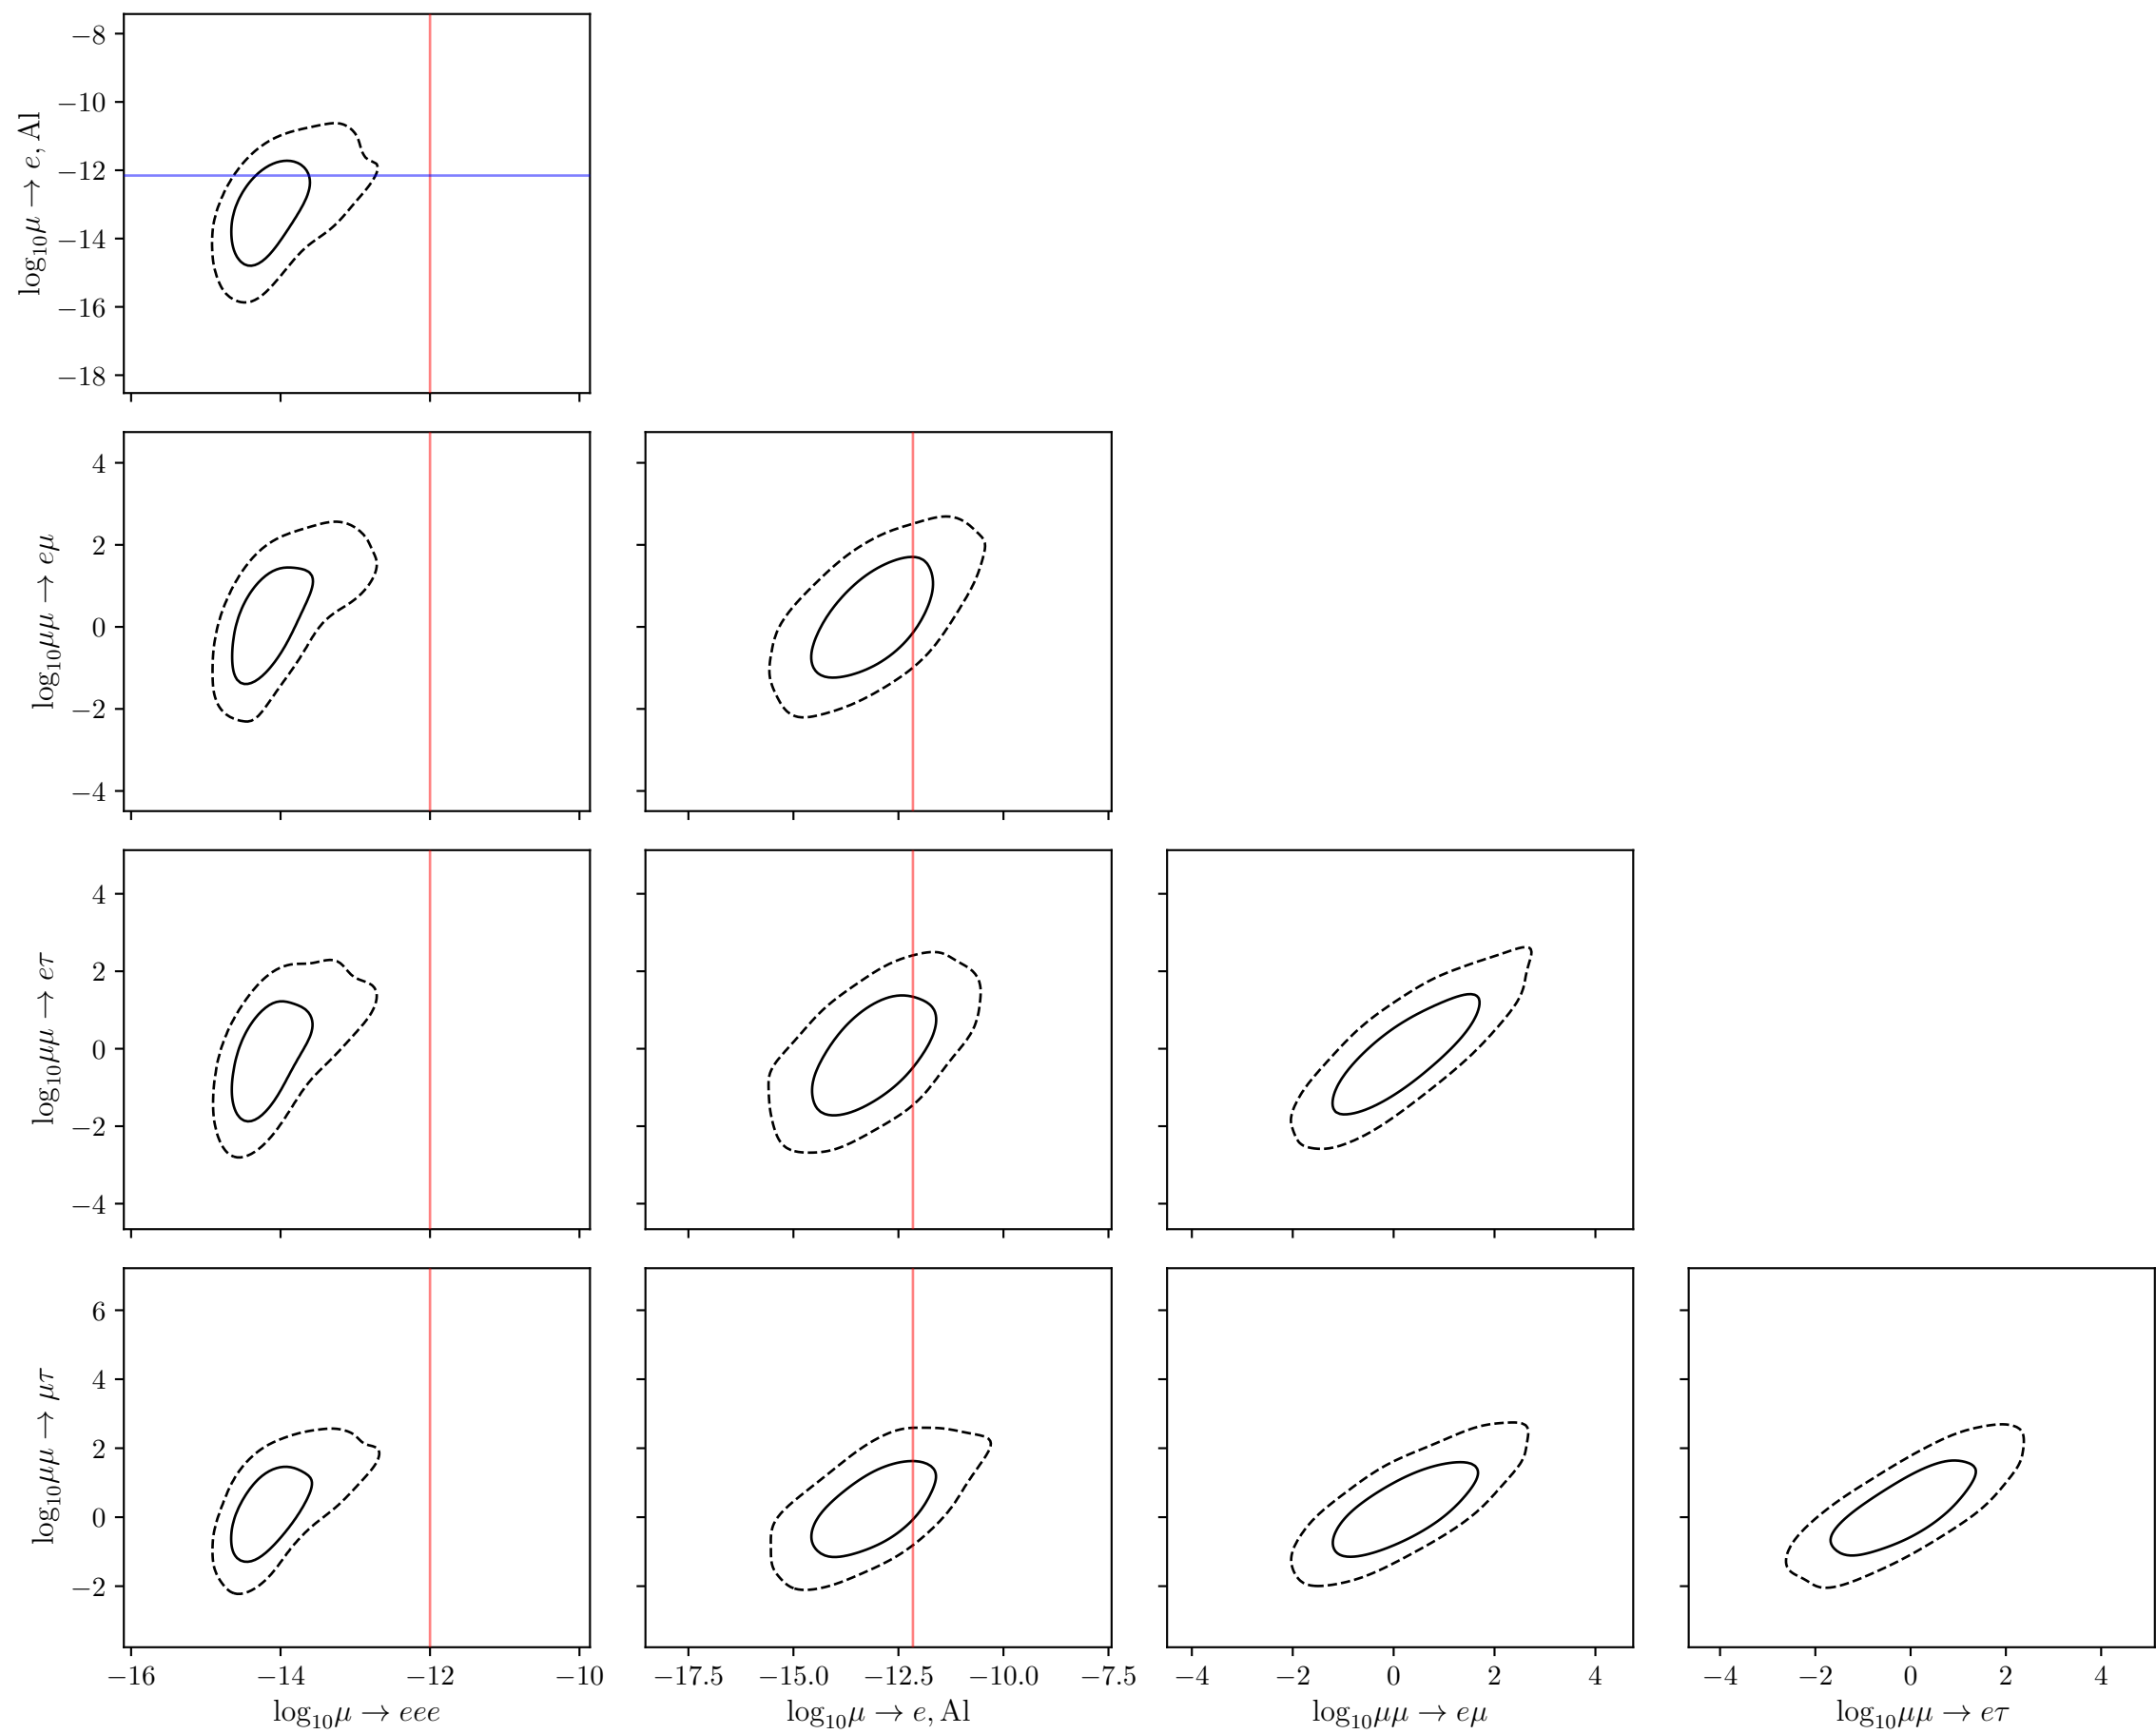

Majorana,  $X_L = \{7, 7, 6\}$ ,  $X_e = \{-1, 2, 6\}$ ,

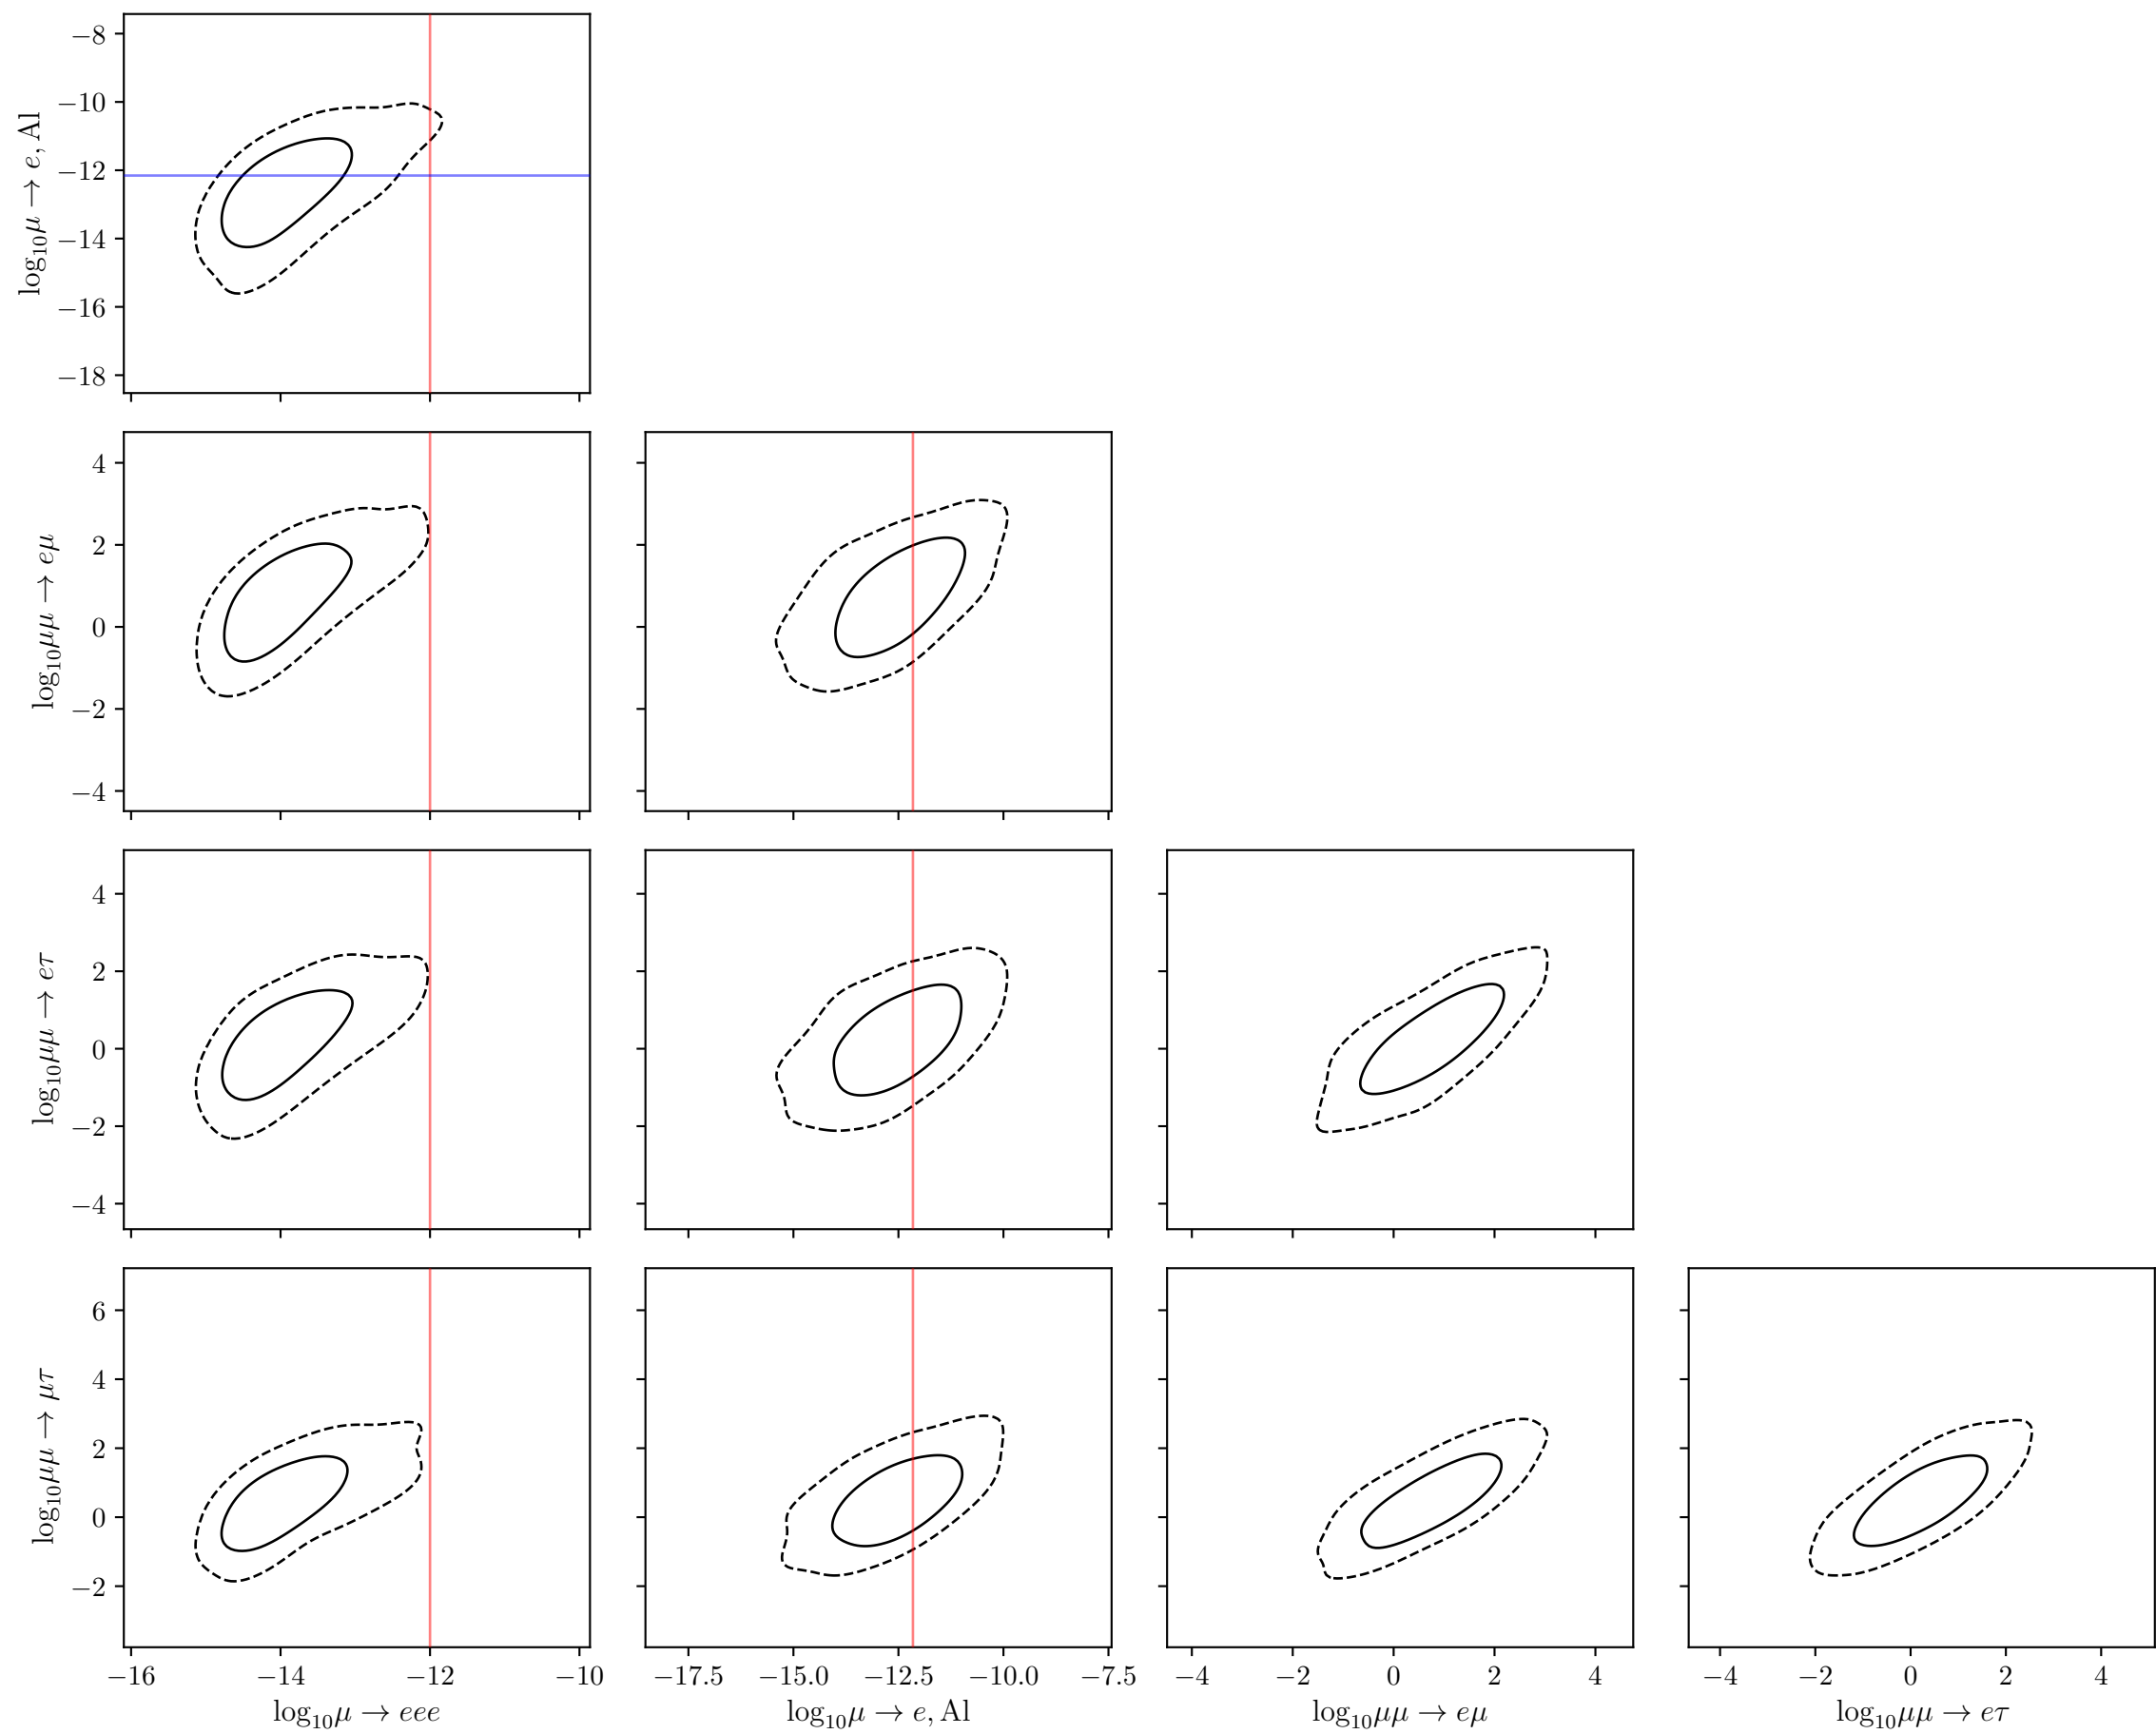

Majorana,  $X_L = \{3, 3, 2\}$ ,  $X_e = \{7, 4, 2\}$ ,

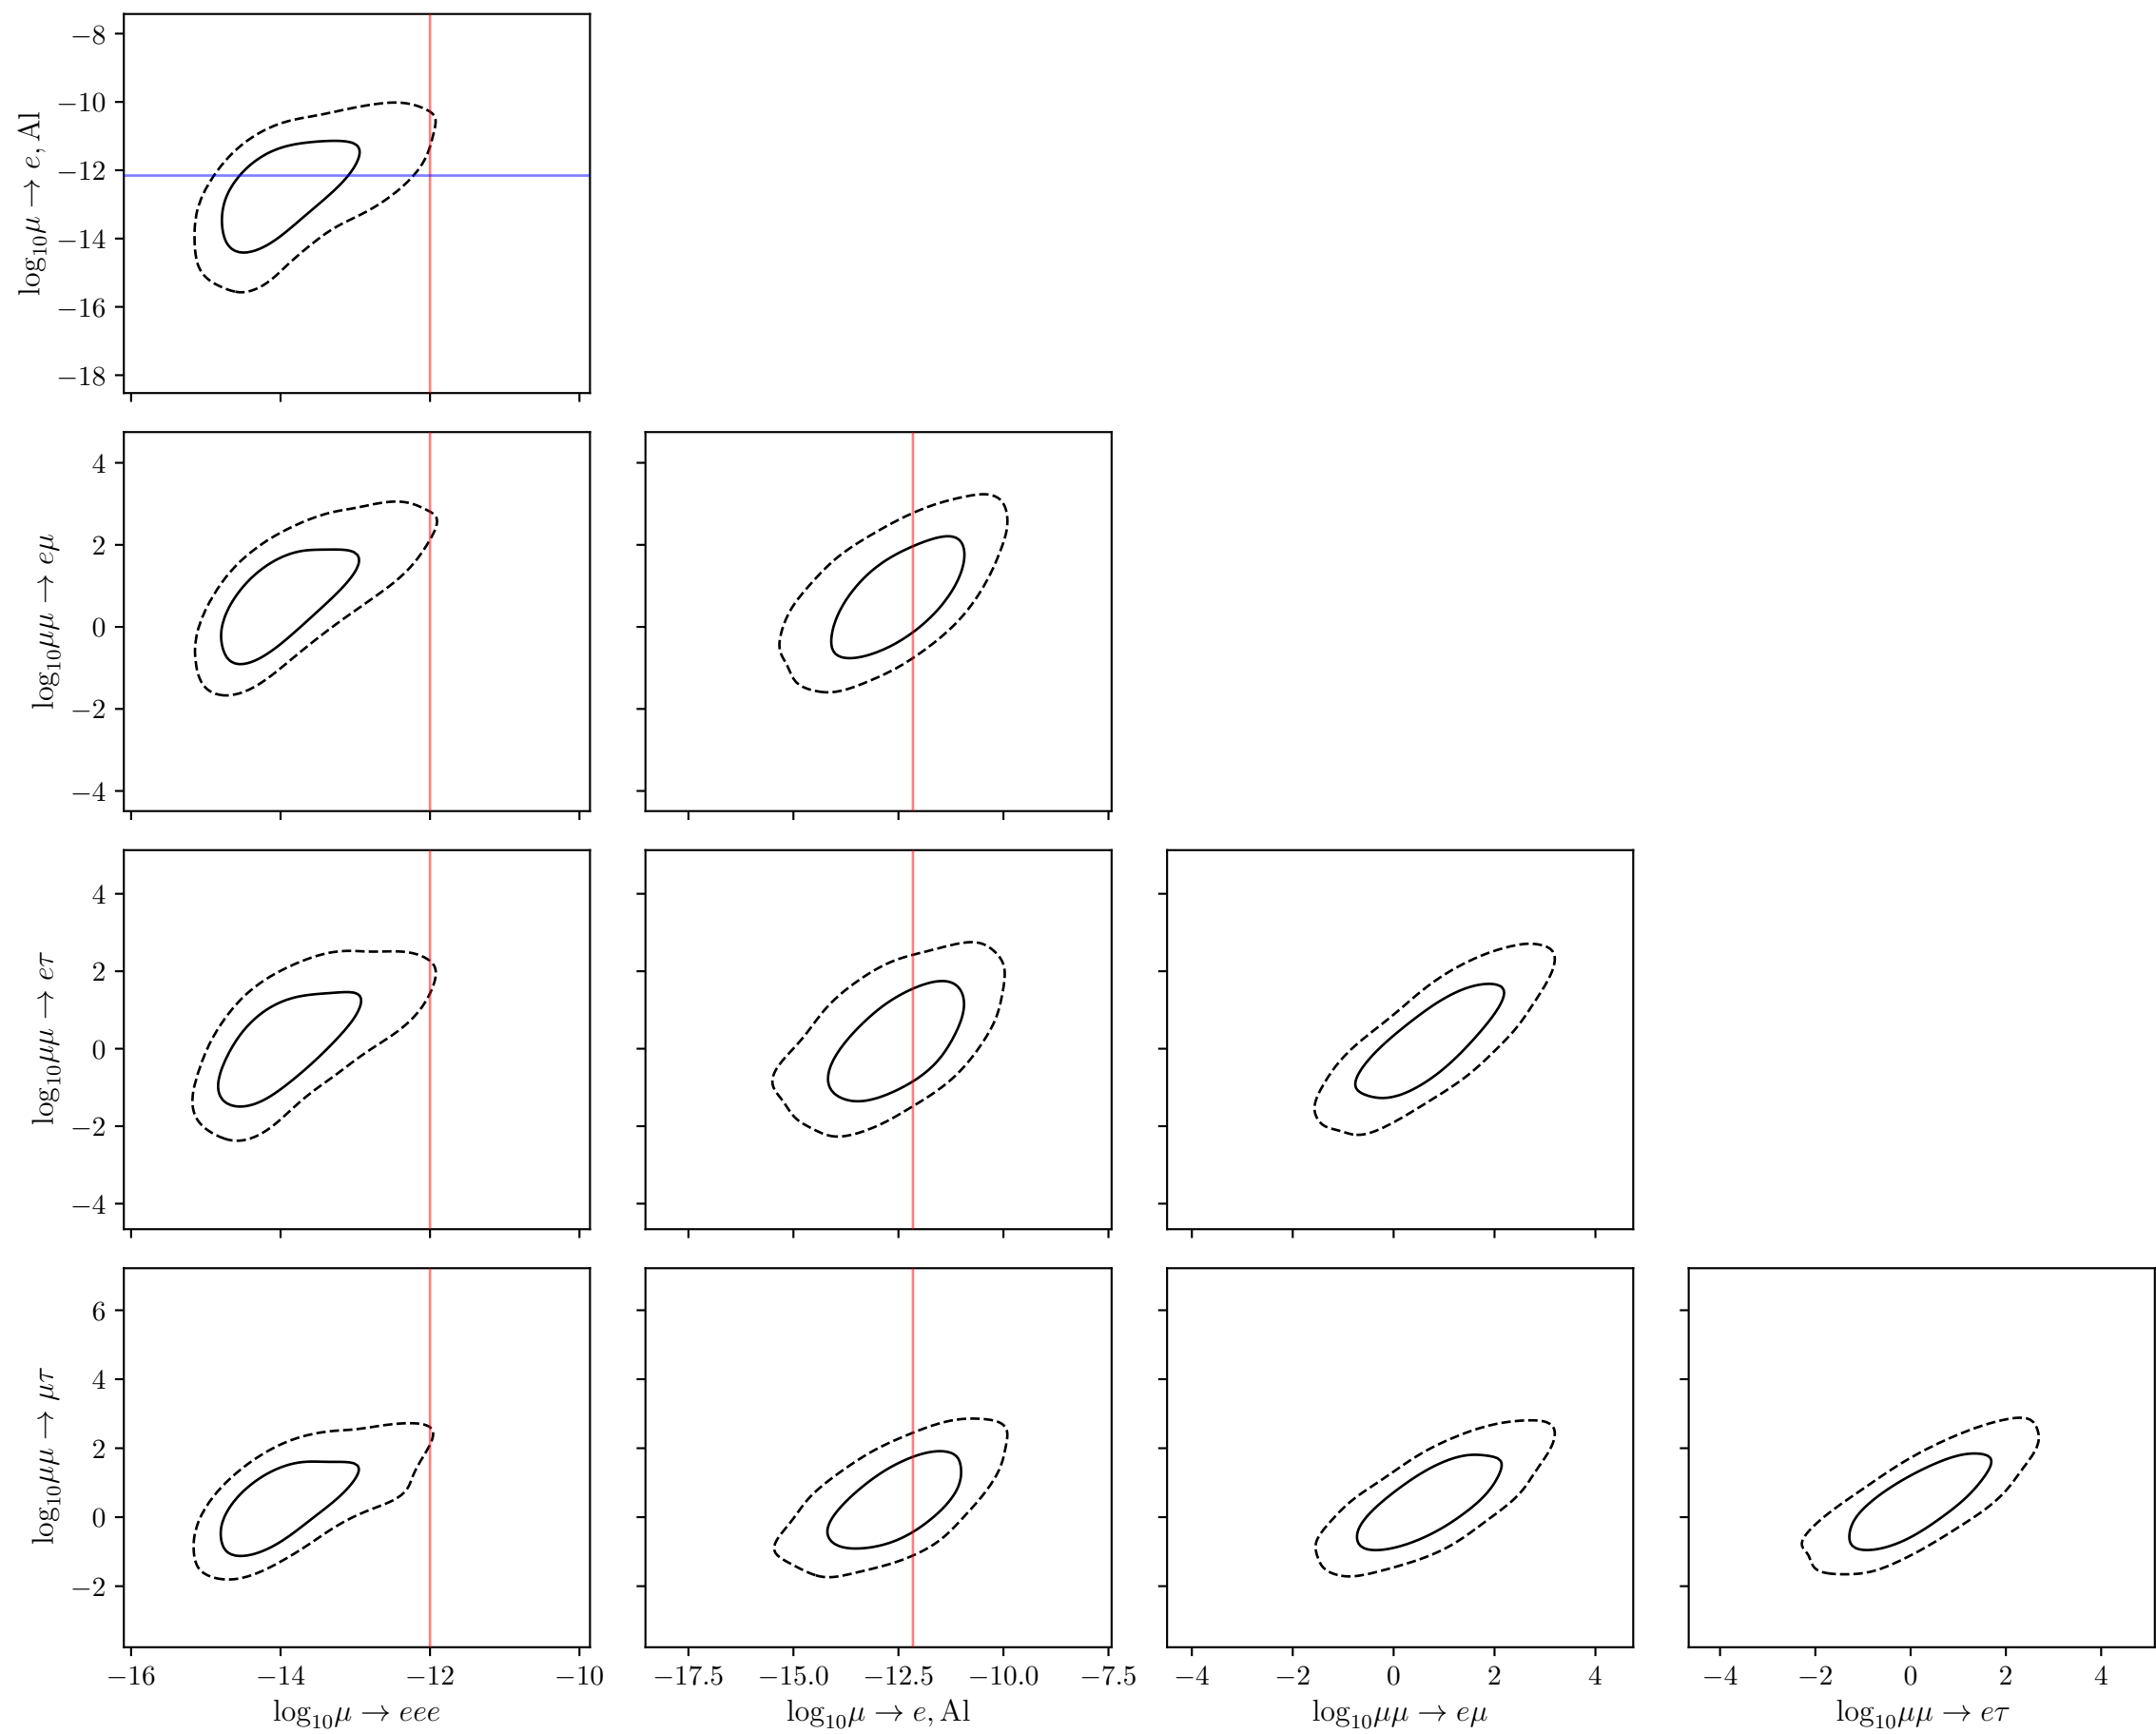

Majorana,  $X_L = \{5, -2, -2\}$ ,  $X_e = \{-1, 0, 6\}$ ,

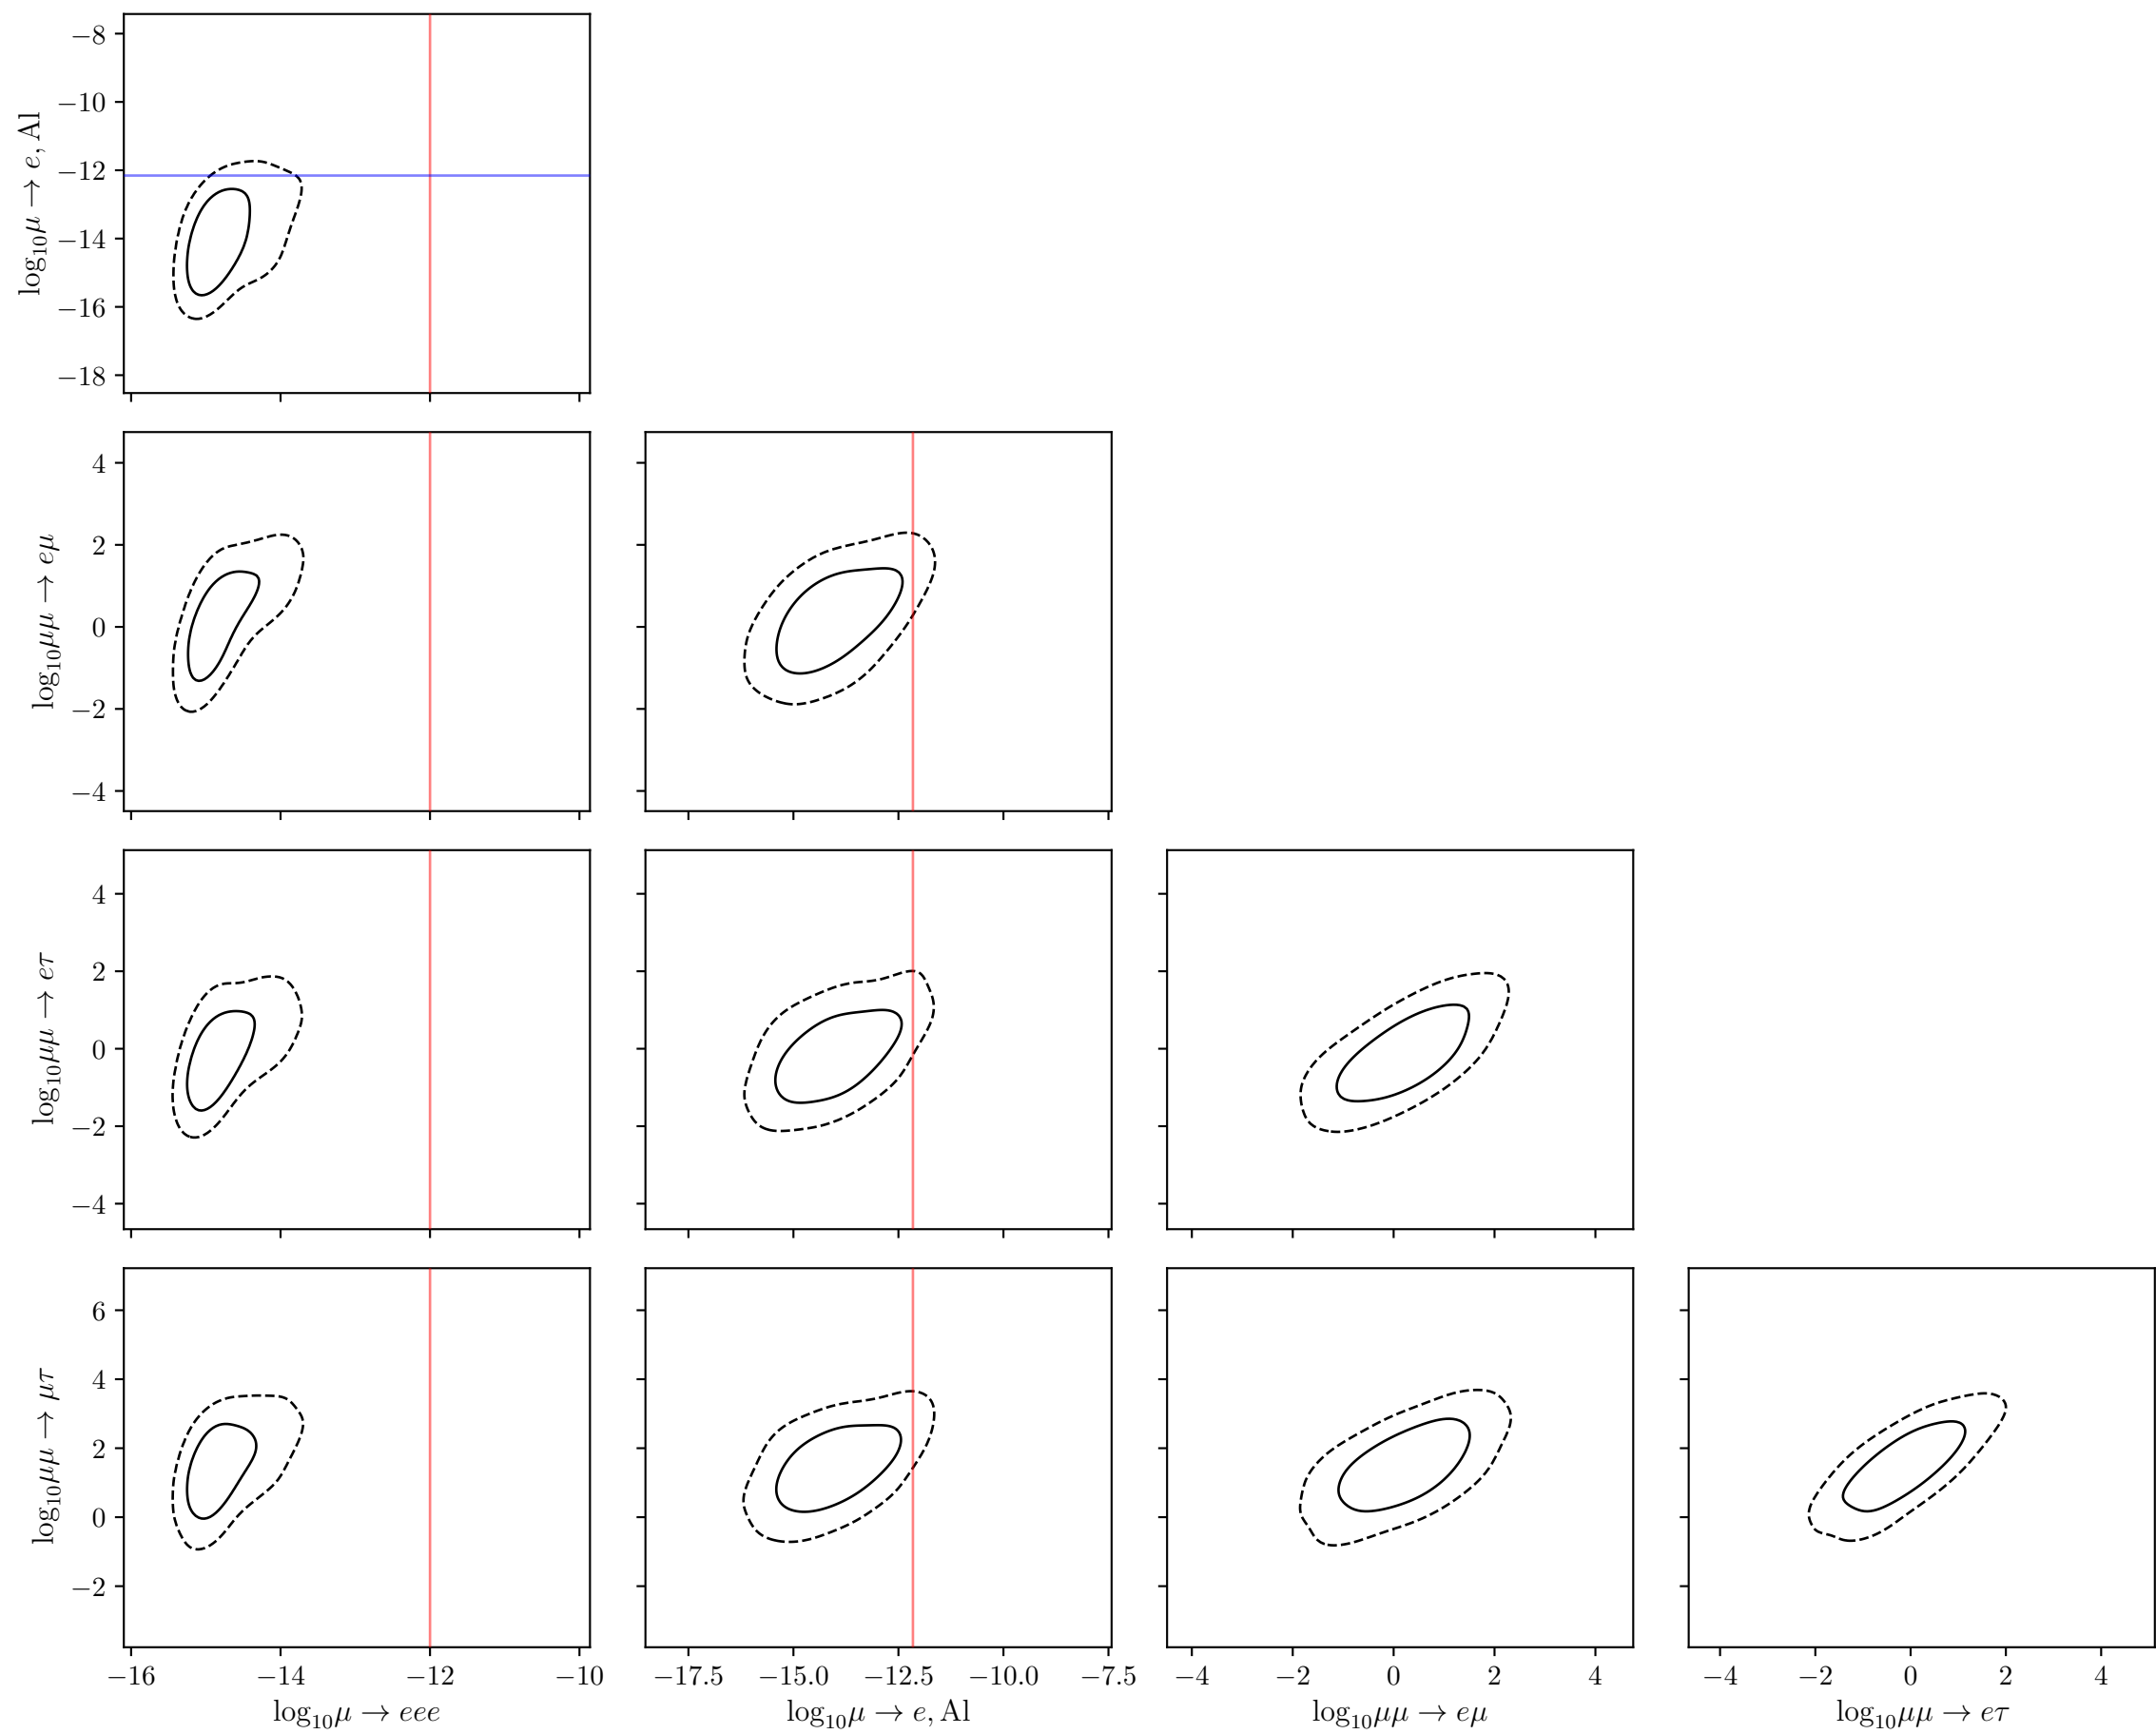

Majorana,  $X_L = \{6, 6, 5\}$ ,  $X_e = \{7, 2, 0\}$ ,

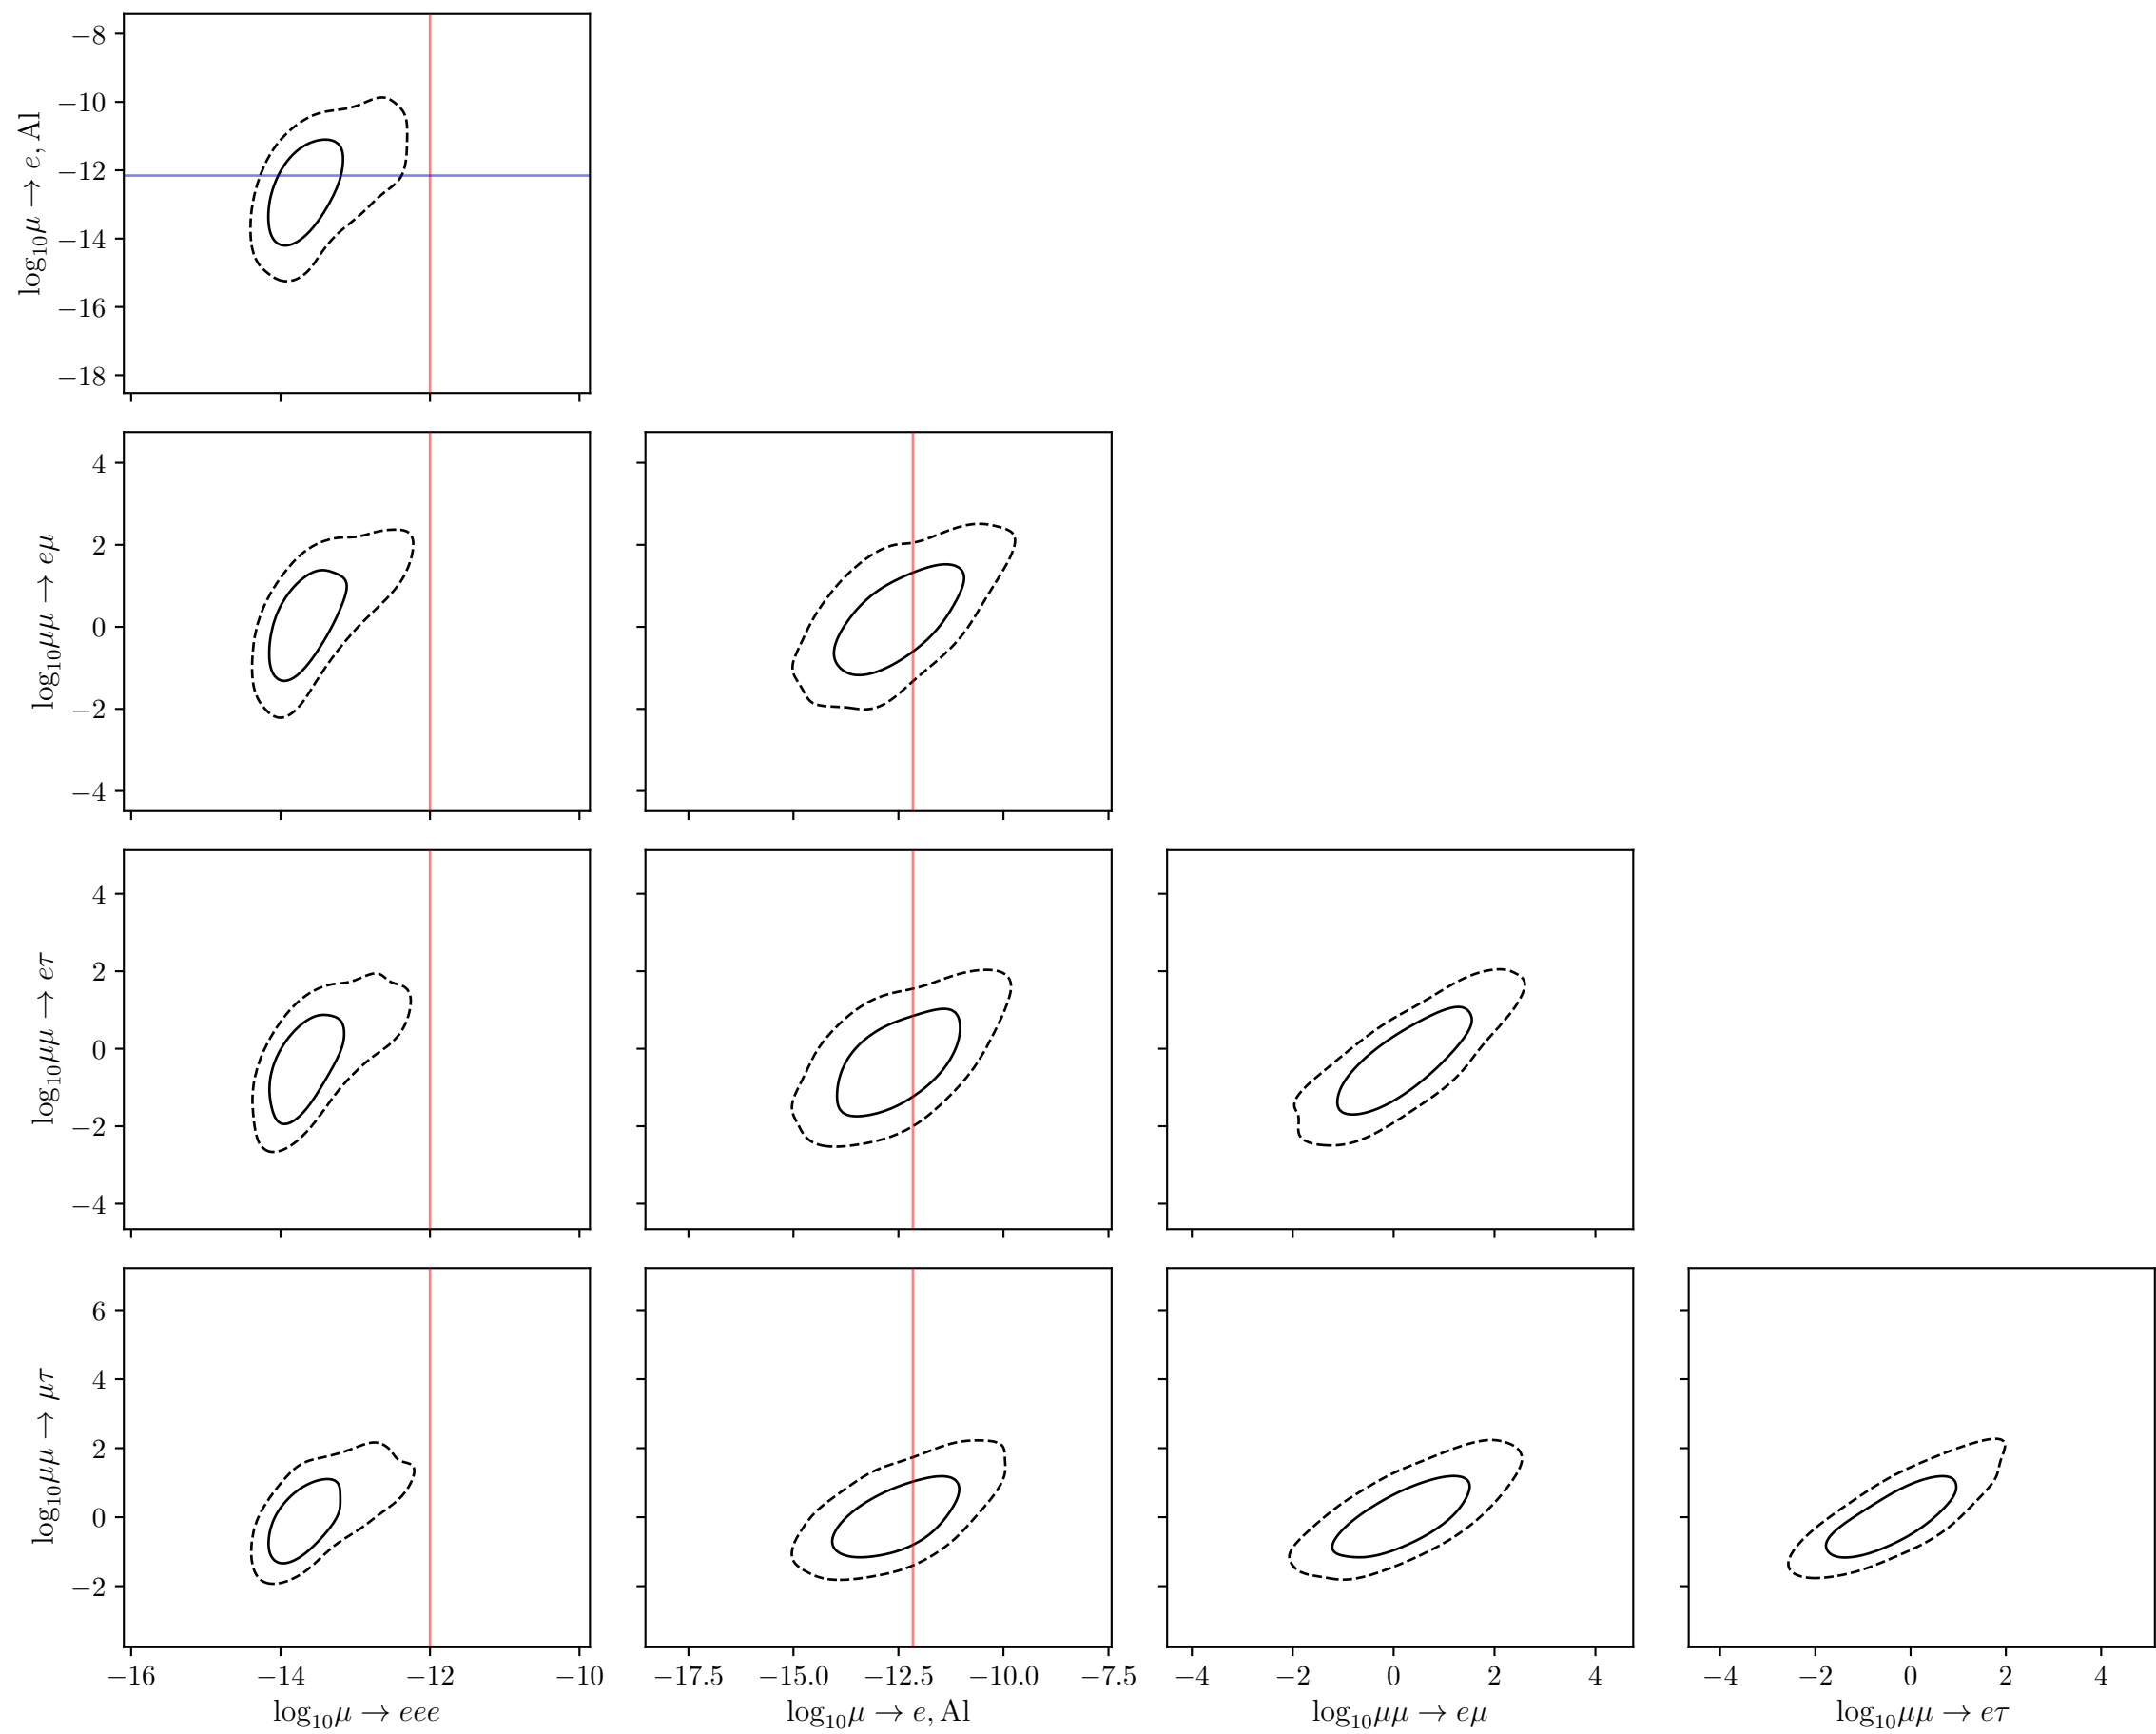



Majorana,  $X_L = \{1, 1, 0\}$ ,  $X_e = \{7, 4, 3\}$ ,

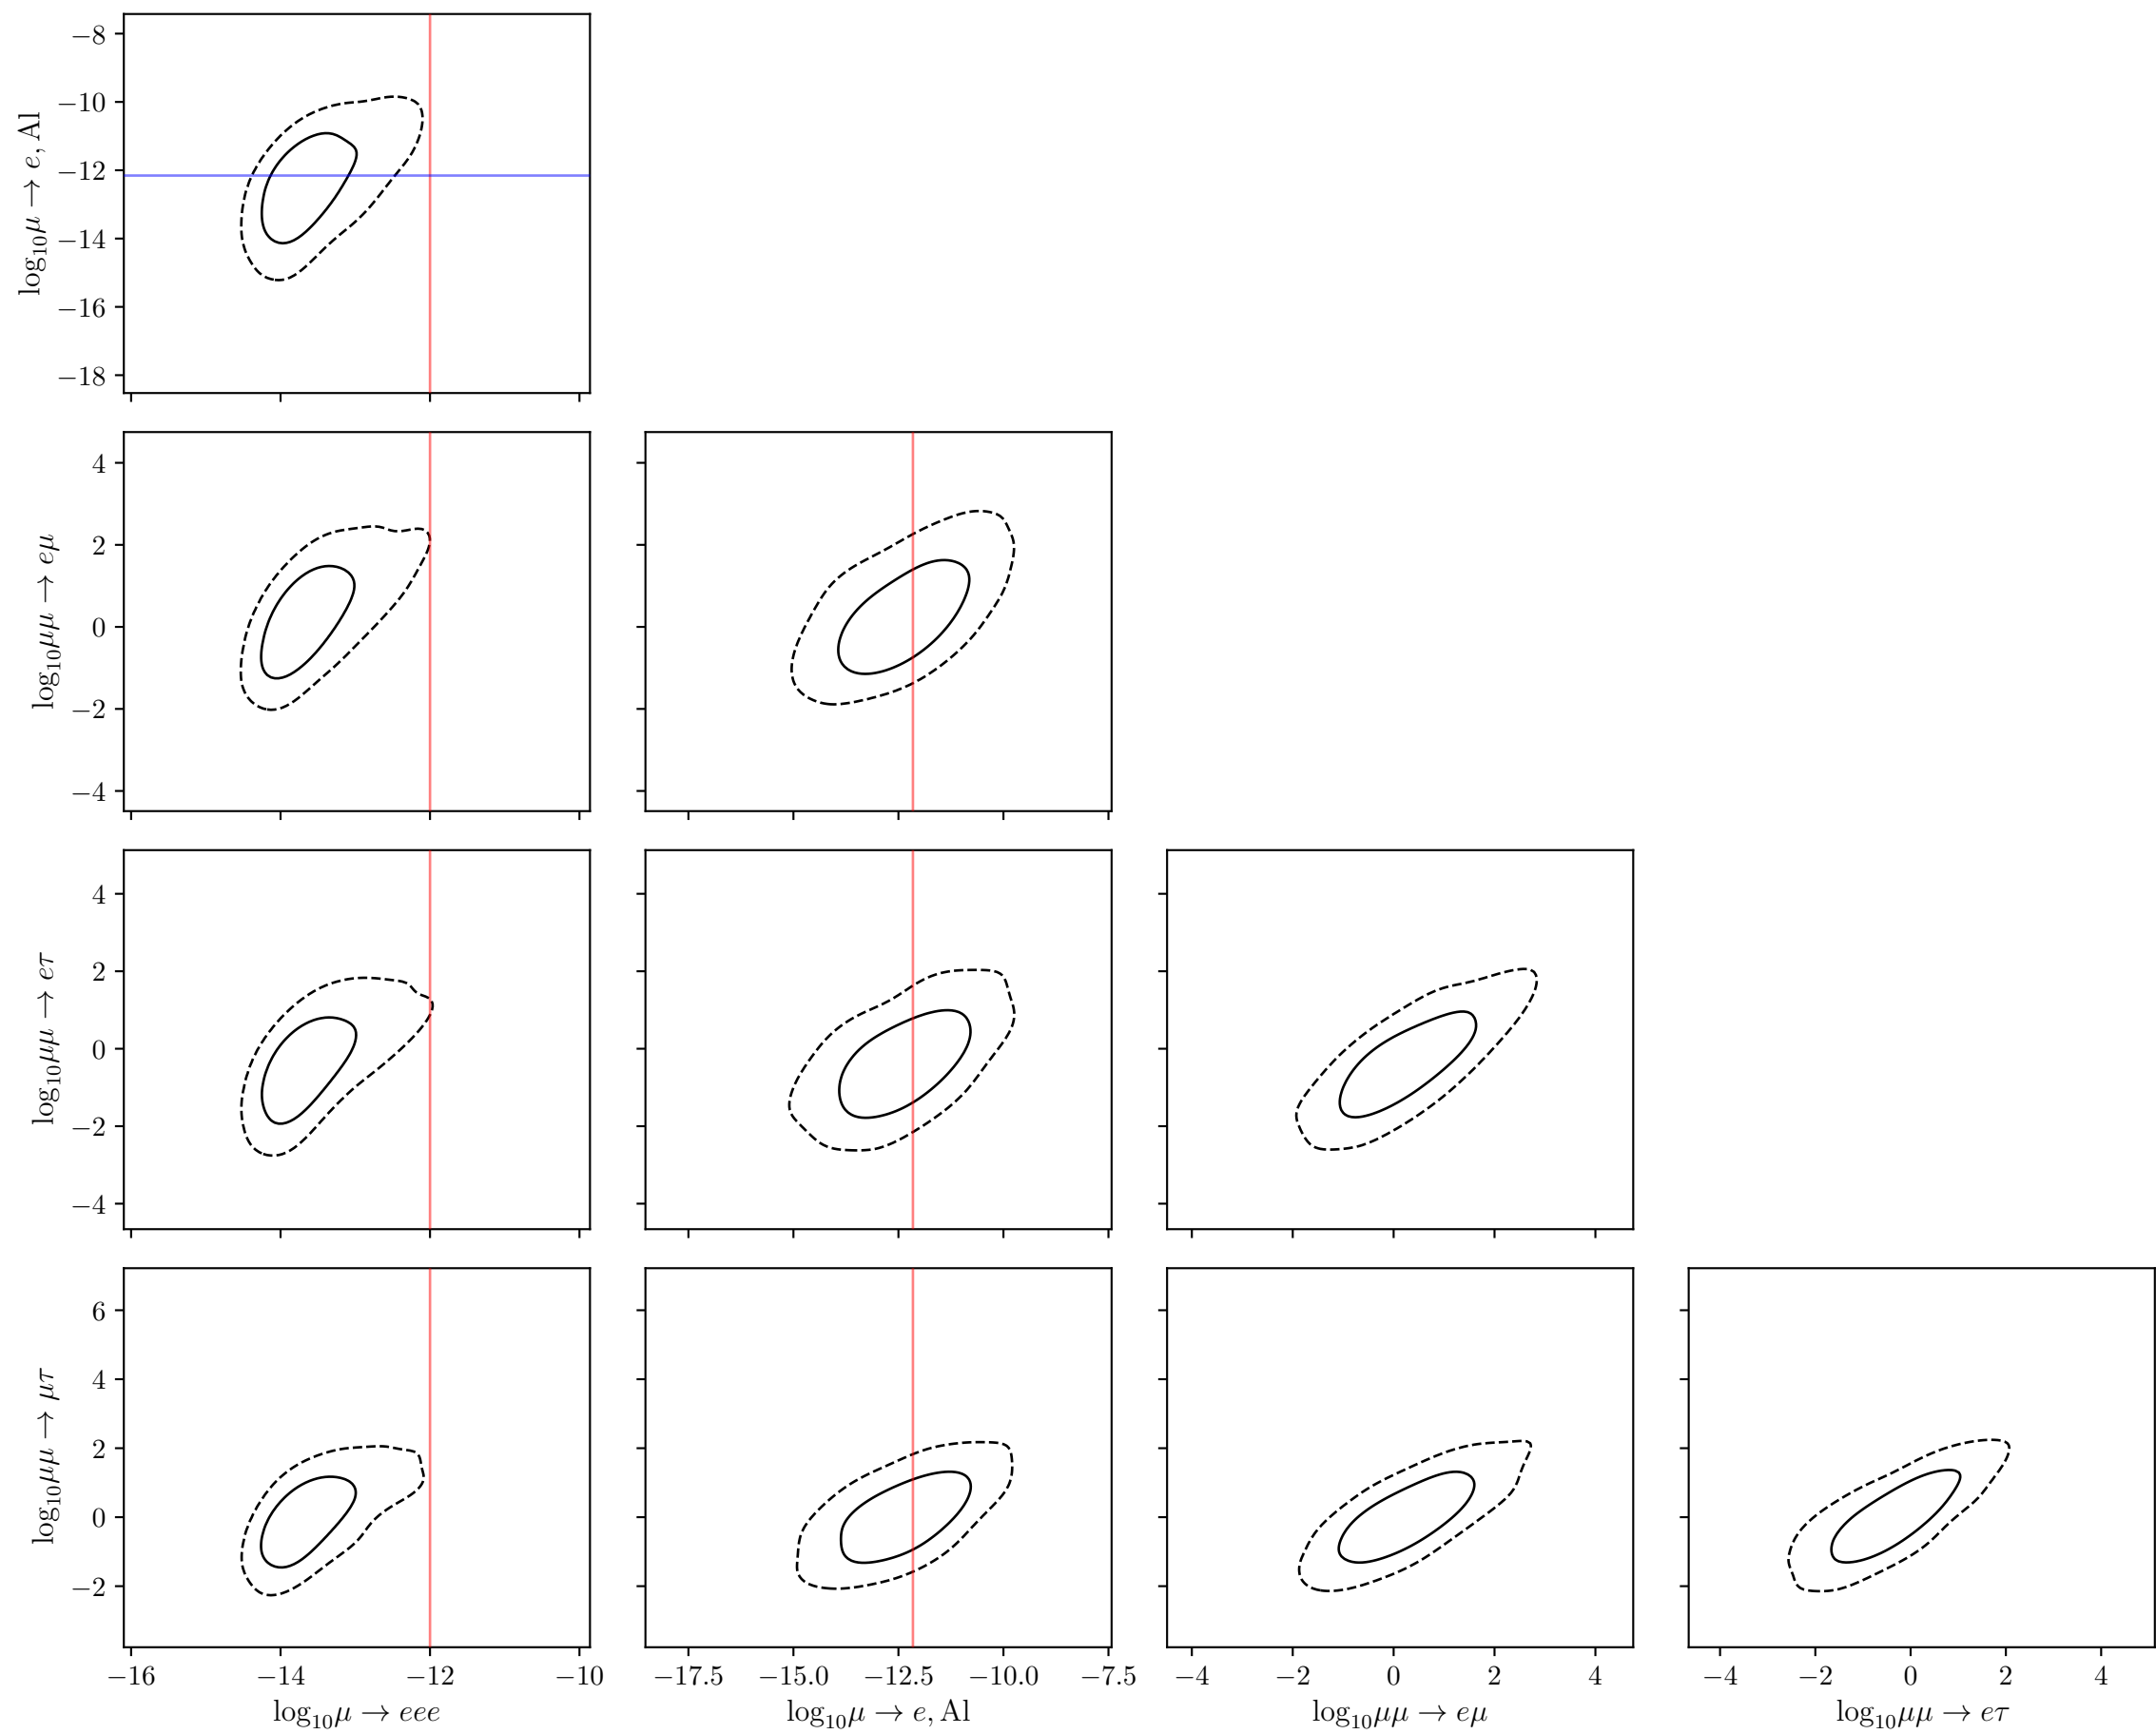

Majorana,  $X_L = \{6, 5, 4\}$ ,  $X_e = \{-1, 1, 4\}$ ,

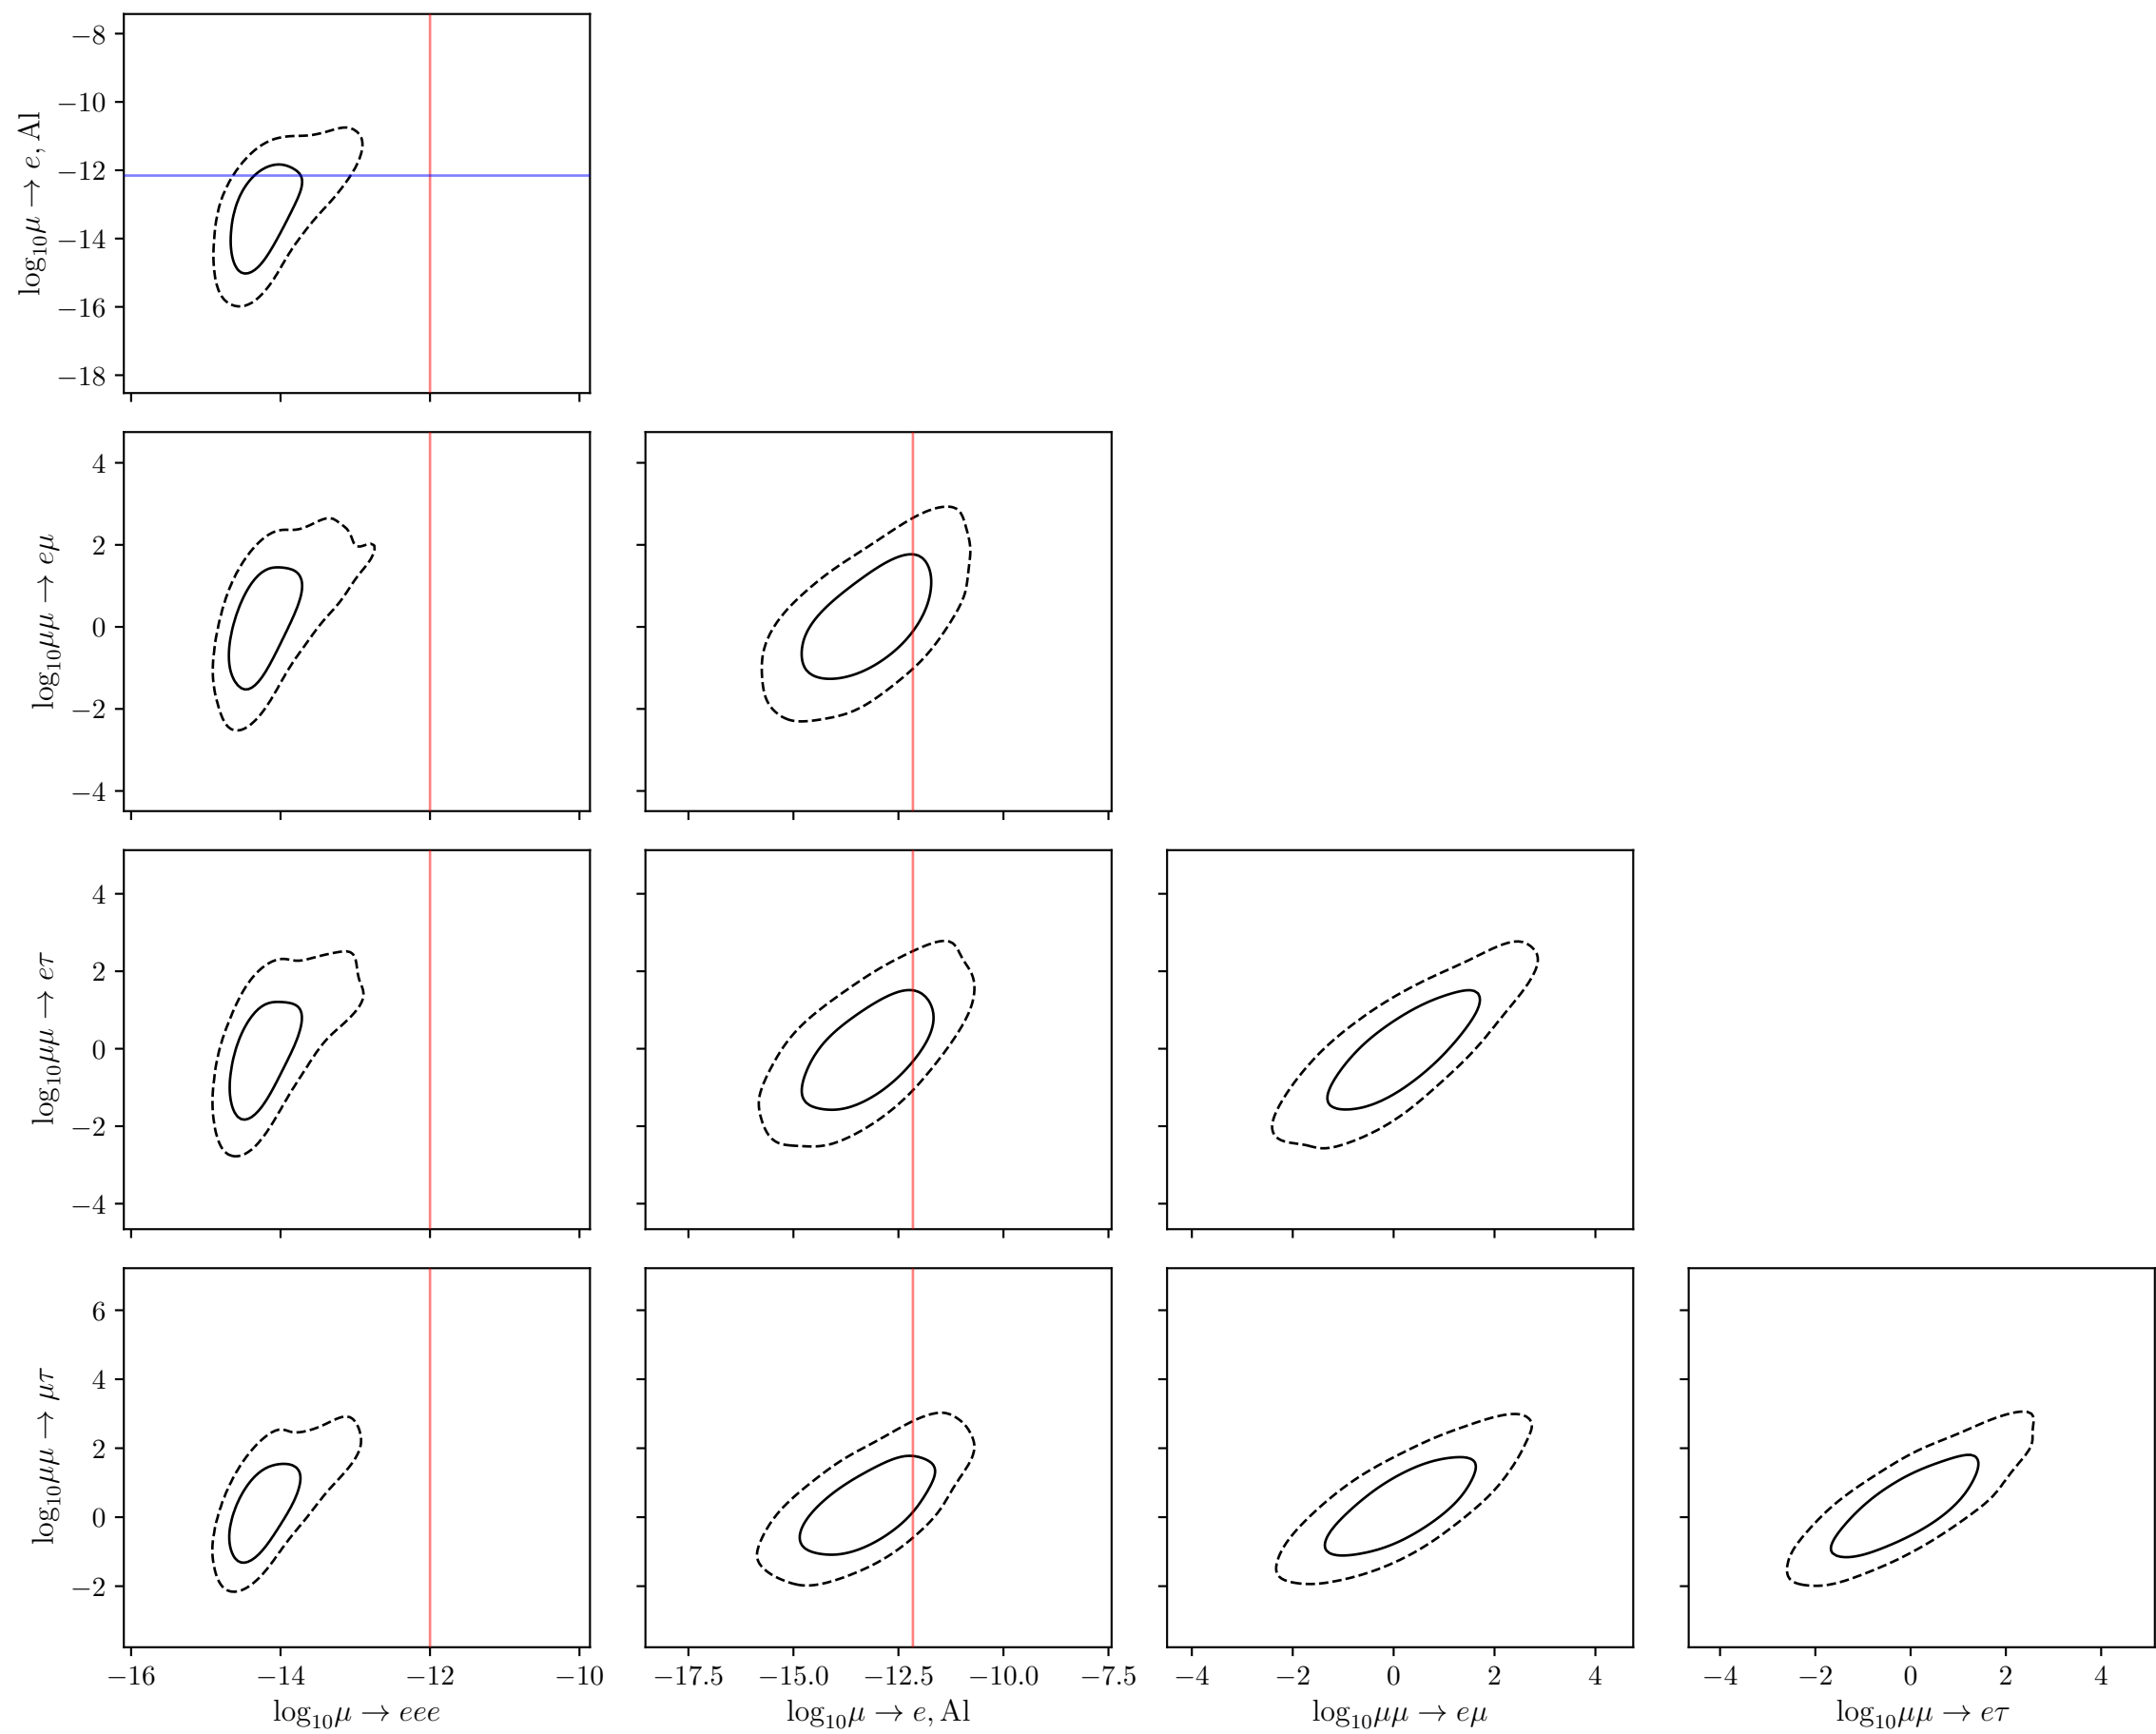

Majorana,  $X_L = \{7, 6, 5\}$ ,  $X_e = \{-2, 0, 3\}$ ,

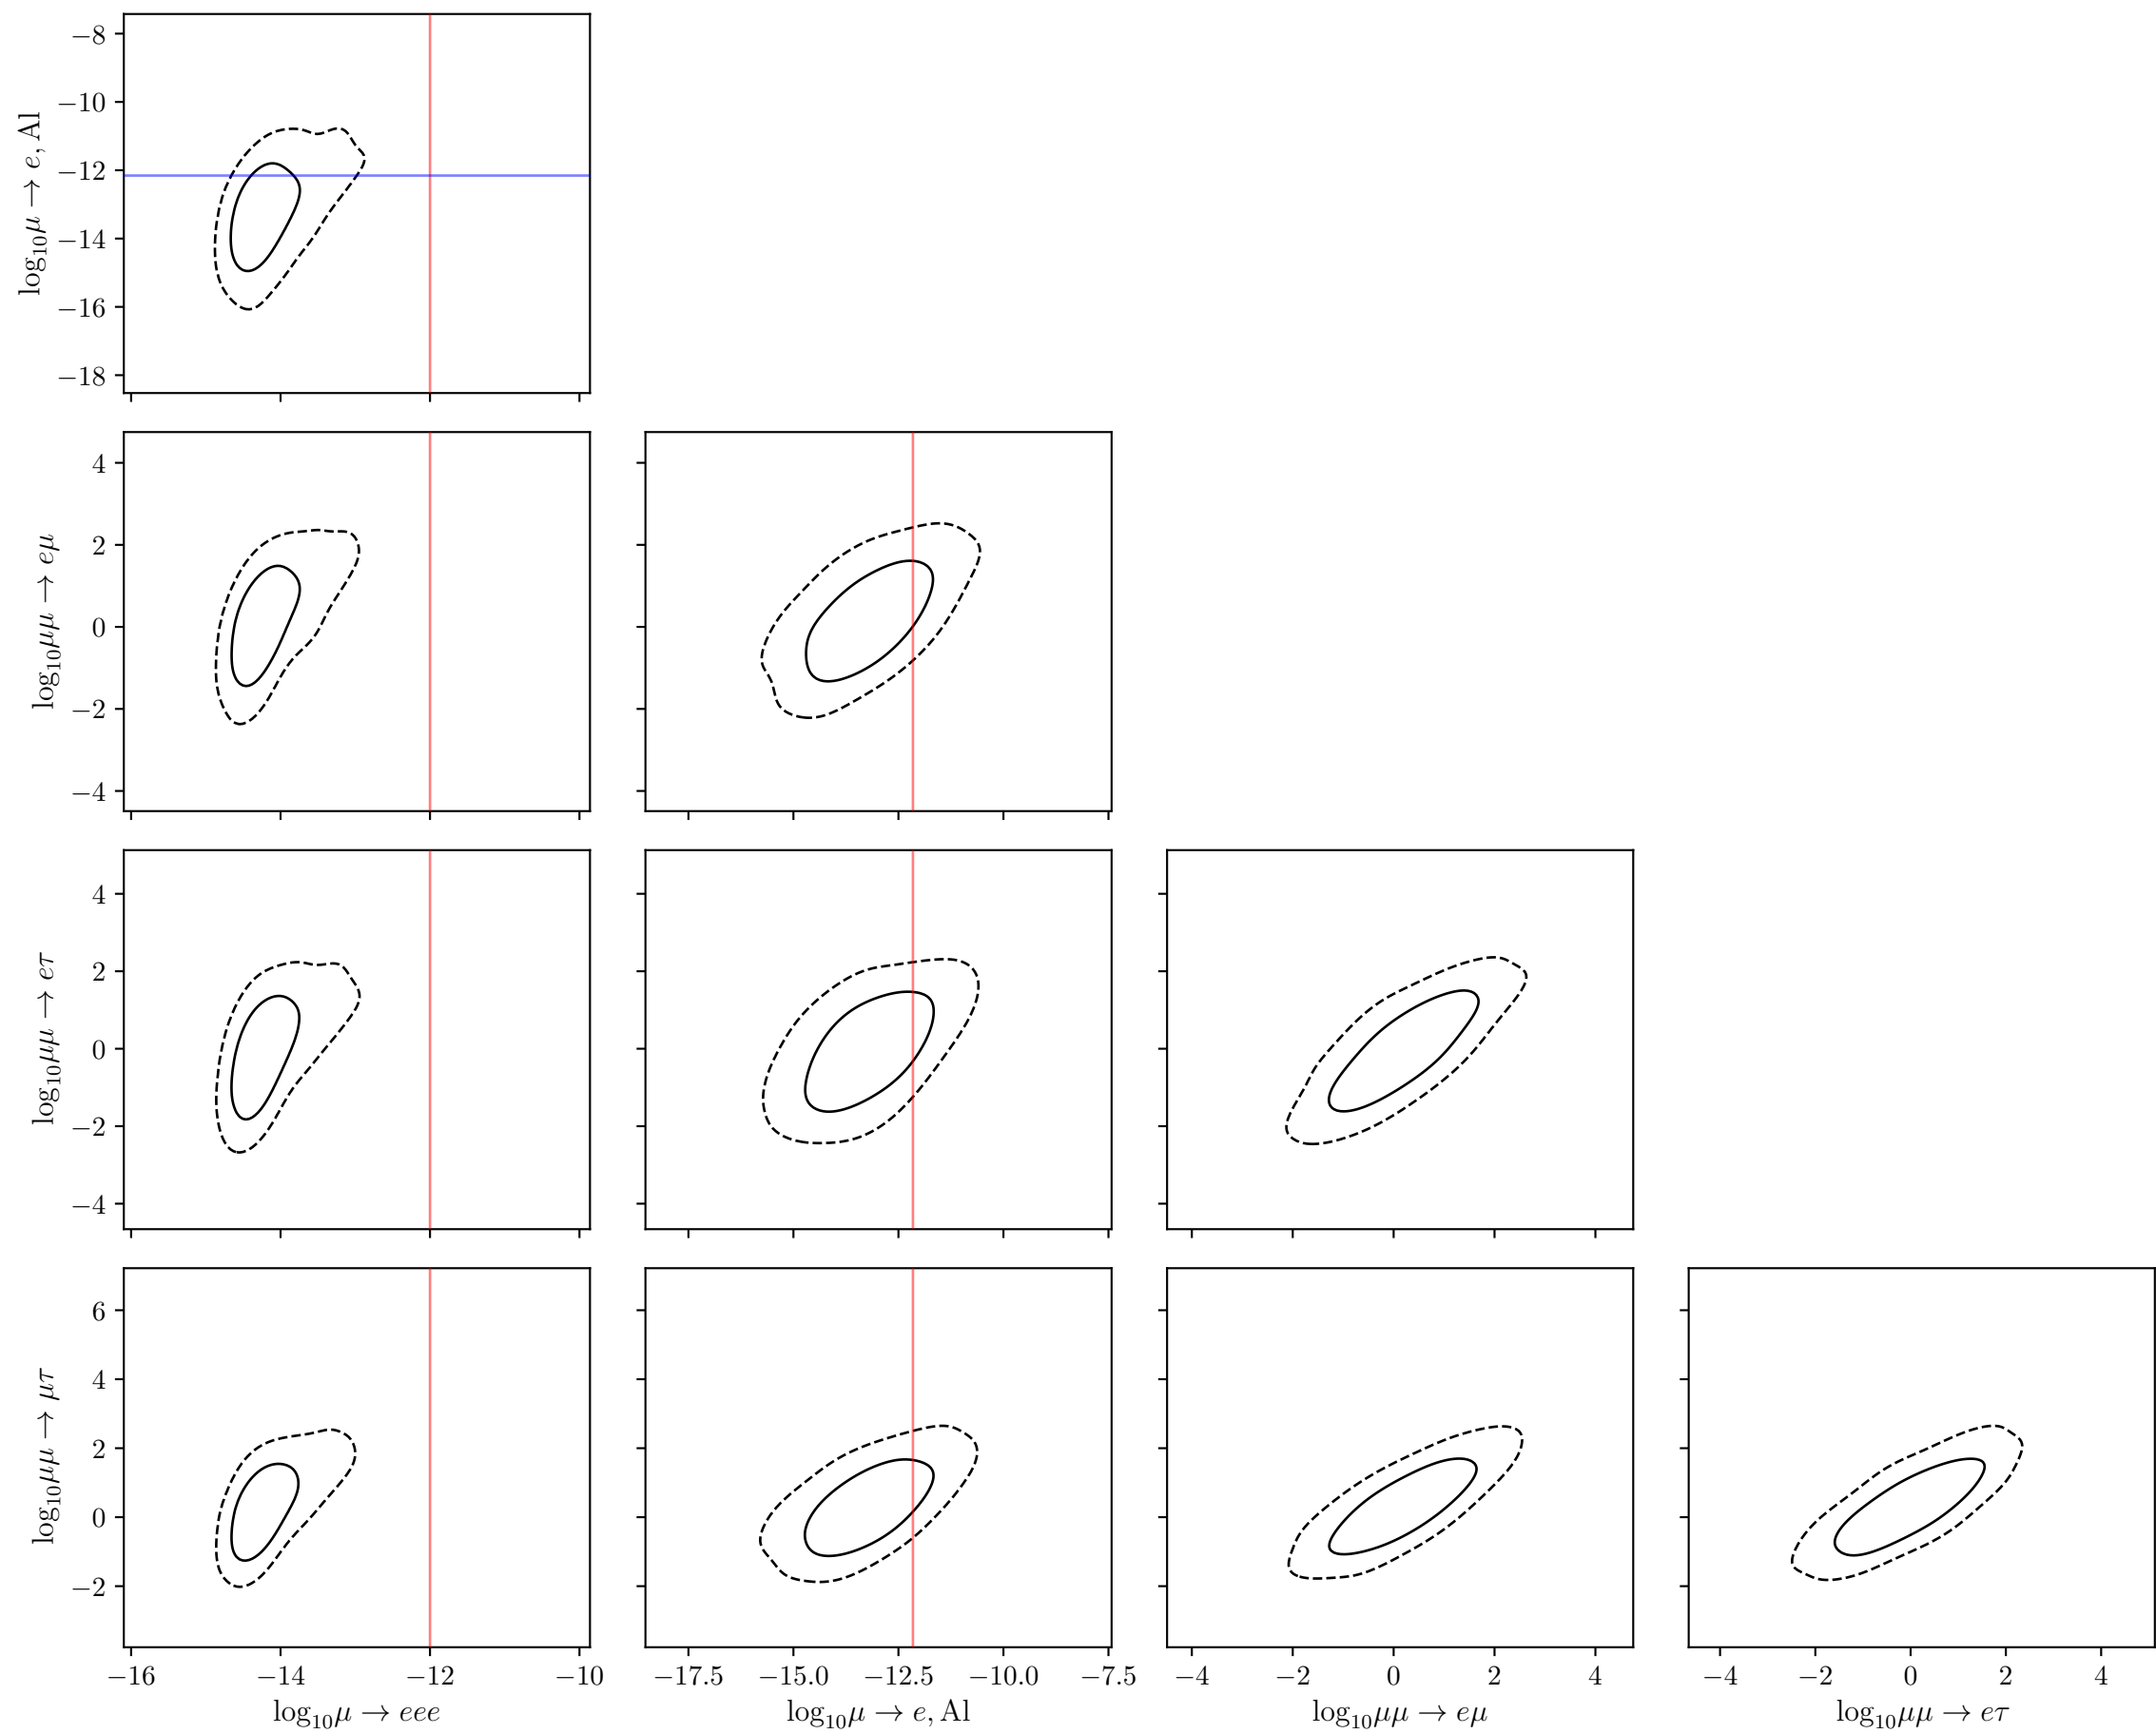

Majorana,  $X_L = \{2, 0, -1\}$ ,  $X_e = \{7, 5, 4\}$ ,

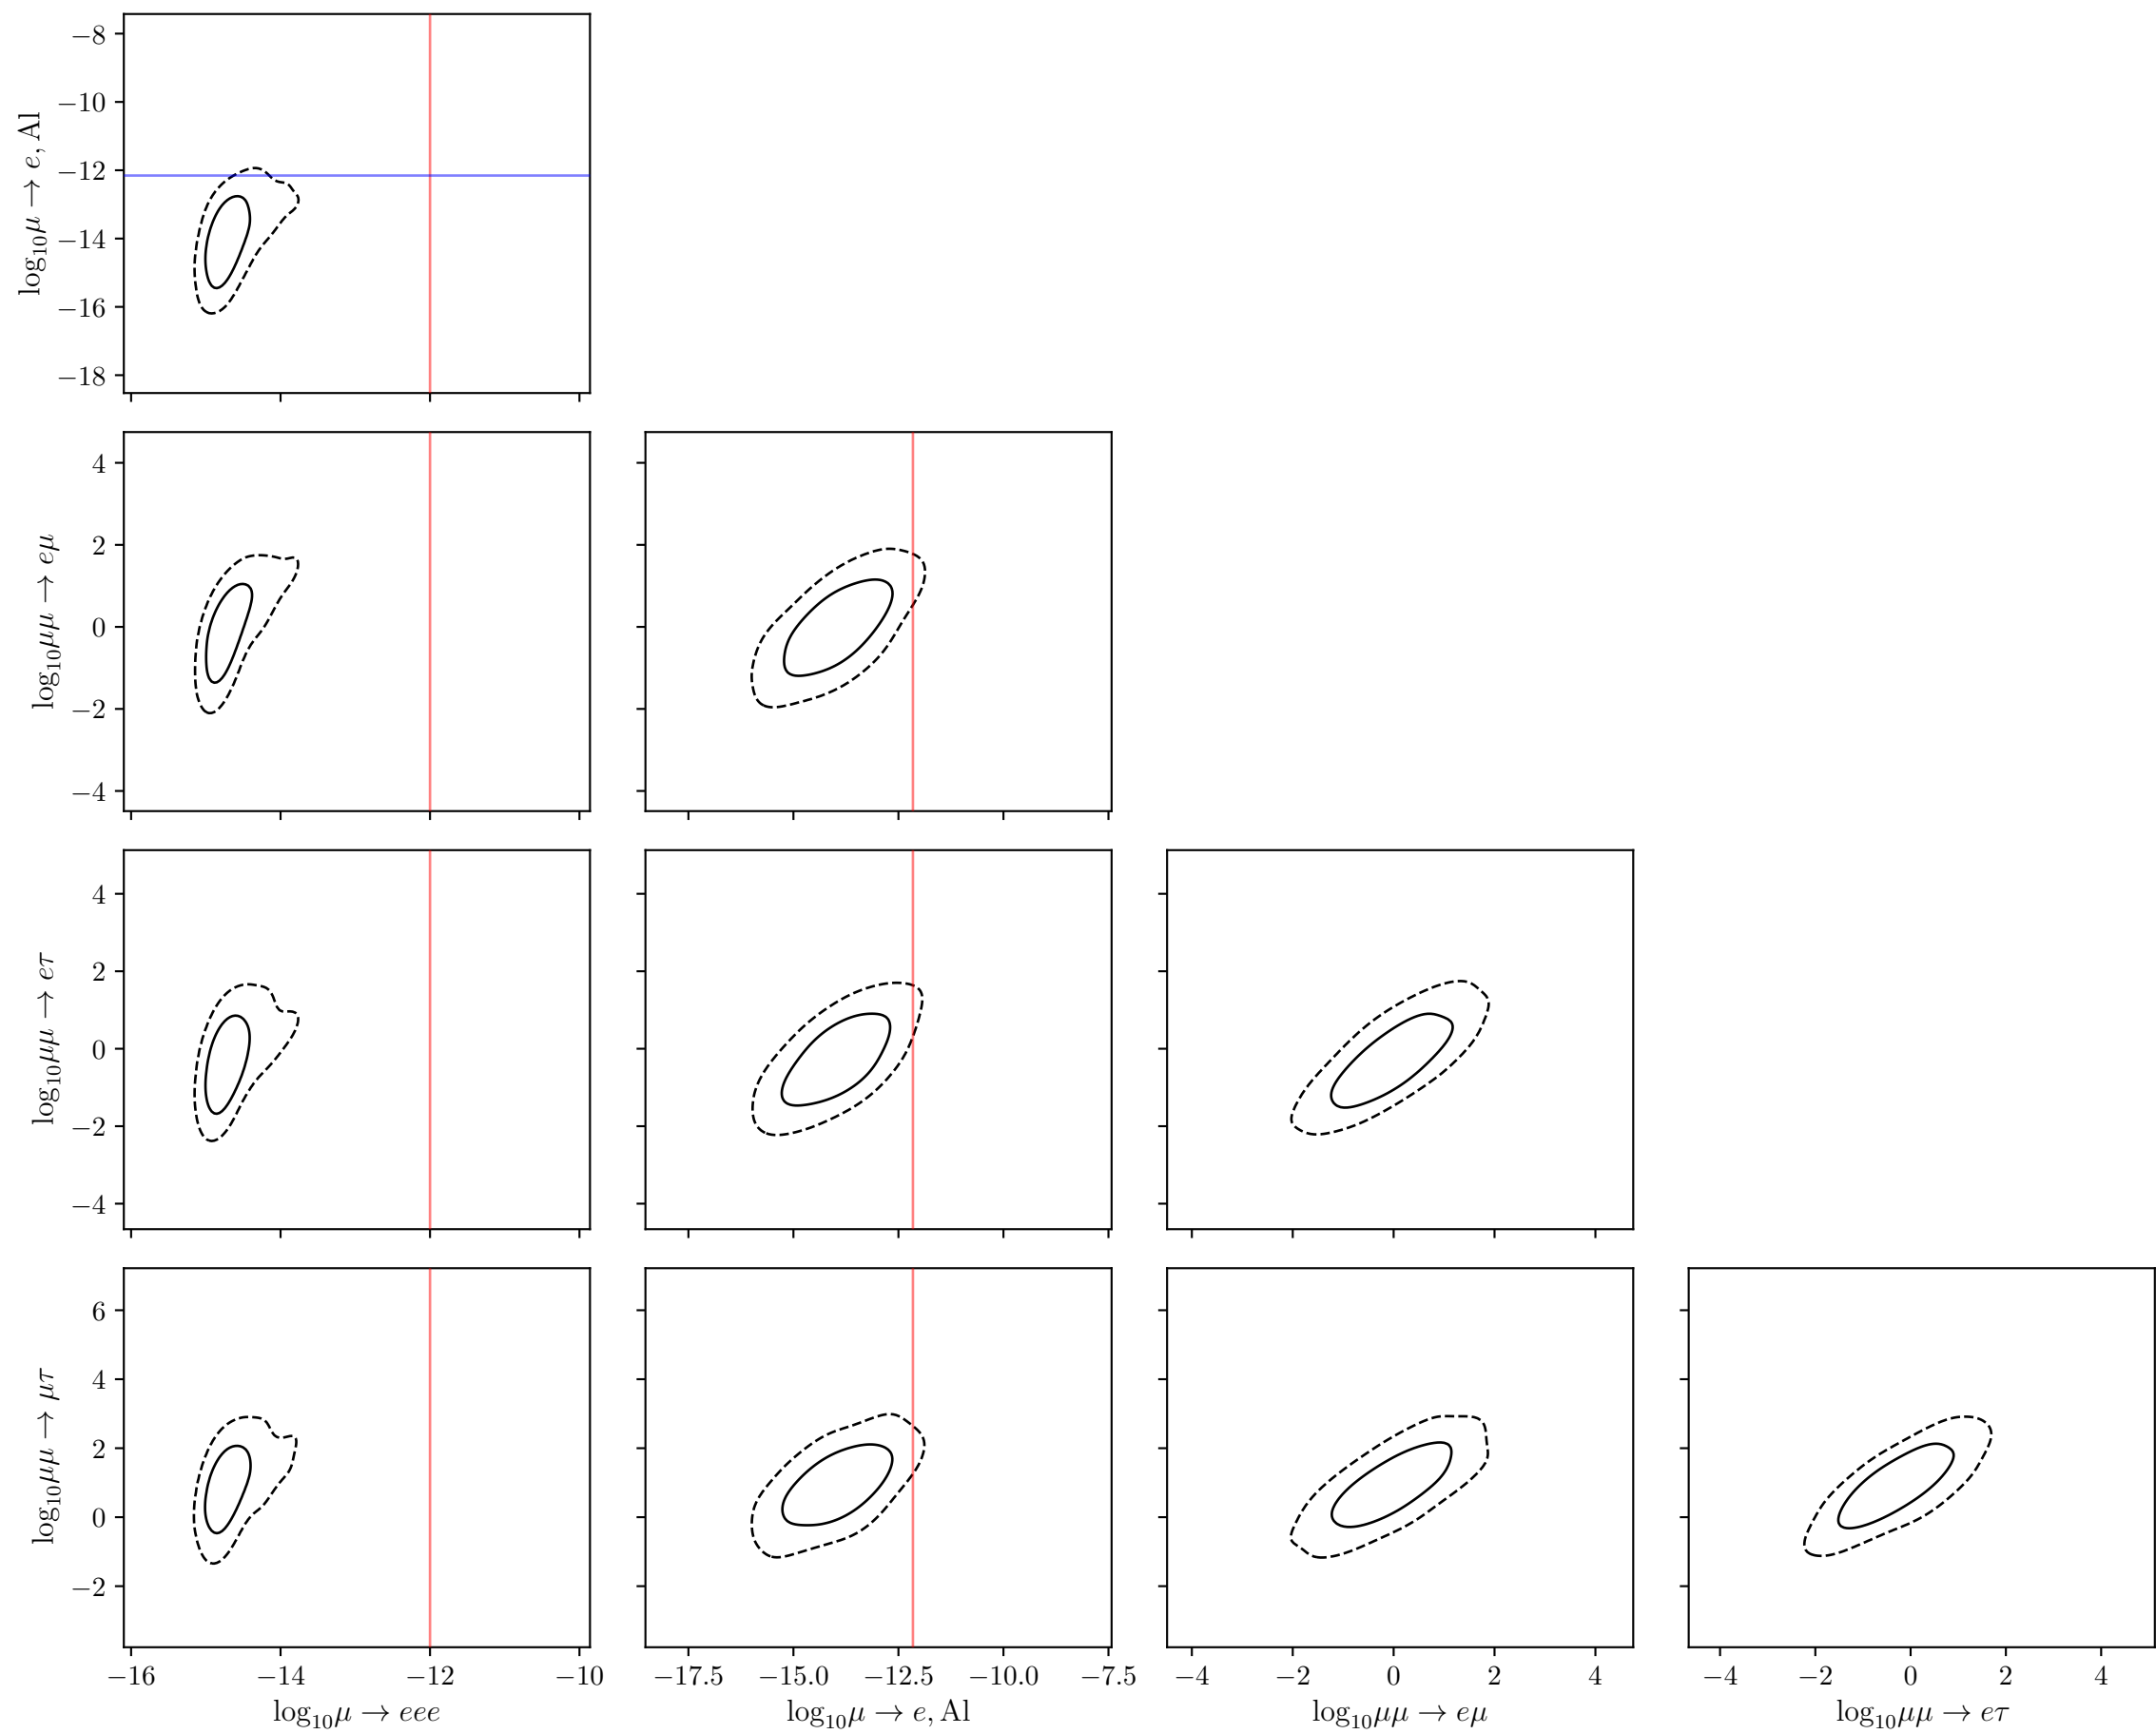

Majorana,  $X_L = \{7, 6, 5\}$ ,  $X_e = \{-1, 1, 4\}$ ,

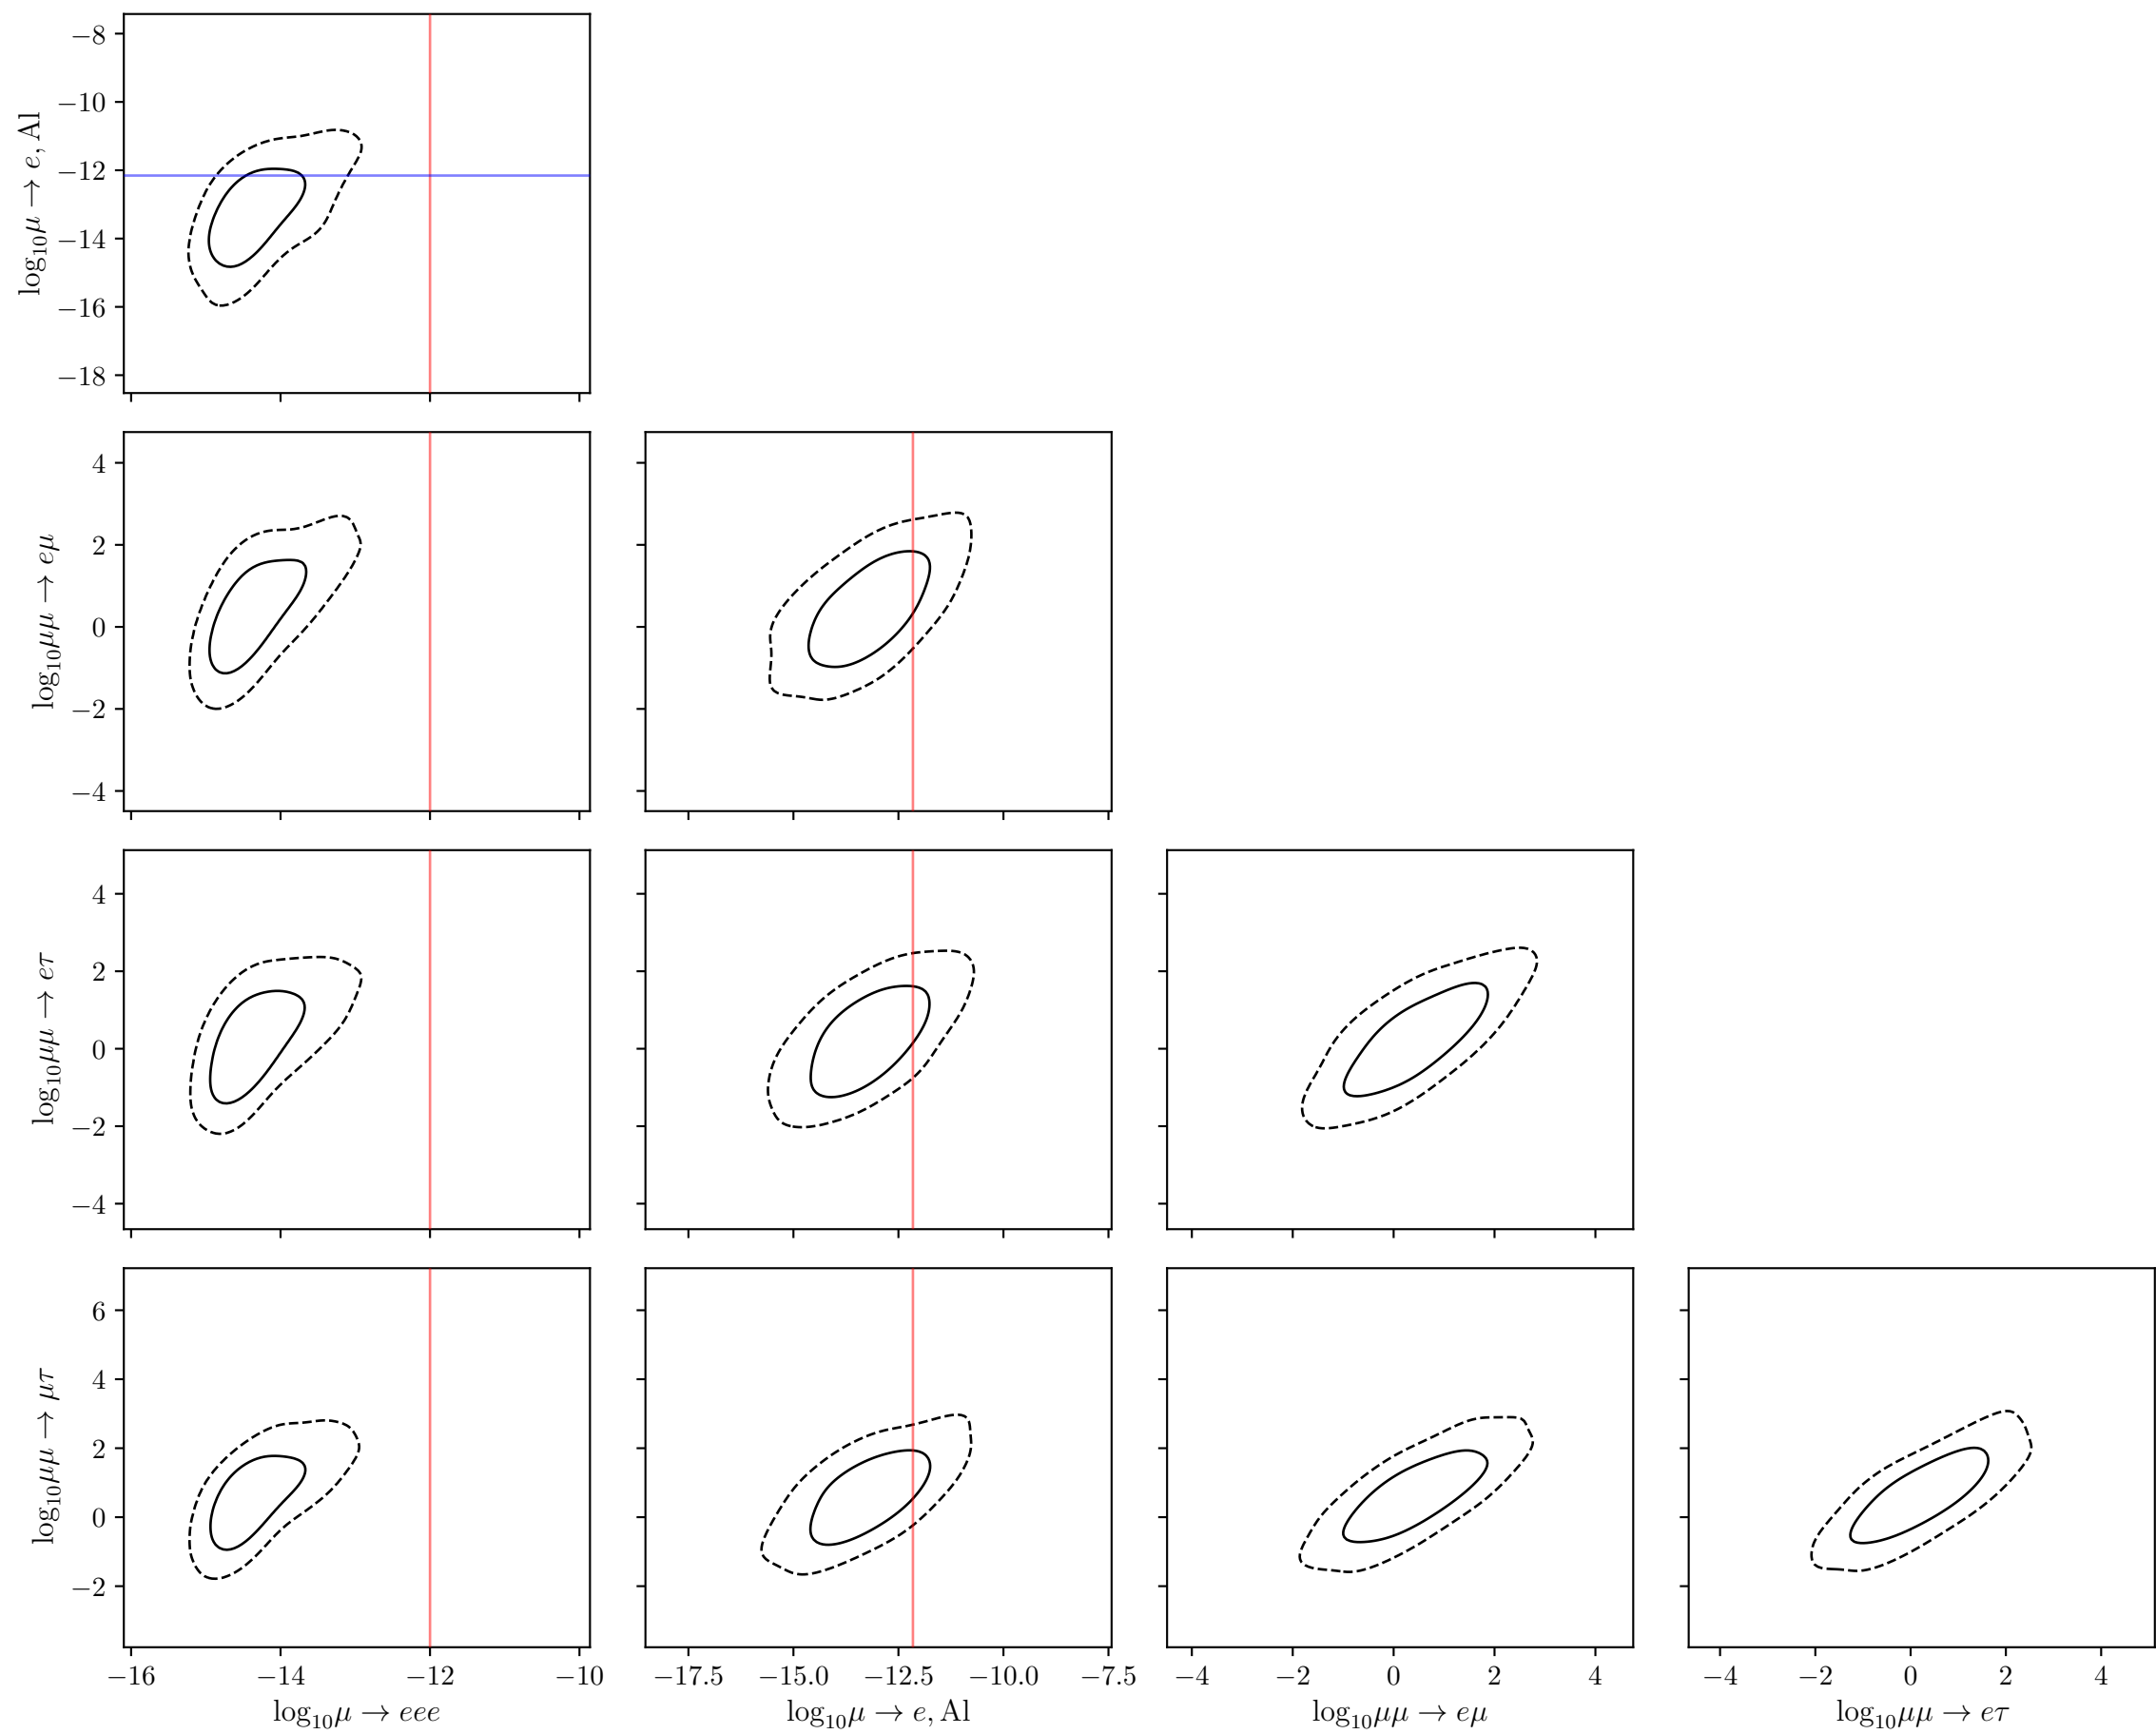

Majorana,  $X_L = \{5, 5, 4\}$ ,  $X_e = \{7, 2, 0\}$ ,

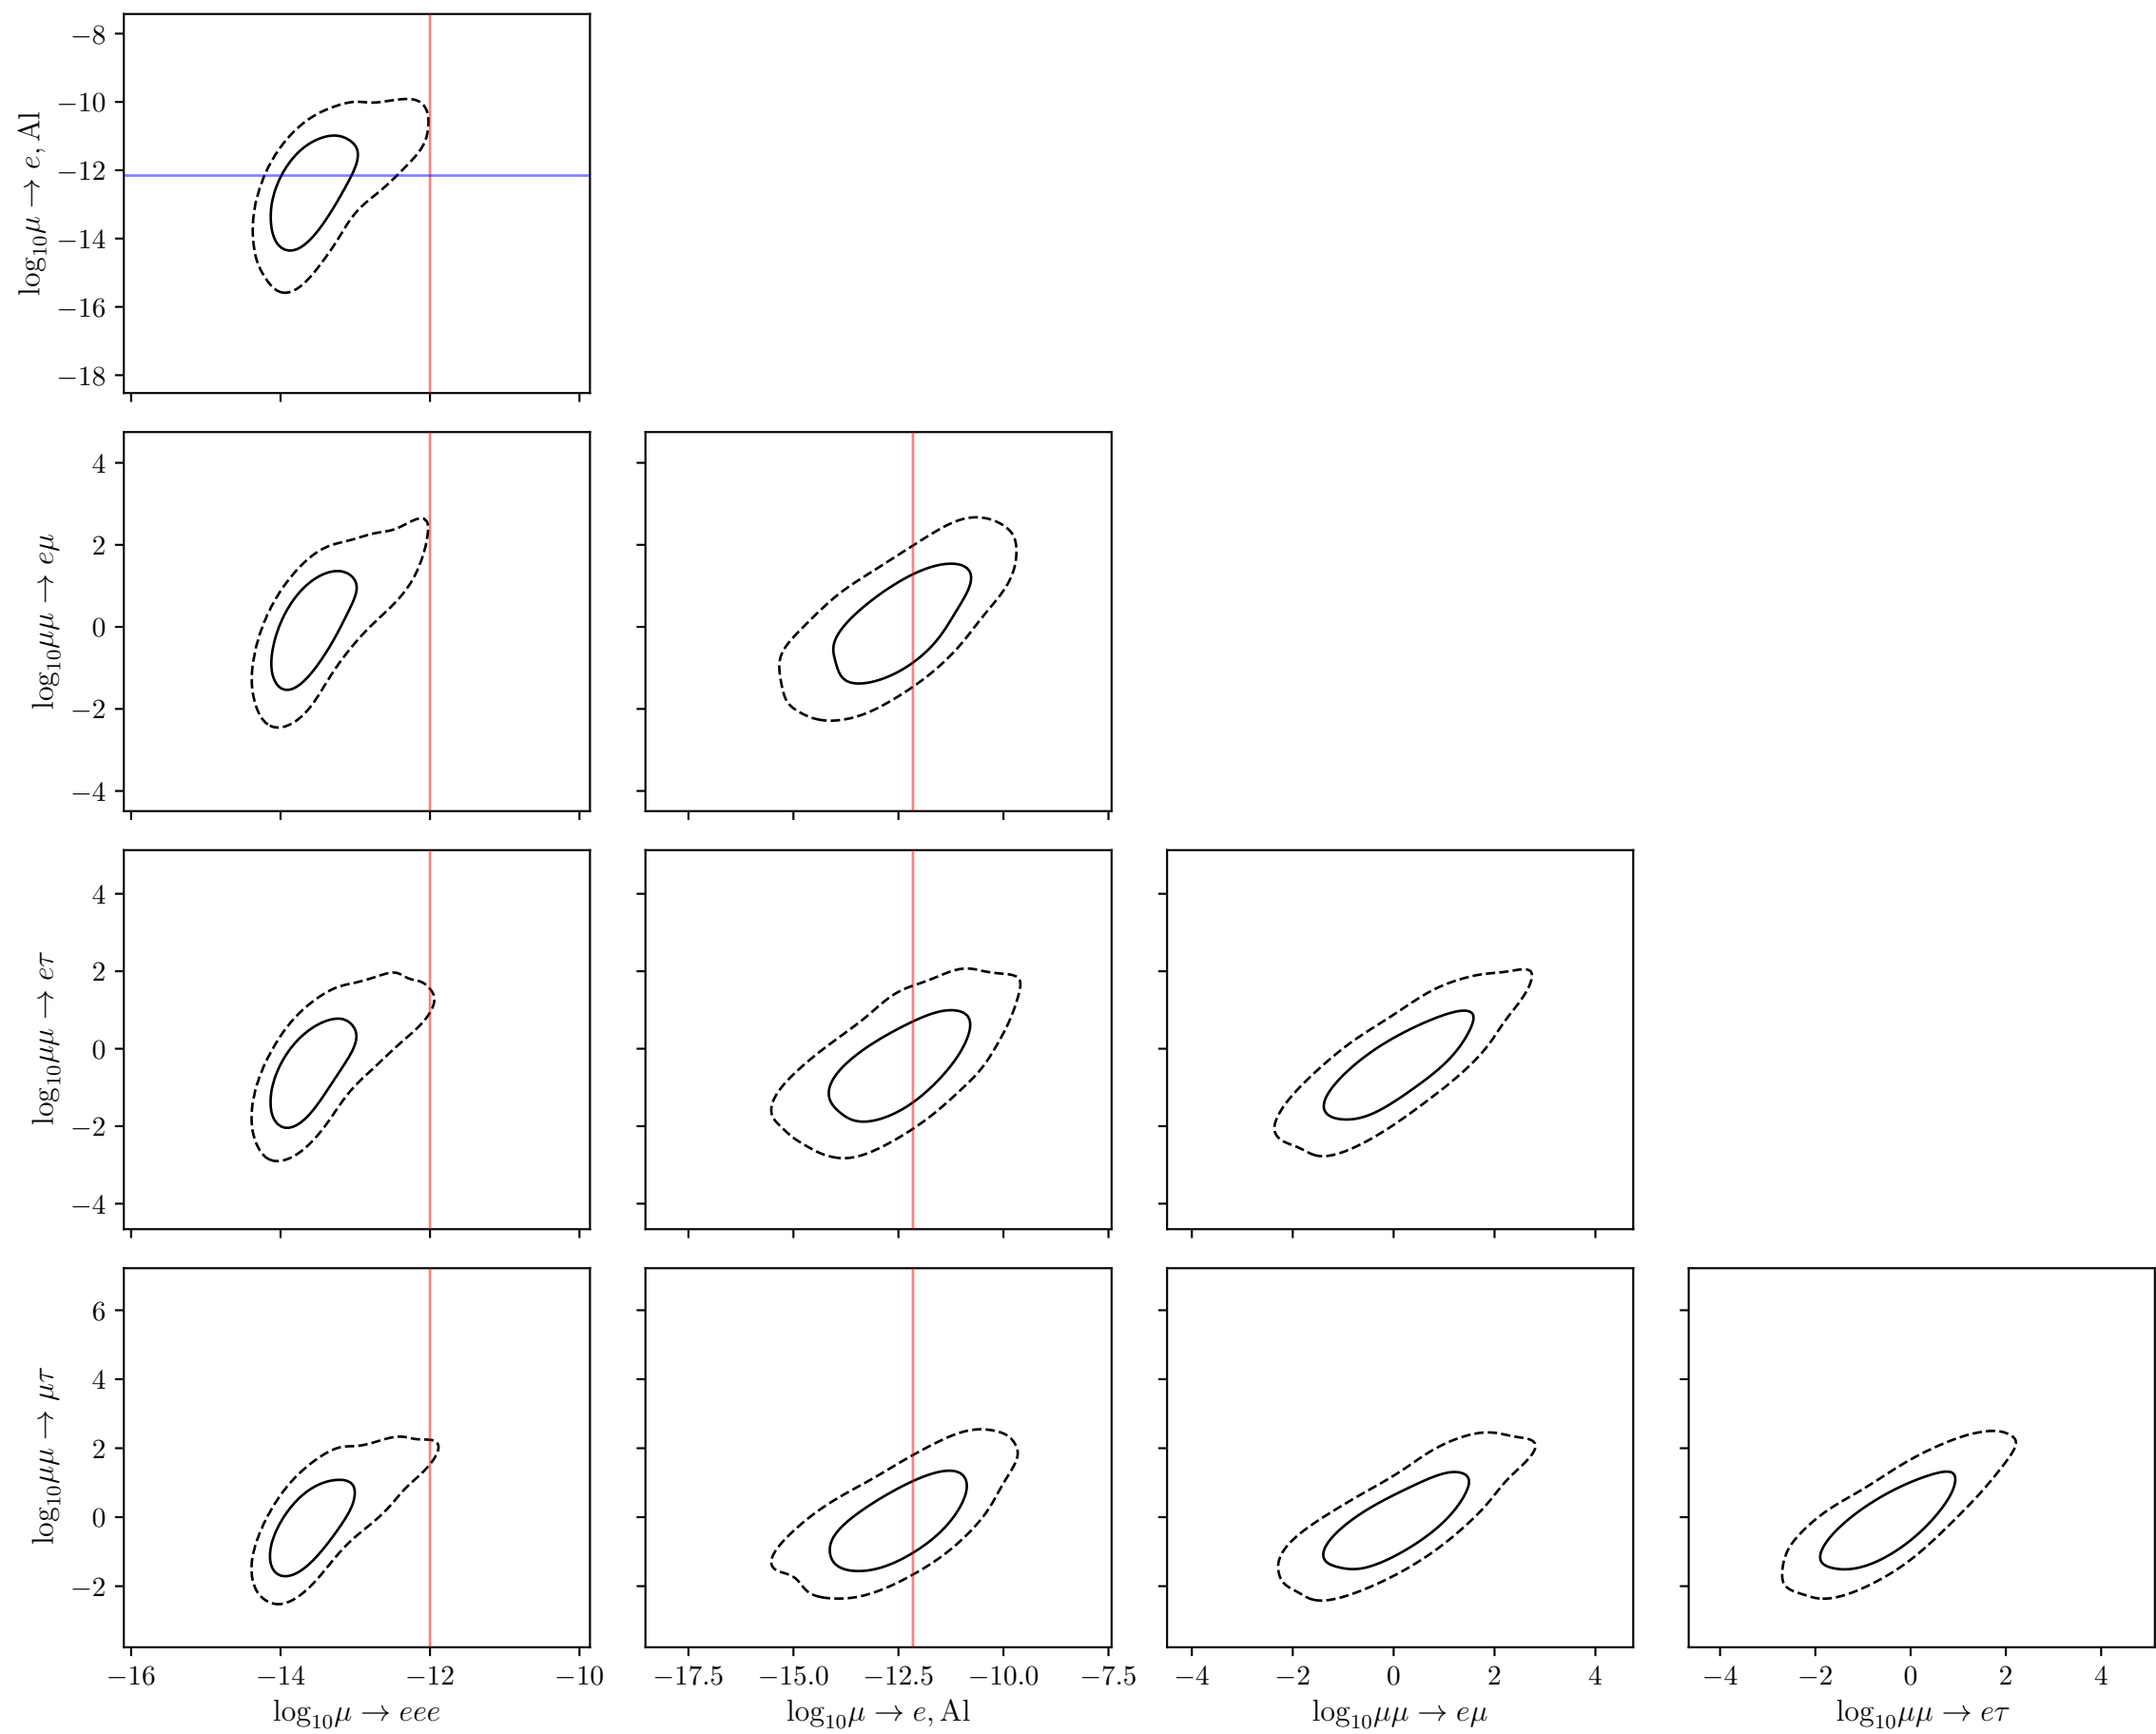

Majorana,  $X_L = \{4, 4, 3\}$ ,  $X_e = \{4, 1, 0\}$ ,

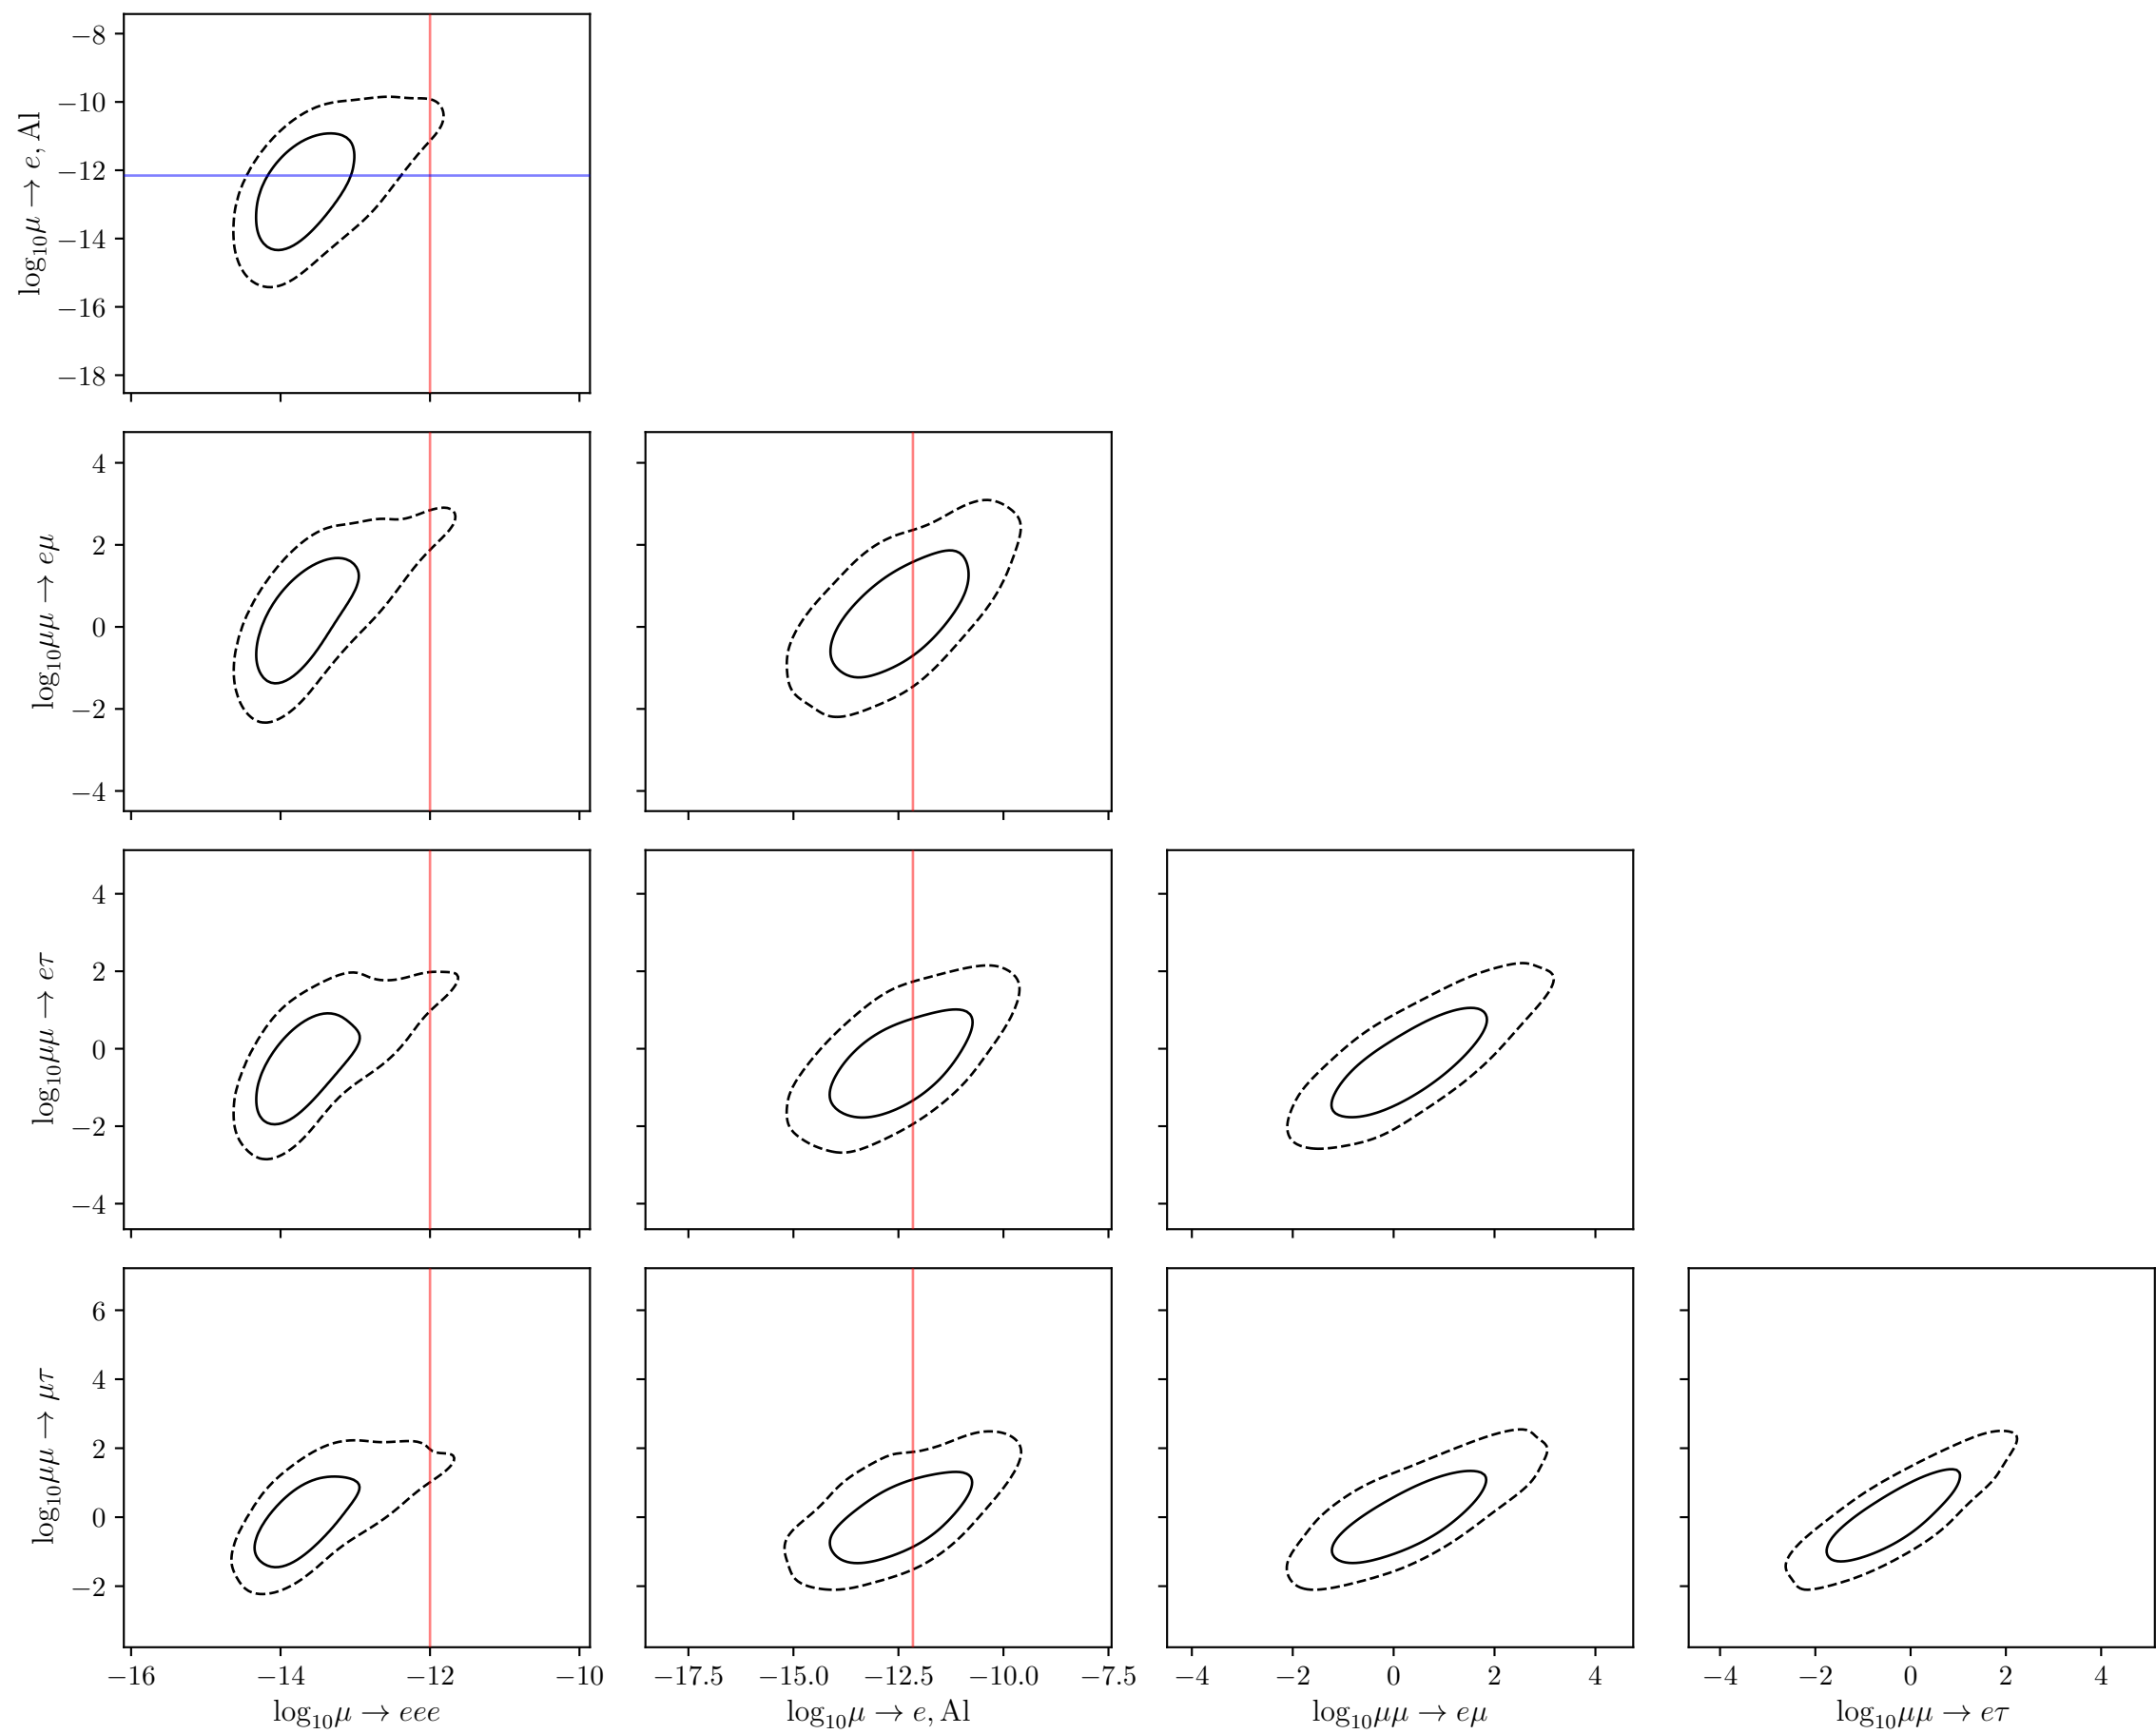

Majorana,  $X_L = \{7, 6, 5\}$ ,  $X_e = \{5, 2, 0\}$ ,

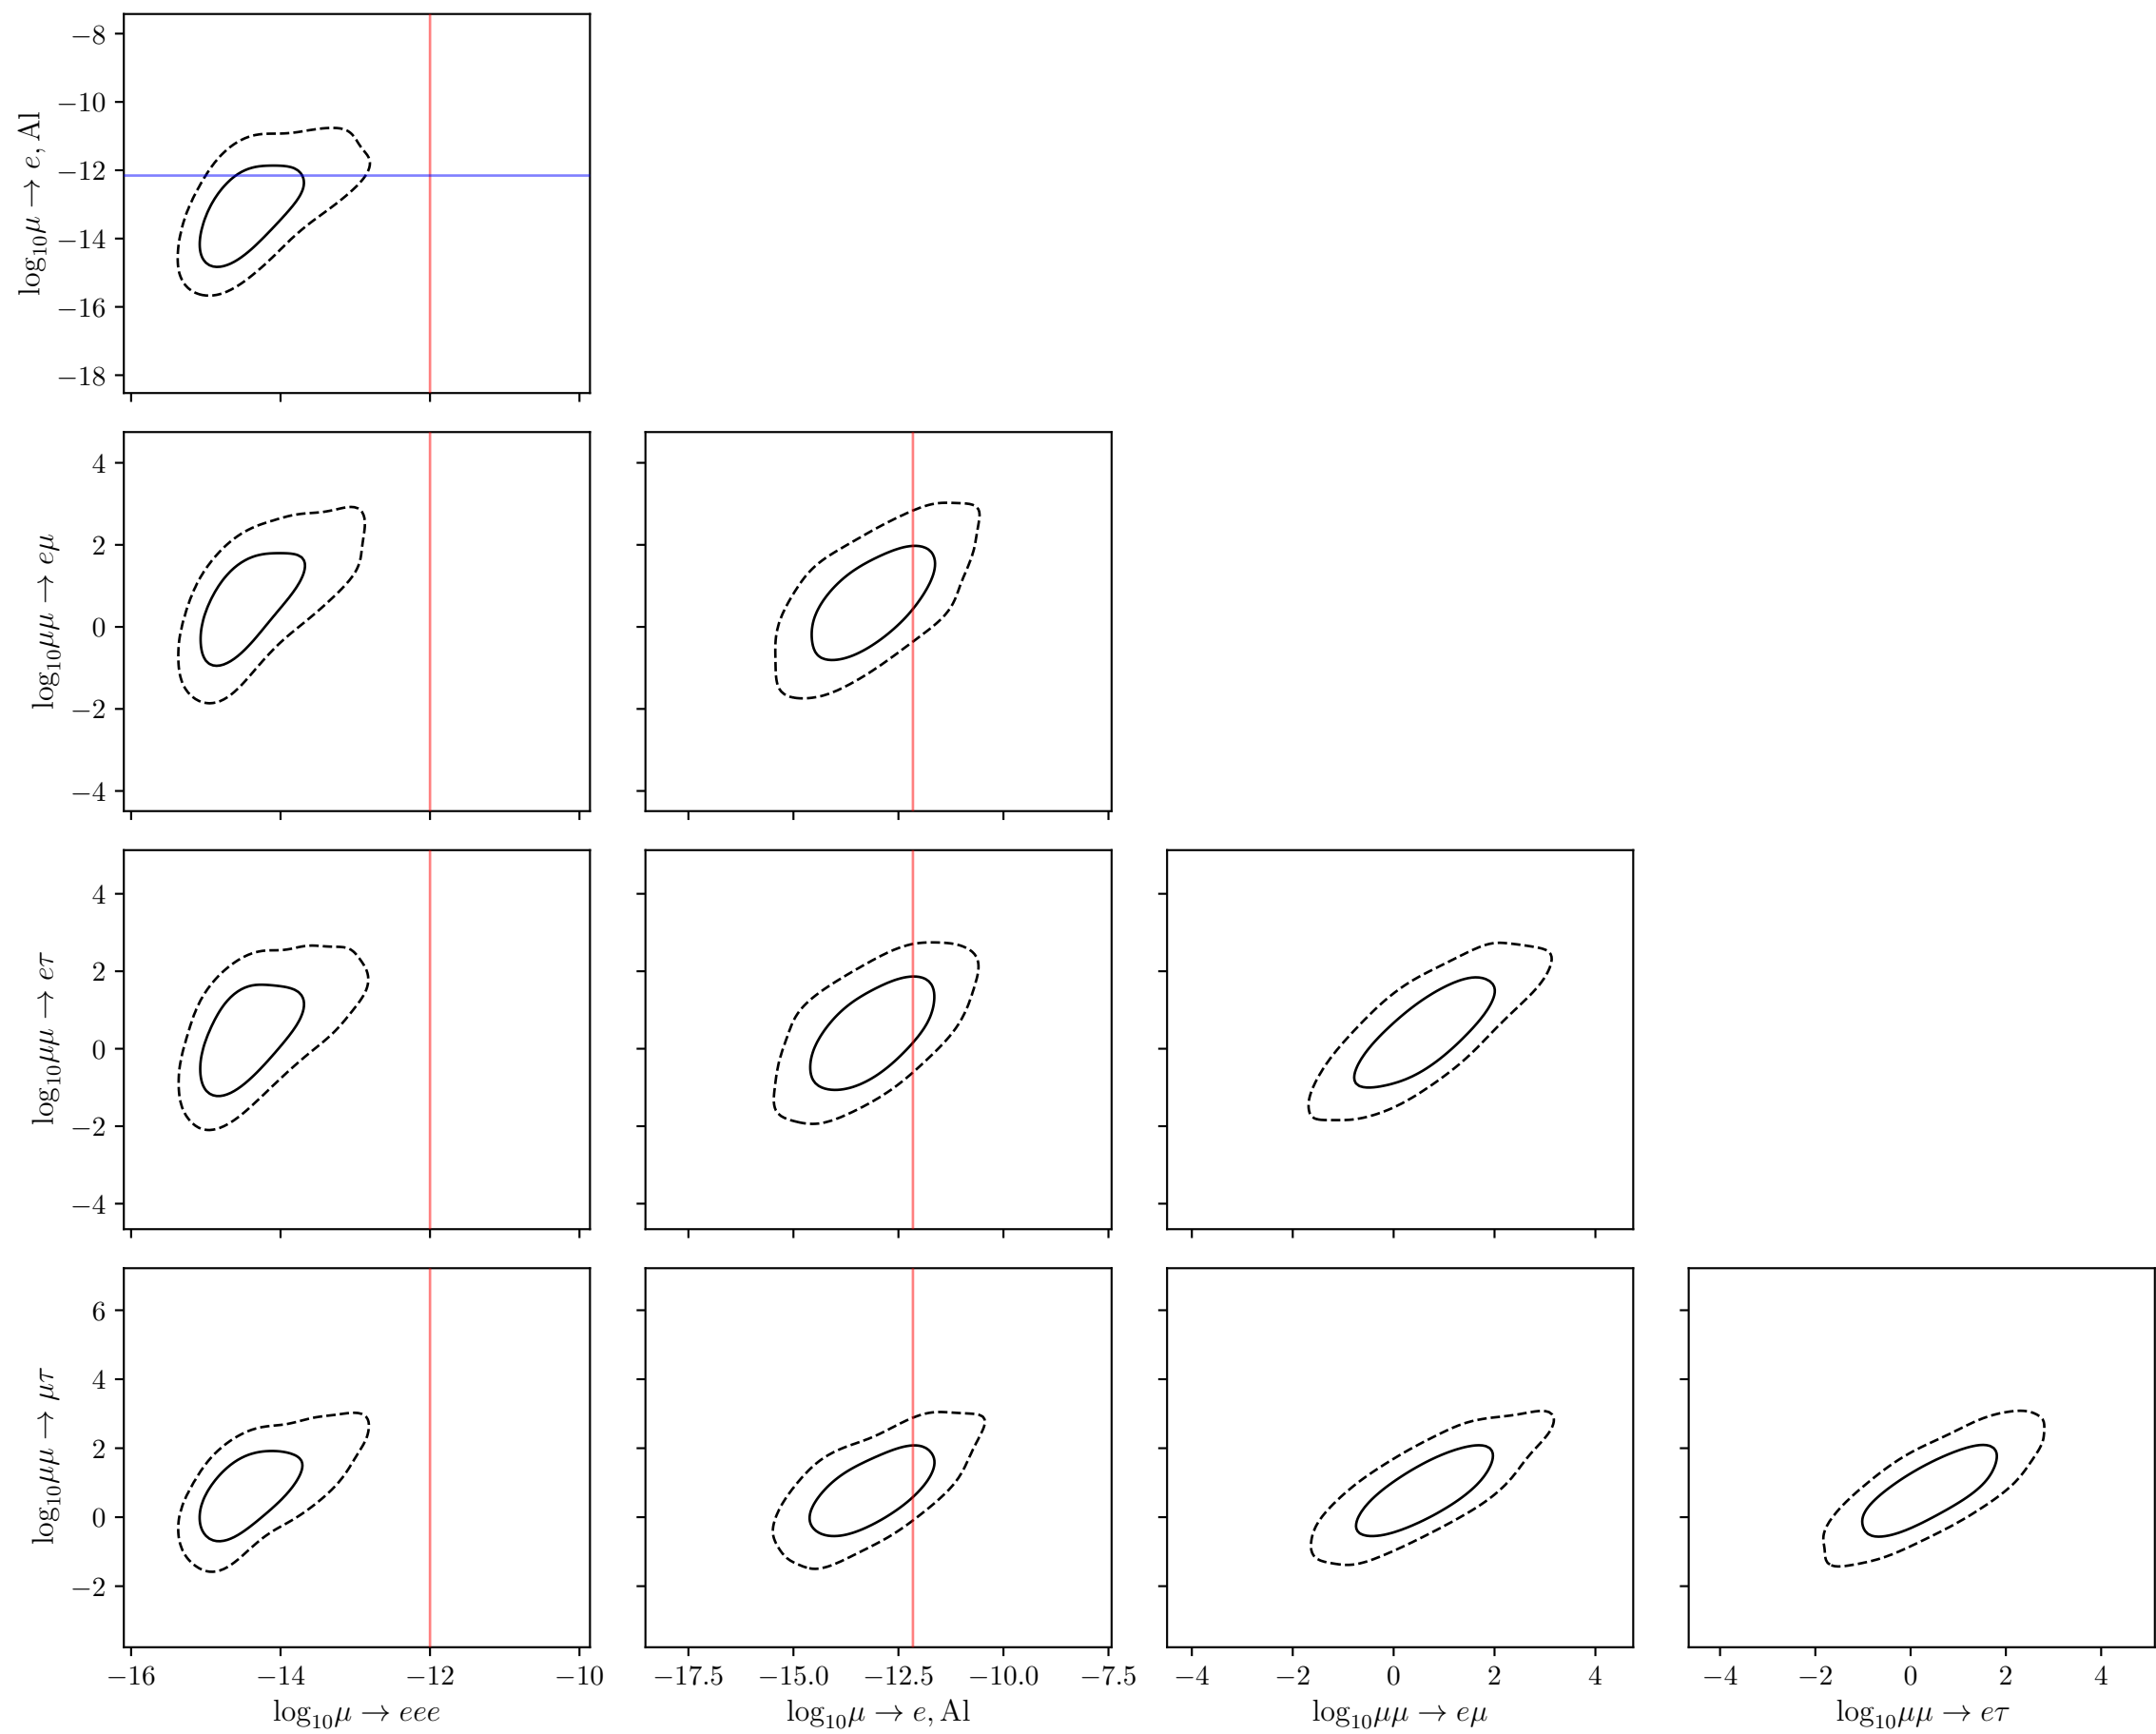



Majorana,  $X_L = \{6, 6, 5\}$ ,  $X_e = \{7, 3, 0\}$ ,

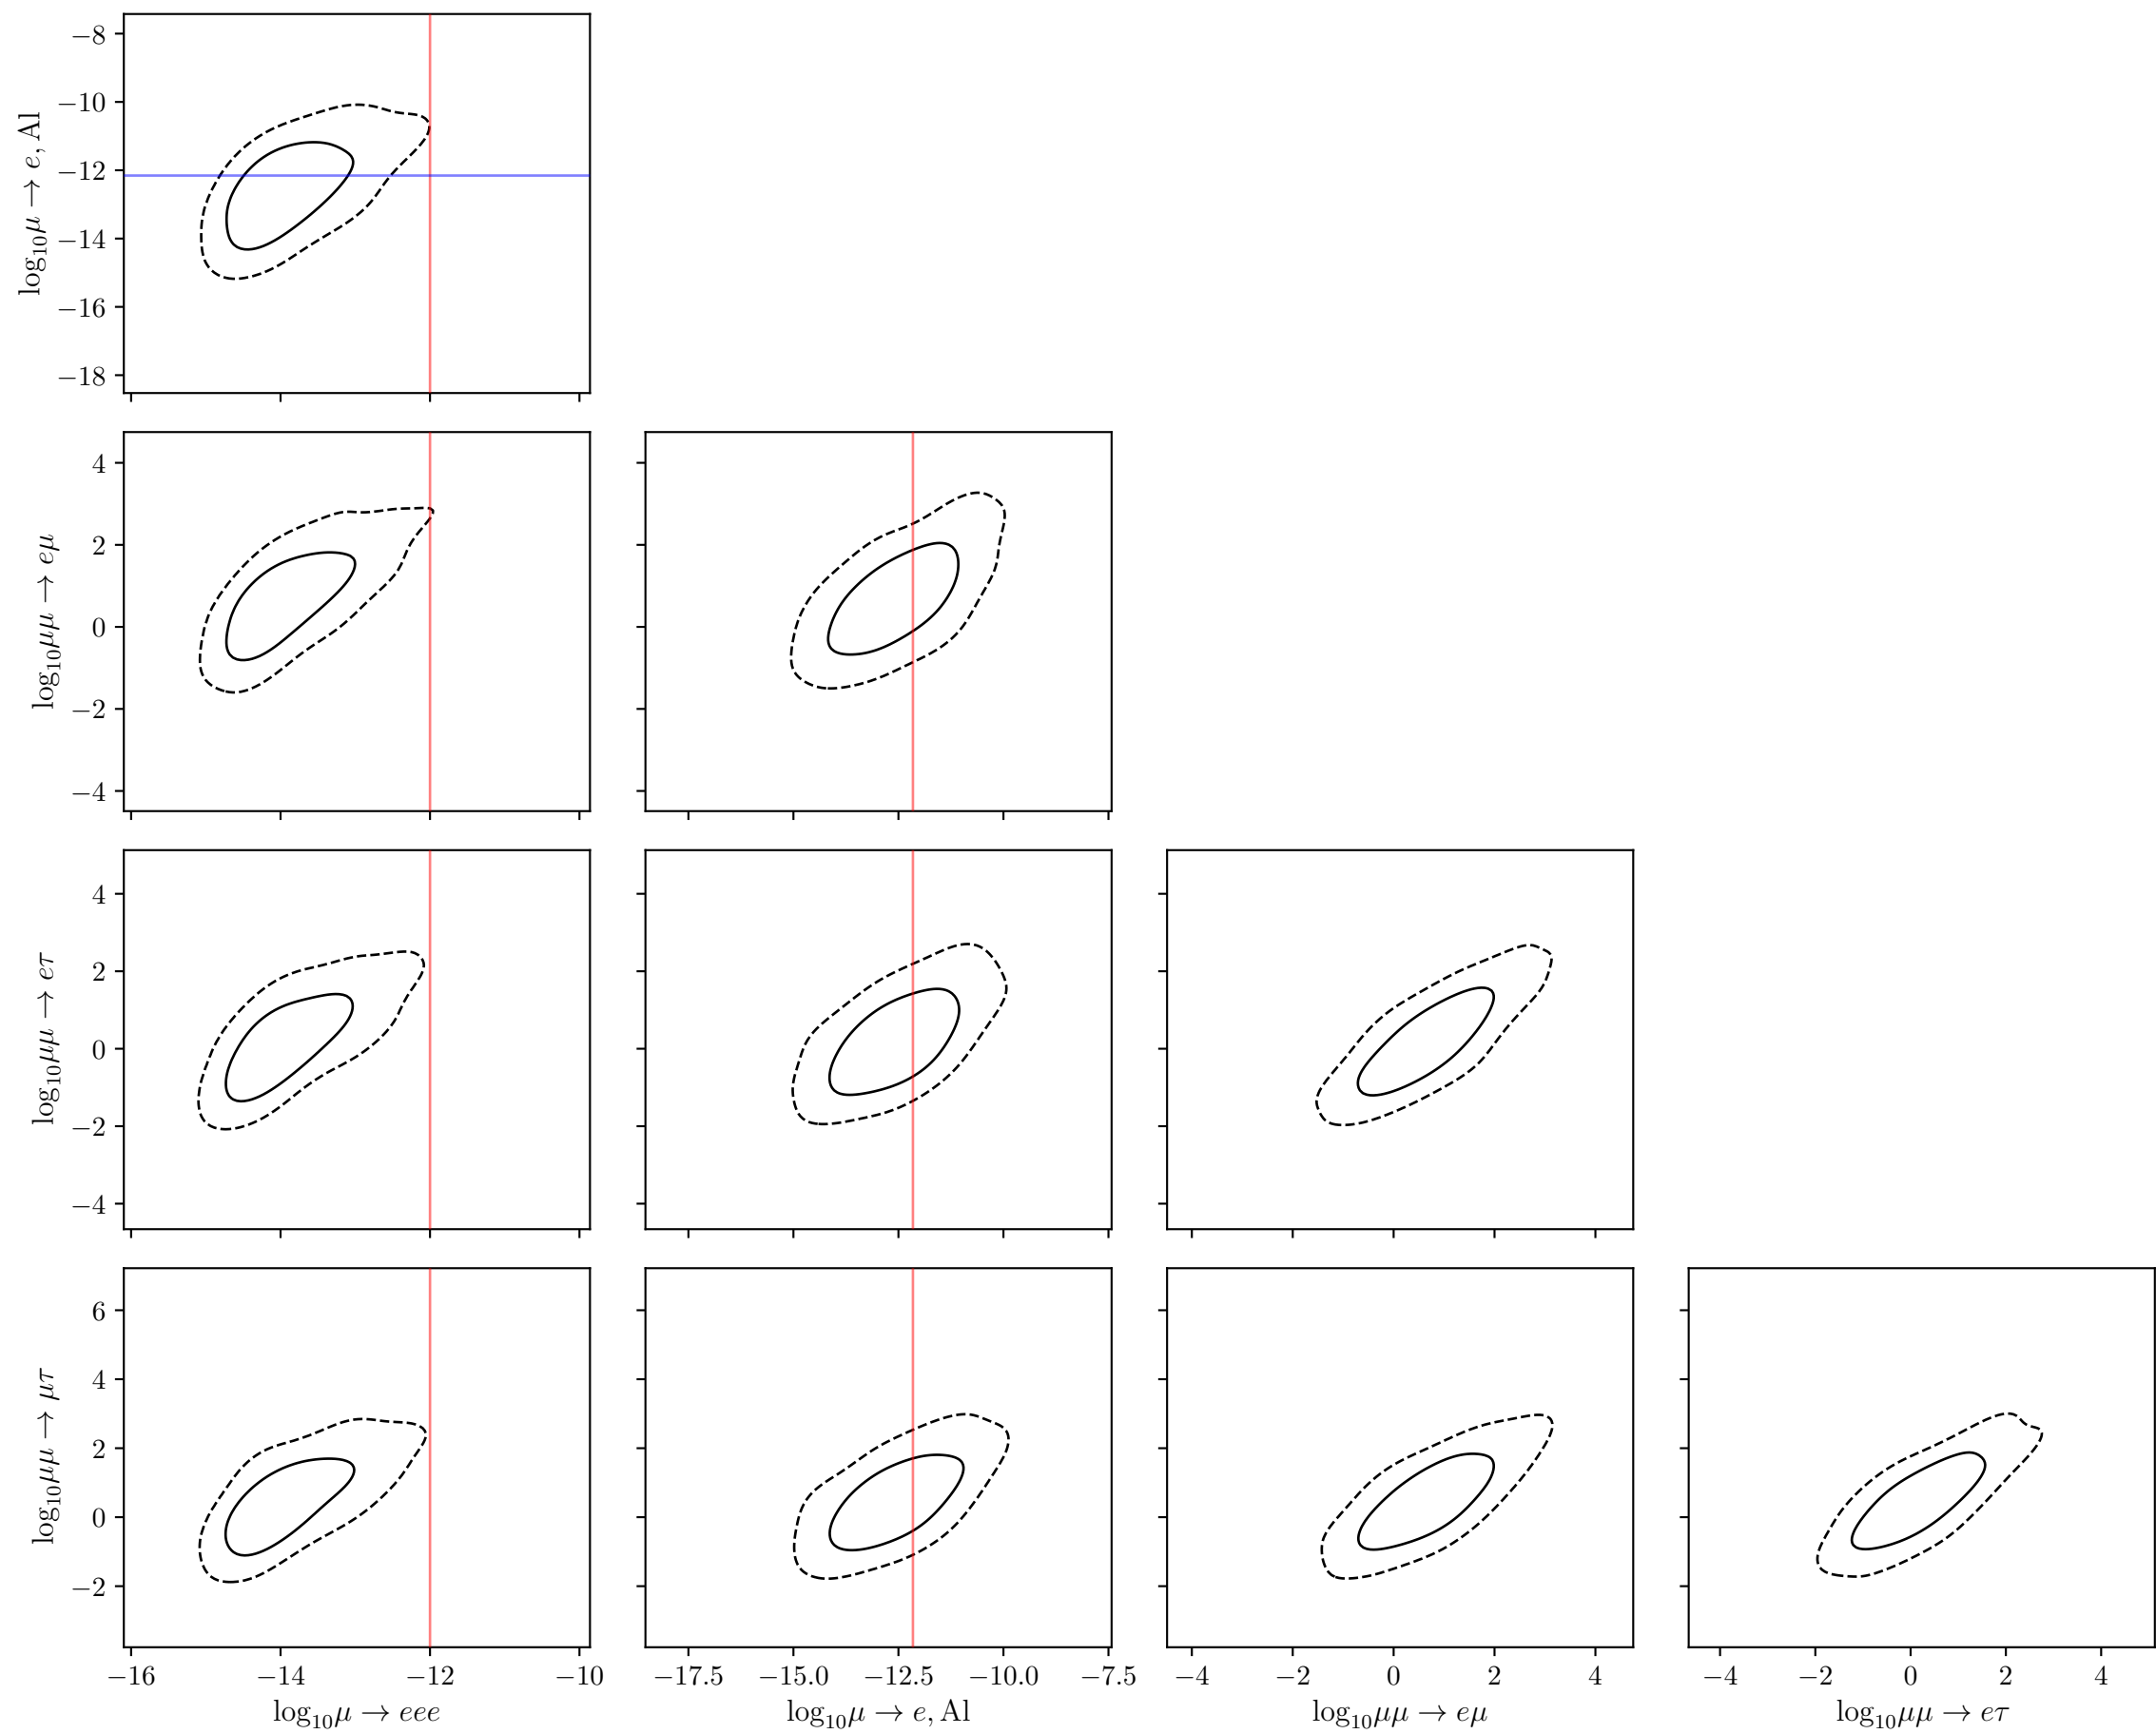

Majorana,  $X_L = \{7, 7, 6\}$ ,  $X_e = \{-3, -2, 1\}$ ,

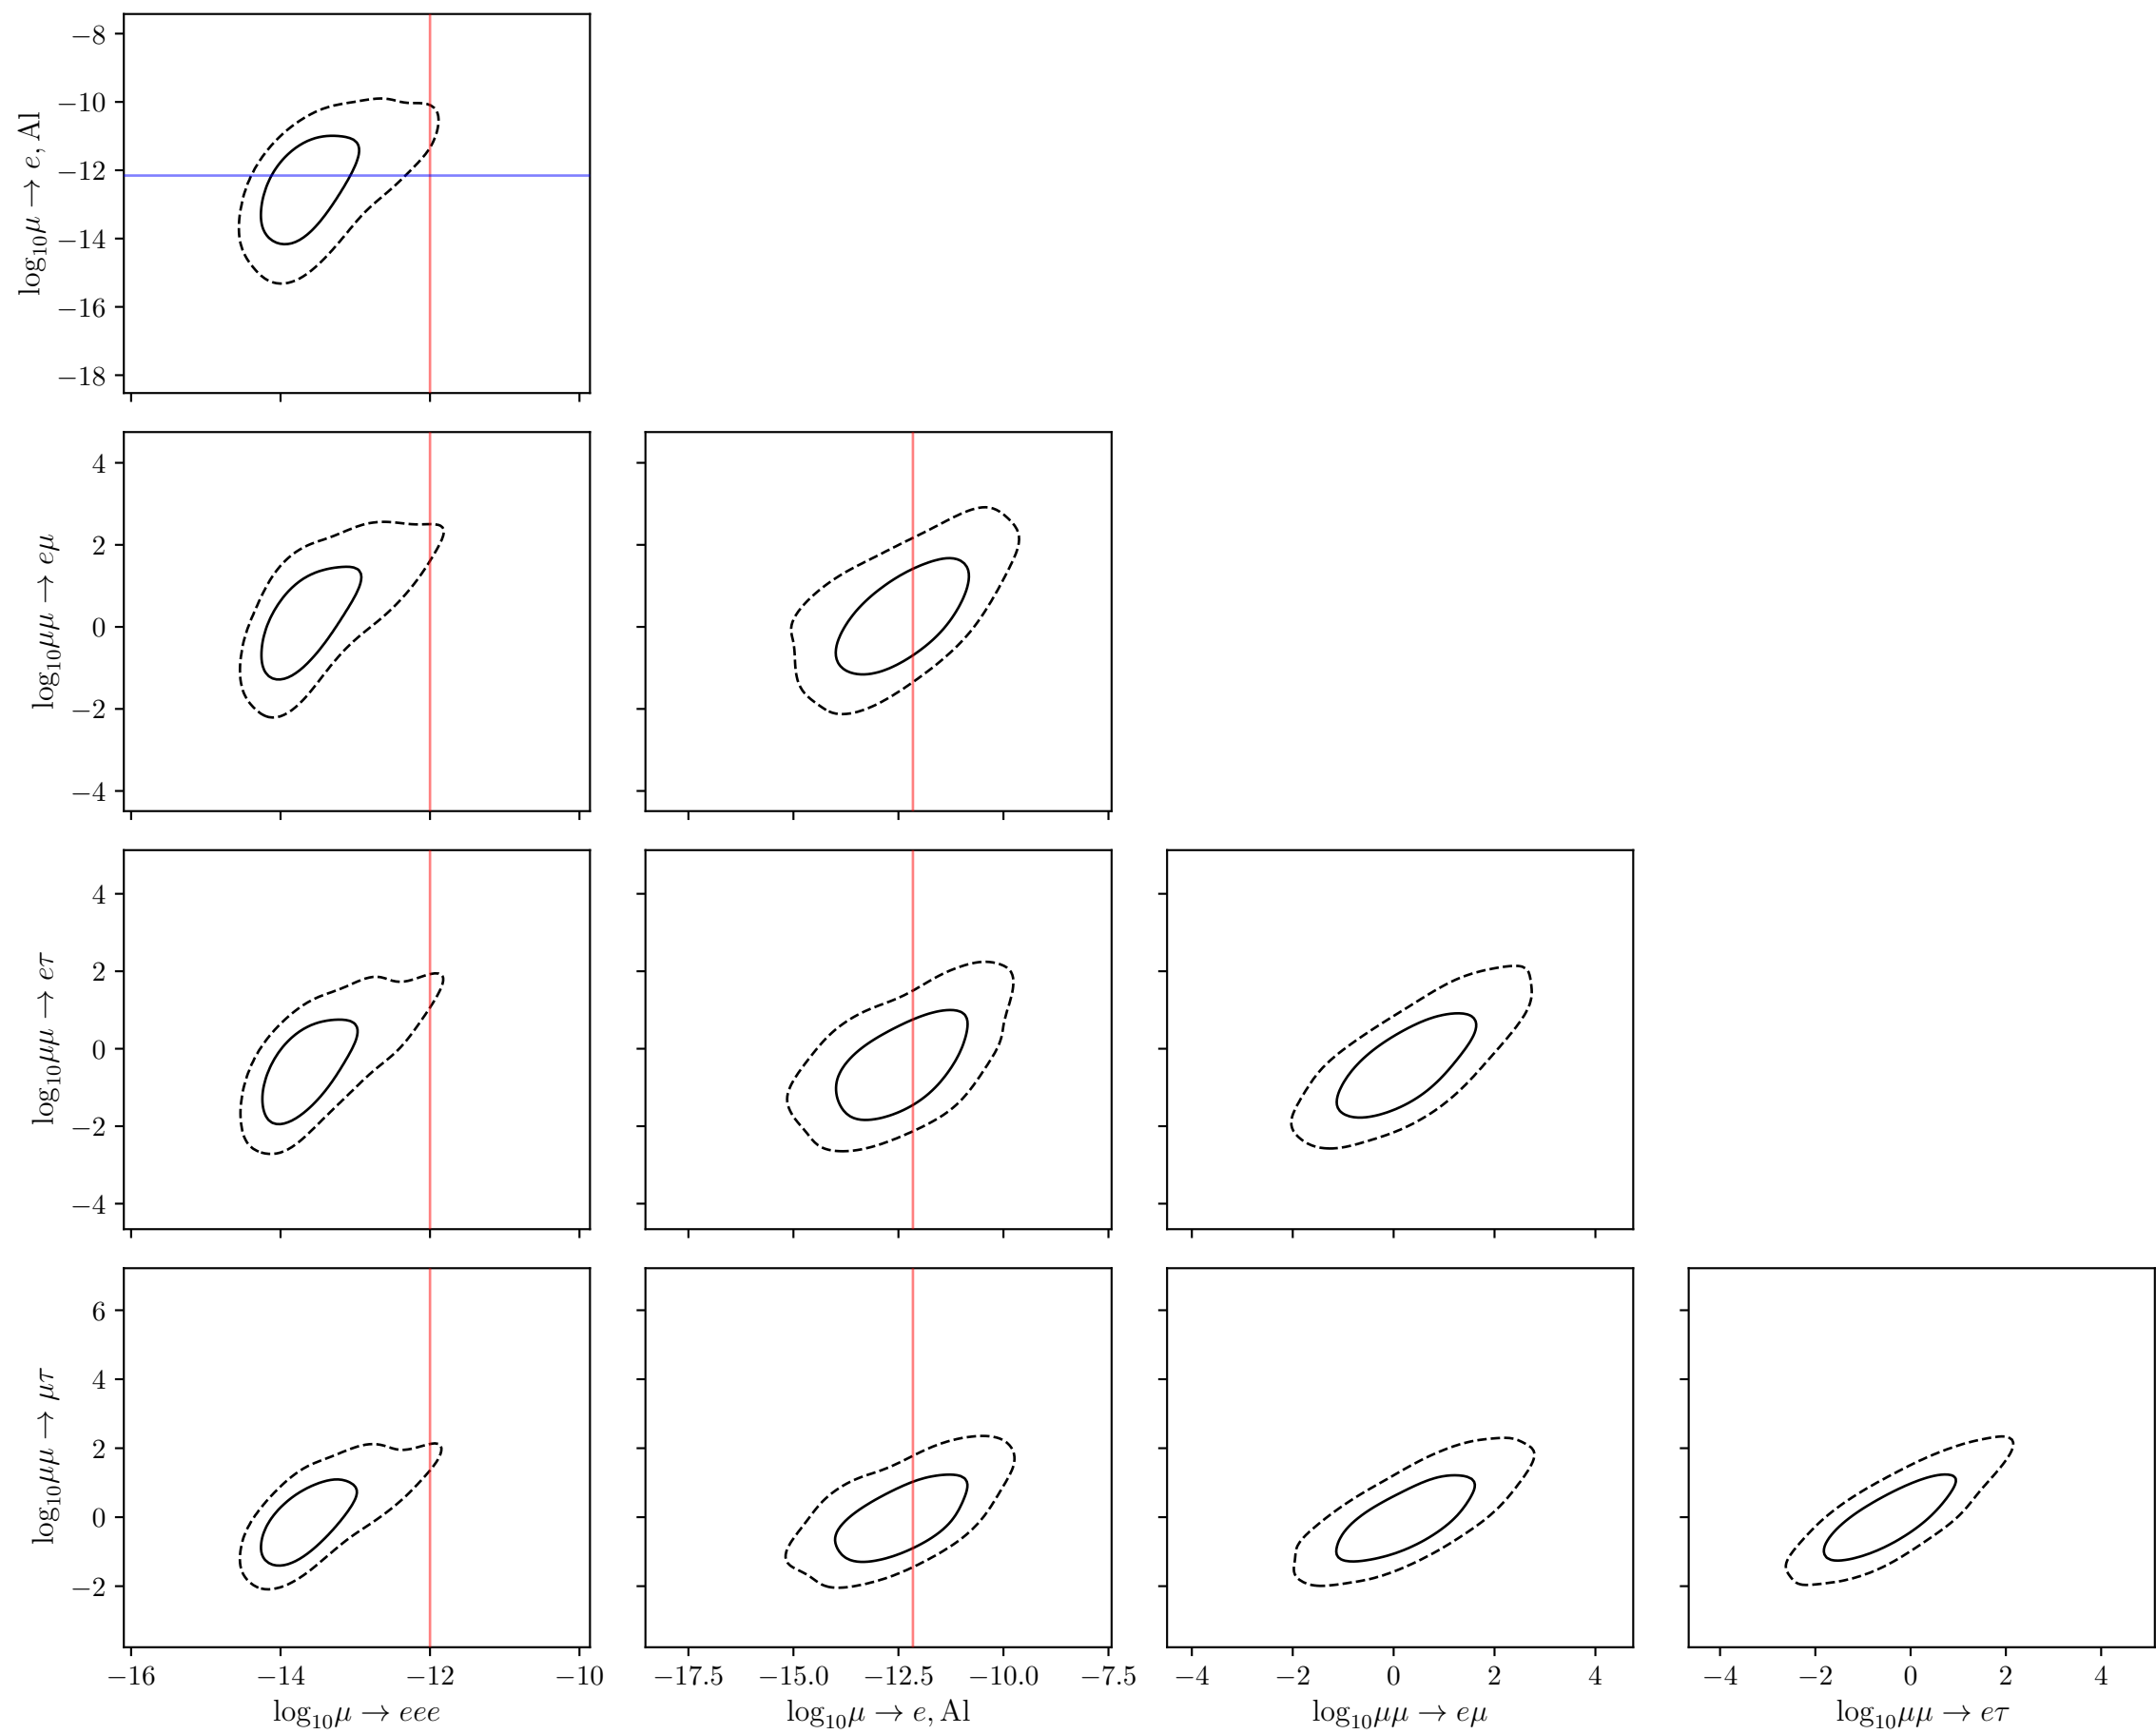

Majorana,  $X_L = \{3, 3, 2\}$ ,  $X_e = \{5, 2, 1\}$ ,

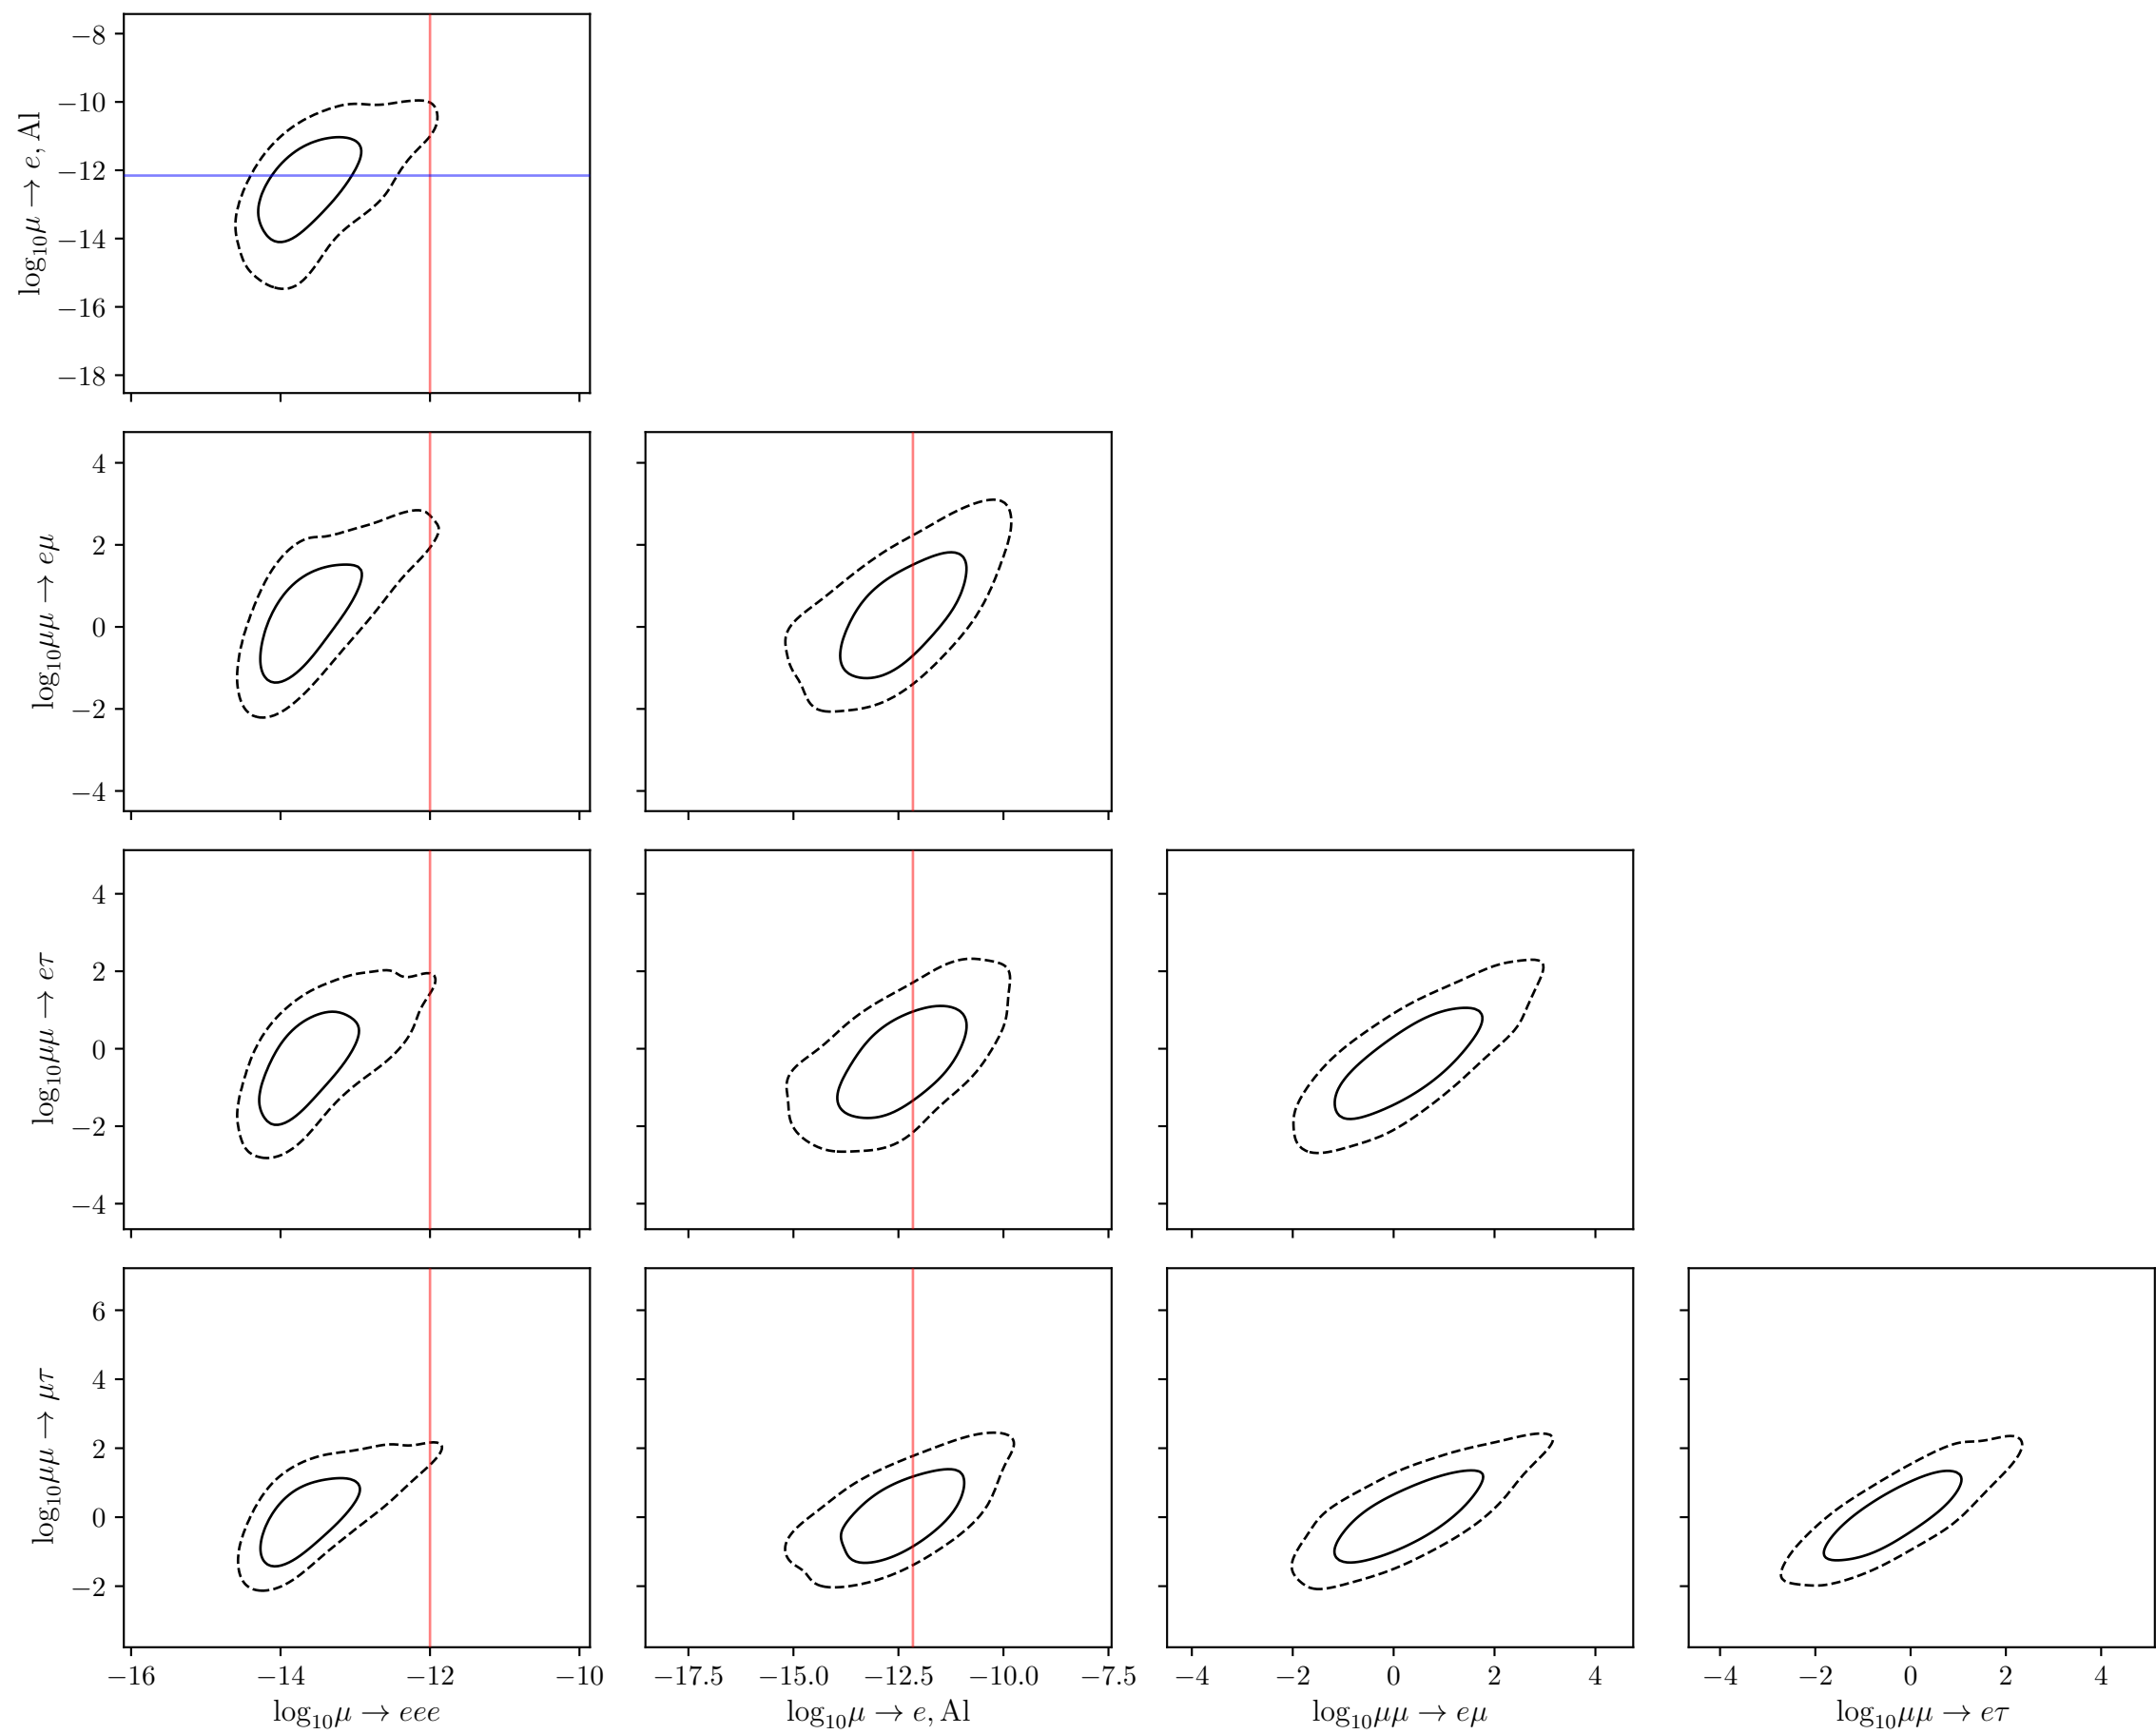

Majorana,  $X_L = \{5, 4, 3\}$ ,  $X_e = \{7, 4, 2\}$ ,

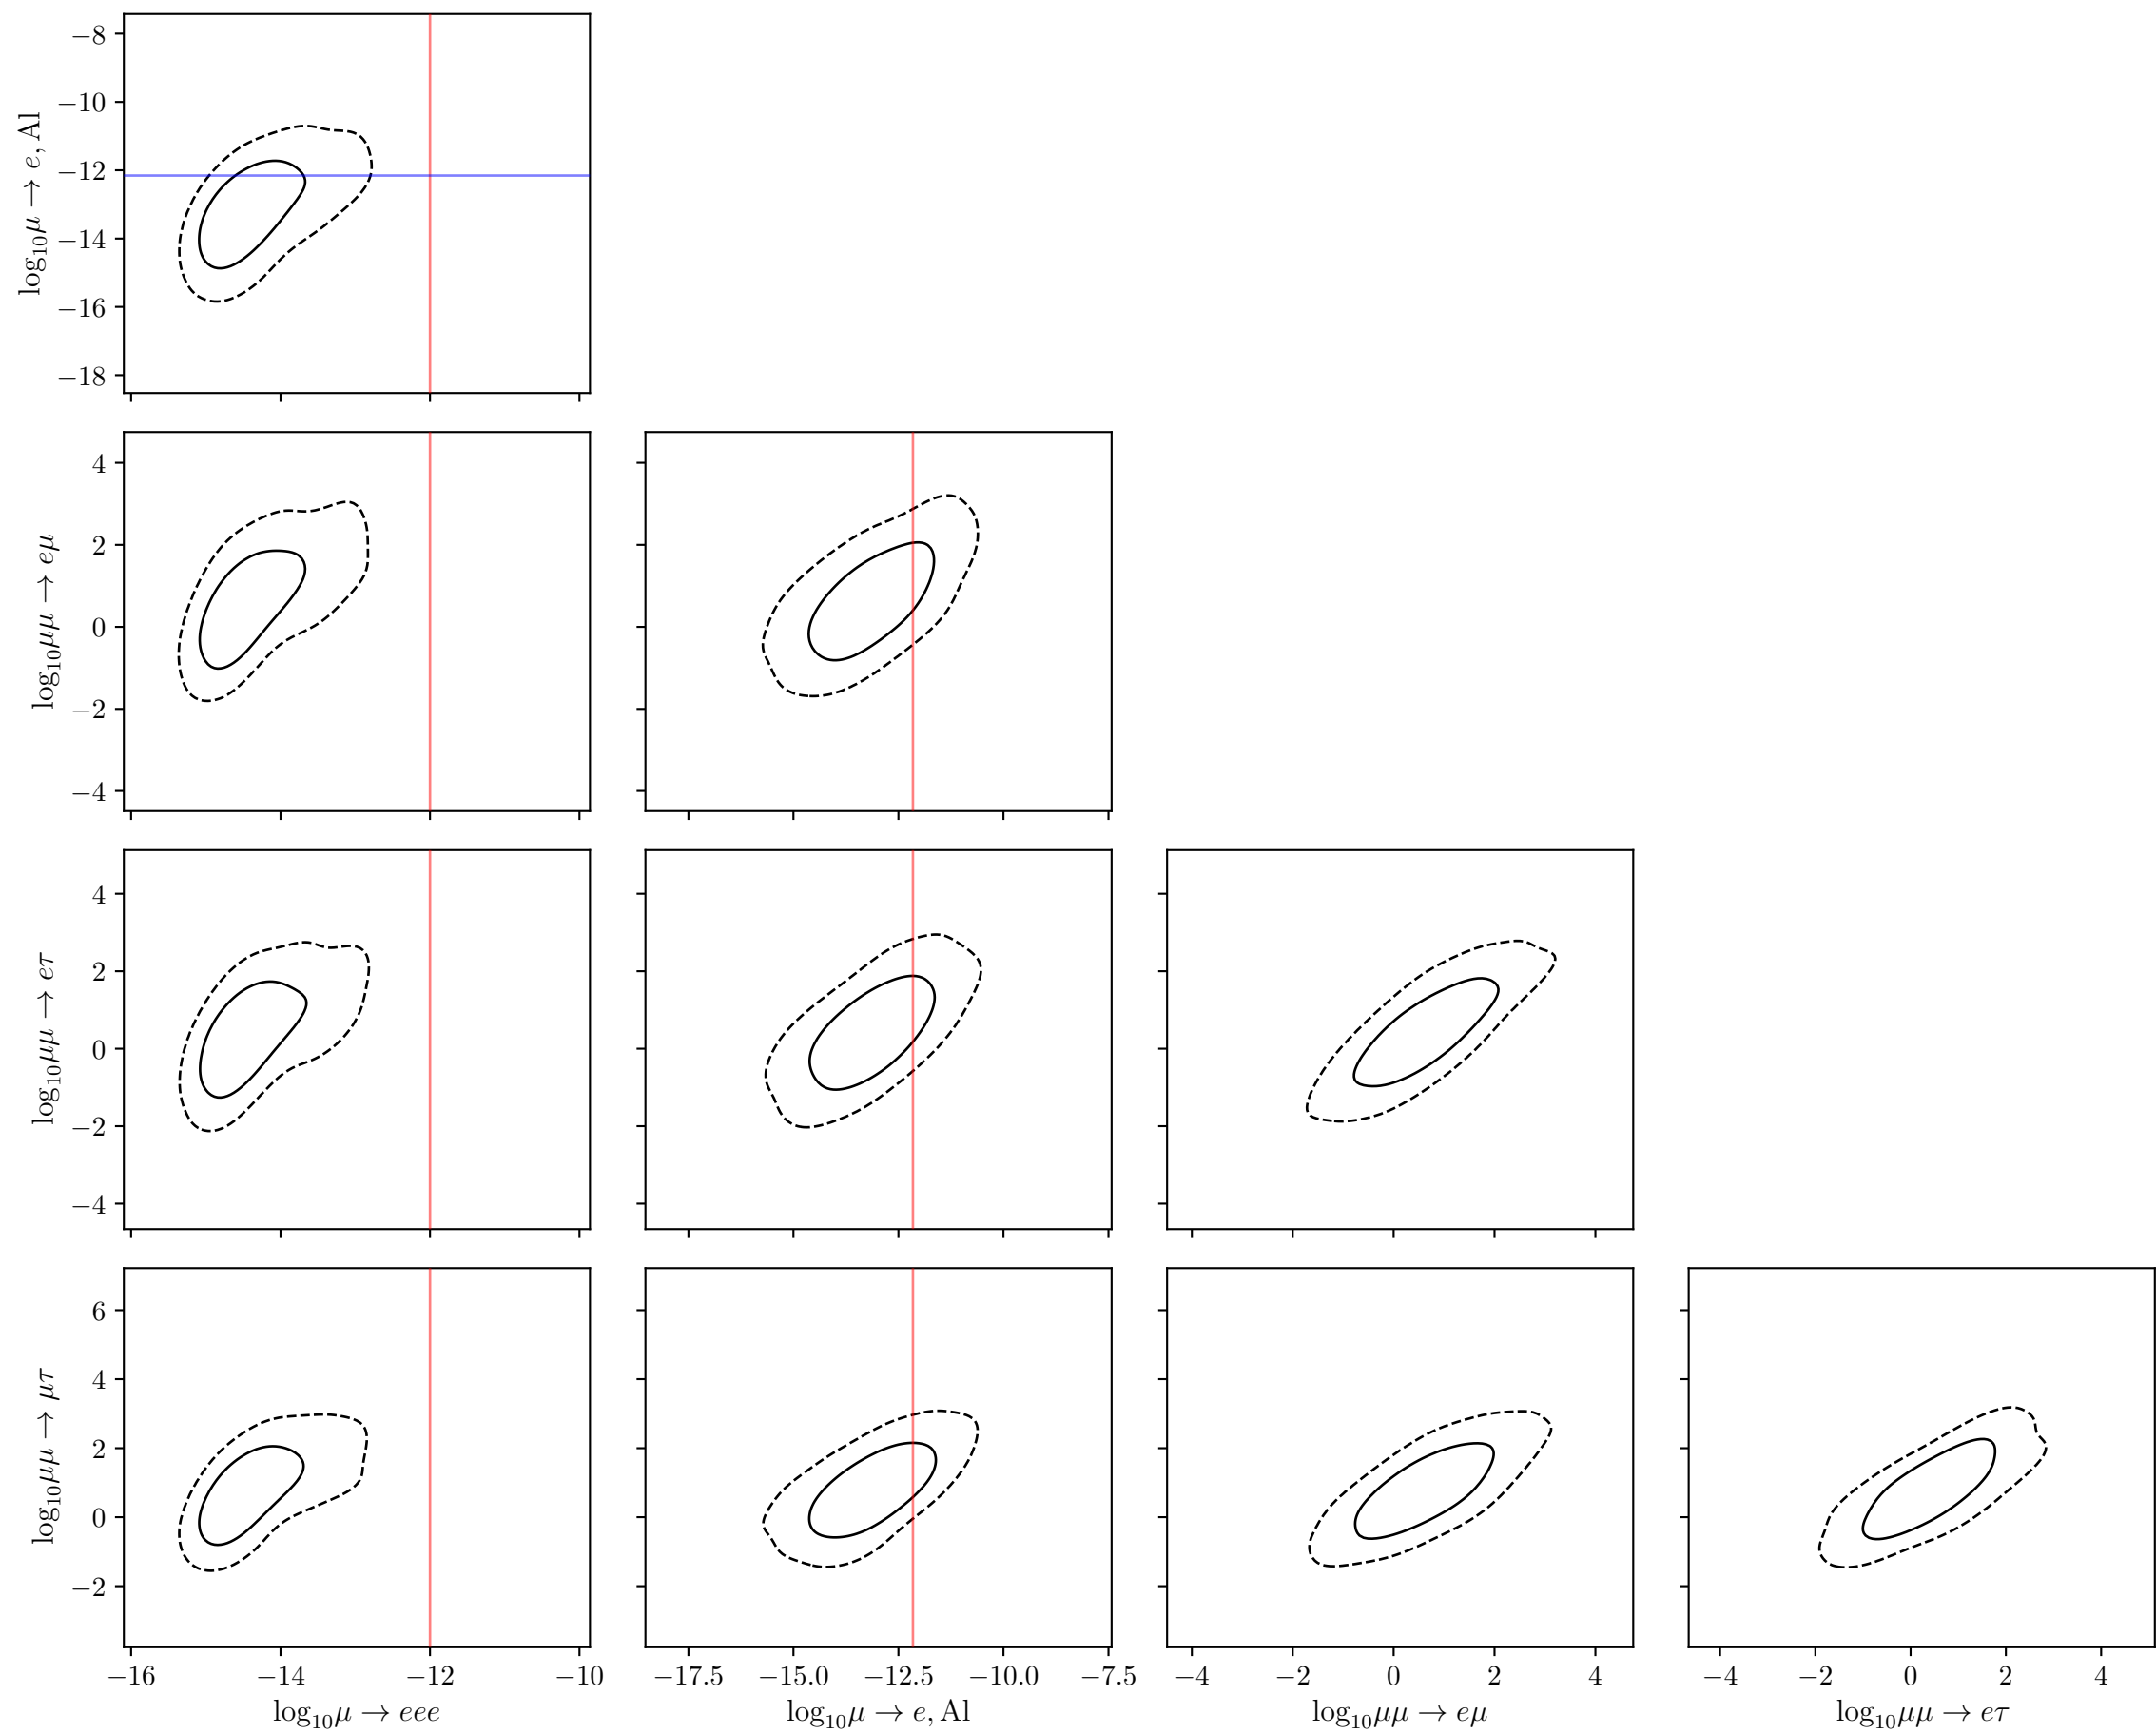

Majorana,  $X_L = \{6, 5, 4\}$ ,  $X_e = \{7, 2, 1\}$ ,

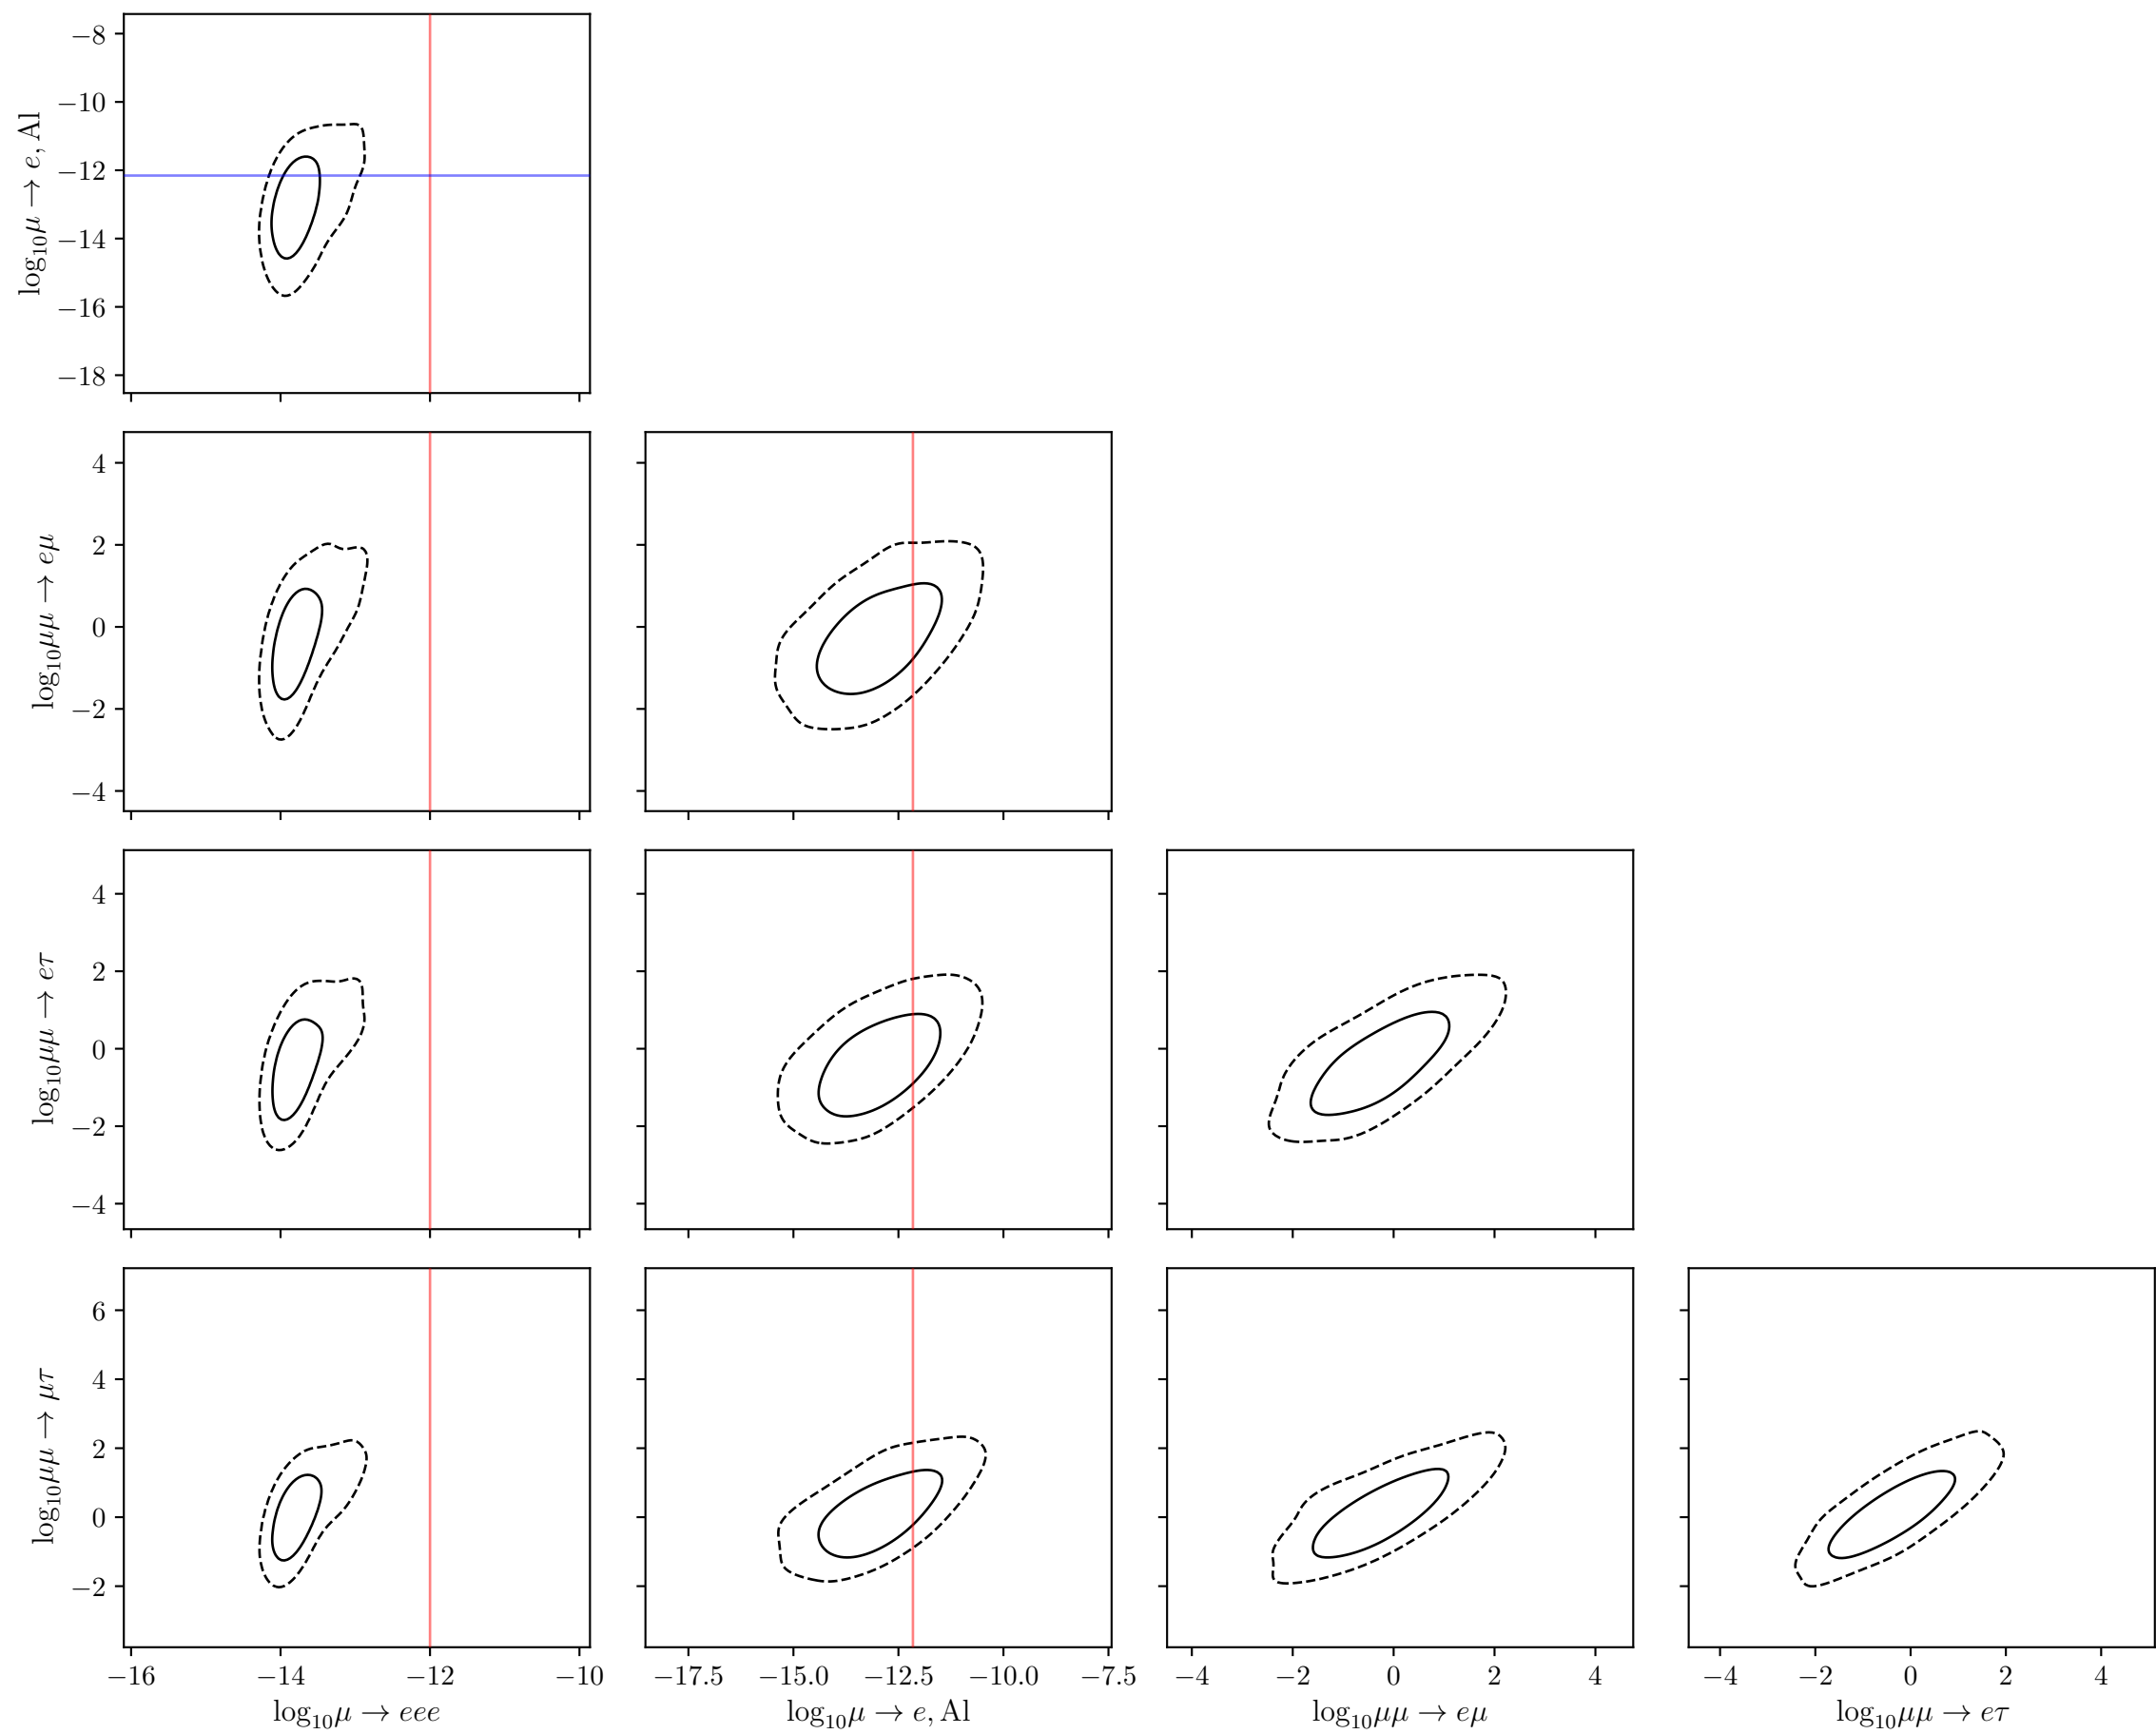

Majorana,  $X_L = \{5, 4, 3\}$ ,  $X_e = \{5, 2, 0\}$ ,

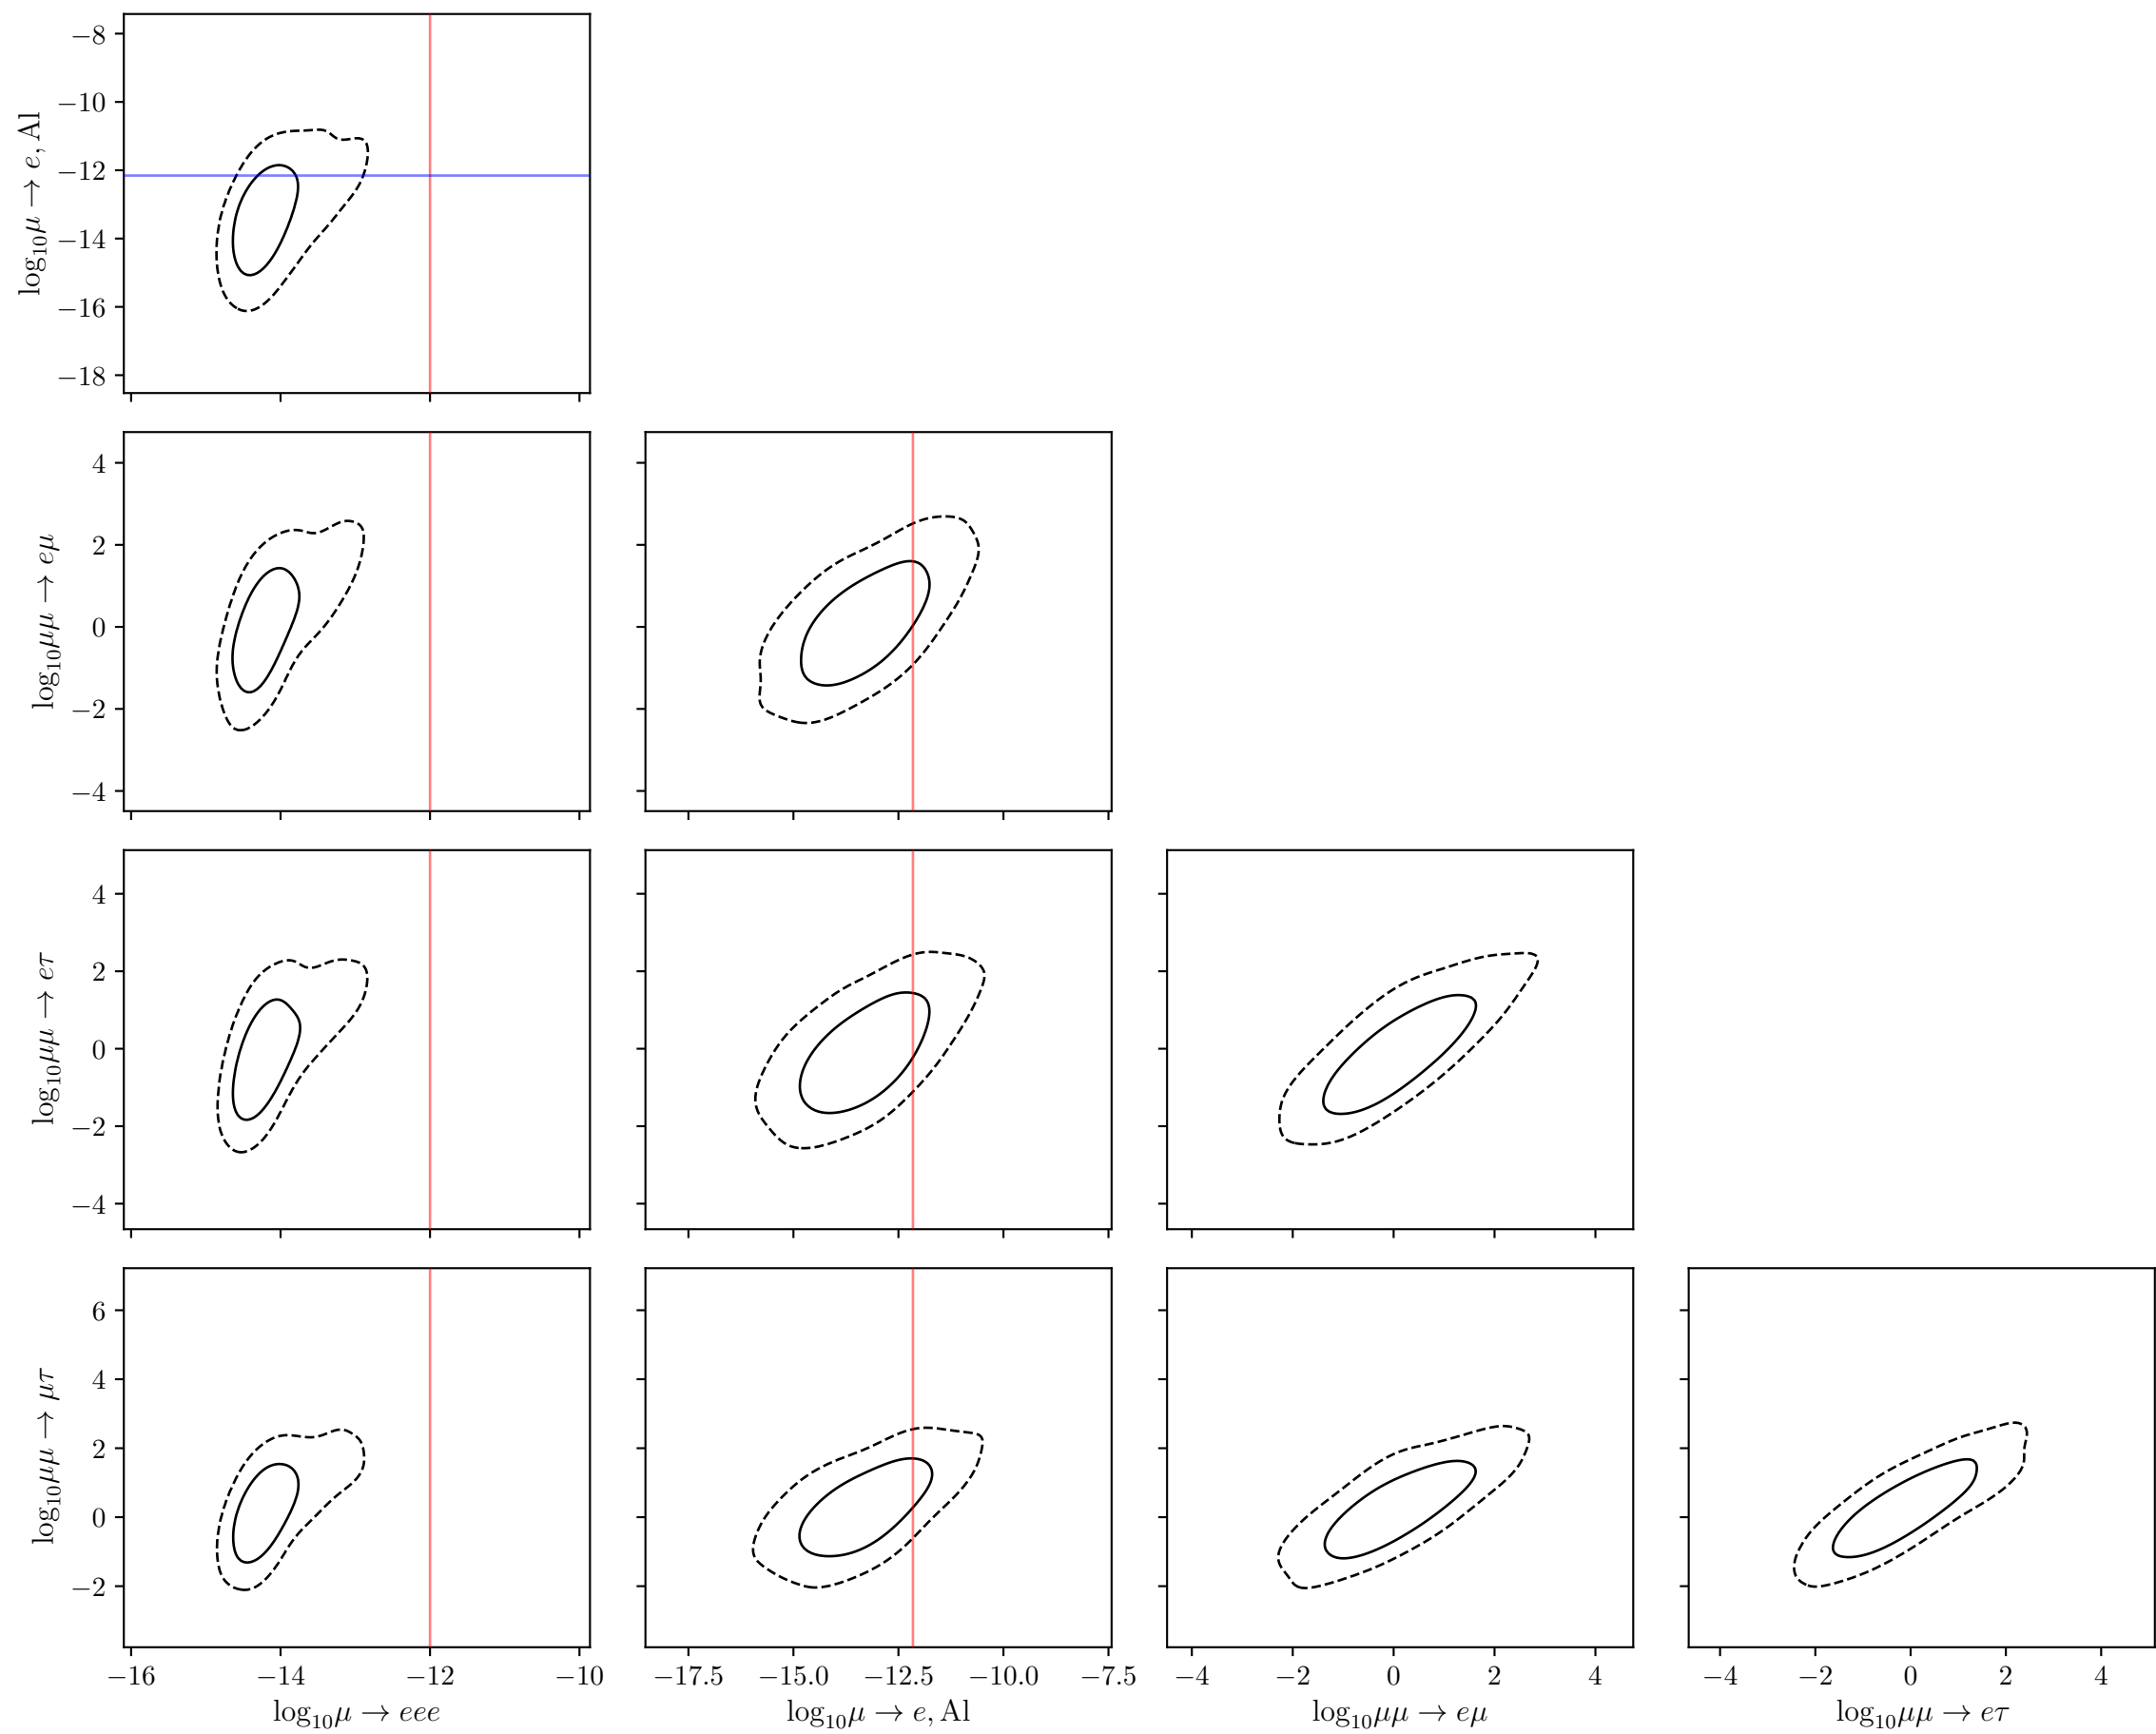

Majorana,  $X_L = \{5, 5, 4\}$ ,  $X_e = \{7, 3, 1\}$ ,

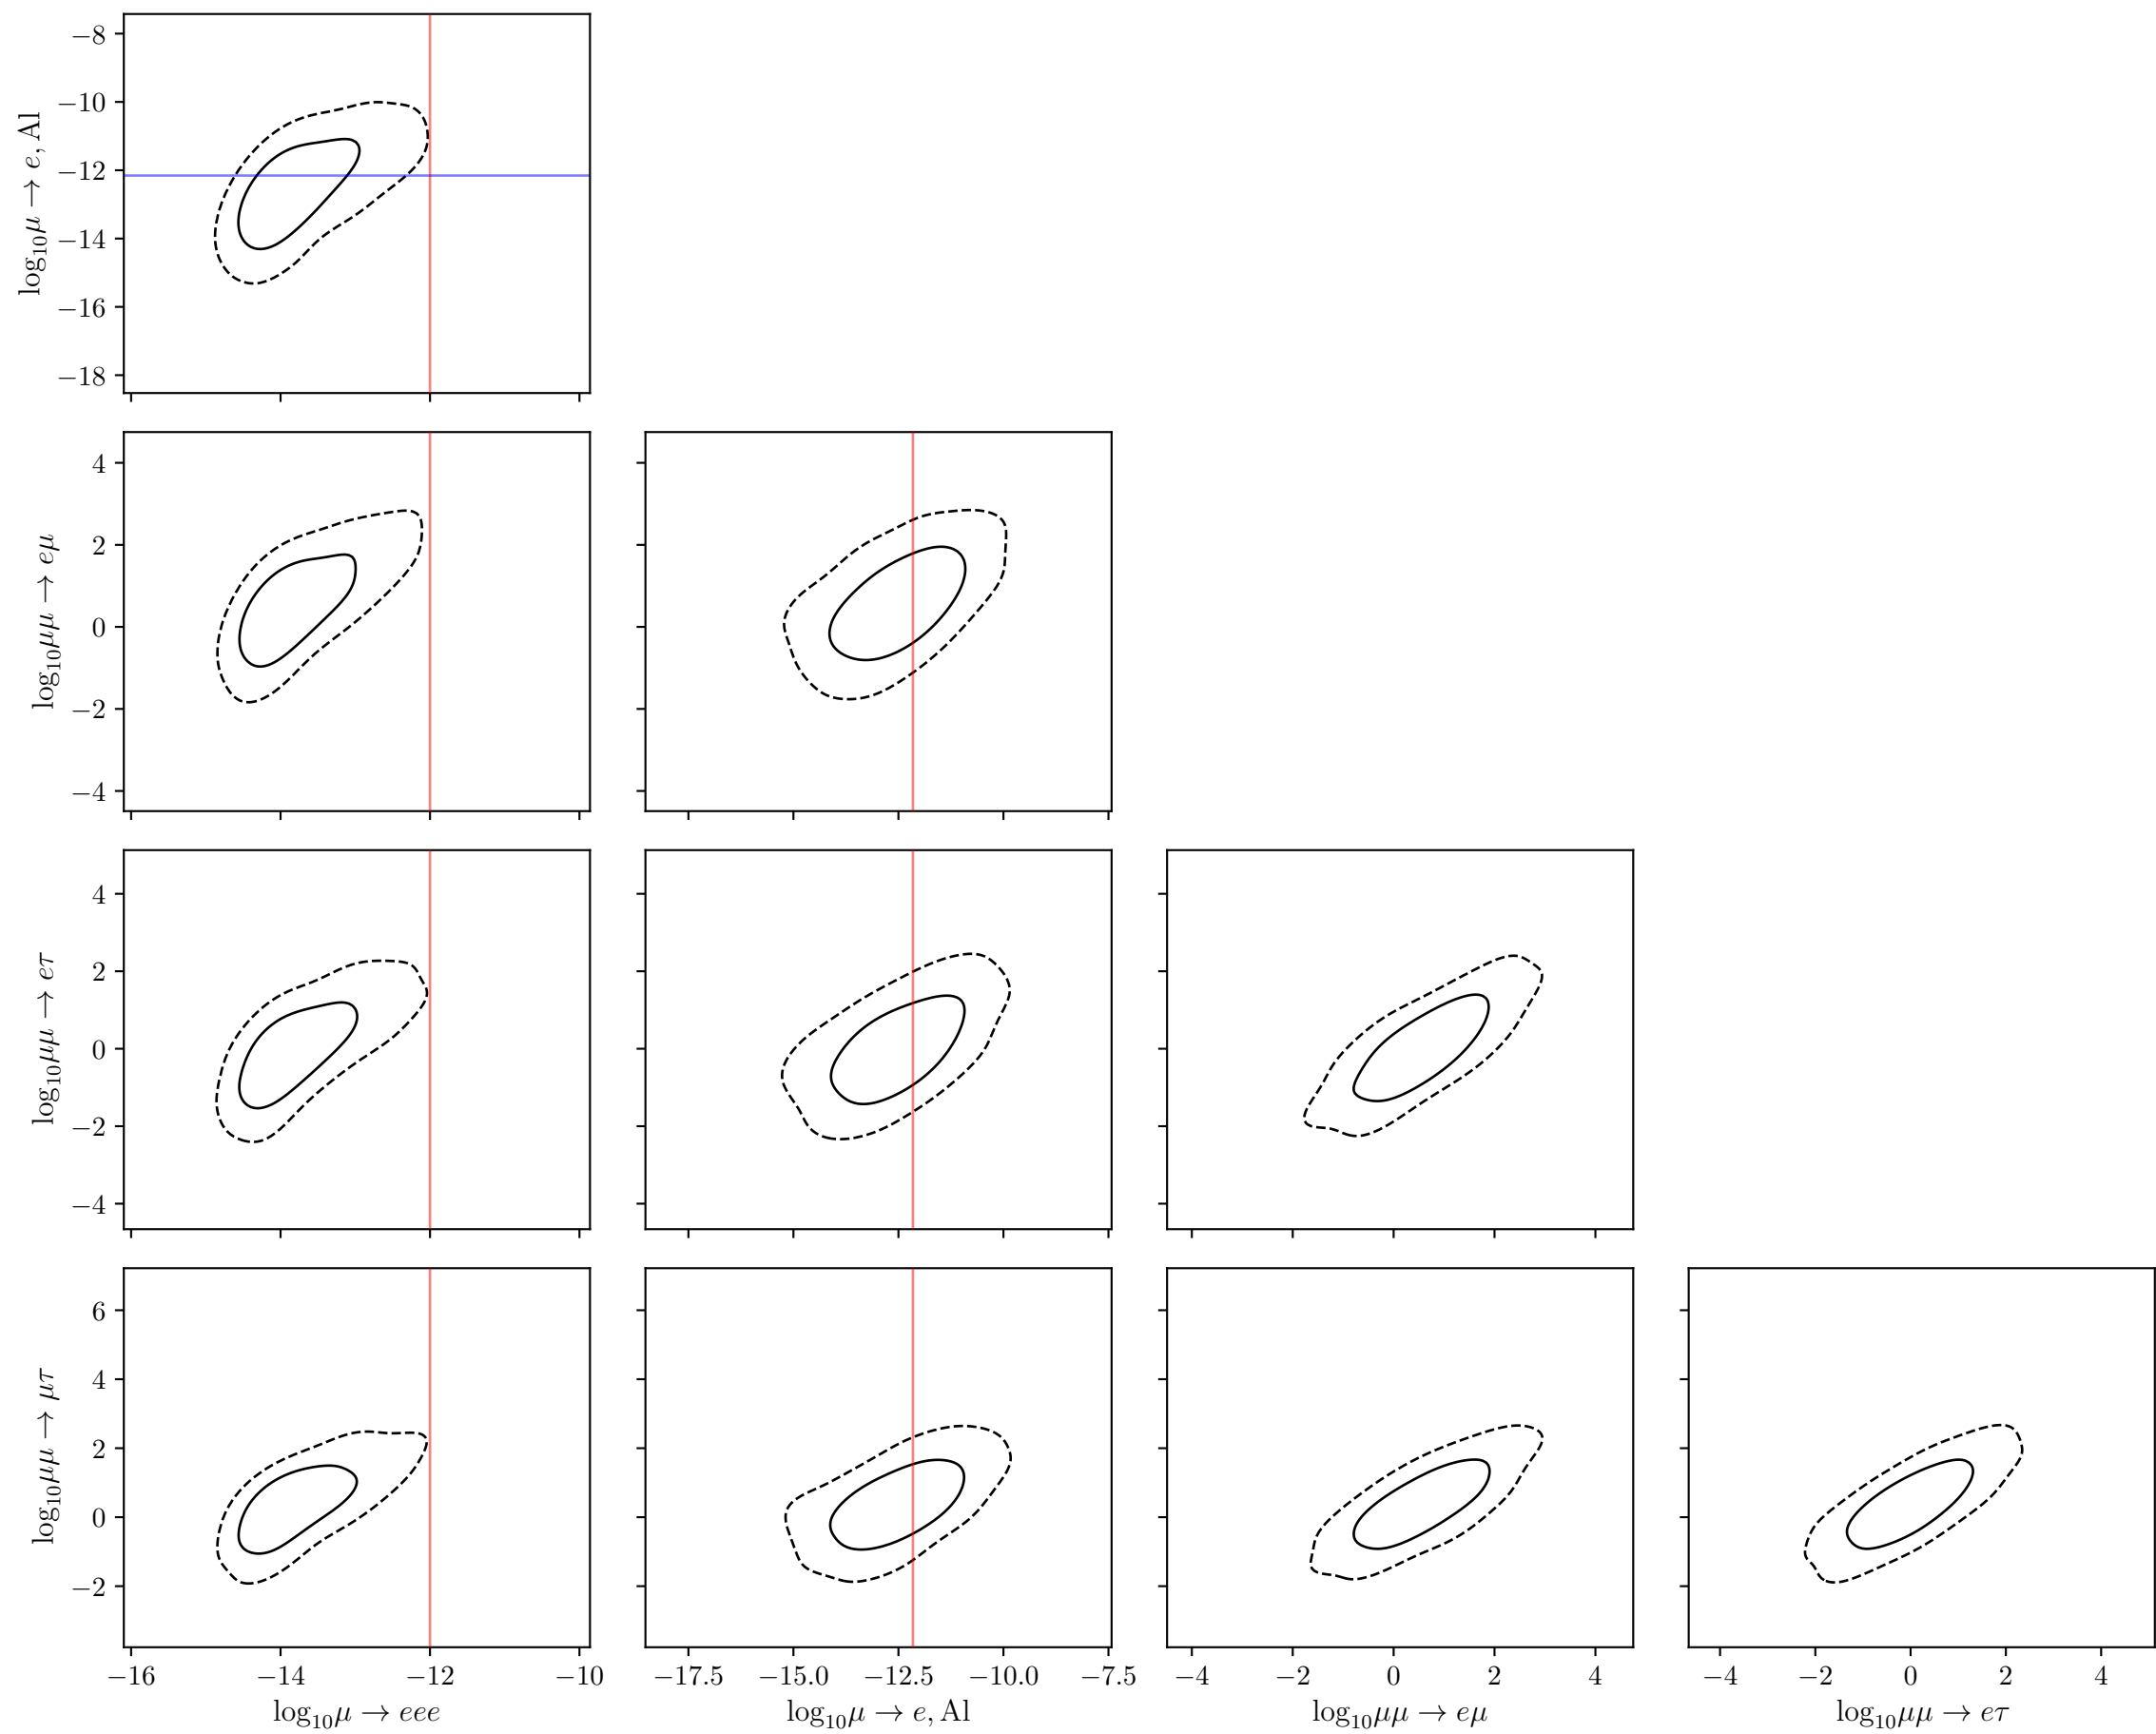

Majorana,  $X_L = \{3, 2, 1\}$ ,  $X_e = \{7, 4, 2\}$ ,

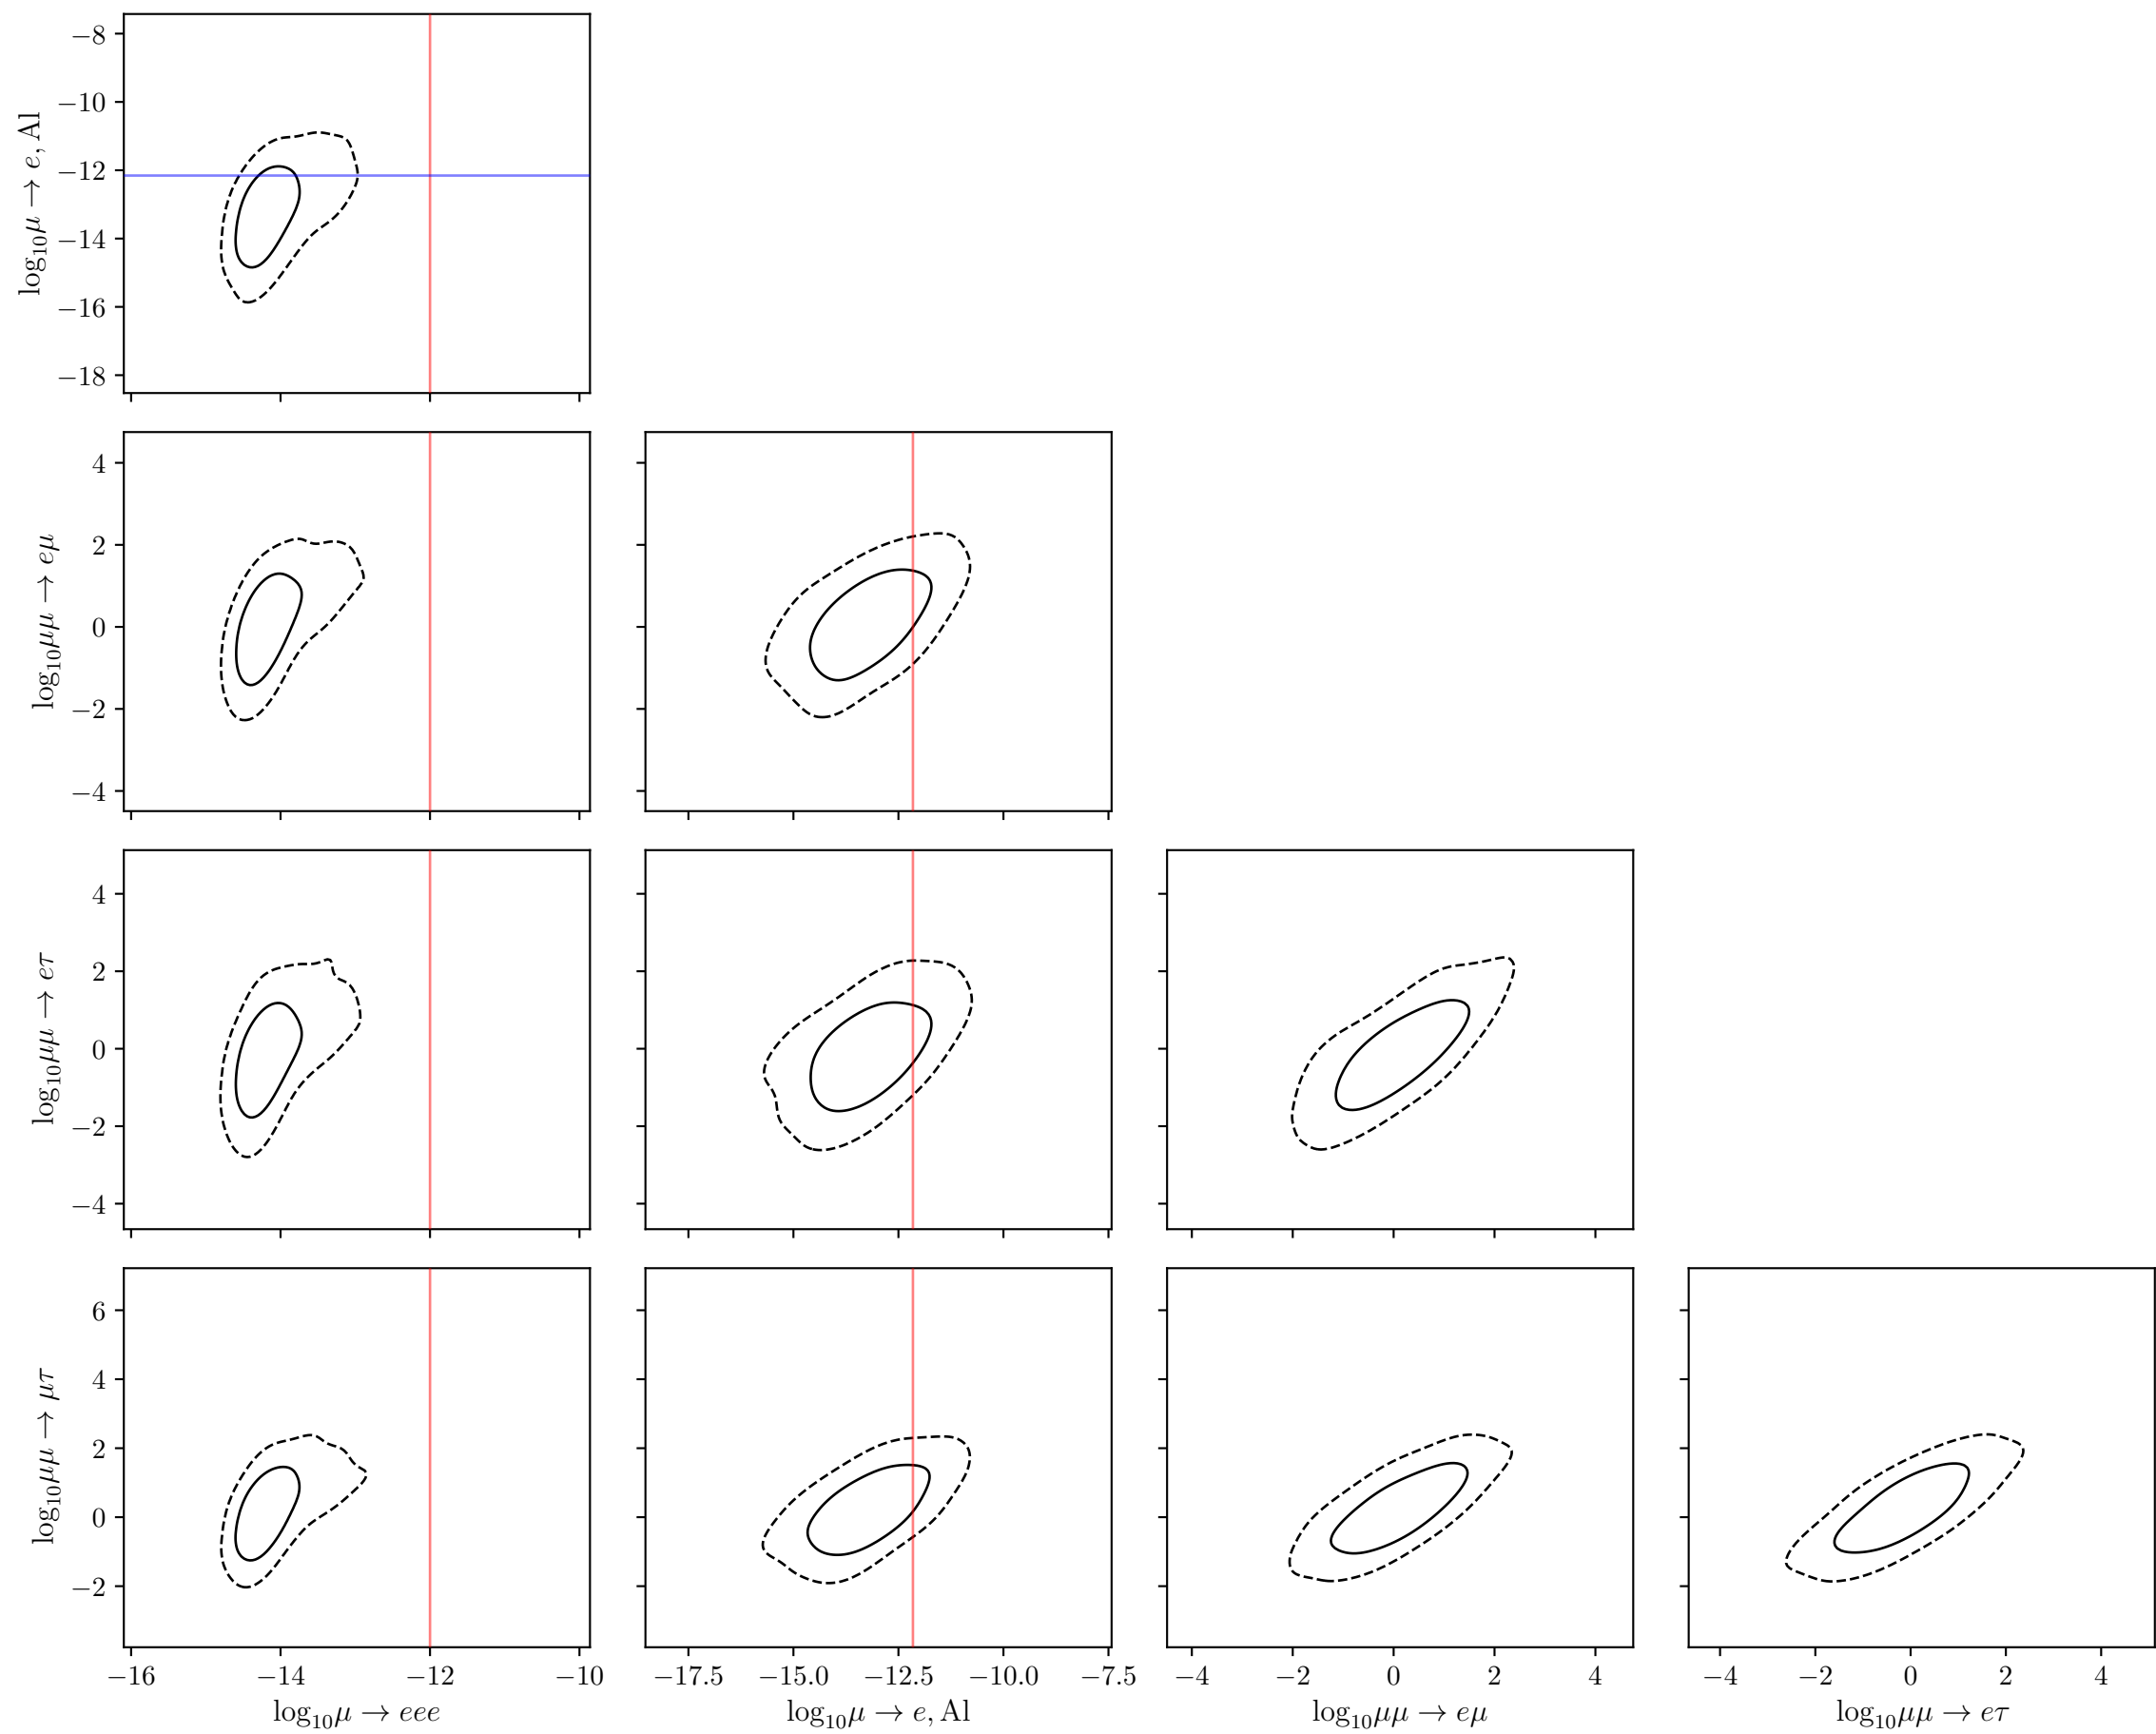



Majorana,  $X_L = \{7, 6, 5\}$ ,  $X_e = \{-1, 1, 6\}$ ,

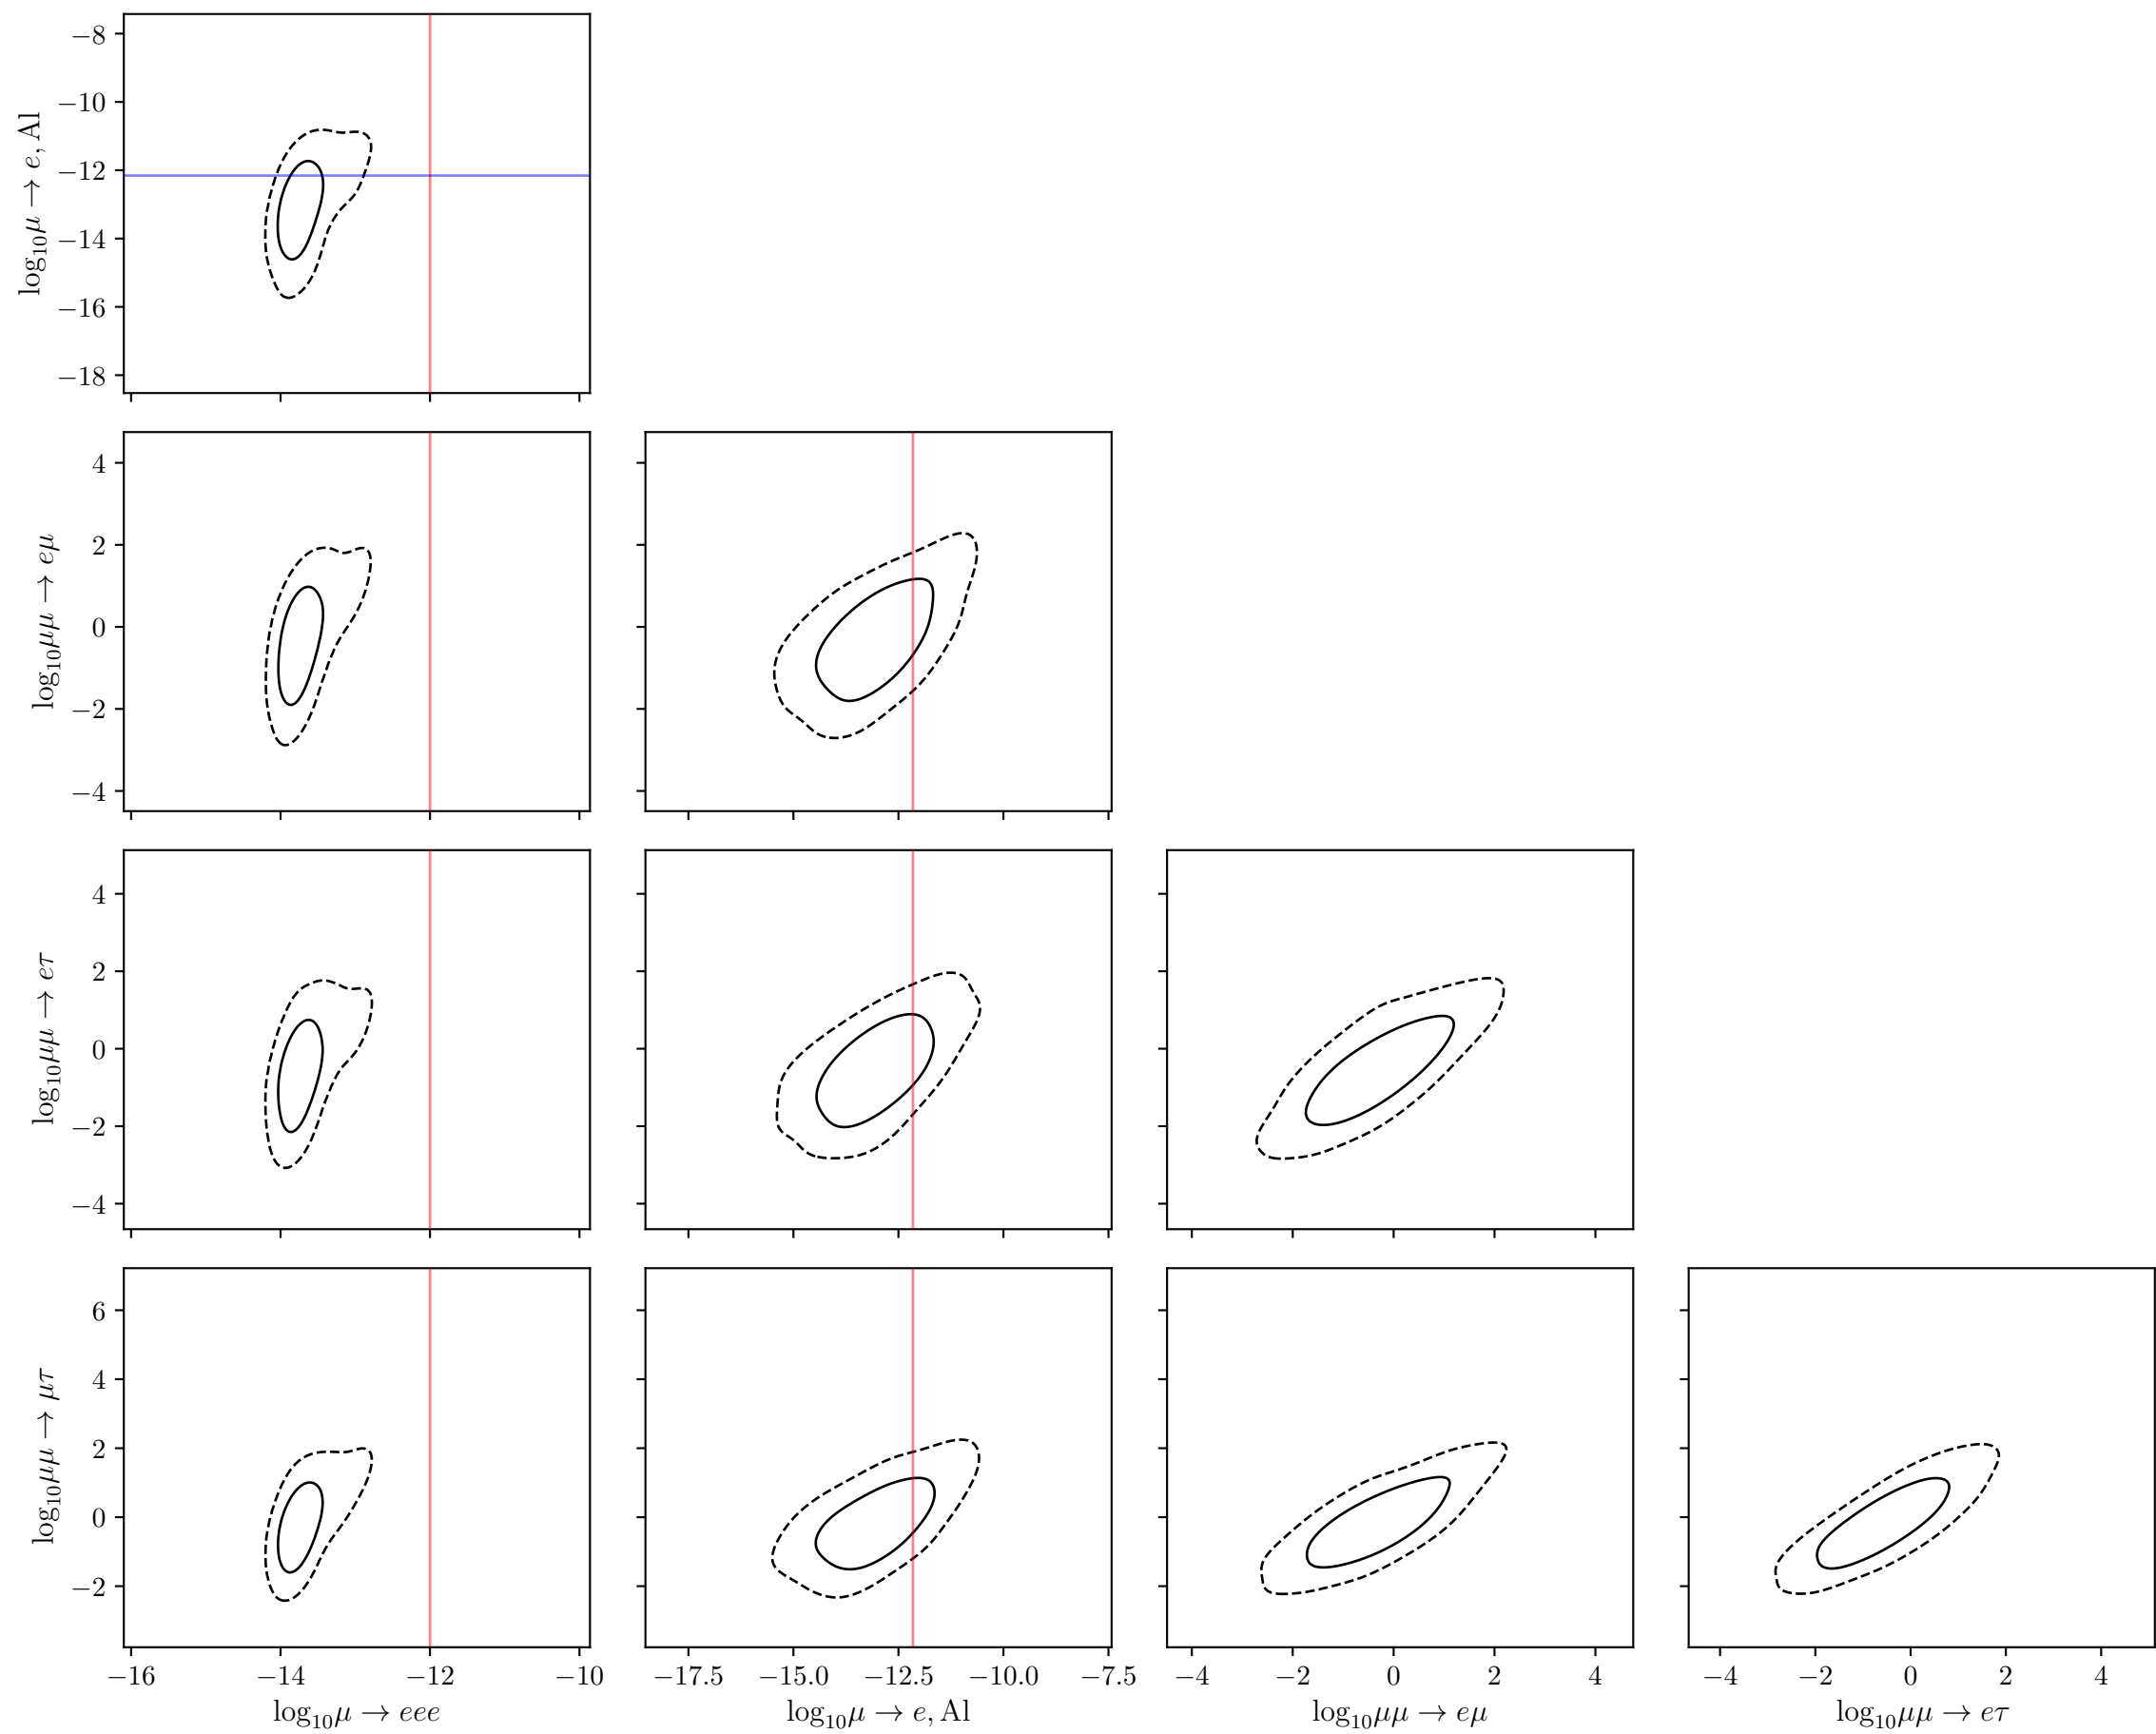

Majorana,  $X_L = \{7, 5, 4\}$ ,  $X_e = \{7, 3, 1\}$ ,

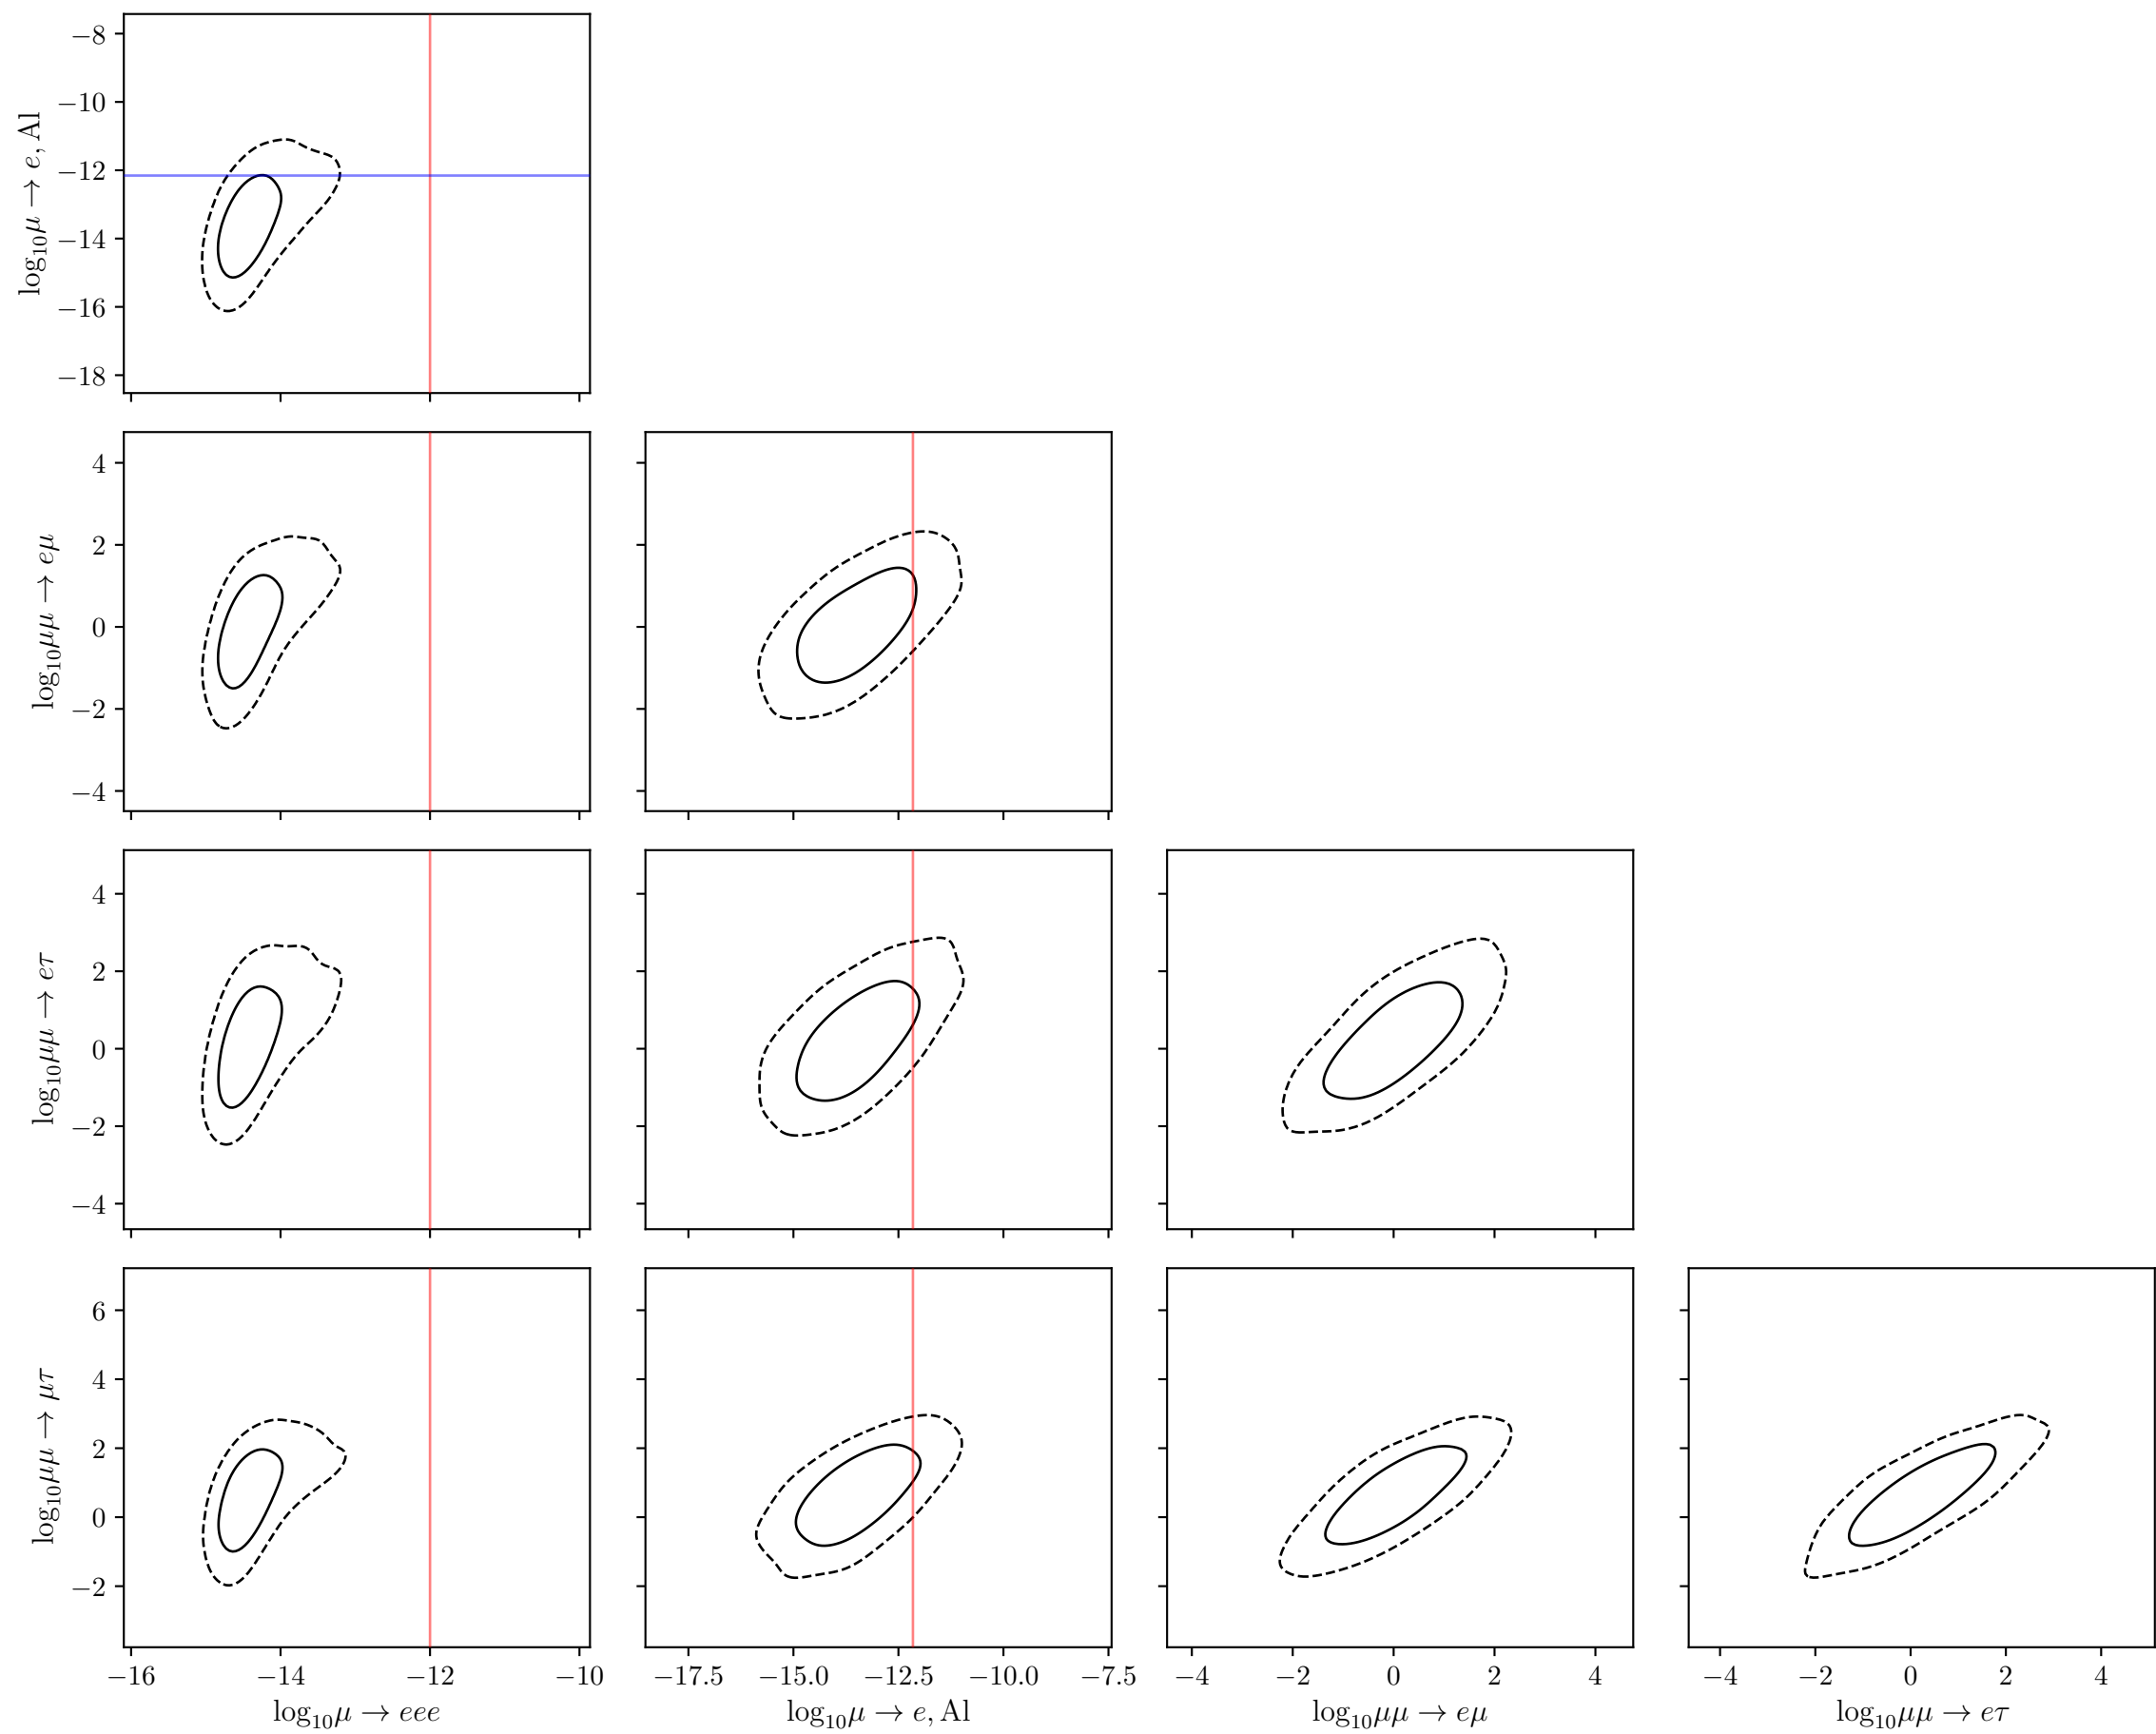

Majorana,  $X_L = \{7, 6, 5\}$ ,  $X_e = \{-1, 2, 7\}$ ,

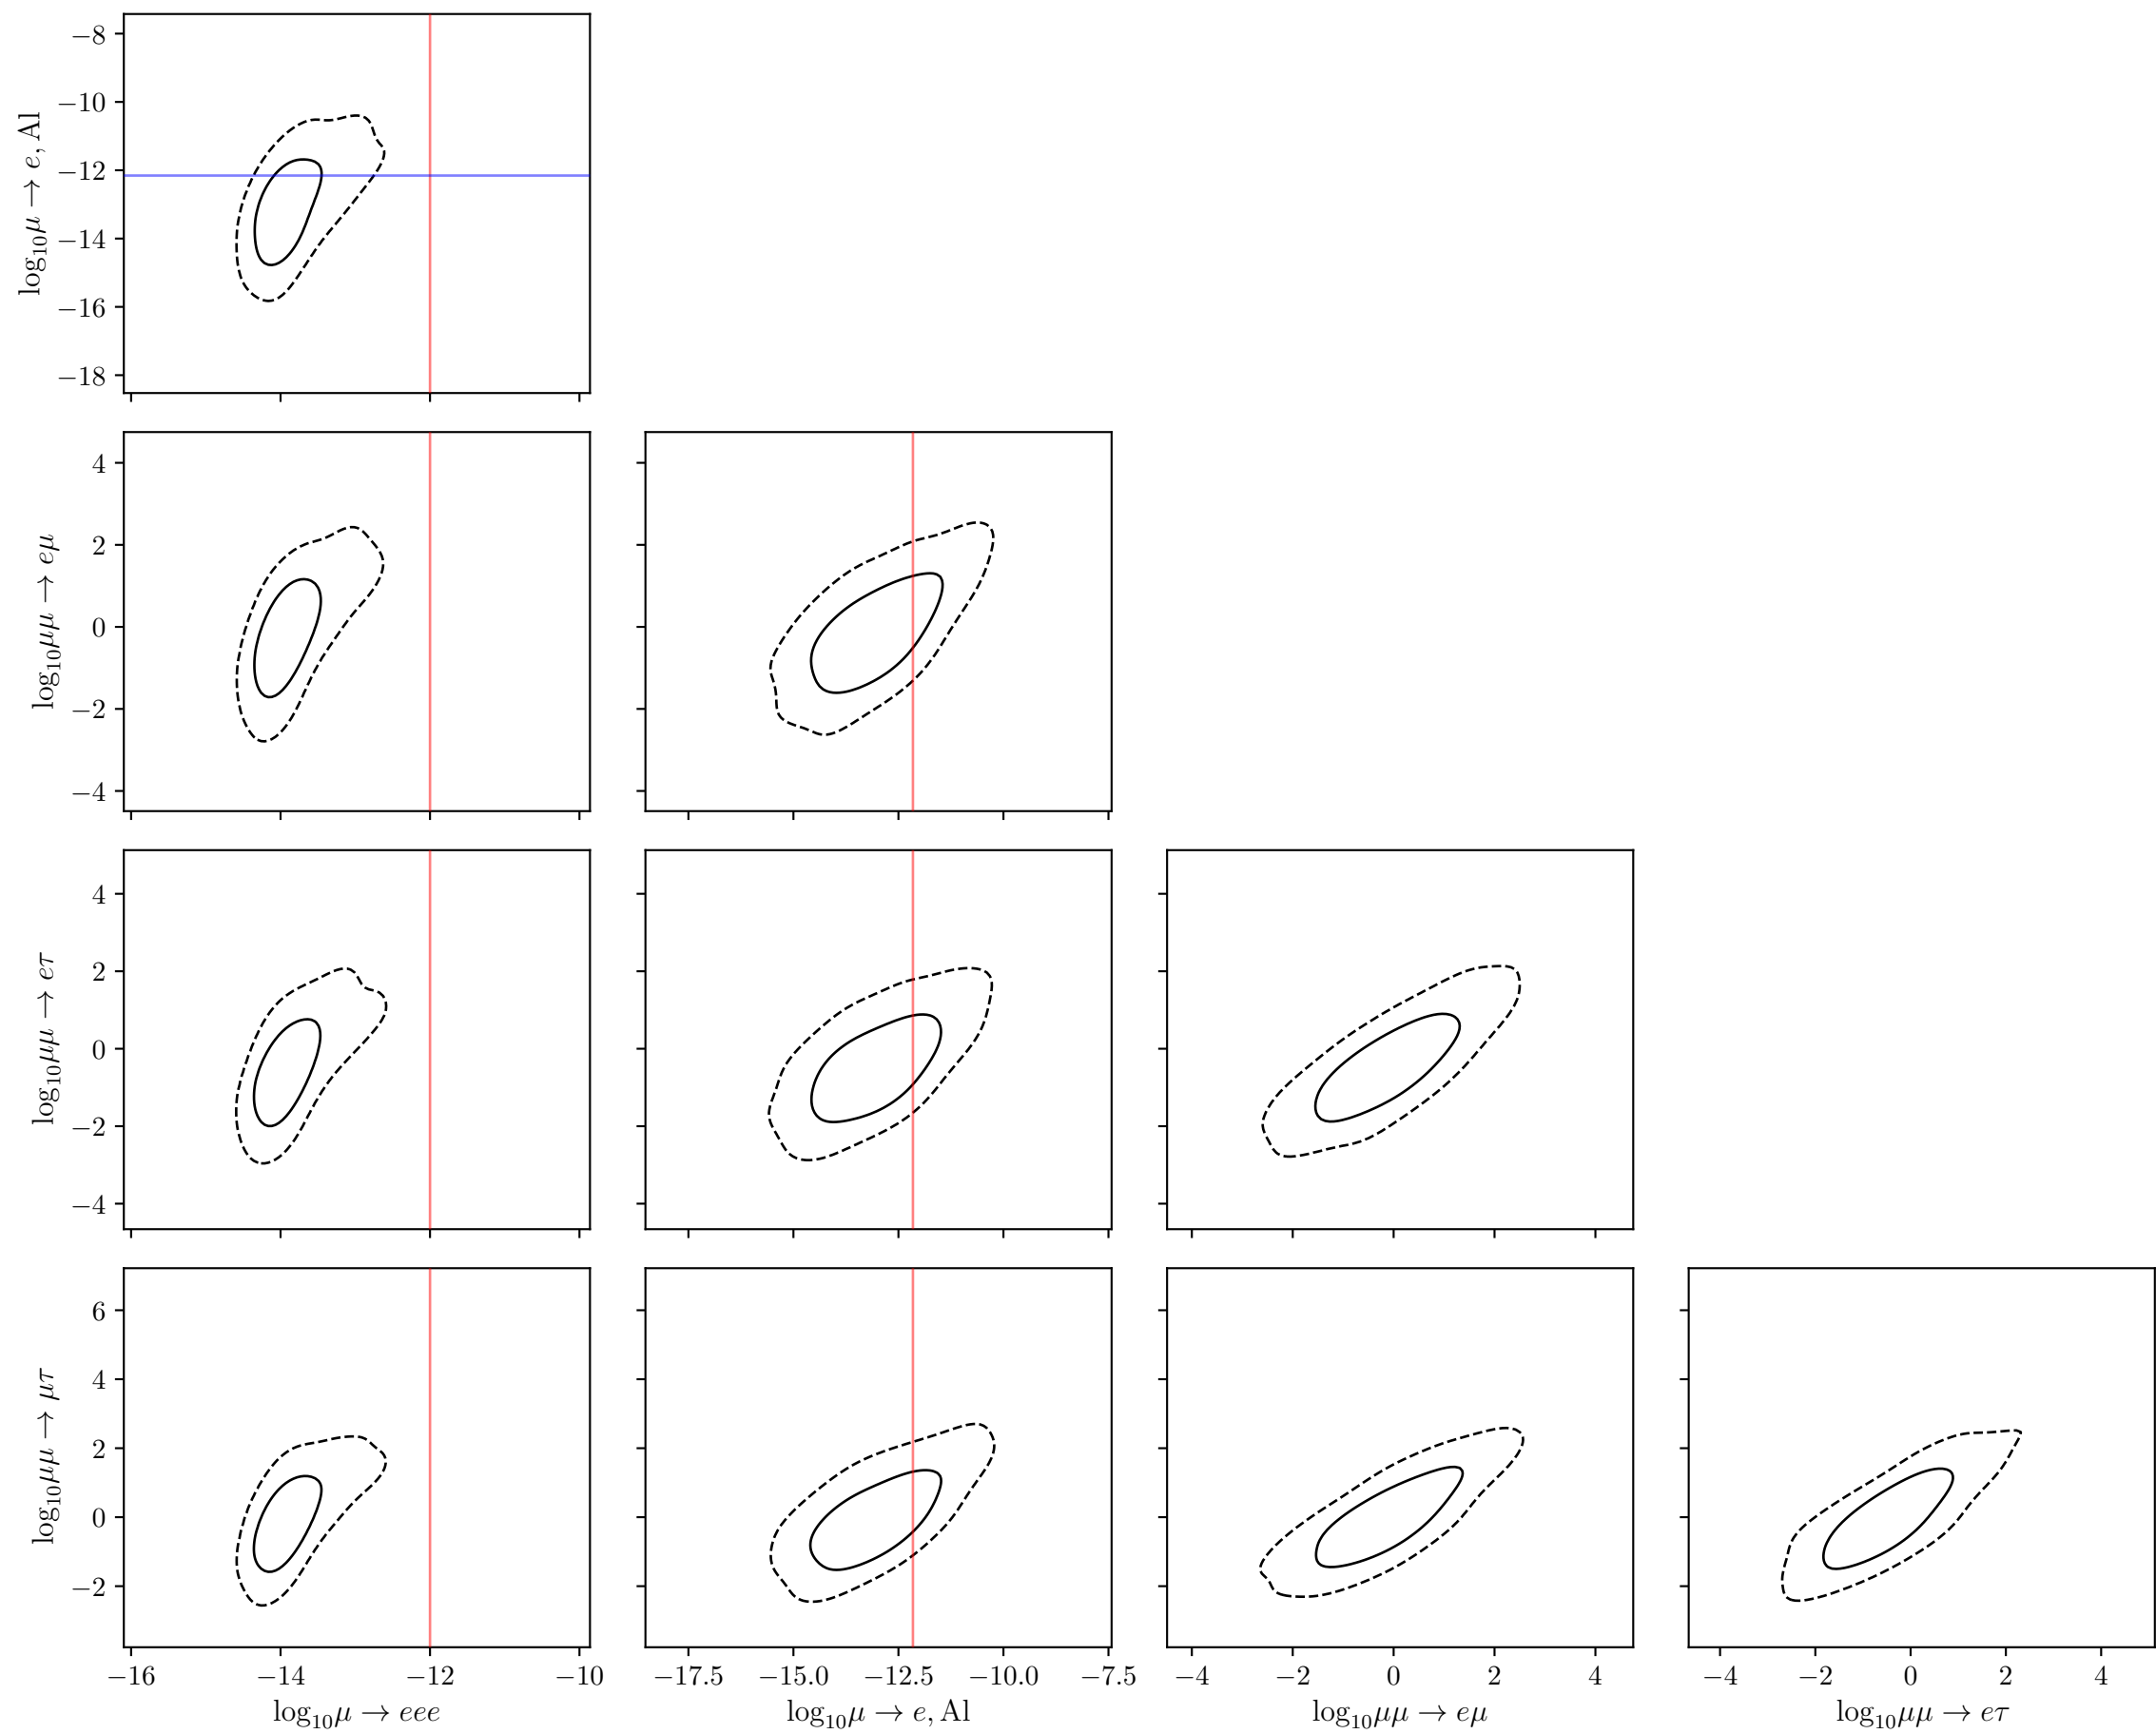

Majorana,  $X_L = \{6, 6, 5\}$ ,  $X_e = \{-1, 1, 6\}$ ,

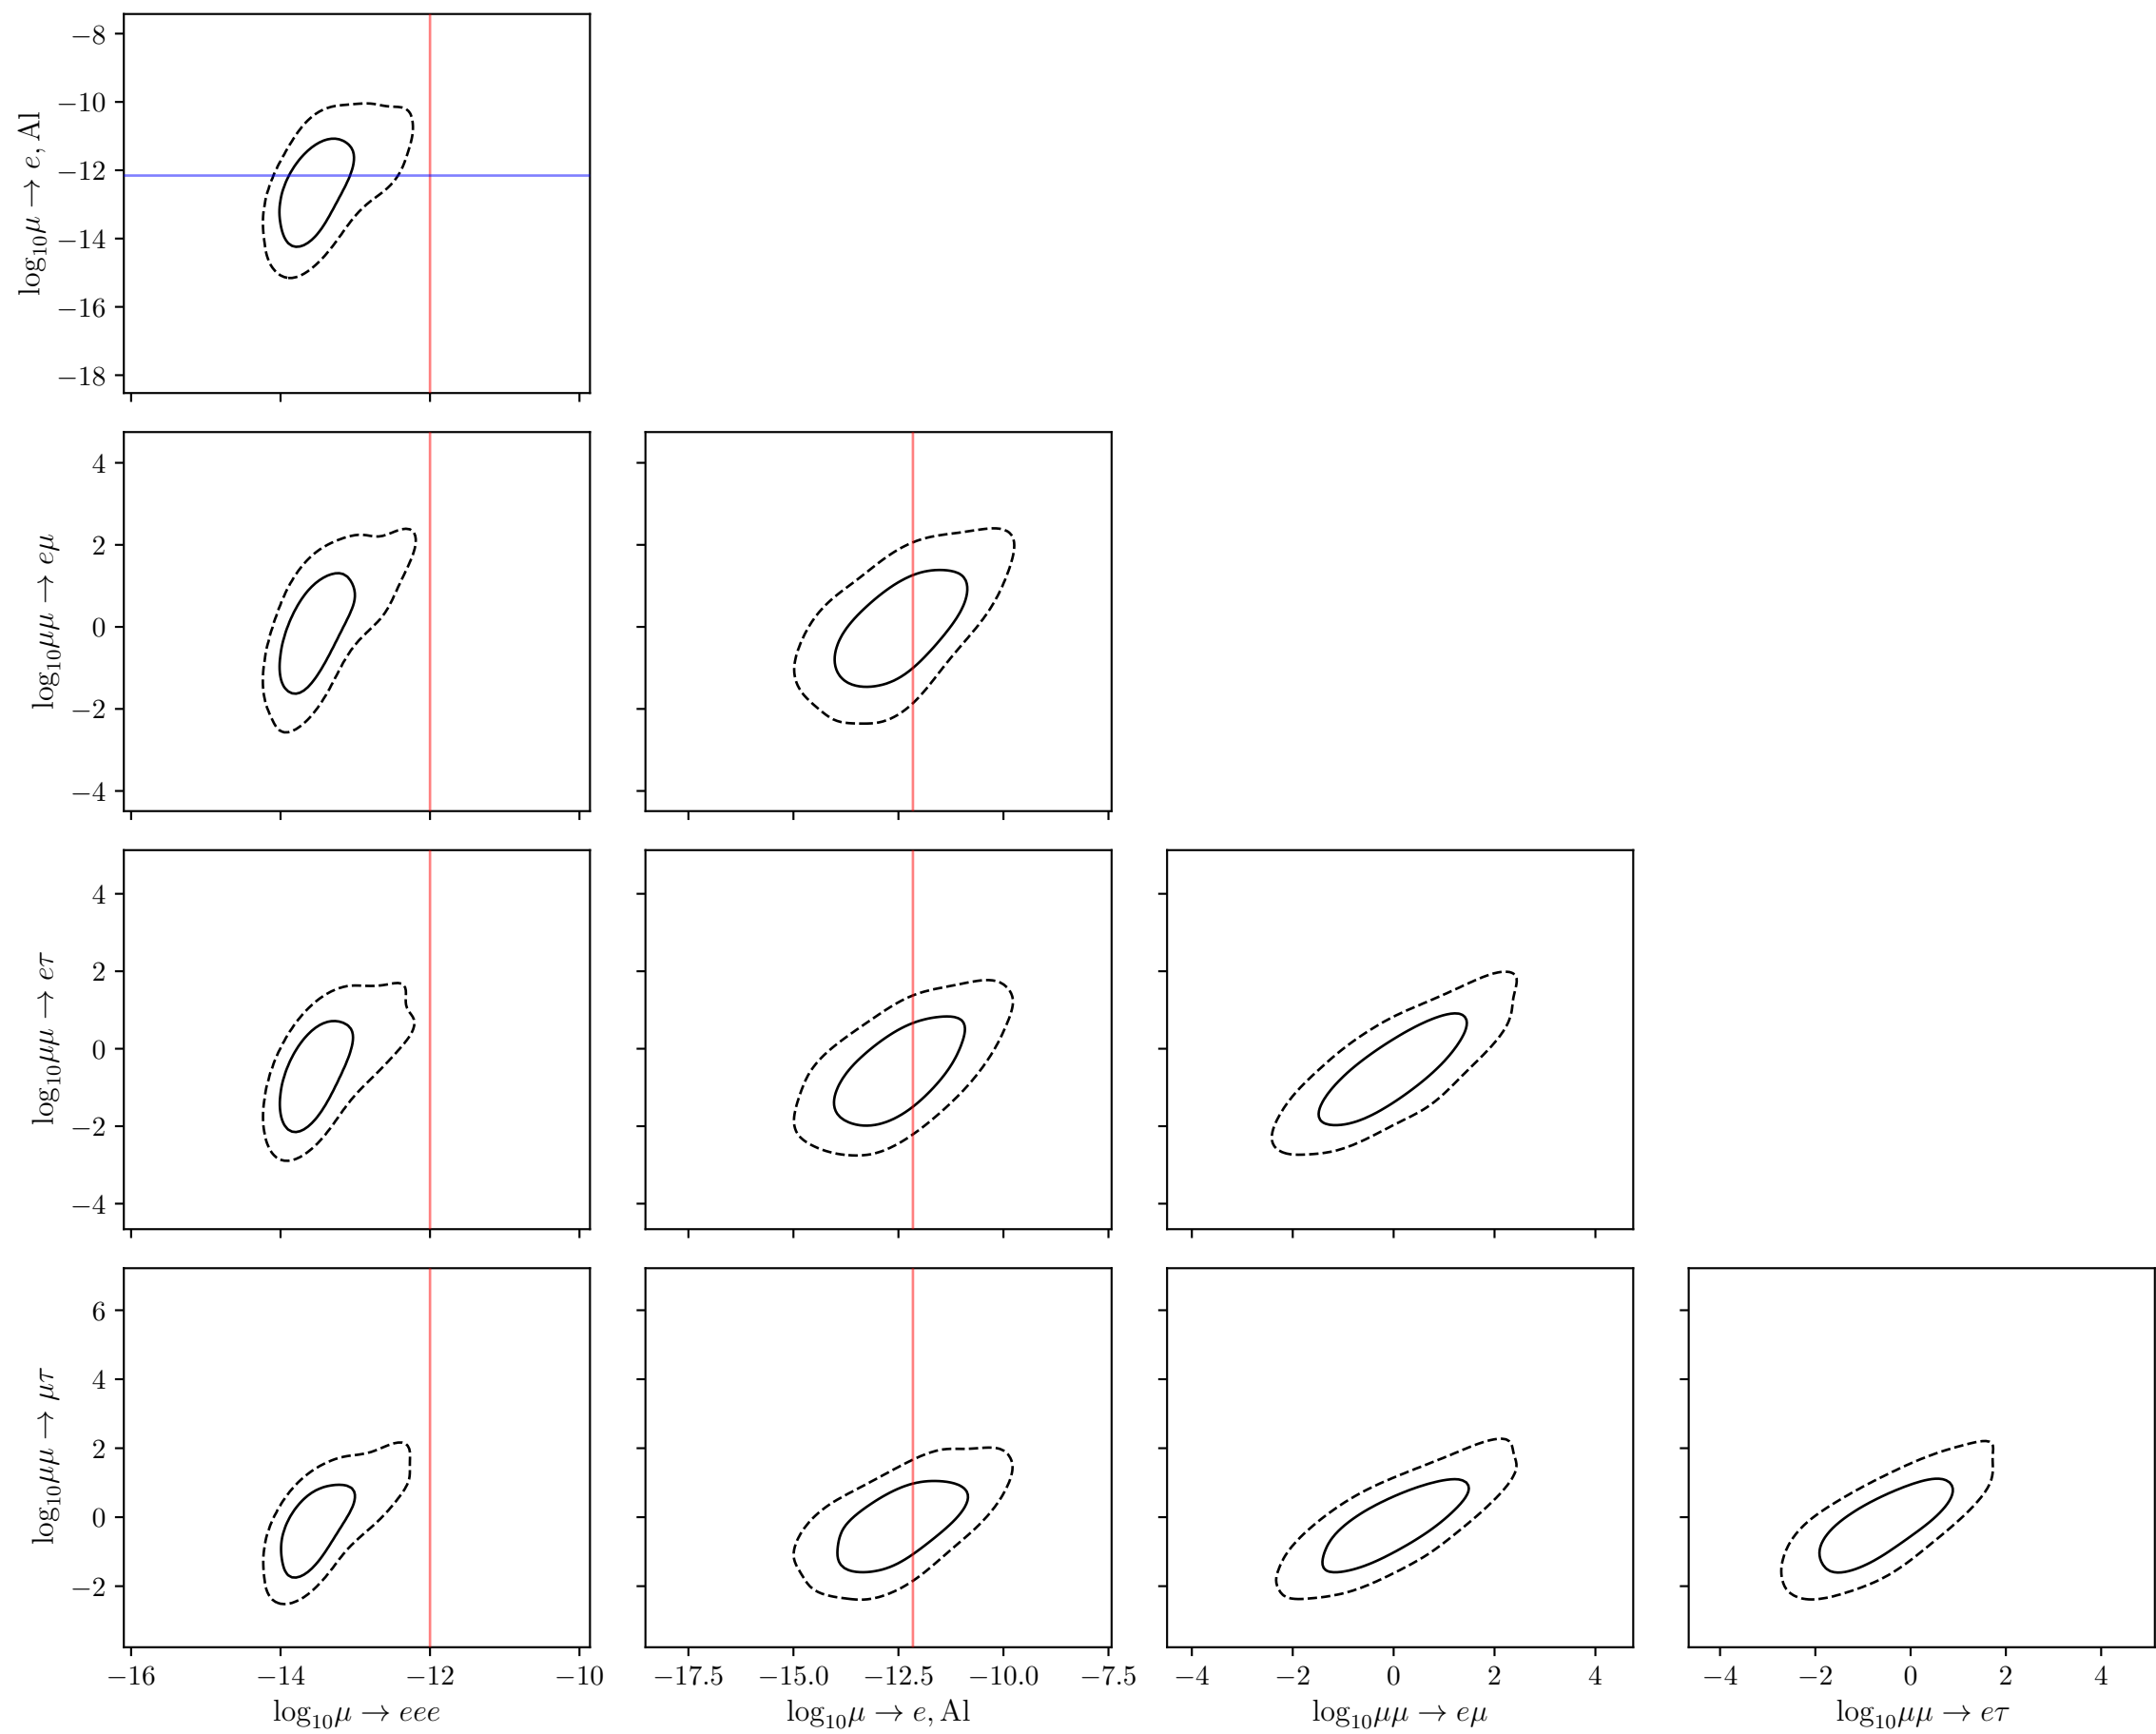

Majorana,  $X_L = \{6, 6, 5\}$ ,  $X_e = \{-2, -1, 2\}$ ,

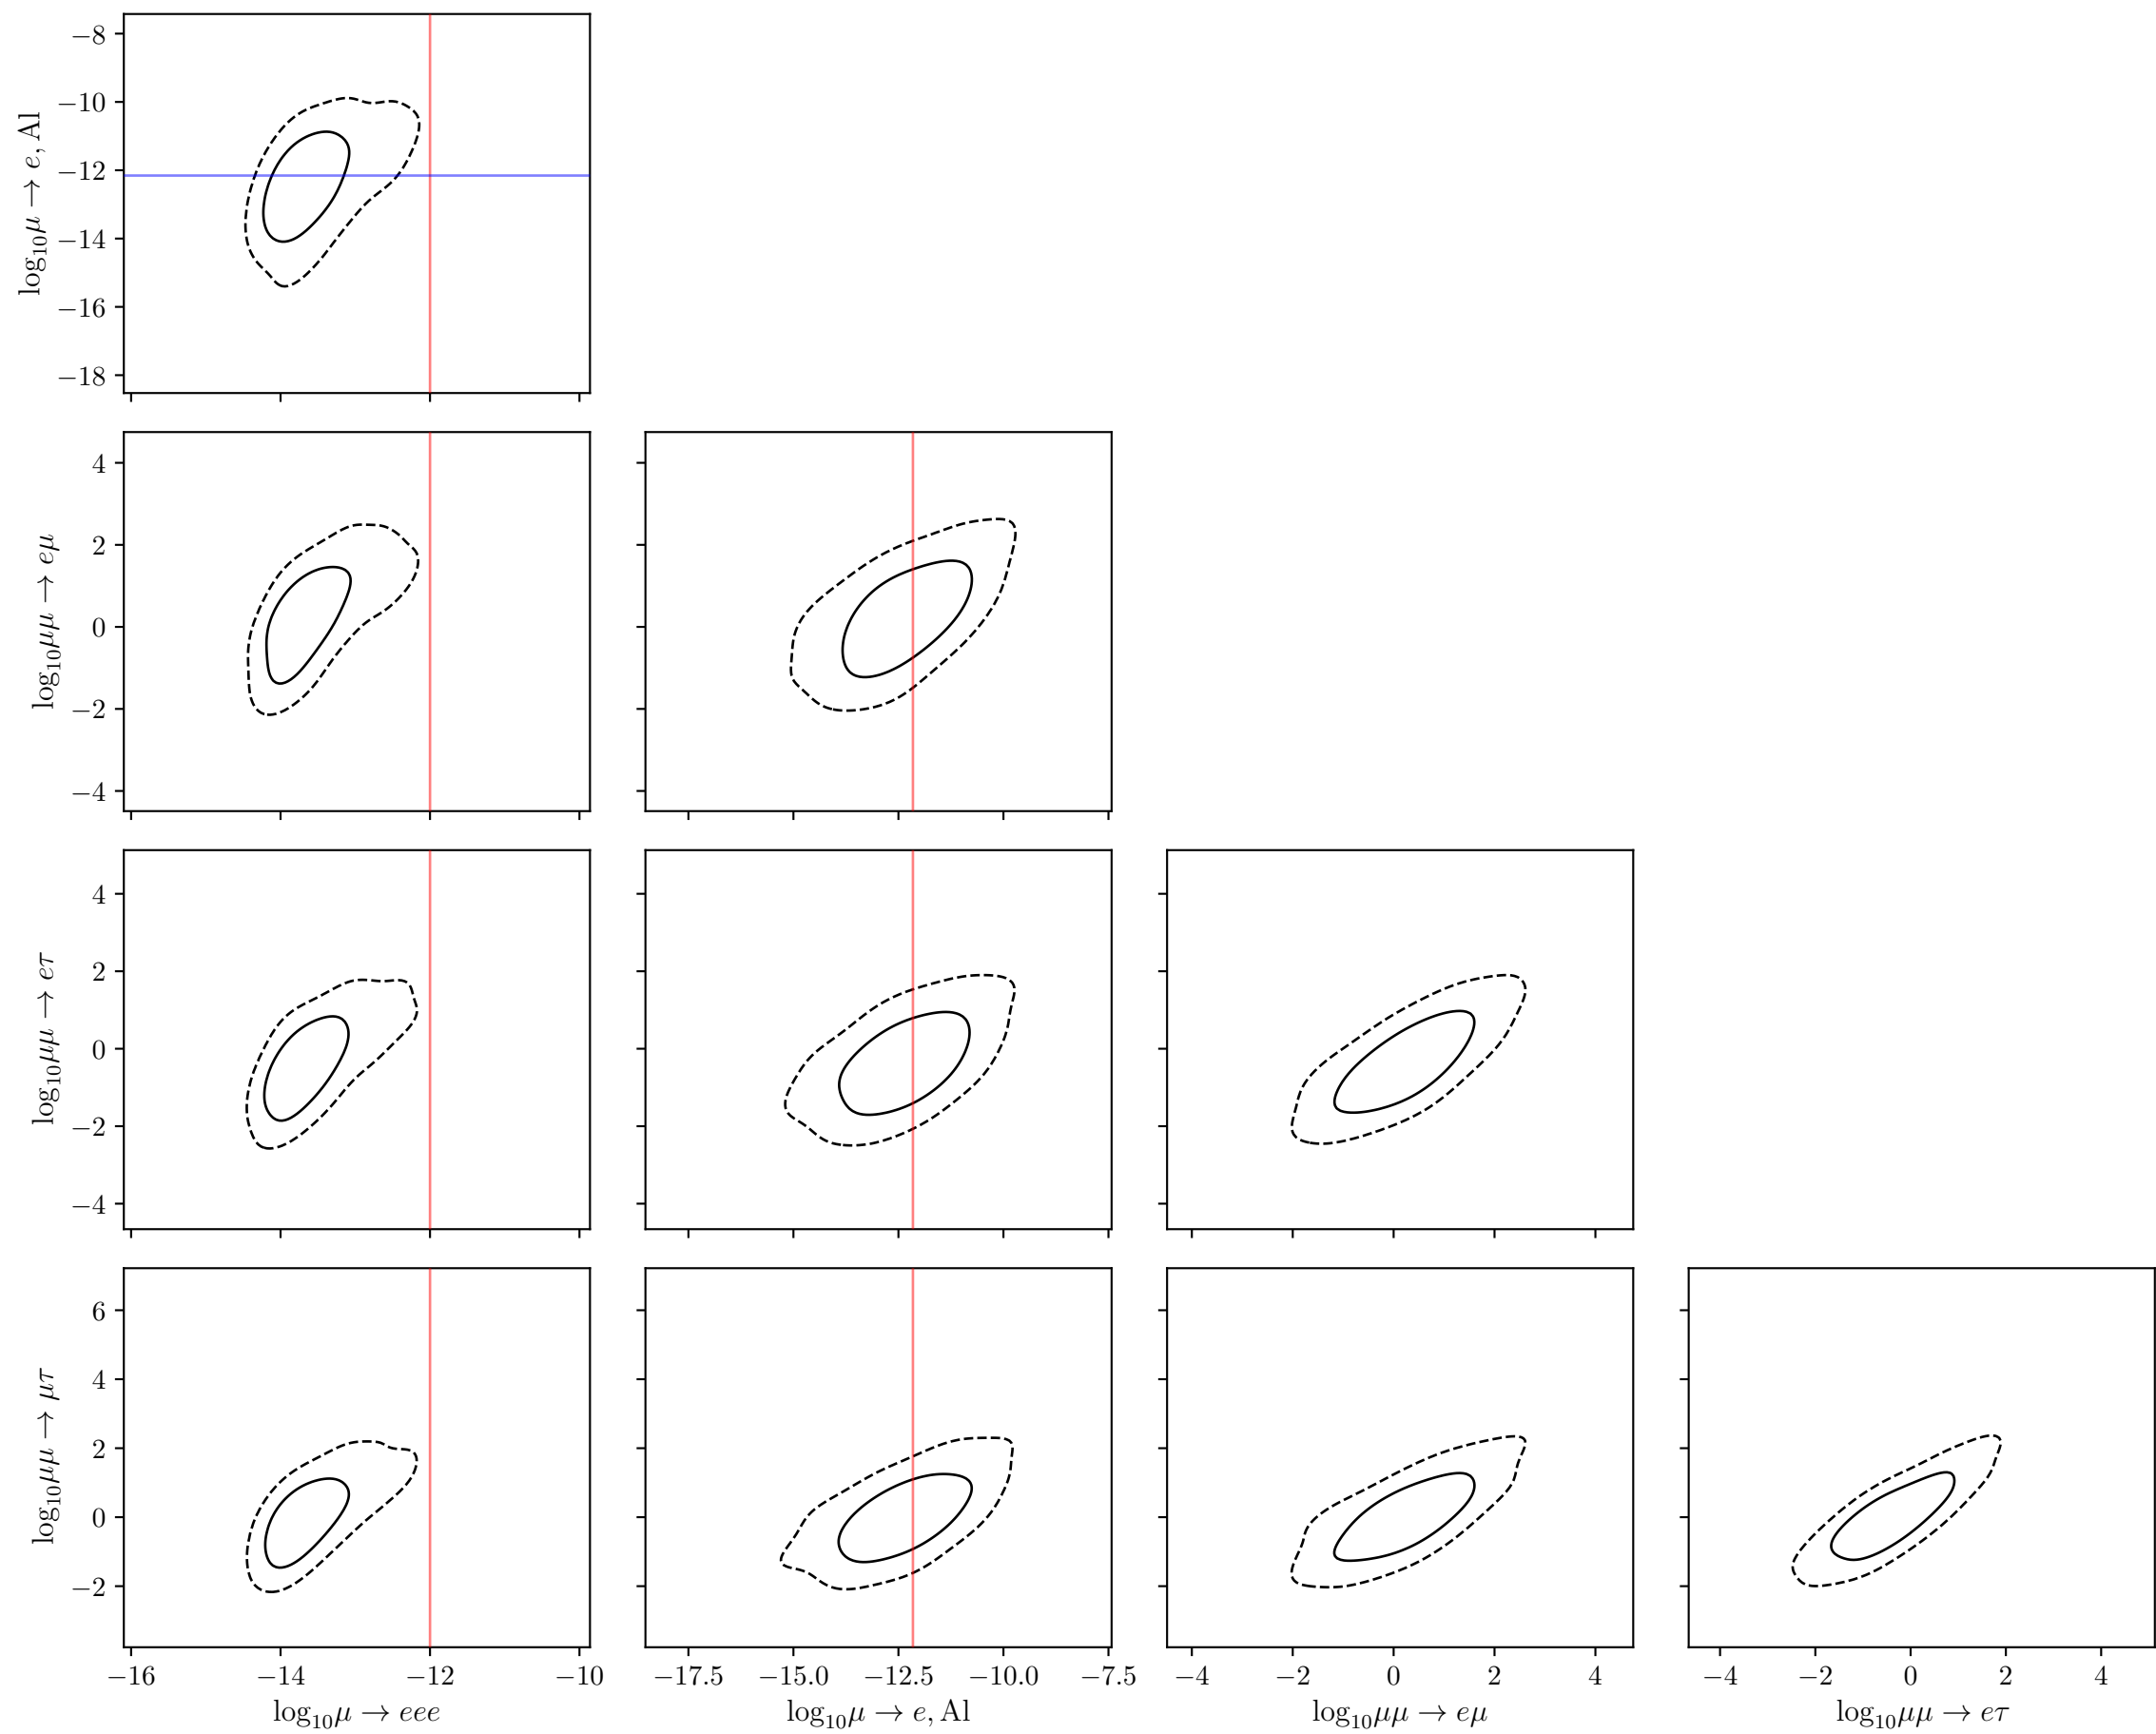

Majorana,  $X_L = \{4, 3, 2\}$ ,  $X_e = \{7, 4, 2\}$ ,

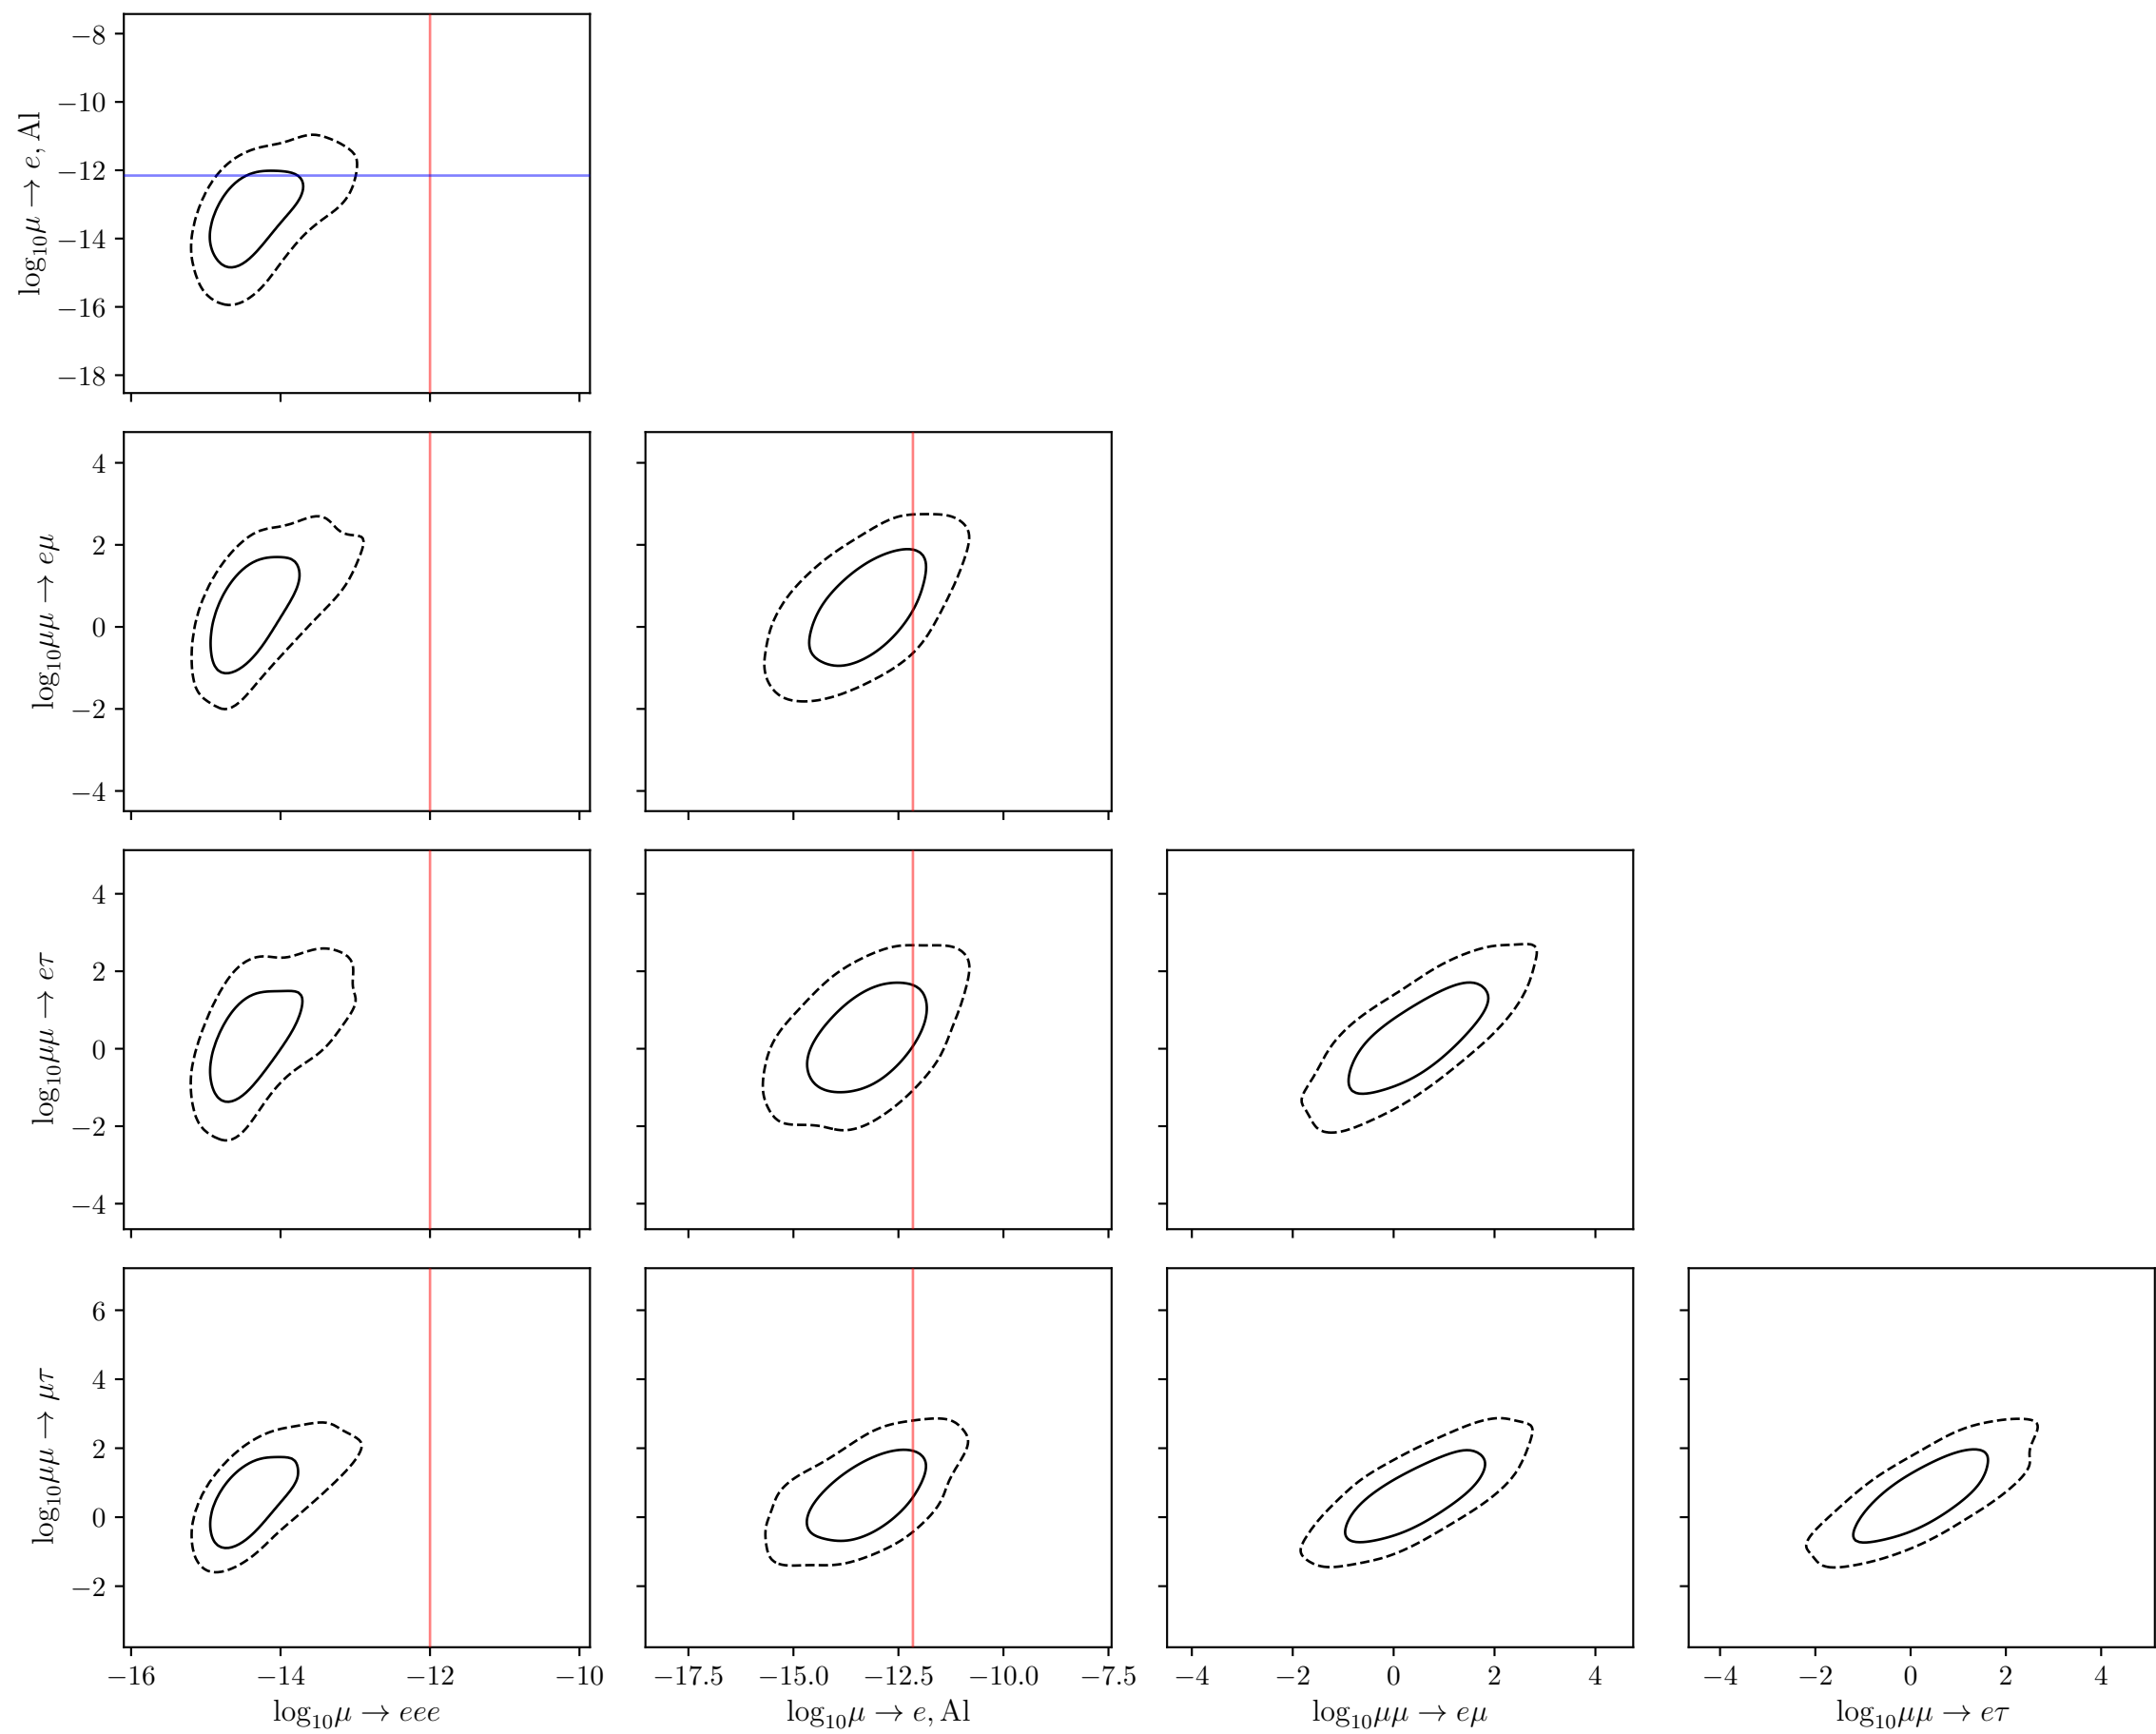

Majorana,  $X_L = \{7, 6, 5\}$ ,  $X_e = \{7, 3, 1\}$ ,

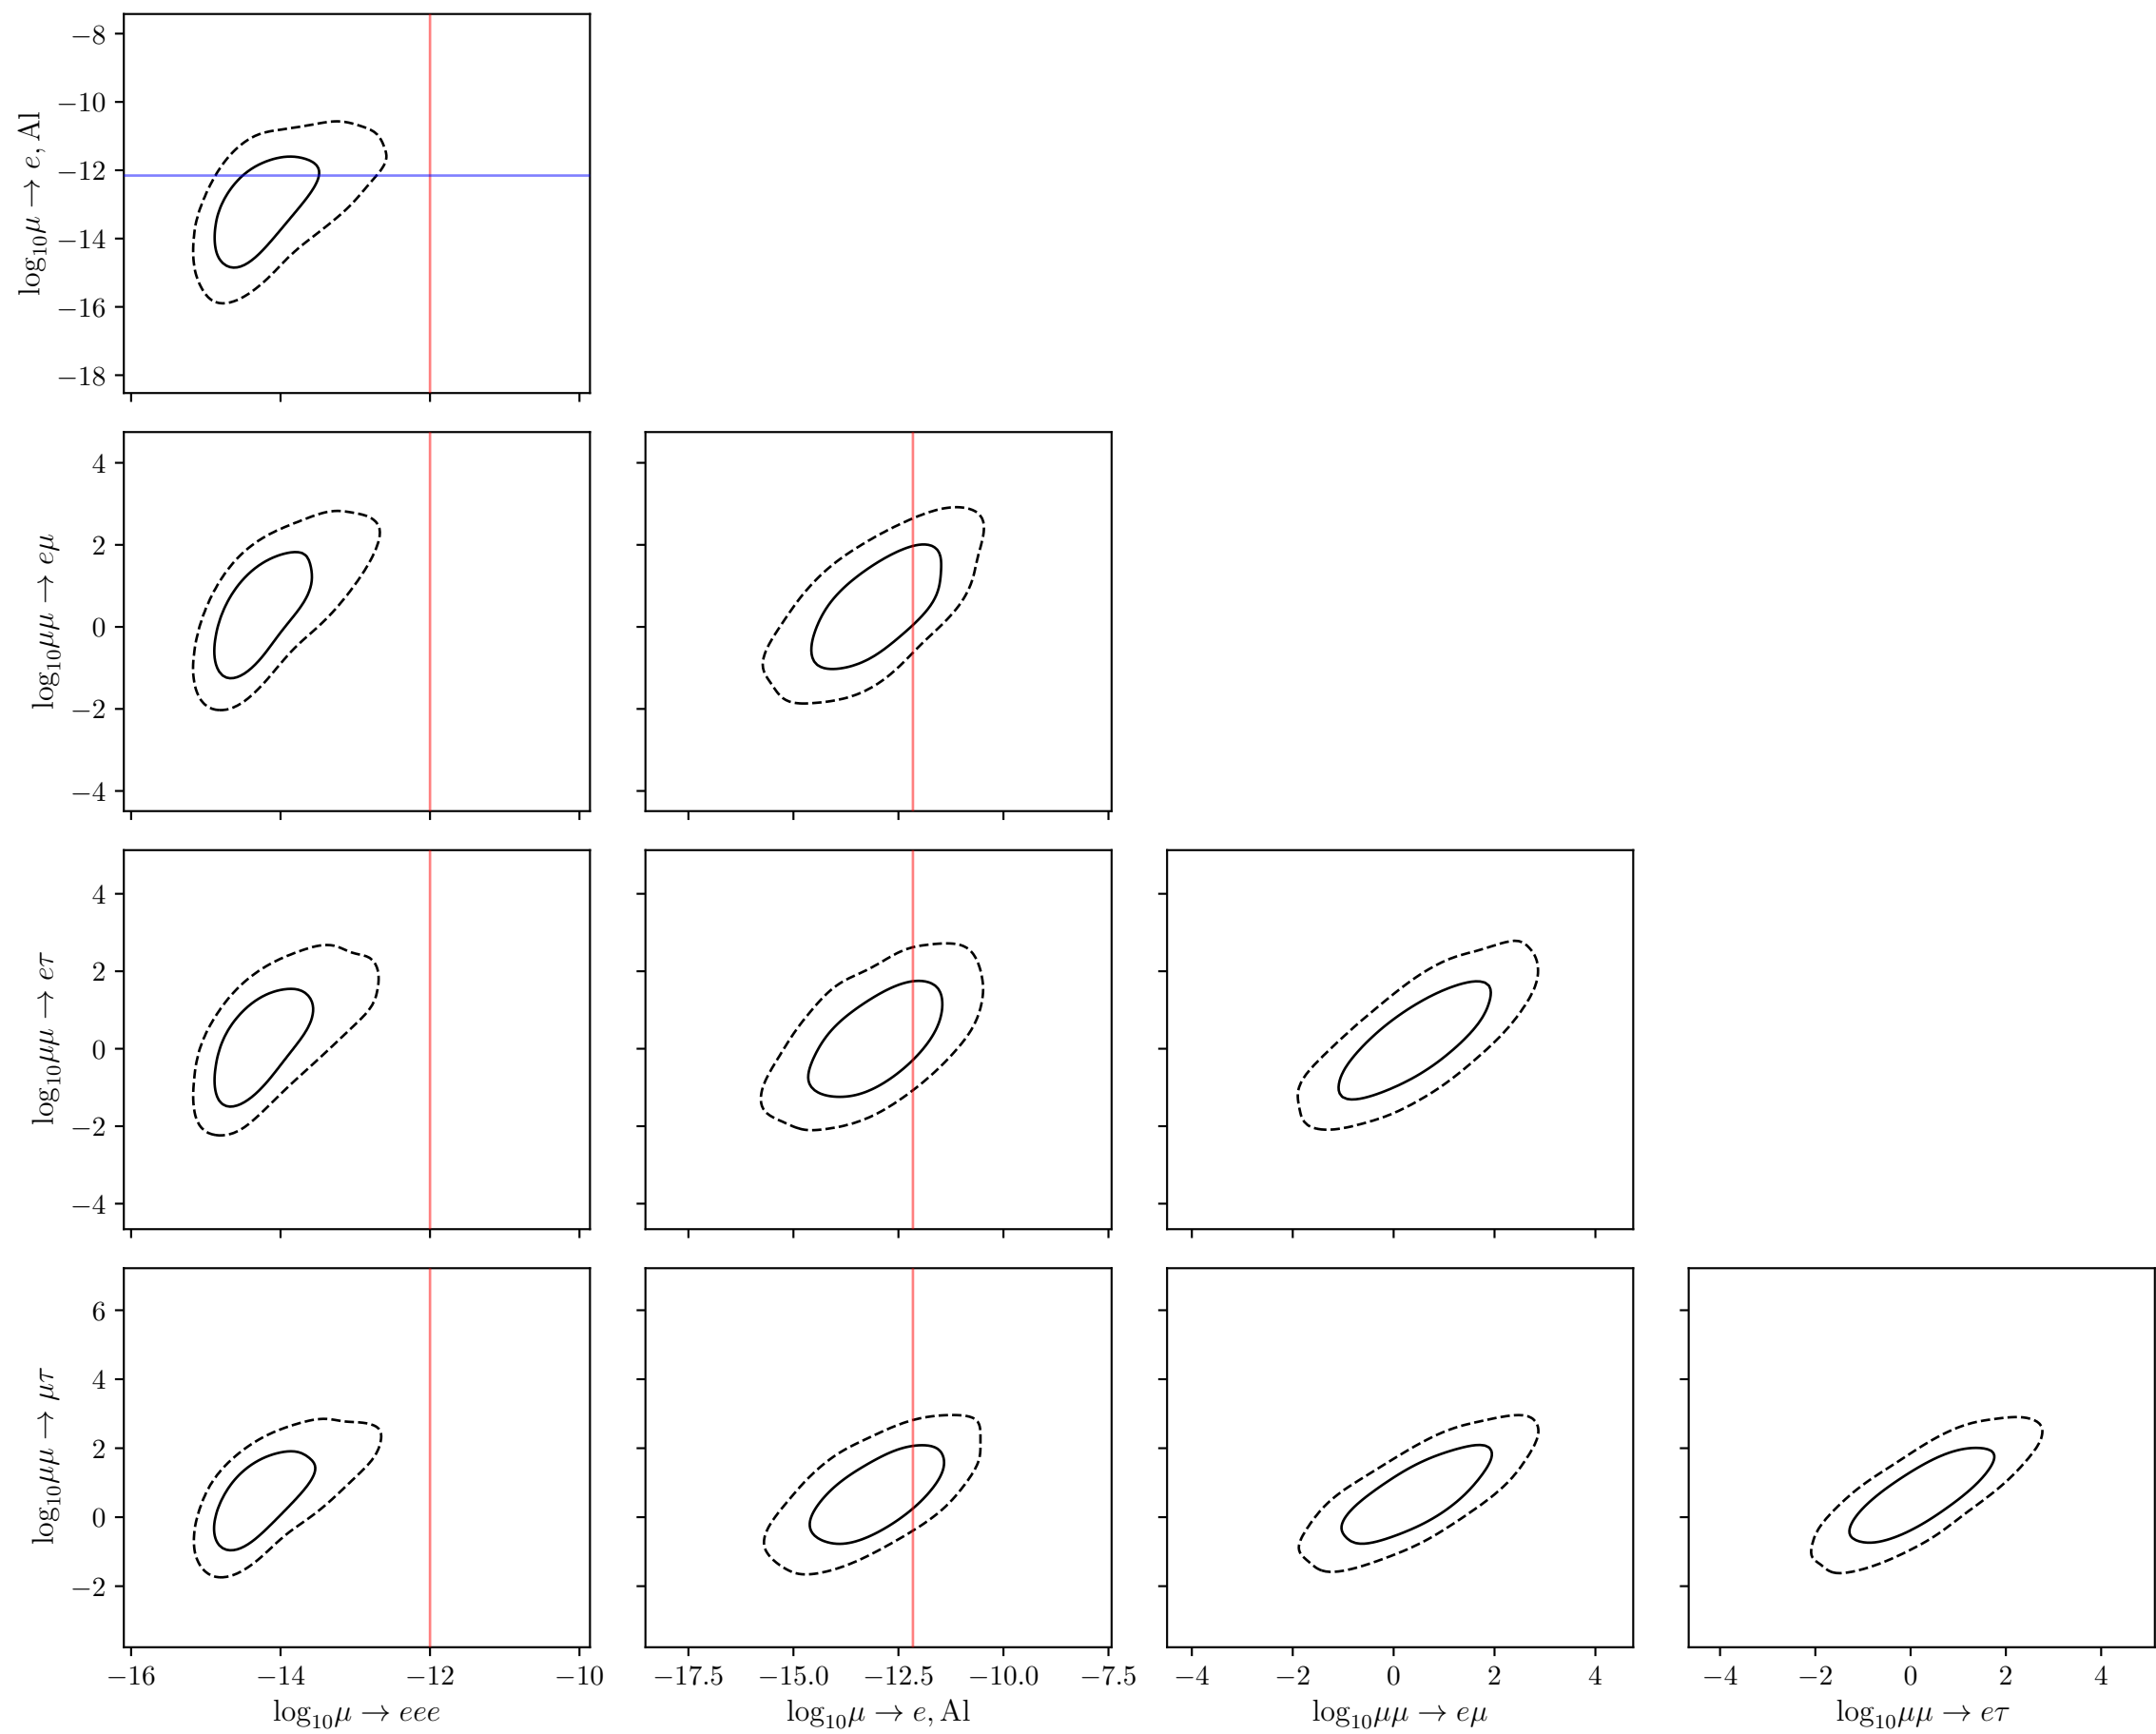

Majorana,  $X_L = \{6, 5, 4\}$ ,  $X_e = \{7, 2, 0\}$ ,

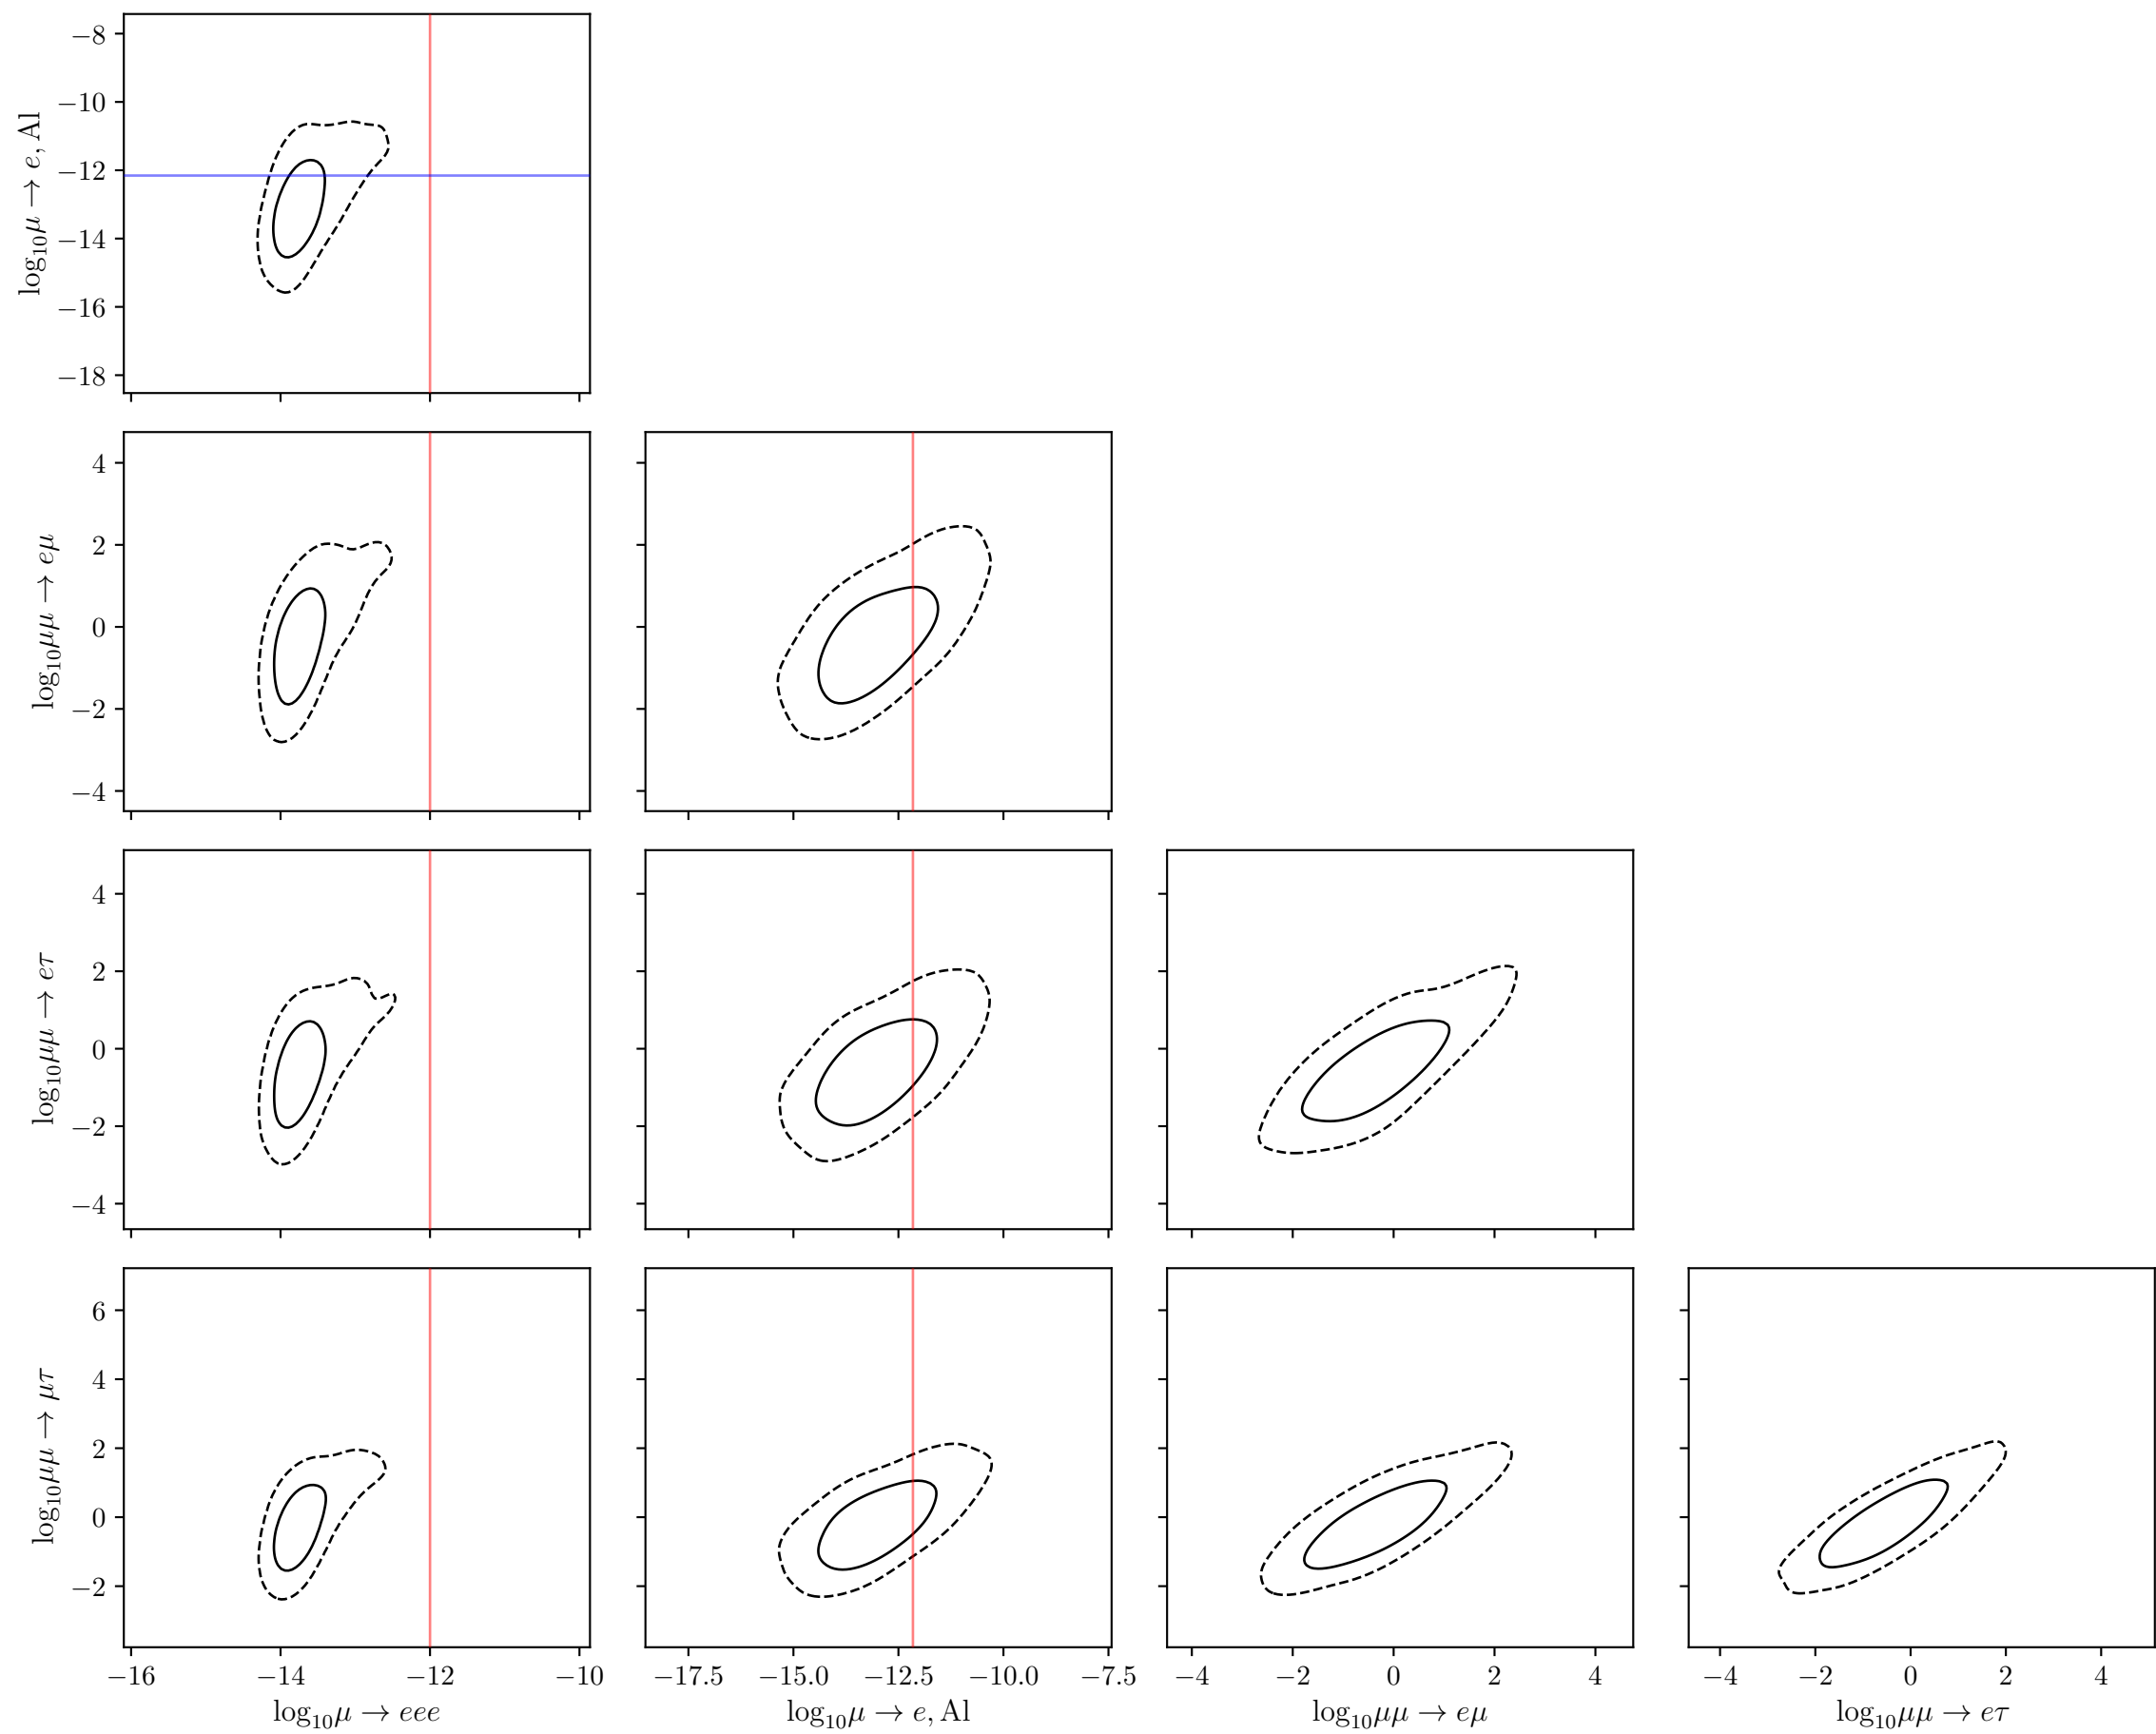



Majorana,  $X_L = \{2, 2, 1\}$ ,  $X_e = \{-7, 2, 6\}$ ,

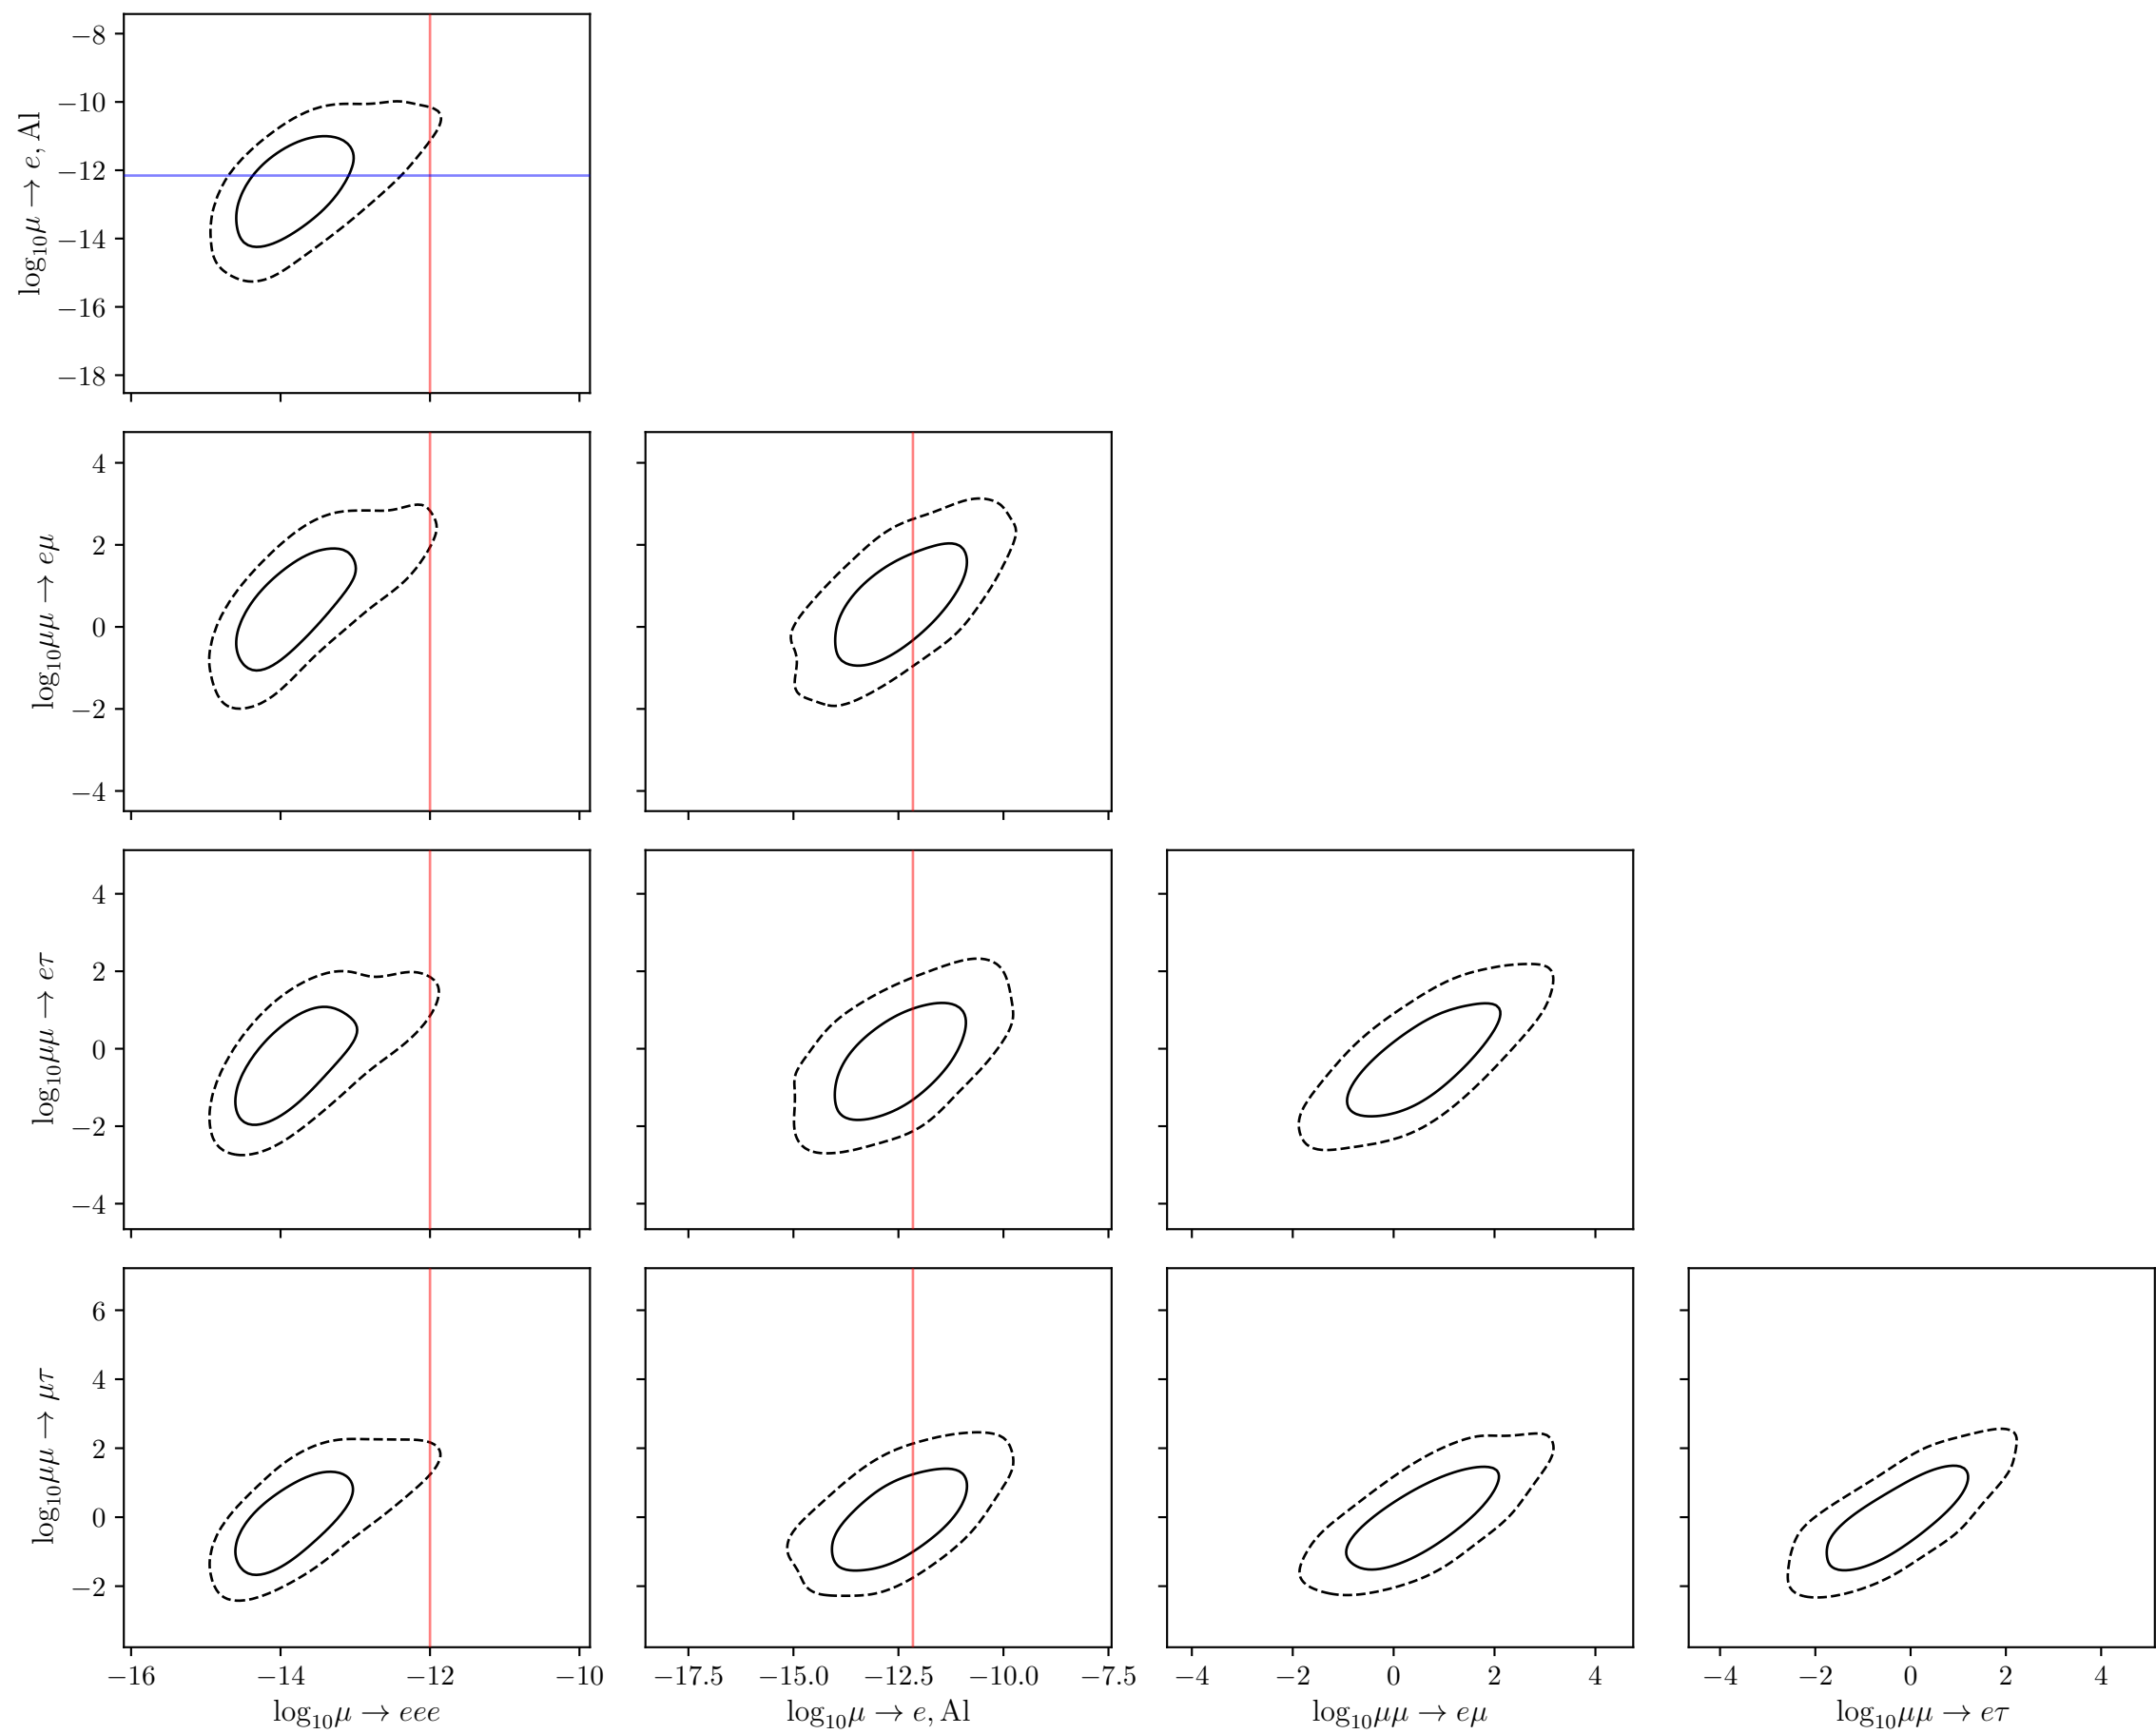

Majorana,  $X_L = \{7, 7, 6\}$ ,  $X_e = \{-2, 0, 5\}$ ,

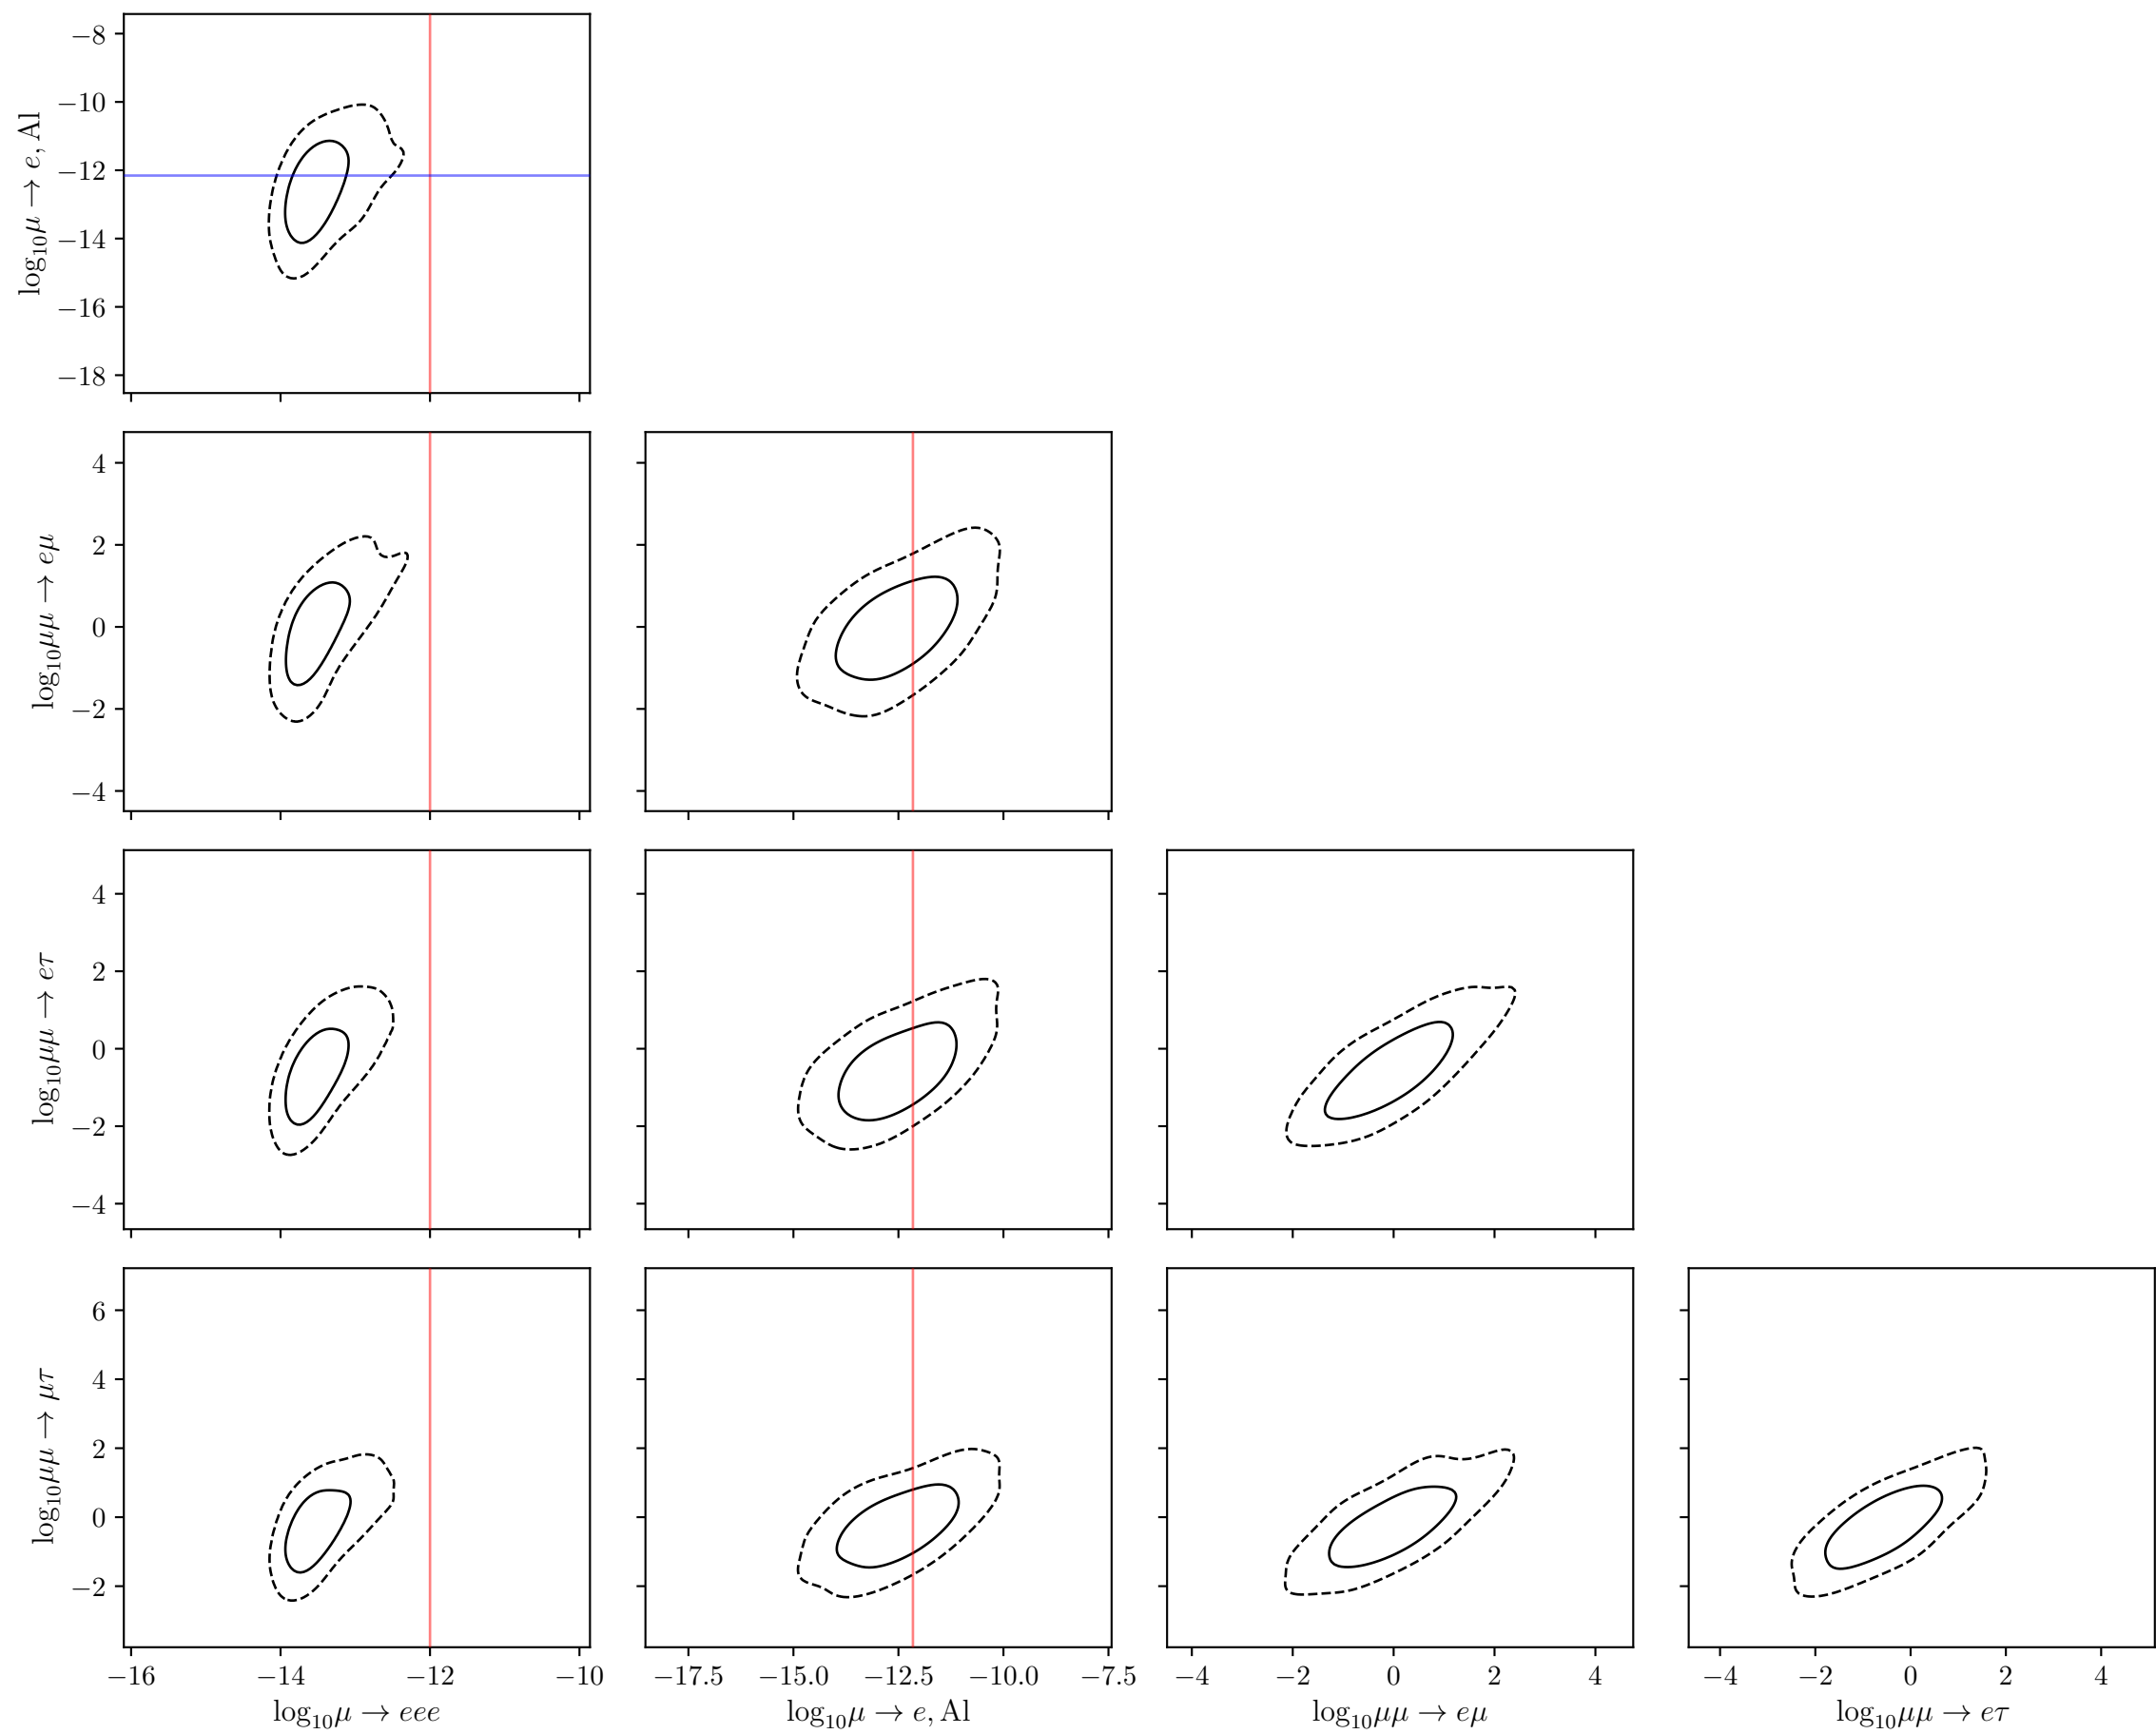

Majorana,  $X_L = \{7, 7, 6\}$ ,  $X_e = \{-2, -1, 3\}$ ,

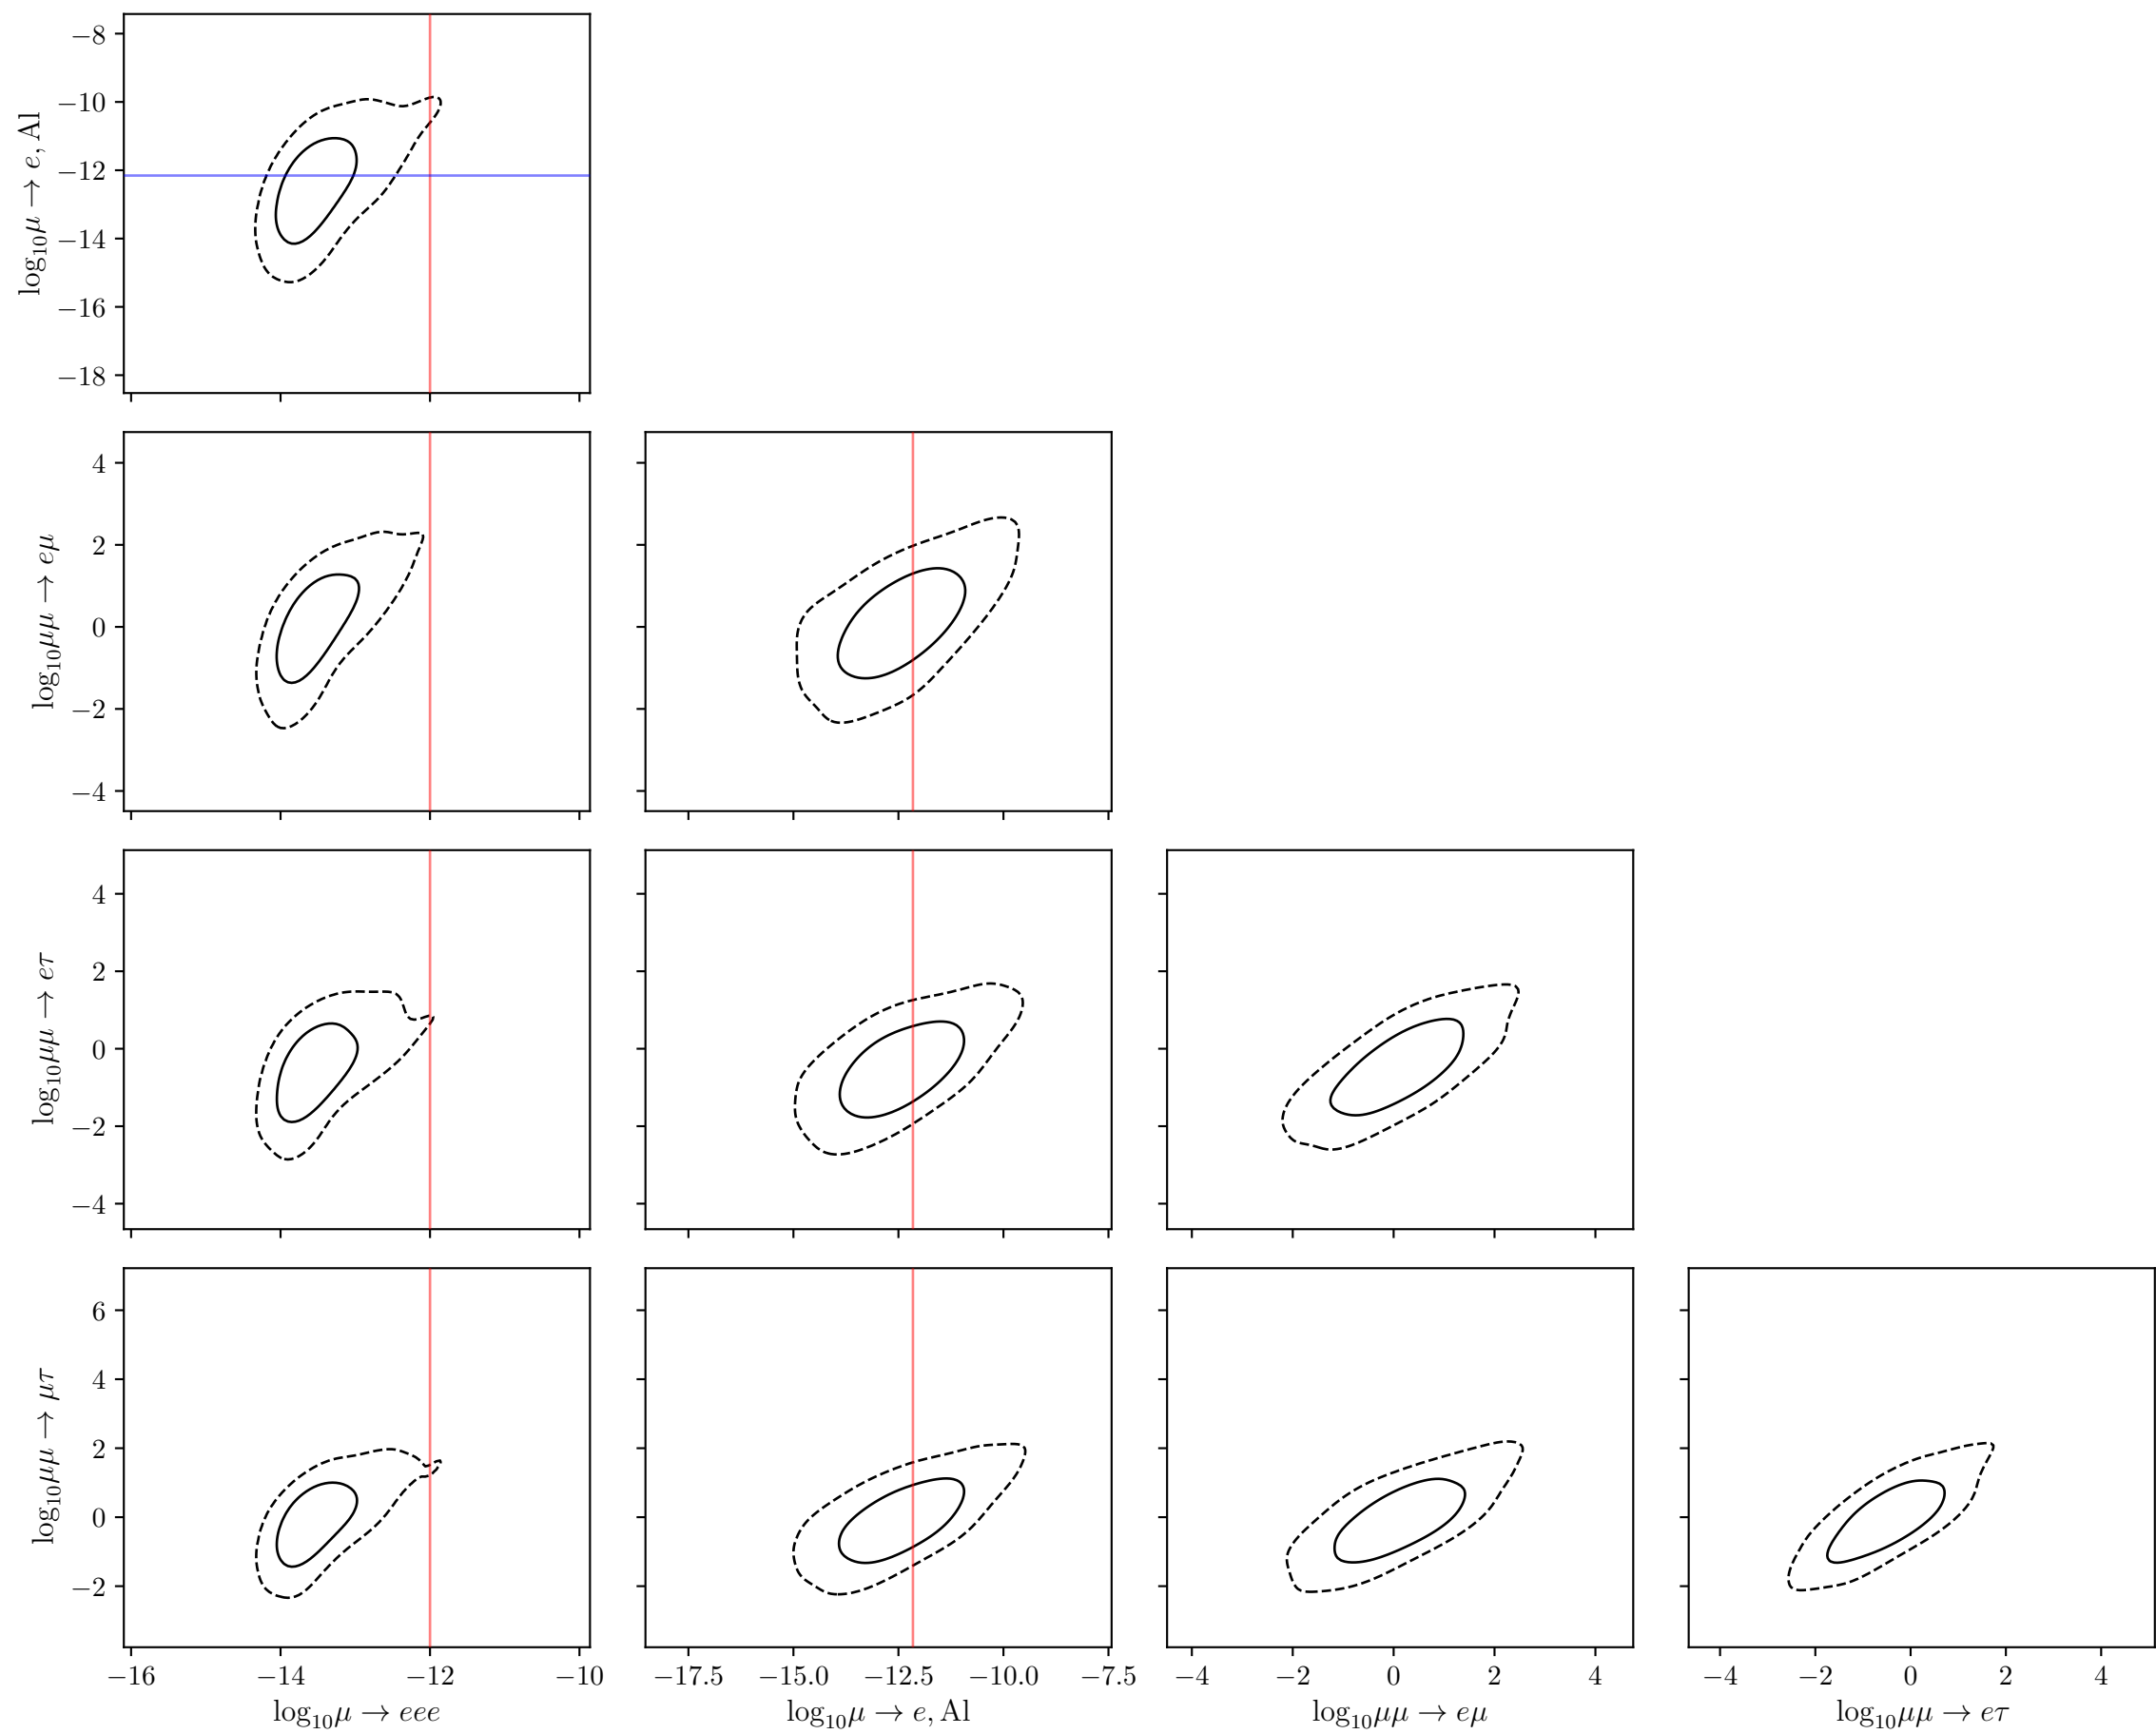

Majorana,  $X_L = \{3, 2, 1\}$ ,  $X_e = \{7, 4, 3\}$ ,

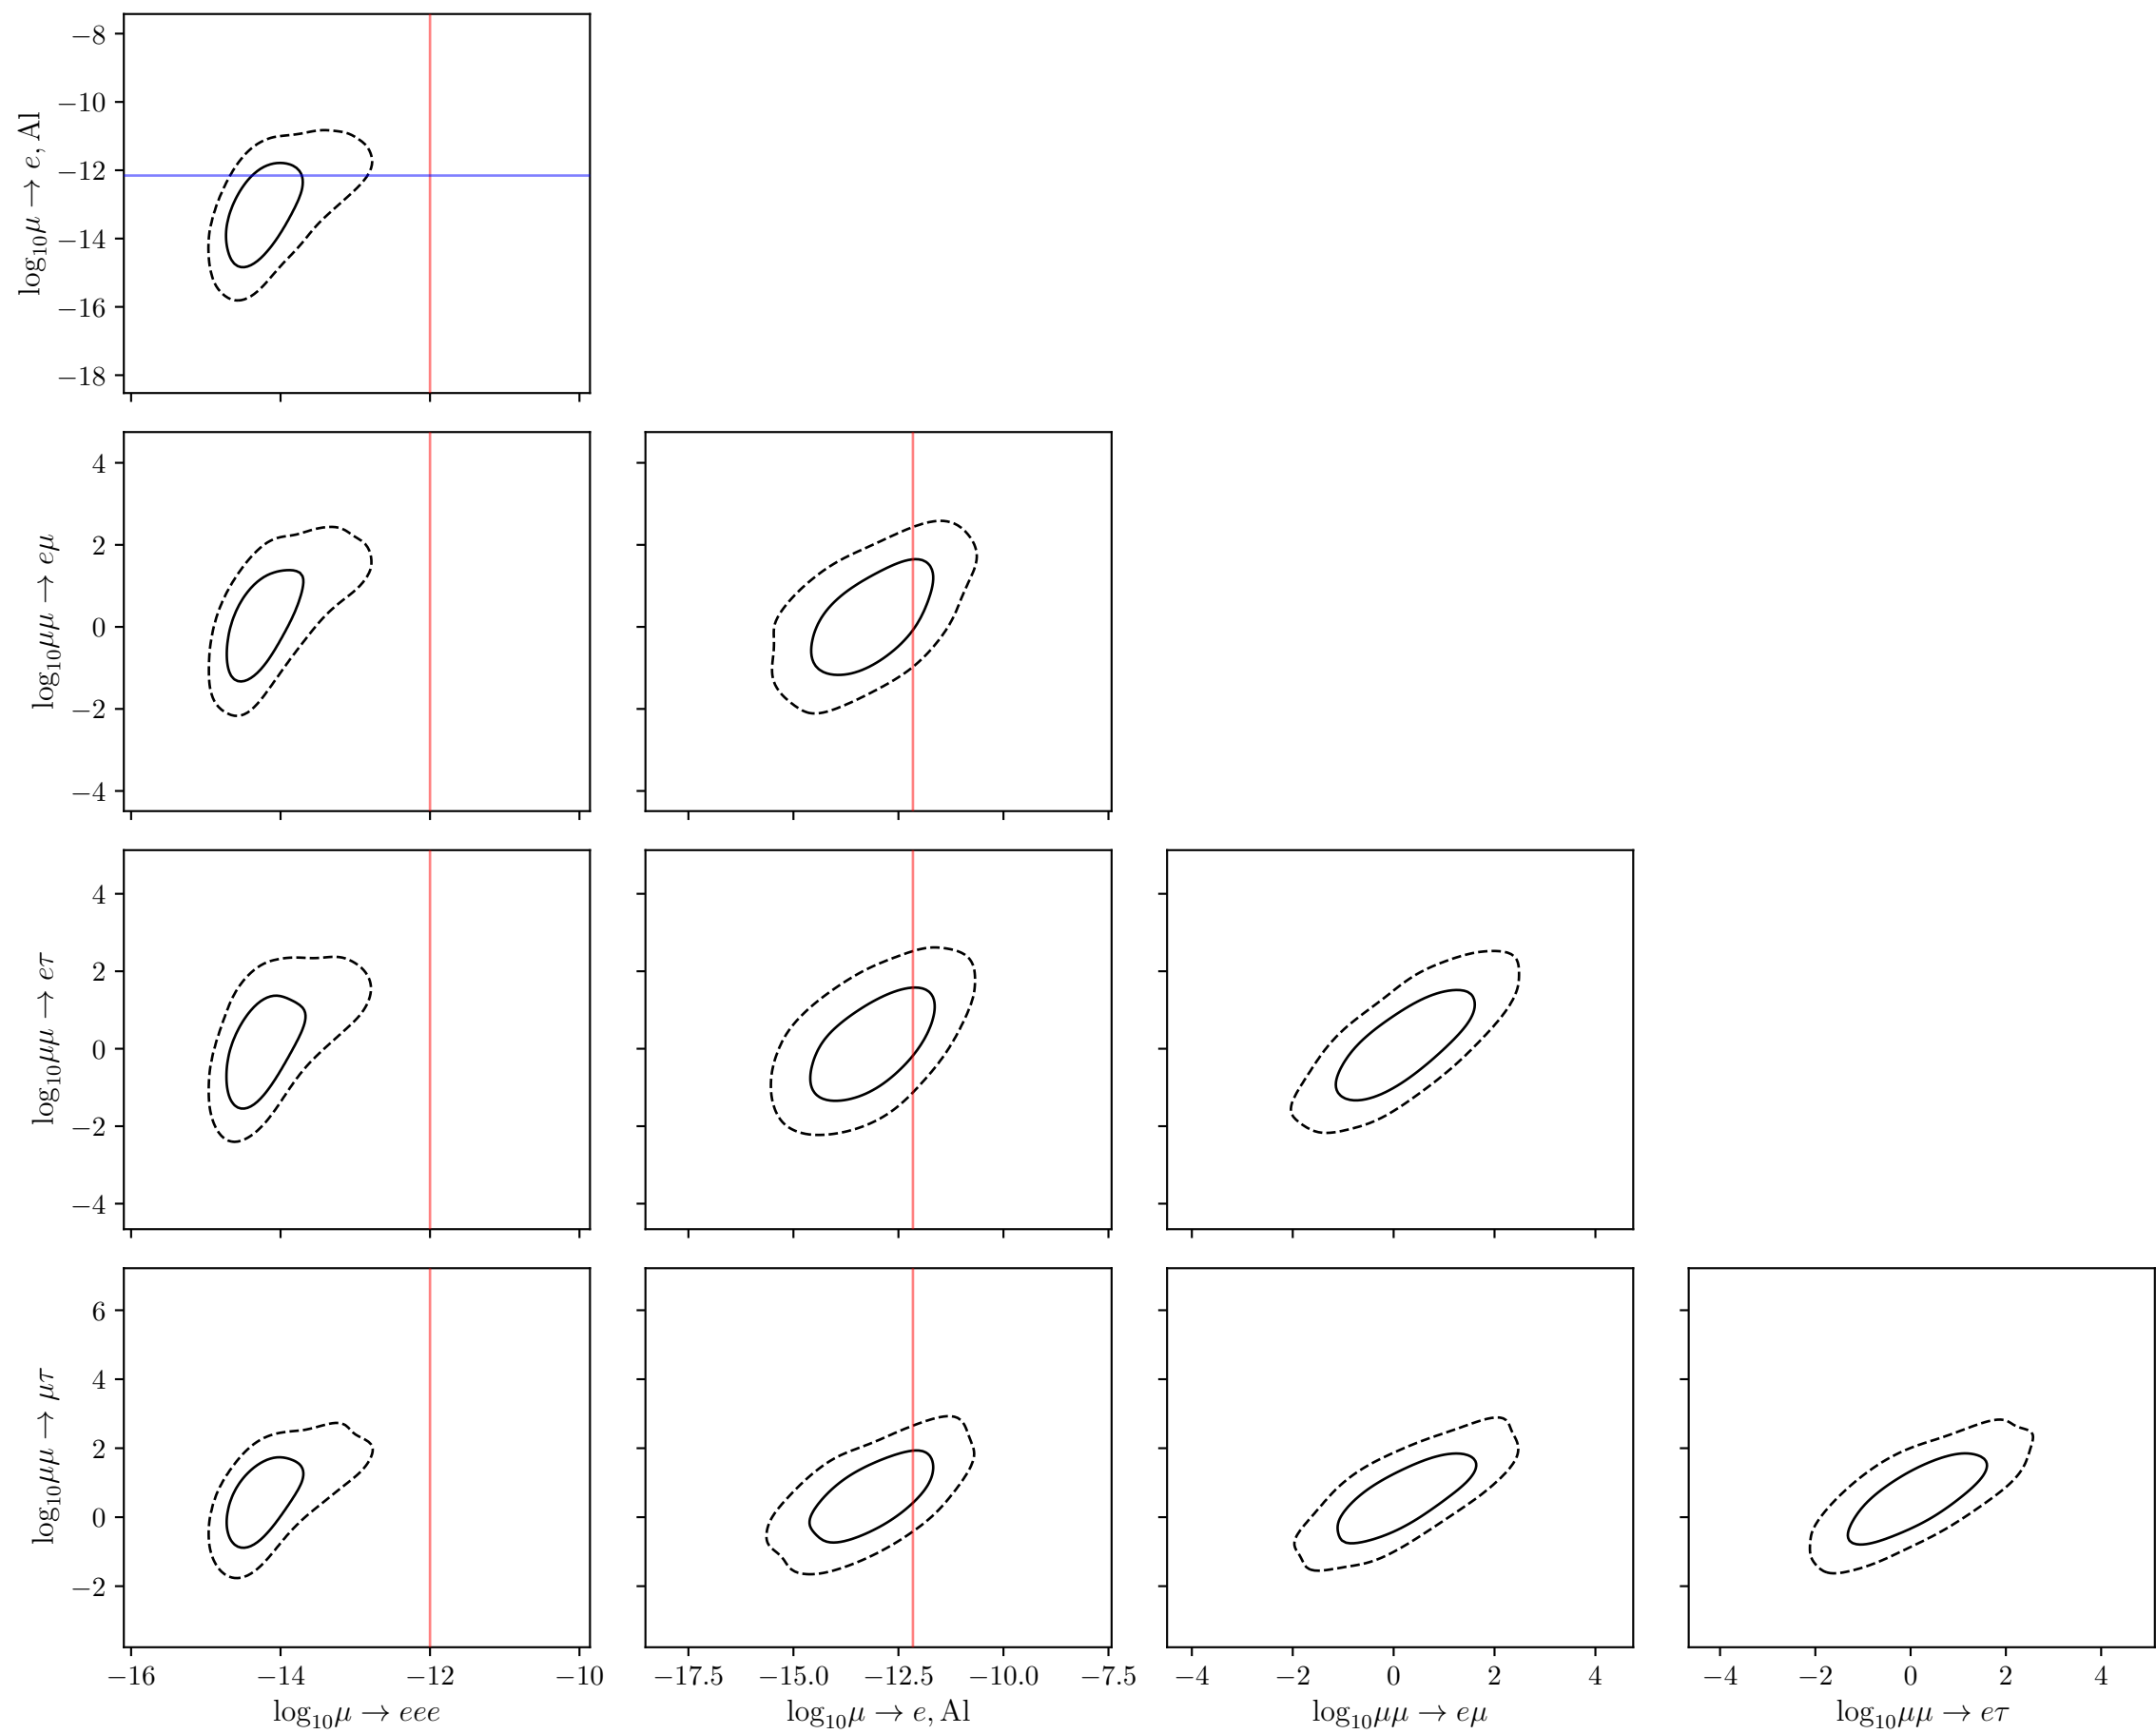

Majorana,  $X_L = \{6, 5, 4\}$ ,  $X_e = \{5, 1, 0\}$ ,

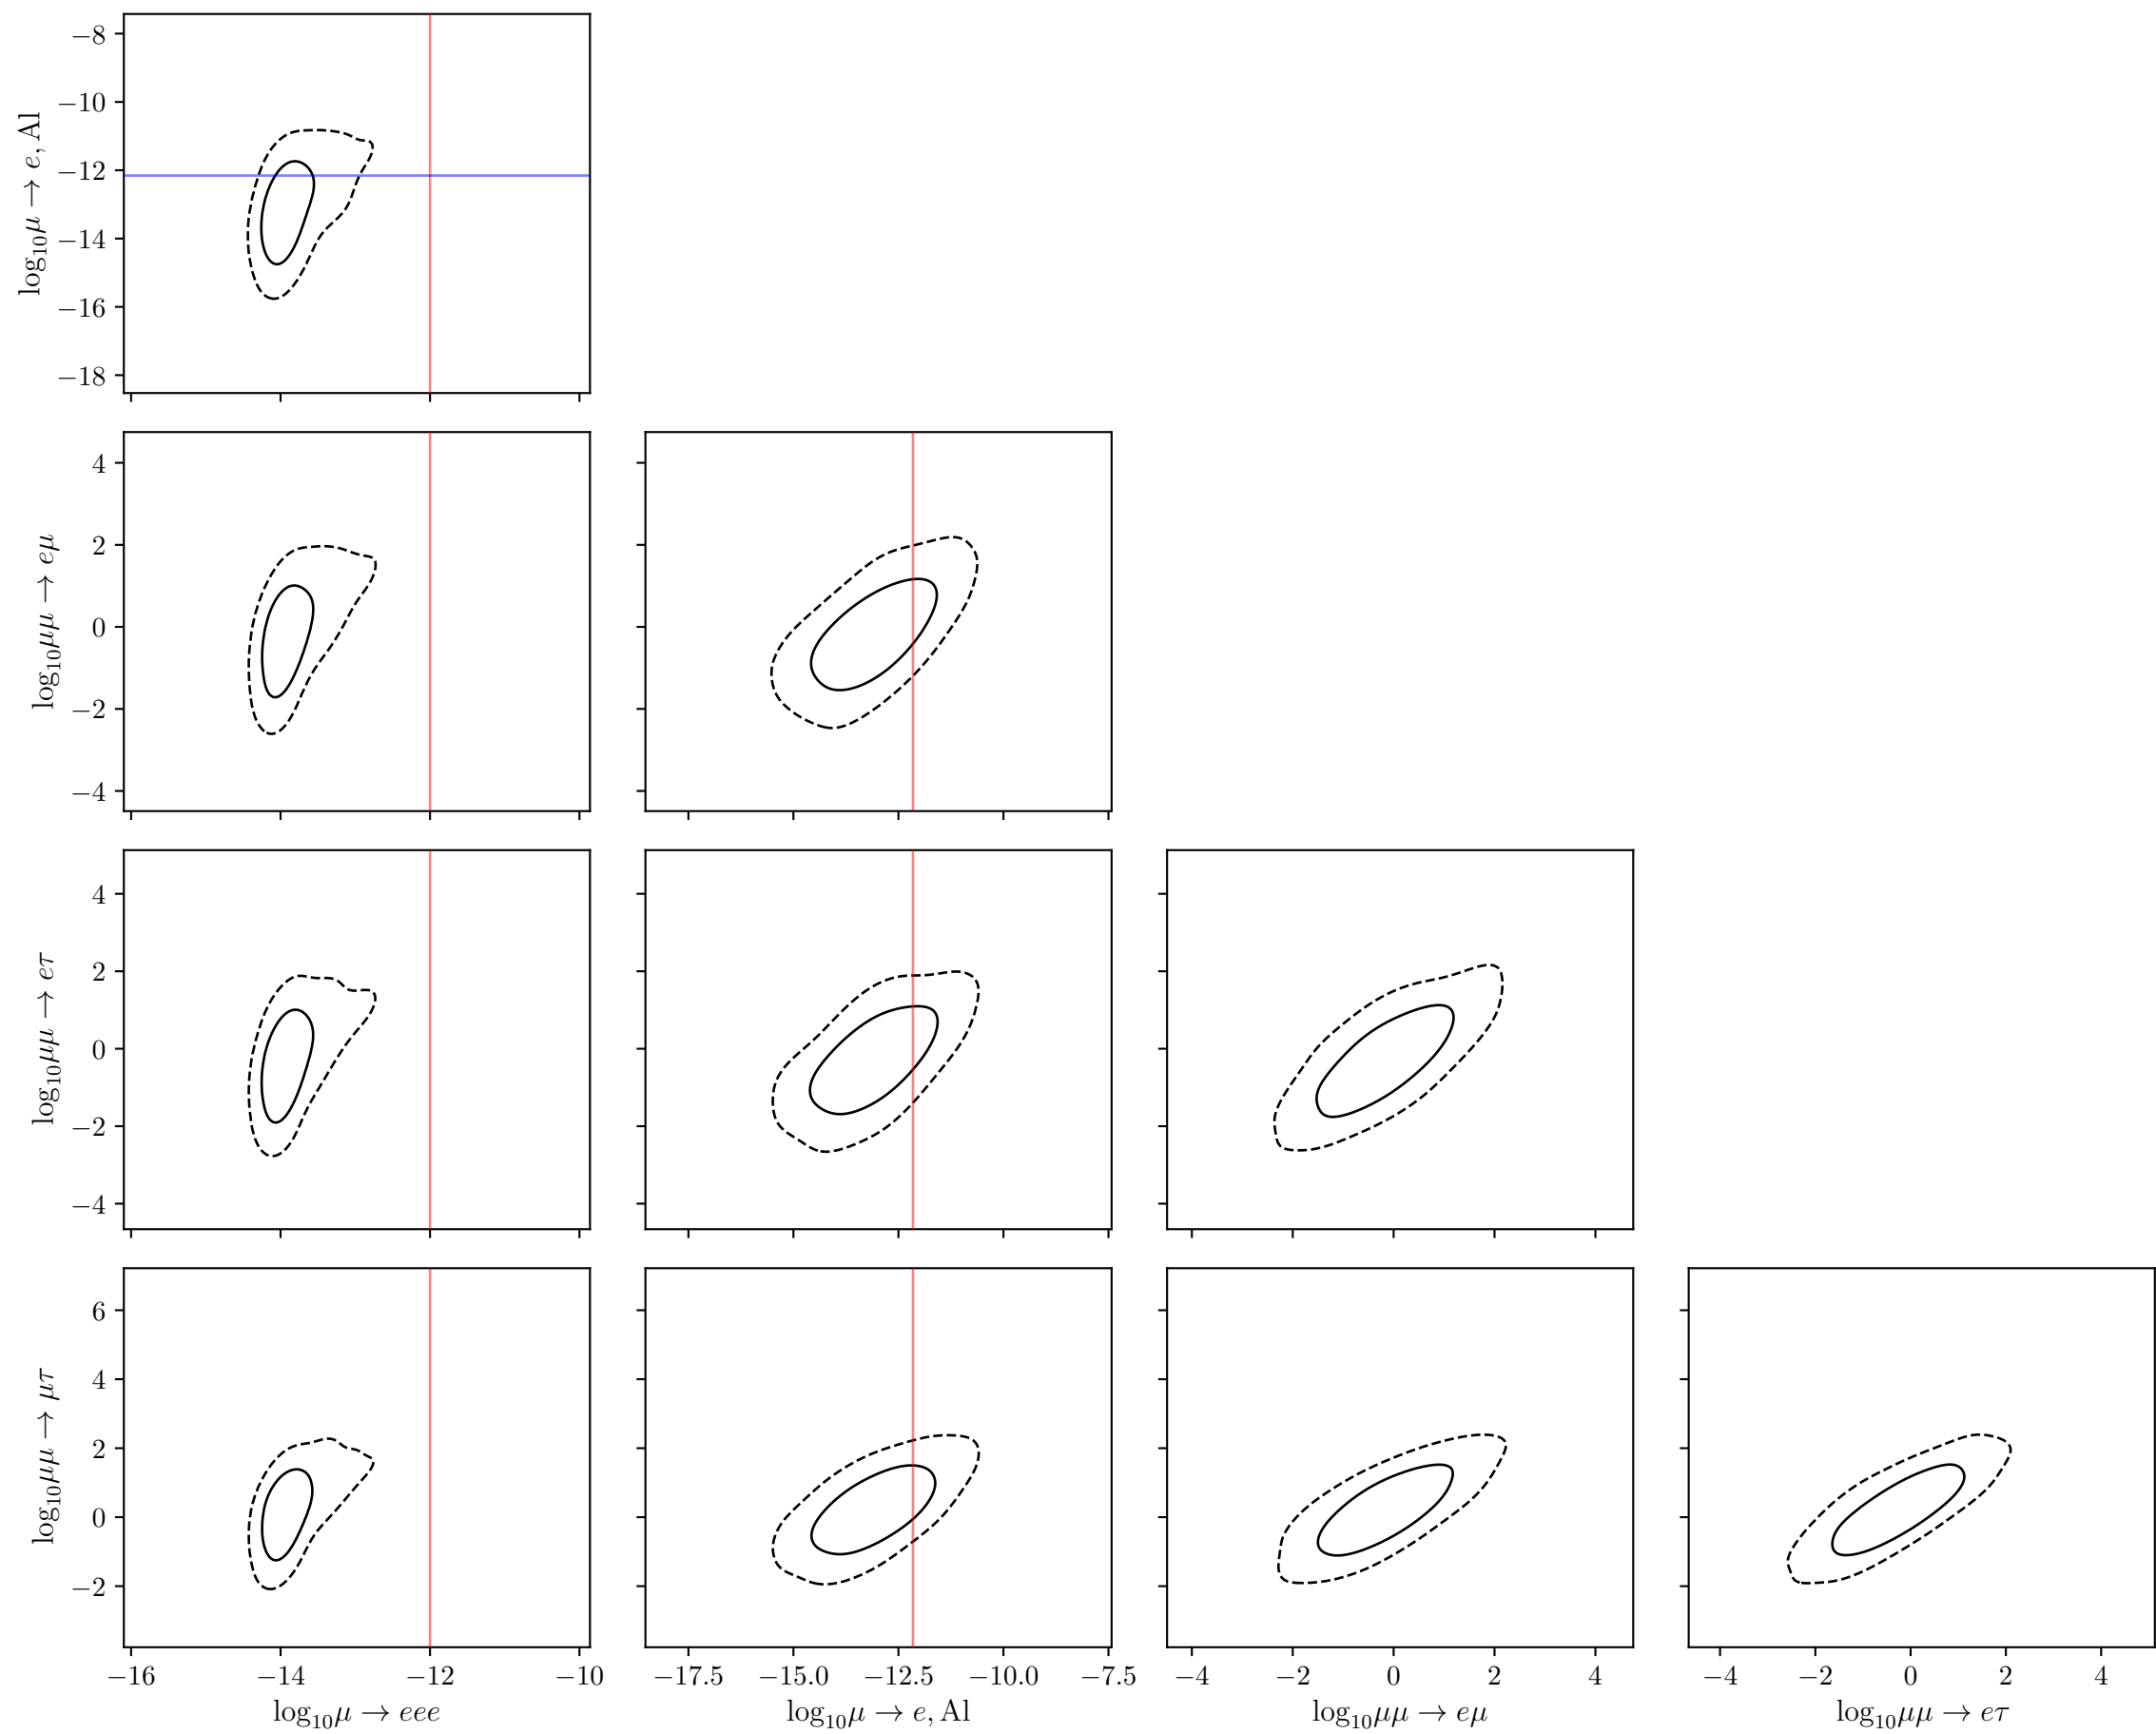

Majorana,  $X_L = \{6, 5, 4\}$ ,  $X_e = \{6, 3, 1\}$ ,

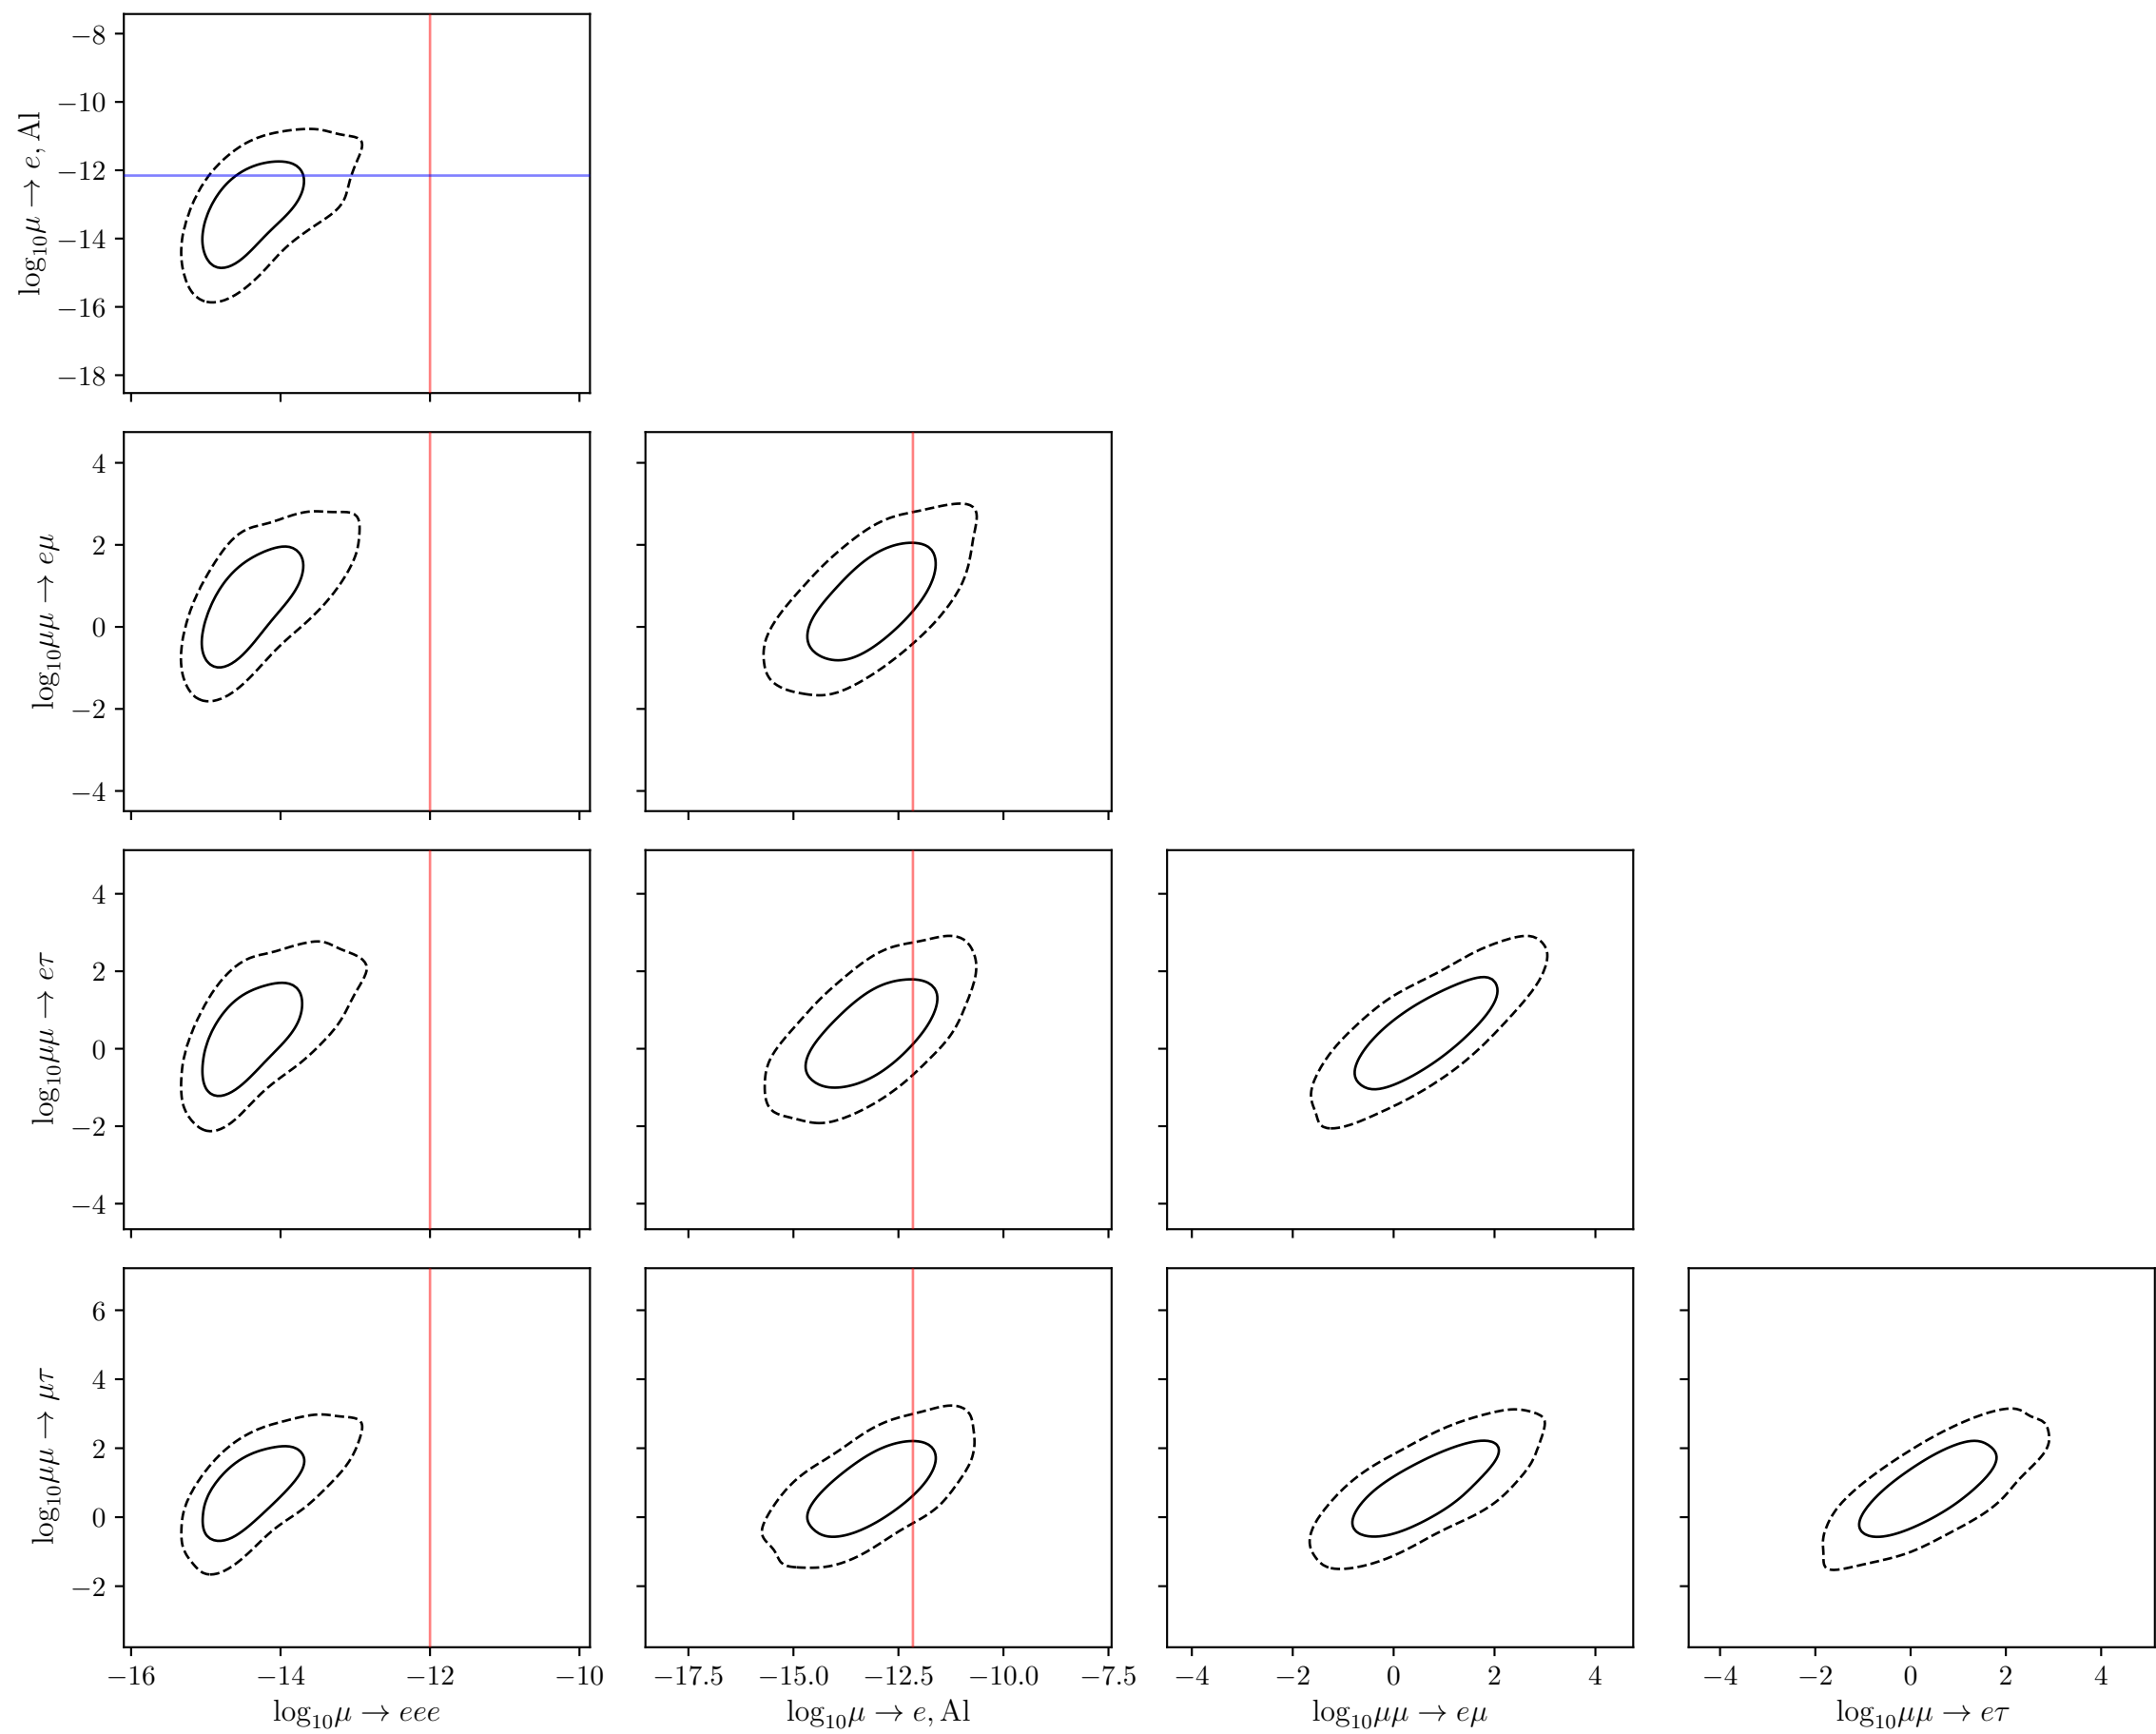

Majorana,  $X_L = \{7, 6, 5\}$ ,  $X_e = \{-1, 0, 4\}$ ,

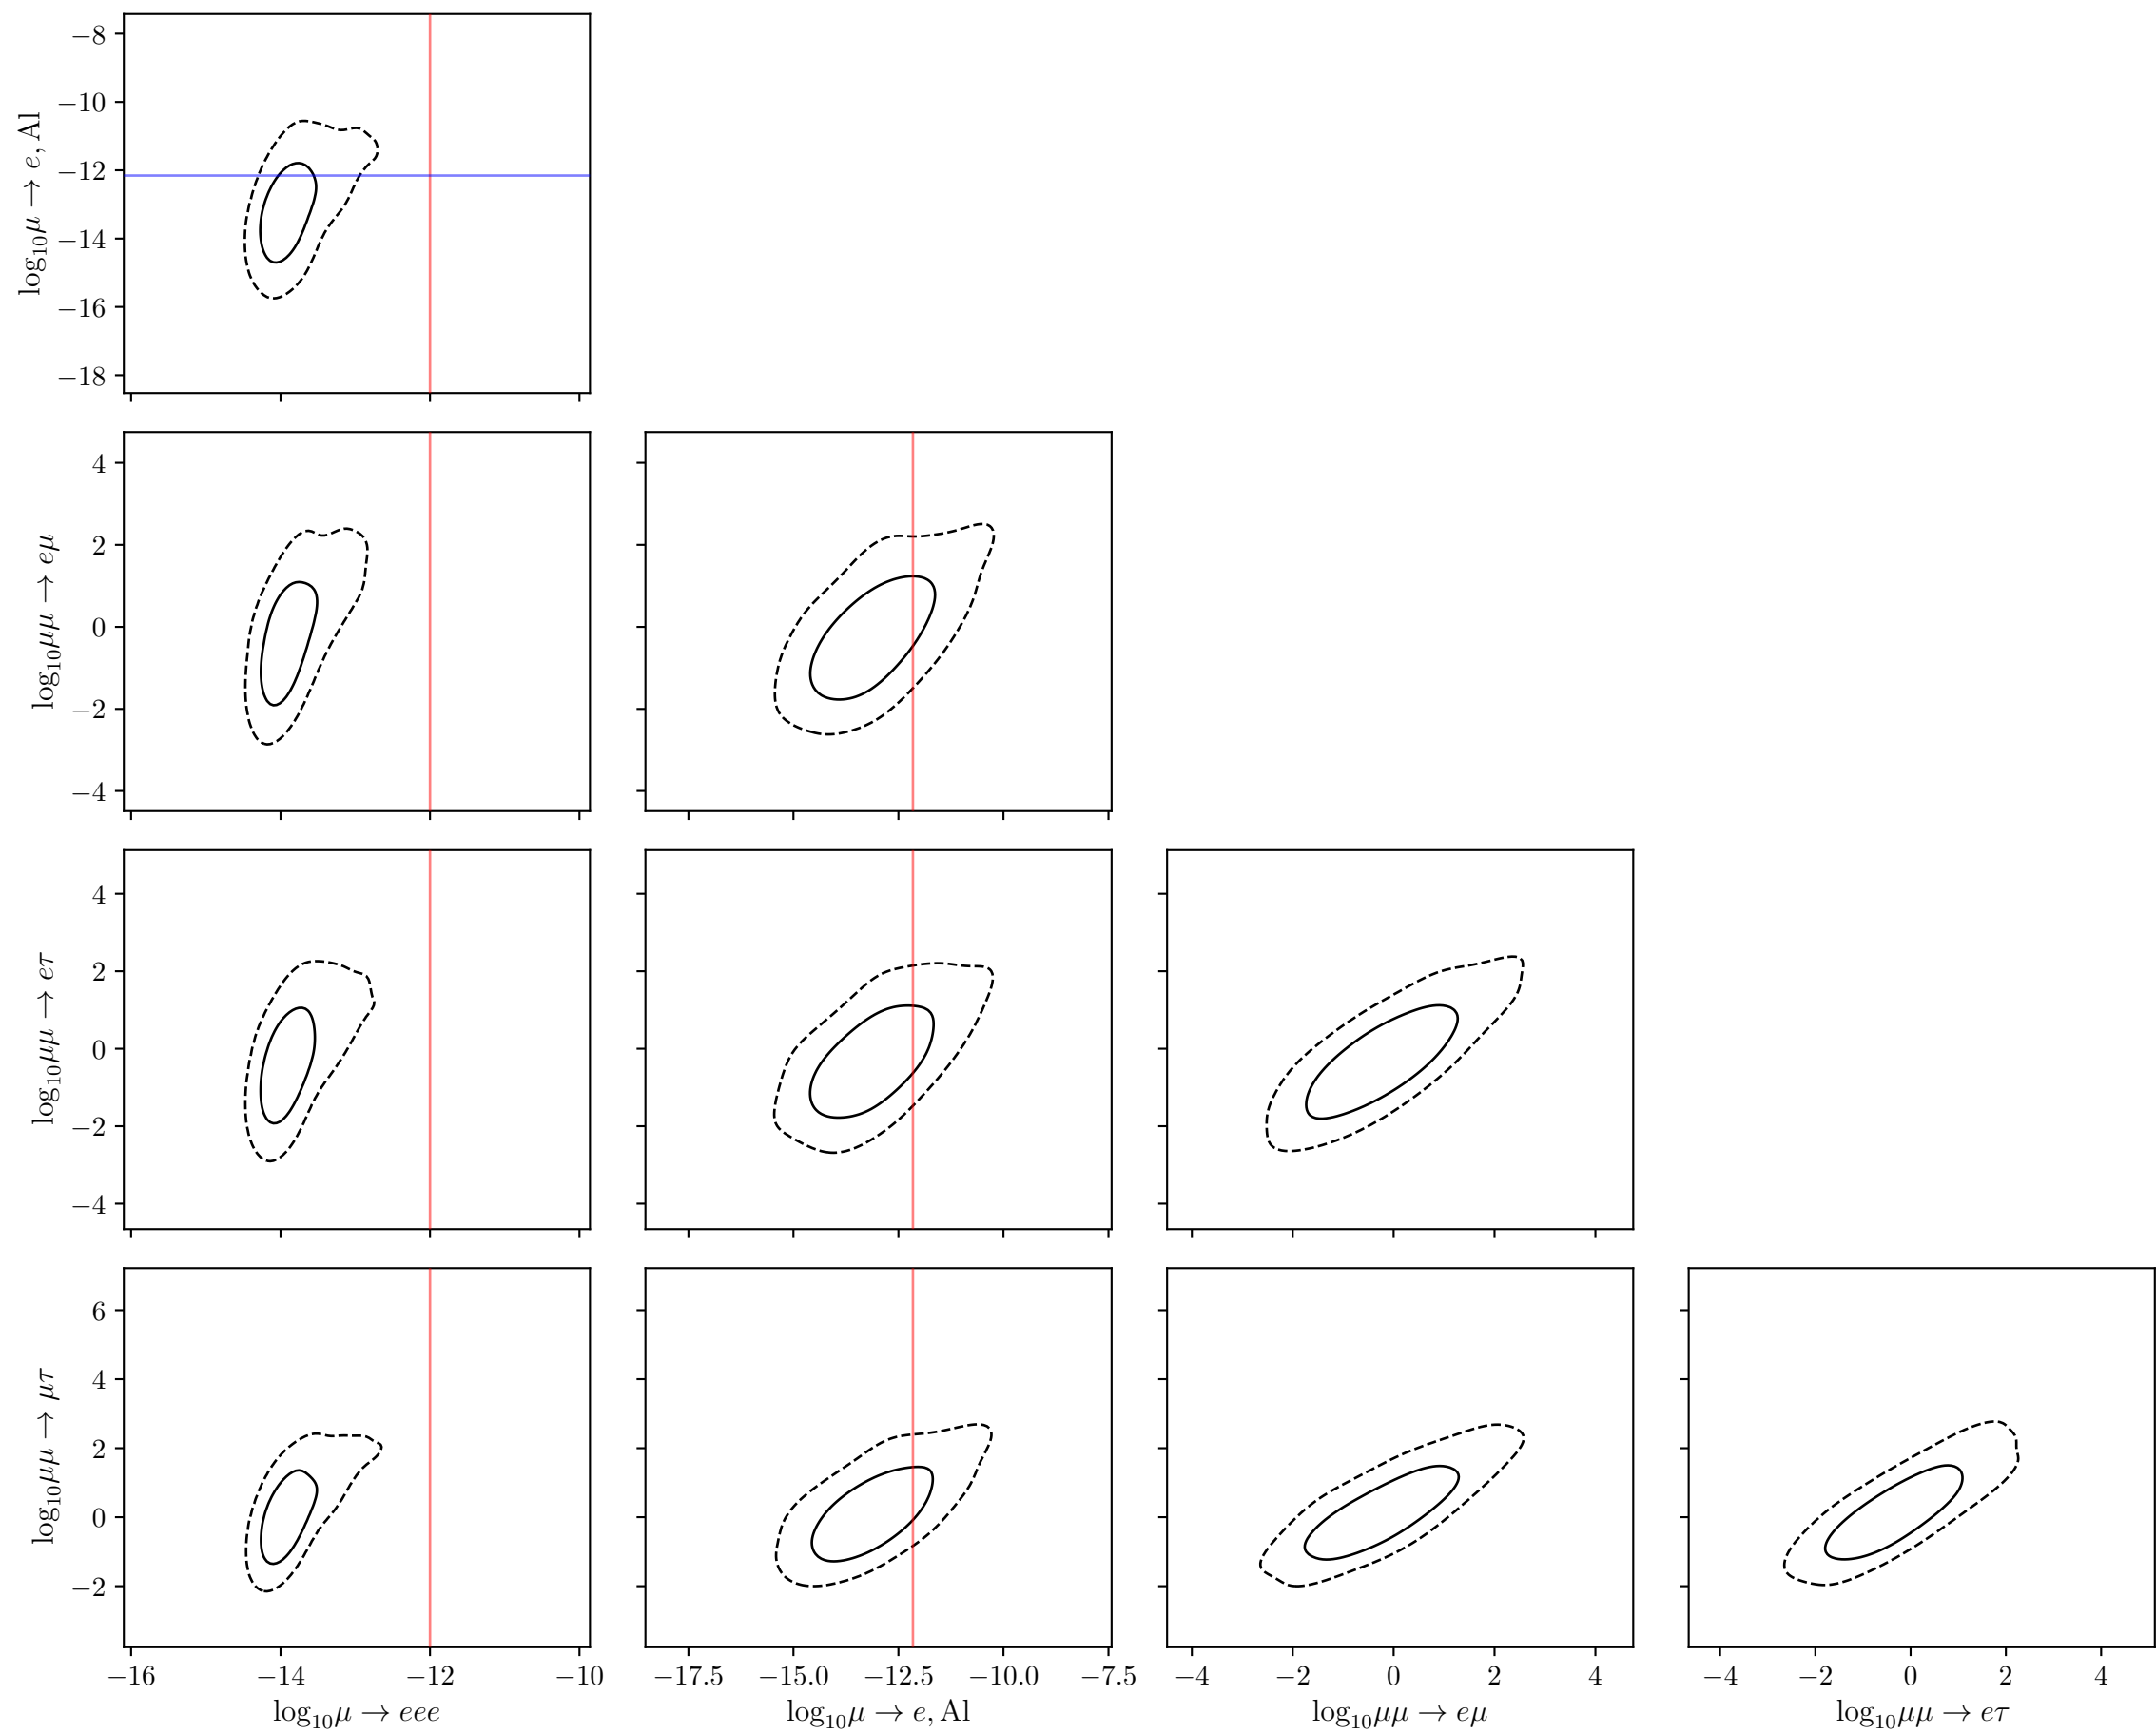

Majorana,  $X_L = \{4, 4, 3\}$ ,  $X_e = \{6, 2, 1\}$ ,

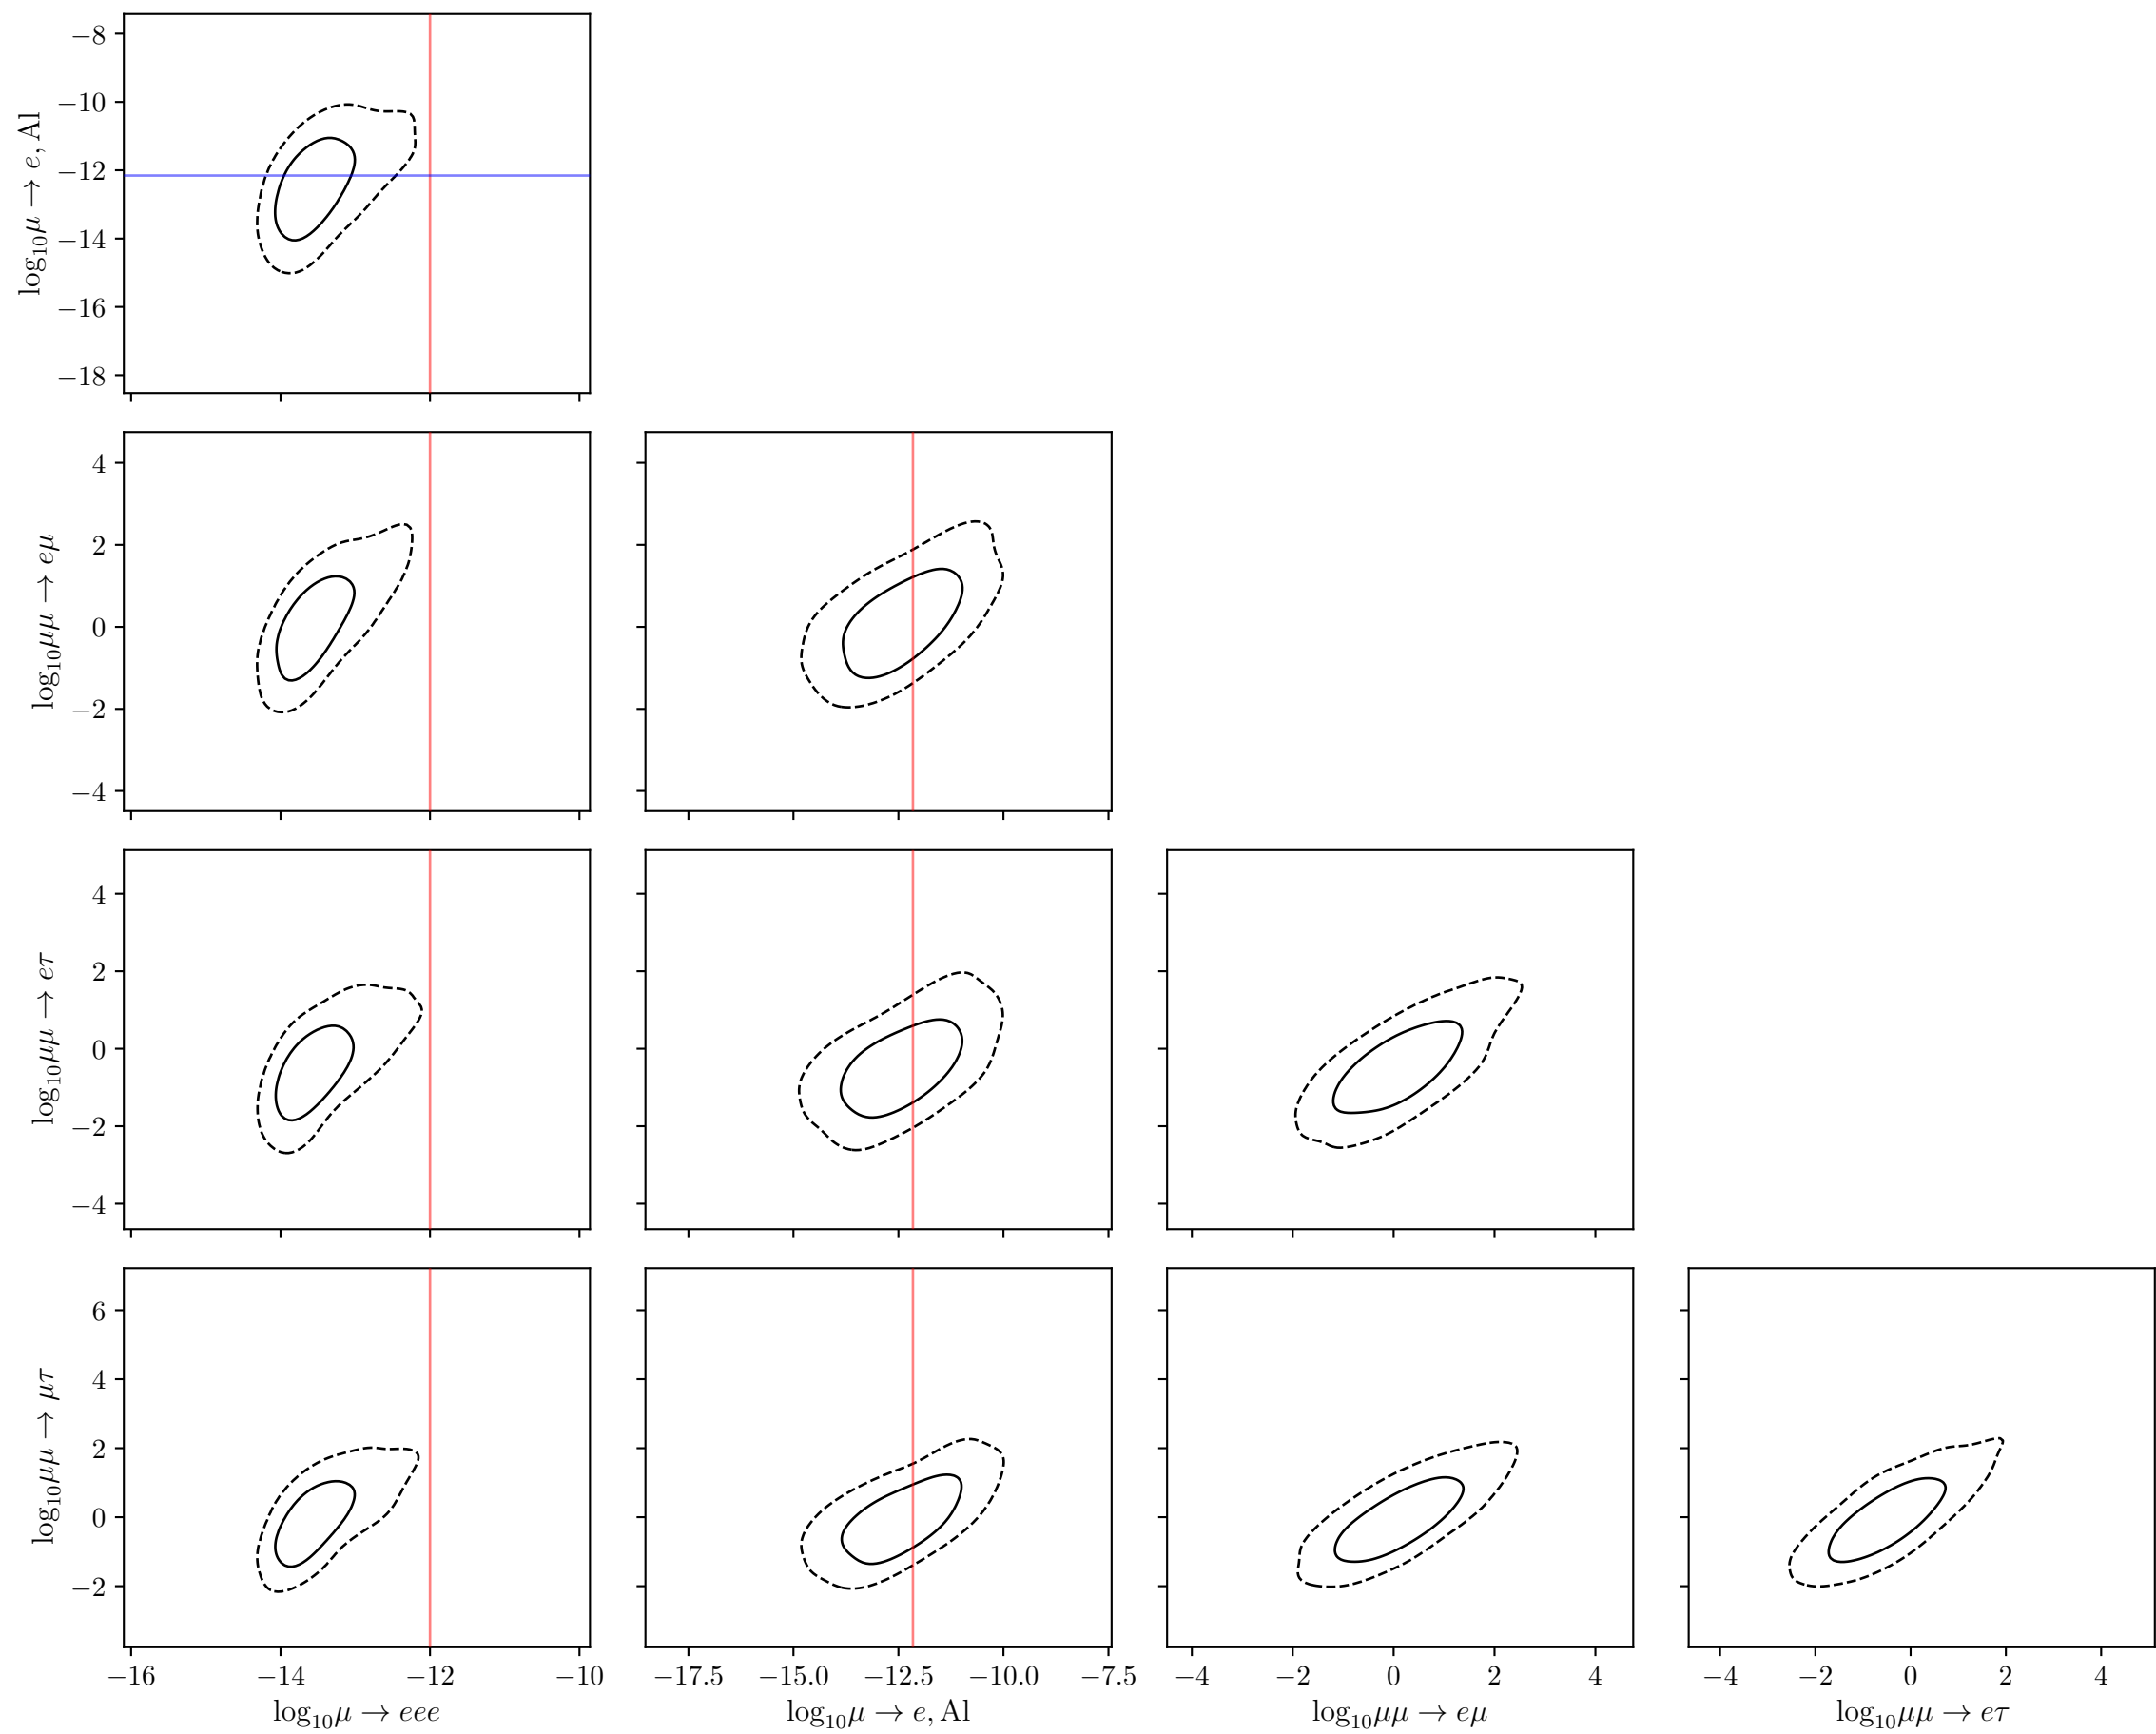



Majorana,  $X_L = \{5, 4, 3\}$ ,  $X_e = \{5, 2, 1\}$ ,

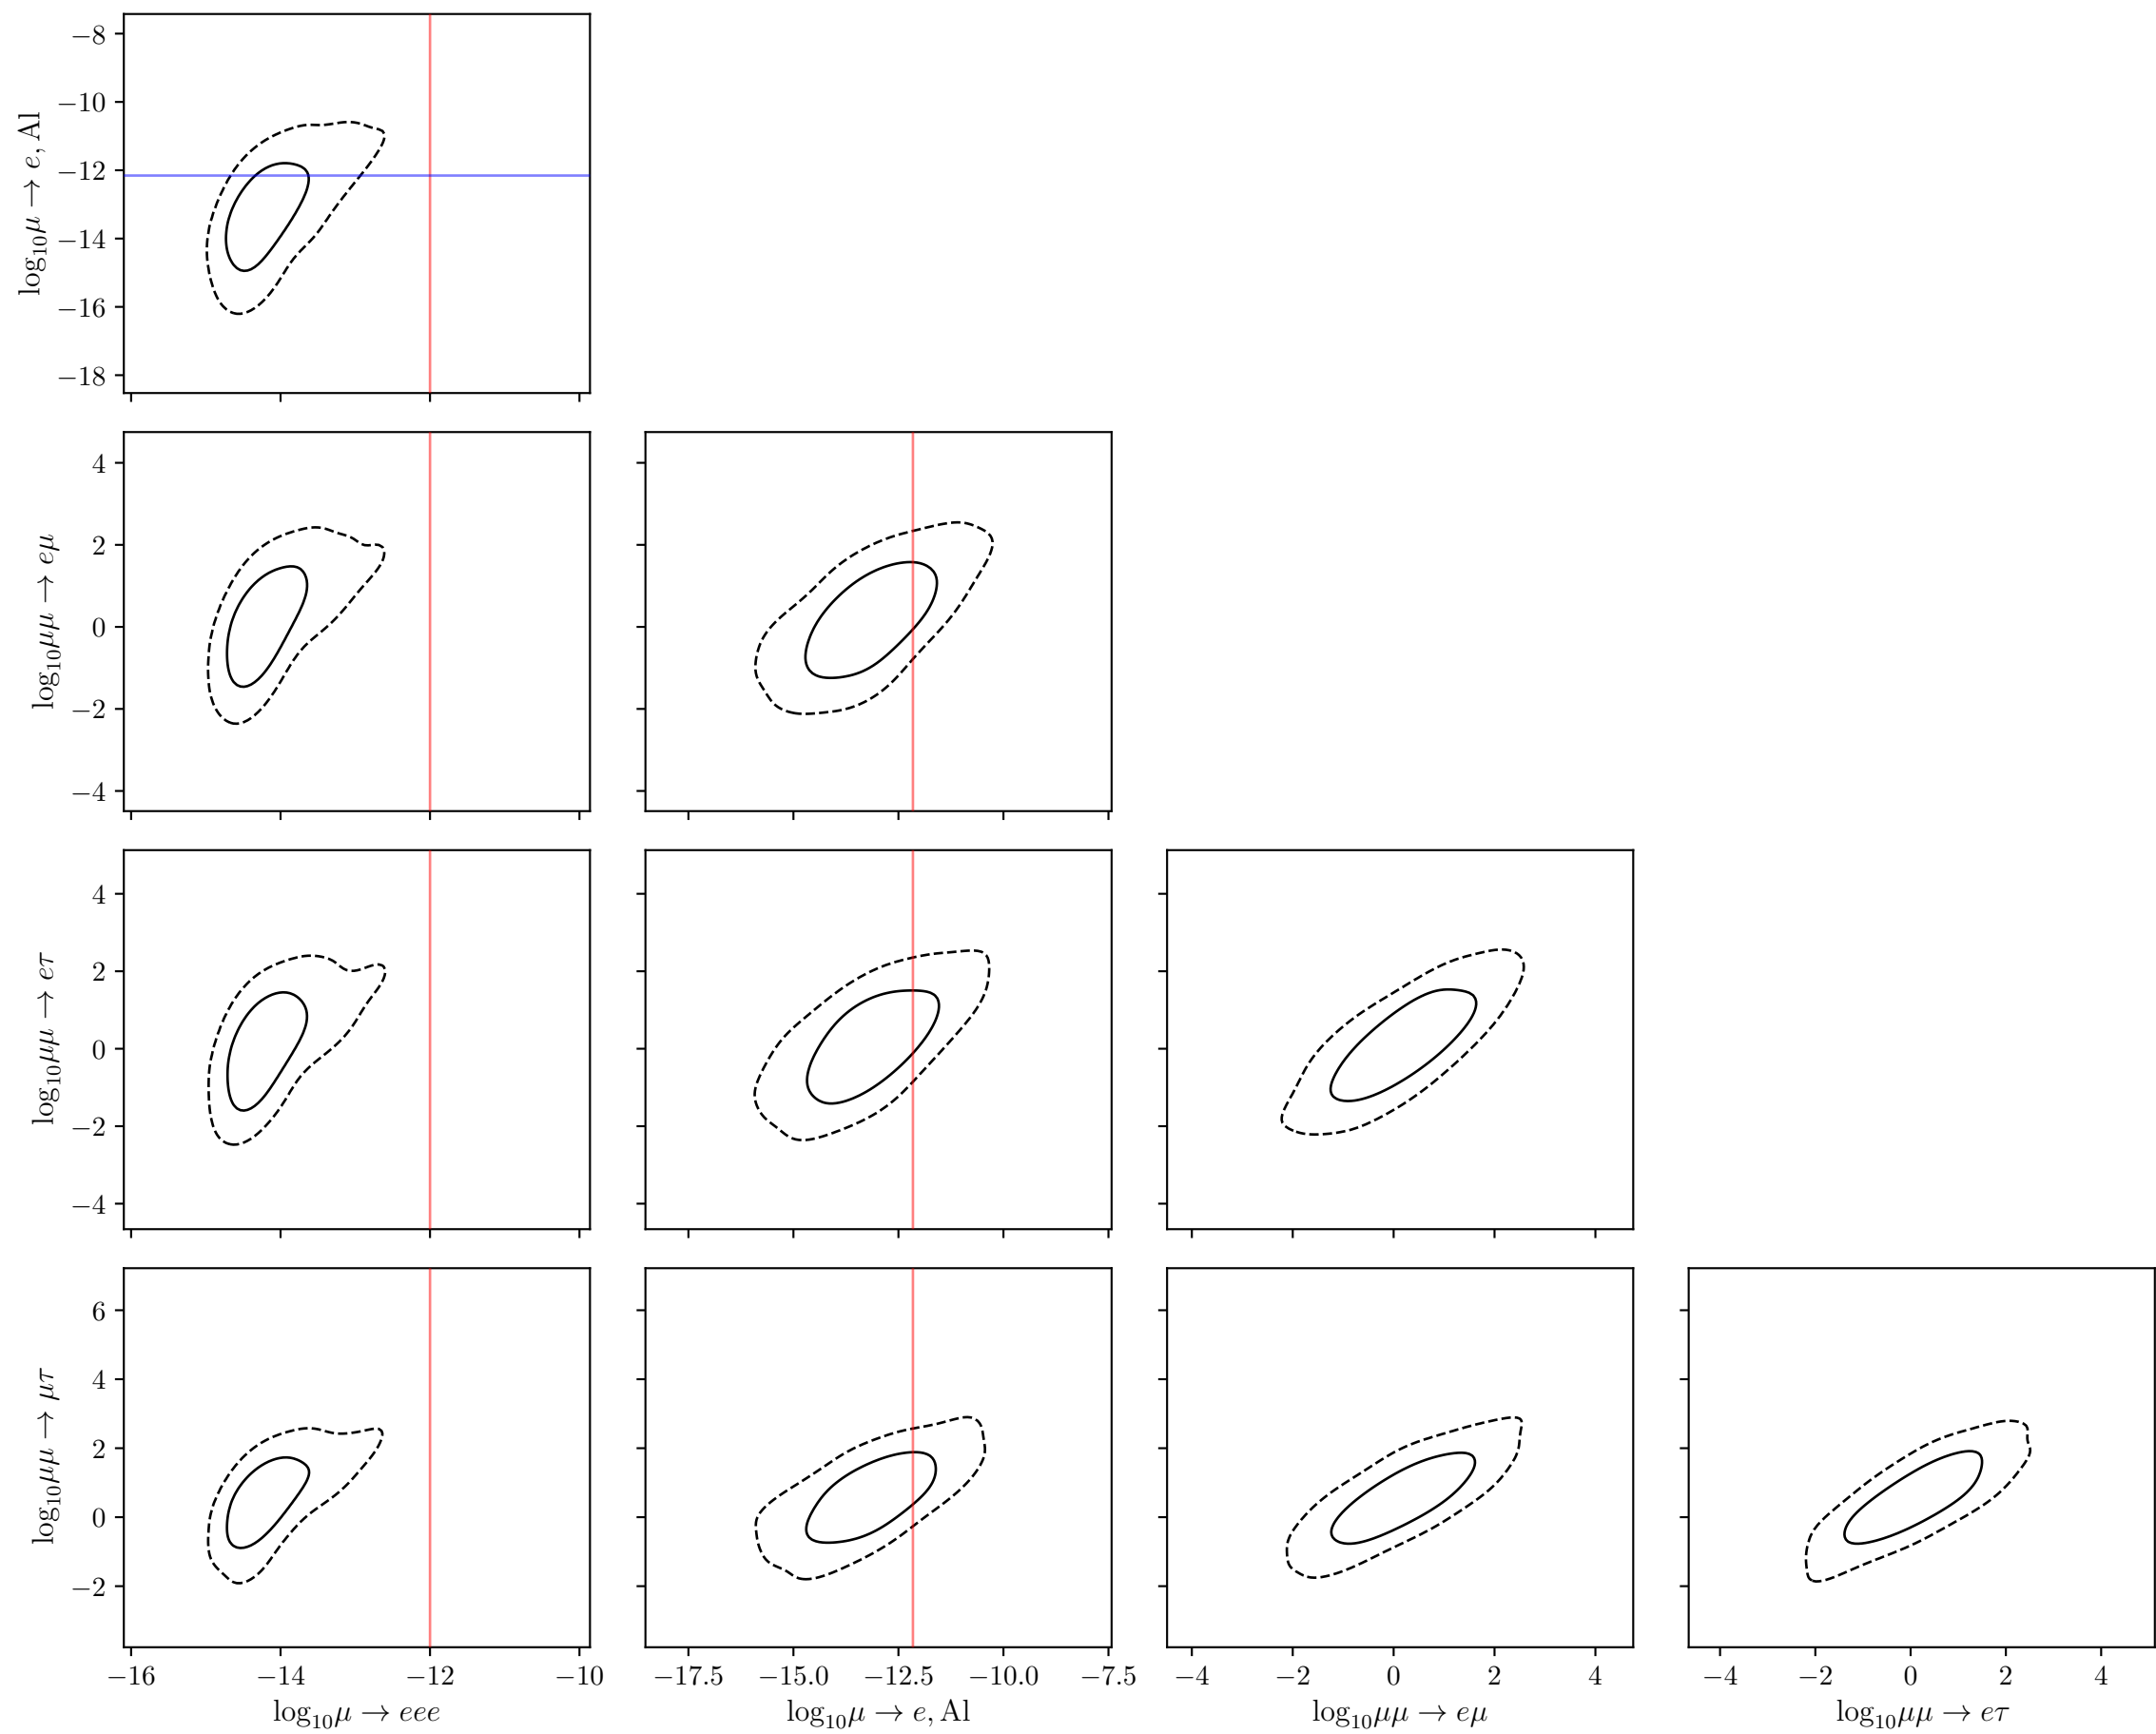

Majorana,  $X_L = \{4, 3, 2\}$ ,  $X_e = \{6, 3, 1\}$ ,

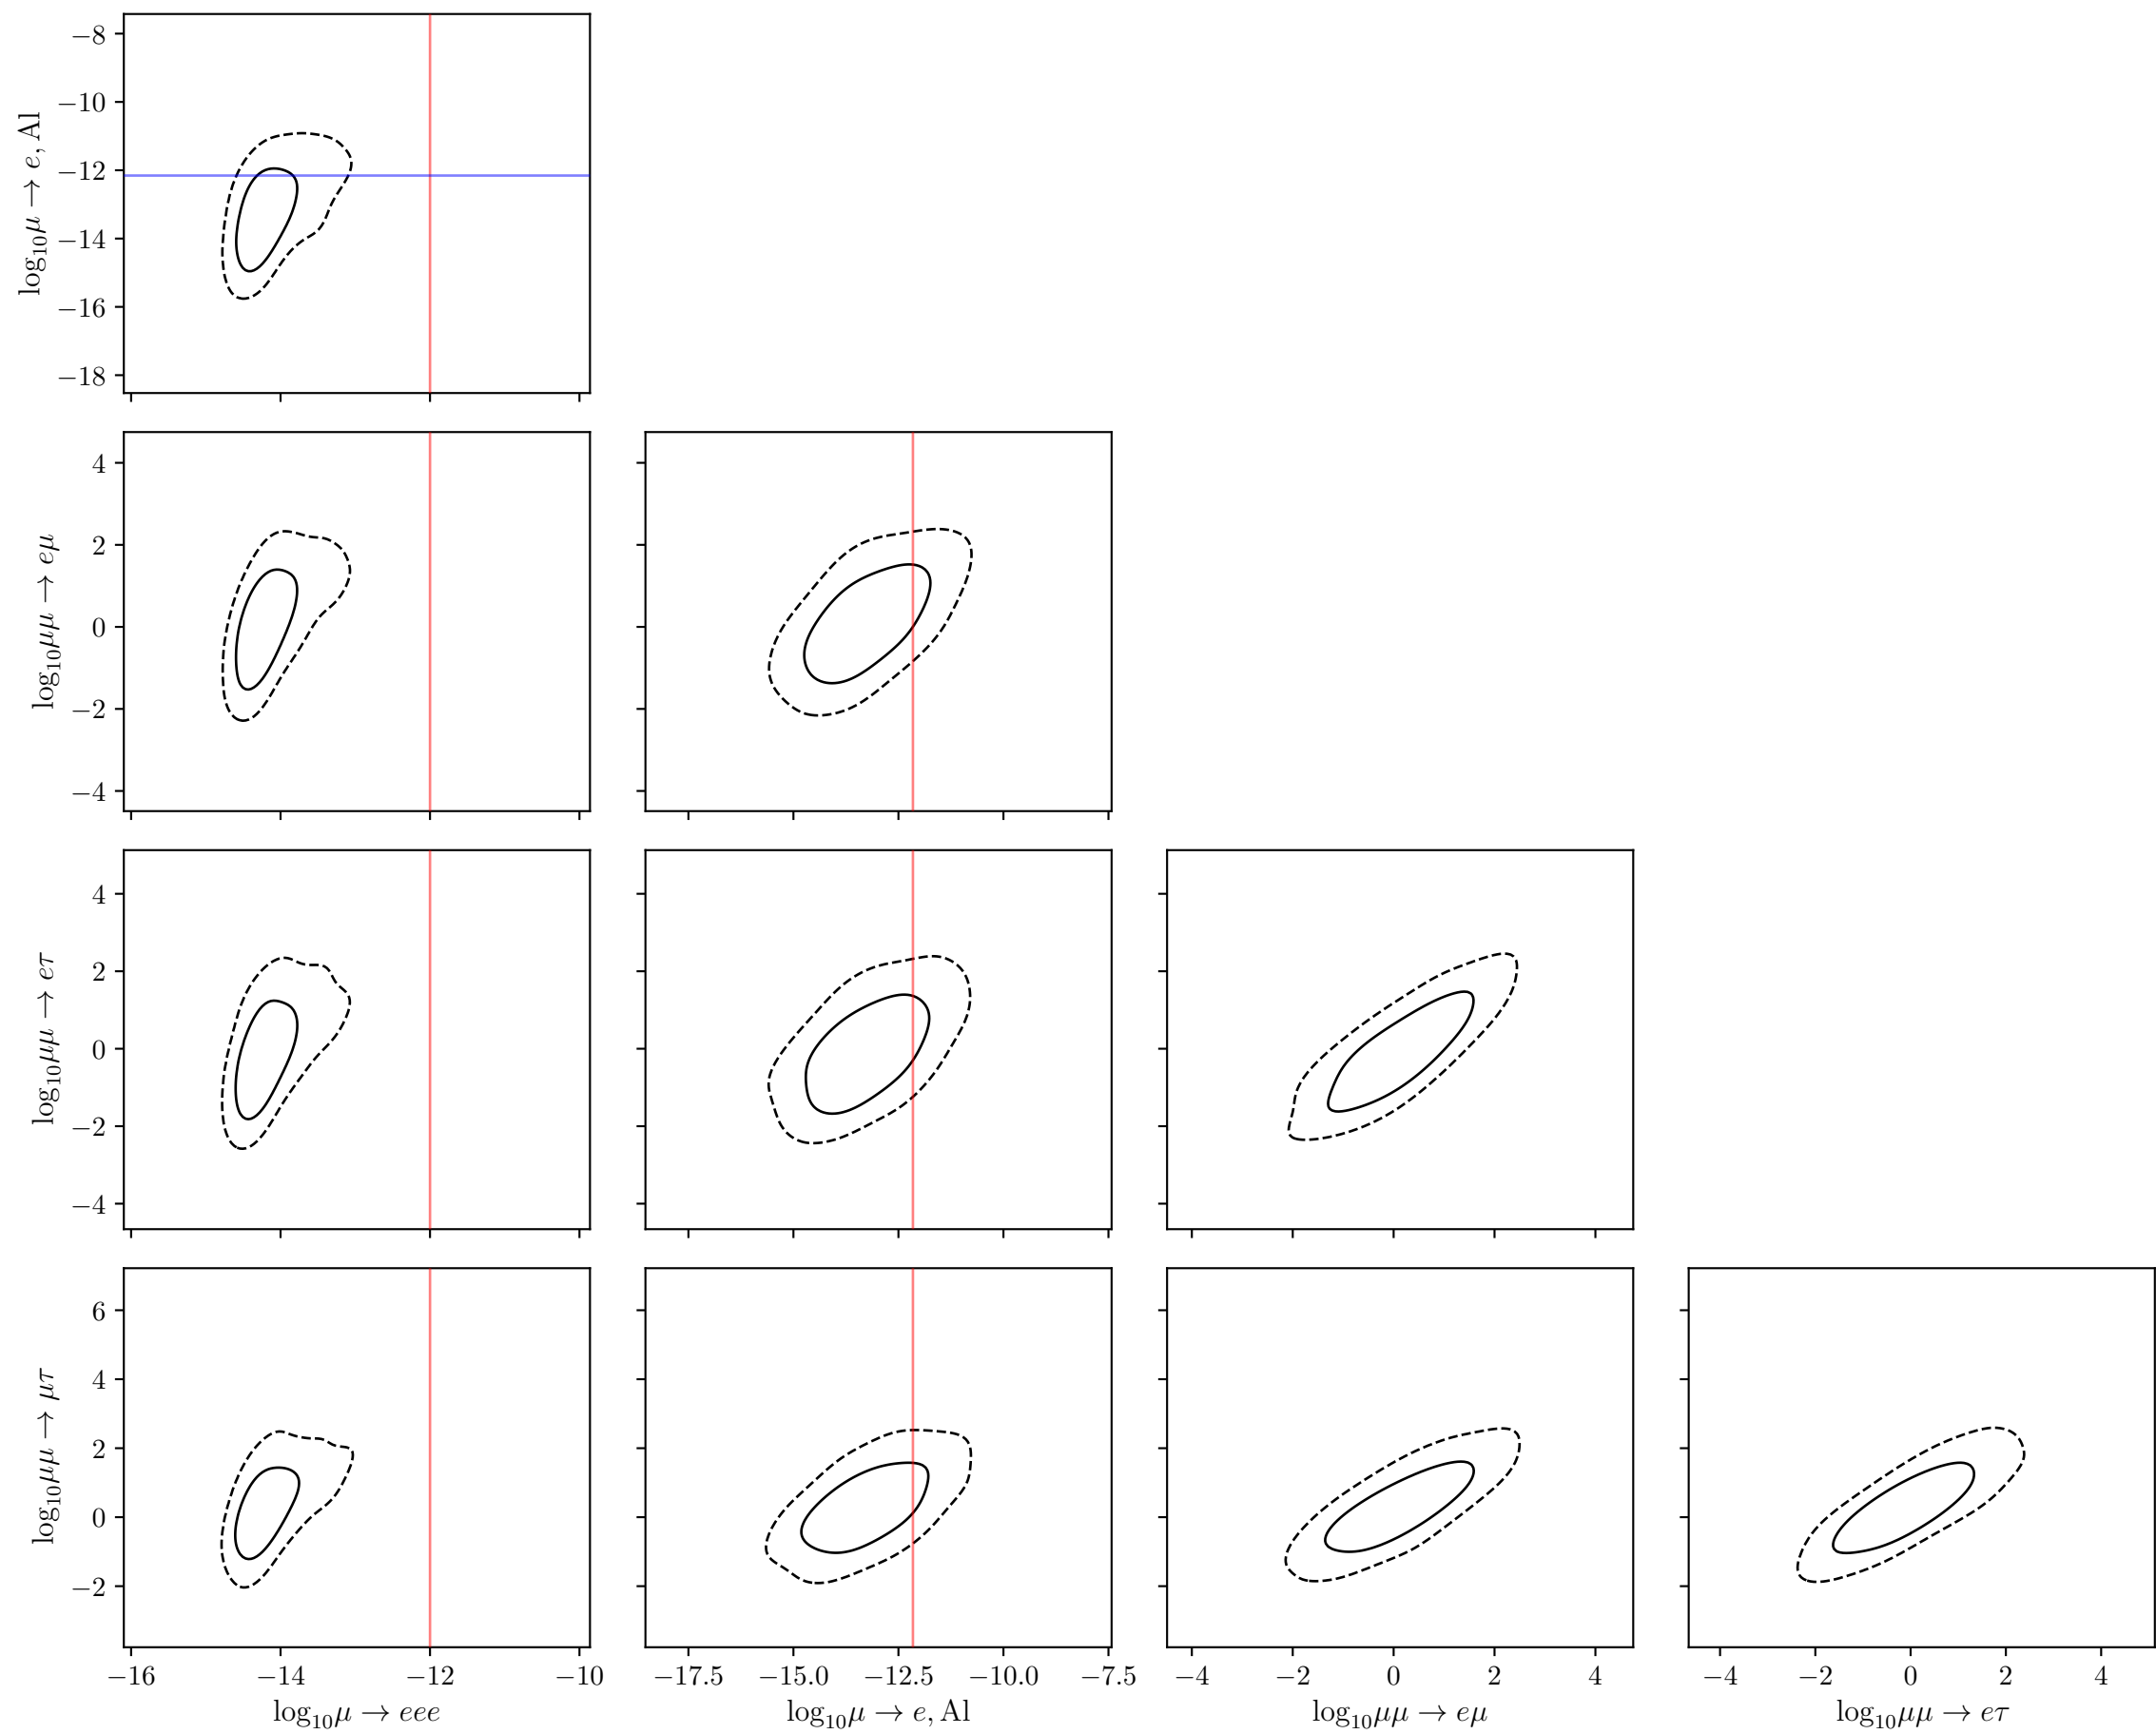

Majorana,  $X_L = \{7, 7, 6\}$ ,  $X_e = \{-3, -1, 3\}$ ,

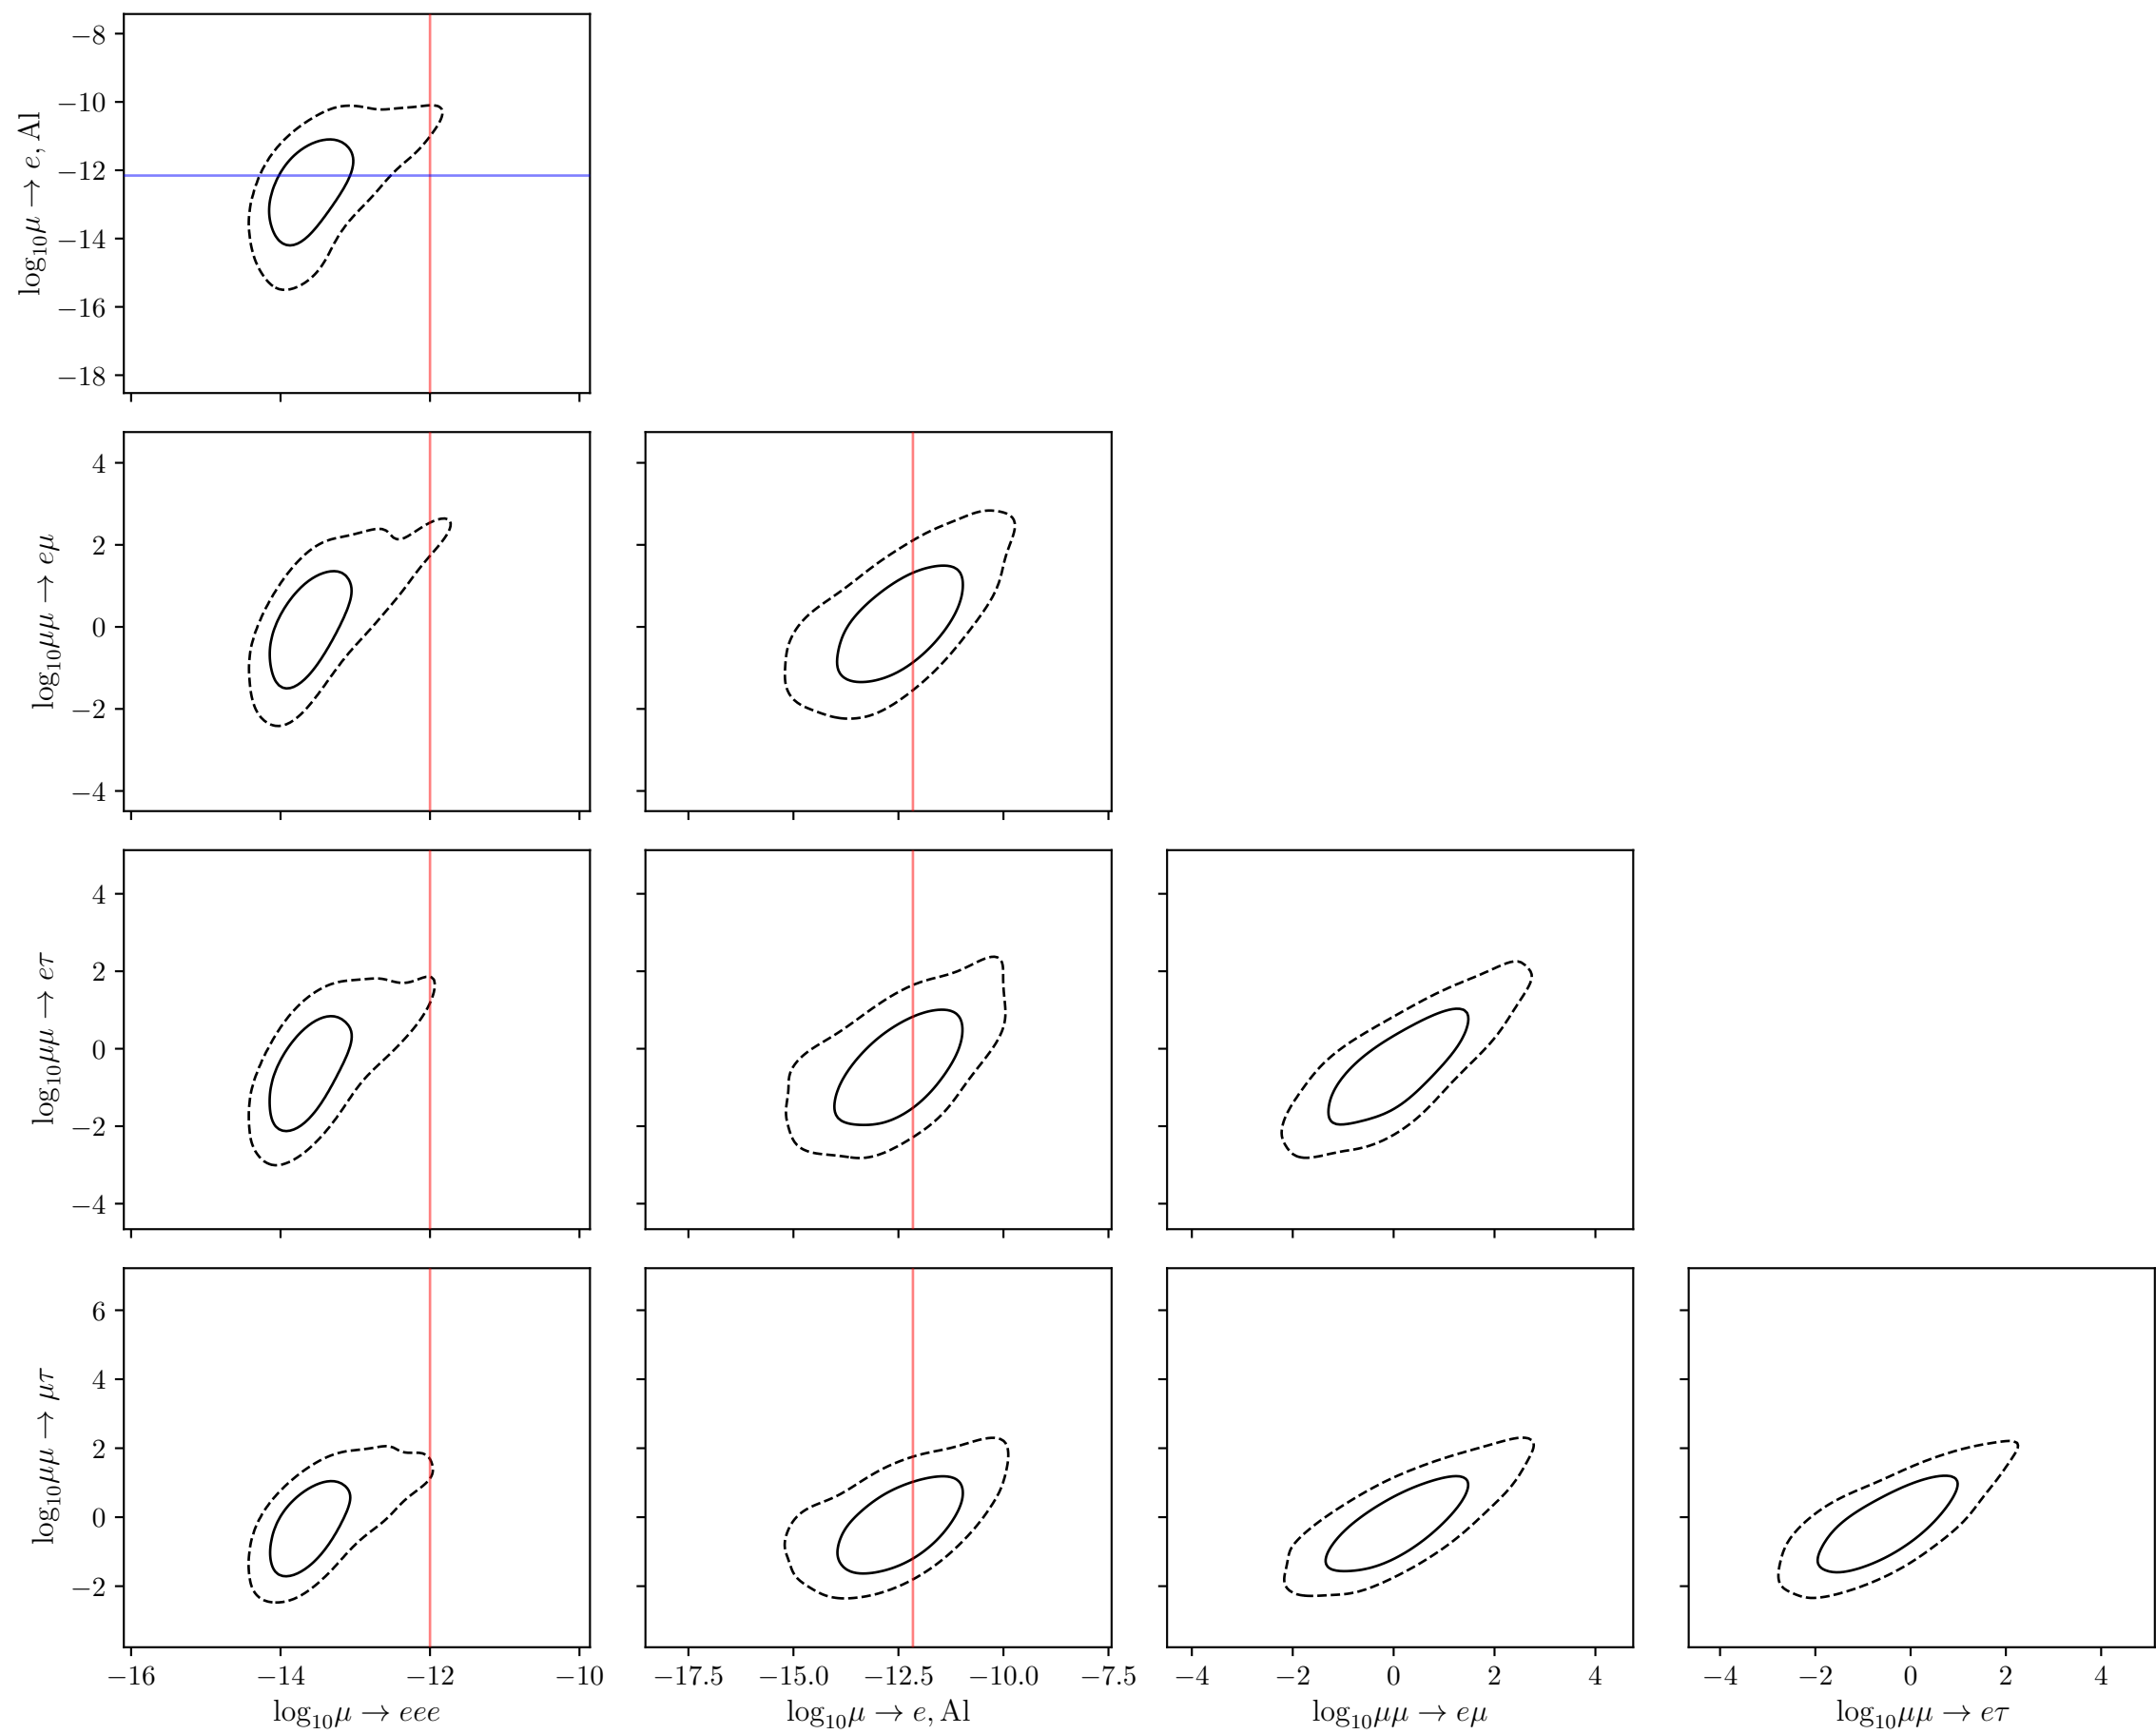

Majorana,  $X_L = \{4, 3, 2\}$ ,  $X_e = \{7, 3, 2\}$ ,

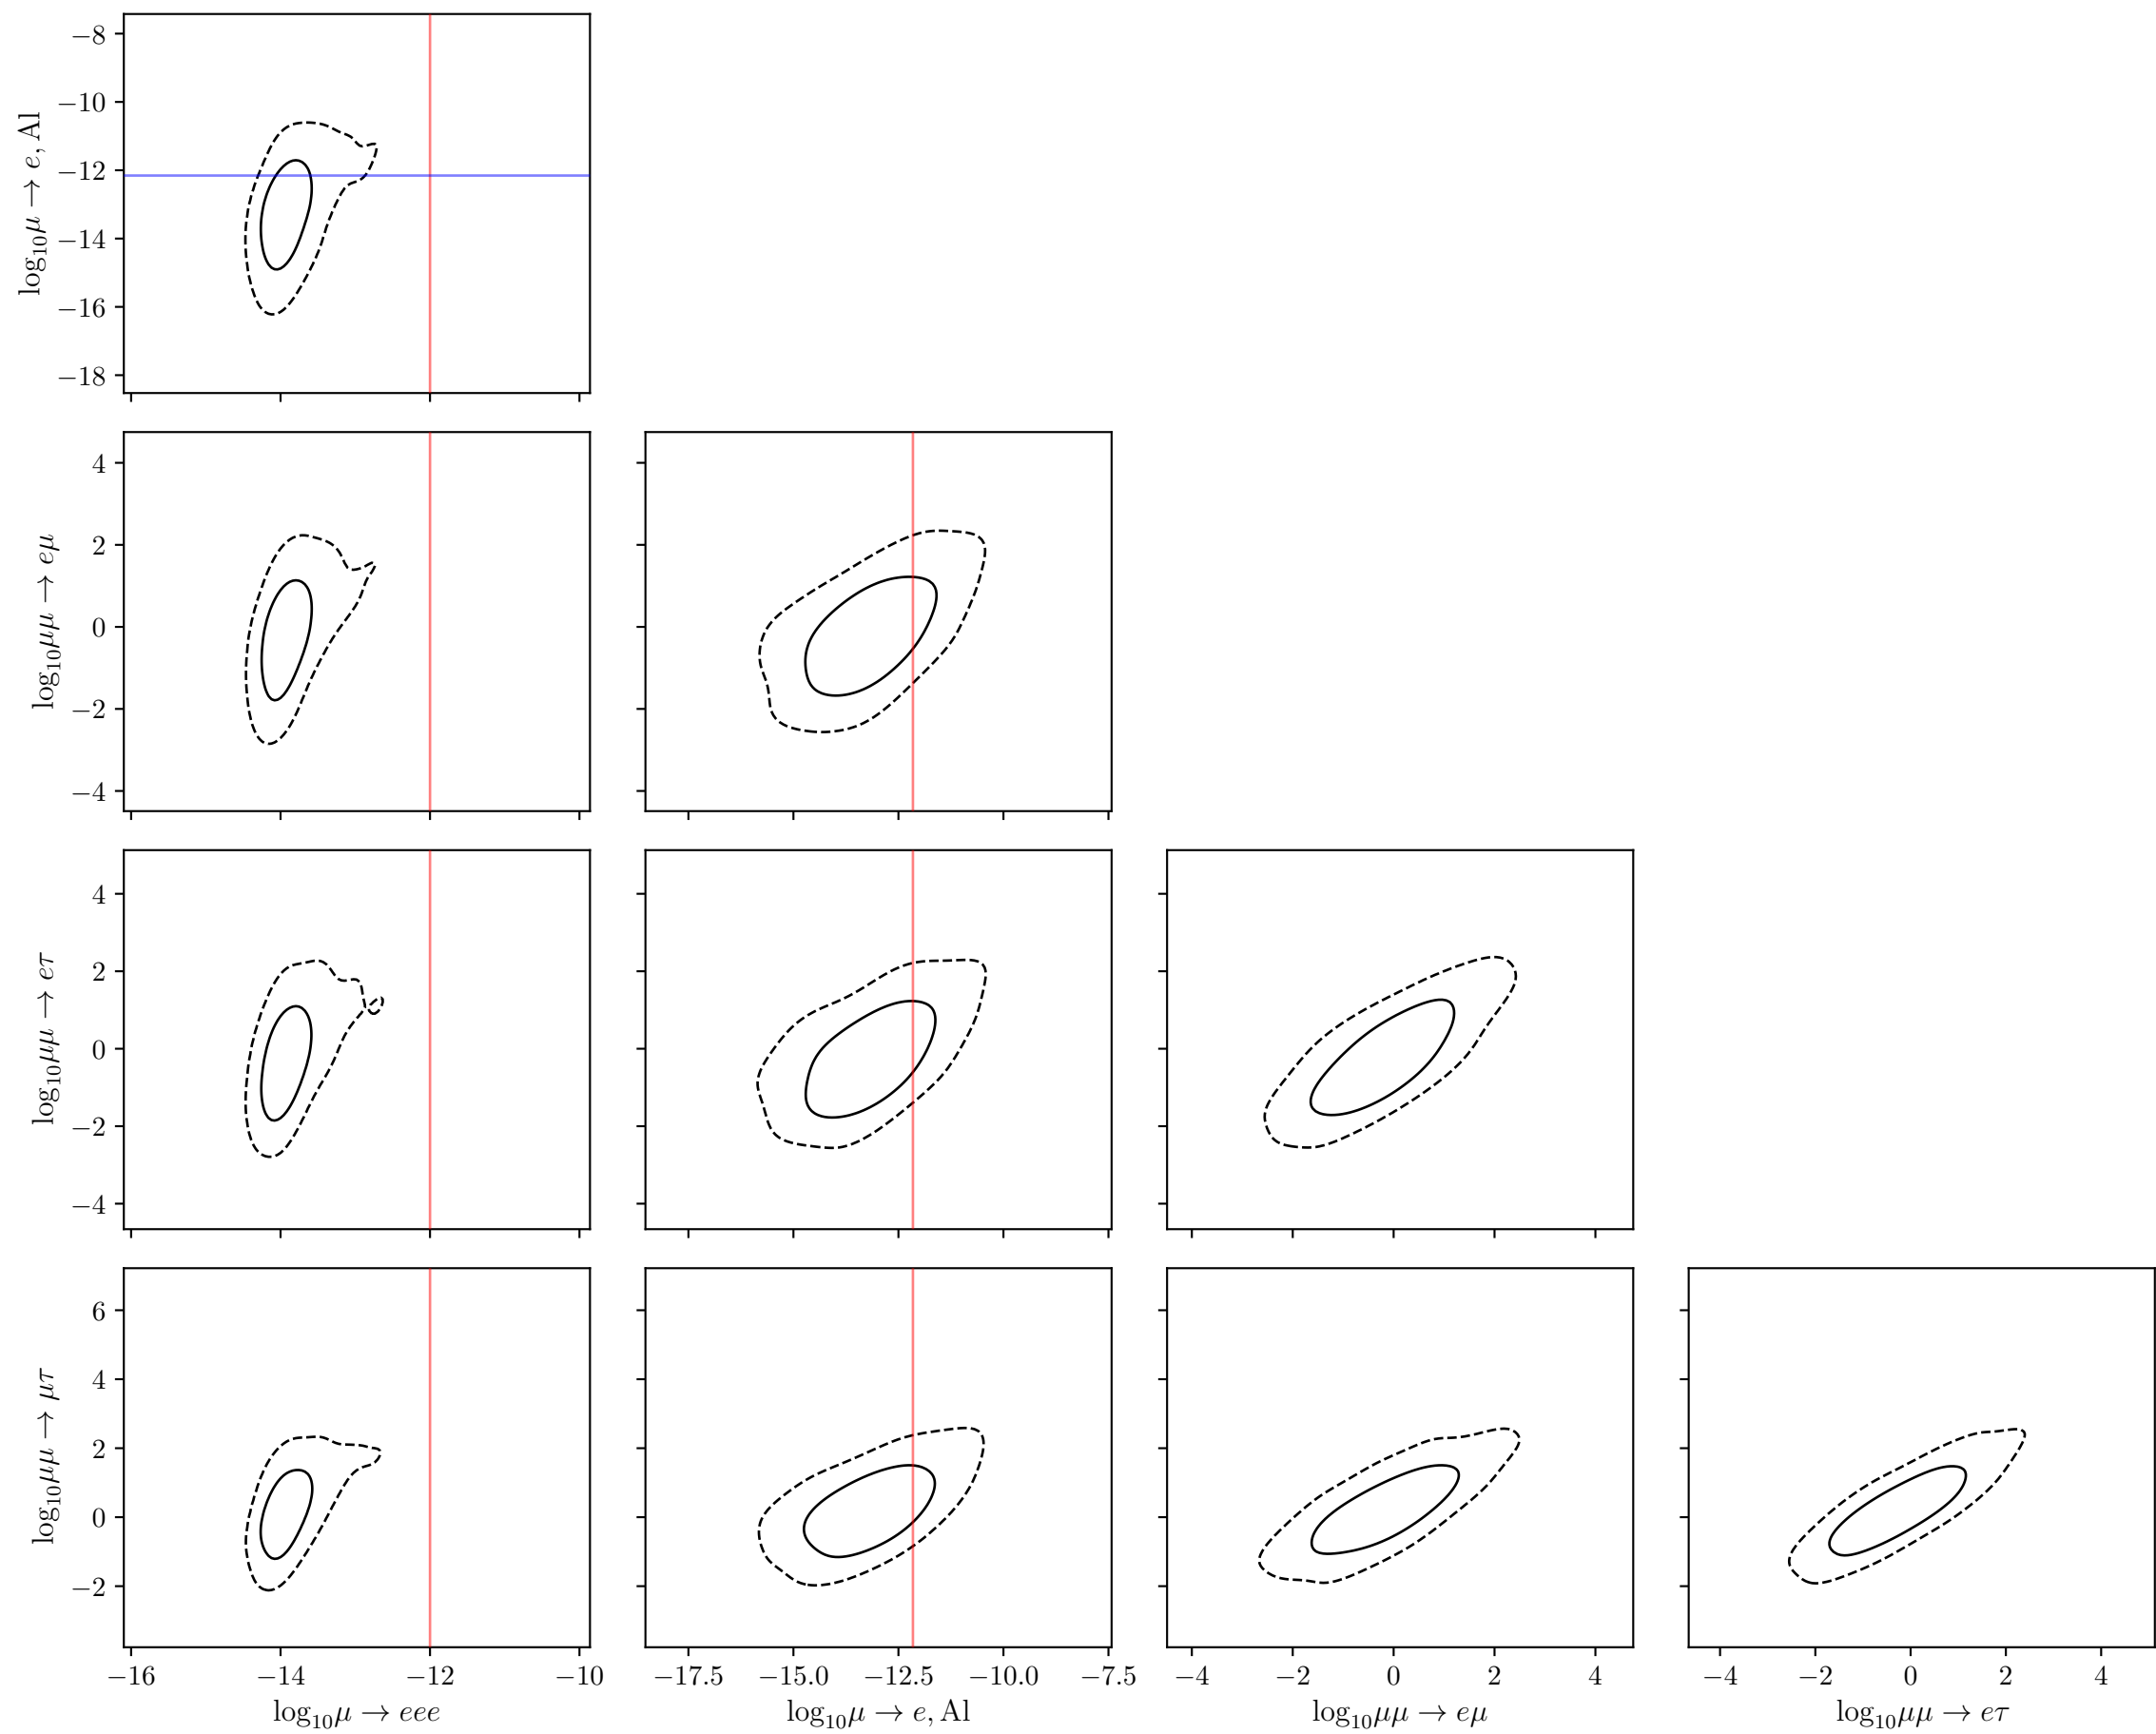

Majorana,  $X_L = \{5, 5, 4\}$ ,  $X_e = \{-1, 0, 3\}$ ,

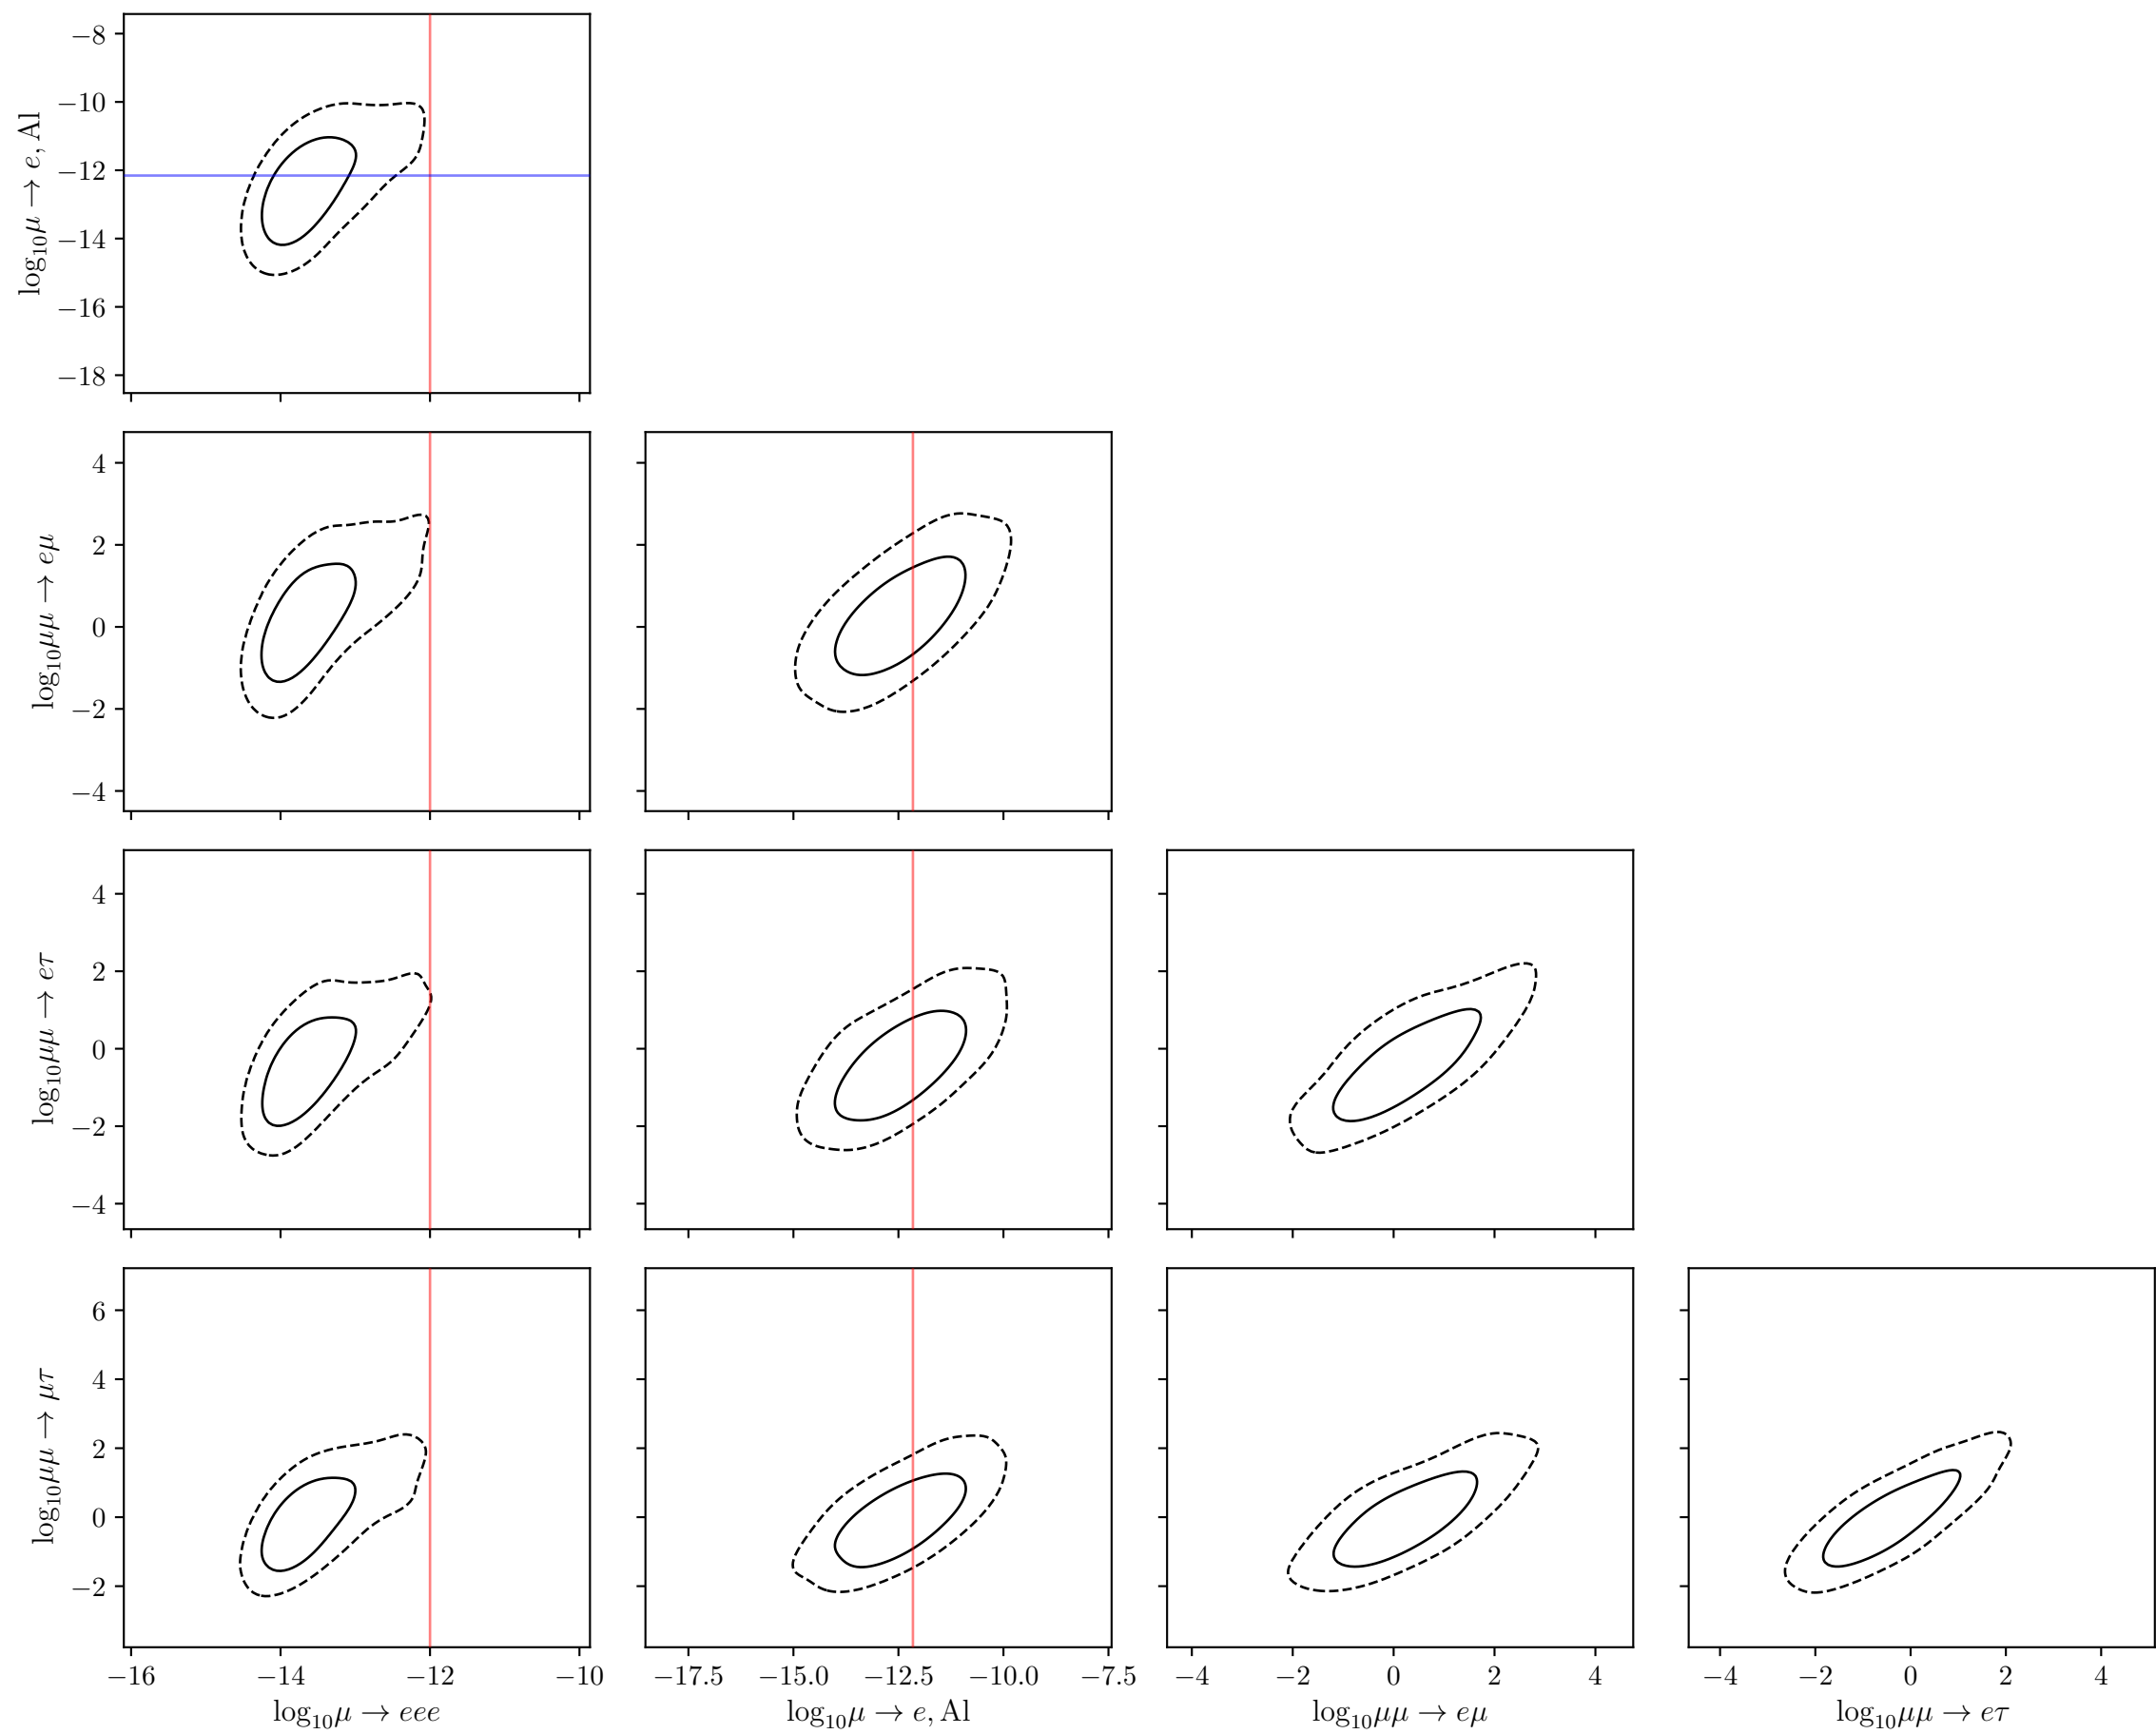

Majorana,  $X_L = \{6, 5, 4\}$ ,  $X_e = \{6, 2, 1\}$ ,

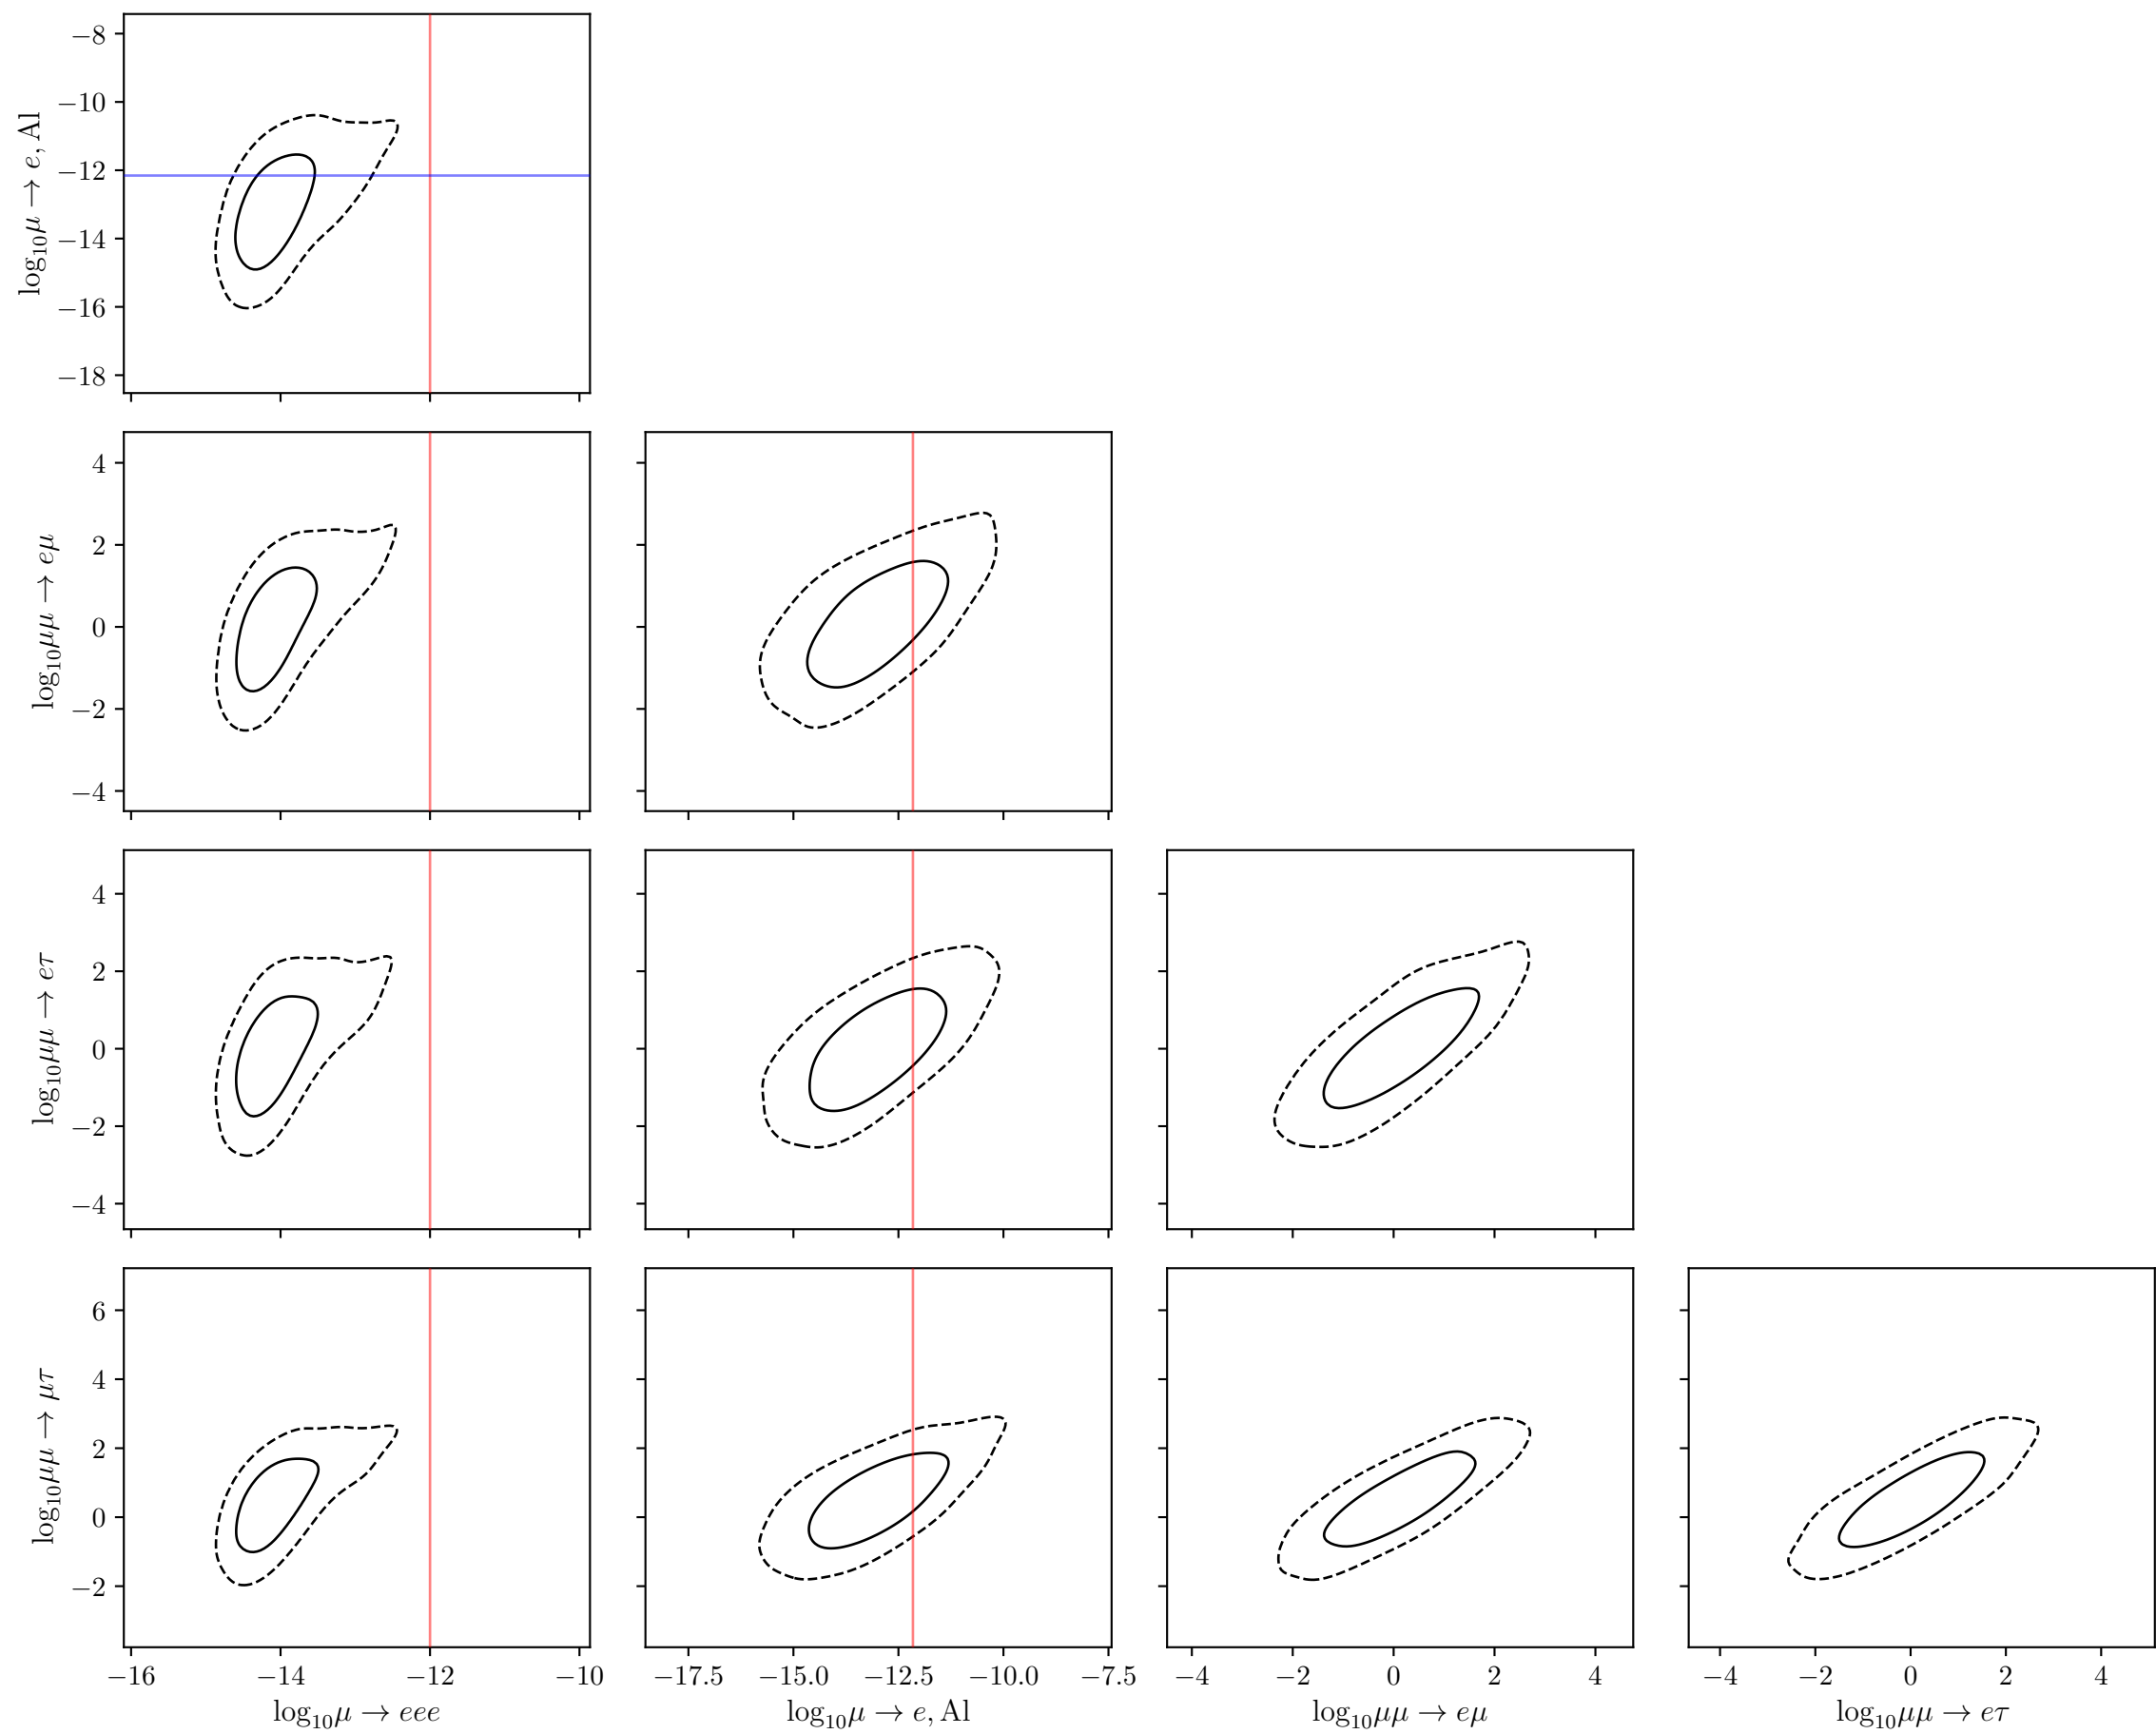

Majorana,  $X_L = \{7, 6, 5\}$ ,  $X_e = \{6, 1, 0\}$ ,

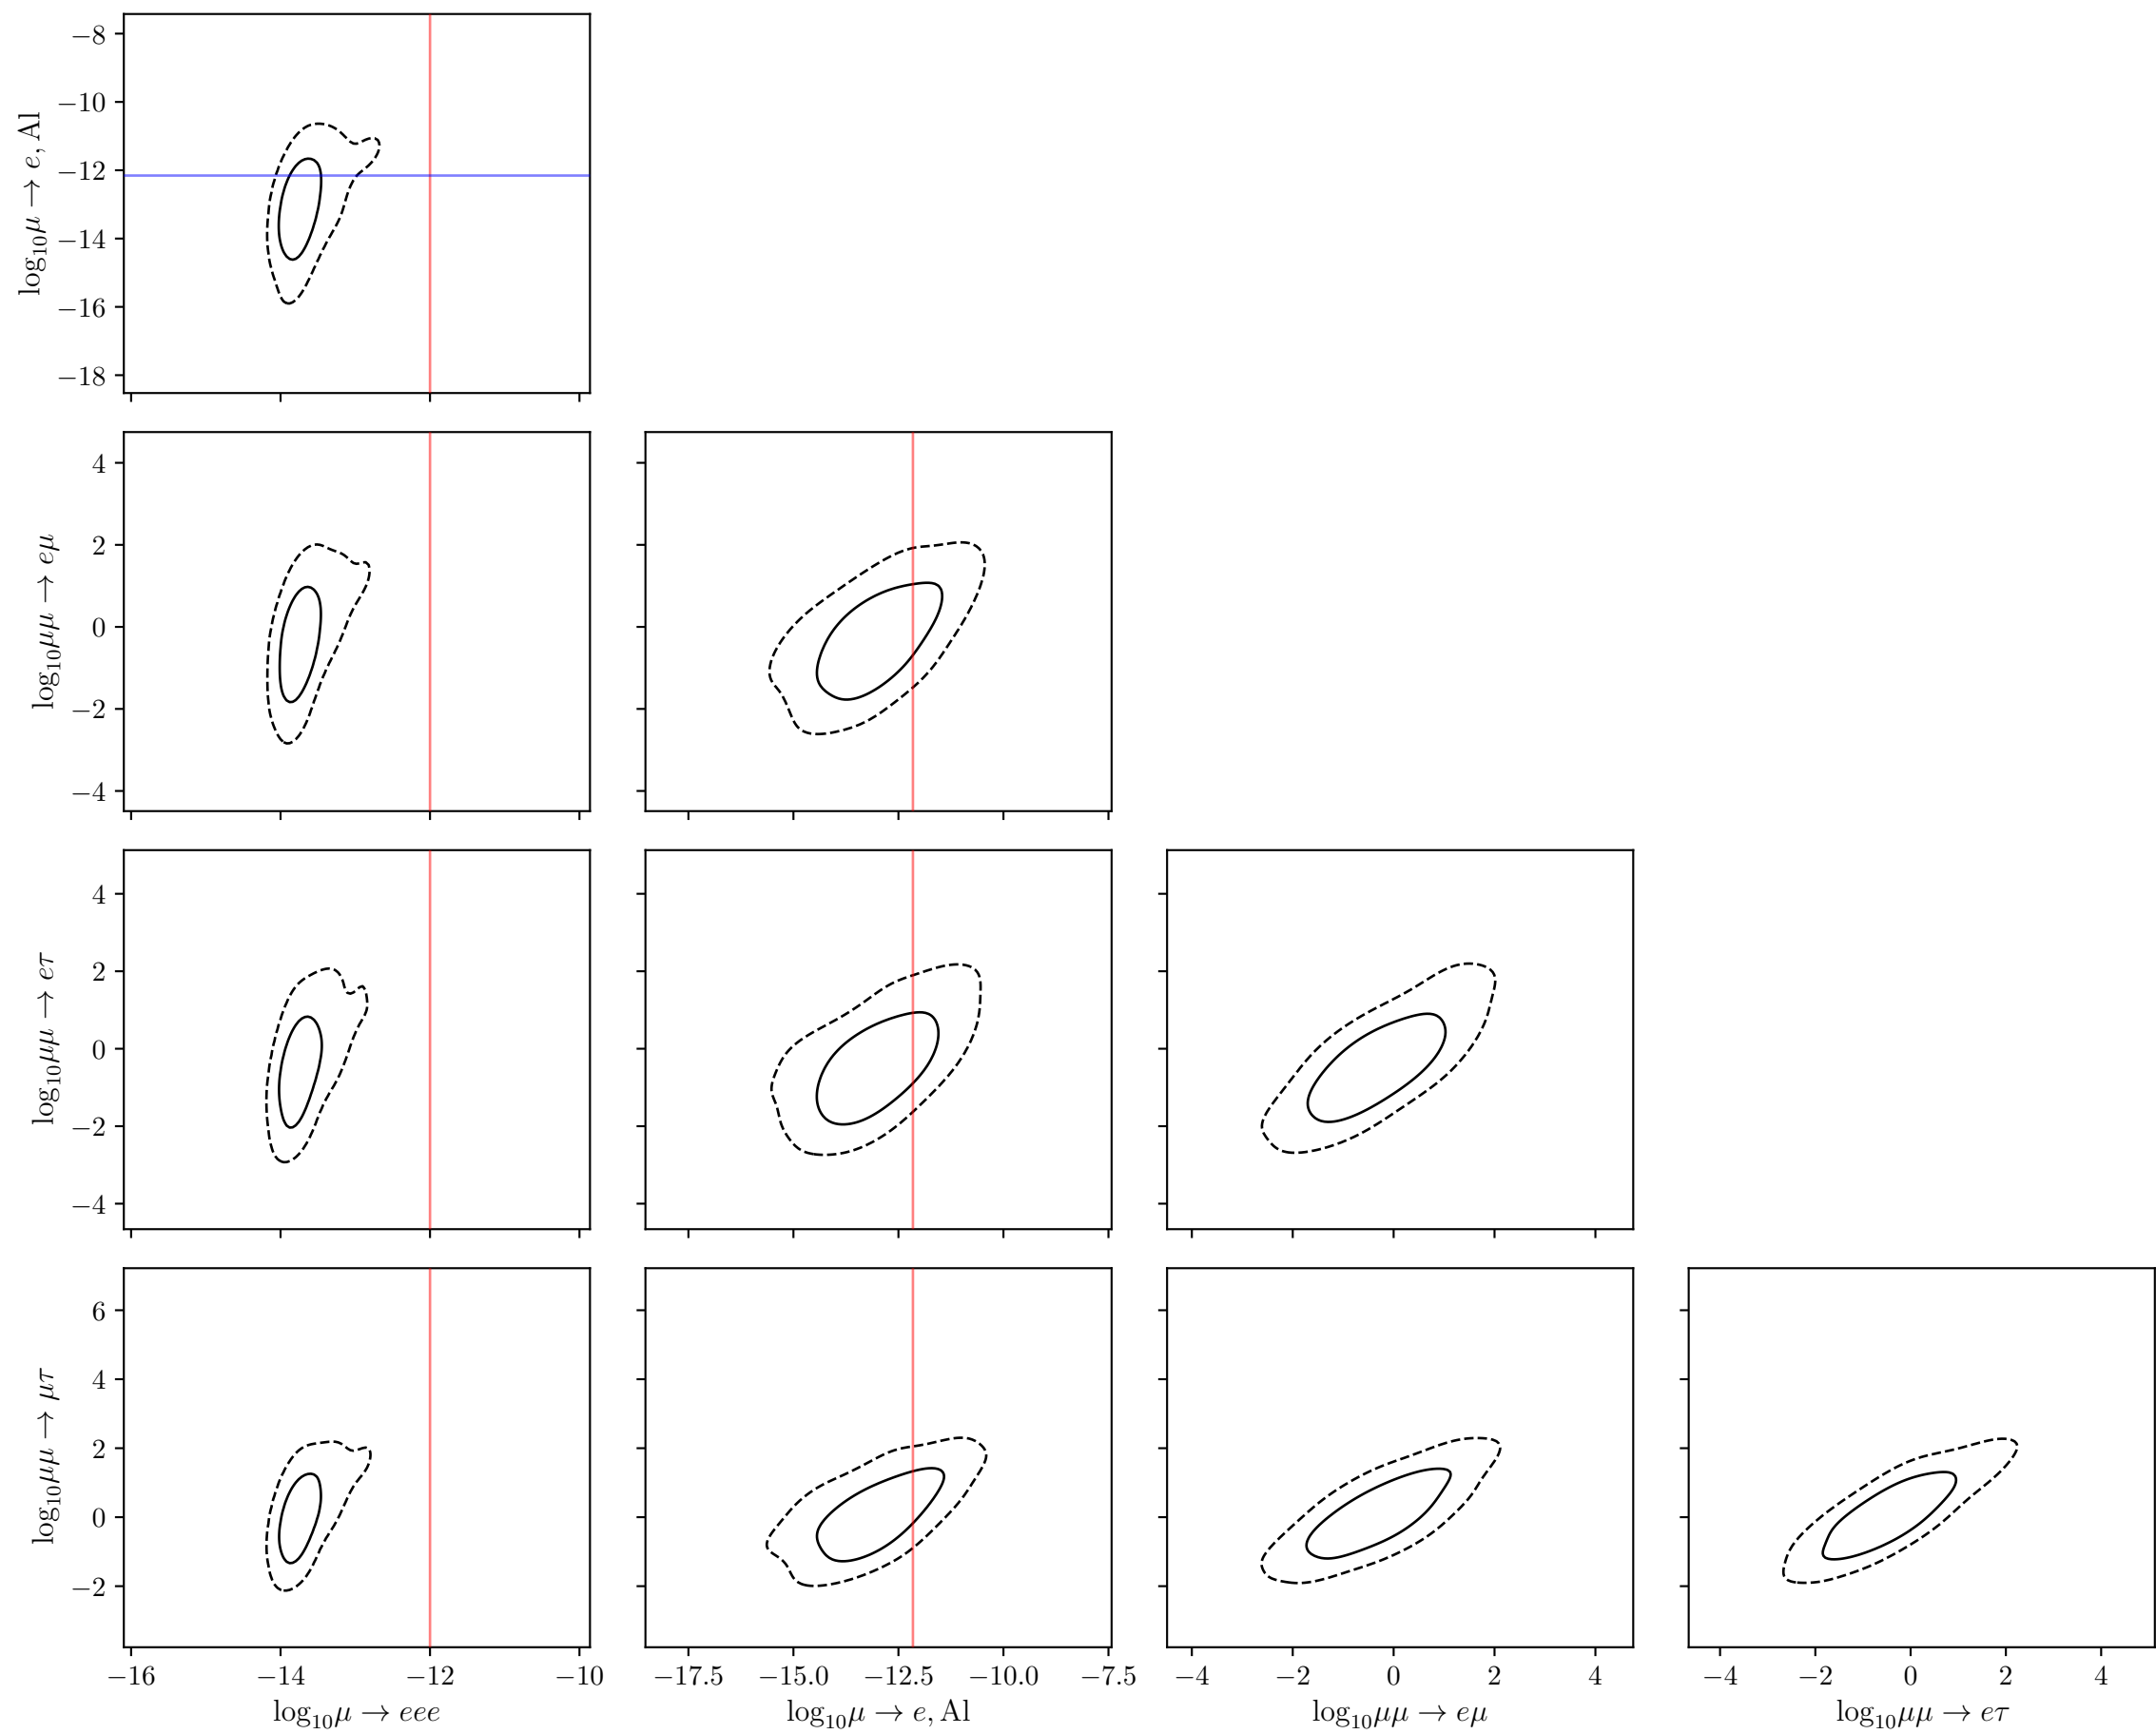

Majorana,  $X_L = \{3, 3, 2\}$ ,  $X_e = \{7, 3, 2\}$ ,

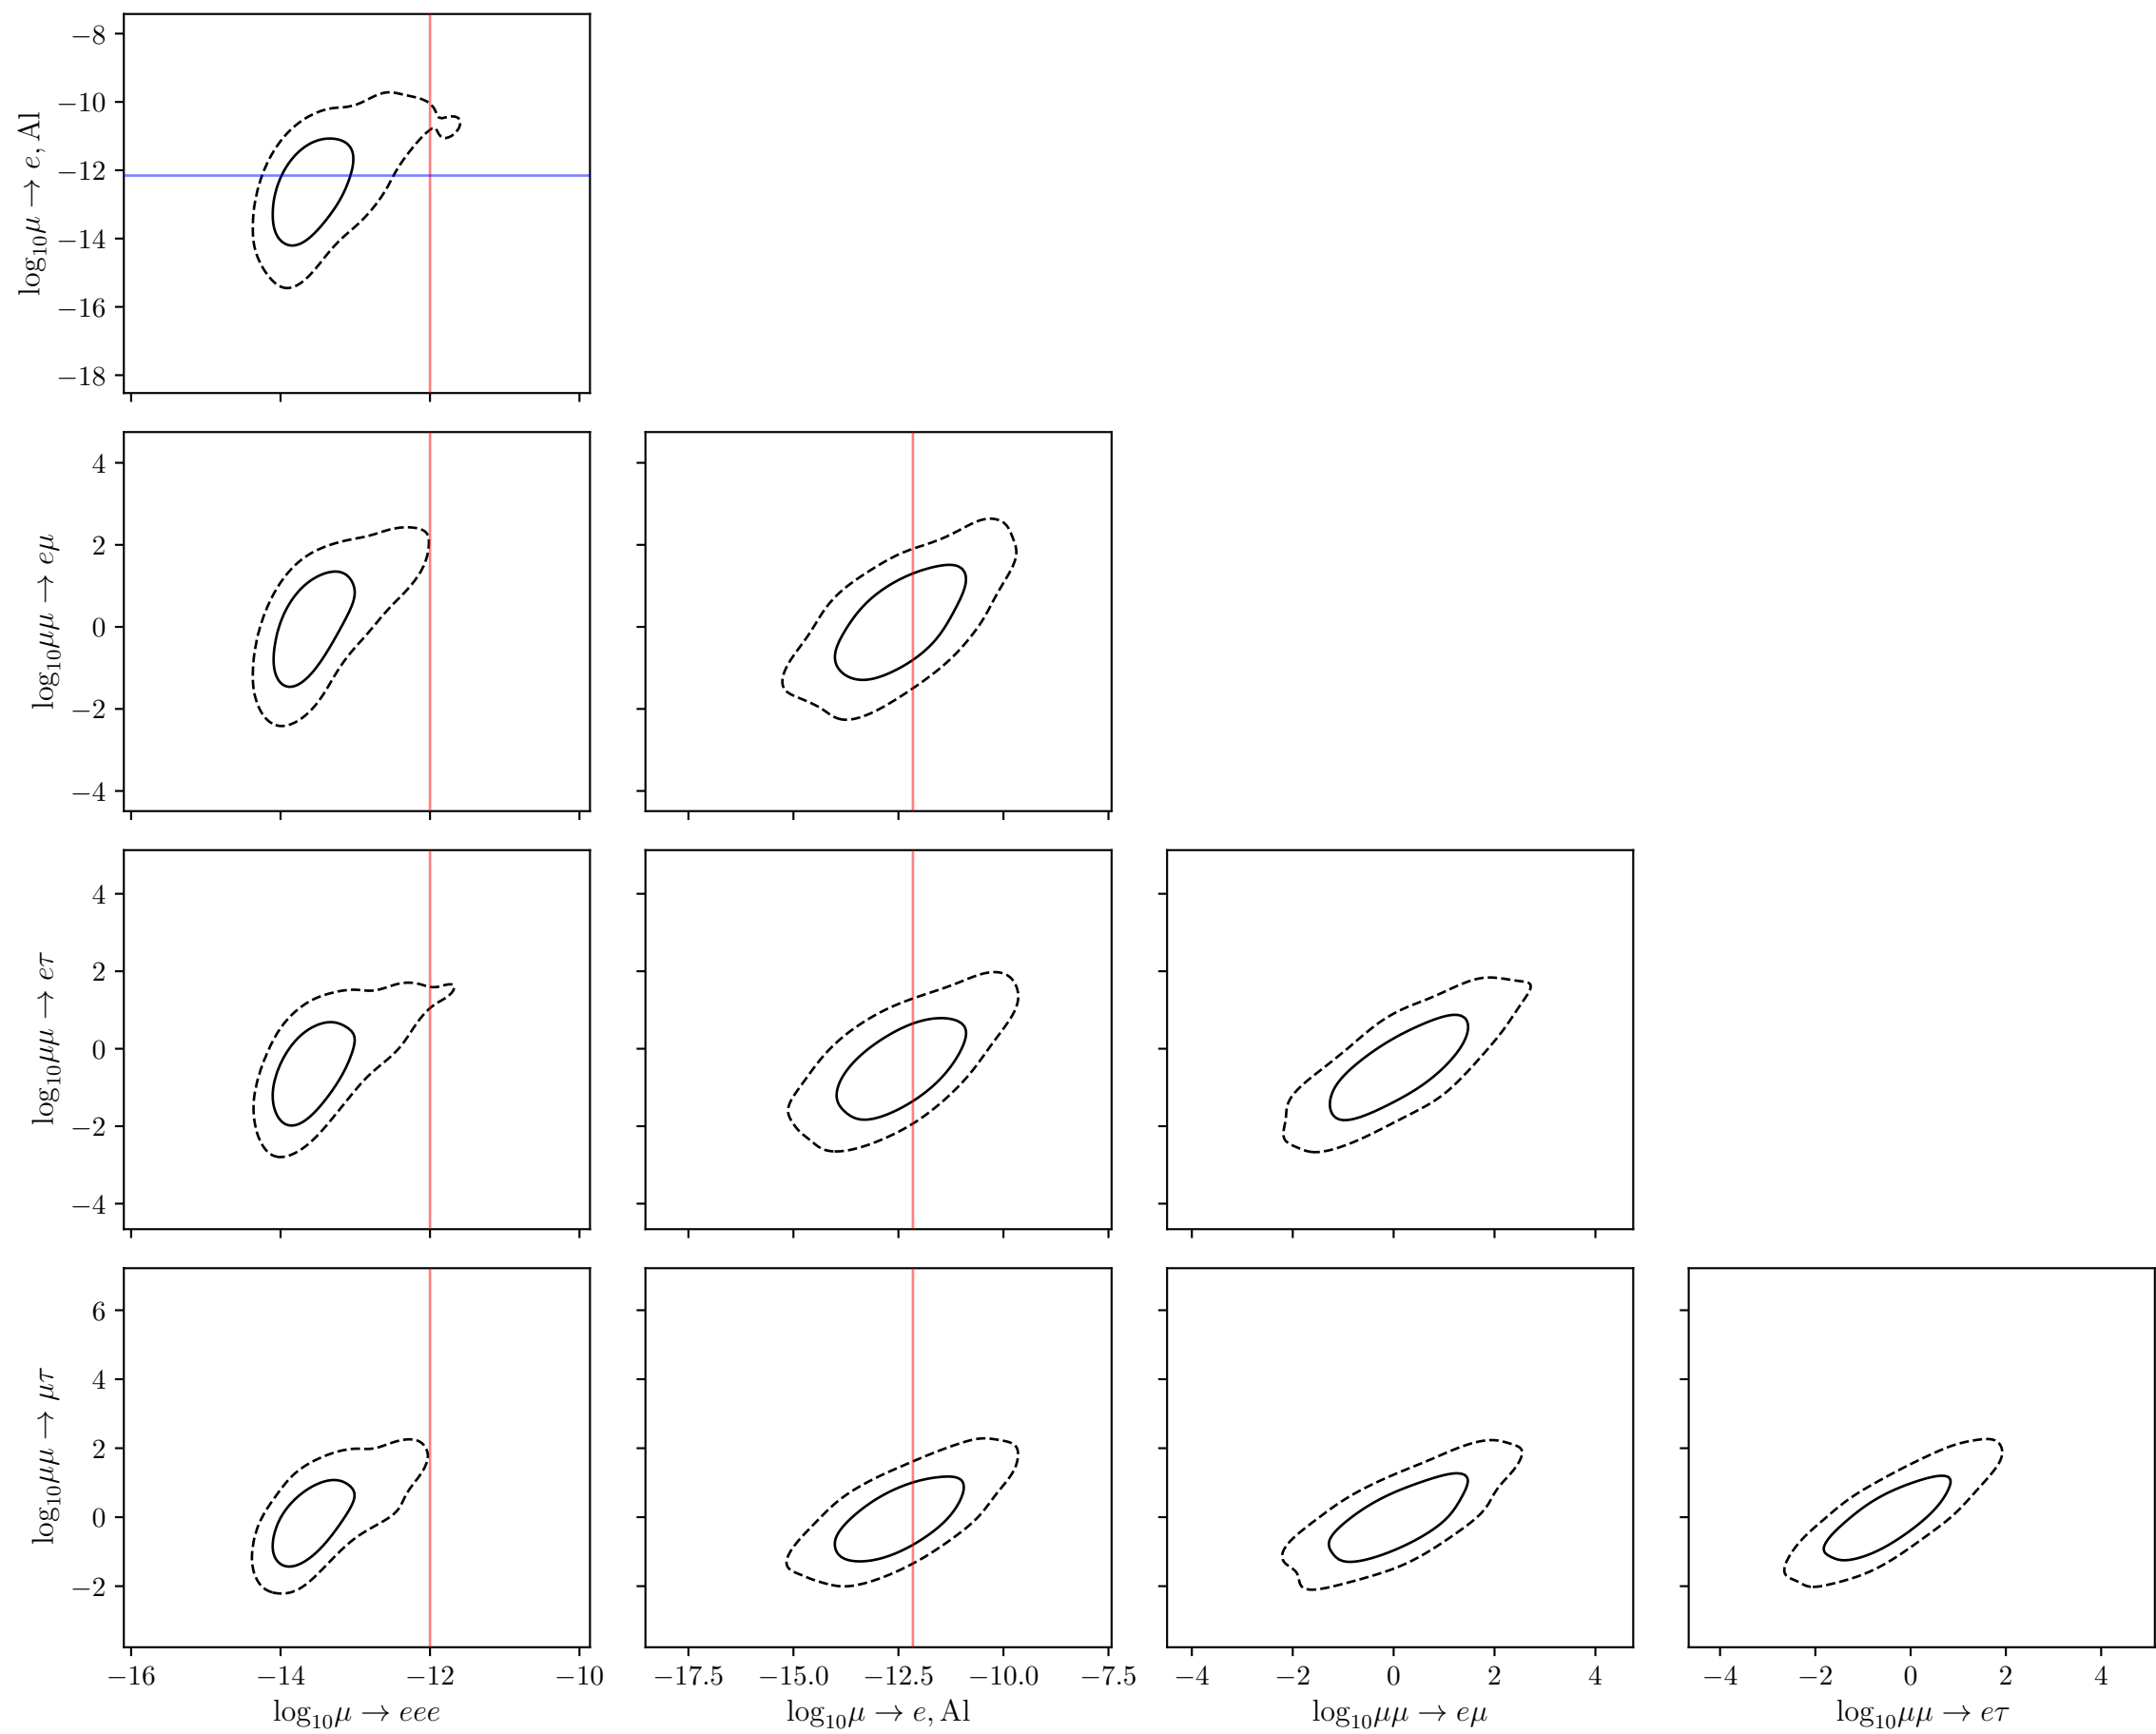



Majorana,  $X_L = \{7, 7, 5\}$ ,  $X_e = \{7, 2, 0\}$ ,

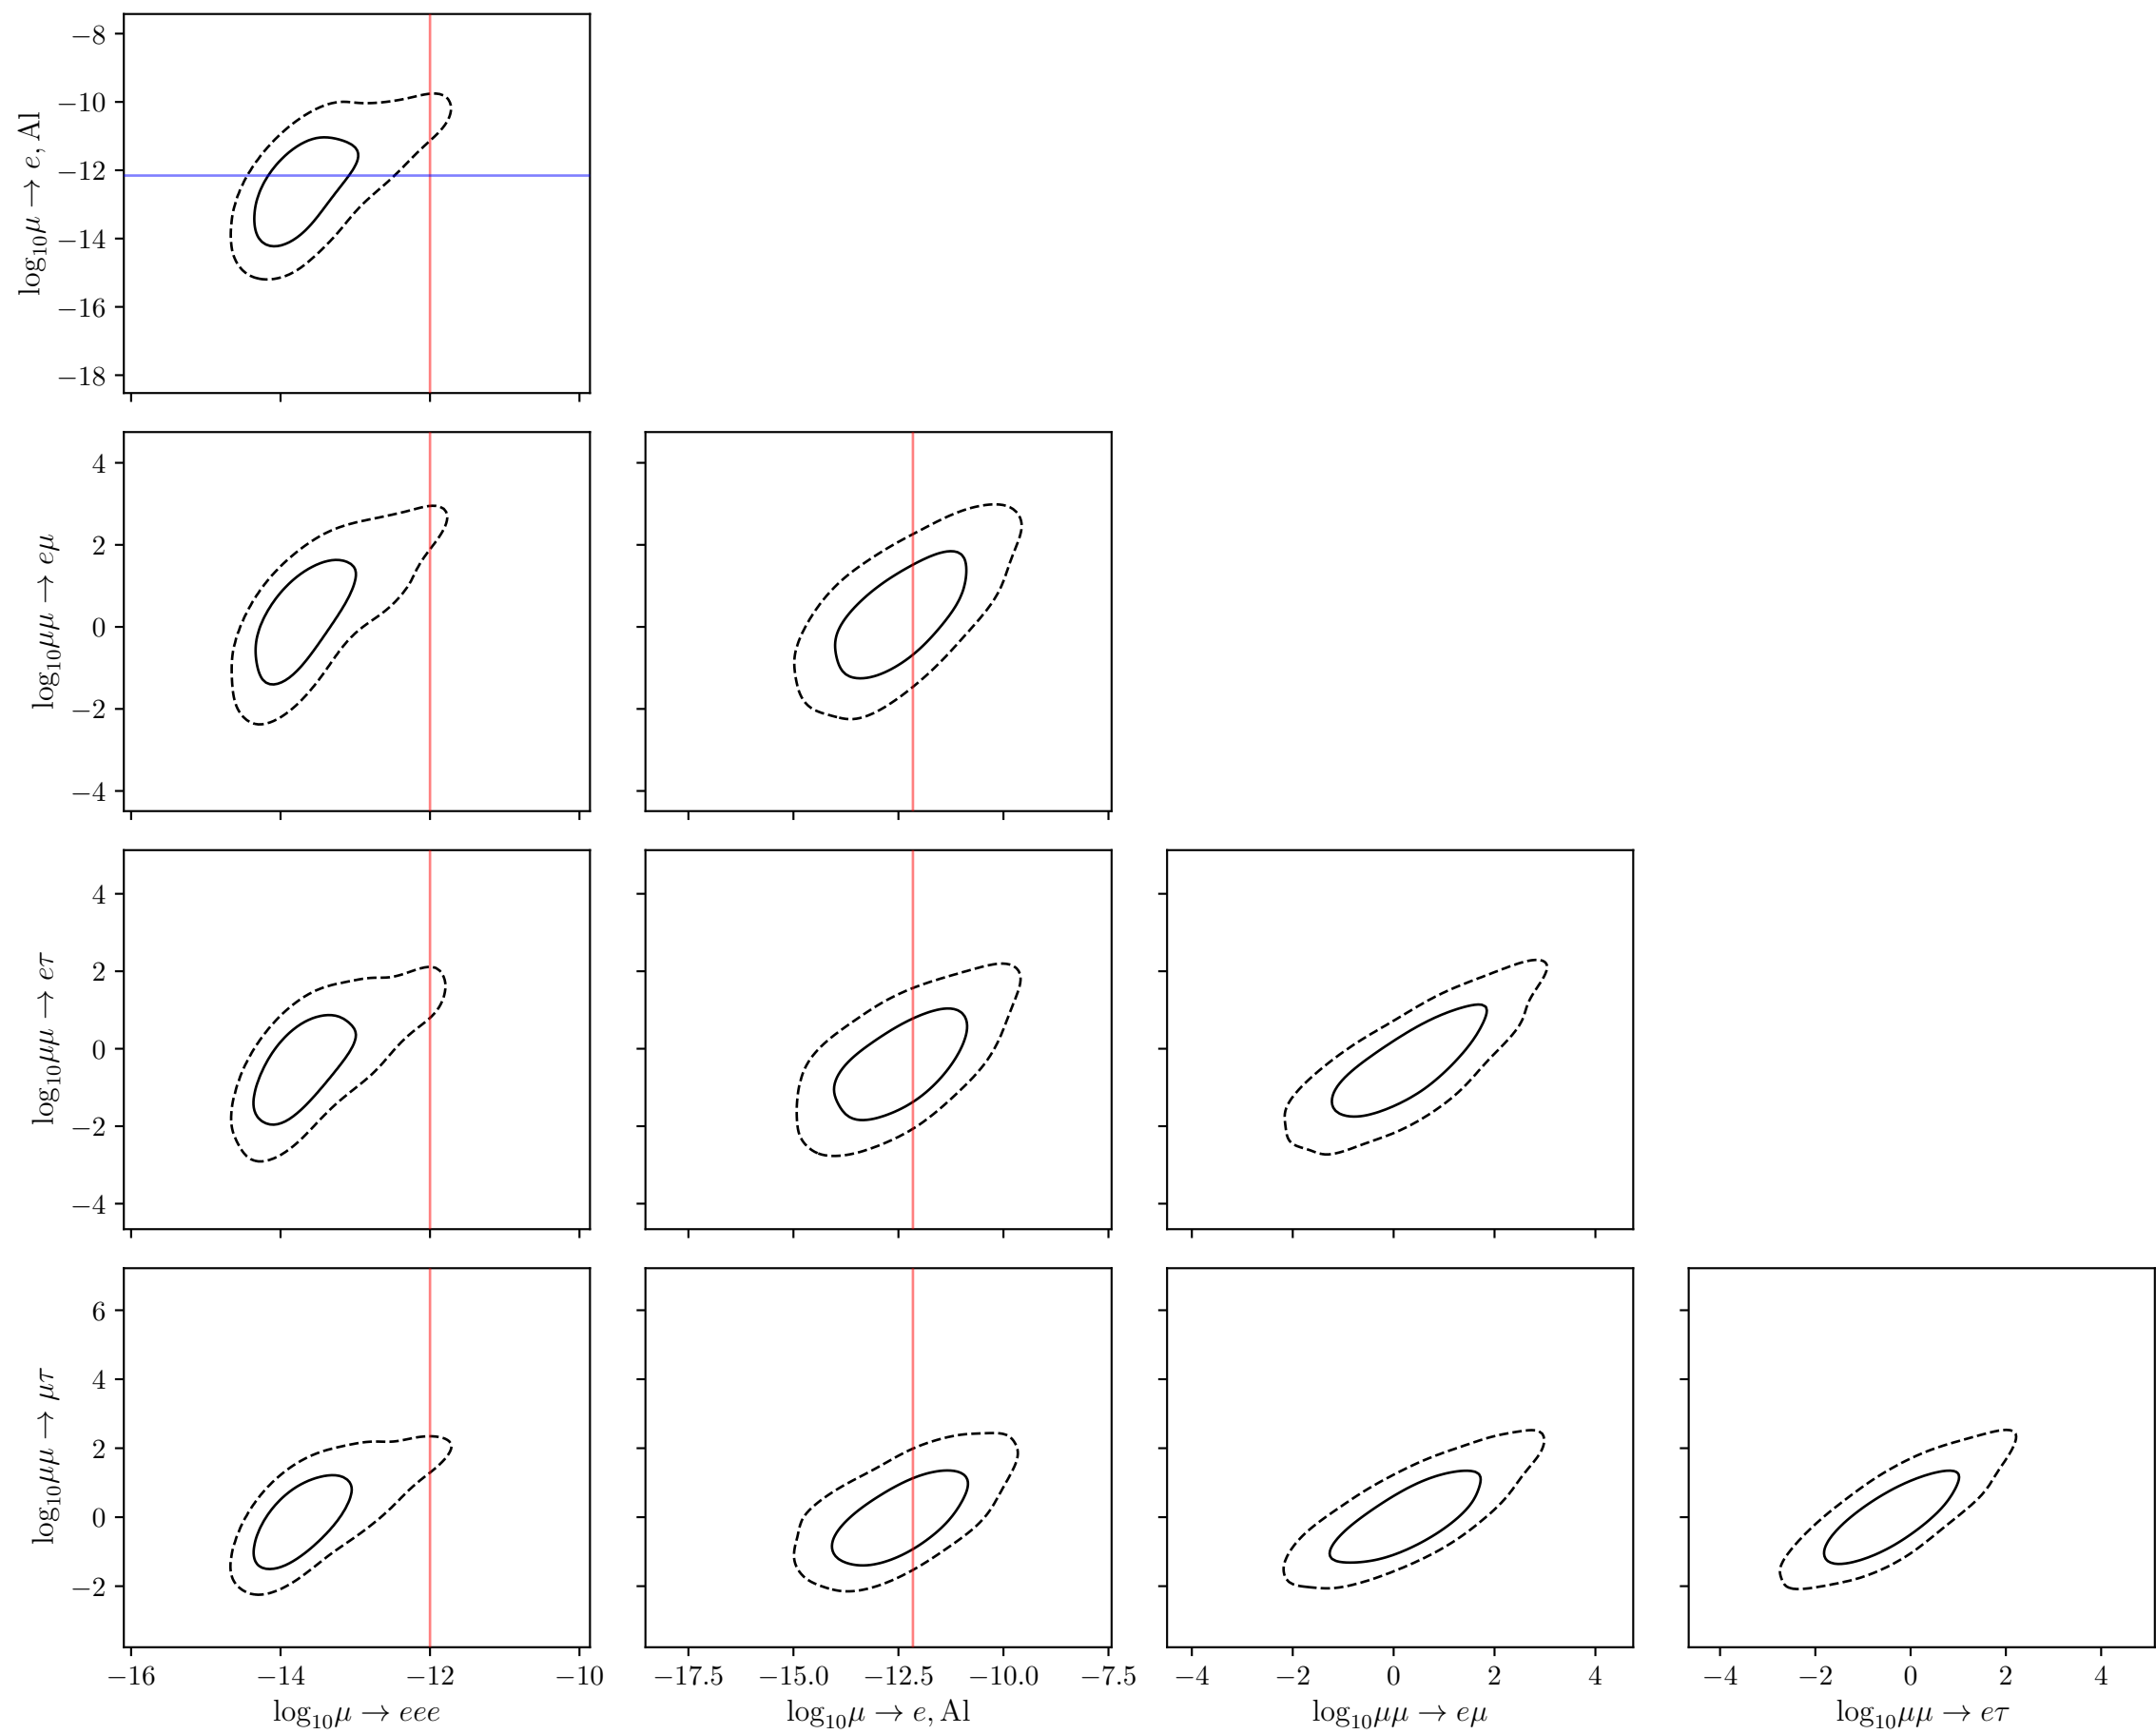

Majorana,  $X_L = \{5, 4, 3\}$ ,  $X_e = \{7, 3, 2\}$ ,

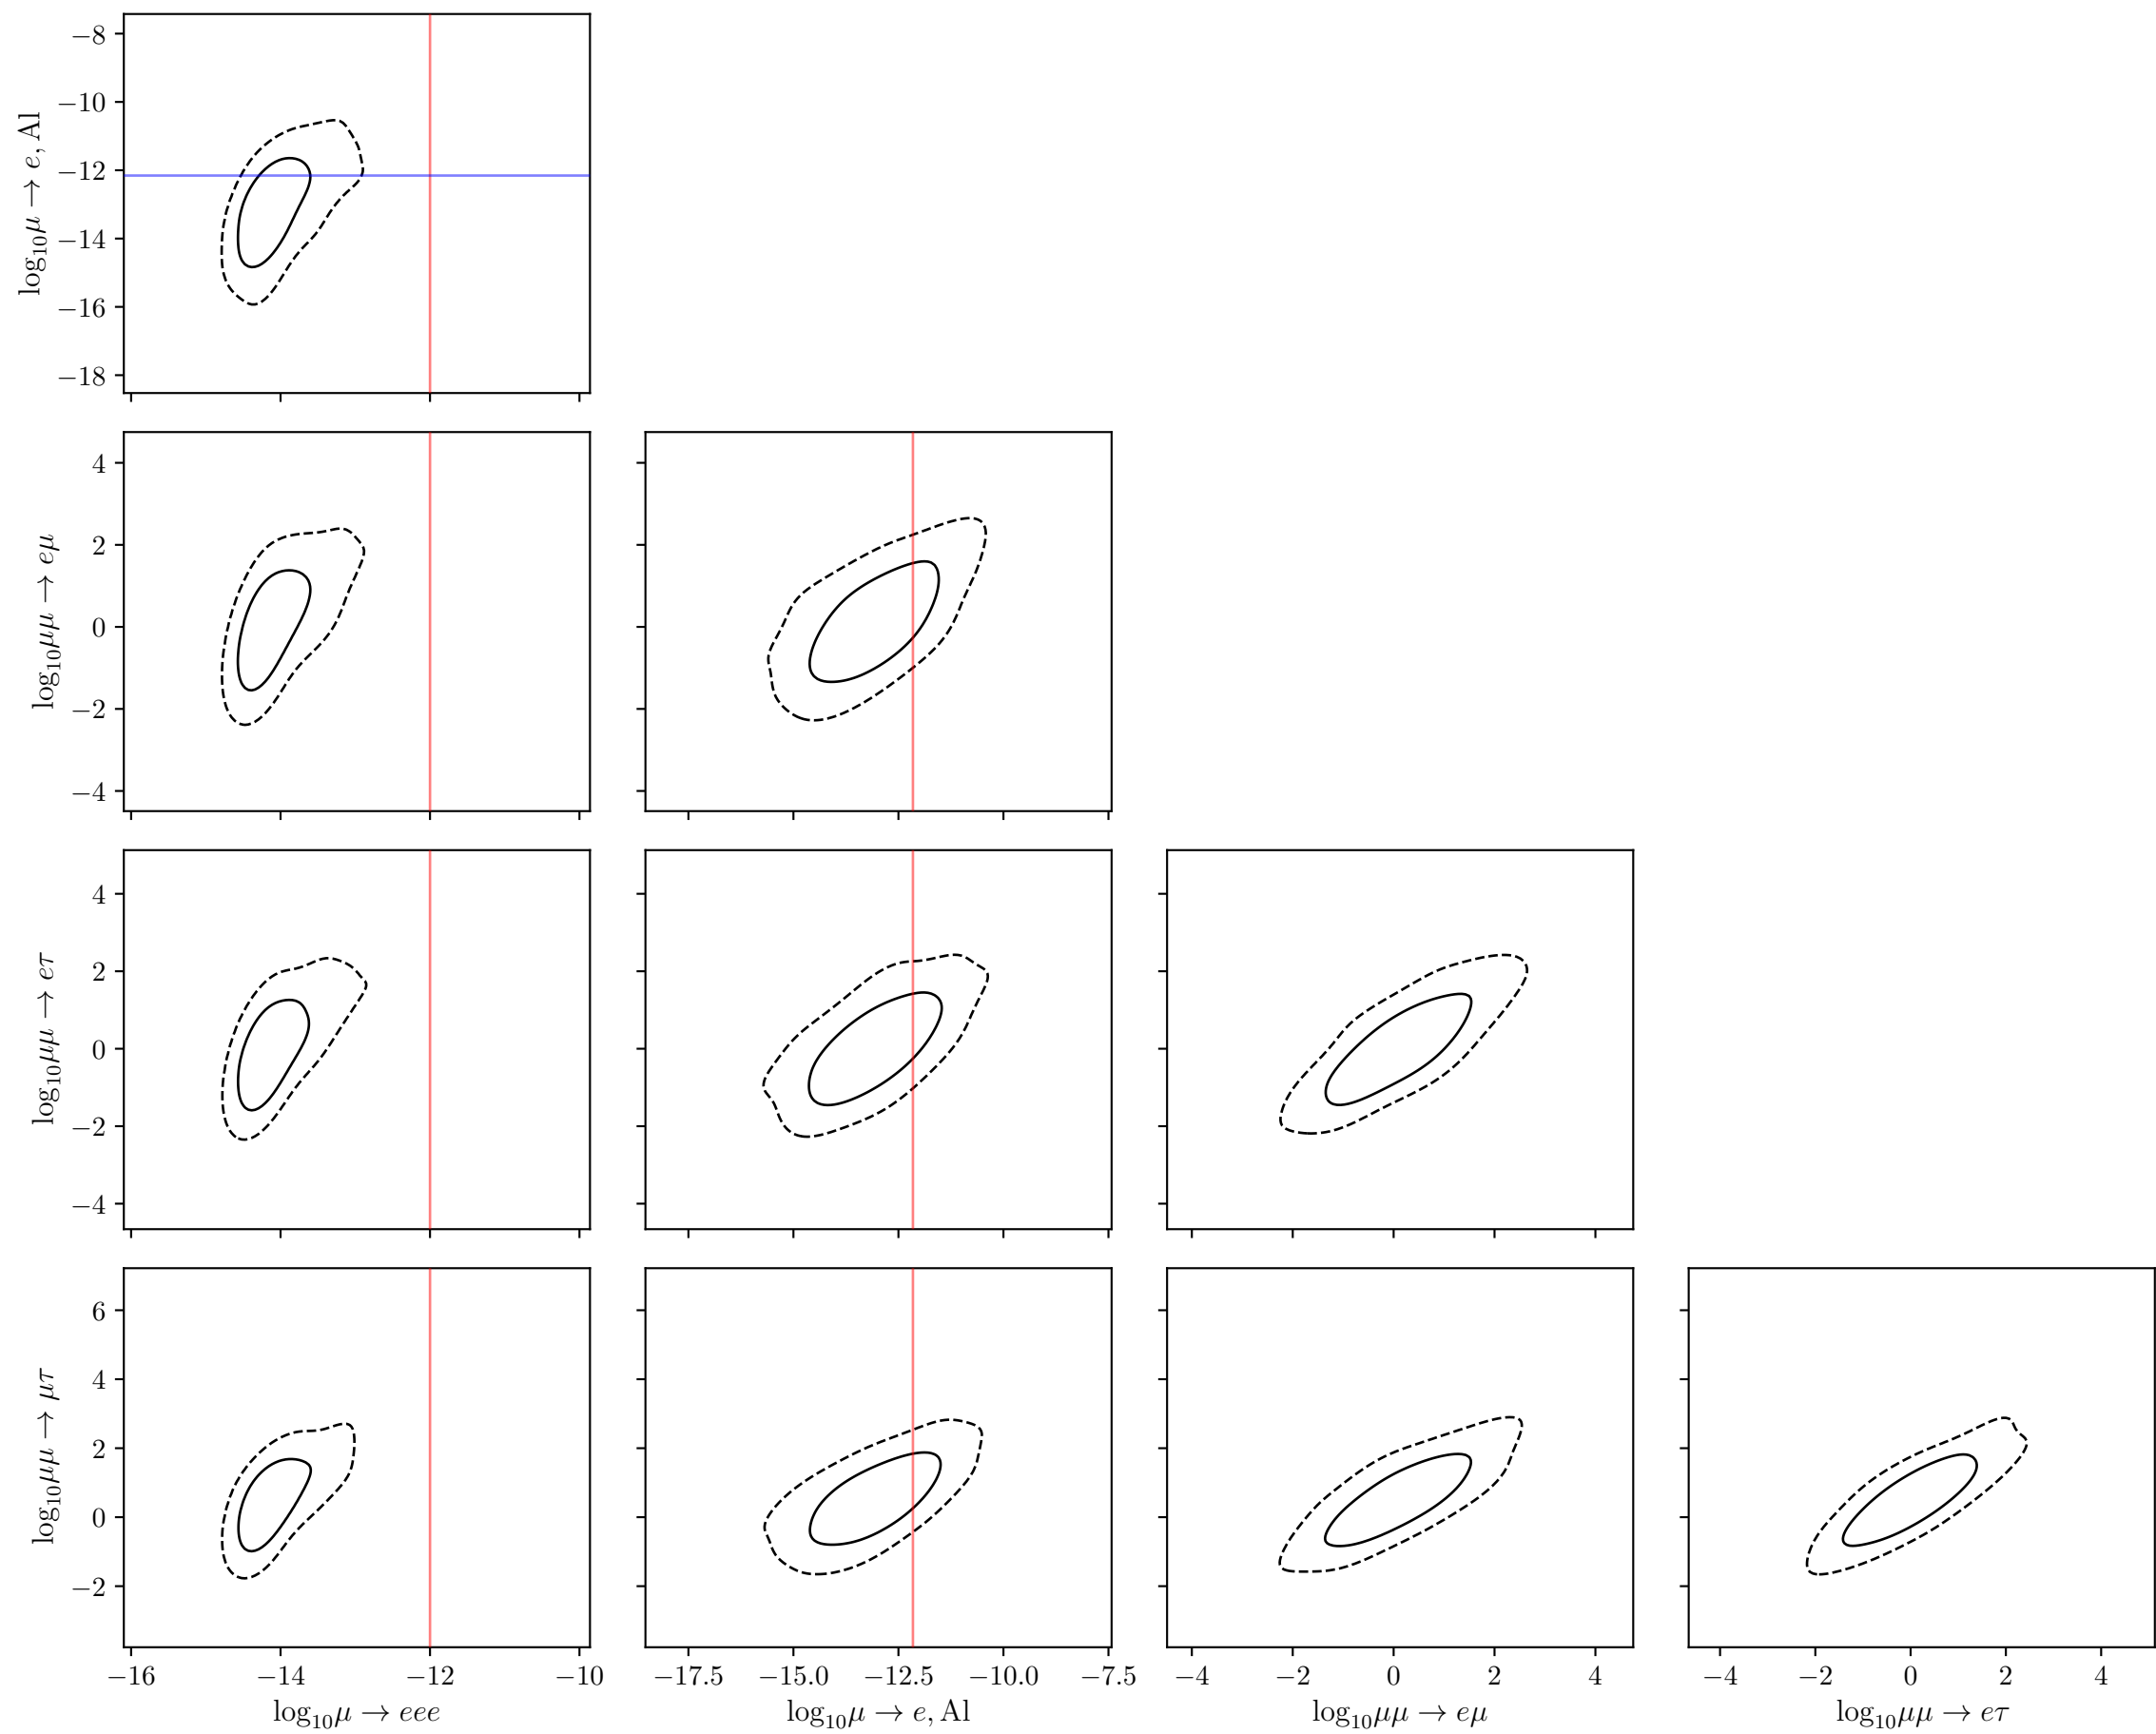

Majorana,  $X_L = \{5, 4, 3\}$ ,  $X_e = \{6, 2, 1\}$ ,

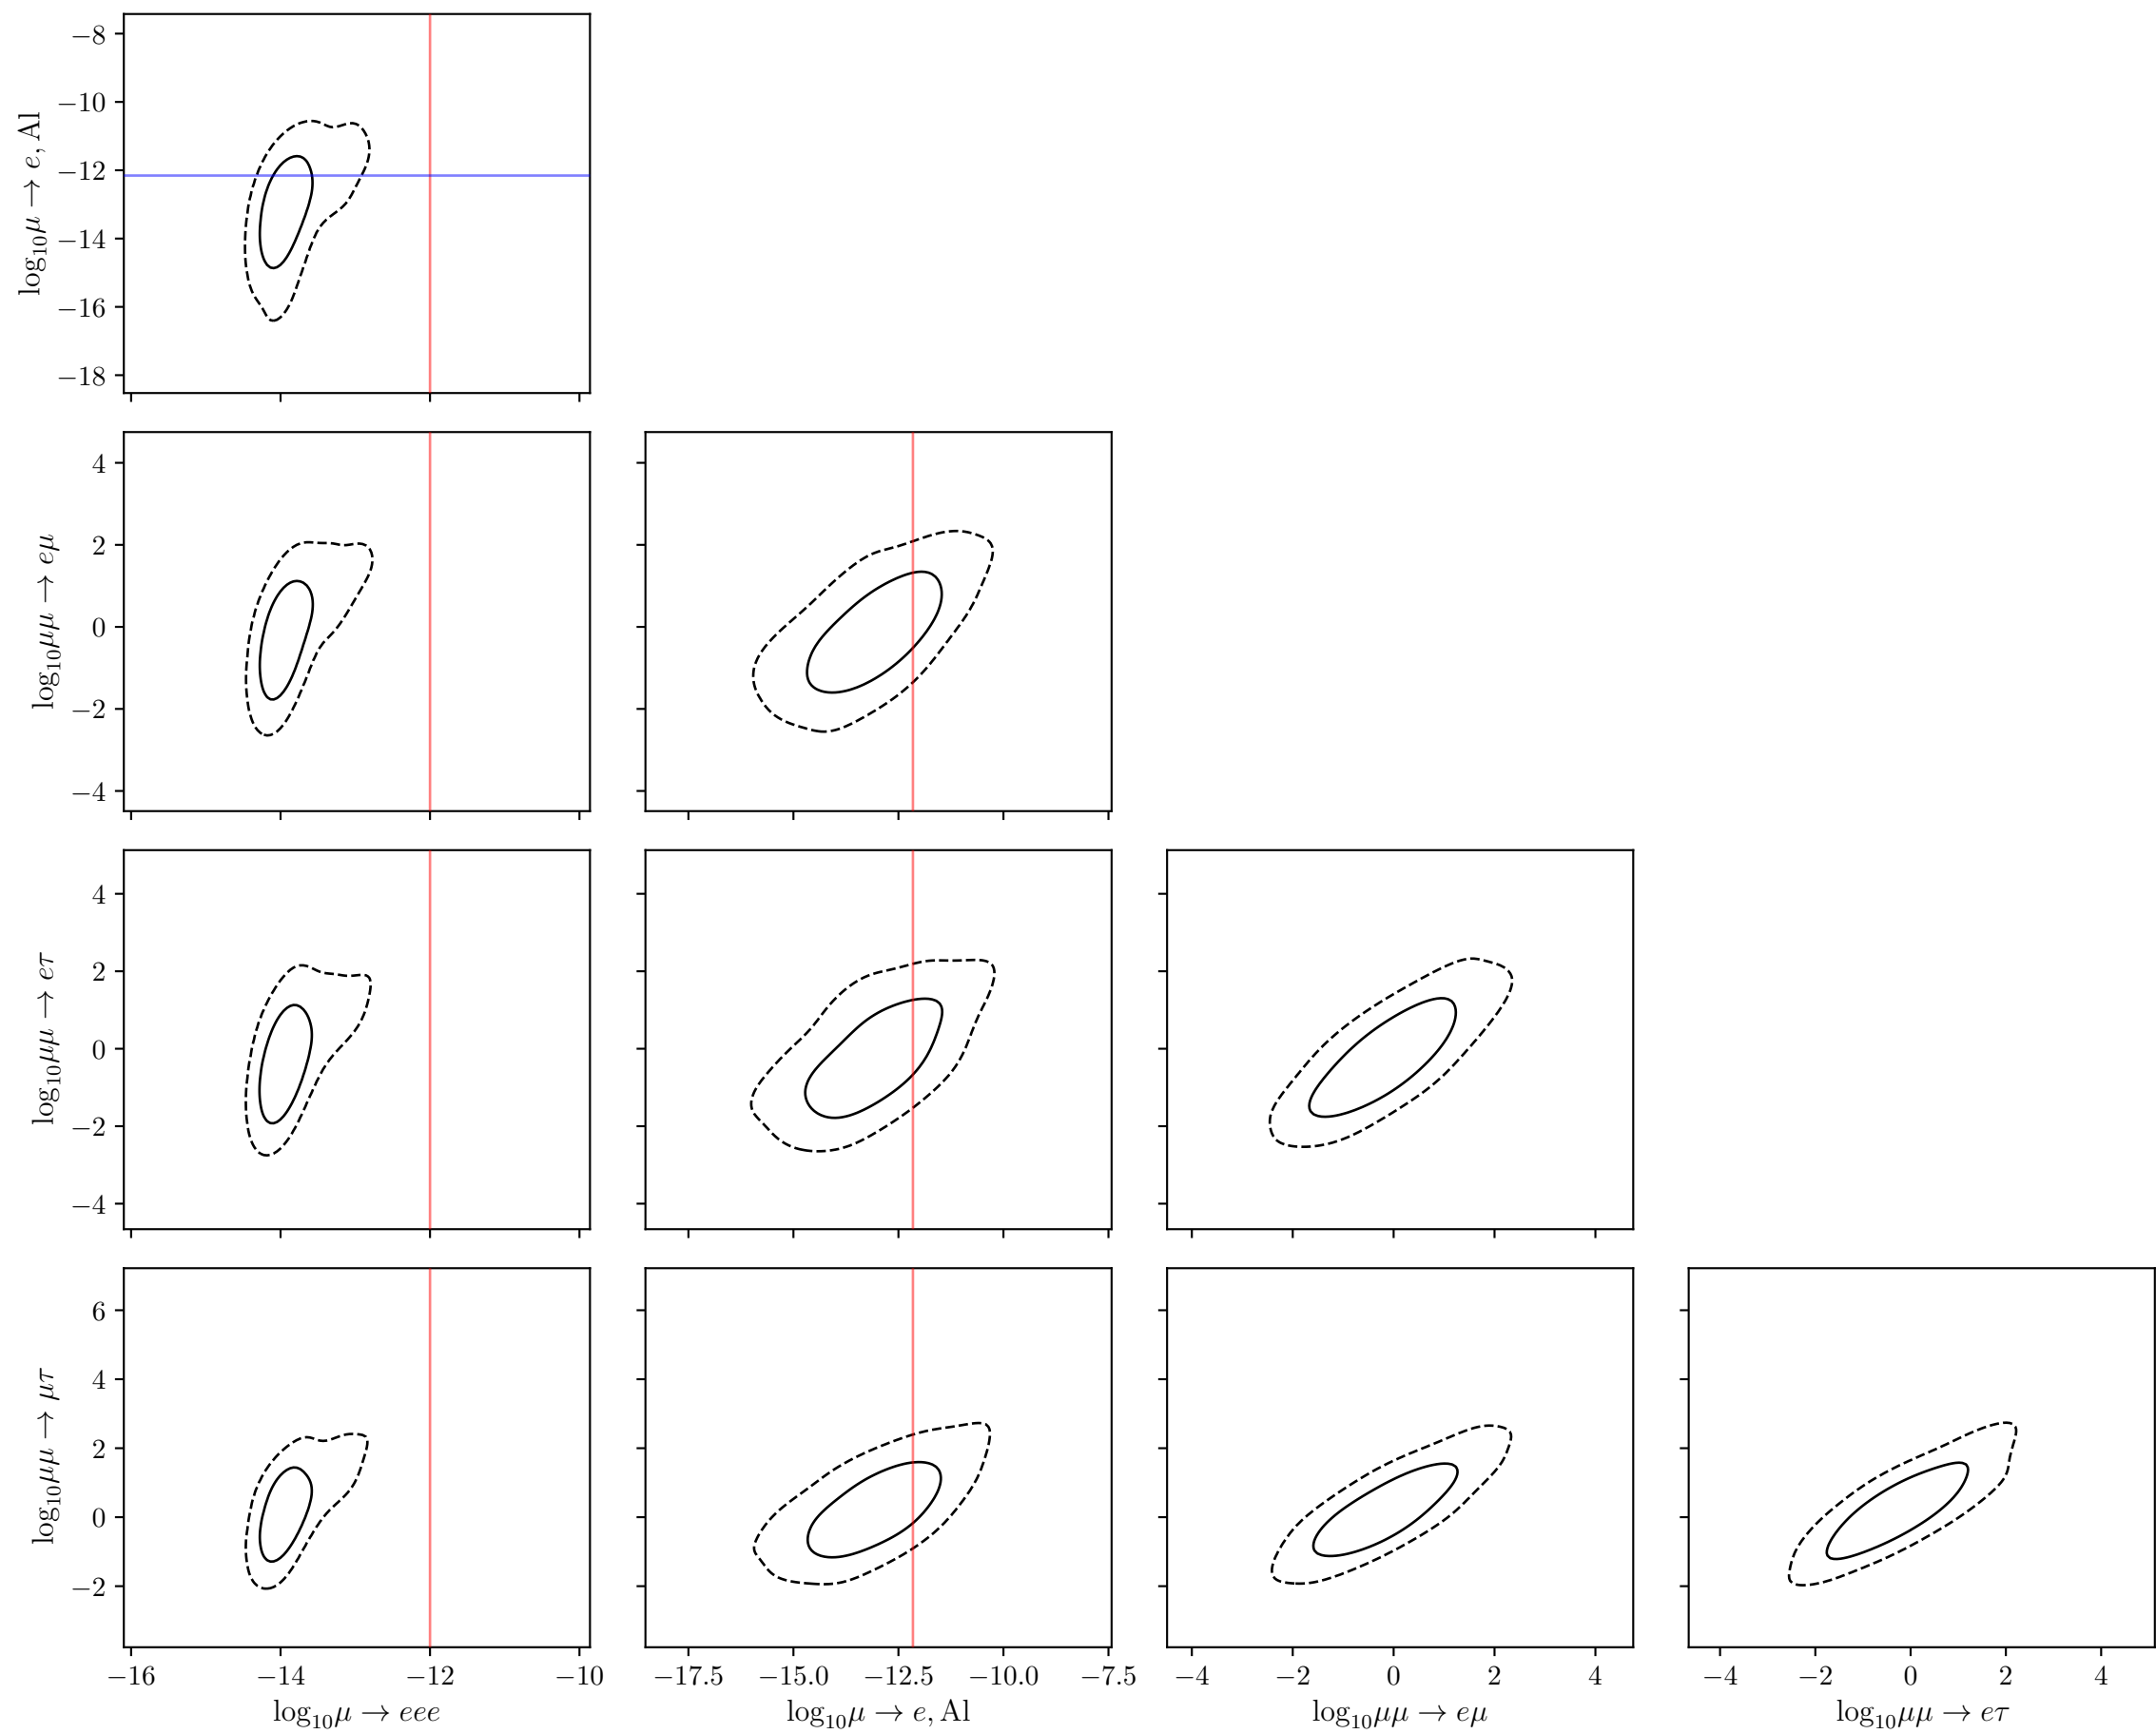

Majorana,  $X_L = \{1, 1, 0\}$ ,  $X_e = \{-6, 3, 7\}$ ,

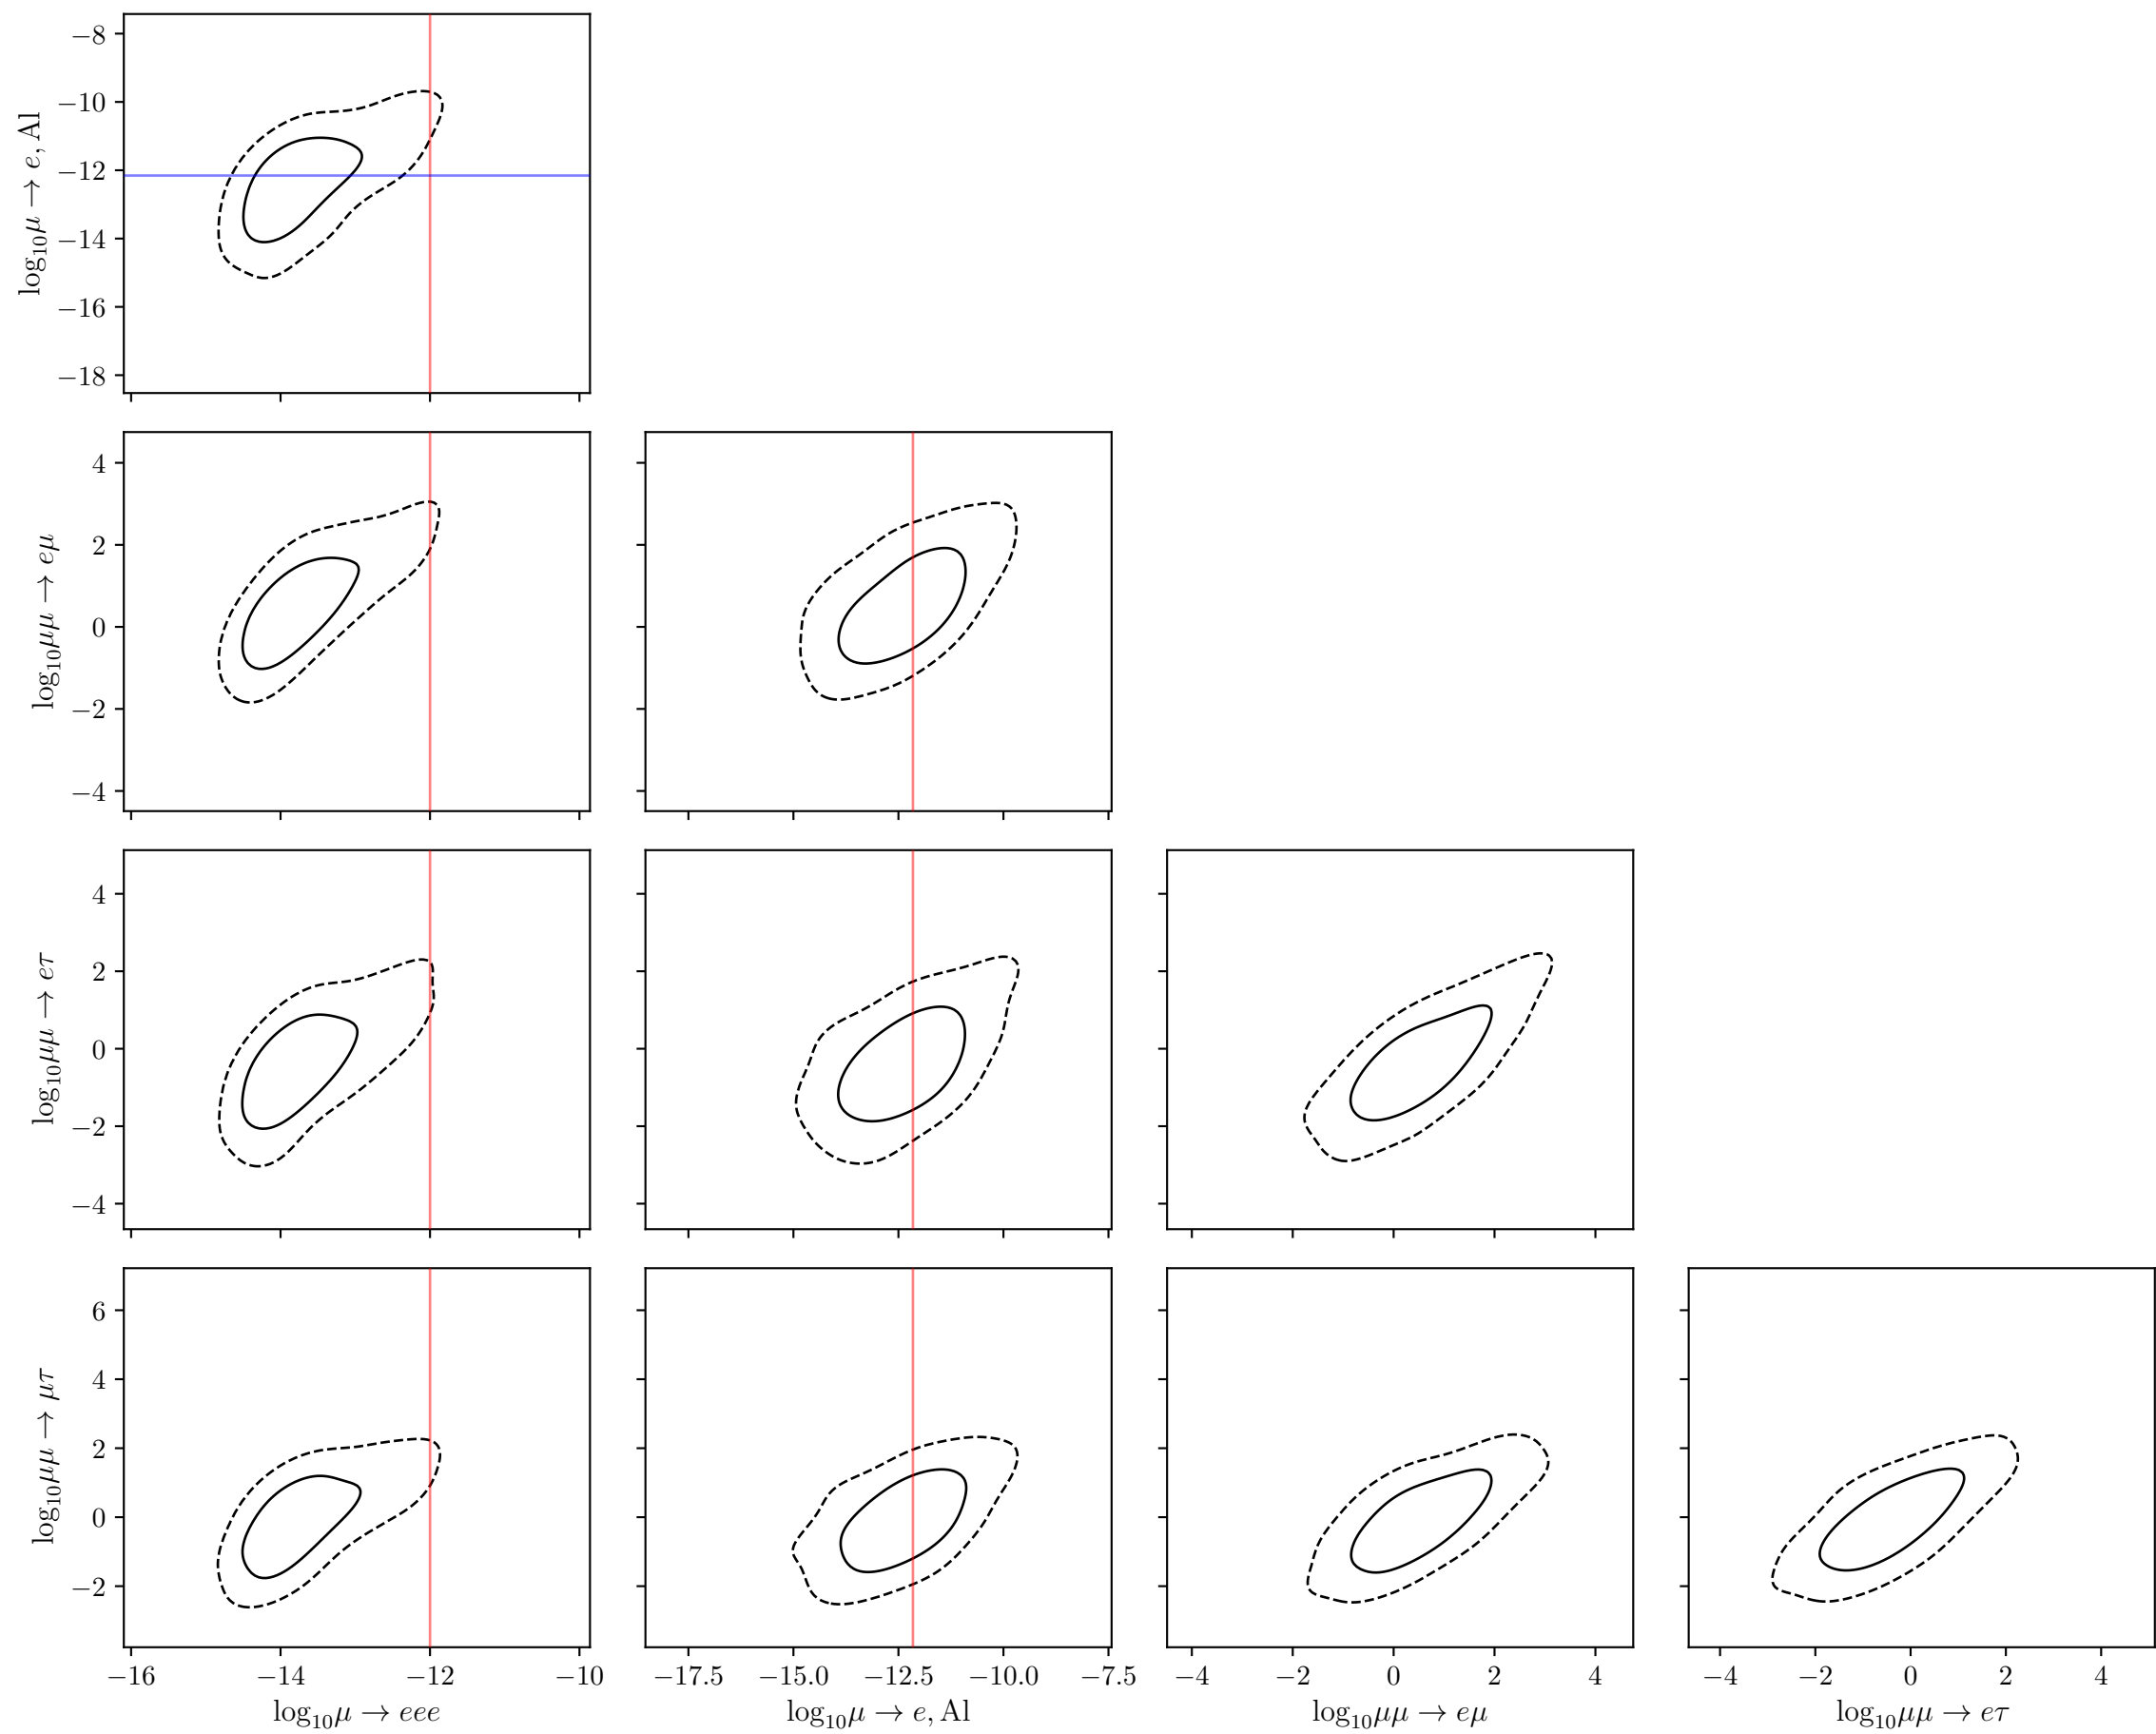

Majorana,  $X_L = \{5, 5, 4\}$ ,  $X_e = \{5, 1, 0\}$ ,

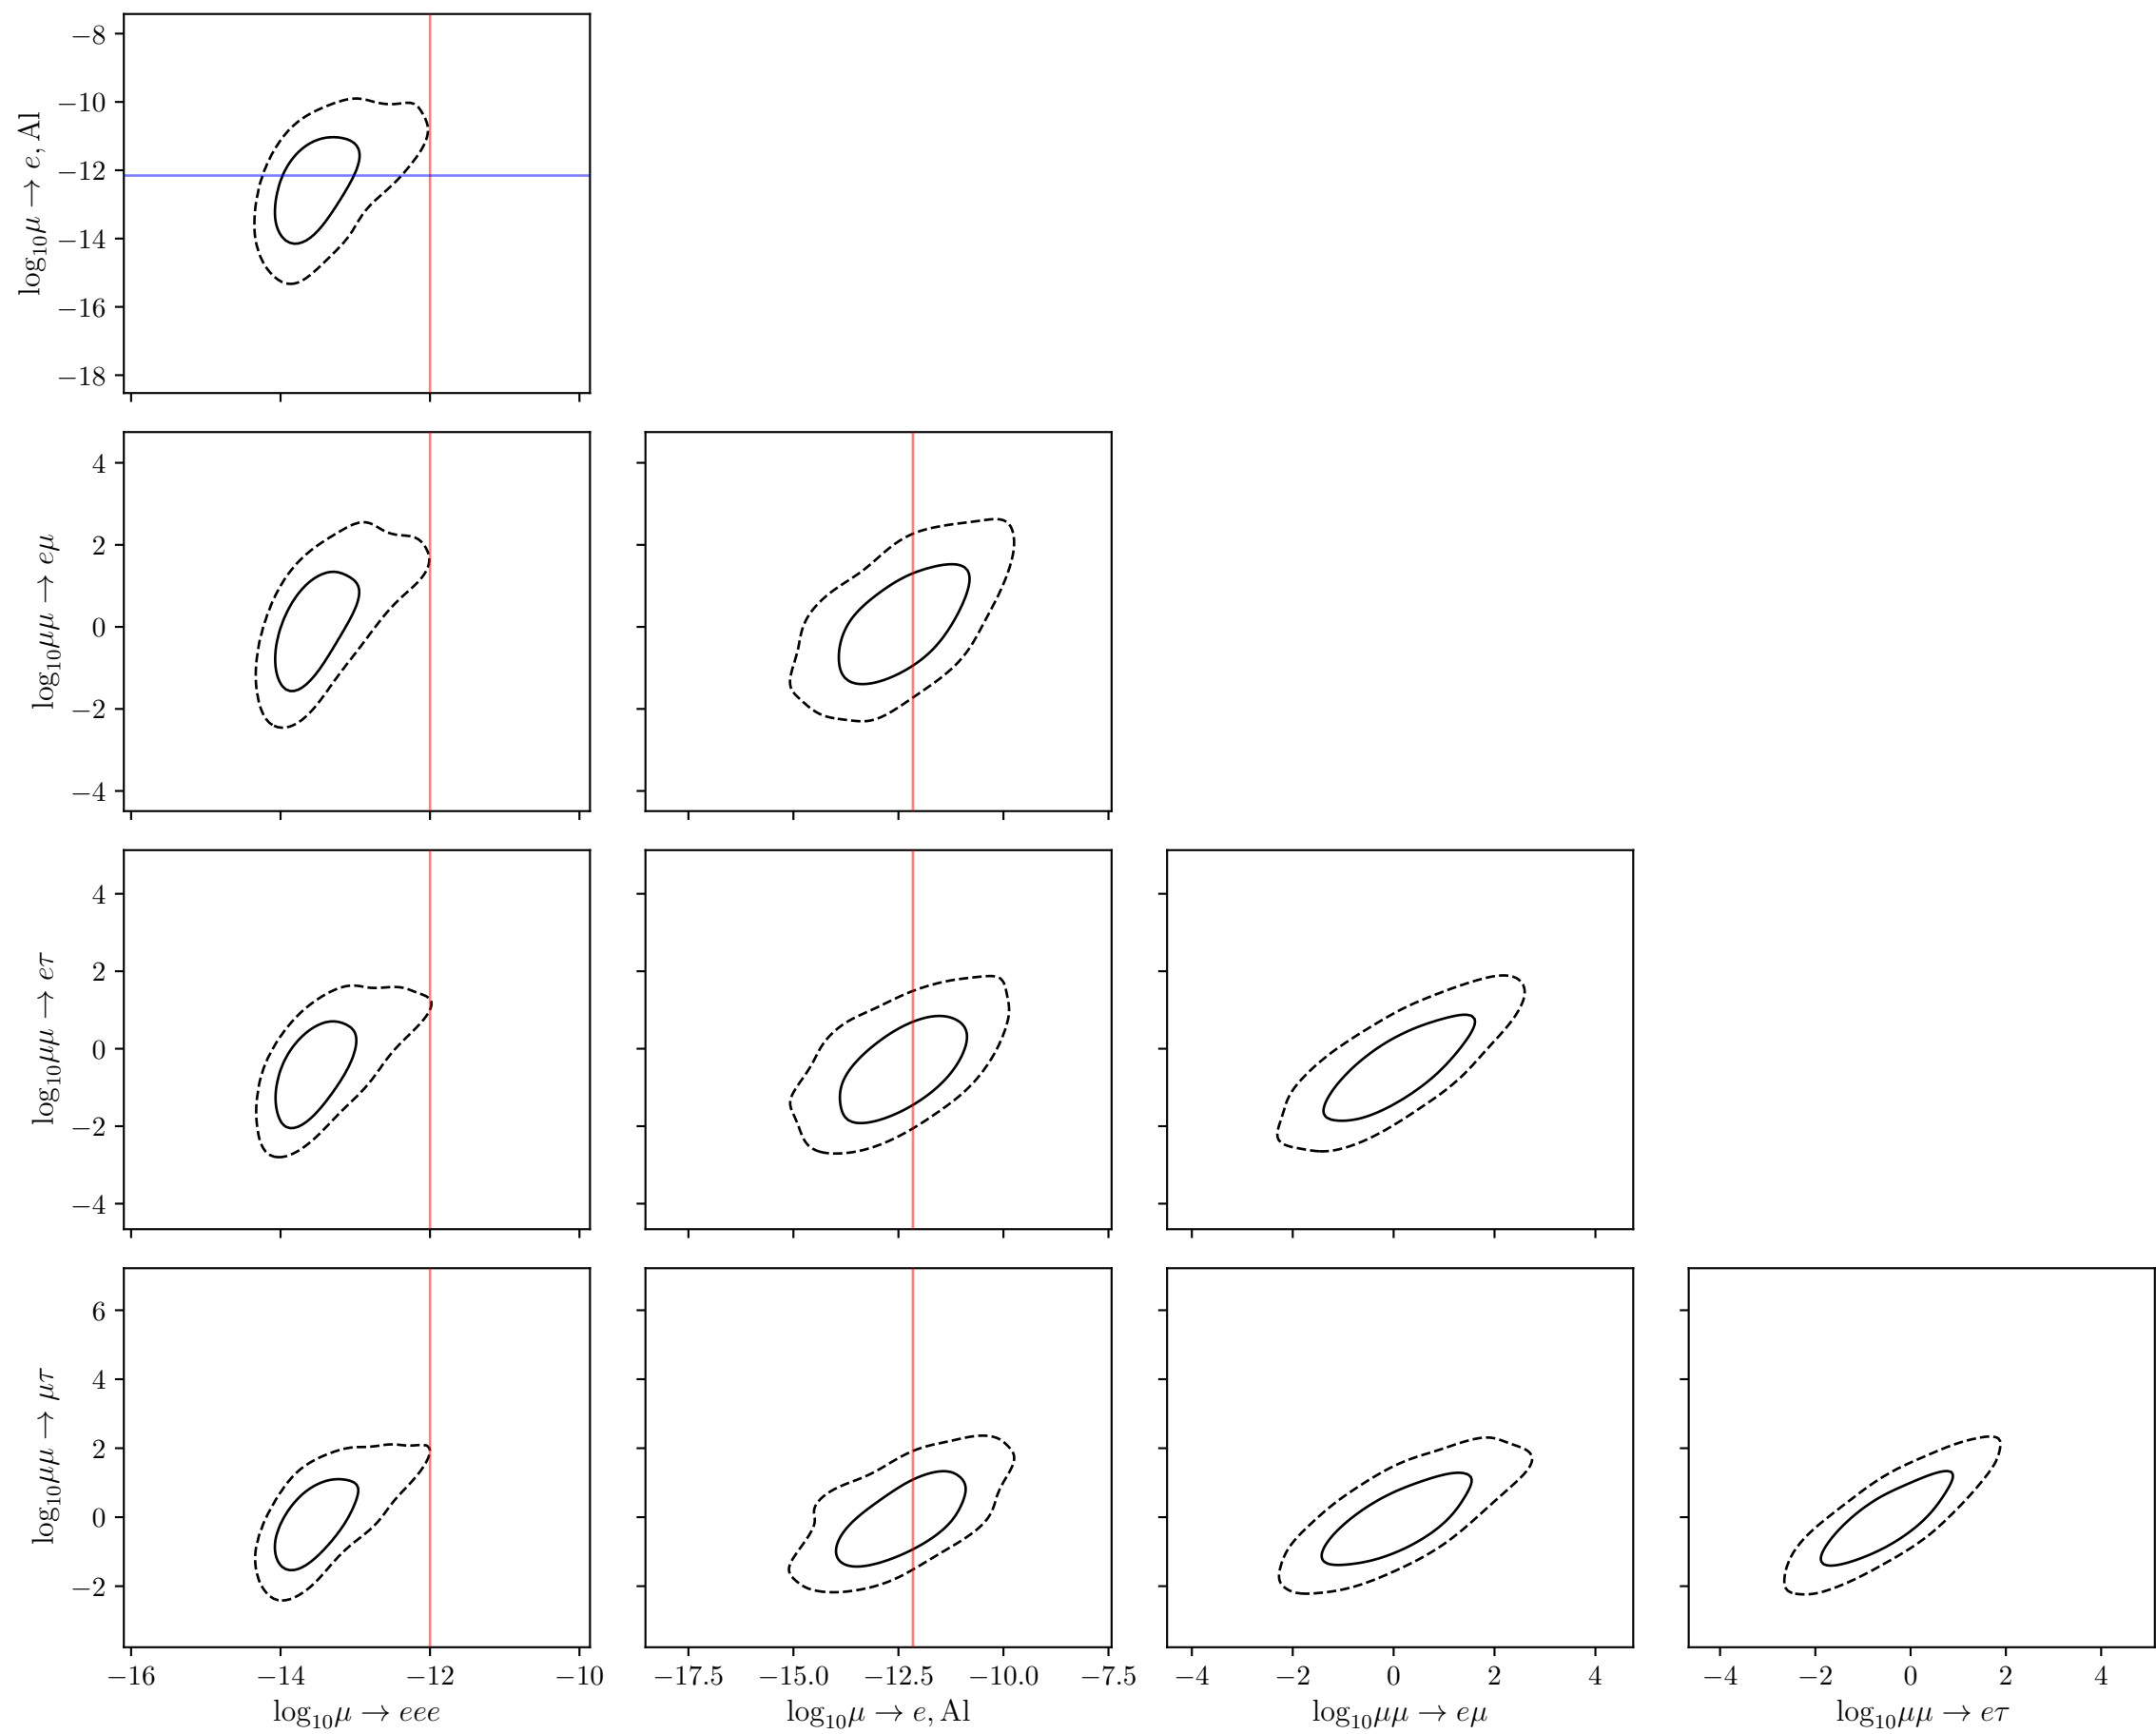

Majorana,  $X_L = \{7, 6, 5\}$ ,  $X_e = \{5, 1, 0\}$ ,

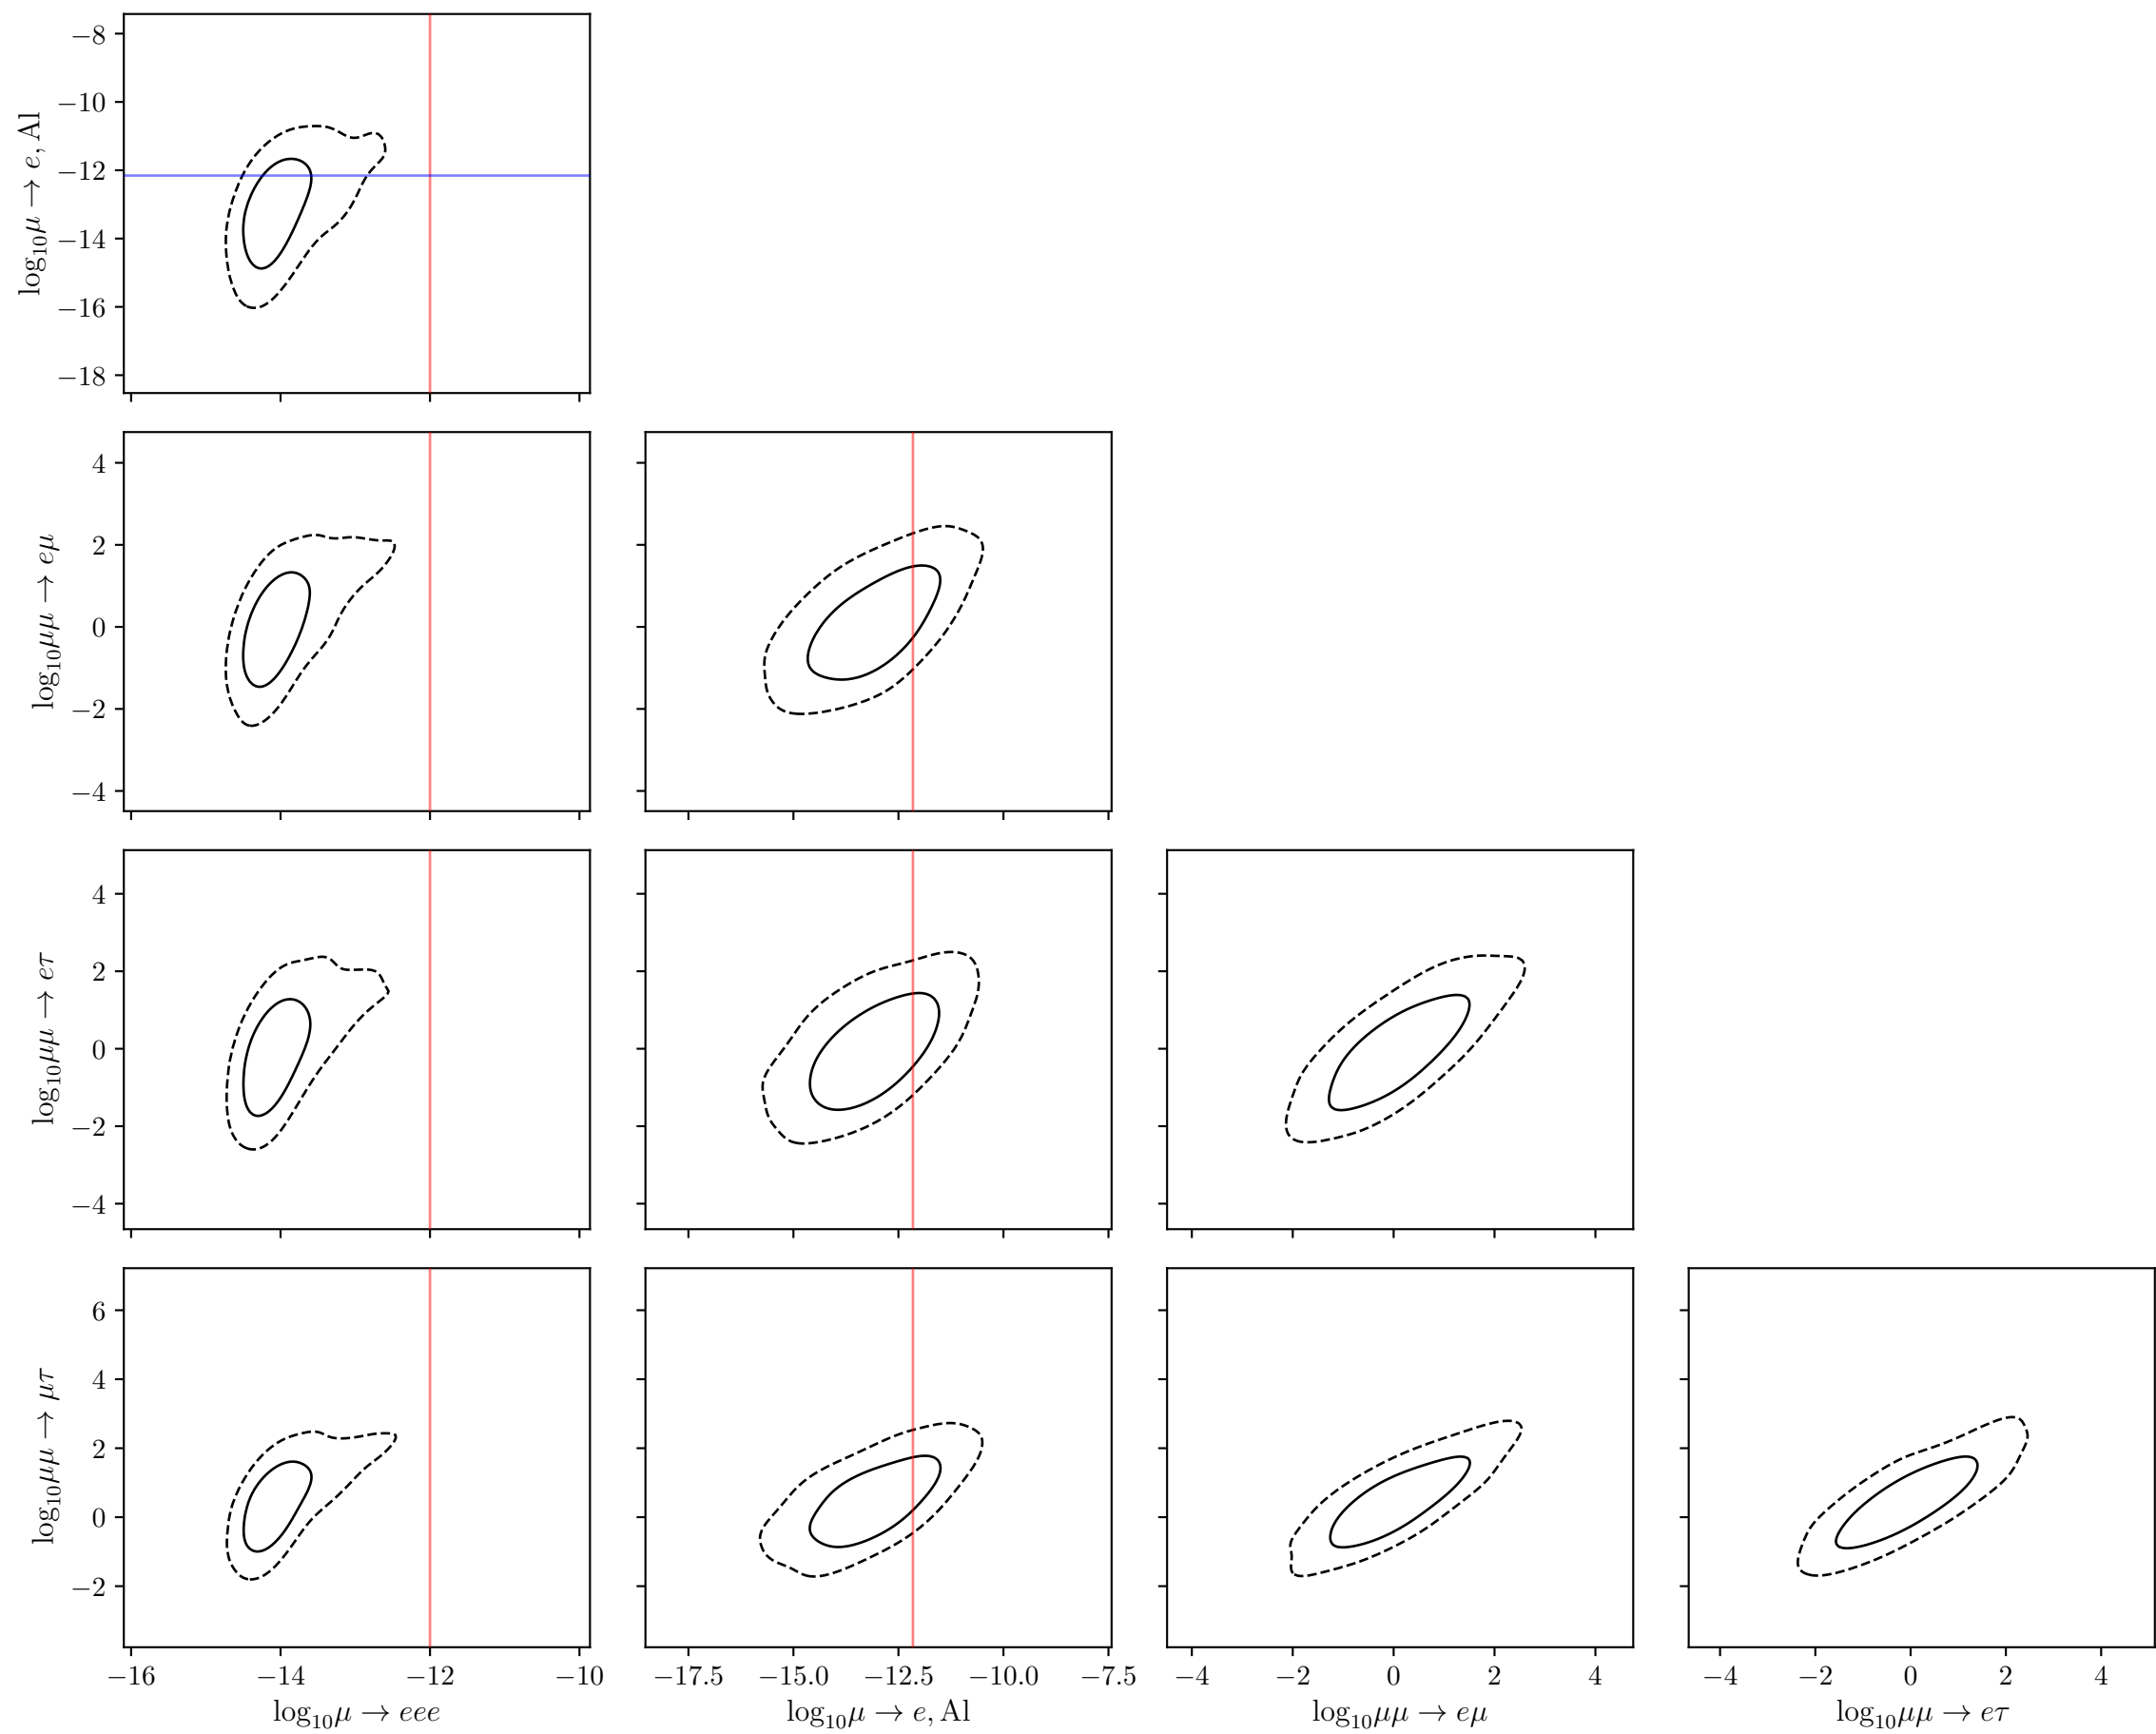

Majorana,  $X_L = \{2, 2, 1\}$ ,  $X_e = \{6, 3, 2\}$ ,

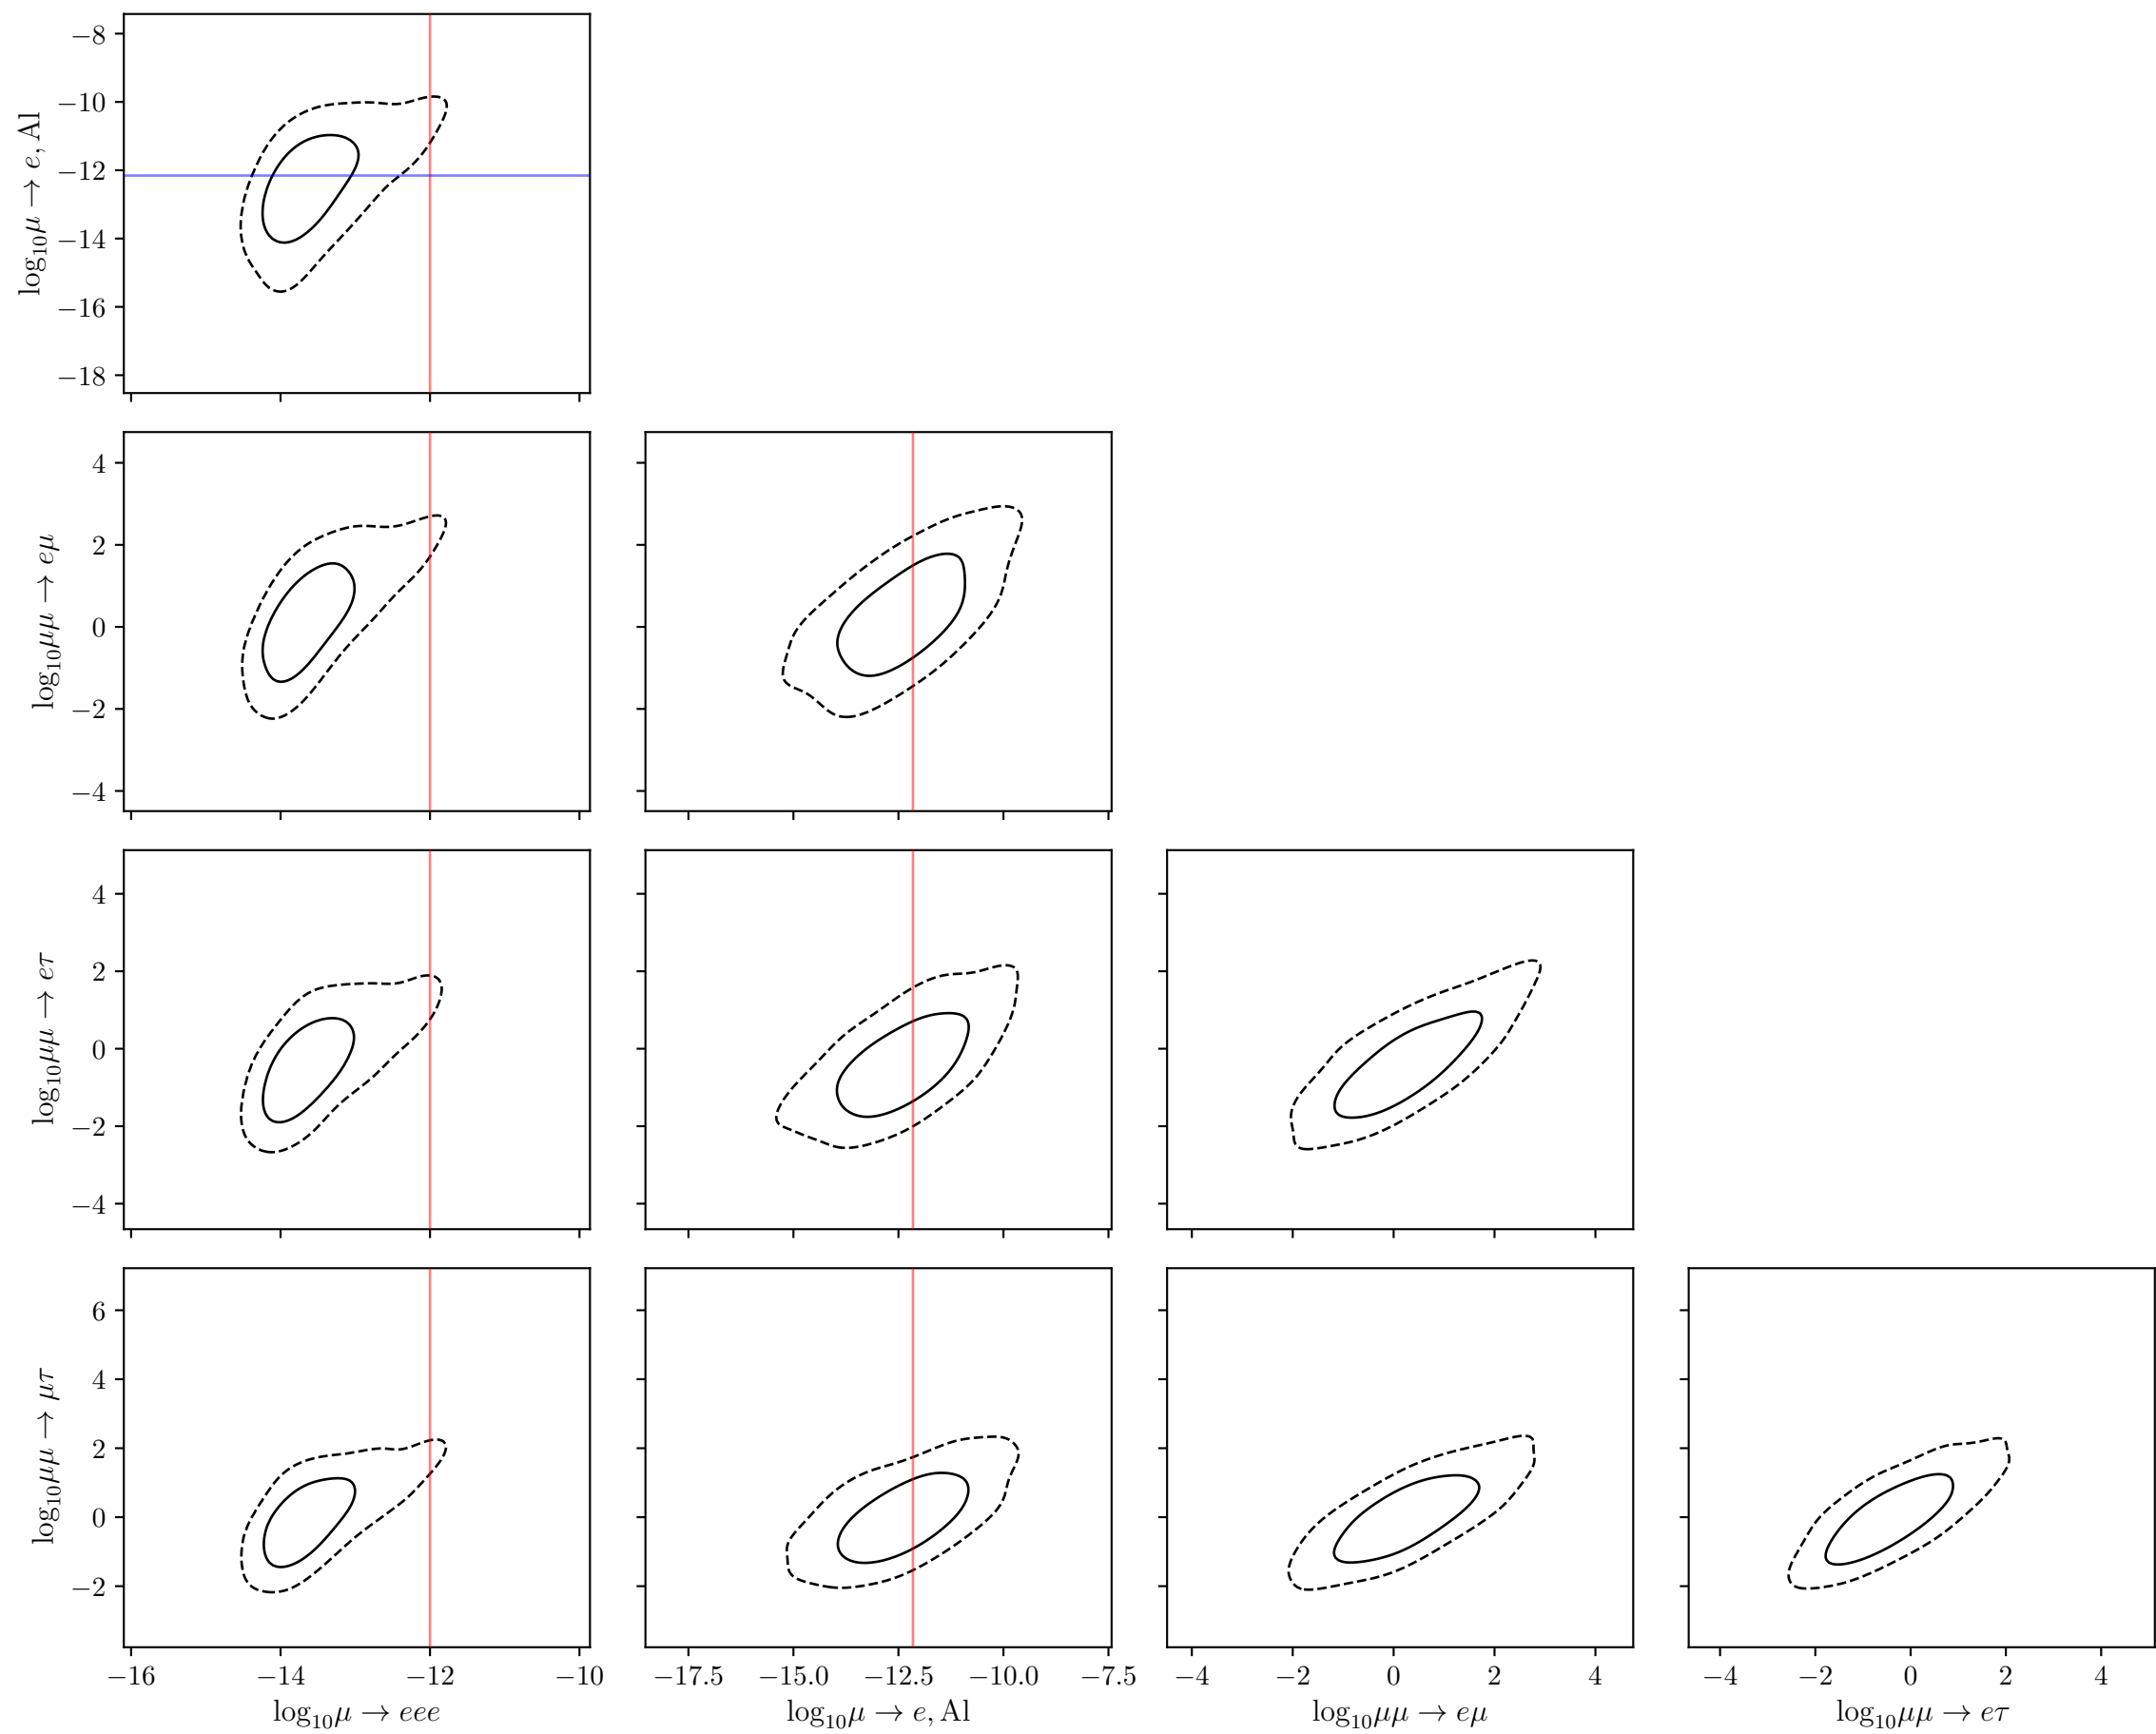

Majorana,  $X_L = \{6, 6, 5\}$ ,  $X_e = \{-1, 0, 4\}$ ,

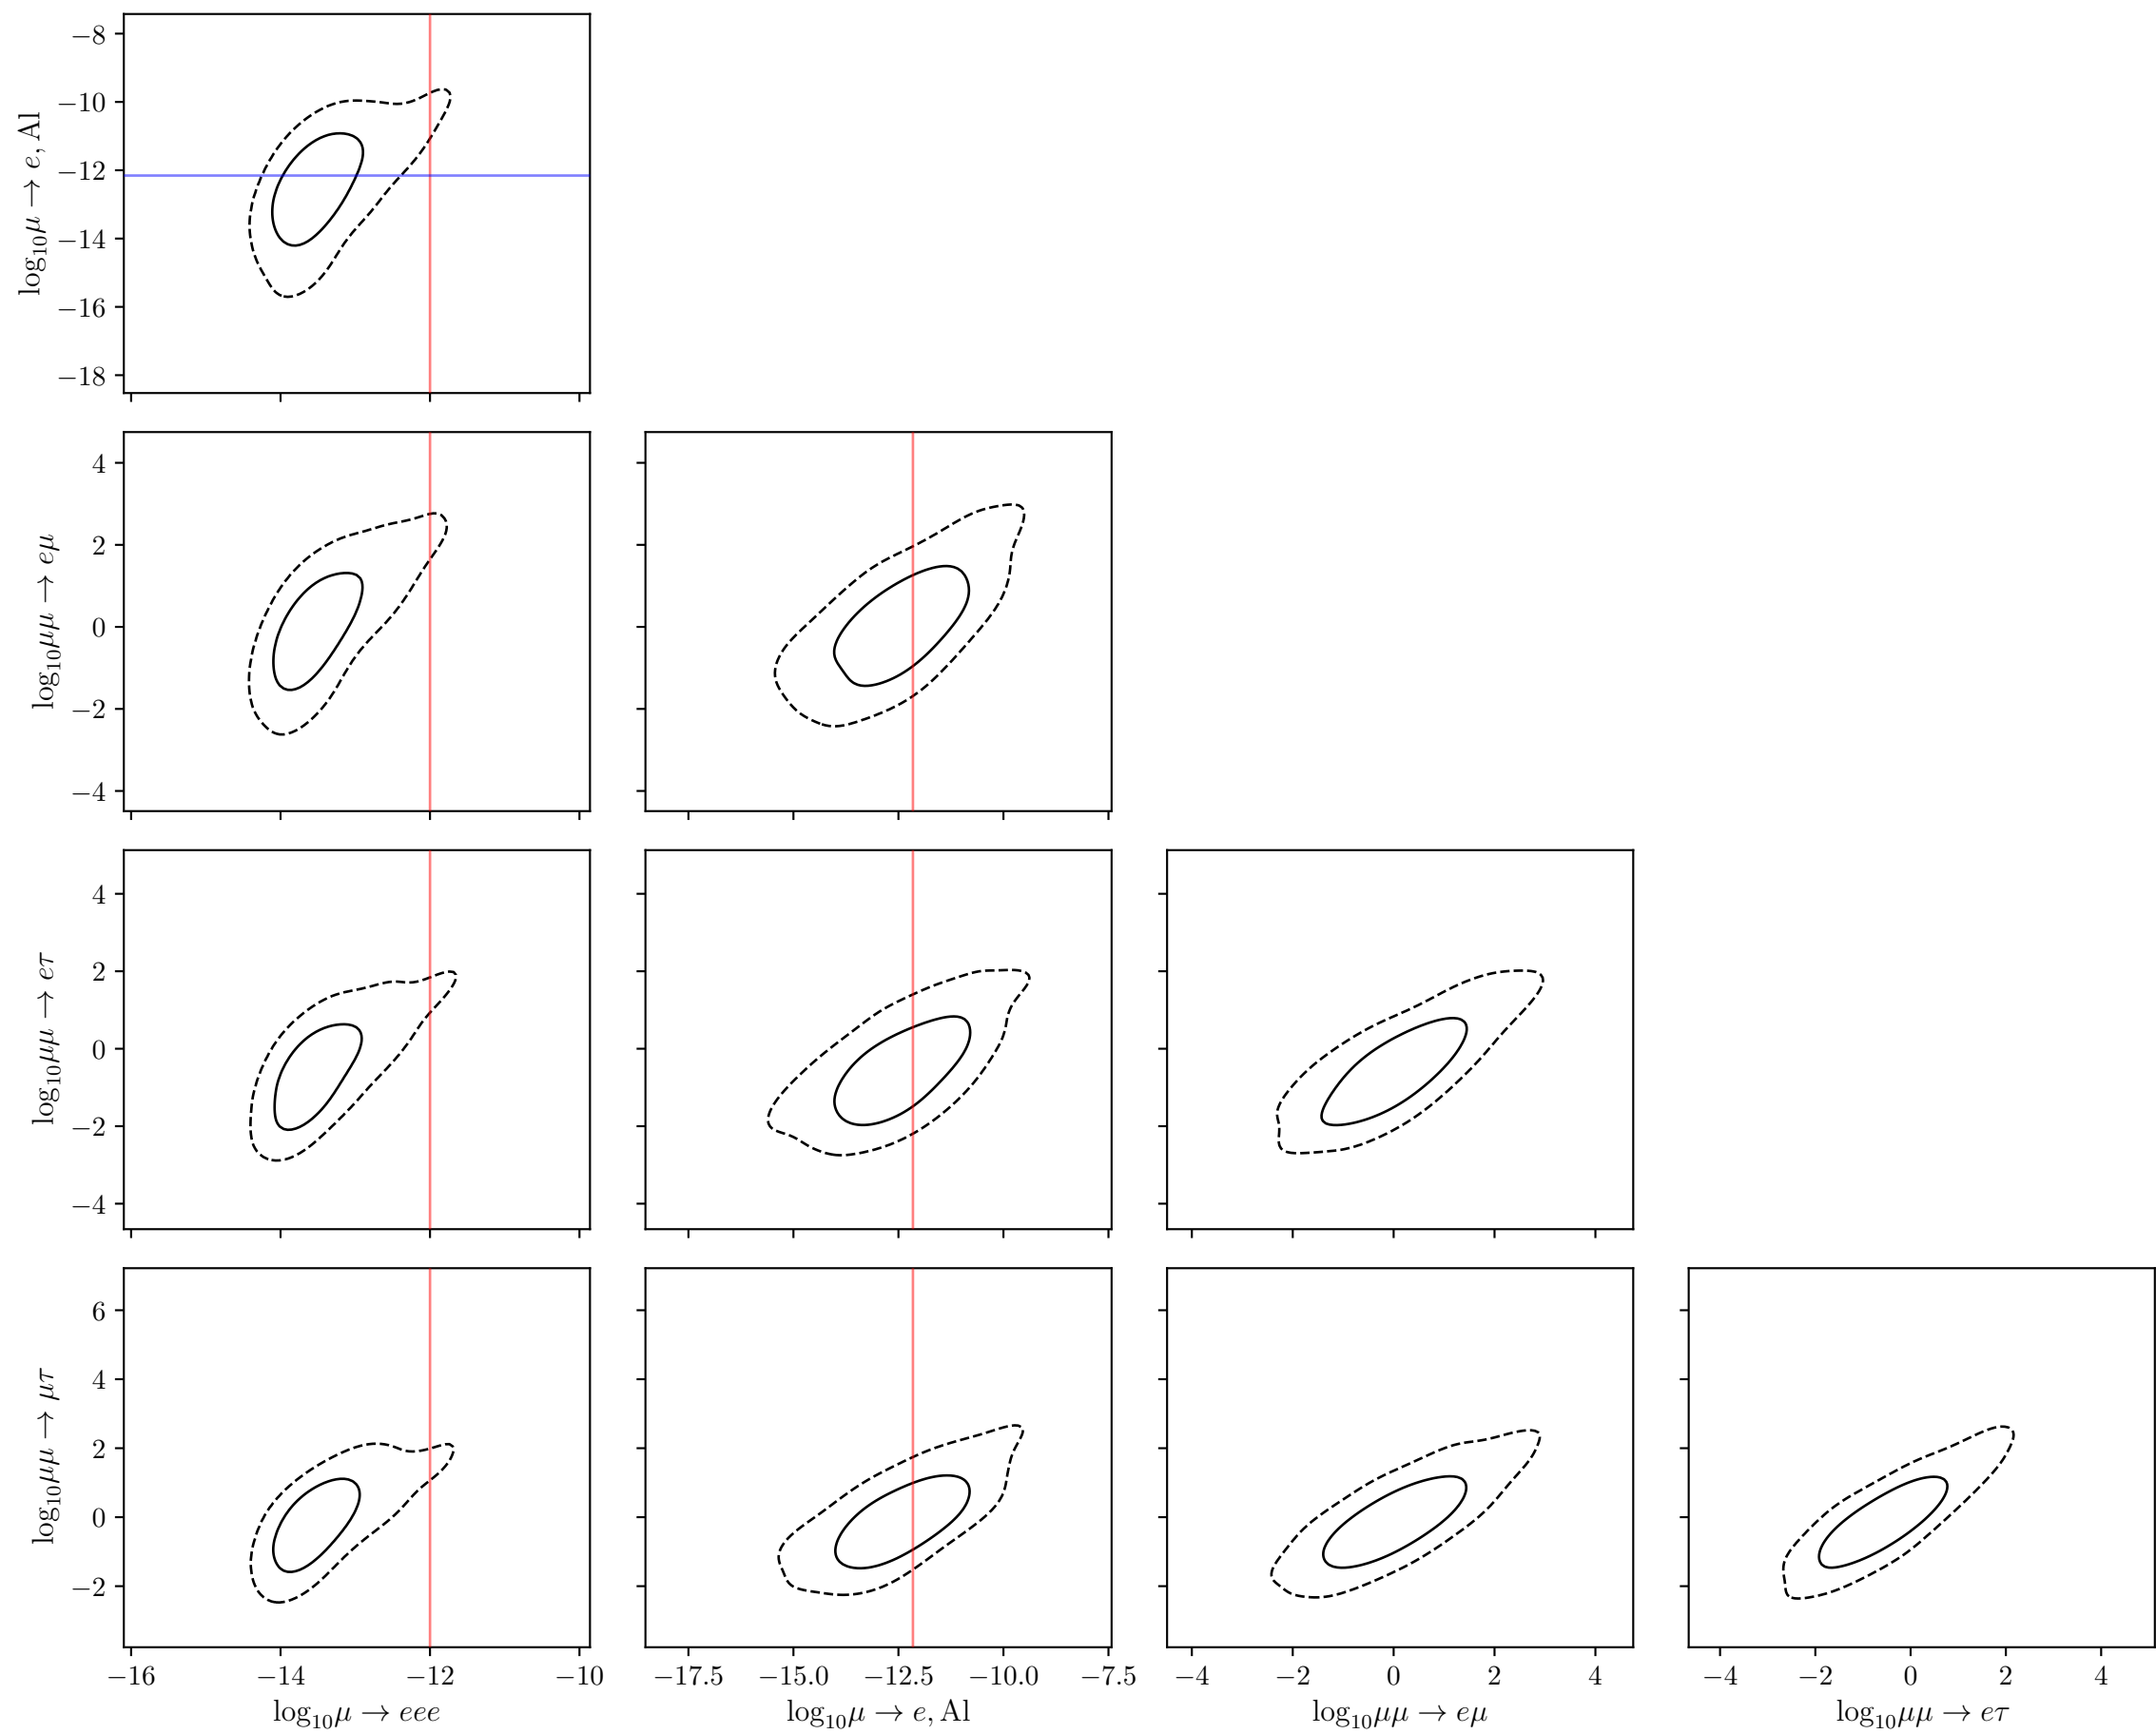



Majorana,  $X_L = \{4, 3, 2\}$ ,  $X_e = \{6, 3, 2\}$ ,

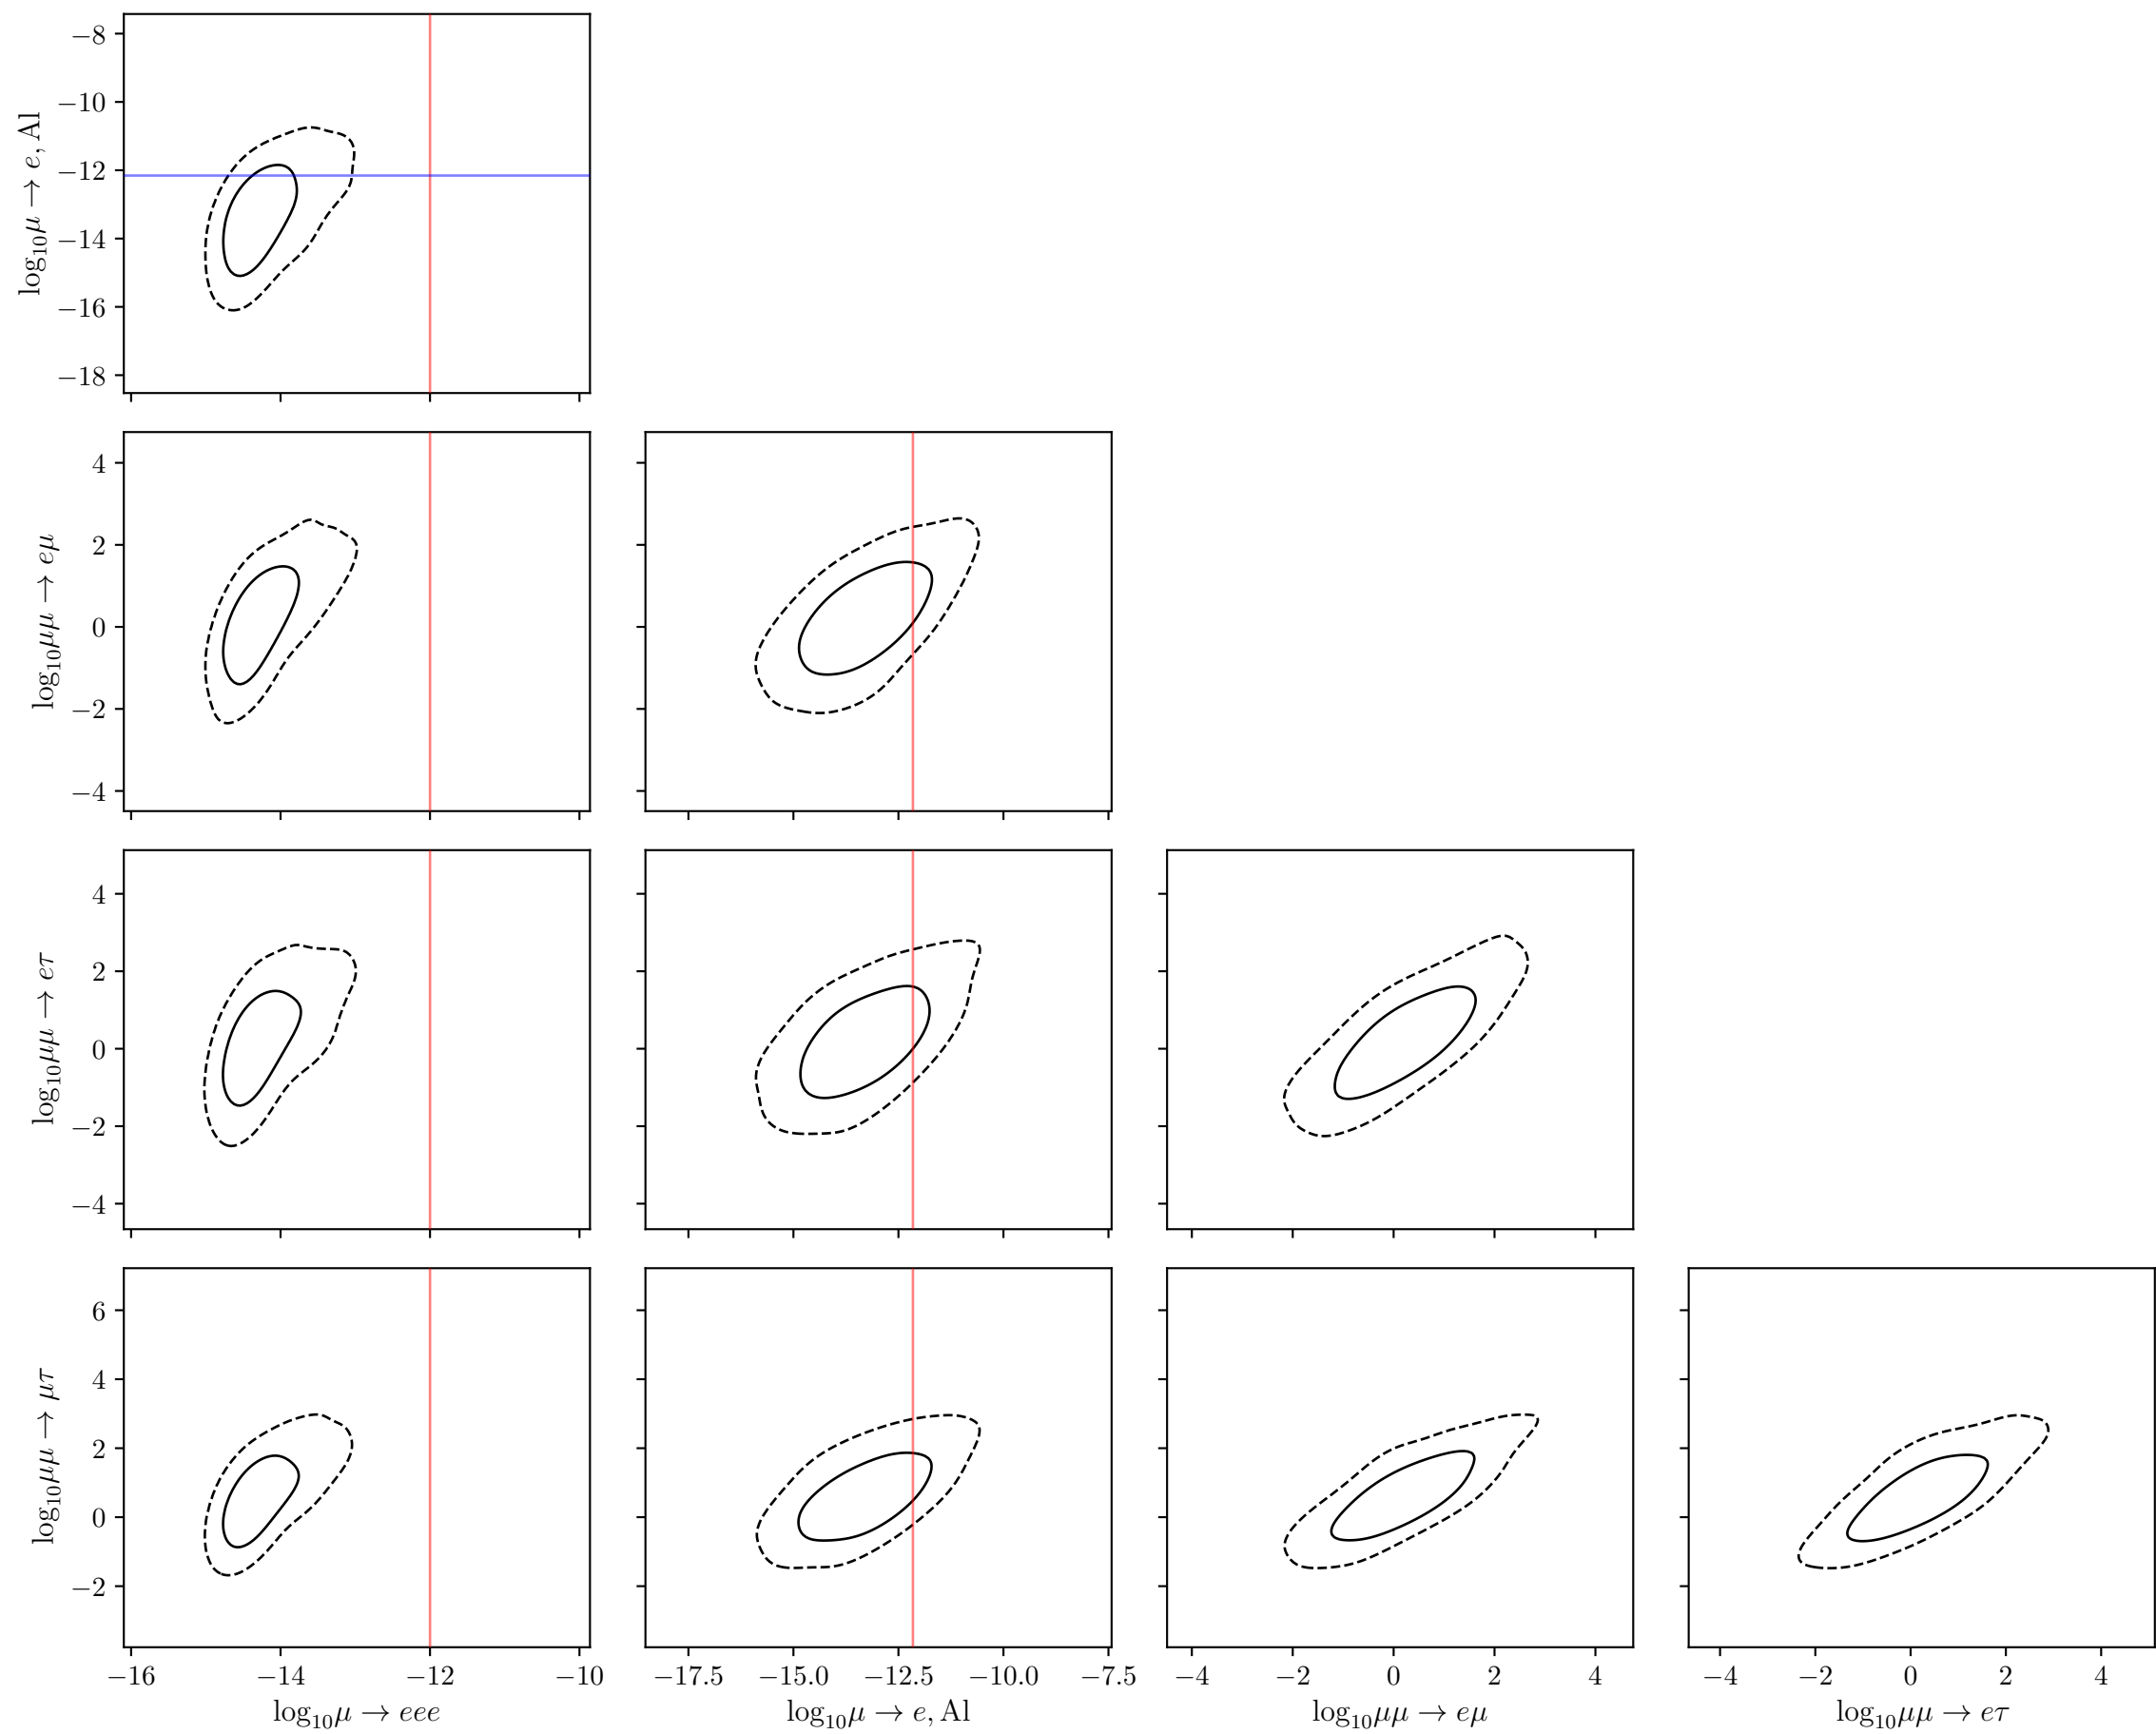

Majorana,  $X_L = \{7, 6, 5\}$ ,  $X_e = \{-1, 0, 3\}$ ,

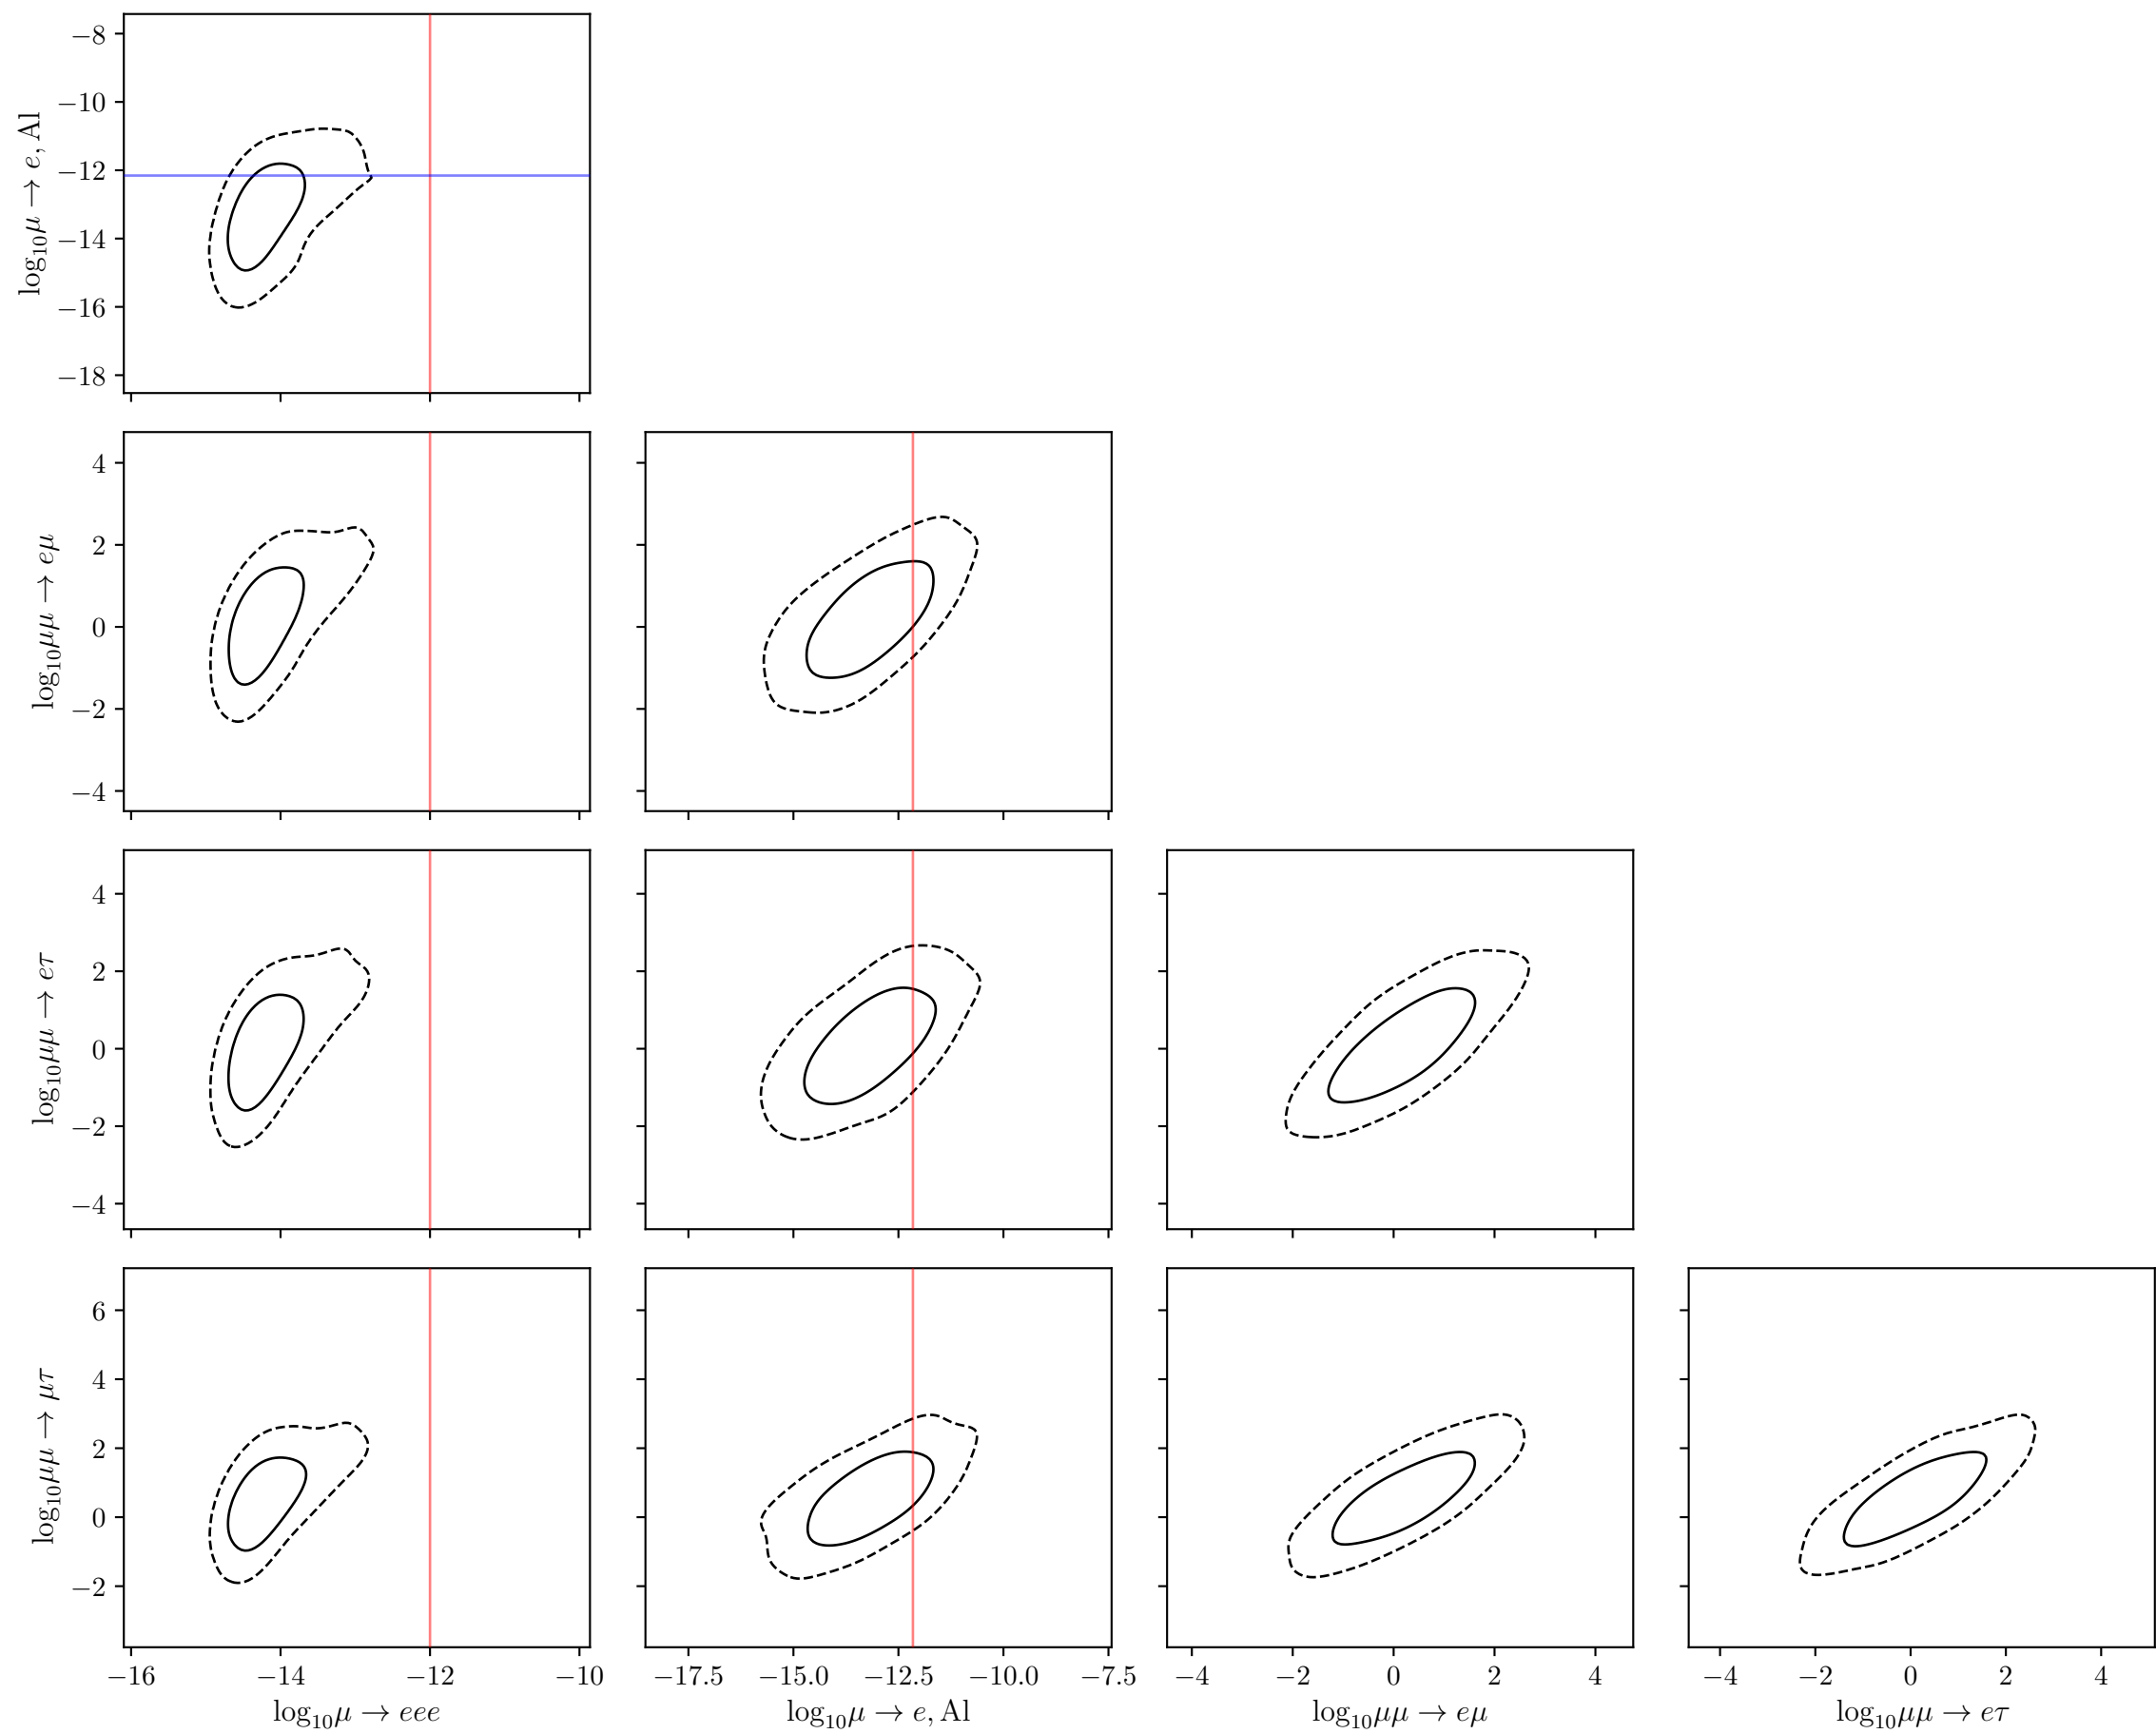

Majorana,  $X_L = \{6, 5, 4\}$ ,  $X_e = \{4, 1, 0\}$ ,

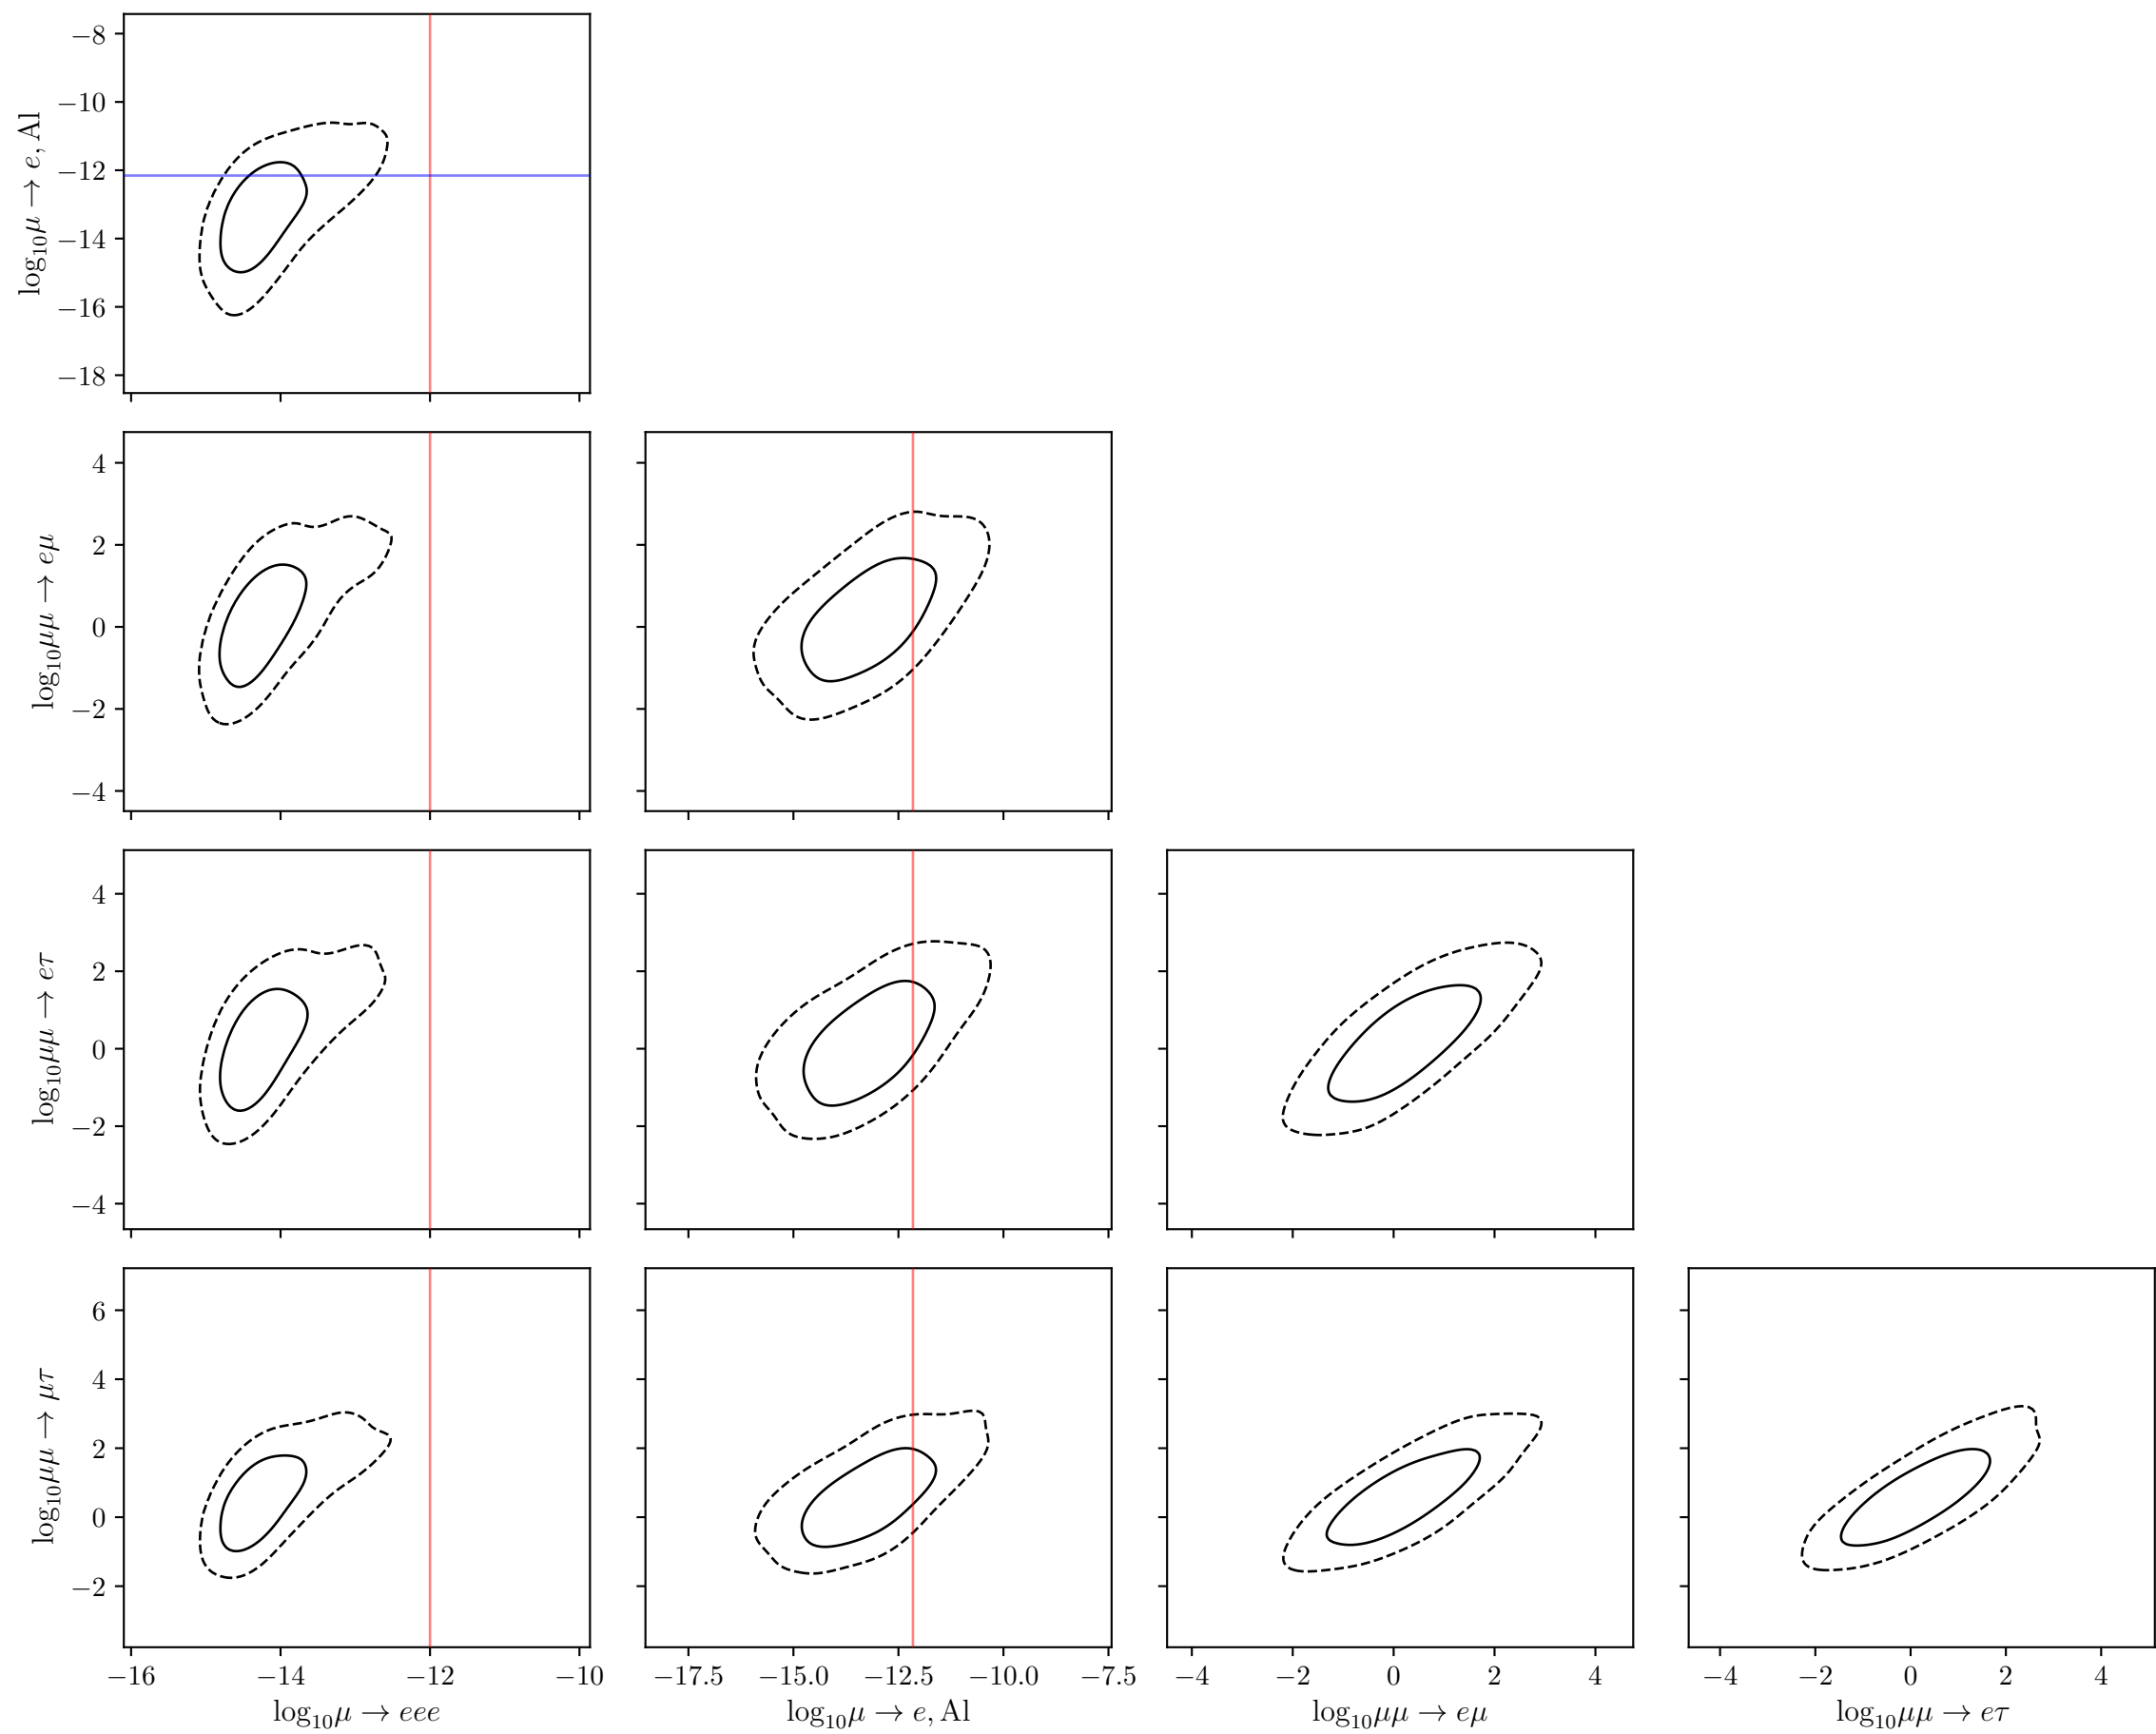

Supplement: Supplementary file 1 [file majorana_correlations_cosmo.pdf]
